# Supplementary material for: Unravelling the nonlinear ideal density response of many-body systems
Source: arXiv:2303.09223 ancillary file (2023-05-05)
Supplement: Supplementary file 1 [file supplementary_-_calculations.pdf]

# Brute force quantum kinetic theory calculations and canonical conjecture calculations of the diagonal non-interacting nonlinear density responses

Panagiotis Tolias<sup>1</sup>, Tobias Dornheim<sup>2,3</sup>, Zhandos Moldabekov<sup>2,3</sup> and Jan Vorberger<sup>3</sup>

<sup>1</sup> *Space and Plasma Physics, Royal Institute of Technology, Stockholm, SE-100 44, Sweden*

<sup>2</sup> *Center for Advanced Systems Understanding (CASUS), D-02826 Görlitz, Germany*

<sup>3</sup> *Helmholtz-Zentrum Dresden-Rossendorf (HZDR), D-01328 Dresden, Germany*

Supplementary material for the paper entitled as “Unravelling the nonlinear ideal density response of many-body systems”. It contains brute force quantum kinetic theory calculations of the diagonal non-interacting linear, quadratic, cubic, quartic and quintic density responses as well as canonical conjecture calculations of the diagonal non-interacting sextic, septic, octic, nonic and decic density responses.

## Contents

### **Part I - Brute force quantum kinetic theory calculations.**

pp.2-3: Quantum kinetic theory approach.

pp.3-6: Linear density response.

pp.7-12: Quadratic density response.

pp.13-30: Cubic density response.

pp.31-69: Quartic density response.

pp.70-149: Quintic density response.

### **Part II - Canonical conjecture calculations.**

pp.150-151: Canonical conjecture approach.

pp.152-154: Sextic density response.

pp.155-157: Septic density response.

pp.158-160: Octic density response.

pp.161-163: Nonic density response.

pp.164-168: Decic density response.

pp.169-169: Summary of high order density responses.

## I. BRUTE FORCE QUANTUM KINETIC THEORY CALCULATIONS

**General.** The starting point is the non-interacting quantum kinetic equation within the Wigner representation, which results from the  $s = 1$  member of the quantum BBGKY hierarchy in absence of particle interactions, *i.e.*,  $U(r) = 0$ . Initially, the system lies in thermodynamic equilibrium following the Fermi-Dirac distribution function  $f_0(\mathbf{p})$ . An external potential energy perturbation  $U_{\text{ext}}(\mathbf{r}, t)$  is applied that perturbs the one-particle Wigner distribution function,  $f(\mathbf{r}, \mathbf{p}, t) = f_0(\mathbf{p}) + f^{\text{ind}}(\mathbf{r}, \mathbf{p}, t)$ . Substitution of the decomposition, without neglecting the nonlinear term, leads to

$$\begin{aligned} \left\{ \frac{\partial}{\partial t} + \mathbf{v} \cdot \frac{\partial}{\partial \mathbf{r}} \right\} f(\mathbf{r}, \mathbf{p}, t) &= -\frac{1}{i\hbar} \int \frac{d^3\lambda d^3\bar{\mathbf{p}}}{(2\pi)^3} \exp[i(\mathbf{p} - \bar{\mathbf{p}}) \cdot \boldsymbol{\lambda}] \left[ U_{\text{ext}}\left(\mathbf{r} + \frac{\hbar}{2}\boldsymbol{\lambda}, t\right) - U_{\text{ext}}\left(\mathbf{r} - \frac{\hbar}{2}\boldsymbol{\lambda}, t\right) \right] f(\mathbf{r}, \bar{\mathbf{p}}, t) \Rightarrow \\ \left\{ \frac{\partial}{\partial t} + \mathbf{v} \cdot \frac{\partial}{\partial \mathbf{r}} \right\} [f_0(\mathbf{p}) + f^{\text{ind}}(\mathbf{r}, \mathbf{p}, t)] &= -\frac{1}{i\hbar} \int \frac{d^3\lambda d^3\bar{\mathbf{p}}}{(2\pi)^3} \exp[i(\mathbf{p} - \bar{\mathbf{p}}) \cdot \boldsymbol{\lambda}] \left[ U_{\text{ext}}\left(\mathbf{r} + \frac{\hbar}{2}\boldsymbol{\lambda}, t\right) - U_{\text{ext}}\left(\mathbf{r} - \frac{\hbar}{2}\boldsymbol{\lambda}, t\right) \right] [f_0(\bar{\mathbf{p}}) + f^{\text{ind}}(\mathbf{r}, \bar{\mathbf{p}}, t)] \\ \left\{ \frac{\partial}{\partial t} + \mathbf{v} \cdot \frac{\partial}{\partial \mathbf{r}} \right\} f^{\text{ind}}(\mathbf{r}, \mathbf{p}, t) &= -\frac{1}{i\hbar} \int \frac{d^3\lambda d^3\bar{\mathbf{p}}}{(2\pi)^3} \exp[i(\mathbf{p} - \bar{\mathbf{p}}) \cdot \boldsymbol{\lambda}] \left[ U_{\text{ext}}\left(\mathbf{r} + \frac{\hbar}{2}\boldsymbol{\lambda}, t\right) - U_{\text{ext}}\left(\mathbf{r} - \frac{\hbar}{2}\boldsymbol{\lambda}, t\right) \right] f_0(\bar{\mathbf{p}}) \\ &\quad - \frac{1}{i\hbar} \int \frac{d^3\lambda d^3\bar{\mathbf{p}}}{(2\pi)^3} \exp[i(\mathbf{p} - \bar{\mathbf{p}}) \cdot \boldsymbol{\lambda}] \left[ U_{\text{ext}}\left(\mathbf{r} + \frac{\hbar}{2}\boldsymbol{\lambda}, t\right) - U_{\text{ext}}\left(\mathbf{r} - \frac{\hbar}{2}\boldsymbol{\lambda}, t\right) \right] f^{\text{ind}}(\mathbf{r}, \bar{\mathbf{p}}, t). \end{aligned}$$

The nonlinear integral equation is Fourier transformed in space and time. The calculation involves the multiplication property  $F(\mathbf{r}, t)G(\mathbf{r}, t) \rightarrow [1/(2\pi)^4] \int d^3k' d\omega' F(\mathbf{k}', \omega') G(\mathbf{k} - \mathbf{k}', \omega - \omega')$  (for the nonlinear term), the shifting property  $F(\mathbf{r} + \mathbf{r}_0, t) \rightarrow e^{i\mathbf{k} \cdot \mathbf{r}_0} F(\mathbf{k}, \omega)$ , the  $\delta$ -function integral  $\delta(\mathbf{r} - \mathbf{r}_0) = [1/(2\pi)^3] \int \exp[i(\mathbf{r} - \mathbf{r}_0) \cdot \boldsymbol{\lambda}] d^3\lambda$  and the  $\delta$ -function definition  $F(\mathbf{r}_0) = \int \delta(\mathbf{r} - \mathbf{r}_0) F(\mathbf{r}) d^3r$  (for the linear term and the nonlinear term). Adding  $i0$  for causality reasons, see also the adiabatic switching of the external perturbation  $U_{\text{ext}}(\mathbf{r}, t)$ , yields the exact nonlinear integral equation

$$\begin{aligned} (-i\omega + i\mathbf{k} \cdot \mathbf{v}) f_{\mathbf{p}, \mathbf{k}, \omega}^{\text{ind}} &= -\frac{1}{i\hbar} \int \frac{d^3\lambda d^3\bar{\mathbf{p}}}{(2\pi)^3} \exp[i(\mathbf{p} - \bar{\mathbf{p}}) \cdot \boldsymbol{\lambda}] \left[ U_{\text{ext}}\left(\mathbf{r} + \frac{\hbar}{2}\boldsymbol{\lambda}, t\right) - U_{\text{ext}}\left(\mathbf{r} - \frac{\hbar}{2}\boldsymbol{\lambda}, t\right) \right]_{\mathbf{k}, \omega} f_0(\bar{\mathbf{p}}) \\ &\quad - \frac{1}{i\hbar} \int \frac{d\omega' d^3k'}{(2\pi)^4} \frac{d^3\lambda d^3\bar{\mathbf{p}}}{(2\pi)^3} \exp[i(\mathbf{p} - \bar{\mathbf{p}}) \cdot \boldsymbol{\lambda}] \left[ U_{\text{ext}}\left(\mathbf{r} + \frac{\hbar}{2}\boldsymbol{\lambda}, t\right) - U_{\text{ext}}\left(\mathbf{r} - \frac{\hbar}{2}\boldsymbol{\lambda}, t\right) \right]_{\mathbf{k}', \omega'} f_{\bar{\mathbf{p}}, \mathbf{k} - \mathbf{k}', \omega - \omega'}^{\text{ind}} \Rightarrow \\ (-i\omega + i\mathbf{k} \cdot \mathbf{v}) f_{\mathbf{p}, \mathbf{k}, \omega}^{\text{ind}} &= -\frac{1}{i\hbar} \int \frac{d^3\lambda d^3\bar{\mathbf{p}}}{(2\pi)^3} \exp[i(\mathbf{p} - \bar{\mathbf{p}}) \cdot \boldsymbol{\lambda}] \left[ \exp\left(i\frac{\hbar}{2}\mathbf{k} \cdot \boldsymbol{\lambda}\right) U_{\mathbf{k}, \omega}^{\text{ext}} - \exp\left(-i\frac{\hbar}{2}\mathbf{k} \cdot \boldsymbol{\lambda}\right) U_{\mathbf{k}, \omega}^{\text{ext}} \right] f_0(\bar{\mathbf{p}}) \\ &\quad - \frac{1}{i\hbar} \int \frac{d\omega' d^3k'}{(2\pi)^4} \frac{d^3\lambda d^3\bar{\mathbf{p}}}{(2\pi)^3} \exp[i(\mathbf{p} - \bar{\mathbf{p}}) \cdot \boldsymbol{\lambda}] \left[ \exp\left(i\frac{\hbar}{2}\mathbf{k}' \cdot \boldsymbol{\lambda}\right) U_{\mathbf{k}', \omega'}^{\text{ext}} - \exp\left(-i\frac{\hbar}{2}\mathbf{k}' \cdot \boldsymbol{\lambda}\right) U_{\mathbf{k}', \omega'}^{\text{ext}} \right] f_{\bar{\mathbf{p}}, \mathbf{k} - \mathbf{k}', \omega - \omega'}^{\text{ind}} \Rightarrow \\ (-i\omega + i\mathbf{k} \cdot \mathbf{v}) f_{\mathbf{p}, \mathbf{k}, \omega}^{\text{ind}} &= -\frac{1}{i\hbar} \int \frac{d^3\lambda d^3\bar{\mathbf{p}}}{(2\pi)^3} \exp[i(\mathbf{p} - \bar{\mathbf{p}}) \cdot \boldsymbol{\lambda}] \left[ \exp\left(i\frac{\hbar}{2}\mathbf{k} \cdot \boldsymbol{\lambda}\right) - \exp\left(-i\frac{\hbar}{2}\mathbf{k} \cdot \boldsymbol{\lambda}\right) \right] f_0(\bar{\mathbf{p}}) U_{\mathbf{k}, \omega}^{\text{ext}} \\ &\quad - \frac{1}{i\hbar} \int \frac{d\omega' d^3k'}{(2\pi)^4} \frac{d^3\lambda d^3\bar{\mathbf{p}}}{(2\pi)^3} \exp[i(\mathbf{p} - \bar{\mathbf{p}}) \cdot \boldsymbol{\lambda}] \left[ \exp\left(i\frac{\hbar}{2}\mathbf{k}' \cdot \boldsymbol{\lambda}\right) - \exp\left(-i\frac{\hbar}{2}\mathbf{k}' \cdot \boldsymbol{\lambda}\right) \right] U_{\mathbf{k}', \omega'}^{\text{ext}} f_{\bar{\mathbf{p}}, \mathbf{k} - \mathbf{k}', \omega - \omega'}^{\text{ind}} \Rightarrow \\ (-i\omega + i\mathbf{k} \cdot \mathbf{v}) f_{\mathbf{p}, \mathbf{k}, \omega}^{\text{ind}} &= -\frac{1}{i\hbar} \int \frac{d^3\lambda d^3\bar{\mathbf{p}}}{(2\pi)^3} \left\{ \exp\left[i\left(\mathbf{p} - \bar{\mathbf{p}} + \frac{\hbar}{2}\mathbf{k}\right) \cdot \boldsymbol{\lambda}\right] - \exp\left[i\left(\mathbf{p} - \bar{\mathbf{p}} - \frac{\hbar}{2}\mathbf{k}\right) \cdot \boldsymbol{\lambda}\right] \right\} f_0(\bar{\mathbf{p}}) U_{\mathbf{k}, \omega}^{\text{ext}} \\ &\quad - \frac{1}{i\hbar} \int \frac{d\omega' d^3k'}{(2\pi)^4} \frac{d^3\lambda d^3\bar{\mathbf{p}}}{(2\pi)^3} \left\{ \exp\left[i\left(\mathbf{p} - \bar{\mathbf{p}} + \frac{\hbar}{2}\mathbf{k}'\right) \cdot \boldsymbol{\lambda}\right] - \exp\left[i\left(\mathbf{p} - \bar{\mathbf{p}} - \frac{\hbar}{2}\mathbf{k}'\right) \cdot \boldsymbol{\lambda}\right] \right\} U_{\mathbf{k}', \omega'}^{\text{ext}} f_{\bar{\mathbf{p}}, \mathbf{k} - \mathbf{k}', \omega - \omega'}^{\text{ind}} \Rightarrow \\ (-i\omega + i\mathbf{k} \cdot \mathbf{v}) f_{\mathbf{p}, \mathbf{k}, \omega}^{\text{ind}} &= -\frac{1}{i\hbar} \int d^3\bar{\mathbf{p}} \left[ \delta\left(\mathbf{p} - \bar{\mathbf{p}} + \frac{\hbar}{2}\mathbf{k}\right) - \delta\left(\mathbf{p} - \bar{\mathbf{p}} - \frac{\hbar}{2}\mathbf{k}\right) \right] f_0(\bar{\mathbf{p}}) U_{\mathbf{k}, \omega}^{\text{ext}} \\ &\quad - \frac{1}{i\hbar} \int \frac{d\omega' d^3k'}{(2\pi)^4} d^3\bar{\mathbf{p}} \left[ \delta\left(\mathbf{p} - \bar{\mathbf{p}} + \frac{\hbar}{2}\mathbf{k}'\right) - \delta\left(\mathbf{p} - \bar{\mathbf{p}} - \frac{\hbar}{2}\mathbf{k}'\right) \right] U_{\mathbf{k}', \omega'}^{\text{ext}} f_{\bar{\mathbf{p}}, \mathbf{k} - \mathbf{k}', \omega - \omega'}^{\text{ind}} \Rightarrow \\ (-i\omega + i\mathbf{k} \cdot \mathbf{v}) f_{\mathbf{p}, \mathbf{k}, \omega}^{\text{ind}} &= -\frac{1}{i\hbar} \left[ f_0\left(\mathbf{p} + \frac{\hbar}{2}\mathbf{k}\right) - f_0\left(\mathbf{p} - \frac{\hbar}{2}\mathbf{k}\right) \right] U_{\mathbf{k}, \omega}^{\text{ext}} \\ &\quad - \frac{1}{i\hbar} \int \frac{d\omega' d^3k'}{(2\pi)^4} \left[ f_{\mathbf{p} + \frac{\hbar}{2}\mathbf{k}', \mathbf{k} - \mathbf{k}', \omega - \omega'}^{\text{ind}} - f_{\mathbf{p} - \frac{\hbar}{2}\mathbf{k}', \mathbf{k} - \mathbf{k}', \omega - \omega'}^{\text{ind}} \right] U_{\mathbf{k}', \omega'}^{\text{ext}} \Rightarrow \\ (\omega - \mathbf{k} \cdot \mathbf{v}) f_{\mathbf{p}, \mathbf{k}, \omega}^{\text{ind}} &= -\frac{1}{\hbar} \left[ f_0\left(\mathbf{p} + \frac{\hbar}{2}\mathbf{k}\right) - f_0\left(\mathbf{p} - \frac{\hbar}{2}\mathbf{k}\right) \right] U_{\mathbf{k}, \omega}^{\text{ext}} - \frac{1}{\hbar} \int \frac{d\omega' d^3k'}{(2\pi)^4} \left[ f_{\mathbf{p} + \frac{\hbar}{2}\mathbf{k}', \mathbf{k} - \mathbf{k}', \omega - \omega'}^{\text{ind}} - f_{\mathbf{p} - \frac{\hbar}{2}\mathbf{k}', \mathbf{k} - \mathbf{k}', \omega - \omega'}^{\text{ind}} \right] U_{\mathbf{k}', \omega'}^{\text{ext}} \Rightarrow \\ f_{\mathbf{p}, \mathbf{k}, \omega}^{\text{ind}} &= -\frac{1}{\hbar} \left[ \frac{f_0\left(\mathbf{p} + \frac{\hbar}{2}\mathbf{k}\right) - f_0\left(\mathbf{p} - \frac{\hbar}{2}\mathbf{k}\right)}{\omega - \mathbf{k} \cdot \mathbf{v} + i0} \right] U_{\mathbf{k}, \omega}^{\text{ext}} - \frac{1}{\hbar} \int \frac{d\omega' d^3k'}{(2\pi)^4} \left[ \frac{f_{\mathbf{p} + \frac{\hbar}{2}\mathbf{k}', \mathbf{k} - \mathbf{k}', \omega - \omega'}^{\text{ind}} - f_{\mathbf{p} - \frac{\hbar}{2}\mathbf{k}', \mathbf{k} - \mathbf{k}', \omega - \omega'}^{\text{ind}}}{\omega - \mathbf{k} \cdot \mathbf{v} + i0} \right] U_{\mathbf{k}', \omega'}^{\text{ext}}. \end{aligned}$$

In view of the wave-particle duality, it is more convenient to employ wavenumbers instead of momenta. Introducing  $\mathbf{p} = \hbar\mathbf{q}$ ,  $\mathbf{v} = (\hbar/m)\mathbf{q}$  and dropping  $\hbar$  from the one-particle distribution function arguments (equilibrium and perturbed) as well as utilizing the identity  $\epsilon_{\mathbf{q}+(1/2)\mathbf{k}} - \epsilon_{\mathbf{q}-(1/2)\mathbf{k}} = [\hbar^2/(2m)](2\mathbf{k} \cdot \mathbf{q})$  where  $\epsilon_q = [\hbar^2/(2m)]q^2$  for the non-interacting Fermi gas, one acquires the equivalent equation

$$\begin{aligned} f_{\mathbf{p},\mathbf{k},\omega}^{\text{ind}} &= -\frac{1}{\hbar} \left[ \frac{f_0(\mathbf{p} + \frac{\hbar}{2}\mathbf{k}) - f_0(\mathbf{p} - \frac{\hbar}{2}\mathbf{k})}{\omega - \mathbf{k} \cdot \mathbf{v} + i0} \right] U_{\mathbf{k},\omega}^{\text{ext}} - \frac{1}{\hbar} \int \frac{d\omega' d^3k'}{(2\pi)^4} \left[ \frac{f_{\mathbf{p}+\frac{\hbar}{2}\mathbf{k}',\mathbf{k}-\mathbf{k}',\omega-\omega'}^{\text{ind}} - f_{\mathbf{p}-\frac{\hbar}{2}\mathbf{k}',\mathbf{k}-\mathbf{k}',\omega-\omega'}^{\text{ind}}}{\omega - \mathbf{k} \cdot \mathbf{v} + i0} \right] U_{\mathbf{k}',\omega'}^{\text{ext}} \Rightarrow \\ f_{\hbar\mathbf{q},\mathbf{k},\omega}^{\text{ind}} &= -\frac{1}{\hbar} \left[ \frac{f_0(\hbar\mathbf{q} + \frac{\hbar}{2}\mathbf{k}) - f_0(\hbar\mathbf{q} - \frac{\hbar}{2}\mathbf{k})}{\omega - \frac{\hbar}{m}\mathbf{k} \cdot \mathbf{q} + i0} \right] U_{\mathbf{k},\omega}^{\text{ext}} - \frac{1}{\hbar} \int \frac{d\omega' d^3k'}{(2\pi)^4} \left[ \frac{f_{\hbar\mathbf{q}+\frac{\hbar}{2}\mathbf{k}',\mathbf{k}-\mathbf{k}',\omega-\omega'}^{\text{ind}} - f_{\hbar\mathbf{q}-\frac{\hbar}{2}\mathbf{k}',\mathbf{k}-\mathbf{k}',\omega-\omega'}^{\text{ind}}}{\omega - \frac{\hbar}{m}\mathbf{k} \cdot \mathbf{q} + i0} \right] U_{\mathbf{k}',\omega'}^{\text{ext}} \Rightarrow \\ f_{\hbar\mathbf{q},\mathbf{k},\omega}^{\text{ind}} &= -\left[ \frac{f_0(\hbar\mathbf{q} + \frac{\hbar}{2}\mathbf{k}) - f_0(\hbar\mathbf{q} - \frac{\hbar}{2}\mathbf{k})}{\hbar\omega - \frac{\hbar^2}{m}\mathbf{k} \cdot \mathbf{q} + i0} \right] U_{\mathbf{k},\omega}^{\text{ext}} - \int \frac{d\omega' d^3k'}{(2\pi)^4} \left[ \frac{f_{\hbar\mathbf{q}+\frac{\hbar}{2}\mathbf{k}',\mathbf{k}-\mathbf{k}',\omega-\omega'}^{\text{ind}} - f_{\hbar\mathbf{q}-\frac{\hbar}{2}\mathbf{k}',\mathbf{k}-\mathbf{k}',\omega-\omega'}^{\text{ind}}}{\hbar\omega - \frac{\hbar^2}{m}\mathbf{k} \cdot \mathbf{q} + i0} \right] U_{\mathbf{k}',\omega'}^{\text{ext}} \Rightarrow \\ f_{\mathbf{q},\mathbf{k},\omega}^{\text{ind}} &= -\left[ \frac{f_0(\mathbf{q} + \frac{1}{2}\mathbf{k}) - f_0(\mathbf{q} - \frac{1}{2}\mathbf{k})}{\hbar\omega - \frac{\hbar^2}{2m}(2\mathbf{k} \cdot \mathbf{q}) + i0} \right] U_{\mathbf{k},\omega}^{\text{ext}} - \int \frac{d\omega' d^3k'}{(2\pi)^4} \left[ \frac{f_{\mathbf{q}+\frac{1}{2}\mathbf{k}',\mathbf{k}-\mathbf{k}',\omega-\omega'}^{\text{ind}} - f_{\mathbf{q}-\frac{1}{2}\mathbf{k}',\mathbf{k}-\mathbf{k}',\omega-\omega'}^{\text{ind}}}{\hbar\omega - \frac{\hbar^2}{2m}(2\mathbf{k} \cdot \mathbf{q}) + i0} \right] U_{\mathbf{k}',\omega'}^{\text{ext}} \Rightarrow \\ f_{\mathbf{q},\mathbf{k},\omega}^{\text{ind}} &= -\left[ \frac{f_0(\mathbf{q} + \frac{1}{2}\mathbf{k}) - f_0(\mathbf{q} - \frac{1}{2}\mathbf{k})}{\hbar\omega - \epsilon_{\mathbf{q}+\frac{1}{2}\mathbf{k}} + \epsilon_{\mathbf{q}-\frac{1}{2}\mathbf{k}} + i0} \right] U_{\mathbf{k},\omega}^{\text{ext}} - \int \frac{d\omega' d^3k'}{(2\pi)^4} \left[ \frac{f_{\mathbf{q}+\frac{1}{2}\mathbf{k}',\mathbf{k}-\mathbf{k}',\omega-\omega'}^{\text{ind}} - f_{\mathbf{q}-\frac{1}{2}\mathbf{k}',\mathbf{k}-\mathbf{k}',\omega-\omega'}^{\text{ind}}}{\hbar\omega - \epsilon_{\mathbf{q}+\frac{1}{2}\mathbf{k}} + \epsilon_{\mathbf{q}-\frac{1}{2}\mathbf{k}} + i0} \right] U_{\mathbf{k}',\omega'}^{\text{ext}}. \end{aligned}$$

The above exact nonlinear integral equation can be solved with the standard method of successive iterations to yield all the high-order non-interacting one-particle Wigner distribution function perturbations in a successive manner. A formal expansion of the type  $f_{\mathbf{q},\mathbf{k},\omega}^{\text{ind}} = \sum_{n=1}^{\infty} f_{\mathbf{q},\mathbf{k},\omega}^{\text{ind},(n)}$ , leads to a general recurrence relation

$$\begin{aligned} f_{\mathbf{q},\mathbf{k},\omega}^{\text{ind},(1)} &= -\left[ \frac{f_0(\mathbf{q} + \frac{1}{2}\mathbf{k}) - f_0(\mathbf{q} - \frac{1}{2}\mathbf{k})}{\hbar\omega - \epsilon_{\mathbf{q}+\frac{1}{2}\mathbf{k}} + \epsilon_{\mathbf{q}-\frac{1}{2}\mathbf{k}} + i0} \right] U_{\mathbf{k},\omega}^{\text{ext}}. \\ f_{\mathbf{q},\mathbf{k},\omega}^{\text{ind},(n)} &= -\int \frac{d\omega' d^3k'}{(2\pi)^4} \left[ \frac{f_{\mathbf{q}+\frac{1}{2}\mathbf{k}',\mathbf{k}-\mathbf{k}',\omega-\omega'}^{\text{ind},(n-1)} - f_{\mathbf{q}-\frac{1}{2}\mathbf{k}',\mathbf{k}-\mathbf{k}',\omega-\omega'}^{\text{ind},(n-1)}}{\hbar\omega - \epsilon_{\mathbf{q}+\frac{1}{2}\mathbf{k}} + \epsilon_{\mathbf{q}-\frac{1}{2}\mathbf{k}} + i0} \right] U_{\mathbf{k}',\omega'}^{\text{ext}}, \quad n \geq 2. \end{aligned}$$

### A. The first-order (linear) ideal density response

The starting point is the first expression of the general recurrence relation, which is the result of linear response theory. Assuming the paramagnetic case for the dropped spin variables, the integration of the first order one-particle distribution function perturbation over the momentum space is connected to the first order density perturbation,  $n_{\text{ind}}^{(1)}(\mathbf{k}, \omega) = 2 \int [d^3q/(2\pi)^3] f_{\mathbf{q},\mathbf{k},\omega}^{\text{ind},(1)}$ . The definition of the first order ideal density response  $\chi_0(\mathbf{k}, \omega) = n_{\text{ind}}^{(1)}(\mathbf{k}, \omega)/U_{\mathbf{k},\omega}^{\text{ext}}$  can now be employed. Note that  $\mathcal{W}_{\mathbf{k},\omega}^{(1),0} = \chi_0^{(1,1)}(\mathbf{k}, \omega) = \chi_0(\mathbf{k}, \omega)$ . After the change of variables  $\mathbf{q} - (1/2)\mathbf{k} \rightarrow \mathbf{q}$ , the standard form of the ideal Lindhard density response emerges

$$\begin{aligned} f_{\mathbf{q},\mathbf{k},\omega}^{\text{ind},(1)} &= -\left[ \frac{f_0(\mathbf{q} + \frac{1}{2}\mathbf{k}) - f_0(\mathbf{q} - \frac{1}{2}\mathbf{k})}{\hbar\omega - \epsilon_{\mathbf{q}+\frac{1}{2}\mathbf{k}} + \epsilon_{\mathbf{q}-\frac{1}{2}\mathbf{k}} + i0} \right] U_{\mathbf{k},\omega}^{\text{ext}} \Rightarrow \\ n_{\text{ind}}^{(1)}(\mathbf{k}, \omega) &= -2 \int \frac{d^3q}{(2\pi)^3} \frac{f_0(\mathbf{q} + \frac{1}{2}\mathbf{k}) - f_0(\mathbf{q} - \frac{1}{2}\mathbf{k})}{\hbar\omega - \epsilon_{\mathbf{q}+\frac{1}{2}\mathbf{k}} + \epsilon_{\mathbf{q}-\frac{1}{2}\mathbf{k}} + i0} U_{\mathbf{k},\omega}^{\text{ext}} \Rightarrow \\ \frac{n_{\text{ind}}^{(1)}(\mathbf{k}, \omega)}{U_{\mathbf{k},\omega}^{\text{ext}}} &= -2 \int \frac{d^3q}{(2\pi)^3} \frac{f_0(\mathbf{q} + \frac{1}{2}\mathbf{k}) - f_0(\mathbf{q} - \frac{1}{2}\mathbf{k})}{\hbar\omega - \epsilon_{\mathbf{q}+\frac{1}{2}\mathbf{k}} + \epsilon_{\mathbf{q}-\frac{1}{2}\mathbf{k}} + i0} \Rightarrow \\ \chi_0(\mathbf{k}, \omega) &= -2 \int \frac{d^3q}{(2\pi)^3} \frac{f_0(\mathbf{q} + \frac{1}{2}\mathbf{k}) - f_0(\mathbf{q} - \frac{1}{2}\mathbf{k})}{\hbar\omega - \epsilon_{\mathbf{q}+\frac{1}{2}\mathbf{k}} + \epsilon_{\mathbf{q}-\frac{1}{2}\mathbf{k}} + i0} \Rightarrow \\ \chi_0(\mathbf{k}, \omega) &= -2 \int \frac{d^3q}{(2\pi)^3} \frac{f_0(\mathbf{q} - \frac{1}{2}\mathbf{k} + \mathbf{k}) - f_0(\mathbf{q} - \frac{1}{2}\mathbf{k})}{\hbar\omega - \epsilon_{\mathbf{q}-\frac{1}{2}\mathbf{k}+\mathbf{k}} + \epsilon_{\mathbf{q}-\frac{1}{2}\mathbf{k}} + i0} \Rightarrow \\ \chi_0(\mathbf{k}, \omega) &= -2 \int \frac{d^3q}{(2\pi)^3} \frac{f_0(\mathbf{q} + \mathbf{k}) - f_0(\mathbf{q})}{\hbar\omega - \epsilon_{\mathbf{q}+\mathbf{k}} + \epsilon_{\mathbf{q}} + i0}. \end{aligned}$$

Another standard form of the ideal Lindhard density response, which straightforwardly leads to numerically friendly simple integral representations for isotropic equilibrium distribution functions, can be obtained by decomposing the single integral into two integrals, proceeding with the variable change  $\mathbf{q} + \mathbf{k} \rightarrow \mathbf{q}$  in the first integral and then unifying:

$$\begin{aligned}\chi_0(\mathbf{k}, \omega) &= -2 \int \frac{d^3q}{(2\pi)^3} \frac{f_0(\mathbf{q} + \mathbf{k}) - f_0(\mathbf{q})}{\hbar\omega - \epsilon_{\mathbf{q}+\mathbf{k}} + \epsilon_{\mathbf{q}} + i0} \Rightarrow \\ \chi_0(\mathbf{k}, \omega) &= -2 \int \frac{d^3q}{(2\pi)^3} \frac{f_0(\mathbf{q} + \mathbf{k})}{\hbar\omega - \epsilon_{\mathbf{q}+\mathbf{k}} + \epsilon_{\mathbf{q}} + i0} + 2 \int \frac{d^3q}{(2\pi)^3} \frac{f_0(\mathbf{q})}{\hbar\omega - \epsilon_{\mathbf{q}+\mathbf{k}} + \epsilon_{\mathbf{q}} + i0} \Rightarrow \\ \chi_0(\mathbf{k}, \omega) &= -2 \int \frac{d^3q}{(2\pi)^3} \frac{f_0(\mathbf{q})}{\hbar\omega - \epsilon_{\mathbf{q}} + \epsilon_{\mathbf{q}-\mathbf{k}} + i0} + 2 \int \frac{d^3q}{(2\pi)^3} \frac{f_0(\mathbf{q})}{\hbar\omega - \epsilon_{\mathbf{q}+\mathbf{k}} + \epsilon_{\mathbf{q}} + i0} \Rightarrow \\ \chi_0(\mathbf{k}, \omega) &= -2 \int \frac{d^3q}{(2\pi)^3} f_0(\mathbf{q}) \left[ \frac{1}{\hbar\omega - \epsilon_{\mathbf{q}} + \epsilon_{\mathbf{q}-\mathbf{k}} + i0} - \frac{1}{\hbar\omega - \epsilon_{\mathbf{q}+\mathbf{k}} + \epsilon_{\mathbf{q}} + i0} \right].\end{aligned}$$

Defining the analytic continuation of the linear ideal density response by setting  $z = \omega + i0$ , we have

$$\chi_0(\mathbf{k}, z) = -2 \int \frac{d^3q}{(2\pi)^3} f_0(\mathbf{q}) \left[ \frac{1}{\hbar z - \epsilon_{\mathbf{q}} + \epsilon_{\mathbf{q}-\mathbf{k}}} - \frac{1}{\hbar z - \epsilon_{\mathbf{q}+\mathbf{k}} + \epsilon_{\mathbf{q}}} \right].$$

We proceed with some algebraic manipulations in the denominators based on  $\epsilon_{\mathbf{q}} = \hbar^2 q^2 / (2m)$ . We assume that  $\mathbf{k} \parallel \hat{\mathbf{z}}$  without loss of generality and employ spherical coordinates. These lead to  $d^3q = q^2 \sin\theta dq d\theta d\phi$  and  $\mathbf{q} \cdot \mathbf{k} = qk \cos\theta$ . The azimuthal integration is trivial and the inclination angle integration is carried out with the variable change  $x = \cos\theta$  and the integral  $\int (x+a)^{-1} = \ln|x+a|$ . A compact form is obtained with the use of elementary logarithmic properties and some straightforward algebra in the logarithmic argument.

$$\begin{aligned}\chi_0(\mathbf{k}, z) &= -2 \int \frac{d^3q}{(2\pi)^3} f_0(\mathbf{q}) \left[ \frac{1}{\hbar z - \frac{\hbar^2}{2m} q^2 + \frac{\hbar^2}{2m} (\mathbf{q} - \mathbf{k})^2} - \frac{1}{\hbar z - \frac{\hbar^2}{2m} (\mathbf{q} + \mathbf{k})^2 + \frac{\hbar^2}{2m} q^2} \right] \Rightarrow \\ \chi_0(\mathbf{k}, z) &= -2 \int \frac{d^3q}{(2\pi)^3} f_0(\mathbf{q}) \left[ \frac{1}{\hbar z + \frac{\hbar^2}{2m} k^2 - \frac{\hbar^2}{m} \mathbf{q} \cdot \mathbf{k}} - \frac{1}{\hbar z - \frac{\hbar^2}{2m} k^2 - \frac{\hbar^2}{m} \mathbf{q} \cdot \mathbf{k}} \right] \Rightarrow \\ \chi_0(\mathbf{k}, z) &= -2 \frac{1}{(2\pi)^3} \int_0^{2\pi} \int_0^\pi \int_0^\infty q^2 f_0(q) \left[ \frac{1}{\hbar z + \frac{\hbar^2}{2m} k^2 - \frac{\hbar^2}{m} qk \cos\theta} - \frac{1}{\hbar z - \frac{\hbar^2}{2m} k^2 - \frac{\hbar^2}{m} qk \cos\theta} \right] \sin\theta dq d\theta d\phi \Rightarrow \\ \chi_0(\mathbf{k}, z) &= -2 \frac{2\pi}{(2\pi)^3} \int_0^\pi \int_0^\infty q^2 f_0(q) \left[ \frac{1}{\hbar z + \frac{\hbar^2}{2m} k^2 - \frac{\hbar^2}{m} qk \cos\theta} - \frac{1}{\hbar z - \frac{\hbar^2}{2m} k^2 - \frac{\hbar^2}{m} qk \cos\theta} \right] \sin\theta dq d\theta \Rightarrow \\ \chi_0(\mathbf{k}, z) &= -2 \frac{2\pi}{(2\pi)^3} \int_0^\infty \left\{ \int_{-1}^{+1} \left[ \frac{1}{\hbar z + \frac{\hbar^2}{2m} k^2 - \frac{\hbar^2}{m} qkx} - \frac{1}{\hbar z - \frac{\hbar^2}{2m} k^2 - \frac{\hbar^2}{m} qkx} \right] dx \right\} q^2 f_0(q) dq \Rightarrow \\ \chi_0(\mathbf{k}, z) &= +2 \frac{1}{(2\pi)^2} \int_0^\infty \left\{ \int_{-1}^{+1} \left[ \frac{1}{\frac{\hbar^2}{m} qkx - \hbar z - \frac{\hbar^2}{2m} k^2} - \frac{1}{\frac{\hbar^2}{m} qkx - \hbar z + \frac{\hbar^2}{2m} k^2} \right] dx \right\} q^2 f_0(q) dq \Rightarrow \\ \chi_0(\mathbf{k}, z) &= +2 \frac{1}{(2\pi)^2} \int_0^\infty \left\{ \int_{-1}^{+1} \left[ \frac{1}{x - \frac{m}{\hbar^2 qk} \hbar z - \frac{m}{\hbar^2 qk} \frac{\hbar^2}{2m} k^2} - \frac{1}{x - \frac{m}{\hbar^2 qk} \hbar z + \frac{m}{\hbar^2 qk} \frac{\hbar^2}{2m} k^2} \right] dx \right\} \frac{m}{\hbar^2 qk} q^2 f_0(q) dq \Rightarrow \\ \chi_0(\mathbf{k}, z) &= +2 \frac{1}{(2\pi)^2} \frac{m}{\hbar^2} \frac{1}{k} \int_0^\infty \left\{ \int_{-1}^{+1} \left[ \frac{1}{x - \frac{m}{\hbar^2} \frac{\hbar z}{qk} - \frac{k^2}{2qk}} - \frac{1}{x - \frac{m}{\hbar^2} \frac{\hbar z}{qk} + \frac{k^2}{2qk}} \right] dx \right\} q f_0(q) dq \Rightarrow \\ \chi_0(\mathbf{k}, z) &= +2 \frac{1}{(2\pi)^2} \frac{m}{\hbar^2} \frac{1}{k} \int_0^\infty \left\{ \ln \left| \frac{1 - \frac{m}{\hbar^2} \frac{\hbar z}{qk} - \frac{k^2}{2qk}}{1 - \frac{m}{\hbar^2} \frac{\hbar z}{qk} + \frac{k^2}{2qk}} \right| + \ln \left| \frac{-1 - \frac{m}{\hbar^2} \frac{\hbar z}{qk} + \frac{k^2}{2qk}}{-1 - \frac{m}{\hbar^2} \frac{\hbar z}{qk} - \frac{k^2}{2qk}} \right| \right\} q f_0(q) dq \Rightarrow \\ \chi_0(\mathbf{k}, z) &= +2 \frac{1}{(2\pi)^2} \frac{m}{\hbar^2} \frac{1}{k} \int_0^\infty \ln \left| \frac{\left(1 - \frac{m}{\hbar^2} \frac{\hbar z}{qk} - \frac{k^2}{2qk}\right) \left(1 + \frac{m}{\hbar^2} \frac{\hbar z}{qk} - \frac{k^2}{2qk}\right)}{\left(1 - \frac{m}{\hbar^2} \frac{\hbar z}{qk} + \frac{k^2}{2qk}\right) \left(1 + \frac{m}{\hbar^2} \frac{\hbar z}{qk} + \frac{k^2}{2qk}\right)} \right| q f_0(q) dq \Rightarrow \\ \chi_0(\mathbf{k}, z) &= +2 \frac{1}{(2\pi)^2} \frac{m}{\hbar^2} \frac{1}{k} \int_0^\infty \ln \left| \frac{\left(1 - \frac{k^2}{2qk}\right)^2 - \frac{m^2}{\hbar^4} \frac{\hbar^2 z^2}{q^2 k^2}}{\left(1 + \frac{k^2}{2qk}\right)^2 - \frac{m^2}{\hbar^4} \frac{\hbar^2 z^2}{q^2 k^2}} \right| q f_0(q) dq.\end{aligned}$$

From the definition of the first order ideal density response as the first order functional derivative of the density with respect to the external potential energy, it is evident that the proper normalization of the Lindhard response is achieved by dividing with  $1/(n\beta)$ . The calculation proceeds with the introduction of the dimensionless complex frequency  $z = (T/\hbar)Z$  as well as of the dimensionless wavenumber  $k = k_F x$ ,  $q = k_F y$ . The utilization of the Fermi energy definition  $E_F = \hbar^2 k_F^2/(2m)$  and the introduction of the degeneracy temperature definition  $\Theta = T/E_F$  ultimately lead to

$$\begin{aligned}
\frac{\chi_0(\mathbf{k}, z)}{n\beta} &= +2 \frac{1}{(2\pi)^2} \frac{1}{n\beta} \frac{m}{\hbar^2} \frac{1}{k} \int_0^\infty \ln \left| \frac{\left(1 - \frac{k^2}{2qk}\right)^2 - \frac{m^2}{\hbar^4} \frac{\hbar^2 z^2}{q^2 k^2}}{\left(1 + \frac{k^2}{2qk}\right)^2 - \frac{m^2}{\hbar^4} \frac{\hbar^2 z^2}{q^2 k^2}} \right| q f_0(q) dq \Rightarrow \\
\frac{\chi_0(\mathbf{x}, Z)}{n\beta} &= +2 \frac{1}{(2\pi)^2} \frac{1}{n\beta} \frac{m}{\hbar^2} \frac{k_F^2}{k_F x} \int_0^\infty \ln \left| \frac{\left(1 - \frac{x^2}{2xy}\right)^2 - \frac{m^2}{\hbar^4} \frac{T^2 Z^2}{k_F^4 x^2 y^2}}{\left(1 + \frac{x^2}{2xy}\right)^2 - \frac{m^2}{\hbar^4} \frac{T^2 Z^2}{k_F^4 x^2 y^2}} \right| y f_0(y) dy \Rightarrow \\
\frac{\chi_0(\mathbf{x}, Z)}{n\beta} &= +2 \frac{1}{(2\pi)^2} \frac{1}{n\beta} \frac{m}{\hbar^2} \frac{k_F^2}{k_F x} \int_0^\infty \ln \left| \frac{\left(1 - \frac{x}{2y}\right)^2 - \frac{4m^2}{\hbar^4 k_F^4} \frac{T^2 Z^2}{4x^2 y^2}}{\left(1 + \frac{x}{2y}\right)^2 - \frac{4m^2}{\hbar^4 k_F^4} \frac{T^2 Z^2}{4x^2 y^2}} \right| y f_0(y) dy \Rightarrow \\
\frac{\chi_0(\mathbf{x}, Z)}{n\beta} &= +2 \frac{1}{(2\pi)^2} \frac{1}{n\beta} \frac{m}{\hbar^2} \frac{k_F^2}{k_F x} \int_0^\infty \ln \left| \frac{\left(1 - \frac{x}{2y}\right)^2 - \left[\frac{T}{\hbar^2 k_F^2/(2m)}\right]^2 \frac{Z^2}{4x^2 y^2}}{\left(1 + \frac{x}{2y}\right)^2 - \left[\frac{T}{\hbar^2 k_F^2/(2m)}\right]^2 \frac{Z^2}{4x^2 y^2}} \right| y f_0(y) dy \Rightarrow \\
\frac{\chi_0(\mathbf{x}, Z)}{n\beta} &= +2 \frac{1}{(2\pi)^2} \frac{1}{n\beta} \frac{m}{\hbar^2} \frac{k_F^2}{k_F x} \int_0^\infty \ln \left| \frac{\left(1 - \frac{x}{2y}\right)^2 - \left[\frac{T}{E_F}\right]^2 \frac{Z^2}{4x^2 y^2}}{\left(1 + \frac{x}{2y}\right)^2 - \left[\frac{T}{E_F}\right]^2 \frac{Z^2}{4x^2 y^2}} \right| y f_0(y) dy \Rightarrow \\
\frac{\chi_0(\mathbf{x}, Z)}{n\beta} &= +2 \frac{1}{(2\pi)^2} \frac{1}{n\beta} \frac{m}{\hbar^2} \frac{k_F^2}{k_F x} \int_0^\infty \ln \left| \frac{\left(1 - \frac{x}{2y}\right)^2 - \Theta^2 \frac{Z^2}{4x^2 y^2}}{\left(1 + \frac{x}{2y}\right)^2 - \Theta^2 \frac{Z^2}{4x^2 y^2}} \right| y f_0(y) dy \Rightarrow \\
\frac{\chi_0(\mathbf{x}, Z)}{n\beta} &= +2 \frac{1}{(2\pi)^2} \frac{1}{n\beta} \frac{m}{\hbar^2} \frac{k_F^2}{k_F x} \int_0^\infty y f_0(y; \Theta) \ln \left| \frac{(2xy - x^2)^2 - \Theta^2 Z^2}{(2xy + x^2)^2 - \Theta^2 Z^2} \right| dy \Rightarrow \\
\frac{\chi_0(\mathbf{x}, Z)}{n\beta} &= + \frac{1}{(2\pi)^2} \frac{1}{n\beta} \frac{2m}{\hbar^2 k_F^2} \frac{k_F^3}{x} \int_0^\infty y f_0(y; \Theta) \ln \left| \frac{(2xy - x^2)^2 - \Theta^2 Z^2}{(2xy + x^2)^2 - \Theta^2 Z^2} \right| dy \Rightarrow \\
\frac{\chi_0(\mathbf{x}, Z)}{n\beta} &= + \frac{1}{(2\pi)^2} \frac{1}{n\beta} \frac{1}{\hbar^2 k_F^2/(2m)} \frac{k_F^3}{x} \int_0^\infty y f_0(y; \Theta) \ln \left| \frac{(2xy - x^2)^2 - \Theta^2 Z^2}{(2xy + x^2)^2 - \Theta^2 Z^2} \right| dy \Rightarrow \\
\frac{\chi_0(\mathbf{x}, Z)}{n\beta} &= + \frac{1}{(2\pi)^2} \frac{k_F^3}{n} \frac{1}{x} \frac{T}{E_F} \int_0^\infty y f_0(y; \Theta) \ln \left| \frac{(2xy - x^2)^2 - \Theta^2 Z^2}{(2xy + x^2)^2 - \Theta^2 Z^2} \right| dy \Rightarrow \\
\frac{\chi_0(\mathbf{x}, Z)}{n\beta} &= + \frac{1}{(2\pi)^2} \frac{k_F^3}{n} \frac{\Theta}{x} \int_0^\infty y f_0(y; \Theta) \ln \left| \frac{(2xy - x^2)^2 - \Theta^2 Z^2}{(2xy + x^2)^2 - \Theta^2 Z^2} \right| dy \Rightarrow \\
\frac{\chi_0(\mathbf{x}, Z)}{n\beta} &= + \frac{1}{(2\pi)^2} \frac{3\pi^2 n}{n} \frac{\Theta}{x} \int_0^\infty y f_0(y; \Theta) \ln \left| \frac{(2xy - x^2)^2 - \Theta^2 Z^2}{(2xy + x^2)^2 - \Theta^2 Z^2} \right| dy \Rightarrow \\
\frac{\chi_0(\mathbf{x}, Z)}{n\beta} &= + \frac{3\pi^2}{4\pi^2} \frac{\Theta}{x} \int_0^\infty y f_0(y; \Theta) \ln \left| \frac{(2xy - x^2)^2 - \Theta^2 Z^2}{(2xy + x^2)^2 - \Theta^2 Z^2} \right| dy \Rightarrow \\
\frac{\chi_0(\mathbf{x}, Z)}{n\beta} &= + \frac{3}{4} \frac{\Theta}{x} \int_0^\infty y f_0(y; \Theta) \ln \left| \frac{(2xy - x^2)^2 - \Theta^2 Z^2}{(2xy + x^2)^2 - \Theta^2 Z^2} \right| dy.
\end{aligned}$$

The static limit simply reads as

$$\begin{aligned}\frac{\chi_0(\mathbf{x})}{n\beta} &= +\frac{3}{4}\frac{\Theta}{x}\int_0^\infty y f_0(y; \Theta) \ln \left| \frac{(2xy - x^2)^2}{(2xy + x^2)^2} \right| dy \Rightarrow \\ \frac{\chi_0(\mathbf{x})}{n\beta} &= +2\frac{3}{4}\frac{\Theta}{x}\int_0^\infty y f_0(y; \Theta) \ln \left| \frac{2xy - x^2}{2xy + x^2} \right| dy \Rightarrow \\ \frac{\chi_0(\mathbf{x})}{n\beta} &= +\frac{3}{2}\frac{\Theta}{x}\int_0^\infty y f_0(y; \Theta) \ln \left| \frac{2y - x}{2y + x} \right| dy \Rightarrow \\ \frac{\chi_0(\mathbf{x})}{n\beta} &= -\frac{3}{2}\frac{\Theta}{x}\int_0^\infty y f_0(y; \Theta) \ln \left| \frac{x + 2y}{x - 2y} \right| dy.\end{aligned}$$

The long wavelength limit of the static Lindhard response is easily obtained by Taylor expanding the two logarithms. The first eleven terms read as

$$\begin{aligned}\frac{\chi_0(\mathbf{x})}{n\beta} &= -\frac{3}{2}\frac{\Theta}{x}\int_0^\infty dy y f_0(y; \Theta) \ln \left| \frac{x + 2y}{x - 2y} \right| \Rightarrow \\ \frac{\chi_0(\mathbf{x})}{n\beta} &= -\frac{3}{2}\Theta\int_0^\infty dy f_0(y; \Theta) \frac{y}{x} \ln \left| \frac{1 + \frac{x}{2y}}{1 - \frac{x}{2y}} \right| \Rightarrow \\ \frac{\chi_0(\mathbf{x})}{n\beta} &= -\frac{3}{2}\Theta\int_0^\infty dy f_0(y; \Theta) \frac{y}{x} \left[ \ln \left| 1 + \frac{x}{2y} \right| - \ln \left| 1 - \frac{x}{2y} \right| \right] \Rightarrow \\ \frac{\chi_0(\mathbf{x})}{n\beta} &= -\frac{3}{2}\Theta\int_0^\infty dy f_0(y; \Theta) \frac{y}{x} \left[ \sum_{n=1}^\infty (-1)^{n+1} \frac{1}{n} \left( \frac{x}{2y} \right)^n + \sum_{n=1}^\infty \frac{1}{n} \left( \frac{x}{2y} \right)^n \right] \Rightarrow \\ \frac{\chi_0(\mathbf{x})}{n\beta} &= -\frac{3}{2}\Theta\int_0^\infty dy f_0(y; \Theta) \frac{y}{x} \sum_{n=1}^\infty [(-1)^{n+1} + 1] \frac{1}{n} \left( \frac{x}{2y} \right)^n \Rightarrow \\ \frac{\chi_0(\mathbf{x})}{n\beta} &= -\frac{3}{2}\Theta\int_0^\infty dy f_0(y; \Theta) \frac{y}{x} \sum_{n=1}^\infty 2\delta_{n,2k-1} \frac{1}{n} \left( \frac{x}{2y} \right)^n \Rightarrow \\ \frac{\chi_0(\mathbf{x})}{n\beta} &= -\frac{3}{2}\Theta\int_0^\infty dy f_0(y; \Theta) \frac{y}{x} \sum_{k=1}^\infty \frac{2}{2k-1} \left( \frac{x}{2y} \right)^{2k-1} \Rightarrow \\ \frac{\chi_0(\mathbf{x})}{n\beta} &= -\frac{3}{2}\Theta\int_0^\infty dy f_0(y; \Theta) \frac{y}{x} \sum_{n=0}^\infty \frac{2}{2n+1} \left( \frac{x}{2y} \right)^{2n+1} \Rightarrow \\ \frac{\chi_0(\mathbf{x})}{n\beta} &= -\frac{3}{2}\Theta\int_0^\infty dy f_0(y; \Theta) \sum_{n=0}^\infty \frac{2}{2n+1} \frac{x}{2y} \frac{y}{x} \left( \frac{x}{2y} \right)^{2n} \Rightarrow \\ \frac{\chi_0(\mathbf{x})}{n\beta} &= -\frac{3}{2}\Theta\int_0^\infty dy f_0(y; \Theta) \sum_{n=0}^\infty \frac{1}{2n+1} \frac{x}{2y} \frac{2y}{x} \left( \frac{x}{2y} \right)^{2n} \Rightarrow \\ \frac{\chi_0(\mathbf{x})}{n\beta} &= -\frac{3}{2}\Theta\int_0^\infty dy f_0(y; \Theta) \sum_{n=0}^\infty \frac{1}{2n+1} \left( \frac{x}{2y} \right)^{2n} \Rightarrow \\ \frac{\chi_0(\mathbf{x})}{n\beta} &\simeq -\frac{3}{2}\Theta\int_0^\infty dy f_0(y; \Theta) \left[ 1 + \frac{1}{3} \left( \frac{x}{2y} \right)^2 + \frac{1}{5} \left( \frac{x}{2y} \right)^4 + \frac{1}{7} \left( \frac{x}{2y} \right)^6 + \frac{1}{9} \left( \frac{x}{2y} \right)^8 + \frac{1}{11} \left( \frac{x}{2y} \right)^{10} \right. \\ &\quad \left. + \frac{1}{13} \left( \frac{x}{2y} \right)^{12} + \frac{1}{15} \left( \frac{x}{2y} \right)^{14} + \frac{1}{17} \left( \frac{x}{2y} \right)^{16} + \frac{1}{19} \left( \frac{x}{2y} \right)^{18} + \frac{1}{21} \left( \frac{x}{2y} \right)^{20} \right] \Rightarrow \\ \frac{\chi_0(\mathbf{x})}{n\beta} &\simeq -\frac{3}{2}\Theta\int_0^\infty dy f_0(y; \Theta) \left[ 1 + \frac{1}{3} \frac{1}{4} \left( \frac{x}{y} \right)^2 + \frac{1}{5} \frac{1}{16} \left( \frac{x}{y} \right)^4 + \frac{1}{7} \frac{1}{64} \left( \frac{x}{y} \right)^6 + \frac{1}{9} \frac{1}{256} \left( \frac{x}{y} \right)^8 + \frac{1}{11} \frac{1}{1024} \left( \frac{x}{y} \right)^{10} \right. \\ &\quad \left. + \frac{1}{13} \frac{1}{4096} \left( \frac{x}{y} \right)^{12} + \frac{1}{15} \frac{1}{16384} \left( \frac{x}{y} \right)^{14} + \frac{1}{17} \frac{1}{65536} \left( \frac{x}{y} \right)^{16} + \frac{1}{19} \frac{1}{262144} \left( \frac{x}{y} \right)^{18} + \frac{1}{21} \frac{1}{1048576} \left( \frac{x}{y} \right)^{20} \right].\end{aligned}$$

## B. The second-order (quadratic) ideal density response

**The general expression.** It is evident that the first and the second expression (for  $n = 2$ ) of the general recurrence relation will be utilized. The relevant arguments of the linear distribution function perturbation are first identified. We simply have

$$\begin{aligned} f_{\mathbf{q},\mathbf{k},\omega}^{\text{ind},(1)} &= - \left[ \frac{f_0(\mathbf{q} + \frac{1}{2}\mathbf{k}) - f_0(\mathbf{q} - \frac{1}{2}\mathbf{k})}{\hbar\omega - \epsilon_{\mathbf{q}+\frac{1}{2}\mathbf{k}} + \epsilon_{\mathbf{q}-\frac{1}{2}\mathbf{k}} + i0} \right] U_{\mathbf{k},\omega}^{\text{ext}} \Rightarrow \\ f_{\mathbf{q}+\frac{1}{2}\mathbf{k}',\mathbf{k}-\mathbf{k}',\omega-\omega'}^{\text{ind},(1)} &= - \left[ \frac{f_0[\mathbf{q} + \frac{1}{2}\mathbf{k}' + \frac{1}{2}(\mathbf{k}-\mathbf{k}')] - f_0[\mathbf{q} + \frac{1}{2}\mathbf{k}' - \frac{1}{2}(\mathbf{k}-\mathbf{k}')] }{\hbar(\omega-\omega') - \epsilon_{\mathbf{q}+\frac{1}{2}\mathbf{k}'+\frac{1}{2}(\mathbf{k}-\mathbf{k}')} + \epsilon_{\mathbf{q}+\frac{1}{2}\mathbf{k}'-\frac{1}{2}(\mathbf{k}-\mathbf{k}')} + i0} \right] U_{\mathbf{k}-\mathbf{k}',\omega-\omega'}^{\text{ext}}, \\ f_{\mathbf{q}-\frac{1}{2}\mathbf{k}',\mathbf{k}-\mathbf{k}',\omega-\omega'}^{\text{ind},(1)} &= - \left[ \frac{f_0[\mathbf{q} - \frac{1}{2}\mathbf{k}' + \frac{1}{2}(\mathbf{k}-\mathbf{k}')] - f_0[\mathbf{q} - \frac{1}{2}\mathbf{k}' - \frac{1}{2}(\mathbf{k}-\mathbf{k}')] }{\hbar(\omega-\omega') - \epsilon_{\mathbf{q}-\frac{1}{2}\mathbf{k}'+\frac{1}{2}(\mathbf{k}-\mathbf{k}')} + \epsilon_{\mathbf{q}-\frac{1}{2}\mathbf{k}'-\frac{1}{2}(\mathbf{k}-\mathbf{k}')} + i0} \right] U_{\mathbf{k}-\mathbf{k}',\omega-\omega'}^{\text{ext}}. \end{aligned}$$

Then, the linear perturbation is substituted into the second-order perturbation of the one-particle distribution function. It is also useful to employ  $\hbar\omega = \hbar(\omega - \omega') + \hbar\omega'$  and  $\mathbf{k} = (\mathbf{k} - \mathbf{k}') + \mathbf{k}'$  in the denominator in order to symmetrize the integral with respect to the arguments of the potential energy perturbations. The integration of the second order one-particle distribution function perturbation over the momentum space is connected to the second order density perturbation,  $n_{\text{ind}}^{(2)}(\mathbf{k}, \omega) = 2 \int [d^3q/(2\pi)^3] f_{\mathbf{q},\mathbf{k},\omega}^{\text{ind},(2)}$ .

$$\begin{aligned} f_{\mathbf{q},\mathbf{k},\omega}^{\text{ind},(2)} &= - \int \frac{d\omega' d^3k'}{(2\pi)^4} \left[ \frac{f_{\mathbf{q}+\frac{1}{2}\mathbf{k}',\mathbf{k}-\mathbf{k}',\omega-\omega'}^{\text{ind},(1)} - f_{\mathbf{q}-\frac{1}{2}\mathbf{k}',\mathbf{k}-\mathbf{k}',\omega-\omega'}^{\text{ind},(1)}}{\hbar\omega - \epsilon_{\mathbf{q}+\frac{1}{2}\mathbf{k}} + \epsilon_{\mathbf{q}-\frac{1}{2}\mathbf{k}} + i0} \right] U_{\mathbf{k}',\omega'}^{\text{ext}} \Rightarrow \\ f_{\mathbf{q},\mathbf{k},\omega}^{\text{ind},(2)} &= - \int \frac{d\omega' d^3k'}{(2\pi)^4} \left[ \frac{f_{\mathbf{q}+\frac{1}{2}\mathbf{k}',\mathbf{k}-\mathbf{k}',\omega-\omega'}^{\text{ind},(1)} - f_{\mathbf{q}-\frac{1}{2}\mathbf{k}',\mathbf{k}-\mathbf{k}',\omega-\omega'}^{\text{ind},(1)}}{\hbar(\omega-\omega') + \hbar\omega' - \epsilon_{\mathbf{q}+\frac{1}{2}\mathbf{k}-\frac{1}{2}\mathbf{k}'+\frac{1}{2}\mathbf{k}'} + \epsilon_{\mathbf{q}-\frac{1}{2}\mathbf{k}+\frac{1}{2}\mathbf{k}'-\frac{1}{2}\mathbf{k}'} + i0} \right] U_{\mathbf{k}',\omega'}^{\text{ext}} \Rightarrow \\ f_{\mathbf{q},\mathbf{k},\omega}^{\text{ind},(2)} &= - \int \frac{d\omega' d^3k'}{(2\pi)^4} \left[ \frac{f_{\mathbf{q}+\frac{1}{2}\mathbf{k}',\mathbf{k}-\mathbf{k}',\omega-\omega'}^{\text{ind},(1)} - f_{\mathbf{q}-\frac{1}{2}\mathbf{k}',\mathbf{k}-\mathbf{k}',\omega-\omega'}^{\text{ind},(1)}}{\hbar(\omega-\omega') + \hbar\omega' - \epsilon_{\mathbf{q}+\frac{1}{2}\mathbf{k}'+\frac{1}{2}(\mathbf{k}-\mathbf{k}')} + \epsilon_{\mathbf{q}-\frac{1}{2}\mathbf{k}'-\frac{1}{2}(\mathbf{k}-\mathbf{k}')} + i0} \right] U_{\mathbf{k}',\omega'}^{\text{ext}} \Rightarrow \\ f_{\mathbf{q},\mathbf{k},\omega}^{\text{ind},(2)} &= - \int \frac{d\omega' d^3k'}{(2\pi)^4} \frac{1}{\hbar(\omega-\omega') + \hbar\omega' - \epsilon_{\mathbf{q}+\frac{1}{2}\mathbf{k}'+\frac{1}{2}(\mathbf{k}-\mathbf{k}')} + \epsilon_{\mathbf{q}-\frac{1}{2}\mathbf{k}'-\frac{1}{2}(\mathbf{k}-\mathbf{k}')} + i0} \\ &\quad \left[ f_{\mathbf{q}+\frac{1}{2}\mathbf{k}',\mathbf{k}-\mathbf{k}',\omega-\omega'}^{\text{ind},(1)} - f_{\mathbf{q}-\frac{1}{2}\mathbf{k}',\mathbf{k}-\mathbf{k}',\omega-\omega'}^{\text{ind},(1)} \right] U_{\mathbf{k}',\omega'}^{\text{ext}} \Rightarrow \\ f_{\mathbf{k},\omega}^{\text{ind},(2)} &= - \int \frac{d\omega' d^3k'}{(2\pi)^4} \frac{d^3q}{(2\pi)^3} \frac{2}{\hbar(\omega-\omega') + \hbar\omega' - \epsilon_{\mathbf{q}+\frac{1}{2}\mathbf{k}'+\frac{1}{2}(\mathbf{k}-\mathbf{k}')} + \epsilon_{\mathbf{q}-\frac{1}{2}\mathbf{k}'-\frac{1}{2}(\mathbf{k}-\mathbf{k}')} + i0} \\ &\quad \left[ f_{\mathbf{q}+\frac{1}{2}\mathbf{k}',\mathbf{k}-\mathbf{k}',\omega-\omega'}^{\text{ind},(1)} - f_{\mathbf{q}-\frac{1}{2}\mathbf{k}',\mathbf{k}-\mathbf{k}',\omega-\omega'}^{\text{ind},(1)} \right] U_{\mathbf{k}',\omega'}^{\text{ext}} \Rightarrow \\ n_{\text{ind}}^{(2)}(\mathbf{k}, \omega) &= + \int \frac{d\omega' d^3k'}{(2\pi)^4} \frac{d^3q}{(2\pi)^3} \frac{2}{\hbar(\omega-\omega') + \hbar\omega' - \epsilon_{\mathbf{q}+\frac{1}{2}\mathbf{k}'+\frac{1}{2}(\mathbf{k}-\mathbf{k}')} + \epsilon_{\mathbf{q}-\frac{1}{2}\mathbf{k}'-\frac{1}{2}(\mathbf{k}-\mathbf{k}')} + i0} U_{\mathbf{k}-\mathbf{k}',\omega-\omega'}^{\text{ext}} U_{\mathbf{k}',\omega'}^{\text{ext}} \\ &\quad \left[ \frac{f_0[\mathbf{q} + \frac{1}{2}\mathbf{k}' + \frac{1}{2}(\mathbf{k}-\mathbf{k}')] - f_0[\mathbf{q} + \frac{1}{2}\mathbf{k}' - \frac{1}{2}(\mathbf{k}-\mathbf{k}')] }{\hbar(\omega-\omega') - \epsilon_{\mathbf{q}+\frac{1}{2}\mathbf{k}'+\frac{1}{2}(\mathbf{k}-\mathbf{k}')} + \epsilon_{\mathbf{q}+\frac{1}{2}\mathbf{k}'-\frac{1}{2}(\mathbf{k}-\mathbf{k}')} + i0} - \frac{f_0[\mathbf{q} - \frac{1}{2}\mathbf{k}' + \frac{1}{2}(\mathbf{k}-\mathbf{k}')] - f_0[\mathbf{q} - \frac{1}{2}\mathbf{k}' - \frac{1}{2}(\mathbf{k}-\mathbf{k}')] }{\hbar(\omega-\omega') - \epsilon_{\mathbf{q}-\frac{1}{2}\mathbf{k}'+\frac{1}{2}(\mathbf{k}-\mathbf{k}')} + \epsilon_{\mathbf{q}-\frac{1}{2}\mathbf{k}'-\frac{1}{2}(\mathbf{k}-\mathbf{k}')} + i0} \right]. \end{aligned}$$

The general definition of the second order density response  $\mathcal{W}_{\mathbf{k}_1,\omega_1;\mathbf{k}_2,\omega_2}^{(2)}$  can now be employed

$$n_{\text{ind}}^{(2)}(\mathbf{k}, \omega) = \int \frac{d\omega' d^3k'}{(2\pi)^4} \mathcal{W}_{\mathbf{k}-\mathbf{k}',\omega-\omega';\mathbf{k}',\omega'}^{(2)} U_{\mathbf{k}-\mathbf{k}',\omega-\omega'}^{\text{ext}} U_{\mathbf{k}',\omega'}^{\text{ext}},$$

in order to acquire an expression for the second order ideal density response  $\mathcal{W}_{\mathbf{k}_1,\omega_1;\mathbf{k}_2,\omega_2}^{(2),0}$ . It is also convenient to set  $\mathbf{k}_1 = \mathbf{k} - \mathbf{k}'$ ,  $\mathbf{k}_2 = \mathbf{k}'$ ,  $\omega_1 = \omega - \omega'$ ,  $\omega_2 = \omega'$ . The calculation proceeds by splitting the four triple integrals and making the variable changes  $\mathbf{q}' = \mathbf{q} + \frac{1}{2}\mathbf{k}_1 + \frac{1}{2}\mathbf{k}_2$ ,  $\mathbf{q}' = \mathbf{q} - \frac{1}{2}\mathbf{k}_1 + \frac{1}{2}\mathbf{k}_2$ ,  $\mathbf{q}' = \mathbf{q} + \frac{1}{2}\mathbf{k}_1 - \frac{1}{2}\mathbf{k}_2$ ,  $\mathbf{q}' = \mathbf{q} - \frac{1}{2}\mathbf{k}_1 - \frac{1}{2}\mathbf{k}_2$  in order to unify the argument of the equilibrium distribution function. It is also beneficial to define the analytic continuation of the second order ideal density response to the complex planes of both frequencies by setting  $z_1 = \omega_1 + i0$ ,  $z_2 = \omega_2 + i0$ .

The four terms are also re-organized into two symmetric terms.

$$\begin{aligned}
\mathcal{W}_{\mathbf{k}-\mathbf{k}', \omega-\omega'; \mathbf{k}', \omega'}^{(2),0} &= \int \frac{d^3 q}{(2\pi)^3} \frac{2}{\hbar(\omega - \omega') + \hbar\omega' - \epsilon_{\mathbf{q}+\frac{1}{2}\mathbf{k}'+\frac{1}{2}(\mathbf{k}-\mathbf{k}')} + \epsilon_{\mathbf{q}-\frac{1}{2}\mathbf{k}'-\frac{1}{2}(\mathbf{k}-\mathbf{k}')} + i0} \\
&\left[ \frac{f_0\left[\mathbf{q} + \frac{1}{2}\mathbf{k}' + \frac{1}{2}(\mathbf{k}-\mathbf{k}')\right] - f_0\left[\mathbf{q} + \frac{1}{2}\mathbf{k}' - \frac{1}{2}(\mathbf{k}-\mathbf{k}')\right]}{\hbar(\omega - \omega') - \epsilon_{\mathbf{q}+\frac{1}{2}\mathbf{k}'+\frac{1}{2}(\mathbf{k}-\mathbf{k}')} + \epsilon_{\mathbf{q}+\frac{1}{2}\mathbf{k}'-\frac{1}{2}(\mathbf{k}-\mathbf{k}')} + i0} - \frac{f_0\left[\mathbf{q} - \frac{1}{2}\mathbf{k}' + \frac{1}{2}(\mathbf{k}-\mathbf{k}')\right] - f_0\left[\mathbf{q} - \frac{1}{2}\mathbf{k}' - \frac{1}{2}(\mathbf{k}-\mathbf{k}')\right]}{\hbar(\omega - \omega') - \epsilon_{\mathbf{q}-\frac{1}{2}\mathbf{k}'+\frac{1}{2}(\mathbf{k}-\mathbf{k}')} + \epsilon_{\mathbf{q}-\frac{1}{2}\mathbf{k}'-\frac{1}{2}(\mathbf{k}-\mathbf{k}')} + i0} \right] \Rightarrow \\
\mathcal{W}_{\mathbf{k}_1, \omega_1; \mathbf{k}_2, \omega_2}^{(2),0} &= \int \frac{d^3 q}{(2\pi)^3} \frac{2}{\hbar\omega_1 + \hbar\omega_2 - \epsilon_{\mathbf{q}+\frac{1}{2}\mathbf{k}_1+\frac{1}{2}\mathbf{k}_2} + \epsilon_{\mathbf{q}-\frac{1}{2}\mathbf{k}_1-\frac{1}{2}\mathbf{k}_2} + i0} \\
&\left[ \frac{f_0\left(\mathbf{q} + \frac{1}{2}\mathbf{k}_1 + \frac{1}{2}\mathbf{k}_2\right) - f_0\left(\mathbf{q} - \frac{1}{2}\mathbf{k}_1 + \frac{1}{2}\mathbf{k}_2\right)}{\hbar\omega_1 - \epsilon_{\mathbf{q}+\frac{1}{2}\mathbf{k}_1+\frac{1}{2}\mathbf{k}_2} + \epsilon_{\mathbf{q}-\frac{1}{2}\mathbf{k}_1+\frac{1}{2}\mathbf{k}_2} + i0} - \frac{f_0\left(\mathbf{q} + \frac{1}{2}\mathbf{k}_1 - \frac{1}{2}\mathbf{k}_2\right) - f_0\left(\mathbf{q} - \frac{1}{2}\mathbf{k}_1 - \frac{1}{2}\mathbf{k}_2\right)}{\hbar\omega_1 - \epsilon_{\mathbf{q}+\frac{1}{2}\mathbf{k}_1-\frac{1}{2}\mathbf{k}_2} + \epsilon_{\mathbf{q}-\frac{1}{2}\mathbf{k}_1-\frac{1}{2}\mathbf{k}_2} + i0} \right] \Rightarrow \\
\mathcal{W}_{\mathbf{k}_1, \omega_1; \mathbf{k}_2, \omega_2}^{(2),0} &= \int \frac{d^3 q}{(2\pi)^3} \frac{2f_0\left(\mathbf{q} + \frac{1}{2}\mathbf{k}_1 + \frac{1}{2}\mathbf{k}_2\right)}{\left(\hbar\omega_1 + \hbar\omega_2 - \epsilon_{\mathbf{q}+\frac{1}{2}\mathbf{k}_1+\frac{1}{2}\mathbf{k}_2} + \epsilon_{\mathbf{q}-\frac{1}{2}\mathbf{k}_1-\frac{1}{2}\mathbf{k}_2} + i0\right) \left(\hbar\omega_1 - \epsilon_{\mathbf{q}+\frac{1}{2}\mathbf{k}_1+\frac{1}{2}\mathbf{k}_2} + \epsilon_{\mathbf{q}-\frac{1}{2}\mathbf{k}_1+\frac{1}{2}\mathbf{k}_2} + i0\right)} \\
&- \int \frac{d^3 q}{(2\pi)^3} \frac{2f_0\left(\mathbf{q} - \frac{1}{2}\mathbf{k}_1 + \frac{1}{2}\mathbf{k}_2\right)}{\left(\hbar\omega_1 + \hbar\omega_2 - \epsilon_{\mathbf{q}+\frac{1}{2}\mathbf{k}_1+\frac{1}{2}\mathbf{k}_2} + \epsilon_{\mathbf{q}-\frac{1}{2}\mathbf{k}_1-\frac{1}{2}\mathbf{k}_2} + i0\right) \left(\hbar\omega_1 - \epsilon_{\mathbf{q}+\frac{1}{2}\mathbf{k}_1+\frac{1}{2}\mathbf{k}_2} + \epsilon_{\mathbf{q}-\frac{1}{2}\mathbf{k}_1+\frac{1}{2}\mathbf{k}_2} + i0\right)} \\
&- \int \frac{d^3 q}{(2\pi)^3} \frac{2f_0\left(\mathbf{q} + \frac{1}{2}\mathbf{k}_1 - \frac{1}{2}\mathbf{k}_2\right)}{\left(\hbar\omega_1 + \hbar\omega_2 - \epsilon_{\mathbf{q}+\frac{1}{2}\mathbf{k}_1+\frac{1}{2}\mathbf{k}_2} + \epsilon_{\mathbf{q}-\frac{1}{2}\mathbf{k}_1-\frac{1}{2}\mathbf{k}_2} + i0\right) \left(\hbar\omega_1 - \epsilon_{\mathbf{q}+\frac{1}{2}\mathbf{k}_1-\frac{1}{2}\mathbf{k}_2} + \epsilon_{\mathbf{q}-\frac{1}{2}\mathbf{k}_1-\frac{1}{2}\mathbf{k}_2} + i0\right)} \\
&+ \int \frac{d^3 q}{(2\pi)^3} \frac{2f_0\left(\mathbf{q} - \frac{1}{2}\mathbf{k}_1 - \frac{1}{2}\mathbf{k}_2\right)}{\left(\hbar\omega_1 + \hbar\omega_2 - \epsilon_{\mathbf{q}+\frac{1}{2}\mathbf{k}_1+\frac{1}{2}\mathbf{k}_2} + \epsilon_{\mathbf{q}-\frac{1}{2}\mathbf{k}_1-\frac{1}{2}\mathbf{k}_2} + i0\right) \left(\hbar\omega_1 - \epsilon_{\mathbf{q}+\frac{1}{2}\mathbf{k}_1-\frac{1}{2}\mathbf{k}_2} + \epsilon_{\mathbf{q}-\frac{1}{2}\mathbf{k}_1-\frac{1}{2}\mathbf{k}_2} + i0\right)} \Rightarrow \\
\mathcal{W}_{\mathbf{k}_1, \omega_1; \mathbf{k}_2, \omega_2}^{(2),0} &= \int \frac{d^3 q'}{(2\pi)^3} \frac{2f_0(q')}{\left(\hbar\omega_1 + \hbar\omega_2 - \epsilon_{q'} + \epsilon_{q'-\frac{1}{2}\mathbf{k}_1-\frac{1}{2}\mathbf{k}_2-\frac{1}{2}\mathbf{k}_1-\frac{1}{2}\mathbf{k}_2} + i0\right) \left(\hbar\omega_1 - \epsilon_{q'} + \epsilon_{q'-\frac{1}{2}\mathbf{k}_1-\frac{1}{2}\mathbf{k}_2-\frac{1}{2}\mathbf{k}_1+\frac{1}{2}\mathbf{k}_2} + i0\right)} \\
&- \int \frac{d^3 q'}{(2\pi)^3} \frac{2f_0(q')}{\left(\hbar\omega_1 + \hbar\omega_2 - \epsilon_{q'+\frac{1}{2}\mathbf{k}_1-\frac{1}{2}\mathbf{k}_2+\frac{1}{2}\mathbf{k}_1+\frac{1}{2}\mathbf{k}_2} + \epsilon_{q'+\frac{1}{2}\mathbf{k}_1-\frac{1}{2}\mathbf{k}_2-\frac{1}{2}\mathbf{k}_1-\frac{1}{2}\mathbf{k}_2} + i0\right) \left(\hbar\omega_1 - \epsilon_{q'+\frac{1}{2}\mathbf{k}_1-\frac{1}{2}\mathbf{k}_2+\frac{1}{2}\mathbf{k}_1+\frac{1}{2}\mathbf{k}_2} + \epsilon_{q'} + i0\right)} \\
&- \int \frac{d^3 q'}{(2\pi)^3} \frac{2f_0(q')}{\left(\hbar\omega_1 + \hbar\omega_2 - \epsilon_{q'-\frac{1}{2}\mathbf{k}_1+\frac{1}{2}\mathbf{k}_2+\frac{1}{2}\mathbf{k}_1+\frac{1}{2}\mathbf{k}_2} + \epsilon_{q'-\frac{1}{2}\mathbf{k}_1+\frac{1}{2}\mathbf{k}_2-\frac{1}{2}\mathbf{k}_1-\frac{1}{2}\mathbf{k}_2} + i0\right) \left(\hbar\omega_1 - \epsilon_{q'} + \epsilon_{q'-\frac{1}{2}\mathbf{k}_1+\frac{1}{2}\mathbf{k}_2-\frac{1}{2}\mathbf{k}_1-\frac{1}{2}\mathbf{k}_2} + i0\right)} \\
&+ \int \frac{d^3 q'}{(2\pi)^3} \frac{2f_0(q')}{\left(\hbar\omega_1 + \hbar\omega_2 - \epsilon_{q'+\frac{1}{2}\mathbf{k}_1+\frac{1}{2}\mathbf{k}_2+\frac{1}{2}\mathbf{k}_1+\frac{1}{2}\mathbf{k}_2} + \epsilon_{q'} + i0\right) \left(\hbar\omega_1 - \epsilon_{q'+\frac{1}{2}\mathbf{k}_1+\frac{1}{2}\mathbf{k}_2+\frac{1}{2}\mathbf{k}_1-\frac{1}{2}\mathbf{k}_2} + \epsilon_{q'} + i0\right)} \Rightarrow \\
\mathcal{W}_{\mathbf{k}_1, \omega_1; \mathbf{k}_2, \omega_2}^{(2),0} &= \int \frac{d^3 q}{(2\pi)^3} \frac{2f_0(q)}{(\hbar\omega_1 + \hbar\omega_2 - \epsilon_{\mathbf{q}} + \epsilon_{\mathbf{q}-\mathbf{k}_1-\mathbf{k}_2} + i0) (\hbar\omega_1 - \epsilon_{\mathbf{q}} + \epsilon_{\mathbf{q}-\mathbf{k}_1} + i0)} \\
&- \int \frac{d^3 q}{(2\pi)^3} \frac{2f_0(q)}{(\hbar\omega_1 + \hbar\omega_2 - \epsilon_{\mathbf{q}+\mathbf{k}_1} + \epsilon_{\mathbf{q}-\mathbf{k}_2} + i0) (\hbar\omega_1 - \epsilon_{\mathbf{q}+\mathbf{k}_1} + \epsilon_{\mathbf{q}} + i0)} \\
&+ \int \frac{d^3 q}{(2\pi)^3} \frac{2f_0(q)}{(\hbar\omega_1 + \hbar\omega_2 - \epsilon_{\mathbf{q}+\mathbf{k}_1+\mathbf{k}_2} + \epsilon_{\mathbf{q}} + i0) (\hbar\omega_1 - \epsilon_{\mathbf{q}+\mathbf{k}_1} + \epsilon_{\mathbf{q}} + i0)} \\
&- \int \frac{d^3 q}{(2\pi)^3} \frac{2f_0(q)}{(\hbar\omega_1 + \hbar\omega_2 - \epsilon_{\mathbf{q}+\mathbf{k}_2} + \epsilon_{\mathbf{q}-\mathbf{k}_1} + i0) (\hbar\omega_1 - \epsilon_{\mathbf{q}} + \epsilon_{\mathbf{q}-\mathbf{k}_1} + i0)} \Rightarrow \\
\mathcal{W}_{\mathbf{k}_1, z_1; \mathbf{k}_2, z_2}^{(2),0} &= \int \frac{d^3 q}{(2\pi)^3} \left[ \frac{2f_0(q)}{(\hbar z_1 + \hbar z_2 - \epsilon_{\mathbf{q}} + \epsilon_{\mathbf{q}-\mathbf{k}_1-\mathbf{k}_2}) (\hbar z_1 - \epsilon_{\mathbf{q}} + \epsilon_{\mathbf{q}-\mathbf{k}_1})} - \frac{2f_0(q)}{(\hbar z_1 + \hbar z_2 - \epsilon_{\mathbf{q}+\mathbf{k}_1} + \epsilon_{\mathbf{q}-\mathbf{k}_2}) (\hbar z_1 - \epsilon_{\mathbf{q}+\mathbf{k}_1} + \epsilon_{\mathbf{q}})} \right] \\
&+ \int \frac{d^3 q}{(2\pi)^3} \left[ \frac{2f_0(q)}{(\hbar z_1 + \hbar z_2 - \epsilon_{\mathbf{q}+\mathbf{k}_1+\mathbf{k}_2} + \epsilon_{\mathbf{q}}) (\hbar z_1 - \epsilon_{\mathbf{q}+\mathbf{k}_1} + \epsilon_{\mathbf{q}})} - \frac{2f_0(q)}{(\hbar z_1 + \hbar z_2 - \epsilon_{\mathbf{q}+\mathbf{k}_2} + \epsilon_{\mathbf{q}-\mathbf{k}_1}) (\hbar z_1 - \epsilon_{\mathbf{q}} + \epsilon_{\mathbf{q}-\mathbf{k}_1})} \right].
\end{aligned}$$

**The symmetric expression and its compact form.** Of particular importance is the symmetric case  $\mathbf{k}_1 = \mathbf{k}_2 = \mathbf{k}$  and  $z_1 = z_2 = z$ , for which a simplified form of the second order ideal density response in terms of the first order ideal density response can be derived,  $\mathcal{W}_{\mathbf{k}, z; \mathbf{k}, z}^{(2),0} = \chi_0^{(2,2)}(\mathbf{k}, z)$ . The calculation is based on splitting the integrands into simple fractions and is facilitated by the fact that the multiplication coefficient of the decomposition turns out to be independent of the integration variable  $\mathbf{q}$ . The cumbersome procedure is carried out separately for each symmetric



[illegible]

$$\begin{aligned}
[\chi_0^{(2,2)}(\mathbf{k}, z)]_2 &= \int \frac{d^3 q}{(2\pi)^3} \left\{ \frac{2f_0(\mathbf{q})}{[\hbar z + \hbar z - \epsilon_{\mathbf{q}+\mathbf{k}+\mathbf{k}} + \epsilon_{\mathbf{q}}][\hbar z - \epsilon_{\mathbf{q}+\mathbf{k}} + \epsilon_{\mathbf{q}}]} - \frac{2f_0(\mathbf{q})}{[\hbar z + \hbar z - \epsilon_{\mathbf{q}+\mathbf{k}} + \epsilon_{\mathbf{q}-\mathbf{k}}][\hbar z - \epsilon_{\mathbf{q}} + \epsilon_{\mathbf{q}-\mathbf{k}}]} \right\} \Rightarrow \\
[\chi_0^{(2,2)}(\mathbf{k}, z)]_2 &= \int \frac{d^3 q}{(2\pi)^3} \left\{ \frac{2f_0(\mathbf{q})}{[2\hbar z - \epsilon_{\mathbf{q}+2\mathbf{k}} + \epsilon_{\mathbf{q}}][\hbar z - \epsilon_{\mathbf{q}+\mathbf{k}} + \epsilon_{\mathbf{q}}]} - \frac{2f_0(\mathbf{q})}{[2\hbar z - \epsilon_{\mathbf{q}+\mathbf{k}} + \epsilon_{\mathbf{q}-\mathbf{k}}][\hbar z - \epsilon_{\mathbf{q}} + \epsilon_{\mathbf{q}-\mathbf{k}}]} \right\} \Rightarrow \\
[\chi_0^{(2,2)}(\mathbf{k}, z)]_2 &= \int \frac{d^3 q}{(2\pi)^3} f_0(\mathbf{q}) \left\{ \frac{1}{[\hbar z - \frac{\epsilon_{\mathbf{q}+2\mathbf{k}} - \epsilon_{\mathbf{q}}}{2}][\hbar z - (\epsilon_{\mathbf{q}+\mathbf{k}} - \epsilon_{\mathbf{q}})]} - \frac{1}{[\hbar z - \frac{\epsilon_{\mathbf{q}+\mathbf{k}} - \epsilon_{\mathbf{q}-\mathbf{k}}}{2}][\hbar z - (\epsilon_{\mathbf{q}} - \epsilon_{\mathbf{q}-\mathbf{k}})]} \right\} \Rightarrow \\
[\chi_0^{(2,2)}(\mathbf{k}, z)]_2 &= \int \frac{d^3 q}{(2\pi)^3} f_0(\mathbf{q}) \left\{ \left[ \frac{1}{\hbar z - \frac{\epsilon_{\mathbf{q}+2\mathbf{k}} - \epsilon_{\mathbf{q}}}{2}} - \frac{1}{\hbar z - (\epsilon_{\mathbf{q}+\mathbf{k}} - \epsilon_{\mathbf{q}})} \right] \frac{1}{\frac{\epsilon_{\mathbf{q}+2\mathbf{k}} - \epsilon_{\mathbf{q}}}{2} - \epsilon_{\mathbf{q}+\mathbf{k}} + \epsilon_{\mathbf{q}}} \right. \\
&\quad \left. - \left[ \frac{1}{\hbar z - \frac{\epsilon_{\mathbf{q}+\mathbf{k}} - \epsilon_{\mathbf{q}-\mathbf{k}}}{2}} - \frac{1}{\hbar z - (\epsilon_{\mathbf{q}} - \epsilon_{\mathbf{q}-\mathbf{k}})} \right] \frac{1}{\frac{\epsilon_{\mathbf{q}+\mathbf{k}} - \epsilon_{\mathbf{q}-\mathbf{k}}}{2} - \epsilon_{\mathbf{q}} + \epsilon_{\mathbf{q}-\mathbf{k}}} \right\} \Rightarrow \\
[\chi_0^{(2,2)}(\mathbf{k}, z)]_2 &= \int \frac{d^3 q}{(2\pi)^3} 2f_0(\mathbf{q}) \left\{ \left[ \frac{1}{\hbar z - \frac{\epsilon_{\mathbf{q}+2\mathbf{k}} - \epsilon_{\mathbf{q}}}{2}} - \frac{1}{\hbar z - (\epsilon_{\mathbf{q}+\mathbf{k}} - \epsilon_{\mathbf{q}})} \right] \frac{1}{\epsilon_{\mathbf{q}+2\mathbf{k}} - \epsilon_{\mathbf{q}} - 2\epsilon_{\mathbf{q}+\mathbf{k}} + 2\epsilon_{\mathbf{q}}} \right. \\
&\quad \left. - \left[ \frac{1}{\hbar z - \frac{\epsilon_{\mathbf{q}+\mathbf{k}} - \epsilon_{\mathbf{q}-\mathbf{k}}}{2}} - \frac{1}{\hbar z - (\epsilon_{\mathbf{q}} - \epsilon_{\mathbf{q}-\mathbf{k}})} \right] \frac{1}{\epsilon_{\mathbf{q}+\mathbf{k}} - \epsilon_{\mathbf{q}-\mathbf{k}} - 2\epsilon_{\mathbf{q}} + 2\epsilon_{\mathbf{q}-\mathbf{k}}} \right\} \Rightarrow \\
[\chi_0^{(2,2)}(\mathbf{k}, z)]_2 &= \int \frac{d^3 q}{(2\pi)^3} 2f_0(\mathbf{q}) \left\{ \left[ \frac{1}{\hbar z - \frac{\epsilon_{\mathbf{q}+2\mathbf{k}} - \epsilon_{\mathbf{q}}}{2}} - \frac{1}{\hbar z - (\epsilon_{\mathbf{q}+\mathbf{k}} - \epsilon_{\mathbf{q}})} \right] \frac{1}{\epsilon_{\mathbf{q}+2\mathbf{k}} - 2\epsilon_{\mathbf{q}+\mathbf{k}} + \epsilon_{\mathbf{q}}} \right. \\
&\quad \left. - \left[ \frac{1}{\hbar z - \frac{\epsilon_{\mathbf{q}+\mathbf{k}} - \epsilon_{\mathbf{q}-\mathbf{k}}}{2}} - \frac{1}{\hbar z - (\epsilon_{\mathbf{q}} - \epsilon_{\mathbf{q}-\mathbf{k}})} \right] \frac{1}{\epsilon_{\mathbf{q}+\mathbf{k}} - 2\epsilon_{\mathbf{q}} + \epsilon_{\mathbf{q}-\mathbf{k}}} \right\} \Rightarrow \\
[\chi_0^{(2,2)}(\mathbf{k}, z)]_2 &= \int \frac{d^3 q}{(2\pi)^3} 2f_0(\mathbf{q}) \left\{ \left[ \frac{1}{\hbar z - \frac{\epsilon_{\mathbf{q}+2\mathbf{k}} - \epsilon_{\mathbf{q}}}{2}} - \frac{1}{\hbar z - (\epsilon_{\mathbf{q}+\mathbf{k}} - \epsilon_{\mathbf{q}})} \right] \frac{1}{\frac{\hbar^2}{2m} [(q+2k)^2 - 2(q+k)^2 + q^2]} \right. \\
&\quad \left. - \left[ \frac{1}{\hbar z - \frac{\epsilon_{\mathbf{q}+\mathbf{k}} - \epsilon_{\mathbf{q}-\mathbf{k}}}{2}} - \frac{1}{\hbar z - (\epsilon_{\mathbf{q}} - \epsilon_{\mathbf{q}-\mathbf{k}})} \right] \frac{1}{\frac{\hbar^2}{2m} [(q+k)^2 - 2q^2 + (q-k)^2]} \right\} \Rightarrow \\
[\chi_0^{(2,2)}(\mathbf{k}, z)]_2 &= \int \frac{d^3 q}{(2\pi)^3} 2f_0(\mathbf{q}) \left\{ \left[ \frac{1}{\hbar z - \frac{\epsilon_{\mathbf{q}+2\mathbf{k}} - \epsilon_{\mathbf{q}}}{2}} - \frac{1}{\hbar z - (\epsilon_{\mathbf{q}+\mathbf{k}} - \epsilon_{\mathbf{q}})} \right] \frac{1}{\frac{\hbar^2}{2m} (q^2 + 4k^2 + 4\mathbf{q} \cdot \mathbf{k} - 2q^2 - 2k^2 - 4\mathbf{q} \cdot \mathbf{k} + q^2)} \right. \\
&\quad \left. - \left[ \frac{1}{\hbar z - \frac{\epsilon_{\mathbf{q}+\mathbf{k}} - \epsilon_{\mathbf{q}-\mathbf{k}}}{2}} - \frac{1}{\hbar z - (\epsilon_{\mathbf{q}} - \epsilon_{\mathbf{q}-\mathbf{k}})} \right] \frac{1}{\frac{\hbar^2}{2m} (q^2 + k^2 + 2\mathbf{q} \cdot \mathbf{k} - 2q^2 + q^2 + k^2 - 2\mathbf{q} \cdot \mathbf{k})} \right\} \Rightarrow \\
[\chi_0^{(2,2)}(\mathbf{k}, z)]_2 &= \int \frac{d^3 q}{(2\pi)^3} 2f_0(\mathbf{q}) \left\{ \left[ \frac{1}{\hbar z - \frac{\epsilon_{\mathbf{q}+2\mathbf{k}} - \epsilon_{\mathbf{q}}}{2}} - \frac{1}{\hbar z - (\epsilon_{\mathbf{q}+\mathbf{k}} - \epsilon_{\mathbf{q}})} \right] \frac{1}{\frac{\hbar^2}{2m} (2k^2)} \right. \\
&\quad \left. - \left[ \frac{1}{\hbar z - \frac{\epsilon_{\mathbf{q}+\mathbf{k}} - \epsilon_{\mathbf{q}-\mathbf{k}}}{2}} - \frac{1}{\hbar z - (\epsilon_{\mathbf{q}} - \epsilon_{\mathbf{q}-\mathbf{k}})} \right] \frac{1}{\frac{\hbar^2}{2m} (2k^2)} \right\} \Rightarrow \\
[\chi_0^{(2,2)}(\mathbf{k}, z)]_2 &= 2 \frac{m}{\hbar^2} \frac{1}{k^2} \int \frac{d^3 q}{(2\pi)^3} f_0(\mathbf{q}) \left[ \frac{1}{\hbar z - \frac{\epsilon_{\mathbf{q}+2\mathbf{k}} - \epsilon_{\mathbf{q}}}{2}} - \frac{1}{\hbar z - (\epsilon_{\mathbf{q}+\mathbf{k}} - \epsilon_{\mathbf{q}})} - \frac{1}{\hbar z - \frac{\epsilon_{\mathbf{q}+\mathbf{k}} - \epsilon_{\mathbf{q}-\mathbf{k}}}{2}} + \frac{1}{\hbar z - (\epsilon_{\mathbf{q}} - \epsilon_{\mathbf{q}-\mathbf{k}})} \right] \Rightarrow \\
[\chi_0^{(2,2)}(\mathbf{k}, z)]_2 &= 2 \frac{m}{\hbar^2} \frac{1}{k^2} \int \frac{d^3 q}{(2\pi)^3} f_0(\mathbf{q}) \left[ \frac{2}{\hbar(2z) - \epsilon_{\mathbf{q}+2\mathbf{k}} + \epsilon_{\mathbf{q}}} - \frac{2}{\hbar(2z) - \epsilon_{\mathbf{q}+\mathbf{k}} + \epsilon_{\mathbf{q}-\mathbf{k}}} + \frac{1}{\hbar z - \epsilon_{\mathbf{q}} + \epsilon_{\mathbf{q}-\mathbf{k}}} - \frac{1}{\hbar z - \epsilon_{\mathbf{q}+\mathbf{k}} + \epsilon_{\mathbf{q}}} \right] \Rightarrow \\
[\chi_0^{(2,2)}(\mathbf{k}, z)]_2 &= -2 \frac{m}{\hbar^2} \frac{1}{k^2} \int \frac{d^3 q}{(2\pi)^3} f_0(\mathbf{q}) \left[ \frac{2}{\hbar(2z) - \epsilon_{\mathbf{q}+\mathbf{k}} + \epsilon_{\mathbf{q}-\mathbf{k}}} - \frac{2}{\hbar(2z) - \epsilon_{\mathbf{q}+2\mathbf{k}} + \epsilon_{\mathbf{q}}} + \frac{1}{\hbar z - \epsilon_{\mathbf{q}+\mathbf{k}} + \epsilon_{\mathbf{q}}} - \frac{1}{\hbar z - \epsilon_{\mathbf{q}} + \epsilon_{\mathbf{q}-\mathbf{k}}} \right].
\end{aligned}$$

Combining the above two symmetric adders, the undesired terms that cannot be expressed in terms of ideal Lindhard density responses cancel out exactly. After appropriate regrouping of the remaining six terms (or more appropriately the remaining four unique terms), the difference of two ideal Lindhard density responses, that are evaluated at different multiple wavenumber and complex frequency arguments, emerges. The so-called second order Mikhailov recursion

relation ultimately reads as

$$\begin{aligned}
\chi_0^{(2,2)}(\mathbf{k}, z) &= -2 \frac{m}{\hbar^2} \frac{1}{k^2} \int \frac{d^3 q}{(2\pi)^3} f_0(\mathbf{q}) \left[ \frac{2}{\hbar(2z) - \epsilon_{\mathbf{q}} + \epsilon_{\mathbf{q}-2\mathbf{k}}} - \frac{2}{\hbar(2z) - \epsilon_{\mathbf{q}+\mathbf{k}} + \epsilon_{\mathbf{q}-\mathbf{k}}} + \frac{1}{\hbar z - \epsilon_{\mathbf{q}+\mathbf{k}} + \epsilon_{\mathbf{q}}} - \frac{1}{\hbar z - \epsilon_{\mathbf{q}} + \epsilon_{\mathbf{q}-\mathbf{k}}} \right. \\
&\quad \left. + \frac{2}{\hbar(2z) - \epsilon_{\mathbf{q}+\mathbf{k}} + \epsilon_{\mathbf{q}-\mathbf{k}}} - \frac{2}{\hbar(2z) - \epsilon_{\mathbf{q}+2\mathbf{k}} + \epsilon_{\mathbf{q}}} + \frac{1}{\hbar z - \epsilon_{\mathbf{q}+\mathbf{k}} + \epsilon_{\mathbf{q}}} - \frac{1}{\hbar z - \epsilon_{\mathbf{q}} + \epsilon_{\mathbf{q}-\mathbf{k}}} \right] \Rightarrow \\
\chi_0^{(2,2)}(\mathbf{k}, z) &= -2 \frac{m}{\hbar^2} \frac{1}{k^2} \int \frac{d^3 q}{(2\pi)^3} f_0(\mathbf{q}) \left[ \frac{2}{\hbar(2z) - \epsilon_{\mathbf{q}} + \epsilon_{\mathbf{q}-2\mathbf{k}}} - \frac{2}{\hbar(2z) - \epsilon_{\mathbf{q}+2\mathbf{k}} + \epsilon_{\mathbf{q}}} + \frac{2}{\hbar z - \epsilon_{\mathbf{q}+\mathbf{k}} + \epsilon_{\mathbf{q}}} - \frac{2}{\hbar z - \epsilon_{\mathbf{q}} + \epsilon_{\mathbf{q}-\mathbf{k}}} \right] \Rightarrow \\
\chi_0^{(2,2)}(\mathbf{k}, z) &= \frac{m}{\hbar^2} \frac{2}{k^2} \left\{ -2 \int \frac{d^3 q}{(2\pi)^3} f_0(\mathbf{q}) \left[ \frac{1}{\hbar(2z) - \epsilon_{\mathbf{q}} + \epsilon_{\mathbf{q}-2\mathbf{k}}} - \frac{1}{\hbar(2z) - \epsilon_{\mathbf{q}+2\mathbf{k}} + \epsilon_{\mathbf{q}}} \right] \right. \\
&\quad \left. + 2 \int \frac{d^3 q}{(2\pi)^3} f_0(\mathbf{q}) \left[ \frac{1}{\hbar z - \epsilon_{\mathbf{q}} + \epsilon_{\mathbf{q}-\mathbf{k}}} - \frac{1}{\hbar z - \epsilon_{\mathbf{q}+\mathbf{k}} + \epsilon_{\mathbf{q}}} \right] \right\} \Rightarrow \\
\chi_0^{(2,2)}(\mathbf{k}, z) &= 2 \frac{m}{\hbar^2} \frac{1}{k^2} [\chi_0(2\mathbf{k}, 2z) - \chi_0(\mathbf{k}, z)] .
\end{aligned}$$

**The normalized compact form of the symmetric expression.** From the definition of the second order ideal density response as the second order functional derivative of the density with respect to the external potential energy, it is evident that the proper normalization is achieved by dividing with  $1/(n\beta^2)$ . In addition from the definition of the first order ideal density response as the first order functional derivative of the density with respect to the external potential energy, it is evident that the proper normalization of the Lindhard response is achieved by dividing with  $1/(n\beta)$ . The calculation proceeds with the introduction of the dimensionless complex frequency  $z = (T/\hbar)Z$  as well as of the dimensionless wavenumber  $k = k_F x$ . The utilization of the Fermi energy definition  $E_F = \hbar^2 k_F^2 / (2m)$  and the introduction of the degeneracy temperature definition  $\Theta = T/E_F$  ultimately lead to

$$\begin{aligned}
\chi_0^{(2,2)}(\mathbf{k}, z) &= 2 \frac{m}{\hbar^2} \frac{1}{k^2} [\chi_0(2\mathbf{k}, 2z) - \chi_0(\mathbf{k}, z)] \Rightarrow \\
\frac{\chi_0^{(2,2)}(\mathbf{k}, z)}{n\beta^2} &= \frac{1}{n\beta^2} 2 \frac{m}{\hbar^2} \frac{1}{k^2} [\chi_0(2\mathbf{k}, 2z) - \chi_0(\mathbf{k}, z)] \Rightarrow \\
\frac{\chi_0^{(2,2)}(\mathbf{k}, z)}{n\beta^2} &= 2 \frac{m}{\hbar^2} \frac{T}{k^2} \left[ \frac{\chi_0(2\mathbf{k}, 2z)}{n\beta} - \frac{\chi_0(\mathbf{k}, z)}{n\beta} \right] \Rightarrow \\
\frac{\chi_0^{(2,2)}(\mathbf{x}, Z)}{n\beta^2} &= 2 \frac{m}{\hbar^2} \frac{T}{k_F^2 x^2} \left[ \frac{\chi_0(2\mathbf{x}, 2Z)}{n\beta} - \frac{\chi_0(\mathbf{x}, Z)}{n\beta} \right] \Rightarrow \\
\frac{\chi_0^{(2,2)}(\mathbf{x}, Z)}{n\beta^2} &= \frac{2m}{\hbar^2 k_F^2} \frac{T}{x^2} \left[ \frac{\chi_0(2\mathbf{x}, 2Z)}{n\beta} - \frac{\chi_0(\mathbf{x}, Z)}{n\beta} \right] \Rightarrow \\
\frac{\chi_0^{(2,2)}(\mathbf{x}, Z)}{n\beta^2} &= \frac{T}{\hbar^2 k_F^2 / 2m} \frac{1}{x^2} \left[ \frac{\chi_0(2\mathbf{x}, 2Z)}{n\beta} - \frac{\chi_0(\mathbf{x}, Z)}{n\beta} \right] \Rightarrow \\
\frac{\chi_0^{(2,2)}(\mathbf{x}, Z)}{n\beta^2} &= \frac{T}{E_F} \frac{1}{x^2} \left[ \frac{\chi_0(2\mathbf{x}, 2Z)}{n\beta} - \frac{\chi_0(\mathbf{x}, Z)}{n\beta} \right] \Rightarrow \\
\frac{\chi_0^{(2,2)}(\mathbf{x}, Z)}{n\beta^2} &= \frac{\Theta}{x^2} \left[ \frac{\chi_0(2\mathbf{x}, 2Z)}{n\beta} - \frac{\chi_0(\mathbf{x}, Z)}{n\beta} \right] \Rightarrow \\
\frac{\chi_0^{(2,2)}(\mathbf{x}, Z)}{n\beta^2} &= \frac{1}{2} \frac{\Theta}{x^2} \left[ 2 \frac{\chi_0(2\mathbf{x}, 2Z)}{n\beta} - 2 \frac{\chi_0(\mathbf{x}, Z)}{n\beta} \right] \Rightarrow \\
\frac{\chi_0^{(2,2)}(\mathbf{x}, Z)}{n\beta^2} &= \frac{1}{2!} \frac{\Theta}{x^2} \left[ 2 \frac{\chi_0(2\mathbf{x}, 2Z)}{n\beta} - 2 \frac{\chi_0(\mathbf{x}, Z)}{n\beta} \right] \Rightarrow \\
\frac{\chi_0^{(2,2)}(\mathbf{x}, Z)}{n\beta^2} &= \frac{1}{(2-1)!} \frac{1}{2!} \frac{\Theta}{x^2} \left[ 2 \frac{\chi_0(2\mathbf{x}, 2Z)}{n\beta} - 2 \frac{\chi_0(\mathbf{x}, Z)}{n\beta} \right] .
\end{aligned}$$

In the final steps, the numerical pre-factors were decomposed into products that were later expressed as factorials with respect to the order of the ideal density response. Ultimately, one has

$$\frac{\chi_0^{(2,2)}(\mathbf{x}, Z)}{n\beta^2} = \frac{1}{(2-1)!} \frac{1}{2!} \frac{\Theta}{x^2} \left[ 2 \frac{\chi_0(2\mathbf{x}, 2Z)}{n\beta} - 2 \frac{\chi_0(\mathbf{x}, Z)}{n\beta} \right].$$

The static limit simply reads as

$$\frac{\chi_0^{(2,2)}(\mathbf{x})}{n\beta^2} = \frac{1}{(2-1)!} \frac{1}{2!} \frac{\Theta}{x^2} \left[ 2 \frac{\chi_0(2\mathbf{x})}{n\beta} - 2 \frac{\chi_0(\mathbf{x})}{n\beta} \right].$$

**The long wavelength limit of the static normalized symmetric expression.** The long-wavelength limit of the static second order ideal density response at the second harmonic should converge. Given the  $1/x^2$  pre-factor and the even parity, this implies that the first term of the small argument expansion of the ideal quadratic density response should cancel out exactly, otherwise the long-wavelength limit of the static case would diverge. We first write down the first two terms of the small argument expansion of the ideal Lindhard density response for the arguments  $2\mathbf{x}$ ,  $\mathbf{x}$ .

$$\begin{aligned} \frac{\chi_0(\mathbf{x})}{n\beta} &\simeq -\frac{3}{2}\Theta \int_0^\infty dy f_0(y; \Theta) \left[ 1 + \frac{1}{12} \left( \frac{x}{y} \right)^2 \right], \\ \frac{\chi_0(2\mathbf{x})}{n\beta} &\simeq -\frac{3}{2}\Theta \int_0^\infty dy f_0(y; \Theta) \left[ 1 + \frac{1}{3} \left( \frac{x}{y} \right)^2 \right]. \end{aligned}$$

Then, we substitute the above in the static limit of the normalized compact form of the second order ideal density response at the second harmonic. We simply re-organize the terms in ascending powers of  $x/y$ . It is straightforward to prove that the first term,  $\propto (x/y)^0$ , cancels out exactly. The leading order term is  $\mathcal{O}[(x/y)^2]$  and leads to finite contribution at the long-wavelength limit,  $\mathcal{O}(y^{-2})$ , after the removal of the  $1/x^2$  pre-factor. It is rather apparent that the remaining improper integral is indeed convergent.

$$\begin{aligned} \frac{\chi_0^{(2,2)}(\mathbf{x})}{n\beta^2} &= \frac{1}{2} \frac{\Theta}{x^2} \left[ 2 \frac{\chi_0(2\mathbf{x})}{n\beta} - 2 \frac{\chi_0(\mathbf{x})}{n\beta} \right] \Rightarrow \\ \frac{\chi_0^{(2,2)}(\mathbf{x})}{n\beta^2} &= -\frac{1}{2} \frac{\Theta}{x^2} \left\{ 2 \frac{3}{2} \Theta \int_0^\infty dy f_0(y; \Theta) \left[ 1 + \frac{1}{3} \left( \frac{x}{y} \right)^2 \right] - 2 \frac{3}{2} \Theta \int_0^\infty dy f_0(y; \Theta) \left[ 1 + \frac{1}{12} \left( \frac{x}{y} \right)^2 \right] \right\} \Rightarrow \\ \frac{\chi_0^{(2,2)}(\mathbf{x})}{n\beta^2} &= -\frac{3}{2} \frac{\Theta^2}{x^2} \left\{ \int_0^\infty dy f_0(y; \Theta) \left[ 1 + \frac{1}{3} \left( \frac{x}{y} \right)^2 \right] - \int_0^\infty dy f_0(y; \Theta) \left[ 1 + \frac{1}{12} \left( \frac{x}{y} \right)^2 \right] \right\} \Rightarrow \\ \frac{\chi_0^{(2,2)}(\mathbf{x})}{n\beta^2} &= +\frac{3}{2} \frac{\Theta^2}{x^2} \int_0^\infty dy f_0(y; \Theta) \left[ 1 + \frac{1}{12} \left( \frac{x}{y} \right)^2 - 1 - \frac{1}{3} \left( \frac{x}{y} \right)^2 \right] \Rightarrow \\ \frac{\chi_0^{(2,2)}(\mathbf{x})}{n\beta^2} &= +\frac{3}{2} \frac{\Theta^2}{x^2} \int_0^\infty dy f_0(y; \Theta) \left[ 1 - 1 + \frac{1}{12} \left( \frac{x}{y} \right)^2 - \frac{4}{12} \left( \frac{x}{y} \right)^2 \right] \Rightarrow \\ \frac{\chi_0^{(2,2)}(\mathbf{x})}{n\beta^2} &= +\frac{3}{2} \frac{\Theta^2}{x^2} \int_0^\infty dy f_0(y; \Theta) \left[ -\frac{3}{12} \left( \frac{x}{y} \right)^2 \right] \Rightarrow \\ \frac{\chi_0^{(2,2)}(\mathbf{x})}{n\beta^2} &= +\frac{3}{2} \frac{\Theta^2}{x^2} \int_0^\infty dy f_0(y; \Theta) \left[ -\frac{1}{4} \left( \frac{x}{y} \right)^2 \right] \Rightarrow \\ \frac{\chi_0^{(2,2)}(\mathbf{x})}{n\beta^2} &= -\frac{3}{2} \frac{1}{4} \frac{\Theta^2}{x^2} \int_0^\infty dy f_0(y; \Theta) \left( \frac{x}{y} \right)^2 \Rightarrow \\ \frac{\chi_0^{(2,2)}(\mathbf{x})}{n\beta^2} &= -\frac{3}{8} \frac{\Theta^2}{x^2} \int_0^\infty dy f_0(y; \Theta) \left( \frac{x}{y} \right)^2 \Rightarrow \\ \frac{\chi_0^{(2,2)}(\mathbf{x})}{n\beta^2} &= -\frac{3}{8} \Theta^2 \int_0^\infty dy f_0(y; \Theta) \frac{1}{x^2} \frac{x^2}{y^2} \Rightarrow \\ \frac{\chi_0^{(2,2)}(\mathbf{x})}{n\beta^2} &= -\frac{3}{8} \Theta^2 \int_0^\infty dy \frac{f_0(y; \Theta)}{y^2}. \end{aligned}$$

### C. The third-order (cubic) ideal density response

**The general expression.** The first and the second expression (for  $n = 2$  and  $n = 3$ ) of the general recurrence relation should now be utilized. Nevertheless, the expression of the second order perturbation of the non-interacting distribution function  $f_{\mathbf{q},\mathbf{k},\omega}^{\text{ind},(2)}$  via the unperturbed distribution function  $f_0(\mathbf{q})$  is readily available from the investigation of the quadratic ideal density response. The relevant arguments of the second order distribution function perturbation are first identified. Note also that it is convenient to set  $\omega' \rightarrow \omega''$  and  $\mathbf{k}' \rightarrow \mathbf{k}''$  for the dummy integration variables in view of the double reciprocal space-time integration as well as to use the symmetrized form  $\hbar\omega = \hbar(\omega - \omega'') + \hbar\omega''$  and  $\mathbf{k} = (\mathbf{k} - \mathbf{k}'') + \mathbf{k}''$  in view of the double convolution definition of the third order density response  $\mathcal{W}_{\mathbf{k},\omega;\mathbf{k}',\omega';\mathbf{k}'',\omega''}^{(3)}$ . We simply have

$$\begin{aligned}
f_{\mathbf{q},\mathbf{k},\omega}^{\text{ind},(2)} &= + \int \frac{d\omega'' d^3 k''}{(2\pi)^4} \frac{1}{\hbar(\omega - \omega'') + \hbar\omega'' - \epsilon_{\mathbf{q}+\frac{1}{2}\mathbf{k}''+\frac{1}{2}(\mathbf{k}-\mathbf{k}'')} + \epsilon_{\mathbf{q}-\frac{1}{2}\mathbf{k}''-\frac{1}{2}(\mathbf{k}-\mathbf{k}'')} + i0} U_{\mathbf{k}-\mathbf{k}'',\omega-\omega''}^{\text{ext}} U_{\mathbf{k}'',\omega''}^{\text{ext}} \\
&\left[ \frac{f_0[\mathbf{q} + \frac{1}{2}\mathbf{k}'' + \frac{1}{2}(\mathbf{k} - \mathbf{k}'')] - f_0[\mathbf{q} + \frac{1}{2}\mathbf{k}'' - \frac{1}{2}(\mathbf{k} - \mathbf{k}'')]}{\hbar(\omega - \omega'') - \epsilon_{\mathbf{q}+\frac{1}{2}\mathbf{k}''+\frac{1}{2}(\mathbf{k}-\mathbf{k}'')} + \epsilon_{\mathbf{q}+\frac{1}{2}\mathbf{k}''-\frac{1}{2}(\mathbf{k}-\mathbf{k}'')} + i0} - \frac{f_0[\mathbf{q} - \frac{1}{2}\mathbf{k}'' + \frac{1}{2}(\mathbf{k} - \mathbf{k}'')] - f_0[\mathbf{q} - \frac{1}{2}\mathbf{k}'' - \frac{1}{2}(\mathbf{k} - \mathbf{k}'')]}{\hbar(\omega - \omega'') - \epsilon_{\mathbf{q}-\frac{1}{2}\mathbf{k}''+\frac{1}{2}(\mathbf{k}-\mathbf{k}'')} + \epsilon_{\mathbf{q}-\frac{1}{2}\mathbf{k}''-\frac{1}{2}(\mathbf{k}-\mathbf{k}'')} + i0} \right] \Rightarrow \\
f_{\mathbf{q}+\frac{1}{2}\mathbf{k}',\mathbf{k}-\mathbf{k}',\omega-\omega'}^{\text{ind},(2)} &= + \int \frac{d\omega'' d^3 k''}{(2\pi)^4} \frac{1}{\hbar(\omega - \omega' - \omega'') + \hbar\omega'' - \epsilon_{\mathbf{q}+\frac{1}{2}\mathbf{k}'+\frac{1}{2}\mathbf{k}''+\frac{1}{2}(\mathbf{k}-\mathbf{k}'-\mathbf{k}'')} + \epsilon_{\mathbf{q}+\frac{1}{2}\mathbf{k}'+\frac{1}{2}\mathbf{k}''-\frac{1}{2}(\mathbf{k}-\mathbf{k}'-\mathbf{k}'')} + i0} \\
&\left\{ \frac{f_0[\mathbf{q} + \frac{1}{2}\mathbf{k}' + \frac{1}{2}\mathbf{k}'' + \frac{1}{2}(\mathbf{k} - \mathbf{k}' - \mathbf{k}'')] - f_0[\mathbf{q} + \frac{1}{2}\mathbf{k}' + \frac{1}{2}\mathbf{k}'' - \frac{1}{2}(\mathbf{k} - \mathbf{k}' - \mathbf{k}'')]}{\hbar(\omega - \omega' - \omega'') - \epsilon_{\mathbf{q}+\frac{1}{2}\mathbf{k}'+\frac{1}{2}\mathbf{k}''+\frac{1}{2}(\mathbf{k}-\mathbf{k}'-\mathbf{k}'')} + \epsilon_{\mathbf{q}+\frac{1}{2}\mathbf{k}'+\frac{1}{2}\mathbf{k}''-\frac{1}{2}(\mathbf{k}-\mathbf{k}'-\mathbf{k}'')} + i0} \right. \\
&\left. - \frac{f_0[\mathbf{q} + \frac{1}{2}\mathbf{k}' - \frac{1}{2}\mathbf{k}'' + \frac{1}{2}(\mathbf{k} - \mathbf{k}' - \mathbf{k}'')] - f_0[\mathbf{q} + \frac{1}{2}\mathbf{k}' - \frac{1}{2}\mathbf{k}'' - \frac{1}{2}(\mathbf{k} - \mathbf{k}' - \mathbf{k}'')]}{\hbar(\omega - \omega' - \omega'') - \epsilon_{\mathbf{q}+\frac{1}{2}\mathbf{k}'-\frac{1}{2}\mathbf{k}''+\frac{1}{2}(\mathbf{k}-\mathbf{k}'-\mathbf{k}'')} + \epsilon_{\mathbf{q}+\frac{1}{2}\mathbf{k}'-\frac{1}{2}\mathbf{k}''-\frac{1}{2}(\mathbf{k}-\mathbf{k}'-\mathbf{k}'')} + i0} \right\} U_{\mathbf{k}-\mathbf{k}'-\mathbf{k}'',\omega-\omega'-\omega''}^{\text{ext}} U_{\mathbf{k}'',\omega''}^{\text{ext}} \Rightarrow \\
f_{\mathbf{q}-\frac{1}{2}\mathbf{k}',\mathbf{k}-\mathbf{k}',\omega-\omega'}^{\text{ind},(2)} &= + \int \frac{d\omega'' d^3 k''}{(2\pi)^4} \frac{1}{\hbar(\omega - \omega' - \omega'') + \hbar\omega'' - \epsilon_{\mathbf{q}-\frac{1}{2}\mathbf{k}'+\frac{1}{2}\mathbf{k}''+\frac{1}{2}(\mathbf{k}-\mathbf{k}'-\mathbf{k}'')} + \epsilon_{\mathbf{q}-\frac{1}{2}\mathbf{k}'-\frac{1}{2}\mathbf{k}''-\frac{1}{2}(\mathbf{k}-\mathbf{k}'-\mathbf{k}'')} + i0} \\
&\left\{ \frac{f_0[\mathbf{q} - \frac{1}{2}\mathbf{k}' + \frac{1}{2}\mathbf{k}'' + \frac{1}{2}(\mathbf{k} - \mathbf{k}' - \mathbf{k}'')] - f_0[\mathbf{q} - \frac{1}{2}\mathbf{k}' + \frac{1}{2}\mathbf{k}'' - \frac{1}{2}(\mathbf{k} - \mathbf{k}' - \mathbf{k}'')]}{\hbar(\omega - \omega' - \omega'') - \epsilon_{\mathbf{q}-\frac{1}{2}\mathbf{k}'+\frac{1}{2}\mathbf{k}''+\frac{1}{2}(\mathbf{k}-\mathbf{k}'-\mathbf{k}'')} + \epsilon_{\mathbf{q}-\frac{1}{2}\mathbf{k}'+\frac{1}{2}\mathbf{k}''-\frac{1}{2}(\mathbf{k}-\mathbf{k}'-\mathbf{k}'')} + i0} \right. \\
&\left. - \frac{f_0[\mathbf{q} - \frac{1}{2}\mathbf{k}' - \frac{1}{2}\mathbf{k}'' + \frac{1}{2}(\mathbf{k} - \mathbf{k}' - \mathbf{k}'')] - f_0[\mathbf{q} - \frac{1}{2}\mathbf{k}' - \frac{1}{2}\mathbf{k}'' - \frac{1}{2}(\mathbf{k} - \mathbf{k}' - \mathbf{k}'')]}{\hbar(\omega - \omega' - \omega'') - \epsilon_{\mathbf{q}-\frac{1}{2}\mathbf{k}'-\frac{1}{2}\mathbf{k}''+\frac{1}{2}(\mathbf{k}-\mathbf{k}'-\mathbf{k}'')} + \epsilon_{\mathbf{q}-\frac{1}{2}\mathbf{k}'-\frac{1}{2}\mathbf{k}''-\frac{1}{2}(\mathbf{k}-\mathbf{k}'-\mathbf{k}'')} + i0} \right\} U_{\mathbf{k}-\mathbf{k}'-\mathbf{k}'',\omega-\omega'-\omega''}^{\text{ext}} U_{\mathbf{k}'',\omega''}^{\text{ext}}.
\end{aligned}$$

Afterwards, the above second order perturbations are substituted into the expression for the third order perturbation of the non-interacting distribution function. Prior to the substitution, it is again convenient to use equivalent form  $\hbar\omega = \hbar(\omega - \omega' - \omega'') + \hbar\omega' + \hbar\omega''$  and  $\mathbf{k} = (\mathbf{k} - \mathbf{k}' - \mathbf{k}'') + \mathbf{k}' + \mathbf{k}''$  in the denominator in order to symmetrize the integrand with respect to the arguments of the potential energy perturbations (again in view of the double convolution definition of the third order density response).

$$\begin{aligned}
f_{\mathbf{q},\mathbf{k},\omega}^{\text{ind},(3)} &= - \int \frac{d\omega' d^3 k'}{(2\pi)^4} \left[ \frac{f_{\mathbf{q}+\frac{1}{2}\mathbf{k}',\mathbf{k}-\mathbf{k}',\omega-\omega'}^{\text{ind},(2)} - f_{\mathbf{q}-\frac{1}{2}\mathbf{k}',\mathbf{k}-\mathbf{k}',\omega-\omega'}^{\text{ind},(2)}}{\hbar\omega - \epsilon_{\mathbf{q}+\frac{1}{2}\mathbf{k}} + \epsilon_{\mathbf{q}-\frac{1}{2}\mathbf{k}} + i0} \right] U_{\mathbf{k}',\omega'}^{\text{ext}} \Rightarrow \\
f_{\mathbf{q},\mathbf{k},\omega}^{\text{ind},(3)} &= - \int \frac{d\omega' d^3 k'}{(2\pi)^4} \left[ \frac{f_{\mathbf{q}+\frac{1}{2}\mathbf{k}',\mathbf{k}-\mathbf{k}',\omega-\omega'}^{\text{ind},(2)} - f_{\mathbf{q}-\frac{1}{2}\mathbf{k}',\mathbf{k}-\mathbf{k}',\omega-\omega'}^{\text{ind},(2)}}{\hbar(\omega - \omega' - \omega'') + \hbar\omega' + \hbar\omega'' - \epsilon_{\mathbf{q}+\frac{1}{2}\mathbf{k}'+\frac{1}{2}\mathbf{k}''+\frac{1}{2}(\mathbf{k}-\mathbf{k}'-\mathbf{k}'')} + \epsilon_{\mathbf{q}-\frac{1}{2}\mathbf{k}'-\frac{1}{2}\mathbf{k}''-\frac{1}{2}(\mathbf{k}-\mathbf{k}'-\mathbf{k}'')} + i0} \right] U_{\mathbf{k}',\omega'}^{\text{ext}}.
\end{aligned}$$

We are now in the position to substitute  $f_{\mathbf{q},\mathbf{k},\omega}^{\text{ind},(2)}$ , or to be more specific  $f_{\mathbf{q}+\frac{1}{2}\mathbf{k}',\mathbf{k}-\mathbf{k}',\omega-\omega'}^{\text{ind},(2)}$  and  $f_{\mathbf{q}-\frac{1}{2}\mathbf{k}',\mathbf{k}-\mathbf{k}',\omega-\omega'}^{\text{ind},(2)}$  into the expression for  $f_{\mathbf{q},\mathbf{k},\omega}^{\text{ind},(3)}$ . The calculation proceeds with the integration of the third order non-interacting distribution function perturbation over the momentum space which yields the third order density perturbation, *i.e.*

$n_{\text{ind}}^{(3)}(\mathbf{k}, \omega) = 2 \int [d^3 q / (2\pi)^3] f_{\mathbf{q}, \mathbf{k}, \omega}^{\text{ind}, (3)}$ , also in the non-interacting case.

$$\begin{aligned}
f_{\mathbf{q}, \mathbf{k}, \omega}^{\text{ind}, (3)} = & - \int \frac{d\omega' d^3 k'}{(2\pi)^4} \frac{d\omega'' d^3 k''}{(2\pi)^4} \left\{ \frac{1}{\hbar(\omega - \omega' - \omega'') + \hbar\omega' + \hbar\omega'' - \epsilon_{\mathbf{q} + \frac{1}{2}\mathbf{k}' + \frac{1}{2}\mathbf{k}'' + \frac{1}{2}(\mathbf{k} - \mathbf{k}' - \mathbf{k}'')} + \epsilon_{\mathbf{q} - \frac{1}{2}\mathbf{k}' - \frac{1}{2}\mathbf{k}'' - \frac{1}{2}(\mathbf{k} - \mathbf{k}' - \mathbf{k}'')} + i0} \right\} \\
& \left\{ \frac{1}{\hbar(\omega - \omega' - \omega'') + \hbar\omega'' - \epsilon_{\mathbf{q} + \frac{1}{2}\mathbf{k}' + \frac{1}{2}\mathbf{k}'' + \frac{1}{2}(\mathbf{k} - \mathbf{k}' - \mathbf{k}'')} + \epsilon_{\mathbf{q} + \frac{1}{2}\mathbf{k}' - \frac{1}{2}\mathbf{k}'' - \frac{1}{2}(\mathbf{k} - \mathbf{k}' - \mathbf{k}'')} + i0} \right. \\
& \left[ \frac{f_0[\mathbf{q} + \frac{1}{2}\mathbf{k}' + \frac{1}{2}\mathbf{k}'' + \frac{1}{2}(\mathbf{k} - \mathbf{k}' - \mathbf{k}'')] - f_0[\mathbf{q} + \frac{1}{2}\mathbf{k}' + \frac{1}{2}\mathbf{k}'' - \frac{1}{2}(\mathbf{k} - \mathbf{k}' - \mathbf{k}'')]}{\hbar(\omega - \omega' - \omega'') - \epsilon_{\mathbf{q} + \frac{1}{2}\mathbf{k}' + \frac{1}{2}\mathbf{k}'' + \frac{1}{2}(\mathbf{k} - \mathbf{k}' - \mathbf{k}'')} + \epsilon_{\mathbf{q} + \frac{1}{2}\mathbf{k}' + \frac{1}{2}\mathbf{k}'' - \frac{1}{2}(\mathbf{k} - \mathbf{k}' - \mathbf{k}'')} + i0} \right. \\
& \left. - \frac{f_0[\mathbf{q} + \frac{1}{2}\mathbf{k}' - \frac{1}{2}\mathbf{k}'' + \frac{1}{2}(\mathbf{k} - \mathbf{k}' - \mathbf{k}'')] - f_0[\mathbf{q} + \frac{1}{2}\mathbf{k}' - \frac{1}{2}\mathbf{k}'' - \frac{1}{2}(\mathbf{k} - \mathbf{k}' - \mathbf{k}'')]}{\hbar(\omega - \omega' - \omega'') - \epsilon_{\mathbf{q} + \frac{1}{2}\mathbf{k}' - \frac{1}{2}\mathbf{k}'' + \frac{1}{2}(\mathbf{k} - \mathbf{k}' - \mathbf{k}'')} + \epsilon_{\mathbf{q} + \frac{1}{2}\mathbf{k}' - \frac{1}{2}\mathbf{k}'' - \frac{1}{2}(\mathbf{k} - \mathbf{k}' - \mathbf{k}'')} + i0} \right] \\
& - \frac{1}{\hbar(\omega - \omega' - \omega'') + \hbar\omega'' - \epsilon_{\mathbf{q} - \frac{1}{2}\mathbf{k}' + \frac{1}{2}\mathbf{k}'' + \frac{1}{2}(\mathbf{k} - \mathbf{k}' - \mathbf{k}'')} + \epsilon_{\mathbf{q} - \frac{1}{2}\mathbf{k}' - \frac{1}{2}\mathbf{k}'' - \frac{1}{2}(\mathbf{k} - \mathbf{k}' - \mathbf{k}'')} + i0} \\
& \left[ \frac{f_0[\mathbf{q} - \frac{1}{2}\mathbf{k}' + \frac{1}{2}\mathbf{k}'' + \frac{1}{2}(\mathbf{k} - \mathbf{k}' - \mathbf{k}'')] - f_0[\mathbf{q} - \frac{1}{2}\mathbf{k}' + \frac{1}{2}\mathbf{k}'' - \frac{1}{2}(\mathbf{k} - \mathbf{k}' - \mathbf{k}'')]}{\hbar(\omega - \omega' - \omega'') - \epsilon_{\mathbf{q} - \frac{1}{2}\mathbf{k}' + \frac{1}{2}\mathbf{k}'' + \frac{1}{2}(\mathbf{k} - \mathbf{k}' - \mathbf{k}'')} + \epsilon_{\mathbf{q} - \frac{1}{2}\mathbf{k}' + \frac{1}{2}\mathbf{k}'' - \frac{1}{2}(\mathbf{k} - \mathbf{k}' - \mathbf{k}'')} + i0} \right. \\
& \left. - \frac{f_0[\mathbf{q} - \frac{1}{2}\mathbf{k}' - \frac{1}{2}\mathbf{k}'' + \frac{1}{2}(\mathbf{k} - \mathbf{k}' - \mathbf{k}'')] - f_0[\mathbf{q} - \frac{1}{2}\mathbf{k}' - \frac{1}{2}\mathbf{k}'' - \frac{1}{2}(\mathbf{k} - \mathbf{k}' - \mathbf{k}'')]}{\hbar(\omega - \omega' - \omega'') - \epsilon_{\mathbf{q} - \frac{1}{2}\mathbf{k}' - \frac{1}{2}\mathbf{k}'' + \frac{1}{2}(\mathbf{k} - \mathbf{k}' - \mathbf{k}'')} + \epsilon_{\mathbf{q} - \frac{1}{2}\mathbf{k}' - \frac{1}{2}\mathbf{k}'' - \frac{1}{2}(\mathbf{k} - \mathbf{k}' - \mathbf{k}'')} + i0} \right] \Bigg\} \\
& \times U_{\mathbf{k} - \mathbf{k}' - \mathbf{k}'', \omega - \omega' - \omega''}^{\text{ext}} U_{\mathbf{k}', \omega'}^{\text{ext}} U_{\mathbf{k}'', \omega''}^{\text{ext}} \Rightarrow \\
n_{\text{ind}}^{(3)}(\mathbf{k}, \omega) = & - \int \frac{d\omega' d^3 k'}{(2\pi)^4} \frac{d\omega'' d^3 k''}{(2\pi)^4} \frac{d^3 q}{(2\pi)^3} \left\{ \frac{2}{\hbar(\omega - \omega' - \omega'') + \hbar\omega' + \hbar\omega'' - \epsilon_{\mathbf{q} + \frac{1}{2}\mathbf{k}' + \frac{1}{2}\mathbf{k}'' + \frac{1}{2}(\mathbf{k} - \mathbf{k}' - \mathbf{k}'')} + \epsilon_{\mathbf{q} - \frac{1}{2}\mathbf{k}' - \frac{1}{2}\mathbf{k}'' - \frac{1}{2}(\mathbf{k} - \mathbf{k}' - \mathbf{k}'')} + i0} \right. \\
& \left\{ \frac{1}{\hbar(\omega - \omega' - \omega'') + \hbar\omega'' - \epsilon_{\mathbf{q} + \frac{1}{2}\mathbf{k}' + \frac{1}{2}\mathbf{k}'' + \frac{1}{2}(\mathbf{k} - \mathbf{k}' - \mathbf{k}'')} + \epsilon_{\mathbf{q} + \frac{1}{2}\mathbf{k}' - \frac{1}{2}\mathbf{k}'' - \frac{1}{2}(\mathbf{k} - \mathbf{k}' - \mathbf{k}'')} + i0} \right. \\
& \left[ \frac{f_0[\mathbf{q} + \frac{1}{2}\mathbf{k}' + \frac{1}{2}\mathbf{k}'' + \frac{1}{2}(\mathbf{k} - \mathbf{k}' - \mathbf{k}'')] - f_0[\mathbf{q} + \frac{1}{2}\mathbf{k}' + \frac{1}{2}\mathbf{k}'' - \frac{1}{2}(\mathbf{k} - \mathbf{k}' - \mathbf{k}'')]}{\hbar(\omega - \omega' - \omega'') - \epsilon_{\mathbf{q} + \frac{1}{2}\mathbf{k}' + \frac{1}{2}\mathbf{k}'' + \frac{1}{2}(\mathbf{k} - \mathbf{k}' - \mathbf{k}'')} + \epsilon_{\mathbf{q} + \frac{1}{2}\mathbf{k}' + \frac{1}{2}\mathbf{k}'' - \frac{1}{2}(\mathbf{k} - \mathbf{k}' - \mathbf{k}'')} + i0} \right. \\
& \left. - \frac{f_0[\mathbf{q} + \frac{1}{2}\mathbf{k}' - \frac{1}{2}\mathbf{k}'' + \frac{1}{2}(\mathbf{k} - \mathbf{k}' - \mathbf{k}'')] - f_0[\mathbf{q} + \frac{1}{2}\mathbf{k}' - \frac{1}{2}\mathbf{k}'' - \frac{1}{2}(\mathbf{k} - \mathbf{k}' - \mathbf{k}'')]}{\hbar(\omega - \omega' - \omega'') - \epsilon_{\mathbf{q} + \frac{1}{2}\mathbf{k}' - \frac{1}{2}\mathbf{k}'' + \frac{1}{2}(\mathbf{k} - \mathbf{k}' - \mathbf{k}'')} + \epsilon_{\mathbf{q} + \frac{1}{2}\mathbf{k}' - \frac{1}{2}\mathbf{k}'' - \frac{1}{2}(\mathbf{k} - \mathbf{k}' - \mathbf{k}'')} + i0} \right] \\
& - \frac{1}{\hbar(\omega - \omega' - \omega'') + \hbar\omega'' - \epsilon_{\mathbf{q} - \frac{1}{2}\mathbf{k}' + \frac{1}{2}\mathbf{k}'' + \frac{1}{2}(\mathbf{k} - \mathbf{k}' - \mathbf{k}'')} + \epsilon_{\mathbf{q} - \frac{1}{2}\mathbf{k}' - \frac{1}{2}\mathbf{k}'' - \frac{1}{2}(\mathbf{k} - \mathbf{k}' - \mathbf{k}'')} + i0} \\
& \left[ \frac{f_0[\mathbf{q} - \frac{1}{2}\mathbf{k}' + \frac{1}{2}\mathbf{k}'' + \frac{1}{2}(\mathbf{k} - \mathbf{k}' - \mathbf{k}'')] - f_0[\mathbf{q} - \frac{1}{2}\mathbf{k}' + \frac{1}{2}\mathbf{k}'' - \frac{1}{2}(\mathbf{k} - \mathbf{k}' - \mathbf{k}'')]}{\hbar(\omega - \omega' - \omega'') - \epsilon_{\mathbf{q} - \frac{1}{2}\mathbf{k}' + \frac{1}{2}\mathbf{k}'' + \frac{1}{2}(\mathbf{k} - \mathbf{k}' - \mathbf{k}'')} + \epsilon_{\mathbf{q} - \frac{1}{2}\mathbf{k}' + \frac{1}{2}\mathbf{k}'' - \frac{1}{2}(\mathbf{k} - \mathbf{k}' - \mathbf{k}'')} + i0} \right. \\
& \left. - \frac{f_0[\mathbf{q} - \frac{1}{2}\mathbf{k}' - \frac{1}{2}\mathbf{k}'' + \frac{1}{2}(\mathbf{k} - \mathbf{k}' - \mathbf{k}'')] - f_0[\mathbf{q} - \frac{1}{2}\mathbf{k}' - \frac{1}{2}\mathbf{k}'' - \frac{1}{2}(\mathbf{k} - \mathbf{k}' - \mathbf{k}'')]}{\hbar(\omega - \omega' - \omega'') - \epsilon_{\mathbf{q} - \frac{1}{2}\mathbf{k}' - \frac{1}{2}\mathbf{k}'' + \frac{1}{2}(\mathbf{k} - \mathbf{k}' - \mathbf{k}'')} + \epsilon_{\mathbf{q} - \frac{1}{2}\mathbf{k}' - \frac{1}{2}\mathbf{k}'' - \frac{1}{2}(\mathbf{k} - \mathbf{k}' - \mathbf{k}'')} + i0} \right] \Bigg\} \\
& \times U_{\mathbf{k} - \mathbf{k}' - \mathbf{k}'', \omega - \omega' - \omega''}^{\text{ext}} U_{\mathbf{k}', \omega'}^{\text{ext}} U_{\mathbf{k}'', \omega''}^{\text{ext}} .
\end{aligned}$$

The above expression has been rewritten in a manner that, after the term by term correspondence with the general approximation-free definition of the third order density response  $\mathcal{W}_{\mathbf{k}_1, \omega_1; \mathbf{k}_2, \omega_2; \mathbf{k}_3, \omega_3}^{(3)}$

$$n_{\text{ind}}^{(3)}(\mathbf{k}, \omega) = \int \frac{d\omega' d^3 k'}{(2\pi)^4} \frac{d\omega'' d^3 k''}{(2\pi)^4} \mathcal{W}_{\mathbf{k} - \mathbf{k}' - \mathbf{k}'', \omega - \omega' - \omega''; \mathbf{k}', \omega'; \mathbf{k}'', \omega''}^{(3)} U_{\mathbf{k} - \mathbf{k}' - \mathbf{k}'', \omega - \omega' - \omega''}^{\text{ext}} U_{\mathbf{k}', \omega'}^{\text{ext}} U_{\mathbf{k}'', \omega''}^{\text{ext}} .$$

it is possible to directly identify the third order ideal density response  $\mathcal{W}_{\mathbf{k}_1, \omega_1; \mathbf{k}_2, \omega_2; \mathbf{k}_3, \omega_3}^{(3), 0}$ . It is particularly convenient to set  $\mathbf{k}_1 = \mathbf{k} - \mathbf{k}' - \mathbf{k}''$ ,  $\mathbf{k}_2 = \mathbf{k}'$ ,  $\mathbf{k}_3 = \mathbf{k}''$ ,  $\omega_1 = \omega - \omega' - \omega''$ ,  $\omega_2 = \omega'$ ,  $\omega_3 = \omega''$ . It is also beneficial to define the analytic continuation of the third order ideal density response to the complex planes of the three frequencies by setting  $z_1 = \omega_1 + i0$ ,  $z_2 = \omega_2 + i0$ ,  $z_3 = \omega_3 + i0$ . The third order ideal density response consists of 8 integrals that involve



The calculation proceeds with the separation of the third order ideal density response to the eight independent integrals that involve triple products of the non-interacting Green's function.

$$\begin{aligned}
&= - \int \frac{d^3 q}{(2\pi)^3} \frac{2f_0 \left[ q + \frac{1}{2} \mathbf{k}_2 + \frac{1}{2} \mathbf{k}_3 + \frac{1}{2} \mathbf{k}_1 \right]}{\left( \hbar z_1 + \hbar z_2 + \hbar z_3 - \epsilon_{q + \frac{1}{2} \mathbf{k}_2 + \frac{1}{2} \mathbf{k}_3 + \frac{1}{2} \mathbf{k}_1} + \epsilon_{q - \frac{1}{2} \mathbf{k}_2 - \frac{1}{2} \mathbf{k}_3 - \frac{1}{2} \mathbf{k}_1} \right) \left( \hbar z_1 - \epsilon_{q + \frac{1}{2} \mathbf{k}_2 + \frac{1}{2} \mathbf{k}_3 + \frac{1}{2} \mathbf{k}_1} + \epsilon_{q + \frac{1}{2} \mathbf{k}_2 + \frac{1}{2} \mathbf{k}_3 - \frac{1}{2} \mathbf{k}_1} \right)} \\
&+ \int \frac{d^3 q}{(2\pi)^3} \frac{2f_0 \left[ q + \frac{1}{2} \mathbf{k}_2 + \frac{1}{2} \mathbf{k}_3 - \frac{1}{2} \mathbf{k}_1 \right]}{\left( \hbar z_1 + \hbar z_2 + \hbar z_3 - \epsilon_{q + \frac{1}{2} \mathbf{k}_2 + \frac{1}{2} \mathbf{k}_3 + \frac{1}{2} \mathbf{k}_1} + \epsilon_{q - \frac{1}{2} \mathbf{k}_2 - \frac{1}{2} \mathbf{k}_3 - \frac{1}{2} \mathbf{k}_1} \right) \left( \hbar z_1 - \epsilon_{q + \frac{1}{2} \mathbf{k}_2 + \frac{1}{2} \mathbf{k}_3 + \frac{1}{2} \mathbf{k}_1} + \epsilon_{q + \frac{1}{2} \mathbf{k}_2 + \frac{1}{2} \mathbf{k}_3 - \frac{1}{2} \mathbf{k}_1} \right)} \\
&+ \int \frac{d^3 q}{(2\pi)^3} \frac{2f_0 \left[ q + \frac{1}{2} \mathbf{k}_2 - \frac{1}{2} \mathbf{k}_3 + \frac{1}{2} \mathbf{k}_1 \right]}{\left( \hbar z_1 + \hbar z_2 + \hbar z_3 - \epsilon_{q + \frac{1}{2} \mathbf{k}_2 + \frac{1}{2} \mathbf{k}_3 + \frac{1}{2} \mathbf{k}_1} + \epsilon_{q - \frac{1}{2} \mathbf{k}_2 - \frac{1}{2} \mathbf{k}_3 - \frac{1}{2} \mathbf{k}_1} \right) \left( \hbar z_1 - \epsilon_{q + \frac{1}{2} \mathbf{k}_2 + \frac{1}{2} \mathbf{k}_3 + \frac{1}{2} \mathbf{k}_1} + \epsilon_{q + \frac{1}{2} \mathbf{k}_2 + \frac{1}{2} \mathbf{k}_3 - \frac{1}{2} \mathbf{k}_1} \right)} \\
&- \int \frac{d^3 q}{(2\pi)^3} \frac{2f_0 \left[ q + \frac{1}{2} \mathbf{k}_2 - \frac{1}{2} \mathbf{k}_3 - \frac{1}{2} \mathbf{k}_1 \right]}{\left( \hbar z_1 + \hbar z_2 + \hbar z_3 - \epsilon_{q + \frac{1}{2} \mathbf{k}_2 + \frac{1}{2} \mathbf{k}_3 + \frac{1}{2} \mathbf{k}_1} + \epsilon_{q - \frac{1}{2} \mathbf{k}_2 - \frac{1}{2} \mathbf{k}_3 - \frac{1}{2} \mathbf{k}_1} \right) \left( \hbar z_1 - \epsilon_{q + \frac{1}{2} \mathbf{k}_2 + \frac{1}{2} \mathbf{k}_3 + \frac{1}{2} \mathbf{k}_1} + \epsilon_{q + \frac{1}{2} \mathbf{k}_2 + \frac{1}{2} \mathbf{k}_3 - \frac{1}{2} \mathbf{k}_1} \right)} \\
&+ \int \frac{d^3 q}{(2\pi)^3} \frac{2f_0 \left[ q - \frac{1}{2} \mathbf{k}_2 + \frac{1}{2} \mathbf{k}_3 + \frac{1}{2} \mathbf{k}_1 \right]}{\left( \hbar z_1 + \hbar z_2 + \hbar z_3 - \epsilon_{q + \frac{1}{2} \mathbf{k}_2 + \frac{1}{2} \mathbf{k}_3 + \frac{1}{2} \mathbf{k}_1} + \epsilon_{q - \frac{1}{2} \mathbf{k}_2 - \frac{1}{2} \mathbf{k}_3 - \frac{1}{2} \mathbf{k}_1} \right) \left( \hbar z_1 - \epsilon_{q - \frac{1}{2} \mathbf{k}_2 + \frac{1}{2} \mathbf{k}_3 + \frac{1}{2} \mathbf{k}_1} + \epsilon_{q - \frac{1}{2} \mathbf{k}_2 + \frac{1}{2} \mathbf{k}_3 - \frac{1}{2} \mathbf{k}_1} \right)} \\
&- \int \frac{d^3 q}{(2\pi)^3} \frac{2f_0 \left[ q - \frac{1}{2} \mathbf{k}_2 + \frac{1}{2} \mathbf{k}_3 - \frac{1}{2} \mathbf{k}_1 \right]}{\left( \hbar z_1 + \hbar z_2 + \hbar z_3 - \epsilon_{q + \frac{1}{2} \mathbf{k}_2 + \frac{1}{2} \mathbf{k}_3 + \frac{1}{2} \mathbf{k}_1} + \epsilon_{q - \frac{1}{2} \mathbf{k}_2 - \frac{1}{2} \mathbf{k}_3 - \frac{1}{2} \mathbf{k}_1} \right) \left( \hbar z_1 - \epsilon_{q - \frac{1}{2} \mathbf{k}_2 + \frac{1}{2} \mathbf{k}_3 + \frac{1}{2} \mathbf{k}_1} + \epsilon_{q - \frac{1}{2} \mathbf{k}_2 + \frac{1}{2} \mathbf{k}_3 - \frac{1}{2} \mathbf{k}_1} \right)} \\
&- \int \frac{d^3 q}{(2\pi)^3} \frac{2f_0 \left[ q - \frac{1}{2} \mathbf{k}_2 - \frac{1}{2} \mathbf{k}_3 + \frac{1}{2} \mathbf{k}_1 \right]}{\left( \hbar z_1 + \hbar z_2 + \hbar z_3 - \epsilon_{q + \frac{1}{2} \mathbf{k}_2 + \frac{1}{2} \mathbf{k}_3 + \frac{1}{2} \mathbf{k}_1} + \epsilon_{q - \frac{1}{2} \mathbf{k}_2 - \frac{1}{2} \mathbf{k}_3 - \frac{1}{2} \mathbf{k}_1} \right) \left( \hbar z_1 - \epsilon_{q - \frac{1}{2} \mathbf{k}_2 + \frac{1}{2} \mathbf{k}_3 + \frac{1}{2} \mathbf{k}_1} + \epsilon_{q - \frac{1}{2} \mathbf{k}_2 + \frac{1}{2} \mathbf{k}_3 - \frac{1}{2} \mathbf{k}_1} \right)} \\
&+ \int \frac{d^3 q}{(2\pi)^3} \frac{2f_0 \left[ q - \frac{1}{2} \mathbf{k}_2 - \frac{1}{2} \mathbf{k}_3 - \frac{1}{2} \mathbf{k}_1 \right]}{\left( \hbar z_1 + \hbar z_2 + \hbar z_3 - \epsilon_{q + \frac{1}{2} \mathbf{k}_2 + \frac{1}{2} \mathbf{k}_3 + \frac{1}{2} \mathbf{k}_1} + \epsilon_{q - \frac{1}{2} \mathbf{k}_2 - \frac{1}{2} \mathbf{k}_3 - \frac{1}{2} \mathbf{k}_1} \right) \left( \hbar z_1 - \epsilon_{q - \frac{1}{2} \mathbf{k}_2 + \frac{1}{2} \mathbf{k}_3 + \frac{1}{2} \mathbf{k}_1} + \epsilon_{q - \frac{1}{2} \mathbf{k}_2 + \frac{1}{2} \mathbf{k}_3 - \frac{1}{2} \mathbf{k}_1} \right)}
\end{aligned}$$

The calculation continues by making the change of variables  $\mathbf{q}' = \mathbf{q} + \frac{1}{2} \mathbf{k}_1 + \frac{1}{2} \mathbf{k}_2 + \frac{1}{2} \mathbf{k}_3$ ,  $\mathbf{q}' = \mathbf{q} - \frac{1}{2} \mathbf{k}_1 - \frac{1}{2} \mathbf{k}_2 - \frac{1}{2} \mathbf{k}_3$ ,  $\mathbf{q}' = \mathbf{q} + \frac{1}{2} \mathbf{k}_1 - \frac{1}{2} \mathbf{k}_2 + \frac{1}{2} \mathbf{k}_3$ ,  $\mathbf{q}' = \mathbf{q} - \frac{1}{2} \mathbf{k}_1 + \frac{1}{2} \mathbf{k}_2 - \frac{1}{2} \mathbf{k}_3$ ,  $\mathbf{q}' = \mathbf{q} + \frac{1}{2} \mathbf{k}_1 - \frac{1}{2} \mathbf{k}_2 - \frac{1}{2} \mathbf{k}_3$ ,  $\mathbf{q}' = \mathbf{q} - \frac{1}{2} \mathbf{k}_1 + \frac{1}{2} \mathbf{k}_2 + \frac{1}{2} \mathbf{k}_3$  at each of the eight integrals respectively in order to unify the argument of the equilibrium distribution function. Finally, one reverts back to the original dummy variable by setting  $\mathbf{q}' \rightarrow \mathbf{q}$  in all the integrals.



$$\begin{aligned} \mathcal{W}_{k,z;k,z;k,z}^{(3),0} &= - \int \frac{d^3 q}{(2\pi)^3} \frac{(hz + \bar{h}z + \bar{h}z - \epsilon_q + \epsilon_{q-k-k})}{2f_0(q)} (\bar{h}z + \bar{h}z - \epsilon_q + \epsilon_{q-k-k}) (\bar{h}z - \epsilon_q) \\ &+ \int \frac{d^3 q}{(2\pi)^3} \frac{(hz + \bar{h}z + \bar{h}z - \epsilon_{q+k} + \epsilon_{q-k-k})}{2f_0(q)} (\bar{h}z + \bar{h}z - \epsilon_{q+k} + \epsilon_{q-k}) (\bar{h}z - \epsilon_{q+k} + \epsilon_q) \\ &+ \int \frac{d^3 q}{(2\pi)^3} \frac{(hz + \bar{h}z + \bar{h}z - \epsilon_{q+k} + \epsilon_{q-k-k})}{2f_0(q)} (\bar{h}z + \bar{h}z - \epsilon_{q+k} + \epsilon_{q-k}) (\bar{h}z - \epsilon_q + \epsilon_{q-k}) \\ &- \int \frac{d^3 q}{(2\pi)^3} \frac{(hz + \bar{h}z + \bar{h}z - \epsilon_{q+k+k} + \epsilon_{q-k})}{2f_0(q)} (\bar{h}z + \bar{h}z - \epsilon_{q+k+k} + \epsilon_q) (\bar{h}z - \epsilon_{q+k} + \epsilon_q) \\ &+ \int \frac{d^3 q}{(2\pi)^3} \frac{(hz + \bar{h}z + \bar{h}z - \epsilon_{q+k} + \epsilon_{q-k-k})}{2f_0(q)} (\bar{h}z + \bar{h}z - \epsilon_{q+k} + \epsilon_{q-k}) (\bar{h}z - \epsilon_q + \epsilon_{q-k}) \\ &- \int \frac{d^3 q}{(2\pi)^3} \frac{(hz + \bar{h}z + \bar{h}z - \epsilon_{q+k+k} + \epsilon_{q-k})}{2f_0(q)} (\bar{h}z + \bar{h}z - \epsilon_{q+k+k} + \epsilon_{q-k}) (\bar{h}z - \epsilon_{q+k} + \epsilon_q) \\ &- \int \frac{d^3 q}{(2\pi)^3} \frac{(hz + \bar{h}z + \bar{h}z - \epsilon_{q+k+k} + \epsilon_{q-k})}{2f_0(q)} (\bar{h}z + \bar{h}z - \epsilon_{q+k+k} + \epsilon_{q-k}) (\bar{h}z - \epsilon_q + \epsilon_{q-k}) \\ &+ \int \frac{d^3 q}{(2\pi)^3} \frac{(hz + \bar{h}z + \bar{h}z - \epsilon_{q+k+k+k} + \epsilon_q)}{2f_0(q)} (\bar{h}z + \bar{h}z - \epsilon_{q+k+k+k} + \epsilon_q) (\bar{h}z - \epsilon_{q+k} + \epsilon_q) \\ &\Rightarrow \chi_0^{(3,3)}(\mathbf{k}, z) = - \int \frac{d^3 q}{(2\pi)^3} \frac{(\bar{h}(3z) - \epsilon_q + \epsilon_{q-3k})}{2f_0(q)} (\bar{h}(2z) - \epsilon_q + \epsilon_{q-2k}) (\bar{h}z - \epsilon_q + \epsilon_{q-k}) \\ &+ \int \frac{d^3 q}{(2\pi)^3} \frac{(\bar{h}(3z) - \epsilon_{q+k} + \epsilon_{q-2k})}{2f_0(q)} (\bar{h}(2z) - \epsilon_{q+k} + \epsilon_{q-k}) (\bar{h}z - \epsilon_{q+k} + \epsilon_q) \\ &+ \int \frac{d^3 q}{(2\pi)^3} \frac{(\bar{h}(3z) - \epsilon_{q+k} + \epsilon_{q-2k})}{2f_0(q)} (\bar{h}(2z) - \epsilon_{q+k} + \epsilon_{q-k}) (\bar{h}z - \epsilon_q + \epsilon_{q-k}) \\ &- \int \frac{d^3 q}{(2\pi)^3} \frac{(\bar{h}(3z) - \epsilon_{q+2k} + \epsilon_{q-k})}{2f_0(q)} (\bar{h}(2z) - \epsilon_{q+2k} + \epsilon_q) (\bar{h}z - \epsilon_{q+k} + \epsilon_q) \\ &+ \int \frac{d^3 q}{(2\pi)^3} \frac{(\bar{h}(3z) - \epsilon_{q+k} + \epsilon_{q-2k})}{2f_0(q)} (\bar{h}(2z) - \epsilon_q + \epsilon_{q-2k}) (\bar{h}z - \epsilon_q + \epsilon_{q-k}) \\ &- \int \frac{d^3 q}{(2\pi)^3} \frac{(\bar{h}(3z) - \epsilon_{q+2k} + \epsilon_{q-k})}{2f_0(q)} (\bar{h}(2z) - \epsilon_{q+2k} + \epsilon_{q-k}) (\bar{h}z - \epsilon_{q+k} + \epsilon_q) \\ &- \int \frac{d^3 q}{(2\pi)^3} \frac{(\bar{h}(3z) - \epsilon_{q+2k} + \epsilon_{q-k})}{2f_0(q)} (\bar{h}(2z) - \epsilon_{q+2k} + \epsilon_{q-k}) (\bar{h}z - \epsilon_q + \epsilon_{q-k}) \\ &+ \int \frac{d^3 q}{(2\pi)^3} \frac{(\bar{h}(3z) - \epsilon_{q+3k} + \epsilon_q)}{2f_0(q)} (\bar{h}(2z) - \epsilon_{q+2k} + \epsilon_q) (\bar{h}z - \epsilon_{q+k} + \epsilon_q) \end{aligned}$$

**The compact form of the symmetric expression.** The calculation proceeds with the separate evaluation of each of the eight contributing integrals. For convenience, in what follows, these contributing integrals have been labelled as  $[\chi_0^{(3,3)}(\mathbf{k}, z)]_1$ ,  $[\chi_0^{(3,3)}(\mathbf{k}, z)]_2$ ,  $[\chi_0^{(3,3)}(\mathbf{k}, z)]_3$ ,  $[\chi_0^{(3,3)}(\mathbf{k}, z)]_4$ ,  $[\chi_0^{(3,3)}(\mathbf{k}, z)]_5$ ,  $[\chi_0^{(3,3)}(\mathbf{k}, z)]_6$ ,  $[\chi_0^{(3,3)}(\mathbf{k}, z)]_7$ ,  $[\chi_0^{(3,3)}(\mathbf{k}, z)]_8$ . The calculation is based on splitting the integrands into simple fractions and is facilitated by the fact that the multiplication coefficient of the decomposition always turns out to be independent of the integration variable  $q$ . For the purposes of the partial fraction decomposition, it is convenient to consider the fractions as functions of the variable  $\hbar z$ . The fractions of the integrands within the contributions  $[\chi_0^{(3,3)}(\mathbf{k}, z)]_1$ ,  $[\chi_0^{(3,3)}(\mathbf{k}, z)]_2$ ,  $[\chi_0^{(3,3)}(\mathbf{k}, z)]_7$ ,  $[\chi_0^{(3,3)}(\mathbf{k}, z)]_8$  have three simple real poles. It is straightforward to demonstrate by solving the emerging  $3 \times 3$  set of equations with respect to  $A, B, C$  that their partial fraction decomposition follows

$$\begin{aligned} \frac{1}{(x-a)(x-b)(x-c)} &= \frac{A}{x-a} + \frac{B}{x-b} + \frac{C}{x-c}, \\ A &= \frac{c-b}{bc(c-b) - ac(c-a) - ab(a-b)}, \\ B &= \frac{a-c}{bc(c-b) - ac(c-a) - ab(a-b)}, \\ C &= \frac{b-a}{bc(c-b) - ac(c-a) - ab(a-b)}. \end{aligned}$$

The fractions of the integrands within the contributions  $[\chi_0^{(3,3)}(\mathbf{k}, z)]_3$ ,  $[\chi_0^{(3,3)}(\mathbf{k}, z)]_4$ ,  $[\chi_0^{(3,3)}(\mathbf{k}, z)]_5$ ,  $[\chi_0^{(3,3)}(\mathbf{k}, z)]_6$  have a simple real pole plus a double real pole. This only becomes apparent when utilizing the algebraic identities  $(\epsilon_{\mathbf{q}+\mathbf{k}} - \epsilon_{\mathbf{q}-2\mathbf{k}})/3 = \epsilon_{\mathbf{q}} - \epsilon_{\mathbf{q}-\mathbf{k}}$  for the  $[\chi_0^{(3,3)}(\mathbf{k}, z)]_3$ ,  $[\chi_0^{(3,3)}(\mathbf{k}, z)]_5$  integrals and  $(\epsilon_{\mathbf{q}+2\mathbf{k}} - \epsilon_{\mathbf{q}-\mathbf{k}})/3 = \epsilon_{\mathbf{q}+\mathbf{k}} - \epsilon_{\mathbf{q}}$  for the  $[\chi_0^{(3,3)}(\mathbf{k}, z)]_4$ ,  $[\chi_0^{(3,3)}(\mathbf{k}, z)]_6$  integrals. It is straightforward to demonstrate by solving the emerging  $3 \times 3$  set of equations with respect to  $A, B, C$  that their partial fraction decomposition now follows

$$\begin{aligned} \frac{1}{(x-a)^2(x-b)} &= \frac{A}{x-a} + \frac{B}{(x-a)^2} + \frac{C}{x-b}, \\ A &= -\frac{1}{(a-b)^2}, \\ B &= \frac{1}{a-b}, \\ C &= \frac{1}{(a-b)^2}. \end{aligned}$$

It is worth pointing out that the utilization of the algebraic identities  $(\epsilon_{\mathbf{q}+\mathbf{k}} - \epsilon_{\mathbf{q}-2\mathbf{k}})/3 = \epsilon_{\mathbf{q}} - \epsilon_{\mathbf{q}-\mathbf{k}}$  for the third harmonic fraction of the  $[\chi_0^{(3,3)}(\mathbf{k}, z)]_2$  integral and  $(\epsilon_{\mathbf{q}+2\mathbf{k}} - \epsilon_{\mathbf{q}-\mathbf{k}})/3 = \epsilon_{\mathbf{q}+\mathbf{k}} - \epsilon_{\mathbf{q}}$  for the third harmonic fraction of the  $[\chi_0^{(3,3)}(\mathbf{k}, z)]_7$  integrals constitutes an essential step in the derivation, which reveals that they can be expressed as first harmonic fractions. Combining the eight contributing integrals, one obtains 24 terms. There are four undesired terms that cannot be expressed in terms of ideal Lindhard density responses, but fortunately they cancel out exactly. After appropriate regrouping of the remaining 20 terms, one ends up with 6 unique terms that can be expressed as an algebraic combination of three ideal Lindhard density responses, that are evaluated at different multiple wavenumber and complex frequency arguments. In particular, the ideal Lindhard density responses of interest are

$$\begin{aligned} \chi_0(\mathbf{k}, z) &= -2 \int \frac{d^3q}{(2\pi)^3} f_0(\mathbf{q}) \left[ \frac{1}{\hbar z - \epsilon_{\mathbf{q}} + \epsilon_{\mathbf{q}-\mathbf{k}}} - \frac{1}{\hbar z - \epsilon_{\mathbf{q}+\mathbf{k}} + \epsilon_{\mathbf{q}}} \right], \\ \chi_0(2\mathbf{k}, 2z) &= -2 \int \frac{d^3q}{(2\pi)^3} f_0(\mathbf{q}) \left[ \frac{1}{\hbar(2z) - \epsilon_{\mathbf{q}} + \epsilon_{\mathbf{q}-2\mathbf{k}}} - \frac{1}{\hbar(2z) - \epsilon_{\mathbf{q}+2\mathbf{k}} + \epsilon_{\mathbf{q}}} \right], \\ \chi_0(3\mathbf{k}, 3z) &= -2 \int \frac{d^3q}{(2\pi)^3} f_0(\mathbf{q}) \left[ \frac{1}{\hbar(3z) - \epsilon_{\mathbf{q}} + \epsilon_{\mathbf{q}-3\mathbf{k}}} - \frac{1}{\hbar(3z) - \epsilon_{\mathbf{q}+3\mathbf{k}} + \epsilon_{\mathbf{q}}} \right]. \end{aligned}$$

Ultimately, the so-called third order Mikhailov recursion relation emerges that expresses the symmetric third order ideal density response in terms of the first order ideal density response. It reads as

$$\chi_0^{(3,3)}(\mathbf{k}, z) = \left( \frac{m}{\hbar^2} \right)^2 \frac{1}{3k^4} [3\chi_0(3\mathbf{k}, 3z) - 8\chi_0(2\mathbf{k}, 2z) + 5\chi_0(\mathbf{k}, z)].$$



$$\begin{aligned}
& \left[ \chi_0^{(3,3)}(\mathbf{k}, z) \right]_2 = + \int \frac{d^3 q}{(2\pi)^3} \frac{2f_0(\mathbf{q})}{(h(3z) - \epsilon_{q+k} + \epsilon_{q-2k}) (h(2z) - \epsilon_{q+k} + \epsilon_{q-k}) (hz - \epsilon_{q+k} + \epsilon_q)} \Rightarrow \\
& = + \frac{1}{3} \int \frac{d^3 q}{(2\pi)^3} \frac{f_0(\mathbf{q})}{\left( hz - \frac{\epsilon_{q+k} - \epsilon_{q-2k}}{3} \right) \left( hz - \frac{\epsilon_{q+k} - \epsilon_{q-k}}{2} \right) (hz - \epsilon_{q+k} + \epsilon_q)} \Rightarrow \\
& = + \frac{1}{3} \int \frac{d^3 q}{(2\pi)^3} \frac{f_0(\mathbf{q})}{\left( \frac{(\epsilon_{q+k} - \epsilon_q) - \frac{\epsilon_{q+k} - \epsilon_{q-k}}{2}}{hz - \frac{\epsilon_{q+k} - \epsilon_{q-2k}}{3}} + \frac{\frac{\epsilon_{q+k} - \epsilon_{q-k}}{2} - (\epsilon_{q+k} - \epsilon_q)}{hz - \frac{\epsilon_{q+k} - \epsilon_{q-k}}{2}} - \frac{\frac{\epsilon_{q+k} - \epsilon_{q-2k}}{3} - (\epsilon_{q+k} - \epsilon_q - 2k)}{hz - \frac{\epsilon_{q+k} - \epsilon_{q-2k}}{3}} \right)} \Rightarrow \\
& = + \int \frac{d^3 q}{(2\pi)^3} \frac{2f_0(\mathbf{q})}{9(\epsilon_{q+k} - \epsilon_{q-k})(\epsilon_{q+k} - \epsilon_q)(2\epsilon_{q+k} + \epsilon_{q-k}) - 4(\epsilon_{q+k} - \epsilon_{q-2k})(\epsilon_{q+k} - \epsilon_q)(3\epsilon_{q+k} + \epsilon_{q-2k}) - (\epsilon_{q+k} - \epsilon_{q-2k})(\epsilon_{q+k} - \epsilon_{q-k})(2\epsilon_{q+k} - 3\epsilon_{q-k} + 3\epsilon_{q-k})} \\
& \quad \left[ \frac{6\epsilon_{q+k} - 6\epsilon_q - 3\epsilon_{q+k} + 3\epsilon_{q-k}}{hz - \frac{\epsilon_{q+k} - \epsilon_{q-2k}}{3}} + \frac{2\epsilon_{q+k} - 2\epsilon_{q-2k} - 6\epsilon_{q+k} + 6\epsilon_q}{hz - \frac{\epsilon_{q+k} - \epsilon_{q-k}}{2}} + \frac{3\epsilon_{q+k} - 3\epsilon_{q-k} - 2\epsilon_{q+k} + 2\epsilon_{q-2k}}{hz - (\epsilon_{q+k} - \epsilon_q)} \right] \Rightarrow \\
& = + \int \frac{d^3 q}{(2\pi)^3} \frac{2f_0(\mathbf{q})}{\left( \frac{6k^2 + 12\mathbf{q} \cdot \mathbf{k} - 3k^2 - 6\mathbf{q} \cdot \mathbf{k} + 3k^2}{hz - \frac{\epsilon_{q+k} - \epsilon_{q-2k}}{3}} + \frac{2k^2 + 4\mathbf{q} \cdot \mathbf{k} - 8k^2 + 8\mathbf{q} \cdot \mathbf{k} - 6k^2 - 12\mathbf{q} \cdot \mathbf{k}}{hz - \frac{\epsilon_{q+k} - \epsilon_{q-k}}{2}} + \frac{3k^2 + 6\mathbf{q} \cdot \mathbf{k} - 3k^2 - 4\mathbf{q} \cdot \mathbf{k} + 8k^2 - 8\mathbf{q} \cdot \mathbf{k}}{hz - (\epsilon_{q+k} - \epsilon_q)} \right)} \Rightarrow \\
& = + \int \frac{d^3 q}{(2\pi)^3} \frac{2f_0(\mathbf{q})}{9(4\mathbf{q} \cdot \mathbf{k})(k^2 + 2\mathbf{q} \cdot \mathbf{k})(2k^2) - 4(6\mathbf{q} \cdot \mathbf{k} - 3k^2)(2\mathbf{q} \cdot \mathbf{k} + k^2)(6k^2) - (6\mathbf{q} \cdot \mathbf{k} - 3k^2)(4\mathbf{q} \cdot \mathbf{k})(-6k^2)} \\
& \quad \left[ \frac{6k^2 + 12\mathbf{q} \cdot \mathbf{k} - 3k^2 - 6\mathbf{q} \cdot \mathbf{k} + 3k^2}{hz - \frac{\epsilon_{q+k} - \epsilon_{q-2k}}{3}} + \frac{2k^2 + 4\mathbf{q} \cdot \mathbf{k} - 8k^2 + 8\mathbf{q} \cdot \mathbf{k} - 6k^2 - 12\mathbf{q} \cdot \mathbf{k}}{hz - \frac{\epsilon_{q+k} - \epsilon_{q-k}}{2}} + \frac{3k^2 + 6\mathbf{q} \cdot \mathbf{k} - 3k^2 - 4\mathbf{q} \cdot \mathbf{k} + 8k^2 - 8\mathbf{q} \cdot \mathbf{k}}{hz - (\epsilon_{q+k} - \epsilon_q)} \right] \Rightarrow \\
& = + \int \frac{d^3 q}{(2\pi)^3} \frac{2f_0(\mathbf{q})}{72k^2(\mathbf{q} \cdot \mathbf{k})(k^2 + 2\mathbf{q} \cdot \mathbf{k}) - 72k^2(2\mathbf{q} \cdot \mathbf{k} - k^2)(2\mathbf{q} \cdot \mathbf{k} + k^2) + 72k^2(2\mathbf{q} \cdot \mathbf{k} - k^2)(\mathbf{q} \cdot \mathbf{k})} \left[ \frac{6k^2}{hz - \frac{\epsilon_{q+k} - \epsilon_{q-2k}}{3}} + \frac{-12k^2}{hz - \frac{\epsilon_{q+k} - \epsilon_{q-k}}{2}} + \frac{6k^2}{hz - (\epsilon_{q+k} - \epsilon_q)} \right] \Rightarrow \\
& = + \int \frac{d^3 q}{(2\pi)^3} \frac{2f_0(\mathbf{q})}{72k^2[(\mathbf{q} \cdot \mathbf{k})(2\mathbf{q} \cdot \mathbf{k} + k^2) + (\mathbf{q} \cdot \mathbf{k})(2\mathbf{q} \cdot \mathbf{k} - k^2) - (2\mathbf{q} \cdot \mathbf{k} - k^2)(2\mathbf{q} \cdot \mathbf{k} + k^2)]} \left[ \frac{6k^2}{hz - \frac{\epsilon_{q+k} - \epsilon_{q-2k}}{3}} + \frac{-12k^2}{hz - \frac{\epsilon_{q+k} - \epsilon_{q-k}}{2}} + \frac{6k^2}{hz - (\epsilon_{q+k} - \epsilon_q)} \right] \Rightarrow \\
& = + \int \frac{d^3 q}{(2\pi)^3} \frac{2f_0(\mathbf{q})}{72k^2[(\mathbf{q} \cdot \mathbf{k})(4\mathbf{q} \cdot \mathbf{k}) - (2\mathbf{q} \cdot \mathbf{k} - k^2)(2\mathbf{q} \cdot \mathbf{k} + k^2)]} \left[ \frac{6k^2}{hz - \frac{\epsilon_{q+k} - \epsilon_{q-2k}}{3}} + \frac{-12k^2}{hz - \frac{\epsilon_{q+k} - \epsilon_{q-k}}{2}} + \frac{6k^2}{hz - (\epsilon_{q+k} - \epsilon_q)} \right] \Rightarrow \\
& = + \int \frac{d^3 q}{(2\pi)^3} \frac{2f_0(\mathbf{q})}{72k^2[4(\mathbf{q} \cdot \mathbf{k})^2 - 4(\mathbf{q} \cdot \mathbf{k})^2 + k^4]} \left[ \frac{6k^2}{hz - \frac{\epsilon_{q+k} - \epsilon_{q-2k}}{3}} + \frac{-12k^2}{hz - \frac{\epsilon_{q+k} - \epsilon_{q-k}}{2}} + \frac{6k^2}{hz - (\epsilon_{q+k} - \epsilon_q)} \right] \Rightarrow \\
& = + \int \frac{d^3 q}{(2\pi)^3} \frac{2f_0(\mathbf{q})}{72k^6} \left[ \frac{6k^2}{hz - \frac{\epsilon_{q+k} - \epsilon_{q-2k}}{3}} + \frac{-12k^2}{hz - \frac{\epsilon_{q+k} - \epsilon_{q-k}}{2}} + \frac{6k^2}{hz - (\epsilon_{q+k} - \epsilon_q)} \right] \Rightarrow \\
& = + \int \frac{d^3 q}{(2\pi)^3} \frac{2f_0(\mathbf{q})}{6k^4} \left[ \frac{1}{hz - \frac{\epsilon_{q+k} - \epsilon_{q-2k}}{3}} - \frac{2}{hz - \frac{\epsilon_{q+k} - \epsilon_{q-k}}{2}} + \frac{1}{hz - (\epsilon_{q+k} - \epsilon_q)} \right] \Rightarrow \\
& = + \int \frac{d^3 q}{(2\pi)^3} \frac{2f_0(\mathbf{q})}{6k^4} \left[ \frac{1}{hz - \epsilon_q + \epsilon_{q-k}} - \frac{2}{hz - \frac{\epsilon_{q+k} - \epsilon_{q-k}}{2}} + \frac{1}{hz - (\epsilon_{q+k} - \epsilon_q)} \right] \Rightarrow \\
& = + \int \frac{d^3 q}{(2\pi)^3} \frac{2f_0(\mathbf{q})}{6k^4} \left[ \frac{1}{hz - \epsilon_q + \epsilon_{q-k}} - \frac{2}{hz - \frac{\epsilon_{q+k} - \epsilon_{q-k}}{2}} + \frac{1}{hz - (\epsilon_{q+k} - \epsilon_q)} \right] \Rightarrow \\
& = + \left( \frac{m}{\hbar^2} \right)^2 \frac{1}{3k^4} \int \frac{d^3 q}{(2\pi)^3} 2f_0(\mathbf{q}) \left[ \frac{1}{hz - \epsilon_q + \epsilon_{q-k}} - \frac{2}{\hbar(2z) - \epsilon_{q+k} + \epsilon_{q-k}} + \frac{1}{hz - \epsilon_{q+k} + \epsilon_q} \right].
\end{aligned}$$



$$\begin{aligned}
\left[ \chi_0^{(3,3)}(\mathbf{k}, z) \right]_4 &= - \int \frac{d^3 q}{(2\pi)^3} \frac{\bar{h}(3z)}{(\bar{h}(3z) - \epsilon_q + 2\mathbf{k} + \epsilon_q - \mathbf{k})} \frac{2f_0(\mathbf{q})}{(\bar{h}(2z) - \epsilon_q + 2\mathbf{k} + \epsilon_q)(\bar{h}z - \epsilon_q + \mathbf{k} + \epsilon_q)} \Rightarrow \\
&= -\frac{1}{3} \int \frac{d^3 q}{(2\pi)^3} \frac{f_0(\mathbf{q})}{\left(\bar{h}z - \frac{\epsilon_q + 2\mathbf{k} - \epsilon_q - \mathbf{k}}{3}\right) \left(\bar{h}z - \frac{\epsilon_q + 2\mathbf{k} - \epsilon_q}{2}\right) (\bar{h}z - \epsilon_q + \mathbf{k} + \epsilon_q)} \Rightarrow \\
&= -\frac{1}{3} \int \frac{d^3 q}{(2\pi)^3} \frac{f_0(\mathbf{q})}{[\bar{h}z - (\epsilon_q + \mathbf{k} - \epsilon_q)] \left(\bar{h}z - \frac{\epsilon_q + 2\mathbf{k} - \epsilon_q}{2}\right) [\bar{h}z - (\epsilon_q + \mathbf{k} - \epsilon_q)]} \Rightarrow \\
&= -\frac{1}{3} \int \frac{d^3 q}{(2\pi)^3} \frac{f_0(\mathbf{q})}{[\bar{h}z - (\epsilon_q + \mathbf{k} - \epsilon_q)] \left(\bar{h}z - \frac{\epsilon_q + 2\mathbf{k} - \epsilon_q}{2}\right) [\bar{h}z - (\epsilon_q + \mathbf{k} - \epsilon_q)]} \Rightarrow \\
&= -\frac{1}{3} \int \frac{d^3 q}{(2\pi)^3} \frac{f_0(\mathbf{q})}{[\bar{h}z - (\epsilon_q + \mathbf{k} - \epsilon_q)]^2 \left(\bar{h}z - \frac{\epsilon_q + 2\mathbf{k} - \epsilon_q}{2}\right)} \Rightarrow \\
&= -\frac{1}{3} \int \frac{d^3 q}{(2\pi)^3} \frac{f_0(\mathbf{q})}{\left[(\epsilon_q + \mathbf{k} - \epsilon_q) - \frac{\epsilon_q + 2\mathbf{k} - \epsilon_q}{2}\right]^2} \left\{ -\frac{1}{[\bar{h}z - (\epsilon_q + \mathbf{k} - \epsilon_q)]} + \frac{(\epsilon_q + \mathbf{k} - \epsilon_q) - \frac{\epsilon_q + 2\mathbf{k} - \epsilon_q}{2}}{[\bar{h}z - (\epsilon_q + \mathbf{k} - \epsilon_q)]^2} + \frac{1}{\left(\bar{h}z - \frac{\epsilon_q + 2\mathbf{k} - \epsilon_q}{2}\right)} \right\} \Rightarrow \\
&= -\frac{1}{3} \int \frac{d^3 q}{(2\pi)^3} \frac{f_0(\mathbf{q})}{\left[(\mathbf{q} + \mathbf{k})^2 - q^2 - \frac{(\mathbf{q} + 2\mathbf{k})^2 - q^2}{2}\right]^2} \left\{ -\frac{1}{[\bar{h}z - (\epsilon_q + \mathbf{k} - \epsilon_q)]} + \frac{1}{2m} \frac{\bar{h}^2 (\mathbf{q} + \mathbf{k})^2 - q^2 - \frac{(\mathbf{q} + 2\mathbf{k})^2 - q^2}{2}}{[\bar{h}z - (\epsilon_q + \mathbf{k} - \epsilon_q)]^2} + \frac{1}{\left(\bar{h}z - \frac{\epsilon_q + 2\mathbf{k} - \epsilon_q}{2}\right)} \right\} \Rightarrow \\
&= -\frac{1}{3} \int \frac{d^3 q}{(2\pi)^3} \frac{f_0(\mathbf{q})}{\left[k^2 + 2\mathbf{q} \cdot \mathbf{k} - \frac{4k^2 + 4\mathbf{q} \cdot \mathbf{k}}{2}\right]^2} \left\{ -\frac{1}{[\bar{h}z - (\epsilon_q + \mathbf{k} - \epsilon_q)]} + \frac{\bar{h}^2 k^2 + 2\mathbf{q} \cdot \mathbf{k} - \frac{4k^2 + 4\mathbf{q} \cdot \mathbf{k}}{2}}{[\bar{h}z - (\epsilon_q + \mathbf{k} - \epsilon_q)]^2} + \frac{1}{\left(\bar{h}z - \frac{\epsilon_q + 2\mathbf{k} - \epsilon_q}{2}\right)} \right\} \Rightarrow \\
&= -\frac{1}{3} \int \frac{d^3 q}{(2\pi)^3} \frac{f_0(\mathbf{q})}{\left[k^2 + 2\mathbf{q} \cdot \mathbf{k} - 2k^2 - 2\mathbf{q} \cdot \mathbf{k}\right]^2} \left\{ -\frac{1}{[\bar{h}z - (\epsilon_q + \mathbf{k} - \epsilon_q)]} + \frac{\bar{h}^2 k^2 + 2\mathbf{q} \cdot \mathbf{k} - 2k^2 - 2\mathbf{q} \cdot \mathbf{k}}{[\bar{h}z - (\epsilon_q + \mathbf{k} - \epsilon_q)]^2} + \frac{1}{\left(\bar{h}z - \frac{\epsilon_q + 2\mathbf{k} - \epsilon_q}{2}\right)} \right\} \Rightarrow \\
&= -\frac{1}{3} \int \frac{d^3 q}{(2\pi)^3} \frac{f_0(\mathbf{q})}{[-k^2]^2} \left\{ -\frac{1}{[\bar{h}z - (\epsilon_q + \mathbf{k} - \epsilon_q)]} + \frac{\bar{h}^2 k^2}{2m} \frac{1}{[\bar{h}z - (\epsilon_q + \mathbf{k} - \epsilon_q)]^2} + \frac{1}{\left(\bar{h}z - \frac{\epsilon_q + 2\mathbf{k} - \epsilon_q}{2}\right)} \right\} \Rightarrow \\
&= - \int \frac{d^3 q}{(2\pi)^3} \frac{f_0(\mathbf{q})}{3k^4} \left\{ -\frac{1}{[\bar{h}z - (\epsilon_q + \mathbf{k} - \epsilon_q)]} - \frac{\bar{h}^2 k^2}{2m} \frac{1}{[\bar{h}z - (\epsilon_q + \mathbf{k} - \epsilon_q)]^2} + \frac{1}{\left(\bar{h}z - \frac{\epsilon_q + 2\mathbf{k} - \epsilon_q}{2}\right)} \right\} \Rightarrow \\
&= - \int \frac{d^3 q}{(2\pi)^3} \frac{f_0(\mathbf{q})}{3k^4} \left\{ \frac{1}{\left(\bar{h}z - \frac{\epsilon_q + 2\mathbf{k} - \epsilon_q}{2}\right)} - \frac{\bar{h}^2 k^2}{2m} \frac{1}{[\bar{h}z - (\epsilon_q + \mathbf{k} - \epsilon_q)]^2} - \frac{1}{[\bar{h}z - (\epsilon_q + \mathbf{k} - \epsilon_q)]} \right\} \Rightarrow \\
&= - \int \frac{d^3 q}{(2\pi)^3} \frac{f_0(\mathbf{q})}{3k^4} \left[ \frac{2}{\bar{h}(2z) - \epsilon_q + 2\mathbf{k} + \epsilon_q} - \frac{\bar{h}^2 k^2}{2m} \frac{1}{(\bar{h}z - \epsilon_q + \mathbf{k} + \epsilon_q)^2} - \frac{1}{\bar{h}z - \epsilon_q + \mathbf{k} + \epsilon_q} \right] \Rightarrow \\
&= - \int \frac{d^3 q}{(2\pi)^3} \frac{f_0(\mathbf{q})}{6k^4} \left[ \frac{4}{\bar{h}(2z) - \epsilon_q + 2\mathbf{k} + \epsilon_q} - \frac{\bar{h}^2 k^2}{2m} \frac{2}{(\bar{h}z - \epsilon_q + \mathbf{k} + \epsilon_q)^2} - \frac{2}{\bar{h}z - \epsilon_q + \mathbf{k} + \epsilon_q} \right] \Rightarrow \\
&= - \left(\frac{m}{\bar{h}^2}\right)^2 \frac{1}{3k^4} \int \frac{d^3 q}{(2\pi)^3} {}_2f_0(\mathbf{q}) \left[ \frac{4}{\bar{h}(2z) - \epsilon_q + 2\mathbf{k} + \epsilon_q} - \frac{\bar{h}^2 k^2}{2m} \frac{2}{(\bar{h}z - \epsilon_q + \mathbf{k} + \epsilon_q)^2} - \frac{2}{\bar{h}z - \epsilon_q + \mathbf{k} + \epsilon_q} \right].
\end{aligned}$$

$$\begin{aligned}
& \left[ \chi_0^{(3,3)}(\mathbf{k}, z) \right]_5 = + \int \frac{d^3 q}{(2\pi)^3} \frac{2f_0(\mathbf{q})}{(h(3z) - \epsilon_{q+\mathbf{k}} + \epsilon_{q-2\mathbf{k}})(h(2z) - \epsilon_q + \epsilon_{q-2\mathbf{k}})(hz - \epsilon_q + \epsilon_{q-\mathbf{k}})} \Rightarrow \\
& = + \frac{1}{3} \int \frac{d^3 q}{(2\pi)^3} \frac{f_0(\mathbf{q})}{\left(hz - \frac{\epsilon_{q+\mathbf{k}} - \epsilon_{q-2\mathbf{k}}}{3}\right) \left(hz - \frac{\epsilon_q - \epsilon_{q-2\mathbf{k}}}{2}\right) (hz - \epsilon_q + \epsilon_{q-\mathbf{k}})} \Rightarrow \\
& = + \frac{1}{3} \int \frac{d^3 q}{(2\pi)^3} \frac{f_0(\mathbf{q})}{[hz - (\epsilon_q - \epsilon_{q-\mathbf{k}})] \left(hz - \frac{\epsilon_q - \epsilon_{q-2\mathbf{k}}}{2}\right) [hz - (\epsilon_q - \epsilon_{q-\mathbf{k}})]} \Rightarrow \\
& = + \frac{1}{3} \int \frac{d^3 q}{(2\pi)^3} \frac{f_0(\mathbf{q})}{[hz - (\epsilon_q - \epsilon_{q-\mathbf{k}})]^2 \left(hz - \frac{\epsilon_q - \epsilon_{q-2\mathbf{k}}}{2}\right)} \Rightarrow \\
& = + \frac{1}{3} \int \frac{d^3 q}{(2\pi)^3} \frac{f_0(\mathbf{q})}{(\epsilon_q - \epsilon_{q-\mathbf{k}}) \left[ -\frac{1}{[hz - (\epsilon_q - \epsilon_{q-\mathbf{k}})]} + \frac{(\epsilon_q - \epsilon_{q-\mathbf{k}}) - \frac{\epsilon_q - \epsilon_{q-2\mathbf{k}}}{2}}{[hz - (\epsilon_q - \epsilon_{q-\mathbf{k}})]^2} + \frac{1}{\left(hz - \frac{\epsilon_q - \epsilon_{q-2\mathbf{k}}}{2}\right)} \right]} \Rightarrow \\
& = + \frac{1}{3} \int \frac{d^3 q}{(2\pi)^3} \frac{\left(\frac{2m}{h^2}\right)^2}{[q^2 - (\mathbf{q} - \mathbf{k})^2 - \frac{q^2 - (\mathbf{q} - 2\mathbf{k})^2}{2}]^2} \frac{f_0(\mathbf{q})}{\left\{ -\frac{1}{[hz - (\epsilon_q - \epsilon_{q-\mathbf{k}})]} + \frac{h^2}{2m} \frac{q^2 - (\mathbf{q} - \mathbf{k})^2}{[hz - (\epsilon_q - \epsilon_{q-\mathbf{k}})]^2} + \frac{1}{\left(hz - \frac{\epsilon_q - \epsilon_{q-2\mathbf{k}}}{2}\right)} \right\}} \Rightarrow \\
& = + \frac{1}{3} \int \frac{d^3 q}{(2\pi)^3} \frac{\left(\frac{2m}{h^2}\right)^2}{[-k^2 + 2\mathbf{q} \cdot \mathbf{k} + \frac{4k^2 - 4\mathbf{q} \cdot \mathbf{k}}{2}]^2} \frac{f_0(\mathbf{q})}{\left\{ -\frac{1}{[hz - (\epsilon_q - \epsilon_{q-\mathbf{k}})]} + \frac{h^2}{2m} \frac{h^2 - k^2 + 2\mathbf{q} \cdot \mathbf{k} + \frac{4k^2 - 4\mathbf{q} \cdot \mathbf{k}}{2}}{[hz - (\epsilon_q - \epsilon_{q-\mathbf{k}})]^2} + \frac{1}{\left(hz - \frac{\epsilon_q - \epsilon_{q-2\mathbf{k}}}{2}\right)} \right\}} \Rightarrow \\
& = + \frac{1}{3} \int \frac{d^3 q}{(2\pi)^3} \frac{\left(\frac{2m}{h^2}\right)^2}{[-k^2 + 2\mathbf{q} \cdot \mathbf{k} + 2k^2 - 2\mathbf{q} \cdot \mathbf{k}]^2} \frac{f_0(\mathbf{q})}{\left\{ -\frac{1}{[hz - (\epsilon_q - \epsilon_{q-\mathbf{k}})]} + \frac{h^2}{2m} \frac{-k^2 + 2\mathbf{q} \cdot \mathbf{k} + 2k^2 - 2\mathbf{q} \cdot \mathbf{k}}{[hz - (\epsilon_q - \epsilon_{q-\mathbf{k}})]^2} + \frac{1}{\left(hz - \frac{\epsilon_q - \epsilon_{q-2\mathbf{k}}}{2}\right)} \right\}} \Rightarrow \\
& = + \frac{1}{3} \int \frac{d^3 q}{(2\pi)^3} \frac{\left(\frac{2m}{h^2}\right)^2}{[k^2]^2} \frac{f_0(\mathbf{q})}{\left\{ -\frac{1}{[hz - (\epsilon_q - \epsilon_{q-\mathbf{k}})]} + \frac{h^2}{2m} \frac{k^2}{[hz - (\epsilon_q - \epsilon_{q-\mathbf{k}})]^2} + \frac{1}{\left(hz - \frac{\epsilon_q - \epsilon_{q-2\mathbf{k}}}{2}\right)} \right\}} \Rightarrow \\
& = + \frac{1}{3} \int \frac{d^3 q}{(2\pi)^3} \frac{\left(\frac{2m}{h^2}\right)^2}{k^4} \frac{f_0(\mathbf{q})}{\left\{ -\frac{1}{[hz - (\epsilon_q - \epsilon_{q-\mathbf{k}})]} + \frac{h^2 k^2}{2m} \frac{1}{[hz - (\epsilon_q - \epsilon_{q-\mathbf{k}})]^2} + \frac{1}{\left(hz - \frac{\epsilon_q - \epsilon_{q-2\mathbf{k}}}{2}\right)} \right\}} \Rightarrow \\
& = + \int \frac{d^3 q}{(2\pi)^3} \frac{\left(\frac{2m}{h^2}\right)^2}{3k^4} \frac{f_0(\mathbf{q})}{\left\{ -\frac{1}{[hz - (\epsilon_q - \epsilon_{q-\mathbf{k}})]} + \frac{h^2 k^2}{2m} \frac{1}{[hz - (\epsilon_q - \epsilon_{q-\mathbf{k}})]^2} + \frac{1}{\left(hz - \frac{\epsilon_q - \epsilon_{q-2\mathbf{k}}}{2}\right)} \right\}} \Rightarrow \\
& = + \int \frac{d^3 q}{(2\pi)^3} \frac{\left(\frac{2m}{h^2}\right)^2}{3k^4} \frac{f_0(\mathbf{q})}{\left[ \frac{1}{hz - \frac{\epsilon_q - \epsilon_{q-2\mathbf{k}}}{2}} + \frac{h^2 k^2}{2m} \frac{1}{(hz - \epsilon_q + \epsilon_{q-\mathbf{k}})^2} - \frac{1}{hz - \epsilon_q + \epsilon_{q-\mathbf{k}}} \right]} \Rightarrow \\
& = + \int \frac{d^3 q}{(2\pi)^3} \frac{\left(\frac{2m}{h^2}\right)^2}{3k^4} \frac{f_0(\mathbf{q})}{\left[ \frac{2}{h(2z) - \epsilon_q + \epsilon_{q-2\mathbf{k}}} + \frac{h^2 k^2}{2m} \frac{1}{(hz - \epsilon_q + \epsilon_{q-\mathbf{k}})^2} - \frac{1}{hz - \epsilon_q + \epsilon_{q-\mathbf{k}}} \right]} \Rightarrow \\
& = + \int \frac{d^3 q}{(2\pi)^3} \frac{\left(\frac{2m}{h^2}\right)^2}{6k^4} \frac{f_0(\mathbf{q})}{\left[ \frac{4}{h(2z) - \epsilon_q + \epsilon_{q-2\mathbf{k}}} + \frac{h^2 k^2}{2m} \frac{2}{(hz - \epsilon_q + \epsilon_{q-\mathbf{k}})^2} - \frac{2}{hz - \epsilon_q + \epsilon_{q-\mathbf{k}}} \right]} \Rightarrow \\
& = + \left(\frac{m}{h^2}\right)^2 \frac{1}{3k^4} \int \frac{d^3 q}{(2\pi)^3} 2f_0(\mathbf{q}) \left[ \frac{4}{h(2z) - \epsilon_q + \epsilon_{q-2\mathbf{k}}} + \frac{h^2 k^2}{2m} \frac{2}{(hz - \epsilon_q + \epsilon_{q-\mathbf{k}})^2} - \frac{2}{hz - \epsilon_q + \epsilon_{q-\mathbf{k}}} \right].
\end{aligned}$$





$$\begin{aligned}
& \left[ \chi_0^{(3,3)}(k, z) \right]_7 = - \int \frac{d^3 q}{(2\pi)^3} \frac{2f_0(q)}{(h(3z) - \epsilon_{q+2k} + \epsilon_{q-k})(h(2z) - \epsilon_{q+k} + \epsilon_{q-k})(h z - \epsilon_q + \epsilon_{q-k})} \Rightarrow \\
& = - \frac{1}{3} \int \frac{d^3 q}{(2\pi)^3} \frac{f_0(q)}{\left( h z - \frac{\epsilon_{q+2k} - \epsilon_{q-k}}{3} \right) \left( h z - \frac{\epsilon_{q+k} - \epsilon_{q-k}}{2} \right) (h z - (\epsilon_q - \epsilon_{q-k}))} \Rightarrow \\
& = - \frac{1}{3} \int \frac{d^3 q}{(2\pi)^3} \frac{f_0(q)}{\left( \frac{\epsilon_q - \epsilon_{q-k}}{h z - \frac{\epsilon_{q+2k} - \epsilon_{q-k}}{3}} + \frac{\epsilon_{q+2k} - \epsilon_{q-k}}{h z - \frac{\epsilon_{q+k} - \epsilon_{q-k}}{2}} + \frac{\epsilon_{q+2k} - \epsilon_{q-k}}{h z - (\epsilon_q - \epsilon_{q-k})} \right)} \Rightarrow \\
& = - \int \frac{d^3 q}{(2\pi)^3} \frac{2f_0(q)}{9(\epsilon_q + k - \epsilon_{q-k})(\epsilon_q - \epsilon_{q-k})(2\epsilon_q - 2\epsilon_{q-k} - \epsilon_{q+k} + \epsilon_{q-k}) - 4(\epsilon_q + 2k - \epsilon_{q-k})(\epsilon_q - \epsilon_{q-k})(3\epsilon_q - 3\epsilon_{q-k} - \epsilon_{q+2k} + \epsilon_{q-k}) - (\epsilon_q + k - \epsilon_{q-k})(2\epsilon_q + 2k - 2\epsilon_{q-k} - 3\epsilon_{q-k} + 3\epsilon_{q-k})} \\
& \quad \left[ \frac{6\epsilon_q - 6\epsilon_{q-k} - 3\epsilon_{q+k} + 3\epsilon_{q-k}}{h z - \frac{\epsilon_{q+2k} - \epsilon_{q-k}}{3}} + \frac{2\epsilon_q + 2k - 2\epsilon_{q-k} - 6\epsilon_q + 6\epsilon_{q-k}}{h z - \frac{\epsilon_{q+k} - \epsilon_{q-k}}{2}} + \frac{3\epsilon_q + k - 3\epsilon_{q-k} - 2\epsilon_{q+2k} + 2\epsilon_{q-k}}{h z - (\epsilon_q - \epsilon_{q-k})} \right] \Rightarrow \\
& = - \int \frac{d^3 q}{(2\pi)^3} \frac{2f_0(q)}{9(4q \cdot k)(2q \cdot k - k^2)(-2k^2 + 4q \cdot k - 4q \cdot k) - 4(4q \cdot k + 3k^2 + 2q \cdot k)(2q \cdot k - k^2)(-6k^2 + 6q \cdot k - 4q \cdot k) - (3k^2 + 6q \cdot k)(4q \cdot k)(6k^2 + 8q \cdot k - 6q \cdot k - 6q \cdot k)} \\
& \quad \left[ \frac{-6k^2 + 12q \cdot k - 3k^2 - 6q \cdot k + 3k^2 - 6q \cdot k}{h z - \frac{\epsilon_{q+2k} - \epsilon_{q-k}}{3}} + \frac{8k^2 + 8q \cdot k - 2k^2 + 4q \cdot k + 6k^2 - 12q \cdot k}{h z - \frac{\epsilon_{q+k} - \epsilon_{q-k}}{2}} + \frac{6q \cdot k + 6q \cdot k - 8k^2 - 8q \cdot k + 2k^2 - 4q \cdot k}{h z - (\epsilon_q - \epsilon_{q-k})} \right] \Rightarrow \\
& = - \int \frac{d^3 q}{(2\pi)^3} \frac{2f_0(q)}{-72k^2(q \cdot k)(2q \cdot k - k^2) + 72k^2(2q \cdot k + k^2)(2q \cdot k - k^2) - 72k^2(q \cdot k)(2q \cdot k + k^2) \left[ \frac{-6k^2}{h z - \frac{\epsilon_{q+2k} - \epsilon_{q-k}}{3}} + \frac{12k^2}{h z - \frac{\epsilon_{q+k} - \epsilon_{q-k}}{2}} + \frac{-6k^2}{h z - (\epsilon_q - \epsilon_{q-k})} \right]} \Rightarrow \\
& = - \int \frac{d^3 q}{(2\pi)^3} \frac{2f_0(q)}{-72k^2(q \cdot k)(4q \cdot k) + 72k^2(2q \cdot k + k^2)(2q \cdot k - k^2) \left[ \frac{-6k^2}{h z - \frac{\epsilon_{q+2k} - \epsilon_{q-k}}{3}} + \frac{12k^2}{h z - \frac{\epsilon_{q+k} - \epsilon_{q-k}}{2}} + \frac{-6k^2}{h z - (\epsilon_q - \epsilon_{q-k})} \right]} \Rightarrow \\
& = - \int \frac{d^3 q}{(2\pi)^3} \frac{2f_0(q)}{-72k^2[4(q \cdot k)^2 - 4(q \cdot k)^2 + k^4] \left[ \frac{-6k^2}{h z - \frac{\epsilon_{q+2k} - \epsilon_{q-k}}{3}} + \frac{12k^2}{h z - \frac{\epsilon_{q+k} - \epsilon_{q-k}}{2}} + \frac{-6k^2}{h z - (\epsilon_q - \epsilon_{q-k})} \right]} \Rightarrow \\
& = - \int \frac{d^3 q}{(2\pi)^3} \frac{2f_0(q)}{-72k^6 \left[ \frac{1}{h z - \frac{\epsilon_{q+2k} - \epsilon_{q-k}}{3}} - \frac{2}{h z - \frac{\epsilon_{q+k} - \epsilon_{q-k}}{2}} + \frac{1}{h z - (\epsilon_q - \epsilon_{q-k})} \right]} \Rightarrow \\
& = - \int \frac{d^3 q}{(2\pi)^3} \frac{2f_0(q)}{6k^4 \left[ \frac{1}{h z - \frac{\epsilon_{q+2k} - \epsilon_{q-k}}{3}} - \frac{2}{h z - \frac{\epsilon_{q+k} - \epsilon_{q-k}}{2}} + \frac{1}{h z - (\epsilon_q - \epsilon_{q-k})} \right]} \Rightarrow \\
& = - \int \frac{d^3 q}{(2\pi)^3} \frac{2f_0(q)}{6k^4 \left[ \frac{1}{h z - \epsilon_{q+k} + \epsilon_q} - \frac{2}{h z - \frac{\epsilon_{q+k} - \epsilon_{q-k}}{2}} + \frac{1}{h z - (\epsilon_q - \epsilon_{q-k})} \right]} \Rightarrow \\
& = - \int \frac{d^3 q}{(2\pi)^3} \frac{2f_0(q)}{6k^4 \left[ \frac{1}{h z - \epsilon_{q+k} + \epsilon_q} - \frac{2}{h z - \frac{\epsilon_{q+k} - \epsilon_{q-k}}{2}} + \frac{1}{h z - (\epsilon_q - \epsilon_{q-k})} \right]} \Rightarrow \\
& = - \left( \frac{m}{\hbar^2} \right)^2 \frac{1}{3k^4} \int \frac{d^3 q}{(2\pi)^3} \frac{2f_0(q)}{3} \left[ \frac{1}{h z - \epsilon_{q+k} + \epsilon_q} - \frac{2}{h(2z) - \epsilon_{q+k} + \epsilon_{q-k}} + \frac{1}{h z - \epsilon_q + \epsilon_{q-k}} \right].
\end{aligned}$$

$$\begin{aligned}
& \left[ \chi_0^{(3,3)}(\mathbf{k}, z) \right]_8 = + \int \frac{d^3 q}{(2\pi)^3} \frac{2f_0(\mathbf{q})}{(h(3z) - \epsilon_q + 3k + \epsilon_q)(h(2z) - \epsilon_q + 2k + \epsilon_q)(h z - \epsilon_q + k + \epsilon_q)} \Rightarrow \\
& = + \frac{1}{3} \int \frac{d^3 q}{(2\pi)^3} \frac{f_0(\mathbf{q})}{\left( h z - \frac{\epsilon_q + 3k - \epsilon_q}{3} \right) \left( h z - \frac{\epsilon_q + 2k - \epsilon_q}{2} \right) (h z - (\epsilon_q + k - \epsilon_q))} \Rightarrow \\
& = + \frac{1}{3} \int \frac{d^3 q}{(2\pi)^3} \frac{f_0(\mathbf{q})}{\frac{\epsilon_q + 2k - \epsilon_q}{2} (\epsilon_q + k - \epsilon_q) \left( (\epsilon_q + k - \epsilon_q) - \frac{\epsilon_q + 3k - \epsilon_q}{3} \right) - \frac{\epsilon_q + 3k - \epsilon_q}{3} \left( \frac{\epsilon_q + 2k - \epsilon_q}{2} - \frac{\epsilon_q + 3k - \epsilon_q}{3} \right)} \\
& \left[ \frac{(\epsilon_q + k - \epsilon_q) - \frac{\epsilon_q + 2k - \epsilon_q}{2} + \frac{\epsilon_q + 3k - \epsilon_q}{3} - (\epsilon_q + k - \epsilon_q)}{h z - \frac{\epsilon_q + 3k - \epsilon_q}{3}} + \frac{\epsilon_q + 2k - \epsilon_q}{h z - \frac{\epsilon_q + 2k - \epsilon_q}{2}} + \frac{\epsilon_q + 3k - \epsilon_q}{h z - (\epsilon_q + k - \epsilon_q)} \right] \Rightarrow \\
& = + \int \frac{d^3 q}{(2\pi)^3} \frac{2f_0(\mathbf{q})}{9(\epsilon_q + 2k - \epsilon_q)(\epsilon_q + k - \epsilon_q)(2\epsilon_q + k - 2\epsilon_q - \epsilon_q + 2k + \epsilon_q) - 4(\epsilon_q + 3k - \epsilon_q)(\epsilon_q + k - \epsilon_q)(3\epsilon_q + k - 3\epsilon_q - \epsilon_q + 2k - 2\epsilon_q - 3\epsilon_q + 2k + 3\epsilon_q)} \\
& \left[ \frac{6\epsilon_q + k - 6\epsilon_q - 3\epsilon_q + 2k + 3\epsilon_q}{h z - \frac{\epsilon_q + 3k - \epsilon_q}{3}} + \frac{2\epsilon_q + 3k - 2\epsilon_q - 6\epsilon_q + k + 6\epsilon_q}{h z - \frac{\epsilon_q + 2k - \epsilon_q}{2}} + \frac{3\epsilon_q + 2k - 3\epsilon_q - 2\epsilon_q + 3k + 2\epsilon_q}{h z - (\epsilon_q + k - \epsilon_q)} \right] \Rightarrow \\
& = + \int \frac{d^3 q}{(2\pi)^3} \frac{2f_0(\mathbf{q})}{9(4k^2 + 4q \cdot k)(k^2 + 2q \cdot k)(2k^2 + 4q \cdot k - 4k^2 - 4q \cdot k) - 4(9k^2 + 6q \cdot k)(2q \cdot k + k^2)(3k^2 + 2q \cdot k)(k^2 + q \cdot k)} \\
& \left[ \frac{6k^2 + 12q \cdot k - 12k^2 - 12q \cdot k}{h z - \frac{\epsilon_q + 3k - \epsilon_q}{3}} + \frac{18k^2 + 12q \cdot k - 6k^2 - 12q \cdot k}{h z - \frac{\epsilon_q + 2k - \epsilon_q}{2}} + \frac{12k^2 + 12q \cdot k - 18k^2 - 12q \cdot k}{h z - (\epsilon_q + k - \epsilon_q)} \right] \Rightarrow \\
& = - \int \frac{d^3 q}{(2\pi)^3} \frac{2f_0(\mathbf{q})}{-72k^2(k^2 + q \cdot k)(k^2 + 2q \cdot k) + 72k^2(3k^2 + 2q \cdot k)(k^2 + 2q \cdot k) - 72k^2(3k^2 + 2q \cdot k)(k^2 + q \cdot k)} \left[ \frac{6k^2}{h z - \frac{\epsilon_q + 3k - \epsilon_q}{3}} - \frac{12k^2}{h z - \frac{\epsilon_q + 2k - \epsilon_q}{2}} + \frac{6k^2}{h z - (\epsilon_q + k - \epsilon_q)} \right] \Rightarrow \\
& = - \int \frac{d^3 q}{(2\pi)^3} \frac{2f_0(\mathbf{q})}{-72k^2[(k^2 + q \cdot k)(k^2 + 2q \cdot k) - (3k^2 + 2q \cdot k)(q \cdot k)]} \left[ \frac{6k^2}{h z - \frac{\epsilon_q + 3k - \epsilon_q}{3}} - \frac{12k^2}{h z - \frac{\epsilon_q + 2k - \epsilon_q}{2}} + \frac{6k^2}{h z - (\epsilon_q + k - \epsilon_q)} \right] \Rightarrow \\
& = - \int \frac{d^3 q}{(2\pi)^3} \frac{2f_0(\mathbf{q})}{-72k^2[k^4 + 3k^2(q \cdot k) + 2(q \cdot k)^2 - 3k^2(q \cdot k) - 2(q \cdot k)^2] - \frac{6k^2}{h z - (\epsilon_q + k - \epsilon_q)}} \left[ \frac{6k^2}{h z - \frac{\epsilon_q + 3k - \epsilon_q}{3}} - \frac{12k^2}{h z - \frac{\epsilon_q + 2k - \epsilon_q}{2}} + \frac{6k^2}{h z - (\epsilon_q + k - \epsilon_q)} \right] \Rightarrow \\
& = - \int \frac{d^3 q}{(2\pi)^3} \frac{2f_0(\mathbf{q})}{-72k^6 \left[ \frac{1}{h z - \frac{\epsilon_q + 3k - \epsilon_q}{3}} - \frac{2}{h z - \frac{\epsilon_q + 2k - \epsilon_q}{2}} + \frac{1}{h z - (\epsilon_q + k - \epsilon_q)} \right]} \Rightarrow \\
& = - \int \frac{d^3 q}{(2\pi)^3} \frac{2f_0(\mathbf{q})}{-72k^6 \left[ \frac{1}{h z - \frac{\epsilon_q + 3k - \epsilon_q}{3}} - \frac{2}{h z - \frac{\epsilon_q + 2k - \epsilon_q}{2}} + \frac{1}{h z - (\epsilon_q + k - \epsilon_q)} \right]} \Rightarrow \\
& = + \int \frac{d^3 q}{(2\pi)^3} \frac{2f_0(\mathbf{q})}{6k^4 \left[ \frac{1}{h z - \frac{\epsilon_q + 3k - \epsilon_q}{3}} - \frac{2}{h z - \frac{\epsilon_q + 2k - \epsilon_q}{2}} + \frac{1}{h z - (\epsilon_q + k - \epsilon_q)} \right]} \Rightarrow \\
& = + \int \frac{d^3 q}{(2\pi)^3} \frac{2f_0(\mathbf{q})}{6k^4 \left[ \frac{1}{h z - \frac{\epsilon_q + 3k - \epsilon_q}{3}} - \frac{2}{h z - \frac{\epsilon_q + 2k - \epsilon_q}{2}} + \frac{1}{h z - (\epsilon_q + k - \epsilon_q)} \right]} \Rightarrow \\
& = + \left( \frac{m}{\hbar^2} \right)^2 \frac{1}{3k^4} \int \frac{d^3 q}{(2\pi)^3} \frac{2f_0(\mathbf{q})}{h(3z) - \epsilon_q + 3k + \epsilon_q - \frac{1}{h(2z) - \epsilon_q + 2k + \epsilon_q} + \frac{1}{h z - \epsilon_q + k + \epsilon_q}}.
\end{aligned}$$

$$\begin{aligned}
\chi_0^{(3,3)}(\mathbf{k}, z) &= + \left( \frac{m}{\hbar^2} \right)^2 \frac{1}{3k^4} \int \frac{d^3 q}{(2\pi)^3} 2f_0(\mathbf{q}) \left[ -\frac{3}{\hbar(3z) - \epsilon_q + \epsilon_{q-3k}} + \frac{4}{\hbar(2z) - \epsilon_q + \epsilon_{q-2k}} - \frac{1}{\hbar z - \epsilon_q + \epsilon_{q-k}} \right] \\
&+ \left( \frac{m}{\hbar^2} \right)^2 \frac{1}{3k^4} \int \frac{d^3 q}{(2\pi)^3} 2f_0(\mathbf{q}) \left[ \frac{1}{\hbar z - \epsilon_q + \epsilon_{q-k}} - \frac{\hbar(2z) - \epsilon_{q+k} + \epsilon_{q-k}}{4} + \frac{1}{\hbar z - \epsilon_{q+k} + \epsilon_q} \right] \\
&+ \left( \frac{m}{\hbar^2} \right)^2 \frac{1}{3k^4} \int \frac{d^3 q}{(2\pi)^3} 2f_0(\mathbf{q}) \left[ \frac{\hbar(2z) - \epsilon_{q+k} + \epsilon_{q-k}}{4} - \frac{\hbar^2 k^2}{2} - \frac{\hbar(2z) - \epsilon_{q+k} + \epsilon_{q-k}}{2} \right] \\
&+ \left( \frac{m}{\hbar^2} \right)^2 \frac{1}{3k^4} \int \frac{d^3 q}{(2\pi)^3} 2f_0(\mathbf{q}) \left[ -\frac{\hbar(2z) - \epsilon_{q+2k} + \epsilon_q}{4} + \frac{\hbar^2 k^2}{2} - \frac{\hbar(2z) - \epsilon_{q+k} + \epsilon_q}{2} \right] \\
&+ \left( \frac{m}{\hbar^2} \right)^2 \frac{1}{3k^4} \int \frac{d^3 q}{(2\pi)^3} 2f_0(\mathbf{q}) \left[ \frac{\hbar(2z) - \epsilon_q + \epsilon_{q-2k}}{4} + \frac{\hbar^2 k^2}{2m} - \frac{\hbar(2z) - \epsilon_{q+k} + \epsilon_q}{2} - \frac{\hbar(2z) - \epsilon_{q+k} + \epsilon_q}{2} \right] \\
&+ \left( \frac{m}{\hbar^2} \right)^2 \frac{1}{3k^4} \int \frac{d^3 q}{(2\pi)^3} 2f_0(\mathbf{q}) \left[ -\frac{\hbar(2z) - \epsilon_{q+k} + \epsilon_{q-k}}{4} - \frac{\hbar^2 k^2}{2m} - \frac{\hbar(2z) - \epsilon_{q+k} + \epsilon_q}{2} + \frac{\hbar(2z) - \epsilon_{q+k} + \epsilon_q}{2} \right] \\
&+ \left( \frac{m}{\hbar^2} \right)^2 \frac{1}{3k^4} \int \frac{d^3 q}{(2\pi)^3} 2f_0(\mathbf{q}) \left[ -\frac{1}{\hbar z - \epsilon_{q+k} + \epsilon_q} + \frac{\hbar(2z) - \epsilon_{q+k} + \epsilon_{q-k}}{4} - \frac{1}{\hbar z - \epsilon_q + \epsilon_{q-k}} \right] \\
&+ \left( \frac{m}{\hbar^2} \right)^2 \frac{1}{3k^4} \int \frac{d^3 q}{(2\pi)^3} 2f_0(\mathbf{q}) \left[ \frac{\hbar(3z) - \epsilon_{q+3k} + \epsilon_q}{3} - \frac{\hbar(2z) - \epsilon_{q+2k} + \epsilon_q}{4} + \frac{1}{\hbar z - \epsilon_{q+k} + \epsilon_q} \right] \Rightarrow \\
\chi_0^{(3,3)}(\mathbf{k}, z) &= + \left( \frac{m}{\hbar^2} \right)^2 \frac{1}{3k^4} \int \frac{d^3 q}{(2\pi)^3} 2f_0(\mathbf{q}) \left[ -\frac{3}{\hbar(3z) - \epsilon_q + \epsilon_{q-3k}} + \frac{4}{\hbar(2z) - \epsilon_q + \epsilon_{q-2k}} - \frac{1}{\hbar z - \epsilon_q + \epsilon_{q-k}} + \frac{1}{\hbar z - \epsilon_{q+k} + \epsilon_q} \right] \\
&+ \frac{4}{\hbar(2z) - \epsilon_{q+k} + \epsilon_{q-k}} - \frac{\hbar^2 k^2}{2m} - \frac{\hbar(2z) - \epsilon_{q+k} + \epsilon_{q-k}}{4} + \frac{\hbar^2 k^2}{2} + \frac{2m}{\hbar(2z) - \epsilon_{q+k} + \epsilon_q} + \frac{\hbar(2z) - \epsilon_{q+k} + \epsilon_q}{2} \\
&+ \frac{\hbar(2z) - \epsilon_q + \epsilon_{q-2k}}{4} + \frac{\hbar^2 k^2}{2} + \frac{2m}{\hbar(2z) - \epsilon_{q+k} + \epsilon_q} - \frac{\hbar(2z) - \epsilon_{q+k} + \epsilon_{q-k}}{4} + \frac{\hbar^2 k^2}{2} + \frac{\hbar(2z) - \epsilon_{q+k} + \epsilon_q}{2} \\
&- \frac{1}{\hbar z - \epsilon_{q+k} + \epsilon_q} + \frac{\hbar(2z) - \epsilon_{q+k} + \epsilon_{q-k}}{4} + \frac{1}{\hbar z - \epsilon_q + \epsilon_{q-k}} - \frac{\hbar(3z) - \epsilon_{q+3k} + \epsilon_q}{3} + \frac{1}{\hbar z - \epsilon_{q+k} + \epsilon_q} \Rightarrow \\
\chi_0^{(3,3)}(\mathbf{k}, z) &= + \left( \frac{m}{\hbar^2} \right)^2 \frac{1}{3k^4} \int \frac{d^3 q}{(2\pi)^3} 2f_0(\mathbf{q}) \left[ -\frac{3}{\hbar(3z) - \epsilon_q + \epsilon_{q-3k}} + \frac{\hbar(3z) - \epsilon_{q+3k} + \epsilon_q}{3} - \frac{\hbar(2z) - \epsilon_{q+2k} + \epsilon_q}{8} - \frac{5}{\hbar z - \epsilon_{q+k} + \epsilon_q} \right] \Rightarrow \\
\chi_0^{(3,3)}(\mathbf{k}, z) &= - \left( \frac{m}{\hbar^2} \right)^2 \frac{1}{3k^4} \int \frac{d^3 q}{(2\pi)^3} 2f_0(\mathbf{q}) \left[ \frac{\hbar(3z) - \epsilon_q + \epsilon_{q-3k}}{3} - \frac{\hbar(3z) - \epsilon_{q+3k} + \epsilon_q}{3} + \frac{\hbar(2z) - \epsilon_{q+2k} + \epsilon_q}{8} - \frac{5}{\hbar z - \epsilon_{q+k} + \epsilon_q} \right] \Rightarrow \\
\chi_0^{(3,3)}(\mathbf{k}, z) &= - \left( \frac{m}{\hbar^2} \right)^2 \frac{3}{3k^4} \int \frac{d^3 q}{(2\pi)^3} 2f_0(\mathbf{q}) \left[ \frac{1}{\hbar(3z) - \epsilon_q + \epsilon_{q-3k}} - \frac{\hbar(3z) - \epsilon_{q+3k} + \epsilon_q}{3} + \frac{\hbar(2z) - \epsilon_{q+2k} + \epsilon_q}{8} - \frac{5}{\hbar z - \epsilon_{q+k} + \epsilon_q} \right] \Rightarrow \\
&- \left( \frac{m}{\hbar^2} \right)^2 \frac{5}{3k^4} \int \frac{d^3 q}{(2\pi)^3} 2f_0(\mathbf{q}) \left[ \frac{1}{\hbar z - \epsilon_q + \epsilon_{q-k}} - \frac{1}{\hbar z - \epsilon_{q+k} + \epsilon_q} \right] \Rightarrow \\
\chi_0^{(3,3)}(\mathbf{k}, z) &= \left( \frac{m}{\hbar^2} \right)^2 \frac{3}{3k^4} \chi_0(3\mathbf{k}, 3z) - \left( \frac{m}{\hbar^2} \right)^2 \frac{8}{3k^4} \chi_0(2\mathbf{k}, 2z) + \frac{5}{3k^4} \chi_0(\mathbf{k}, z) \Rightarrow \\
\chi_0^{(3,3)}(\mathbf{k}, z) &= \left( \frac{m}{\hbar^2} \right)^2 \frac{1}{3k^4} [3\chi_0(3\mathbf{k}, 3z) - 8\chi_0(2\mathbf{k}, 2z) + 5\chi_0(\mathbf{k}, z)] .
\end{aligned}$$

**The normalized compact form of the symmetric expression.** From the definition of the third order ideal density response as the third order functional derivative of the density with respect to the external potential energy, it is evident that the proper normalization is achieved by dividing with  $1/(n\beta^3)$ . In addition from the definition of the first order ideal density response as the first order functional derivative of the density with respect to the external potential energy, it is evident that the proper normalization of the Lindhard response is achieved by dividing with  $1/(n\beta)$ . The calculation proceeds with the introduction of the dimensionless complex frequency  $z = (T/\hbar)Z$  as well as of the dimensionless wavenumber  $k = k_F x$ . The utilization of the Fermi energy definition  $E_F = \hbar^2 k_F^2 / (2m)$  and the introduction of the degeneracy temperature definition  $\Theta = T/E_F$  ultimately lead to

$$\begin{aligned}
\chi_0^{(3,3)}(\mathbf{k}, z) &= \left(\frac{m}{\hbar^2}\right)^2 \frac{1}{3k^4} [3\chi_0(3\mathbf{k}, 3z) - 8\chi_0(2\mathbf{k}, 2z) + 5\chi_0(\mathbf{k}, z)] \Rightarrow \\
\frac{\chi_0^{(3,3)}(\mathbf{k}, z)}{n\beta^3} &= + \frac{1}{n\beta^3} \left(\frac{m}{\hbar^2}\right)^2 \frac{1}{3k^4} [3\chi_0(3\mathbf{k}, 3z) - 8\chi_0(2\mathbf{k}, 2z) + 5\chi_0(\mathbf{k}, z)] \Rightarrow \\
\frac{\chi_0^{(3,3)}(\mathbf{k}, z)}{n\beta^3} &= + \left(\frac{m}{\hbar^2}\right)^2 \frac{T^2}{3k^4} \left[3\frac{\chi_0(3\mathbf{k}, 3z)}{n\beta} - 8\frac{\chi_0(2\mathbf{k}, 2z)}{n\beta} + 5\frac{\chi_0(\mathbf{k}, z)}{n\beta}\right] \Rightarrow \\
\frac{\chi_0^{(3,3)}(\mathbf{x}, Z)}{n\beta^3} &= + \left(\frac{m}{\hbar^2}\right)^2 \frac{T^2}{3k_F^4 x^4} \left[3\frac{\chi_0(3\mathbf{x}, 3Z)}{n\beta} - 8\frac{\chi_0(2\mathbf{x}, 2Z)}{n\beta} + 5\frac{\chi_0(\mathbf{x}, Z)}{n\beta}\right] \Rightarrow \\
\frac{\chi_0^{(3,3)}(\mathbf{x}, Z)}{n\beta^3} &= + \left(\frac{2m}{\hbar^2 k_F^2}\right)^2 \frac{1}{2^2} \frac{T^2}{3x^4} \left[3\frac{\chi_0(3\mathbf{x}, 3Z)}{n\beta} - 8\frac{\chi_0(2\mathbf{x}, 2Z)}{n\beta} + 5\frac{\chi_0(\mathbf{x}, Z)}{n\beta}\right] \Rightarrow \\
\frac{\chi_0^{(3,3)}(\mathbf{x}, Z)}{n\beta^3} &= + \frac{T^2}{[\hbar^2 k_F^2 / (2m)]^2} \frac{1}{2^2} \frac{1}{3x^4} \left[3\frac{\chi_0(3\mathbf{x}, 3Z)}{n\beta} - 8\frac{\chi_0(2\mathbf{x}, 2Z)}{n\beta} + 5\frac{\chi_0(\mathbf{x}, Z)}{n\beta}\right] \Rightarrow \\
\frac{\chi_0^{(3,3)}(\mathbf{x}, Z)}{n\beta^3} &= + \frac{T^2}{E_F^2} \frac{1}{2^2} \frac{1}{3x^4} \left[3\frac{\chi_0(3\mathbf{x}, 3Z)}{n\beta} - 8\frac{\chi_0(2\mathbf{x}, 2Z)}{n\beta} + 5\frac{\chi_0(\mathbf{x}, Z)}{n\beta}\right] \Rightarrow \\
\frac{\chi_0^{(3,3)}(\mathbf{x}, Z)}{n\beta^3} &= + \frac{1}{2^2} \frac{1}{3} \frac{\Theta^2}{x^4} \left[3\frac{\chi_0(3\mathbf{x}, 3Z)}{n\beta} - 8\frac{\chi_0(2\mathbf{x}, 2Z)}{n\beta} + 5\frac{\chi_0(\mathbf{x}, Z)}{n\beta}\right] \Rightarrow \\
\frac{\chi_0^{(3,3)}(\mathbf{x}, Z)}{n\beta^3} &= + \frac{1}{12} \frac{\Theta^2}{x^4} \left[3\frac{\chi_0(3\mathbf{x}, 3Z)}{n\beta} - 8\frac{\chi_0(2\mathbf{x}, 2Z)}{n\beta} + 5\frac{\chi_0(\mathbf{x}, Z)}{n\beta}\right] \Rightarrow \\
\frac{\chi_0^{(3,3)}(\mathbf{x}, Z)}{n\beta^3} &= + \frac{1}{2} \frac{1}{2 \times 3} \frac{\Theta^2}{x^4} \left[3\frac{\chi_0(3\mathbf{x}, 3Z)}{n\beta} - 8\frac{\chi_0(2\mathbf{x}, 2Z)}{n\beta} + 5\frac{\chi_0(\mathbf{x}, Z)}{n\beta}\right] \Rightarrow \\
\frac{\chi_0^{(3,3)}(\mathbf{x}, Z)}{n\beta^3} &= + \frac{1}{2!} \frac{1}{3!} \frac{\Theta^2}{x^4} \left[3\frac{\chi_0(3\mathbf{x}, 3Z)}{n\beta} - 8\frac{\chi_0(2\mathbf{x}, 2Z)}{n\beta} + 5\frac{\chi_0(\mathbf{x}, Z)}{n\beta}\right] \Rightarrow \\
\frac{\chi_0^{(3,3)}(\mathbf{x}, Z)}{n\beta^3} &= + \frac{1}{(3-1)!} \frac{1}{3!} \frac{\Theta^2}{x^4} \left[3\frac{\chi_0(3\mathbf{x}, 3Z)}{n\beta} - 8\frac{\chi_0(2\mathbf{x}, 2Z)}{n\beta} + 5\frac{\chi_0(\mathbf{x}, Z)}{n\beta}\right].
\end{aligned}$$

In the final steps, the numerical pre-factors were decomposed into products that were later expressed as factorials with respect to the order of the ideal density response. Ultimately, one has

$$\frac{\chi_0^{(3,3)}(\mathbf{x}, Z)}{n\beta^3} = + \frac{1}{(3-1)!} \frac{1}{3!} \frac{\Theta^2}{x^4} \left[3\frac{\chi_0(3\mathbf{x}, 3Z)}{n\beta} - 8\frac{\chi_0(2\mathbf{x}, 2Z)}{n\beta} + 5\frac{\chi_0(\mathbf{x}, Z)}{n\beta}\right].$$

The static limit simply reads as

$$\frac{\chi_0^{(3,3)}(\mathbf{x})}{n\beta^3} = + \frac{1}{(3-1)!} \frac{1}{3!} \frac{\Theta^2}{x^4} \left[3\frac{\chi_0(3\mathbf{x})}{n\beta} - 8\frac{\chi_0(2\mathbf{x})}{n\beta} + 5\frac{\chi_0(\mathbf{x})}{n\beta}\right].$$

**The long wavelength limit of the static normalized symmetric expression.** The long-wavelength limit of the static third order ideal density response at the third harmonic should converge. Given the  $1/x^4$  pre-factor and the even parity, this implies that the first two terms of the small argument expansion of the ideal cubic density response should cancel out exactly, otherwise the long-wavelength limit of the static case would diverge. We first write down the first three terms of the small argument expansion of the ideal Lindhard density response for the arguments  $3\mathbf{x}$ ,  $2\mathbf{x}$ ,  $\mathbf{x}$ .

$$\begin{aligned}\frac{\chi_0(\mathbf{x})}{n\beta} &\simeq -\frac{3}{2}\Theta \int_0^\infty dy f_0(y; \Theta) \left[ 1 + \frac{1}{12} \left(\frac{x}{y}\right)^2 + \frac{1}{5} \frac{1}{16} \left(\frac{x}{y}\right)^4 \right], \\ \frac{\chi_0(2\mathbf{x})}{n\beta} &\simeq -\frac{3}{2}\Theta \int_0^\infty dy f_0(y; \Theta) \left[ 1 + \frac{1}{3} \left(\frac{x}{y}\right)^2 + \frac{1}{5} \left(\frac{x}{y}\right)^4 \right], \\ \frac{\chi_0(3\mathbf{x})}{n\beta} &\simeq -\frac{3}{2}\Theta \int_0^\infty dy f_0(y; \Theta) \left[ 1 + \frac{3}{4} \left(\frac{x}{y}\right)^2 + \frac{1}{5} \frac{81}{16} \left(\frac{x}{y}\right)^4 \right].\end{aligned}$$

Then, we substitute the above in the static limit of the normalized compact form of the third order ideal density response at the third harmonic

$$\begin{aligned}\frac{\chi_0^{(3,3)}(\mathbf{x})}{n\beta^3} &= +\frac{1}{(3-1)!} \frac{1}{3!} \frac{\Theta^2}{x^4} \left[ 3 \frac{\chi_0(3\mathbf{x})}{n\beta} - 8 \frac{\chi_0(2\mathbf{x})}{n\beta} + 5 \frac{\chi_0(\mathbf{x})}{n\beta} \right] \Rightarrow \\ \frac{\chi_0^{(3,3)}(\mathbf{x})}{n\beta^3} &= -\frac{1}{(3-1)!} \frac{1}{3!} \frac{\Theta^2}{x^4} \left\{ 3 \frac{3}{2} \Theta \int_0^\infty dy f_0(y; \Theta) \left[ 1 + \frac{3}{4} \left(\frac{x}{y}\right)^2 + \frac{1}{5} \frac{81}{16} \left(\frac{x}{y}\right)^4 \right] \right. \\ &\quad \left. - 8 \frac{3}{2} \Theta \int_0^\infty dy f_0(y; \Theta) \left[ 1 + \frac{1}{3} \left(\frac{x}{y}\right)^2 + \frac{1}{5} \left(\frac{x}{y}\right)^4 \right] \right. \\ &\quad \left. + 5 \frac{3}{2} \Theta \int_0^\infty dy f_0(y; \Theta) \left[ 1 + \frac{1}{12} \left(\frac{x}{y}\right)^2 + \frac{1}{5} \frac{1}{16} \left(\frac{x}{y}\right)^4 \right] \right\} \Rightarrow \\ \frac{\chi_0^{(3,3)}(\mathbf{x})}{n\beta^3} &= -\frac{1}{(3-1)!} \frac{1}{3!} \frac{\Theta^2}{x^4} \left\{ \frac{3}{2} \Theta \int_0^\infty dy f_0(y; \Theta) \left[ +3 + 3 \frac{3}{4} \left(\frac{x}{y}\right)^2 + 3 \frac{1}{5} \frac{81}{16} \left(\frac{x}{y}\right)^4 \right] \right. \\ &\quad \left. + \frac{3}{2} \Theta \int_0^\infty dy f_0(y; \Theta) \left[ -8 - 8 \frac{1}{3} \left(\frac{x}{y}\right)^2 - 8 \frac{1}{5} \left(\frac{x}{y}\right)^4 \right] \right. \\ &\quad \left. + \frac{3}{2} \Theta \int_0^\infty dy f_0(y; \Theta) \left[ +5 + 5 \frac{1}{12} \left(\frac{x}{y}\right)^2 + 5 \frac{1}{5} \frac{1}{16} \left(\frac{x}{y}\right)^4 \right] \right\} \Rightarrow \\ \frac{\chi_0^{(3,3)}(\mathbf{x})}{n\beta^3} &= -\frac{1}{(3-1)!} \frac{1}{3!} \frac{\Theta^2}{x^4} \frac{3}{2} \Theta \int_0^\infty dy f_0(y; \Theta) \left[ +3 + 3 \frac{3}{4} \left(\frac{x}{y}\right)^2 + 3 \frac{1}{5} \frac{81}{16} \left(\frac{x}{y}\right)^4 \right. \\ &\quad \left. - 8 - 8 \frac{1}{3} \left(\frac{x}{y}\right)^2 - 8 \frac{1}{5} \left(\frac{x}{y}\right)^4 + 5 + 5 \frac{1}{12} \left(\frac{x}{y}\right)^2 + 5 \frac{1}{5} \frac{1}{16} \left(\frac{x}{y}\right)^4 \right] \Rightarrow \\ \frac{\chi_0^{(3,3)}(\mathbf{x})}{n\beta^3} &= -\frac{1}{(3-1)!} \frac{1}{3!} \frac{\Theta^2}{x^4} \frac{3}{2} \Theta \int_0^\infty dy f_0(y; \Theta) \left[ 3 + \frac{9}{4} \left(\frac{x}{y}\right)^2 + \frac{243}{80} \left(\frac{x}{y}\right)^4 \right. \\ &\quad \left. - 8 - \frac{8}{3} \left(\frac{x}{y}\right)^2 - \frac{8}{5} \left(\frac{x}{y}\right)^4 + 5 + \frac{5}{12} \left(\frac{x}{y}\right)^2 + \frac{5}{80} \left(\frac{x}{y}\right)^4 \right] \Rightarrow \\ \frac{\chi_0^{(3,3)}(\mathbf{x})}{n\beta^3} &= -\frac{1}{(3-1)!} \frac{1}{3!} \frac{\Theta^2}{x^4} \frac{3}{2} \Theta \int_0^\infty dy f_0(y; \Theta) \left[ 3 + \frac{27}{12} \left(\frac{x}{y}\right)^2 + \frac{243}{80} \left(\frac{x}{y}\right)^4 \right. \\ &\quad \left. - 8 - \frac{32}{12} \left(\frac{x}{y}\right)^2 - \frac{128}{80} \left(\frac{x}{y}\right)^4 + 5 + \frac{5}{12} \left(\frac{x}{y}\right)^2 + \frac{5}{80} \left(\frac{x}{y}\right)^4 \right].\end{aligned}$$

We simply re-organize the terms in ascending powers of  $x/y$ . It is straightforward to prove that the first two terms,  $\propto (x/y)^0, (x/y)^2$ , cancel out exactly. The leading order term is  $\mathcal{O}[(x/y)^4]$  and leads to finite contribution at the long-wavelength limit,  $\mathcal{O}(y^{-4})$ , after the removal of the  $1/x^4$  pre-factor. It is rather apparent that the remaining improper integral is indeed convergent.

$$\begin{aligned}
\frac{\chi_0^{(3,3)}(\mathbf{x})}{n\beta^3} &= -\frac{1}{(3-1)!} \frac{1}{3!} \frac{\Theta^2}{x^4} \frac{3}{2} \Theta \int_0^\infty dy f_0(y; \Theta) \left[ 3 + \frac{27}{12} \left(\frac{x}{y}\right)^2 + \frac{243}{80} \left(\frac{x}{y}\right)^4 \right. \\
&\quad \left. - 8 - \frac{32}{12} \left(\frac{x}{y}\right)^2 - \frac{128}{80} \left(\frac{x}{y}\right)^4 + 5 + \frac{5}{12} \left(\frac{x}{y}\right)^2 + \frac{5}{80} \left(\frac{x}{y}\right)^4 \right] \Rightarrow \\
\frac{\chi_0^{(3,3)}(\mathbf{x})}{n\beta^3} &= -\frac{1}{(3-1)!} \frac{1}{3!} \frac{\Theta^2}{x^4} \frac{3}{2} \Theta \int_0^\infty dy f_0(y; \Theta) \left[ 3 - 8 + 5 + \frac{27}{12} \left(\frac{x}{y}\right)^2 - \frac{32}{12} \left(\frac{x}{y}\right)^2 + \frac{5}{12} \left(\frac{x}{y}\right)^2 \right. \\
&\quad \left. + \frac{243}{80} \left(\frac{x}{y}\right)^4 - \frac{128}{80} \left(\frac{x}{y}\right)^4 + \frac{5}{80} \left(\frac{x}{y}\right)^4 \right] \Rightarrow \\
\frac{\chi_0^{(3,3)}(\mathbf{x})}{n\beta^3} &= -\frac{1}{(3-1)!} \frac{1}{3!} \frac{\Theta^2}{x^4} \frac{3}{2} \Theta \int_0^\infty dy f_0(y; \Theta) \left[ (3 - 8 + 5) + \left(\frac{27}{12} - \frac{32}{12} + \frac{5}{12}\right) \left(\frac{x}{y}\right)^2 \right. \\
&\quad \left. + \left(\frac{243}{80} - \frac{128}{80} + \frac{5}{80}\right) \left(\frac{x}{y}\right)^4 \right] \Rightarrow \\
\frac{\chi_0^{(3,3)}(\mathbf{x})}{n\beta^3} &= -\frac{1}{(3-1)!} \frac{1}{3!} \frac{\Theta^2}{x^4} \frac{3}{2} \Theta \int_0^\infty dy f_0(y; \Theta) \left[ (8 - 8) + \frac{27 - 32 + 5}{12} \left(\frac{x}{y}\right)^2 + \frac{243 - 128 + 5}{80} \left(\frac{x}{y}\right)^4 \right] \Rightarrow \\
\frac{\chi_0^{(3,3)}(\mathbf{x})}{n\beta^3} &= -\frac{1}{(3-1)!} \frac{1}{3!} \frac{\Theta^2}{x^4} \frac{3}{2} \Theta \int_0^\infty dy f_0(y; \Theta) \left[ (8 - 8) + \frac{32 - 32}{12} \left(\frac{x}{y}\right)^2 + \frac{248 - 128}{80} \left(\frac{x}{y}\right)^4 \right] \Rightarrow \\
\frac{\chi_0^{(3,3)}(\mathbf{x})}{n\beta^3} &= -\frac{1}{(3-1)!} \frac{1}{3!} \frac{\Theta^2}{x^4} \frac{3}{2} \Theta \int_0^\infty dy f_0(y; \Theta) \frac{248 - 128}{80} \left(\frac{x}{y}\right)^4 \Rightarrow \\
\frac{\chi_0^{(3,3)}(\mathbf{x})}{n\beta^3} &= -\frac{1}{(3-1)!} \frac{1}{3!} \frac{\Theta^2}{x^4} \frac{3}{2} \Theta \int_0^\infty dy f_0(y; \Theta) \frac{120}{80} \left(\frac{x}{y}\right)^4 \Rightarrow \\
\frac{\chi_0^{(3,3)}(\mathbf{x})}{n\beta^3} &= -\frac{1}{(3-1)!} \frac{1}{3!} \frac{\Theta^2}{x^4} \frac{3}{2} \Theta \int_0^\infty dy f_0(y; \Theta) \frac{3}{2} \left(\frac{x}{y}\right)^4 \Rightarrow \\
\frac{\chi_0^{(3,3)}(\mathbf{x})}{n\beta^3} &= -\frac{1}{(3-1)!} \frac{1}{3!} \frac{\Theta^2}{x^4} \frac{3}{2} \frac{3}{2} \Theta \int_0^\infty dy f_0(y; \Theta) \left(\frac{x}{y}\right)^4 \Rightarrow \\
\frac{\chi_0^{(3,3)}(\mathbf{x})}{n\beta^3} &= -\frac{1}{2} \frac{1}{6} \frac{3}{2} \frac{3}{2} \frac{\Theta^2}{x^4} \Theta \int_0^\infty dy f_0(y; \Theta) \left(\frac{x}{y}\right)^4 \Rightarrow \\
\frac{\chi_0^{(3,3)}(\mathbf{x})}{n\beta^3} &= -\frac{1}{12} \frac{9}{4} \frac{\Theta^3}{x^4} \int_0^\infty dy f_0(y; \Theta) \left(\frac{x}{y}\right)^4 \Rightarrow \\
\frac{\chi_0^{(3,3)}(\mathbf{x})}{n\beta^3} &= -\frac{3}{16} \frac{\Theta^3}{x^4} \int_0^\infty dy f_0(y; \Theta) \left(\frac{x}{y}\right)^4 \Rightarrow \\
\frac{\chi_0^{(3,3)}(\mathbf{x})}{n\beta^3} &= -\frac{3}{16} \Theta^3 \int_0^\infty dy f_0(y; \Theta) \frac{1}{x^4} \frac{x^4}{y^4} \Rightarrow \\
\frac{\chi_0^{(3,3)}(\mathbf{x})}{n\beta^3} &= -\frac{3}{16} \Theta^3 \int_0^\infty dy \frac{f_0(y; \Theta)}{y^4}.
\end{aligned}$$

31

[illegible]



Afterwards, the above third order perturbations are substituted into the general expression for the fourth order perturbation of the non-interacting distribution function. Prior to the substitution, it is again convenient to use the equivalent form  $\hbar\omega = \hbar(\omega - \omega' - \omega'' - \omega''') + \hbar\omega' + \hbar\omega'' + \hbar\omega'''$  and  $\mathbf{k} = (\mathbf{k} - \mathbf{k}' - \mathbf{k}'' - \mathbf{k}''') + \mathbf{k}' + \mathbf{k}'' + \mathbf{k}'''$  in the denominator in order to symmetrize the integrand with respect to the arguments of the potential energy perturbations (again in view of the triple convolution definition of the fourth order density response). The expression is then slightly restructured in order to facilitate the direct substitution of the cumbersome  $f_{\mathbf{q},\mathbf{k},\omega}^{\text{ind},(3)}, f_{\mathbf{q}-\frac{1}{2}\mathbf{k}',\mathbf{k}-\mathbf{k}',\omega-\omega'}, f_{\mathbf{q}-\frac{1}{2}\mathbf{k}',\mathbf{k}-\mathbf{k}',\omega-\omega'}^{\text{ind},(3)}$  terms without any misprints.

$$\begin{aligned}
f_{\mathbf{q},\mathbf{k},\omega}^{\text{ind},(n)} &= - \int \frac{d\omega' d^3 k'}{(2\pi)^4} \left[ \frac{f_{\mathbf{q}+\frac{1}{2}\mathbf{k}',\mathbf{k}-\mathbf{k}',\omega-\omega'}^{\text{ind},(n-1)} - f_{\mathbf{q}-\frac{1}{2}\mathbf{k}',\mathbf{k}-\mathbf{k}',\omega-\omega'}^{\text{ind},(n-1)}}{\hbar\omega - \epsilon_{\mathbf{q}+\frac{1}{2}\mathbf{k}} + \epsilon_{\mathbf{q}-\frac{1}{2}\mathbf{k}}} + \epsilon_{\mathbf{q}-\frac{1}{2}\mathbf{k}} \right] U_{\mathbf{k}',\omega'}^{\text{ext}} \Rightarrow \\
f_{\mathbf{q},\mathbf{k},\omega}^{\text{ind},(4)} &= - \int \frac{d\omega' d^3 k'}{(2\pi)^4} \left[ \frac{f_{\mathbf{q}+\frac{1}{2}\mathbf{k}',\mathbf{k}-\mathbf{k}',\omega-\omega'}^{\text{ind},(3)} - f_{\mathbf{q}-\frac{1}{2}\mathbf{k}',\mathbf{k}-\mathbf{k}',\omega-\omega'}^{\text{ind},(3)}}{\hbar\omega - \epsilon_{\mathbf{q}+\frac{1}{2}\mathbf{k}} + \epsilon_{\mathbf{q}-\frac{1}{2}\mathbf{k}}} + \epsilon_{\mathbf{q}-\frac{1}{2}\mathbf{k}} \right] U_{\mathbf{k}',\omega'}^{\text{ext}} \Rightarrow \\
f_{\mathbf{q},\mathbf{k},\omega}^{\text{ind},(4)} &= - \int \frac{d\omega' d^3 k'}{(2\pi)^4} \left[ \frac{f_{\mathbf{q}+\frac{1}{2}\mathbf{k}',\mathbf{k}-\mathbf{k}',\omega-\omega'}^{\text{ind},(3)} - \epsilon_{\mathbf{q}+\frac{1}{2}\mathbf{k}',\mathbf{k}-\mathbf{k}',\omega-\omega'} + \hbar\omega'' + \hbar\omega'''}{\hbar(\omega - \omega' - \omega'' - \omega''') + \hbar\omega' + \hbar\omega'' + \hbar\omega'''} - \epsilon_{\mathbf{q}+\frac{1}{2}\mathbf{k}',\mathbf{k}-\mathbf{k}',\omega-\omega'} + \hbar\omega'' + \hbar\omega'''} + \epsilon_{\mathbf{q}-\frac{1}{2}\mathbf{k}',\mathbf{k}-\mathbf{k}',\omega-\omega'} - \hbar\omega'' - \hbar\omega'''} \right] U_{\mathbf{k}',\omega'}^{\text{ext}} \Rightarrow \\
f_{\mathbf{q},\mathbf{k},\omega}^{\text{ind},(4)} &= - \int \frac{d\omega' d^3 k'}{(2\pi)^4} \left[ \frac{f_{\mathbf{q}+\frac{1}{2}\mathbf{k}',\mathbf{k}-\mathbf{k}',\omega-\omega'}^{\text{ind},(3)} - \epsilon_{\mathbf{q}+\frac{1}{2}\mathbf{k}',\mathbf{k}-\mathbf{k}',\omega-\omega'} + \hbar\omega'' + \hbar\omega'''}{\hbar(\omega - \omega' - \omega'' - \omega''') + \hbar\omega' + \hbar\omega'' + \hbar\omega'''} - \epsilon_{\mathbf{q}+\frac{1}{2}\mathbf{k}',\mathbf{k}-\mathbf{k}',\omega-\omega'} + \hbar\omega'' + \hbar\omega'''} + \epsilon_{\mathbf{q}-\frac{1}{2}\mathbf{k}',\mathbf{k}-\mathbf{k}',\omega-\omega'} - \hbar\omega'' - \hbar\omega'''} \right] U_{\mathbf{k}',\omega'}^{\text{ext}} \\
&\quad + \int \frac{d\omega' d^3 k'}{(2\pi)^4} \left[ \frac{f_{\mathbf{q}-\frac{1}{2}\mathbf{k}',\mathbf{k}-\mathbf{k}',\omega-\omega'}^{\text{ind},(3)} - \epsilon_{\mathbf{q}-\frac{1}{2}\mathbf{k}',\mathbf{k}-\mathbf{k}',\omega-\omega'} + \hbar\omega'' + \hbar\omega'''}{\hbar(\omega - \omega' - \omega'' - \omega''') + \hbar\omega' + \hbar\omega'' + \hbar\omega'''} - \epsilon_{\mathbf{q}-\frac{1}{2}\mathbf{k}',\mathbf{k}-\mathbf{k}',\omega-\omega'} + \hbar\omega'' + \hbar\omega'''} + \epsilon_{\mathbf{q}+\frac{1}{2}\mathbf{k}',\mathbf{k}-\mathbf{k}',\omega-\omega'} - \hbar\omega'' - \hbar\omega'''} \right] U_{\mathbf{k}',\omega'}^{\text{ext}} \Rightarrow \\
f_{\mathbf{q},\mathbf{k},\omega}^{\text{ind},(4)} &= - \int \frac{d\omega' d^3 k'}{(2\pi)^4} \left[ \frac{1}{\hbar(\omega - \omega' - \omega'' - \omega''') + \hbar\omega' + \hbar\omega'' + \hbar\omega'''} - \epsilon_{\mathbf{q}+\frac{1}{2}\mathbf{k}',\mathbf{k}-\mathbf{k}',\omega-\omega'} + \hbar\omega'' + \hbar\omega'''} + \epsilon_{\mathbf{q}-\frac{1}{2}\mathbf{k}',\mathbf{k}-\mathbf{k}',\omega-\omega'} - \hbar\omega'' - \hbar\omega'''} \right] U_{\mathbf{k}',\omega'}^{\text{ind},(3)} \\
&\quad + \int \frac{d\omega' d^3 k'}{(2\pi)^4} \left[ \frac{1}{\hbar(\omega - \omega' - \omega'' - \omega''') + \hbar\omega' + \hbar\omega'' + \hbar\omega'''} - \epsilon_{\mathbf{q}+\frac{1}{2}\mathbf{k}',\mathbf{k}-\mathbf{k}',\omega-\omega'} + \hbar\omega'' + \hbar\omega'''} + \epsilon_{\mathbf{q}-\frac{1}{2}\mathbf{k}',\mathbf{k}-\mathbf{k}',\omega-\omega'} - \hbar\omega'' - \hbar\omega'''} \right] U_{\mathbf{k}',\omega'}^{\text{ind},(3)}
\end{aligned}$$

We are now in the position to substitute  $f_{\mathbf{q},\mathbf{k},\omega}^{\text{ind},(3)}$  into  $f_{\mathbf{q},\mathbf{k},\omega}^{\text{ind},(4)}$ . The calculation proceeds with the integration of the fourth order non-interacting distribution function perturbation over the momentum space which yields the fourth order density perturbation,  $n_{\text{ind}}^{(4)}(\mathbf{k}, \omega) = 2 \int [d^3 q / (2\pi)^3] f_{\mathbf{q},\mathbf{k},\omega}^{\text{ind},(4)}$ , also in the non-interacting case. The  $n_{\text{ind}}^{(4)}(\mathbf{k}, \omega)$  expression is automatically written in a manner that, after the term by term correspondence with the general approximation-free definition of the fourth order density response  $\mathcal{W}_{\mathbf{k}_1,\omega_1;\mathbf{k}_2,\omega_2;\mathbf{k}_3,\omega_3;\mathbf{k}_4,\omega_4}^{(4)}$

$$n_{\text{ind}}^{(4)}(\mathbf{k}, \omega) = \int \frac{d^3 k' d\omega' d^3 k'' d\omega'' d^3 k''' d\omega'''}{(2\pi)^4 (2\pi)^4 (2\pi)^4} \mathcal{W}_{\mathbf{k}-\mathbf{k}',\mathbf{k}-\mathbf{k}',\mathbf{k}-\mathbf{k}',\mathbf{k}-\mathbf{k}',\mathbf{k}-\mathbf{k}',\mathbf{k}-\mathbf{k}',\mathbf{k}-\mathbf{k}',\mathbf{k}-\mathbf{k}'}^{\text{ind},(4)}$$

it is possible to directly identify the fourth order ideal density response  $\mathcal{W}_{\mathbf{k}_1,\omega_1;\mathbf{k}_2,\omega_2;\mathbf{k}_3,\omega_3;\mathbf{k}_4,\omega_4}^{(4),0}$ . It is particularly convenient to set  $\mathbf{k}_1 = \mathbf{k} - \mathbf{k}' - \mathbf{k}'' - \mathbf{k}'''$ ,  $\mathbf{k}_2 = \mathbf{k}'$ ,  $\mathbf{k}_3 = \mathbf{k}''$ ,  $\mathbf{k}_4 = \mathbf{k}'''$ ,  $\omega_1 = \omega - \omega' - \omega'' - \omega'''$ ,  $\omega_2 = \omega'$ ,  $\omega_3 = \omega''$ ,  $\omega_4 = \omega'''$ . It is also beneficial to define the analytic continuation of the fourth order ideal density response to the complex planes of the four frequencies by setting  $z_1 = \omega_1 + i0$ ,  $z_2 = \omega_2 + i0$ ,  $z_3 = \omega_3 + i0$ ,  $z_4 = \omega_4 + i0$ . The calculation proceeds with the separation of the fourth order ideal density response to the sixteen independent integrals that involve quadruple products of the non-interacting Green's function. The calculation finishes by making the change of variables  $\mathbf{q}' = \mathbf{q} + \frac{1}{2}\mathbf{k}_1 + \frac{1}{2}\mathbf{k}_2 + \frac{1}{2}\mathbf{k}_3 + \frac{1}{2}\mathbf{k}_4$ ,  $\mathbf{q}' = \mathbf{q} + \frac{1}{2}\mathbf{k}_1 + \frac{1}{2}\mathbf{k}_2 + \frac{1}{2}\mathbf{k}_3 + \frac{1}{2}\mathbf{k}_4$ ,  $\mathbf{q}' = \mathbf{q} + \frac{1}{2}\mathbf{k}_1 + \frac{1}{2}\mathbf{k}_2 + \frac{1}{2}\mathbf{k}_3 + \frac{1}{2}\mathbf{k}_4$ ,  $\mathbf{q}' = \mathbf{q} + \frac{1}{2}\mathbf{k}_1 + \frac{1}{2}\mathbf{k}_2 + \frac{1}{2}\mathbf{k}_3 + \frac{1}{2}\mathbf{k}_4$ ,  $\mathbf{q}' = \mathbf{q} + \frac{1}{2}\mathbf{k}_1 + \frac{1}{2}\mathbf{k}_2 + \frac{1}{2}\mathbf{k}_3 + \frac{1}{2}\mathbf{k}_4$ ,  $\mathbf{q}' = \mathbf{q} + \frac{1}{2}\mathbf{k}_1 + \frac{1}{2}\mathbf{k}_2 + \frac{1}{2}\mathbf{k}_3 + \frac{1}{2}\mathbf{k}_4$ ,  $\mathbf{q}' = \mathbf{q} + \frac{1}{2}\mathbf{k}_1 + \frac{1}{2}\mathbf{k}_2 + \frac{1}{2}\mathbf{k}_3 + \frac{1}{2}\mathbf{k}_4$ ,  $\mathbf{q}' = \mathbf{q} + \frac{1}{2}\mathbf{k}_1 + \frac{1}{2}\mathbf{k}_2 + \frac{1}{2}\mathbf{k}_3 + \frac{1}{2}\mathbf{k}_4$ , at each of the sixteen integrals respectively in order to unify the argument of the equilibrium distribution function. Finally, one reverts back to the original dummy variable by setting  $\mathbf{q}' \rightarrow \mathbf{q}$  in all the integrals.



[illegible]

[illegible]



[illegible]















**The compact form of the symmetric expression.** The calculation proceeds with the separate evaluation of each of the 16 contributing integrals. For convenience, in what follows, these contributing integrals have been labelled as  $\left[\chi_0^{(4,4)}(\mathbf{k}, z)\right]_1, \left[\chi_0^{(4,4)}(\mathbf{k}, z)\right]_2, \left[\chi_0^{(4,4)}(\mathbf{k}, z)\right]_3, \left[\chi_0^{(4,4)}(\mathbf{k}, z)\right]_4, \left[\chi_0^{(4,4)}(\mathbf{k}, z)\right]_5, \left[\chi_0^{(4,4)}(\mathbf{k}, z)\right]_6, \left[\chi_0^{(4,4)}(\mathbf{k}, z)\right]_7, \left[\chi_0^{(4,4)}(\mathbf{k}, z)\right]_8, \left[\chi_0^{(4,4)}(\mathbf{k}, z)\right]_9, \left[\chi_0^{(4,4)}(\mathbf{k}, z)\right]_{10}, \left[\chi_0^{(4,4)}(\mathbf{k}, z)\right]_{11}, \left[\chi_0^{(4,4)}(\mathbf{k}, z)\right]_{12}, \left[\chi_0^{(4,4)}(\mathbf{k}, z)\right]_{13}, \left[\chi_0^{(4,4)}(\mathbf{k}, z)\right]_{14}, \left[\chi_0^{(4,4)}(\mathbf{k}, z)\right]_{15}, \left[\chi_0^{(4,4)}(\mathbf{k}, z)\right]_{16}$ . The calculation is based on splitting the integrands into simple fractions and is facilitated by the fact that the multiplication coefficient of the decomposition always turns out to be independent of the integration variable  $q$ . For the purposes of the partial fraction decomposition, it is convenient to consider the fractions as functions of the variable  $\hbar z$ . The fractions of the integrands within the contributions  $\left[\chi_0^{(4,4)}(\mathbf{k}, z)\right]_1, \left[\chi_0^{(4,4)}(\mathbf{k}, z)\right]_2, \left[\chi_0^{(4,4)}(\mathbf{k}, z)\right]_{15}, \left[\chi_0^{(4,4)}(\mathbf{k}, z)\right]_{16}$ , have four simple real poles. It is straightforward to demonstrate by solving the emerging  $4 \times 4$  set of equations that their partial fraction decomposition follows

$$\frac{1}{(x-a)(x-b)(x-c)(x-d)} = \frac{1}{(a-b)(a-c)(a-d)(x-a)} - \frac{1}{(a-b)(b-c)(b-d)(x-b)} + \frac{1}{(a-c)(b-c)(c-d)(x-c)} - \frac{1}{(a-d)(b-d)(c-d)(x-d)}.$$

The fractions of the integrands within the contributions  $\left[\chi_0^{(4,4)}(\mathbf{k}, z)\right]_5, \left[\chi_0^{(4,4)}(\mathbf{k}, z)\right]_6, \left[\chi_0^{(4,4)}(\mathbf{k}, z)\right]_{11}, \left[\chi_0^{(4,4)}(\mathbf{k}, z)\right]_{12}$ , have two double real poles. This only becomes apparent when utilizing the algebraic identities  $(\epsilon_{\mathbf{q}+\mathbf{k}} - \epsilon_{\mathbf{q}-3\mathbf{k}})/4 = (\epsilon_{\mathbf{q}} - \epsilon_{\mathbf{q}-2\mathbf{k}})/2$ ,  $(\epsilon_{\mathbf{q}+\mathbf{k}} - \epsilon_{\mathbf{q}-2\mathbf{k}})/3 = \epsilon_{\mathbf{q}} - \epsilon_{\mathbf{q}-\mathbf{k}}$  for  $\left[\chi_0^{(4,4)}(\mathbf{k}, z)\right]_5$ , the algebraic identities  $(\epsilon_{\mathbf{q}+2\mathbf{k}} - \epsilon_{\mathbf{q}-2\mathbf{k}})/4 = (\epsilon_{\mathbf{q}+\mathbf{k}} - \epsilon_{\mathbf{q}-\mathbf{k}})/2$ ,  $(\epsilon_{\mathbf{q}+2\mathbf{k}} - \epsilon_{\mathbf{q}-\mathbf{k}})/3 = \epsilon_{\mathbf{q}+\mathbf{k}} - \epsilon_{\mathbf{q}}$  for  $\left[\chi_0^{(4,4)}(\mathbf{k}, z)\right]_6$ , the algebraic identities  $(\epsilon_{\mathbf{q}+2\mathbf{k}} - \epsilon_{\mathbf{q}-2\mathbf{k}})/4 = (\epsilon_{\mathbf{q}+\mathbf{k}} - \epsilon_{\mathbf{q}-\mathbf{k}})/2$ ,  $(\epsilon_{\mathbf{q}+\mathbf{k}} - \epsilon_{\mathbf{q}-2\mathbf{k}})/3 = \epsilon_{\mathbf{q}} - \epsilon_{\mathbf{q}-\mathbf{k}}$  for  $\left[\chi_0^{(4,4)}(\mathbf{k}, z)\right]_{11}$ , and the algebraic identities  $(\epsilon_{\mathbf{q}+3\mathbf{k}} - \epsilon_{\mathbf{q}-\mathbf{k}})/4 = (\epsilon_{\mathbf{q}+2\mathbf{k}} - \epsilon_{\mathbf{q}})/2$ ,  $(\epsilon_{\mathbf{q}+2\mathbf{k}} - \epsilon_{\mathbf{q}-\mathbf{k}})/3 = \epsilon_{\mathbf{q}+\mathbf{k}} - \epsilon_{\mathbf{q}}$  for  $\left[\chi_0^{(4,4)}(\mathbf{k}, z)\right]_{12}$ . It is straightforward to demonstrate by solving the emerging  $4 \times 4$  set of equations that their partial fraction decomposition follows

$$\frac{1}{(x-a)^2(x-b)^2} = \frac{1}{(a-b)^3} \left[ \frac{2}{x-b} - \frac{2}{x-a} + \frac{a-b}{(x-b)^2} + \frac{a-b}{(x-a)^2} \right].$$

The fractions of the integrands within the contributions  $\left[\chi_0^{(4,4)}(\mathbf{k}, z)\right]_3, \left[\chi_0^{(4,4)}(\mathbf{k}, z)\right]_4, \left[\chi_0^{(4,4)}(\mathbf{k}, z)\right]_7, \left[\chi_0^{(4,4)}(\mathbf{k}, z)\right]_8, \left[\chi_0^{(4,4)}(\mathbf{k}, z)\right]_9, \left[\chi_0^{(4,4)}(\mathbf{k}, z)\right]_{10}, \left[\chi_0^{(4,4)}(\mathbf{k}, z)\right]_{13}, \left[\chi_0^{(4,4)}(\mathbf{k}, z)\right]_{14}$ , have two simple real poles and one double real pole. This only becomes apparent when utilizing the algebraic identities  $(\epsilon_{\mathbf{q}+\mathbf{k}} - \epsilon_{\mathbf{q}-2\mathbf{k}})/3 = \epsilon_{\mathbf{q}} - \epsilon_{\mathbf{q}-\mathbf{k}}$  for  $\left[\chi_0^{(4,4)}(\mathbf{k}, z)\right]_3$ ,  $(\epsilon_{\mathbf{q}+2\mathbf{k}} - \epsilon_{\mathbf{q}-\mathbf{k}})/3 = \epsilon_{\mathbf{q}+\mathbf{k}} - \epsilon_{\mathbf{q}}$  for  $\left[\chi_0^{(4,4)}(\mathbf{k}, z)\right]_4$ ,  $(\epsilon_{\mathbf{q}+2\mathbf{k}} - \epsilon_{\mathbf{q}-2\mathbf{k}})/4 = (\epsilon_{\mathbf{q}+\mathbf{k}} - \epsilon_{\mathbf{q}-\mathbf{k}})/2$  for  $\left[\chi_0^{(4,4)}(\mathbf{k}, z)\right]_7$ ,  $(\epsilon_{\mathbf{q}+3\mathbf{k}} - \epsilon_{\mathbf{q}-\mathbf{k}})/4 = (\epsilon_{\mathbf{q}+2\mathbf{k}} - \epsilon_{\mathbf{q}})/2$  for  $\left[\chi_0^{(4,4)}(\mathbf{k}, z)\right]_8$ ,  $(\epsilon_{\mathbf{q}+\mathbf{k}} - \epsilon_{\mathbf{q}-3\mathbf{k}})/4 = (\epsilon_{\mathbf{q}} - \epsilon_{\mathbf{q}-2\mathbf{k}})/2$  for  $\left[\chi_0^{(4,4)}(\mathbf{k}, z)\right]_9$ ,  $(\epsilon_{\mathbf{q}+2\mathbf{k}} - \epsilon_{\mathbf{q}-2\mathbf{k}})/4 = (\epsilon_{\mathbf{q}+\mathbf{k}} - \epsilon_{\mathbf{q}-\mathbf{k}})/2$  for  $\left[\chi_0^{(4,4)}(\mathbf{k}, z)\right]_{10}$ ,  $(\epsilon_{\mathbf{q}+\mathbf{k}} - \epsilon_{\mathbf{q}-2\mathbf{k}})/3 = \epsilon_{\mathbf{q}} - \epsilon_{\mathbf{q}-\mathbf{k}}$  for  $\left[\chi_0^{(4,4)}(\mathbf{k}, z)\right]_{13}$ ,  $(\epsilon_{\mathbf{q}+2\mathbf{k}} - \epsilon_{\mathbf{q}-\mathbf{k}})/3 = \epsilon_{\mathbf{q}+\mathbf{k}} - \epsilon_{\mathbf{q}}$  for  $\left[\chi_0^{(4,4)}(\mathbf{k}, z)\right]_{14}$ . It is straightforward to demonstrate by solving the emerging  $4 \times 4$  set of equations that their partial fraction decomposition follows

$$\frac{1}{(x-a)(x-b)(x-c)^2} = \frac{1}{(a-b)(a-c)^2(x-a)} - \frac{1}{(a-b)(b-c)^2(x-b)} + \frac{a+b-2c}{(a-c)^2(b-c)^2(x-c)} + \frac{1}{(a-c)(b-c)(x-c)^2}.$$

It is worth pointing out that for all the eight latter contributions we have  $a+b-2c=0$  and, thus, this leads to

$$\frac{1}{(x-a)(x-b)(x-c)^2} = \frac{1}{(a-b)(a-c)^2(x-a)} - \frac{1}{(a-b)(b-c)^2(x-b)} + \frac{1}{(a-c)(b-c)(x-c)^2}.$$

Given the above, there are  $4 \times 4 = 16$  terms from the first group of contributions,  $4 \times 4 = 16$  terms from the second group of contributions and  $8 \times 3 = 24$  terms from the third group of contributions. These translates to  $16+16+24 = 56$  terms that constitute the ideal fourth order density response  $\chi_0^{(4,4)}(\mathbf{k}, z)$ .

The *first contribution* is characterized by four simple poles. We first identify and calculate the coefficients  $a, b, c, d$ .

$$\begin{aligned}
\left[\chi_0^{(4,4)}(\mathbf{k}, z)\right]_1 &= + \int \frac{d^3q}{(2\pi)^3} \frac{2f_0(\mathbf{q})}{(4\hbar z - \epsilon_{\mathbf{q}} + \epsilon_{\mathbf{q}-4\mathbf{k}})(3\hbar z - \epsilon_{\mathbf{q}} + \epsilon_{\mathbf{q}-3\mathbf{k}})(2\hbar z - \epsilon_{\mathbf{q}} + \epsilon_{\mathbf{q}-2\mathbf{k}})(\hbar z - \epsilon_{\mathbf{q}} + \epsilon_{\mathbf{q}-\mathbf{k}})} \Rightarrow \\
\left[\chi_0^{(4,4)}(\mathbf{k}, z)\right]_1 &= + \int \frac{d^3q}{(2\pi)^3} \frac{f_0(\mathbf{q})}{12} \frac{1}{\left[\hbar z - \frac{\epsilon_{\mathbf{q}} - \epsilon_{\mathbf{q}-4\mathbf{k}}}{4}\right] \left[\hbar z - \frac{\epsilon_{\mathbf{q}} - \epsilon_{\mathbf{q}-3\mathbf{k}}}{3}\right] \left[\hbar z - \frac{\epsilon_{\mathbf{q}} - \epsilon_{\mathbf{q}-2\mathbf{k}}}{2}\right] [\hbar z - (\epsilon_{\mathbf{q}} - \epsilon_{\mathbf{q}-\mathbf{k}})]} \Rightarrow \\
a &= \frac{\epsilon_{\mathbf{q}} - \epsilon_{\mathbf{q}-4\mathbf{k}}}{4} = \frac{\hbar^2}{2m} \frac{q^2 - (\mathbf{q} - 4\mathbf{k})^2}{4} = \frac{\hbar^2}{2m} \frac{-16k^2 + 8\mathbf{q} \cdot \mathbf{k}}{4} = \frac{\hbar^2}{2m} (-4k^2 + 2\mathbf{q} \cdot \mathbf{k}), \\
b &= \frac{\epsilon_{\mathbf{q}} - \epsilon_{\mathbf{q}-3\mathbf{k}}}{3} = \frac{\hbar^2}{2m} \frac{q^2 - (\mathbf{q} - 3\mathbf{k})^2}{3} = \frac{\hbar^2}{2m} \frac{-9k^2 + 6\mathbf{q} \cdot \mathbf{k}}{3} = \frac{\hbar^2}{2m} (-3k^2 + 2\mathbf{q} \cdot \mathbf{k}), \\
c &= \frac{\epsilon_{\mathbf{q}} - \epsilon_{\mathbf{q}-2\mathbf{k}}}{2} = \frac{\hbar^2}{2m} \frac{q^2 - (\mathbf{q} - 2\mathbf{k})^2}{2} = \frac{\hbar^2}{2m} \frac{-4k^2 + 4\mathbf{q} \cdot \mathbf{k}}{2} = \frac{\hbar^2}{2m} (-2k^2 + 2\mathbf{q} \cdot \mathbf{k}), \\
d &= \epsilon_{\mathbf{q}} - \epsilon_{\mathbf{q}-\mathbf{k}} = \frac{\hbar^2}{2m} [q^2 - (\mathbf{q} - \mathbf{k})^2] = \frac{\hbar^2}{2m} (-k^2 + 2\mathbf{q} \cdot \mathbf{k}).
\end{aligned}$$

Then, we compute all the possible differences between these four coefficients. Note that  $q^2$  and  $\mathbf{q} \cdot \mathbf{k}$  terms vanish.

$$\begin{aligned}
a - b &= \frac{\hbar^2}{2m} (-4k^2 + 2\mathbf{q} \cdot \mathbf{k} + 3k^2 - 2\mathbf{q} \cdot \mathbf{k}) = \frac{\hbar^2}{2m} (-4k^2 + 3k^2) = \frac{\hbar^2}{2m} (-k^2), \\
b - c &= \frac{\hbar^2}{2m} (-3k^2 + 2\mathbf{q} \cdot \mathbf{k} + 2k^2 - 2\mathbf{q} \cdot \mathbf{k}) = \frac{\hbar^2}{2m} (-3k^2 + 2k^2) = \frac{\hbar^2}{2m} (-k^2), \\
c - d &= \frac{\hbar^2}{2m} (-2k^2 + 2\mathbf{q} \cdot \mathbf{k} + k^2 - 2\mathbf{q} \cdot \mathbf{k}) = \frac{\hbar^2}{2m} (-2k^2 + k^2) = \frac{\hbar^2}{2m} (-k^2), \\
a - c &= \frac{\hbar^2}{2m} (-4k^2 + 2\mathbf{q} \cdot \mathbf{k} + 2k^2 - 2\mathbf{q} \cdot \mathbf{k}) = \frac{\hbar^2}{2m} (-4k^2 + 2k^2) = \frac{\hbar^2}{2m} (-2k^2), \\
a - d &= \frac{\hbar^2}{2m} (-4k^2 + 2\mathbf{q} \cdot \mathbf{k} + k^2 - 2\mathbf{q} \cdot \mathbf{k}) = \frac{\hbar^2}{2m} (-4k^2 + k^2) = \frac{\hbar^2}{2m} (-3k^2), \\
b - d &= \frac{\hbar^2}{2m} (-3k^2 + 2\mathbf{q} \cdot \mathbf{k} + k^2 - 2\mathbf{q} \cdot \mathbf{k}) = \frac{\hbar^2}{2m} (-3k^2 + k^2) = \frac{\hbar^2}{2m} (-2k^2).
\end{aligned}$$

Afterwards, we compute all the triple difference combinations that are present in the partial fraction decomposition.

$$\begin{aligned}
(a - b)(a - c)(a - d) &= \frac{\hbar^2}{2m} (-k^2) \frac{\hbar^2}{2m} (-2k^2) \frac{\hbar^2}{2m} (-3k^2) = - \left(\frac{\hbar^2}{2m}\right)^3 (k^2)(2k^2)(3k^2) = - \left(\frac{\hbar^2}{2m}\right)^3 (6k^6), \\
(a - b)(b - c)(b - d) &= \frac{\hbar^2}{2m} (-k^2) \frac{\hbar^2}{2m} (-k^2) \frac{\hbar^2}{2m} (-2k^2) = - \left(\frac{\hbar^2}{2m}\right)^3 (k^2)(k^2)(2k^2) = - \left(\frac{\hbar^2}{2m}\right)^3 (2k^6), \\
(a - c)(b - c)(c - d) &= \frac{\hbar^2}{2m} (-2k^2) \frac{\hbar^2}{2m} (-k^2) \frac{\hbar^2}{2m} (-k^2) = - \left(\frac{\hbar^2}{2m}\right)^3 (2k^2)(k^2)(k^2) = - \left(\frac{\hbar^2}{2m}\right)^3 (2k^6), \\
(a - d)(b - d)(c - d) &= \frac{\hbar^2}{2m} (-3k^2) \frac{\hbar^2}{2m} (-2k^2) \frac{\hbar^2}{2m} (-k^2) = - \left(\frac{\hbar^2}{2m}\right)^3 (3k^2)(2k^2)(k^2) = - \left(\frac{\hbar^2}{2m}\right)^3 (6k^6).
\end{aligned}$$

Finally, we substitute the above in the contribution and perform some straightforward algebra.

$$\begin{aligned}
\left[\chi_0^{(4,4)}(\mathbf{k}, z)\right]_1 &= - \int \frac{d^3q}{(2\pi)^3} \left(\frac{2m}{\hbar^2}\right)^3 \frac{f_0(\mathbf{q})}{12} \frac{1}{6k^6} \left[ \frac{1}{\hbar z - \frac{\epsilon_{\mathbf{q}} - \epsilon_{\mathbf{q}-4\mathbf{k}}}{4}} - \frac{3}{\hbar z - \frac{\epsilon_{\mathbf{q}} - \epsilon_{\mathbf{q}-3\mathbf{k}}}{3}} + \frac{3}{\hbar z - \frac{\epsilon_{\mathbf{q}} - \epsilon_{\mathbf{q}-2\mathbf{k}}}{2}} - \frac{1}{\hbar z - \epsilon_{\mathbf{q}} + \epsilon_{\mathbf{q}-\mathbf{k}}} \right] \Rightarrow \\
\left[\chi_0^{(4,4)}(\mathbf{k}, z)\right]_1 &= - \int \frac{d^3q}{(2\pi)^3} \left(\frac{m}{\hbar^2}\right)^3 \frac{2f_0(\mathbf{q})}{18} \frac{1}{k^6} \left[ \frac{1}{\hbar z - \frac{\epsilon_{\mathbf{q}} - \epsilon_{\mathbf{q}-4\mathbf{k}}}{4}} - \frac{3}{\hbar z - \frac{\epsilon_{\mathbf{q}} - \epsilon_{\mathbf{q}-3\mathbf{k}}}{3}} + \frac{3}{\hbar z - \frac{\epsilon_{\mathbf{q}} - \epsilon_{\mathbf{q}-2\mathbf{k}}}{2}} - \frac{1}{\hbar z - \epsilon_{\mathbf{q}} + \epsilon_{\mathbf{q}-\mathbf{k}}} \right] \Rightarrow \\
\left[\chi_0^{(4,4)}(\mathbf{k}, z)\right]_1 &= - \left(\frac{m}{\hbar^2}\right)^3 \frac{1}{18k^6} \int \frac{d^3q}{(2\pi)^3} 2f_0(\mathbf{q}) \left[ \frac{1}{\hbar z - \frac{\epsilon_{\mathbf{q}} - \epsilon_{\mathbf{q}-4\mathbf{k}}}{4}} - \frac{3}{\hbar z - \frac{\epsilon_{\mathbf{q}} - \epsilon_{\mathbf{q}-3\mathbf{k}}}{3}} + \frac{3}{\hbar z - \frac{\epsilon_{\mathbf{q}} - \epsilon_{\mathbf{q}-2\mathbf{k}}}{2}} - \frac{1}{\hbar z - \epsilon_{\mathbf{q}} + \epsilon_{\mathbf{q}-\mathbf{k}}} \right] \Rightarrow \\
\left[\chi_0^{(4,4)}(\mathbf{k}, z)\right]_1 &= - \left(\frac{m}{\hbar^2}\right)^3 \frac{1}{18k^6} \int \frac{d^3q}{(2\pi)^3} 2f_0(\mathbf{q}) \left[ \frac{4}{4\hbar z - \epsilon_{\mathbf{q}} + \epsilon_{\mathbf{q}-4\mathbf{k}}} - \frac{9}{3\hbar z - \epsilon_{\mathbf{q}} + \epsilon_{\mathbf{q}-3\mathbf{k}}} + \frac{6}{2\hbar z - \epsilon_{\mathbf{q}} + \epsilon_{\mathbf{q}-2\mathbf{k}}} - \frac{1}{\hbar z - \epsilon_{\mathbf{q}} + \epsilon_{\mathbf{q}-\mathbf{k}}} \right]
\end{aligned}$$

The *second contribution* is characterized by four simple poles. We first identify and calculate the coefficients  $a, b, c, d$ .

$$\begin{aligned}
\left[\chi_0^{(4,4)}(\mathbf{k}, z)\right]_2 &= - \int \frac{d^3q}{(2\pi)^3} \frac{2f_0(\mathbf{q})}{(4\hbar z - \epsilon_{\mathbf{q}+\mathbf{k}} + \epsilon_{\mathbf{q}-3\mathbf{k}})(3\hbar z - \epsilon_{\mathbf{q}+\mathbf{k}} + \epsilon_{\mathbf{q}-2\mathbf{k}})(2\hbar z - \epsilon_{\mathbf{q}+\mathbf{k}} + \epsilon_{\mathbf{q}-\mathbf{k}})(\hbar z - \epsilon_{\mathbf{q}+\mathbf{k}} + \epsilon_{\mathbf{q}})} \Rightarrow \\
\left[\chi_0^{(4,4)}(\mathbf{k}, z)\right]_2 &= - \int \frac{d^3q}{(2\pi)^3} \frac{f_0(\mathbf{q})}{12} \frac{1}{\left[\hbar z - \frac{\epsilon_{\mathbf{q}+\mathbf{k}} - \epsilon_{\mathbf{q}-3\mathbf{k}}}{4}\right] \left[\hbar z - \frac{\epsilon_{\mathbf{q}+\mathbf{k}} - \epsilon_{\mathbf{q}-2\mathbf{k}}}{3}\right] \left[\hbar z - \frac{\epsilon_{\mathbf{q}+\mathbf{k}} - \epsilon_{\mathbf{q}-\mathbf{k}}}{2}\right] [\hbar z - (\epsilon_{\mathbf{q}+\mathbf{k}} - \epsilon_{\mathbf{q}})]} \Rightarrow \\
a = \frac{\epsilon_{\mathbf{q}+\mathbf{k}} - \epsilon_{\mathbf{q}-3\mathbf{k}}}{4} &= \frac{\hbar^2}{2m} \frac{(\mathbf{q} + \mathbf{k})^2 - (\mathbf{q} - 3\mathbf{k})^2}{4} = \frac{\hbar^2}{2m} \frac{k^2 + 2\mathbf{q} \cdot \mathbf{k} - 9k^2 + 6\mathbf{q} \cdot \mathbf{k}}{4} = \frac{\hbar^2}{2m} \frac{-8k^2 + 8\mathbf{q} \cdot \mathbf{k}}{4} = \frac{\hbar^2}{2m} (-2k^2 + 2\mathbf{q} \cdot \mathbf{k}) , \\
b = \frac{\epsilon_{\mathbf{q}+\mathbf{k}} - \epsilon_{\mathbf{q}-2\mathbf{k}}}{3} &= \frac{\hbar^2}{2m} \frac{(\mathbf{q} + \mathbf{k})^2 - (\mathbf{q} - 2\mathbf{k})^2}{3} = \frac{\hbar^2}{2m} \frac{k^2 + 2\mathbf{q} \cdot \mathbf{k} - 4k^2 + 4\mathbf{q} \cdot \mathbf{k}}{3} = \frac{\hbar^2}{2m} \frac{-3k^2 + 6\mathbf{q} \cdot \mathbf{k}}{3} = \frac{\hbar^2}{2m} (-k^2 + 2\mathbf{q} \cdot \mathbf{k}) , \\
c = \frac{\epsilon_{\mathbf{q}+\mathbf{k}} - \epsilon_{\mathbf{q}-\mathbf{k}}}{2} &= \frac{\hbar^2}{2m} \frac{(\mathbf{q} + \mathbf{k})^2 - (\mathbf{q} - \mathbf{k})^2}{2} = \frac{\hbar^2}{2m} \frac{k^2 + 2\mathbf{q} \cdot \mathbf{k} - k^2 + 2\mathbf{q} \cdot \mathbf{k}}{2} = \frac{\hbar^2}{2m} \frac{4\mathbf{q} \cdot \mathbf{k}}{2} = \frac{\hbar^2}{2m} (2\mathbf{q} \cdot \mathbf{k}) , \\
d = \epsilon_{\mathbf{q}+\mathbf{k}} - \epsilon_{\mathbf{q}} &= \frac{\hbar^2}{2m} [(\mathbf{q} + \mathbf{k})^2 - q^2] = \frac{\hbar^2}{2m} (k^2 + 2\mathbf{q} \cdot \mathbf{k}) .
\end{aligned}$$

Then, we compute all the possible differences between these four coefficients. Note that  $q^2$  and  $\mathbf{q} \cdot \mathbf{k}$  terms vanish.

$$\begin{aligned}
a - b &= \frac{\hbar^2}{2m} (-2k^2 + 2\mathbf{q} \cdot \mathbf{k} + k^2 - 2\mathbf{q} \cdot \mathbf{k}) = \frac{\hbar^2}{2m} (-2k^2 + k^2) = \frac{\hbar^2}{2m} (-k^2) , \\
b - c &= \frac{\hbar^2}{2m} (-k^2 + 2\mathbf{q} \cdot \mathbf{k} - 2\mathbf{q} \cdot \mathbf{k}) = \frac{\hbar^2}{2m} (-k^2) , \\
c - d &= \frac{\hbar^2}{2m} (2\mathbf{q} \cdot \mathbf{k} - k^2 - 2\mathbf{q} \cdot \mathbf{k}) = \frac{\hbar^2}{2m} (-k^2) , \\
a - c &= \frac{\hbar^2}{2m} (-2k^2 + 2\mathbf{q} \cdot \mathbf{k} - 2\mathbf{q} \cdot \mathbf{k}) = \frac{\hbar^2}{2m} (-2k^2) , \\
a - d &= \frac{\hbar^2}{2m} (-2k^2 + 2\mathbf{q} \cdot \mathbf{k} - k^2 - 2\mathbf{q} \cdot \mathbf{k}) = \frac{\hbar^2}{2m} (-2k^2 - k^2) = \frac{\hbar^2}{2m} (-3k^2) , \\
b - d &= \frac{\hbar^2}{2m} (-k^2 + 2\mathbf{q} \cdot \mathbf{k} - k^2 - 2\mathbf{q} \cdot \mathbf{k}) = \frac{\hbar^2}{2m} (-k^2 - k^2) = \frac{\hbar^2}{2m} (-2k^2) .
\end{aligned}$$

Afterwards, we compute all the triple difference combinations that are present in the partial fraction decomposition.

$$\begin{aligned}
(a - b)(a - c)(a - d) &= \frac{\hbar^2}{2m} (-k^2) \frac{\hbar^2}{2m} (-2k^2) \frac{\hbar^2}{2m} (-3k^2) = - \left(\frac{\hbar^2}{2m}\right)^3 (k^2)(2k^2)(3k^2) = - \left(\frac{\hbar^2}{2m}\right)^3 (6k^6) , \\
(a - b)(b - c)(b - d) &= \frac{\hbar^2}{2m} (-k^2) \frac{\hbar^2}{2m} (-k^2) \frac{\hbar^2}{2m} (-2k^2) = - \left(\frac{\hbar^2}{2m}\right)^3 (k^2)(k^2)(2k^2) = - \left(\frac{\hbar^2}{2m}\right)^3 (2k^6) , \\
(a - c)(b - c)(c - d) &= \frac{\hbar^2}{2m} (-2k^2) \frac{\hbar^2}{2m} (-k^2) \frac{\hbar^2}{2m} (-k^2) = - \left(\frac{\hbar^2}{2m}\right)^3 (2k^2)(k^2)(k^2) = - \left(\frac{\hbar^2}{2m}\right)^3 (2k^6) , \\
(a - d)(b - d)(c - d) &= \frac{\hbar^2}{2m} (-3k^2) \frac{\hbar^2}{2m} (-2k^2) \frac{\hbar^2}{2m} (-k^2) = - \left(\frac{\hbar^2}{2m}\right)^3 (3k^2)(2k^2)(k^2) = - \left(\frac{\hbar^2}{2m}\right)^3 (6k^6) .
\end{aligned}$$

Finally, we substitute the above in the contribution and perform some straightforward algebra.

$$\begin{aligned}
\left[\chi_0^{(4,4)}(\mathbf{k}, z)\right]_2 &= + \int \frac{d^3q}{(2\pi)^3} \left(\frac{2m}{\hbar^2}\right)^3 \frac{f_0(\mathbf{q})}{12} \frac{1}{6k^6} \left[ \frac{1}{\hbar z - \frac{\epsilon_{\mathbf{q}+\mathbf{k}} - \epsilon_{\mathbf{q}-3\mathbf{k}}}{4}} - \frac{3}{\hbar z - \frac{\epsilon_{\mathbf{q}+\mathbf{k}} - \epsilon_{\mathbf{q}-2\mathbf{k}}}{3}} + \frac{3}{\hbar z - \frac{\epsilon_{\mathbf{q}+\mathbf{k}} - \epsilon_{\mathbf{q}-\mathbf{k}}}{2}} - \frac{1}{\hbar z - \epsilon_{\mathbf{q}+\mathbf{k}} + \epsilon_{\mathbf{q}}} \right] \Rightarrow \\
\left[\chi_0^{(4,4)}(\mathbf{k}, z)\right]_2 &= + \int \frac{d^3q}{(2\pi)^3} \left(\frac{m}{\hbar^2}\right)^3 \frac{2f_0(\mathbf{q})}{18} \frac{1}{k^6} \left[ \frac{1}{\hbar z - \frac{\epsilon_{\mathbf{q}+\mathbf{k}} - \epsilon_{\mathbf{q}-3\mathbf{k}}}{4}} - \frac{3}{\hbar z - \frac{\epsilon_{\mathbf{q}+\mathbf{k}} - \epsilon_{\mathbf{q}-2\mathbf{k}}}{3}} + \frac{3}{\hbar z - \frac{\epsilon_{\mathbf{q}+\mathbf{k}} - \epsilon_{\mathbf{q}-\mathbf{k}}}{2}} - \frac{1}{\hbar z - \epsilon_{\mathbf{q}+\mathbf{k}} + \epsilon_{\mathbf{q}}} \right] \Rightarrow \\
\left[\chi_0^{(4,4)}(\mathbf{k}, z)\right]_2 &= + \left(\frac{m}{\hbar^2}\right)^3 \frac{1}{18k^6} \int \frac{d^3q}{(2\pi)^3} 2f_0(\mathbf{q}) \left[ \frac{1}{\hbar z - \frac{\epsilon_{\mathbf{q}+\mathbf{k}} - \epsilon_{\mathbf{q}-3\mathbf{k}}}{4}} - \frac{3}{\hbar z - \frac{\epsilon_{\mathbf{q}+\mathbf{k}} - \epsilon_{\mathbf{q}-2\mathbf{k}}}{3}} + \frac{3}{\hbar z - \frac{\epsilon_{\mathbf{q}+\mathbf{k}} - \epsilon_{\mathbf{q}-\mathbf{k}}}{2}} - \frac{1}{\hbar z - \epsilon_{\mathbf{q}+\mathbf{k}} + \epsilon_{\mathbf{q}}} \right] \Rightarrow \\
\left[\chi_0^{(4,4)}(\mathbf{k}, z)\right]_2 &= + \left(\frac{m}{\hbar^2}\right)^3 \frac{1}{18k^6} \int \frac{d^3q}{(2\pi)^3} 2f_0(\mathbf{q}) \left[ \frac{4}{4\hbar z - \epsilon_{\mathbf{q}+\mathbf{k}} + \epsilon_{\mathbf{q}-3\mathbf{k}}} - \frac{9}{3\hbar z - \epsilon_{\mathbf{q}+\mathbf{k}} + \epsilon_{\mathbf{q}-2\mathbf{k}}} + \frac{6}{2\hbar z - \epsilon_{\mathbf{q}+\mathbf{k}} + \epsilon_{\mathbf{q}-\mathbf{k}}} - \frac{1}{\hbar z - \epsilon_{\mathbf{q}+\mathbf{k}} + \epsilon_{\mathbf{q}}} \right] \Rightarrow
\end{aligned}$$

The *third contribution* is characterized by two simple poles and one double pole. This becomes apparrent from the algebraic identity  $(\epsilon_{\mathbf{q}+\mathbf{k}} - \epsilon_{\mathbf{q}-2\mathbf{k}})/3 = \epsilon_{\mathbf{q}} - \epsilon_{\mathbf{q}-\mathbf{k}}$ . We first identify and calculate the coefficients  $a, b, c$ .

$$\begin{aligned}
\left[\chi_0^{(4,4)}(\mathbf{k}, z)\right]_3 &= - \int \frac{d^3q}{(2\pi)^3} \frac{2f_0(\mathbf{q})}{(4\hbar z - \epsilon_{\mathbf{q}+\mathbf{k}} + \epsilon_{\mathbf{q}-3\mathbf{k}})(3\hbar z - \epsilon_{\mathbf{q}+\mathbf{k}} + \epsilon_{\mathbf{q}-2\mathbf{k}})(2\hbar z - \epsilon_{\mathbf{q}+\mathbf{k}} + \epsilon_{\mathbf{q}-\mathbf{k}})(\hbar z - \epsilon_{\mathbf{q}} + \epsilon_{\mathbf{q}-\mathbf{k}})} \Rightarrow \\
\left[\chi_0^{(4,4)}(\mathbf{k}, z)\right]_3 &= - \int \frac{d^3q}{(2\pi)^3} \frac{f_0(\mathbf{q})}{12} \frac{1}{\left[\hbar z - \frac{\epsilon_{\mathbf{q}+\mathbf{k}} - \epsilon_{\mathbf{q}-3\mathbf{k}}}{4}\right] \left[\hbar z - \frac{\epsilon_{\mathbf{q}+\mathbf{k}} - \epsilon_{\mathbf{q}-2\mathbf{k}}}{3}\right] \left[\hbar z - \frac{\epsilon_{\mathbf{q}+\mathbf{k}} - \epsilon_{\mathbf{q}-\mathbf{k}}}{2}\right] [\hbar z - (\epsilon_{\mathbf{q}} - \epsilon_{\mathbf{q}-\mathbf{k}})]} \Rightarrow \\
\left[\chi_0^{(4,4)}(\mathbf{k}, z)\right]_3 &= - \int \frac{d^3q}{(2\pi)^3} \frac{f_0(\mathbf{q})}{12} \frac{1}{\left[\hbar z - \frac{\epsilon_{\mathbf{q}+\mathbf{k}} - \epsilon_{\mathbf{q}-3\mathbf{k}}}{4}\right] [\hbar z - (\epsilon_{\mathbf{q}} - \epsilon_{\mathbf{q}-\mathbf{k}})] \left[\hbar z - \frac{\epsilon_{\mathbf{q}+\mathbf{k}} - \epsilon_{\mathbf{q}-\mathbf{k}}}{2}\right] [\hbar z - (\epsilon_{\mathbf{q}} - \epsilon_{\mathbf{q}-\mathbf{k}})]} \Rightarrow \\
\left[\chi_0^{(4,4)}(\mathbf{k}, z)\right]_3 &= - \int \frac{d^3q}{(2\pi)^3} \frac{f_0(\mathbf{q})}{12} \frac{1}{\left[\hbar z - \frac{\epsilon_{\mathbf{q}+\mathbf{k}} - \epsilon_{\mathbf{q}-3\mathbf{k}}}{4}\right] \left[\hbar z - \frac{\epsilon_{\mathbf{q}+\mathbf{k}} - \epsilon_{\mathbf{q}-\mathbf{k}}}{2}\right] [\hbar z - (\epsilon_{\mathbf{q}} - \epsilon_{\mathbf{q}-\mathbf{k}})]^2} \Rightarrow \\
a = \frac{\epsilon_{\mathbf{q}+\mathbf{k}} - \epsilon_{\mathbf{q}-3\mathbf{k}}}{4} &= \frac{\hbar^2}{2m} \frac{(\mathbf{q} + \mathbf{k})^2 - (\mathbf{q} - 3\mathbf{k})^2}{4} = \frac{\hbar^2}{2m} \frac{k^2 + 2\mathbf{q} \cdot \mathbf{k} - 9k^2 + 6\mathbf{q} \cdot \mathbf{k}}{4} = \frac{\hbar^2}{2m} \frac{-8k^2 + 8\mathbf{q} \cdot \mathbf{k}}{4} = \frac{\hbar^2}{2m} (-2k^2 + 2\mathbf{q} \cdot \mathbf{k}) , \\
b = \frac{\epsilon_{\mathbf{q}+\mathbf{k}} - \epsilon_{\mathbf{q}-\mathbf{k}}}{2} &= \frac{\hbar^2}{2m} \frac{(\mathbf{q} + \mathbf{k})^2 - (\mathbf{q} - \mathbf{k})^2}{2} = \frac{\hbar^2}{2m} \frac{k^2 + 2\mathbf{q} \cdot \mathbf{k} - k^2 + 2\mathbf{q} \cdot \mathbf{k}}{2} = \frac{\hbar^2}{2m} \frac{4\mathbf{q} \cdot \mathbf{k}}{2} = \frac{\hbar^2}{2m} (2\mathbf{q} \cdot \mathbf{k}) , \\
c = \epsilon_{\mathbf{q}} - \epsilon_{\mathbf{q}-\mathbf{k}} &= \frac{\hbar^2}{2m} [q^2 - (\mathbf{q} - \mathbf{k})^2] = \frac{\hbar^2}{2m} (-k^2 + 2\mathbf{q} \cdot \mathbf{k}) .
\end{aligned}$$

Then, we compute all the relevant differences between these three coefficients. Note that the  $q^2$  and  $\mathbf{q} \cdot \mathbf{k}$  terms vanish.

$$\begin{aligned}
a - b &= \frac{\hbar^2}{2m} (-2k^2 + 2\mathbf{q} \cdot \mathbf{k} - 2\mathbf{q} \cdot \mathbf{k}) = \frac{\hbar^2}{2m} (-2k^2) = -\frac{\hbar^2}{2m} (2k^2) , \\
a - c &= \frac{\hbar^2}{2m} (-2k^2 + 2\mathbf{q} \cdot \mathbf{k} + k^2 - 2\mathbf{q} \cdot \mathbf{k}) = \frac{\hbar^2}{2m} (-2k^2 + k^2) = \frac{\hbar^2}{2m} (-k^2) = -\frac{\hbar^2}{2m} (k^2) , \\
b - c &= \frac{\hbar^2}{2m} (2\mathbf{q} \cdot \mathbf{k} + k^2 - 2\mathbf{q} \cdot \mathbf{k}) = \frac{\hbar^2}{2m} (k^2) , \\
a + b - 2c &= \frac{\hbar^2}{2m} (-2k^2 + 2\mathbf{q} \cdot \mathbf{k} + 2\mathbf{q} \cdot \mathbf{k} + 2k^2 - 4\mathbf{q} \cdot \mathbf{k}) = \frac{\hbar^2}{2m} (-2k^2 + 2k^2) = 0 .
\end{aligned}$$

Afterwards, we compute all the algebraic combinations that are present in the partial fraction decomposition.

$$\begin{aligned}
(a - b)(a - c)^2 &= - \left(\frac{\hbar^2}{2m}\right)^3 (2k^2) (k^2)^2 = - \left(\frac{\hbar^2}{2m}\right)^3 (2k^6) , \\
(a - b)(b - c)^2 &= - \left(\frac{\hbar^2}{2m}\right)^3 (2k^2) (k^2)^2 = - \left(\frac{\hbar^2}{2m}\right)^3 (2k^6) , \\
(a - c)^2(b - c)^2 &= \left(\frac{\hbar^2}{2m}\right)^4 (k^2)^2 (k^2)^2 = \left(\frac{\hbar^2}{2m}\right)^4 (k^8) , \\
(a - c)(b - c) &= - \left(\frac{\hbar^2}{2m}\right)^2 (k^2) (k^2) = - \left(\frac{\hbar^2}{2m}\right)^2 (k^4) = - \frac{1}{2k^2} \frac{2m}{\hbar^2} \left(\frac{\hbar^2}{2m}\right)^3 (2k^6) .
\end{aligned}$$

Finally, we substitute and perform some algebra. We also introduce the compact notation  $\epsilon_{\mathbf{k}} = (\hbar^2 k^2)/(2m)$ .

$$\begin{aligned}
\left[\chi_0^{(4,4)}(\mathbf{k}, z)\right]_3 &= + \int \frac{d^3q}{(2\pi)^3} \left(\frac{2m}{\hbar^2}\right)^3 \frac{f_0(\mathbf{q})}{12} \frac{1}{2k^6} \left\{ \frac{1}{\hbar z - \frac{\epsilon_{\mathbf{q}+\mathbf{k}} - \epsilon_{\mathbf{q}-3\mathbf{k}}}{4}} - \frac{1}{\hbar z - \frac{\epsilon_{\mathbf{q}+\mathbf{k}} - \epsilon_{\mathbf{q}-\mathbf{k}}}{2}} + \frac{\hbar^2 k^2}{2m} \frac{2}{(\hbar z - \epsilon_{\mathbf{q}} + \epsilon_{\mathbf{q}-\mathbf{k}})^2} \right\} \Rightarrow \\
\left[\chi_0^{(4,4)}(\mathbf{k}, z)\right]_3 &= + \int \frac{d^3q}{(2\pi)^3} \left(\frac{2m}{\hbar^2}\right)^3 \frac{f_0(\mathbf{q})}{12} \frac{1}{2k^6} \left\{ \frac{1}{\hbar z - \frac{\epsilon_{\mathbf{q}+\mathbf{k}} - \epsilon_{\mathbf{q}-3\mathbf{k}}}{4}} - \frac{1}{\hbar z - \frac{\epsilon_{\mathbf{q}+\mathbf{k}} - \epsilon_{\mathbf{q}-\mathbf{k}}}{2}} + \frac{2\epsilon_{\mathbf{k}}}{(\hbar z - \epsilon_{\mathbf{q}} + \epsilon_{\mathbf{q}-\mathbf{k}})^2} \right\} \Rightarrow \\
\left[\chi_0^{(4,4)}(\mathbf{k}, z)\right]_3 &= + \left(\frac{m}{\hbar^2}\right)^3 \frac{1}{18k^6} \int \frac{d^3q}{(2\pi)^3} 2f_0(\mathbf{q}) \left\{ \frac{3}{\hbar z - \frac{\epsilon_{\mathbf{q}+\mathbf{k}} - \epsilon_{\mathbf{q}-3\mathbf{k}}}{4}} - \frac{3}{\hbar z - \frac{\epsilon_{\mathbf{q}+\mathbf{k}} - \epsilon_{\mathbf{q}-\mathbf{k}}}{2}} + \frac{6\epsilon_{\mathbf{k}}}{(\hbar z - \epsilon_{\mathbf{q}} + \epsilon_{\mathbf{q}-\mathbf{k}})^2} \right\} \Rightarrow \\
\left[\chi_0^{(4,4)}(\mathbf{k}, z)\right]_3 &= + \left(\frac{m}{\hbar^2}\right)^3 \frac{1}{18k^6} \int \frac{d^3q}{(2\pi)^3} 2f_0(\mathbf{q}) \left\{ \frac{12}{4\hbar z - \epsilon_{\mathbf{q}+\mathbf{k}} + \epsilon_{\mathbf{q}-3\mathbf{k}}} - \frac{6}{2\hbar z - \epsilon_{\mathbf{q}+\mathbf{k}} + \epsilon_{\mathbf{q}-\mathbf{k}}} + \frac{6\epsilon_{\mathbf{k}}}{(\hbar z - \epsilon_{\mathbf{q}} + \epsilon_{\mathbf{q}-\mathbf{k}})^2} \right\} .
\end{aligned}$$



The *fourth contribution* is characterized by two simple poles and one double pole. This becomes apparrent from the algebraic identity  $(\epsilon_{\mathbf{q}+2\mathbf{k}} - \epsilon_{\mathbf{q}-\mathbf{k}})/3 = \epsilon_{\mathbf{q}+\mathbf{k}} - \epsilon_{\mathbf{q}}$ . We first identify and calculate the coefficients  $a, b, c$ .

$$\begin{aligned}
\left[\chi_0^{(4,4)}(\mathbf{k}, z)\right]_4 &= + \int \frac{d^3q}{(2\pi)^3} \frac{2f_0(\mathbf{q})}{(4\hbar z - \epsilon_{\mathbf{q}+2\mathbf{k}} + \epsilon_{\mathbf{q}-2\mathbf{k}})(3\hbar z - \epsilon_{\mathbf{q}+2\mathbf{k}} + \epsilon_{\mathbf{q}-\mathbf{k}})(2\hbar z - \epsilon_{\mathbf{q}+2\mathbf{k}} + \epsilon_{\mathbf{q}})(\hbar z - \epsilon_{\mathbf{q}+\mathbf{k}} + \epsilon_{\mathbf{q}})} \Rightarrow \\
\left[\chi_0^{(4,4)}(\mathbf{k}, z)\right]_4 &= + \int \frac{d^3q}{(2\pi)^3} \frac{f_0(\mathbf{q})}{12} \frac{1}{\left[\hbar z - \frac{\epsilon_{\mathbf{q}+2\mathbf{k}} - \epsilon_{\mathbf{q}-2\mathbf{k}}}{4}\right] \left[\hbar z - \frac{\epsilon_{\mathbf{q}+2\mathbf{k}} - \epsilon_{\mathbf{q}-\mathbf{k}}}{3}\right] \left[\hbar z - \frac{\epsilon_{\mathbf{q}+2\mathbf{k}} - \epsilon_{\mathbf{q}}}{2}\right] [\hbar z - (\epsilon_{\mathbf{q}+\mathbf{k}} - \epsilon_{\mathbf{q}})]} \Rightarrow \\
\left[\chi_0^{(4,4)}(\mathbf{k}, z)\right]_4 &= + \int \frac{d^3q}{(2\pi)^3} \frac{f_0(\mathbf{q})}{12} \frac{1}{\left[\hbar z - \frac{\epsilon_{\mathbf{q}+2\mathbf{k}} - \epsilon_{\mathbf{q}-2\mathbf{k}}}{4}\right] [\hbar z - (\epsilon_{\mathbf{q}+\mathbf{k}} - \epsilon_{\mathbf{q}})] \left[\hbar z - \frac{\epsilon_{\mathbf{q}+2\mathbf{k}} - \epsilon_{\mathbf{q}}}{2}\right] [\hbar z - (\epsilon_{\mathbf{q}+\mathbf{k}} - \epsilon_{\mathbf{q}})]} \Rightarrow \\
\left[\chi_0^{(4,4)}(\mathbf{k}, z)\right]_4 &= + \int \frac{d^3q}{(2\pi)^3} \frac{f_0(\mathbf{q})}{12} \frac{1}{\left[\hbar z - \frac{\epsilon_{\mathbf{q}+2\mathbf{k}} - \epsilon_{\mathbf{q}-2\mathbf{k}}}{4}\right] \left[\hbar z - \frac{\epsilon_{\mathbf{q}+2\mathbf{k}} - \epsilon_{\mathbf{q}}}{2}\right] [\hbar z - (\epsilon_{\mathbf{q}+\mathbf{k}} - \epsilon_{\mathbf{q}})]^2} \Rightarrow \\
a &= \frac{\epsilon_{\mathbf{q}+2\mathbf{k}} - \epsilon_{\mathbf{q}-2\mathbf{k}}}{4} = \frac{\hbar^2}{2m} \frac{(\mathbf{q} + 2\mathbf{k})^2 - (\mathbf{q} - 2\mathbf{k})^2}{4} = \frac{\hbar^2}{2m} \frac{4k^2 + 4\mathbf{q} \cdot \mathbf{k} - 4k^2 + 4\mathbf{q} \cdot \mathbf{k}}{4} = \frac{\hbar^2}{2m} \frac{8\mathbf{q} \cdot \mathbf{k}}{4} = \frac{\hbar^2}{2m} (2\mathbf{q} \cdot \mathbf{k}) , \\
b &= \frac{\epsilon_{\mathbf{q}+2\mathbf{k}} - \epsilon_{\mathbf{q}}}{2} = \frac{\hbar^2}{2m} \frac{(\mathbf{q} + 2\mathbf{k})^2 - \mathbf{q}^2}{2} = \frac{\hbar^2}{2m} \frac{4k^2 + 4\mathbf{q} \cdot \mathbf{k}}{2} = \frac{\hbar^2}{2m} (2k^2 + 2\mathbf{q} \cdot \mathbf{k}) , \\
c &= \epsilon_{\mathbf{q}+\mathbf{k}} - \epsilon_{\mathbf{q}} = \frac{\hbar^2}{2m} [(\mathbf{q} + \mathbf{k})^2 - \mathbf{q}^2] = \frac{\hbar^2}{2m} (k^2 + 2\mathbf{q} \cdot \mathbf{k}) .
\end{aligned}$$

Then, we compute all the relevant differences between these three coefficients. Note that the  $q^2$  and  $\mathbf{q} \cdot \mathbf{k}$  terms vanish.

$$\begin{aligned}
a - b &= \frac{\hbar^2}{2m} (2\mathbf{q} \cdot \mathbf{k} - 2k^2 - 2\mathbf{q} \cdot \mathbf{k}) = \frac{\hbar^2}{2m} (-2k^2) = -\frac{\hbar^2}{2m} (2k^2) , \\
a - c &= \frac{\hbar^2}{2m} (2\mathbf{q} \cdot \mathbf{k} - k^2 - 2\mathbf{q} \cdot \mathbf{k}) = \frac{\hbar^2}{2m} (-k^2) = -\frac{\hbar^2}{2m} (k^2) , \\
b - c &= \frac{\hbar^2}{2m} (2k^2 + 2\mathbf{q} \cdot \mathbf{k} - k^2 - 2\mathbf{q} \cdot \mathbf{k}) = \frac{\hbar^2}{2m} (2k^2 - k^2) = \frac{\hbar^2}{2m} (k^2) , \\
a + b - 2c &= \frac{\hbar^2}{2m} (2\mathbf{q} \cdot \mathbf{k} + 2k^2 + 2\mathbf{q} \cdot \mathbf{k} - 2k^2 - 4\mathbf{q} \cdot \mathbf{k}) = \frac{\hbar^2}{2m} (+2k^2 - 2k^2) = 0 .
\end{aligned}$$

Afterwards, we compute all the algebraic combinations that are present in the partial fraction decomposition.

$$\begin{aligned}
(a - b)(a - c)^2 &= -\left(\frac{\hbar^2}{2m}\right)^3 (2k^2) (k^2)^2 = -\left(\frac{\hbar^2}{2m}\right)^3 (2k^6) , \\
(a - b)(b - c)^2 &= -\left(\frac{\hbar^2}{2m}\right)^3 (2k^2) (k^2)^2 = -\left(\frac{\hbar^2}{2m}\right)^3 (2k^6) , \\
(a - c)^2(b - c)^2 &= \left(\frac{\hbar^2}{2m}\right)^4 (k^2)^2 (k^2)^2 = \left(\frac{\hbar^2}{2m}\right)^4 (k^8) , \\
(a - c)(b - c) &= -\left(\frac{\hbar^2}{2m}\right)^2 (k^2) (k^2) = -\left(\frac{\hbar^2}{2m}\right)^2 (k^4) = -\frac{1}{2k^2} \frac{2m}{\hbar^2} \left(\frac{\hbar^2}{2m}\right)^3 (2k^6) .
\end{aligned}$$

Finally, we substitute and perform some algebra. We also introduce the compact notation  $\epsilon_{\mathbf{k}} = (\hbar^2 k^2)/(2m)$ .

$$\begin{aligned}
\left[\chi_0^{(4,4)}(\mathbf{k}, z)\right]_4 &= - \int \frac{d^3q}{(2\pi)^3} \left(\frac{2m}{\hbar^2}\right)^3 \frac{f_0(\mathbf{q})}{12} \frac{1}{2k^6} \left\{ \frac{1}{\hbar z - \frac{\epsilon_{\mathbf{q}+2\mathbf{k}} - \epsilon_{\mathbf{q}-2\mathbf{k}}}{4}} - \frac{1}{\hbar z - \frac{\epsilon_{\mathbf{q}+2\mathbf{k}} - \epsilon_{\mathbf{q}}}{2}} + \frac{\hbar^2 k^2}{2m} \frac{2}{(\hbar z - \epsilon_{\mathbf{q}+\mathbf{k}} + \epsilon_{\mathbf{q}})^2} \right\} \Rightarrow \\
\left[\chi_0^{(4,4)}(\mathbf{k}, z)\right]_4 &= - \int \frac{d^3q}{(2\pi)^3} \left(\frac{2m}{\hbar^2}\right)^3 \frac{f_0(\mathbf{q})}{12} \frac{1}{2k^6} \left\{ \frac{1}{\hbar z - \frac{\epsilon_{\mathbf{q}+2\mathbf{k}} - \epsilon_{\mathbf{q}-2\mathbf{k}}}{4}} - \frac{1}{\hbar z - \frac{\epsilon_{\mathbf{q}+2\mathbf{k}} - \epsilon_{\mathbf{q}}}{2}} + \frac{2\epsilon_{\mathbf{k}}}{(\hbar z - \epsilon_{\mathbf{q}+\mathbf{k}} + \epsilon_{\mathbf{q}})^2} \right\} \Rightarrow \\
\left[\chi_0^{(4,4)}(\mathbf{k}, z)\right]_4 &= - \left(\frac{m}{\hbar^2}\right)^3 \frac{1}{18k^6} \int \frac{d^3q}{(2\pi)^3} 2f_0(\mathbf{q}) \left\{ \frac{3}{\hbar z - \frac{\epsilon_{\mathbf{q}+2\mathbf{k}} - \epsilon_{\mathbf{q}-2\mathbf{k}}}{4}} - \frac{3}{\hbar z - \frac{\epsilon_{\mathbf{q}+2\mathbf{k}} - \epsilon_{\mathbf{q}}}{2}} + \frac{6\epsilon_{\mathbf{k}}}{(\hbar z - \epsilon_{\mathbf{q}+\mathbf{k}} + \epsilon_{\mathbf{q}})^2} \right\} \Rightarrow \\
\left[\chi_0^{(4,4)}(\mathbf{k}, z)\right]_4 &= - \left(\frac{m}{\hbar^2}\right)^3 \frac{1}{18k^6} \int \frac{d^3q}{(2\pi)^3} 2f_0(\mathbf{q}) \left\{ \frac{12}{4\hbar z - \epsilon_{\mathbf{q}+2\mathbf{k}} + \epsilon_{\mathbf{q}-2\mathbf{k}}} - \frac{6}{2\hbar z - \epsilon_{\mathbf{q}+2\mathbf{k}} + \epsilon_{\mathbf{q}}} + \frac{6\epsilon_{\mathbf{k}}}{(\hbar z - \epsilon_{\mathbf{q}+\mathbf{k}} + \epsilon_{\mathbf{q}})^2} \right\} .
\end{aligned}$$

The *fifth contribution* is characterized by two double poles. This becomes apparrent from the two algebraic identities  $(\epsilon_{\mathbf{q}+\mathbf{k}} - \epsilon_{\mathbf{q}-3\mathbf{k}})/4 = (\epsilon_{\mathbf{q}} - \epsilon_{\mathbf{q}-2\mathbf{k}})/2$  and  $(\epsilon_{\mathbf{q}+\mathbf{k}} - \epsilon_{\mathbf{q}-2\mathbf{k}})/3 = \epsilon_{\mathbf{q}} - \epsilon_{\mathbf{q}-\mathbf{k}}$ . We identify and calculate the coefficients  $a, b$ .

$$\begin{aligned}
\left[\chi_0^{(4,4)}(\mathbf{k}, z)\right]_5 &= - \int \frac{d^3 q}{(2\pi)^3} \frac{2f_0(\mathbf{q})}{(4\hbar z - \epsilon_{\mathbf{q}+\mathbf{k}} + \epsilon_{\mathbf{q}-3\mathbf{k}})(3\hbar z - \epsilon_{\mathbf{q}+\mathbf{k}} + \epsilon_{\mathbf{q}-2\mathbf{k}})(2\hbar z - \epsilon_{\mathbf{q}} + \epsilon_{\mathbf{q}-2\mathbf{k}})(\hbar z - \epsilon_{\mathbf{q}} + \epsilon_{\mathbf{q}-\mathbf{k}})} \Rightarrow \\
\left[\chi_0^{(4,4)}(\mathbf{k}, z)\right]_5 &= - \int \frac{d^3 q}{(2\pi)^3} \frac{f_0(\mathbf{q})}{12} \frac{1}{\left[\hbar z - \frac{\epsilon_{\mathbf{q}+\mathbf{k}} - \epsilon_{\mathbf{q}-3\mathbf{k}}}{4}\right] \left[\hbar z - \frac{\epsilon_{\mathbf{q}+\mathbf{k}} - \epsilon_{\mathbf{q}-2\mathbf{k}}}{3}\right] \left[\hbar z - \frac{\epsilon_{\mathbf{q}} - \epsilon_{\mathbf{q}-2\mathbf{k}}}{2}\right] [\hbar z - (\epsilon_{\mathbf{q}} - \epsilon_{\mathbf{q}-\mathbf{k}})]} \Rightarrow \\
\left[\chi_0^{(4,4)}(\mathbf{k}, z)\right]_5 &= - \int \frac{d^3 q}{(2\pi)^3} \frac{f_0(\mathbf{q})}{12} \frac{1}{\left[\hbar z - \frac{\epsilon_{\mathbf{q}} - \epsilon_{\mathbf{q}-2\mathbf{k}}}{2}\right] [\hbar z - (\epsilon_{\mathbf{q}} - \epsilon_{\mathbf{q}-\mathbf{k}})] \left[\hbar z - \frac{\epsilon_{\mathbf{q}} - \epsilon_{\mathbf{q}-2\mathbf{k}}}{2}\right] [\hbar z - (\epsilon_{\mathbf{q}} - \epsilon_{\mathbf{q}-\mathbf{k}})]} \Rightarrow \\
\left[\chi_0^{(4,4)}(\mathbf{k}, z)\right]_5 &= - \int \frac{d^3 q}{(2\pi)^3} \frac{f_0(\mathbf{q})}{12} \frac{1}{\left[\hbar z - \frac{\epsilon_{\mathbf{q}} - \epsilon_{\mathbf{q}-2\mathbf{k}}}{2}\right]^2 [\hbar z - (\epsilon_{\mathbf{q}} - \epsilon_{\mathbf{q}-\mathbf{k}})]^2} \Rightarrow \\
a &= \frac{\epsilon_{\mathbf{q}} - \epsilon_{\mathbf{q}-2\mathbf{k}}}{2} = \frac{\hbar^2}{2m} \frac{q^2 - (\mathbf{q} - 2\mathbf{k})^2}{2} = \frac{\hbar^2}{2m} \frac{-4k^2 + 4\mathbf{q} \cdot \mathbf{k}}{2} = \frac{\hbar^2}{2m} (-2k^2 + 2\mathbf{q} \cdot \mathbf{k}) , \\
b &= \epsilon_{\mathbf{q}} - \epsilon_{\mathbf{q}-\mathbf{k}} = \frac{\hbar^2}{2m} [q^2 - (\mathbf{q} - \mathbf{k})^2] = \frac{\hbar^2}{2m} (-k^2 + 2\mathbf{q} \cdot \mathbf{k}) .
\end{aligned}$$

Then, we compute all the difference between the two coefficients, as well as the difference's square and cube. Note that  $q^2$  and  $\mathbf{q} \cdot \mathbf{k}$  terms vanish.

$$\begin{aligned}
(a - b) &= \frac{\hbar^2}{2m} (-2k^2 + 2\mathbf{q} \cdot \mathbf{k} + k^2 - 2\mathbf{q} \cdot \mathbf{k}) = \frac{\hbar^2}{2m} (-2k^2 + k^2) = \frac{\hbar^2}{2m} (-k^2) , \\
(a - b)^2 &= + \left(\frac{\hbar^2}{2m}\right)^2 (k^4) , \\
(a - b)^3 &= - \left(\frac{\hbar^2}{2m}\right)^3 (k^6) .
\end{aligned}$$

Finally, we substitute the above in the contribution and also perform some straightforward algebra. We introduce the compact notation  $\epsilon_{\mathbf{k}} = (\hbar^2 k^2)/(2m)$  for brevity.

$$\begin{aligned}
\left[\chi_0^{(4,4)}(\mathbf{k}, z)\right]_5 &= + \int \frac{d^3 q}{(2\pi)^3} \left(\frac{2m}{\hbar^2}\right)^3 \frac{f_0(\mathbf{q})}{12k^6} \left\{ \frac{2}{\hbar z - (\epsilon_{\mathbf{q}} - \epsilon_{\mathbf{q}-\mathbf{k}})} - \frac{2}{\hbar z - \frac{\epsilon_{\mathbf{q}} - \epsilon_{\mathbf{q}-2\mathbf{k}}}{2}} - \frac{\hbar^2 k^2}{2m} \frac{1}{[\hbar z - (\epsilon_{\mathbf{q}} - \epsilon_{\mathbf{q}-\mathbf{k}})]^2} - \frac{\hbar^2 k^2}{2m} \frac{1}{\left[\hbar z - \frac{\epsilon_{\mathbf{q}} - \epsilon_{\mathbf{q}-2\mathbf{k}}}{2}\right]^2} \right\} \\
\left[\chi_0^{(4,4)}(\mathbf{k}, z)\right]_5 &= + \int \frac{d^3 q}{(2\pi)^3} \left(\frac{2m}{\hbar^2}\right)^3 \frac{f_0(\mathbf{q})}{12k^6} \left\{ \frac{2}{\hbar z - (\epsilon_{\mathbf{q}} - \epsilon_{\mathbf{q}-\mathbf{k}})} - \frac{2}{\hbar z - \frac{\epsilon_{\mathbf{q}} - \epsilon_{\mathbf{q}-2\mathbf{k}}}{2}} - \frac{\epsilon_{\mathbf{k}}}{[\hbar z - (\epsilon_{\mathbf{q}} - \epsilon_{\mathbf{q}-\mathbf{k}})]^2} - \frac{\epsilon_{\mathbf{k}}}{\left[\hbar z - \frac{\epsilon_{\mathbf{q}} - \epsilon_{\mathbf{q}-2\mathbf{k}}}{2}\right]^2} \right\} \\
\left[\chi_0^{(4,4)}(\mathbf{k}, z)\right]_5 &= + \int \frac{d^3 q}{(2\pi)^3} \left(\frac{m}{\hbar^2}\right)^3 \frac{8f_0(\mathbf{q})}{12k^6} \left\{ \frac{2}{\hbar z - (\epsilon_{\mathbf{q}} - \epsilon_{\mathbf{q}-\mathbf{k}})} - \frac{2}{\hbar z - \frac{\epsilon_{\mathbf{q}} - \epsilon_{\mathbf{q}-2\mathbf{k}}}{2}} - \frac{\epsilon_{\mathbf{k}}}{[\hbar z - (\epsilon_{\mathbf{q}} - \epsilon_{\mathbf{q}-\mathbf{k}})]^2} - \frac{\epsilon_{\mathbf{k}}}{\left[\hbar z - \frac{\epsilon_{\mathbf{q}} - \epsilon_{\mathbf{q}-2\mathbf{k}}}{2}\right]^2} \right\} \\
\left[\chi_0^{(4,4)}(\mathbf{k}, z)\right]_5 &= + \int \frac{d^3 q}{(2\pi)^3} \left(\frac{m}{\hbar^2}\right)^3 \frac{2f_0(\mathbf{q})}{3k^6} \left\{ \frac{2}{\hbar z - (\epsilon_{\mathbf{q}} - \epsilon_{\mathbf{q}-\mathbf{k}})} - \frac{2}{\hbar z - \frac{\epsilon_{\mathbf{q}} - \epsilon_{\mathbf{q}-2\mathbf{k}}}{2}} - \frac{\epsilon_{\mathbf{k}}}{[\hbar z - (\epsilon_{\mathbf{q}} - \epsilon_{\mathbf{q}-\mathbf{k}})]^2} - \frac{\epsilon_{\mathbf{k}}}{\left[\hbar z - \frac{\epsilon_{\mathbf{q}} - \epsilon_{\mathbf{q}-2\mathbf{k}}}{2}\right]^2} \right\} \\
\left[\chi_0^{(4,4)}(\mathbf{k}, z)\right]_5 &= + \left(\frac{m}{\hbar^2}\right)^3 \frac{1}{3k^6} \int \frac{d^3 q}{(2\pi)^3} 2f_0(\mathbf{q}) \left\{ \frac{2}{\hbar z - (\epsilon_{\mathbf{q}} - \epsilon_{\mathbf{q}-\mathbf{k}})} - \frac{2}{\hbar z - \frac{\epsilon_{\mathbf{q}} - \epsilon_{\mathbf{q}-2\mathbf{k}}}{2}} - \frac{\epsilon_{\mathbf{k}}}{[\hbar z - (\epsilon_{\mathbf{q}} - \epsilon_{\mathbf{q}-\mathbf{k}})]^2} - \frac{\epsilon_{\mathbf{k}}}{\left[\hbar z - \frac{\epsilon_{\mathbf{q}} - \epsilon_{\mathbf{q}-2\mathbf{k}}}{2}\right]^2} \right\} \\
\left[\chi_0^{(4,4)}(\mathbf{k}, z)\right]_5 &= + \left(\frac{m}{\hbar^2}\right)^3 \frac{1}{18k^6} \int \frac{d^3 q}{(2\pi)^3} 2f_0(\mathbf{q}) \left\{ \frac{12}{\hbar z - \epsilon_{\mathbf{q}} + \epsilon_{\mathbf{q}-\mathbf{k}}} - \frac{24}{2\hbar z - \epsilon_{\mathbf{q}} + \epsilon_{\mathbf{q}-2\mathbf{k}}} - \frac{6\epsilon_{\mathbf{k}}}{(\hbar z - \epsilon_{\mathbf{q}} + \epsilon_{\mathbf{q}-\mathbf{k}})^2} - \frac{24\epsilon_{\mathbf{k}}}{(2\hbar z - \epsilon_{\mathbf{q}} + \epsilon_{\mathbf{q}-2\mathbf{k}})^2} \right\}
\end{aligned}$$

The *sixth contribution* is characterized by two double poles. This becomes apparant from the two algebraic identities  $(\epsilon_{\mathbf{q}+2\mathbf{k}} - \epsilon_{\mathbf{q}-2\mathbf{k}})/4 = (\epsilon_{\mathbf{q}+\mathbf{k}} - \epsilon_{\mathbf{q}-\mathbf{k}})/2$ ,  $(\epsilon_{\mathbf{q}+2\mathbf{k}} - \epsilon_{\mathbf{q}-\mathbf{k}})/3 = \epsilon_{\mathbf{q}+\mathbf{k}} - \epsilon_{\mathbf{q}}$ . We identify and calculate the coefficients  $a, b$ .

$$\begin{aligned}
\left[\chi_0^{(4,4)}(\mathbf{k}, z)\right]_6 &= + \int \frac{d^3q}{(2\pi)^3} \frac{2f_0(\mathbf{q})}{(4\hbar z - \epsilon_{\mathbf{q}+2\mathbf{k}} + \epsilon_{\mathbf{q}-2\mathbf{k}})(3\hbar z - \epsilon_{\mathbf{q}+2\mathbf{k}} + \epsilon_{\mathbf{q}-\mathbf{k}})(2\hbar z - \epsilon_{\mathbf{q}+\mathbf{k}} + \epsilon_{\mathbf{q}-\mathbf{k}})(\hbar z - \epsilon_{\mathbf{q}+\mathbf{k}} + \epsilon_{\mathbf{q}})} \Rightarrow \\
\left[\chi_0^{(4,4)}(\mathbf{k}, z)\right]_6 &= + \int \frac{d^3q}{(2\pi)^3} \frac{f_0(\mathbf{q})}{12} \frac{1}{\left[\hbar z - \frac{\epsilon_{\mathbf{q}+2\mathbf{k}} - \epsilon_{\mathbf{q}-2\mathbf{k}}}{4}\right] \left[\hbar z - \frac{\epsilon_{\mathbf{q}+2\mathbf{k}} - \epsilon_{\mathbf{q}-\mathbf{k}}}{3}\right] \left[\hbar z - \frac{\epsilon_{\mathbf{q}+\mathbf{k}} - \epsilon_{\mathbf{q}-\mathbf{k}}}{2}\right] [\hbar z - (\epsilon_{\mathbf{q}+\mathbf{k}} - \epsilon_{\mathbf{q}})]} \Rightarrow \\
\left[\chi_0^{(4,4)}(\mathbf{k}, z)\right]_6 &= + \int \frac{d^3q}{(2\pi)^3} \frac{f_0(\mathbf{q})}{12} \frac{1}{\left[\hbar z - \frac{\epsilon_{\mathbf{q}+\mathbf{k}} - \epsilon_{\mathbf{q}-\mathbf{k}}}{2}\right] [\hbar z - (\epsilon_{\mathbf{q}+\mathbf{k}} - \epsilon_{\mathbf{q}})] \left[\hbar z - \frac{\epsilon_{\mathbf{q}+\mathbf{k}} - \epsilon_{\mathbf{q}-\mathbf{k}}}{2}\right] [\hbar z - (\epsilon_{\mathbf{q}+\mathbf{k}} - \epsilon_{\mathbf{q}})]} \Rightarrow \\
\left[\chi_0^{(4,4)}(\mathbf{k}, z)\right]_6 &= + \int \frac{d^3q}{(2\pi)^3} \frac{f_0(\mathbf{q})}{12} \frac{1}{\left[\hbar z - \frac{\epsilon_{\mathbf{q}+\mathbf{k}} - \epsilon_{\mathbf{q}-\mathbf{k}}}{2}\right]^2 [\hbar z - (\epsilon_{\mathbf{q}+\mathbf{k}} - \epsilon_{\mathbf{q}})]^2} \Rightarrow \\
a = \frac{\epsilon_{\mathbf{q}+\mathbf{k}} - \epsilon_{\mathbf{q}-\mathbf{k}}}{2} &= \frac{\hbar^2}{2m} \frac{(\mathbf{q} + \mathbf{k})^2 - (\mathbf{q} - \mathbf{k})^2}{2} = \frac{\hbar^2}{2m} \frac{k^2 + 2\mathbf{q} \cdot \mathbf{k} - k^2 + 2\mathbf{q} \cdot \mathbf{k}}{2} = \frac{\hbar^2}{2m} \frac{4\mathbf{q} \cdot \mathbf{k}}{2} = \frac{\hbar^2}{2m} (2\mathbf{q} \cdot \mathbf{k}) \\
b = \epsilon_{\mathbf{q}+\mathbf{k}} - \epsilon_{\mathbf{q}} &= \frac{\hbar^2}{2m} [(\mathbf{q} + \mathbf{k})^2 - q^2] = \frac{\hbar^2}{2m} (k^2 + 2\mathbf{q} \cdot \mathbf{k}) .
\end{aligned}$$

Then, we compute all the difference between the two coefficients, as well as the difference's square and cube. Note that the  $q^2$  and  $\mathbf{q} \cdot \mathbf{k}$  terms vanish.

$$\begin{aligned}
(a - b) &= \frac{\hbar^2}{2m} (2\mathbf{q} \cdot \mathbf{k} - k^2 - 2\mathbf{q} \cdot \mathbf{k}) = \frac{\hbar^2}{2m} (-k^2) = -\frac{\hbar^2}{2m} (k^2) , \\
(a - b)^2 &= \left(\frac{\hbar^2}{2m}\right)^2 (k^4) , \\
(a - b)^3 &= -\left(\frac{\hbar^2}{2m}\right)^3 (k^6) .
\end{aligned}$$

Finally, we substitute the above in the contribution and also perform some straightforward algebra. We introduce the compact notation  $\epsilon_{\mathbf{k}} = (\hbar^2 k^2)/(2m)$  for brevity.

$$\begin{aligned}
\left[\chi_0^{(4,4)}(\mathbf{k}, z)\right]_6 &= - \int \frac{d^3q}{(2\pi)^3} \left(\frac{2m}{\hbar^2}\right)^3 \frac{f_0(\mathbf{q})}{12k^6} \left\{ \frac{2}{\hbar z - \epsilon_{\mathbf{q}+\mathbf{k}} + \epsilon_{\mathbf{q}}} - \frac{2}{\hbar z - \frac{\epsilon_{\mathbf{q}+\mathbf{k}} - \epsilon_{\mathbf{q}-\mathbf{k}}}{2}} - \frac{\hbar^2 k^2}{2m} \frac{1}{(\hbar z - \epsilon_{\mathbf{q}+\mathbf{k}} + \epsilon_{\mathbf{q}})^2} - \frac{\hbar^2 k^2}{2m} \frac{1}{\left(\hbar z - \frac{\epsilon_{\mathbf{q}+\mathbf{k}} - \epsilon_{\mathbf{q}-\mathbf{k}}}{2}\right)^2} \right\} \\
\left[\chi_0^{(4,4)}(\mathbf{k}, z)\right]_6 &= - \int \frac{d^3q}{(2\pi)^3} \left(\frac{2m}{\hbar^2}\right)^3 \frac{f_0(\mathbf{q})}{12k^6} \left\{ \frac{2}{\hbar z - \epsilon_{\mathbf{q}+\mathbf{k}} + \epsilon_{\mathbf{q}}} - \frac{2}{\hbar z - \frac{\epsilon_{\mathbf{q}+\mathbf{k}} - \epsilon_{\mathbf{q}-\mathbf{k}}}{2}} - \frac{\epsilon_{\mathbf{k}}}{(\hbar z - \epsilon_{\mathbf{q}+\mathbf{k}} + \epsilon_{\mathbf{q}})^2} - \frac{\epsilon_{\mathbf{k}}}{\left(\hbar z - \frac{\epsilon_{\mathbf{q}+\mathbf{k}} - \epsilon_{\mathbf{q}-\mathbf{k}}}{2}\right)^2} \right\} \\
\left[\chi_0^{(4,4)}(\mathbf{k}, z)\right]_6 &= - \int \frac{d^3q}{(2\pi)^3} \left(\frac{m}{\hbar^2}\right)^3 \frac{8f_0(\mathbf{q})}{12k^6} \left\{ \frac{2}{\hbar z - \epsilon_{\mathbf{q}+\mathbf{k}} + \epsilon_{\mathbf{q}}} - \frac{2}{\hbar z - \frac{\epsilon_{\mathbf{q}+\mathbf{k}} - \epsilon_{\mathbf{q}-\mathbf{k}}}{2}} - \frac{\epsilon_{\mathbf{k}}}{(\hbar z - \epsilon_{\mathbf{q}+\mathbf{k}} + \epsilon_{\mathbf{q}})^2} - \frac{\epsilon_{\mathbf{k}}}{\left(\hbar z - \frac{\epsilon_{\mathbf{q}+\mathbf{k}} - \epsilon_{\mathbf{q}-\mathbf{k}}}{2}\right)^2} \right\} \\
\left[\chi_0^{(4,4)}(\mathbf{k}, z)\right]_6 &= - \int \frac{d^3q}{(2\pi)^3} \left(\frac{m}{\hbar^2}\right)^3 \frac{2f_0(\mathbf{q})}{3k^6} \left\{ \frac{2}{\hbar z - \epsilon_{\mathbf{q}+\mathbf{k}} + \epsilon_{\mathbf{q}}} - \frac{2}{\hbar z - \frac{\epsilon_{\mathbf{q}+\mathbf{k}} - \epsilon_{\mathbf{q}-\mathbf{k}}}{2}} - \frac{\epsilon_{\mathbf{k}}}{(\hbar z - \epsilon_{\mathbf{q}+\mathbf{k}} + \epsilon_{\mathbf{q}})^2} - \frac{\epsilon_{\mathbf{k}}}{\left(\hbar z - \frac{\epsilon_{\mathbf{q}+\mathbf{k}} - \epsilon_{\mathbf{q}-\mathbf{k}}}{2}\right)^2} \right\} \\
\left[\chi_0^{(4,4)}(\mathbf{k}, z)\right]_6 &= - \left(\frac{m}{\hbar^2}\right)^3 \frac{1}{3k^6} \int \frac{d^3q}{(2\pi)^3} 2f_0(\mathbf{q}) \left\{ \frac{2}{\hbar z - \epsilon_{\mathbf{q}+\mathbf{k}} + \epsilon_{\mathbf{q}}} - \frac{2}{\hbar z - \frac{\epsilon_{\mathbf{q}+\mathbf{k}} - \epsilon_{\mathbf{q}-\mathbf{k}}}{2}} - \frac{\epsilon_{\mathbf{k}}}{(\hbar z - \epsilon_{\mathbf{q}+\mathbf{k}} + \epsilon_{\mathbf{q}})^2} - \frac{\epsilon_{\mathbf{k}}}{\left(\hbar z - \frac{\epsilon_{\mathbf{q}+\mathbf{k}} - \epsilon_{\mathbf{q}-\mathbf{k}}}{2}\right)^2} \right\} \\
\left[\chi_0^{(4,4)}(\mathbf{k}, z)\right]_6 &= - \left(\frac{m}{\hbar^2}\right)^3 \frac{1}{18k^6} \int \frac{d^3q}{(2\pi)^3} 2f_0(\mathbf{q}) \left\{ \frac{12}{\hbar z - \epsilon_{\mathbf{q}+\mathbf{k}} + \epsilon_{\mathbf{q}}} - \frac{24}{2\hbar z - \epsilon_{\mathbf{q}+\mathbf{k}} + \epsilon_{\mathbf{q}-\mathbf{k}}} - \frac{6\epsilon_{\mathbf{k}}}{(\hbar z - \epsilon_{\mathbf{q}+\mathbf{k}} + \epsilon_{\mathbf{q}})^2} - \frac{24\epsilon_{\mathbf{k}}}{(2\hbar z - \epsilon_{\mathbf{q}+\mathbf{k}} + \epsilon_{\mathbf{q}-\mathbf{k}})^2} \right\}
\end{aligned}$$

The *seventh contribution* is characterized by two simple poles and one double pole. This becomes apparrent from the algebraic identity  $(\epsilon_{q+2k} - \epsilon_{q-2k})/4 = (\epsilon_{q+k} - \epsilon_{q-k})/2$ . We first identify and calculate the coefficients  $a, b, c$ .

$$\begin{aligned}
[\chi_0^{(4,4)}(\mathbf{k}, z)]_7 &= + \int \frac{d^3q}{(2\pi)^3} \frac{2f_0(\mathbf{q})}{(4\hbar z - \epsilon_{q+2k} + \epsilon_{q-2k})(3\hbar z - \epsilon_{q+2k} + \epsilon_{q-k})(2\hbar z - \epsilon_{q+k} + \epsilon_{q-k})(\hbar z - \epsilon_q + \epsilon_{q-k})} \Rightarrow \\
[\chi_0^{(4,4)}(\mathbf{k}, z)]_7 &= + \int \frac{d^3q}{(2\pi)^3} \frac{f_0(\mathbf{q})}{12} \frac{1}{\left[\hbar z - \frac{\epsilon_{q+2k} - \epsilon_{q-2k}}{4}\right] \left[\hbar z - \frac{\epsilon_{q+2k} - \epsilon_{q-k}}{3}\right] \left[\hbar z - \frac{\epsilon_{q+k} - \epsilon_{q-k}}{2}\right] [\hbar z - (\epsilon_q - \epsilon_{q-k})]} \Rightarrow \\
[\chi_0^{(4,4)}(\mathbf{k}, z)]_7 &= + \int \frac{d^3q}{(2\pi)^3} \frac{f_0(\mathbf{q})}{12} \frac{1}{\left[\hbar z - \frac{\epsilon_{q+k} - \epsilon_{q-k}}{2}\right] \left[\hbar z - \frac{\epsilon_{q+2k} - \epsilon_{q-k}}{3}\right] \left[\hbar z - \frac{\epsilon_{q+k} - \epsilon_{q-k}}{2}\right] [\hbar z - (\epsilon_q - \epsilon_{q-k})]} \Rightarrow \\
[\chi_0^{(4,4)}(\mathbf{k}, z)]_7 &= + \int \frac{d^3q}{(2\pi)^3} \frac{f_0(\mathbf{q})}{12} \frac{1}{\left[\hbar z - \frac{\epsilon_{q+2k} - \epsilon_{q-k}}{3}\right] [\hbar z - (\epsilon_q - \epsilon_{q-k})] \left[\hbar z - \frac{\epsilon_{q+k} - \epsilon_{q-k}}{2}\right]^2} \Rightarrow \\
a &= \frac{\epsilon_{q+2k} - \epsilon_{q-k}}{3} = \frac{\hbar^2}{2m} \frac{(\mathbf{q} + 2\mathbf{k})^2 - (\mathbf{q} - \mathbf{k})^2}{3} = \frac{\hbar^2}{2m} \frac{4k^2 + 4\mathbf{q} \cdot \mathbf{k} - k^2 + 2\mathbf{q} \cdot \mathbf{k}}{3} = \frac{\hbar^2}{2m} \frac{3k^2 + 6\mathbf{q} \cdot \mathbf{k}}{3} = \frac{\hbar^2}{2m} (k^2 + 2\mathbf{q} \cdot \mathbf{k}), \\
b &= \epsilon_q - \epsilon_{q-k} = \frac{\hbar^2}{2m} [q^2 - (\mathbf{q} - \mathbf{k})^2] = \frac{\hbar^2}{2m} (-k^2 + 2\mathbf{q} \cdot \mathbf{k}), \\
c &= \frac{\epsilon_{q+k} - \epsilon_{q-k}}{2} = \frac{\hbar^2}{2m} \frac{(\mathbf{q} + \mathbf{k})^2 - (\mathbf{q} - \mathbf{k})^2}{2} = \frac{\hbar^2}{2m} \frac{k^2 + 2\mathbf{q} \cdot \mathbf{k} - k^2 + 2\mathbf{q} \cdot \mathbf{k}}{2} = \frac{\hbar^2}{2m} \frac{4\mathbf{q} \cdot \mathbf{k}}{2} = \frac{\hbar^2}{2m} (2\mathbf{q} \cdot \mathbf{k}).
\end{aligned}$$

Then, we compute all the relevant differences between these three coefficients. Note that the  $q^2$  and  $\mathbf{q} \cdot \mathbf{k}$  terms vanish.

$$\begin{aligned}
a - b &= \frac{\hbar^2}{2m} (k^2 + 2\mathbf{q} \cdot \mathbf{k} + k^2 - 2\mathbf{q} \cdot \mathbf{k}) = \frac{\hbar^2}{2m} (2k^2), \\
a - c &= \frac{\hbar^2}{2m} (k^2 + 2\mathbf{q} \cdot \mathbf{k} - 2\mathbf{q} \cdot \mathbf{k}) = \frac{\hbar^2}{2m} (k^2), \\
b - c &= \frac{\hbar^2}{2m} (-k^2 + 2\mathbf{q} \cdot \mathbf{k} - 2\mathbf{q} \cdot \mathbf{k}) = -\frac{\hbar^2}{2m} (k^2), \\
a + b - 2c &= \frac{\hbar^2}{2m} (k^2 + 2\mathbf{q} \cdot \mathbf{k} - k^2 + 2\mathbf{q} \cdot \mathbf{k} - 4\mathbf{q} \cdot \mathbf{k}) = \frac{\hbar^2}{2m} (k^2 - k^2) = 0.
\end{aligned}$$

Afterwards, we compute all the algebraic combinations that are present in the partial fraction decomposition.

$$\begin{aligned}
(a - b)(a - c)^2 &= + \left(\frac{\hbar^2}{2m}\right)^3 (2k^2) (k^2)^2 = + \left(\frac{\hbar^2}{2m}\right)^3 (2k^6), \\
(a - b)(b - c)^2 &= + \left(\frac{\hbar^2}{2m}\right)^3 (2k^2) (k^2)^2 = + \left(\frac{\hbar^2}{2m}\right)^3 (2k^6), \\
(a - c)^2(b - c)^2 &= + \left(\frac{\hbar^2}{2m}\right)^4 (k^2)^2 (k^2)^2 = + \left(\frac{\hbar^2}{2m}\right)^4 (k^8), \\
(a - c)(b - c) &= - \left(\frac{\hbar^2}{2m}\right)^2 (k^2) (k^2) = - \left(\frac{\hbar^2}{2m}\right)^2 (k^4) = - \frac{1}{2k^2} \frac{2m}{\hbar^2} \left(\frac{\hbar^2}{2m}\right)^3 (2k^6).
\end{aligned}$$

Finally, we substitute and perform some algebra. We also introduce the compact notation  $\epsilon_{\mathbf{k}} = (\hbar^2 k^2)/(2m)$ .

$$\begin{aligned}
[\chi_0^{(4,4)}(\mathbf{k}, z)]_7 &= + \int \frac{d^3q}{(2\pi)^3} \left(\frac{2m}{\hbar^2}\right)^3 \frac{f_0(\mathbf{q})}{12} \frac{1}{2k^6} \left\{ \frac{1}{\hbar z - \frac{\epsilon_{q+2k} - \epsilon_{q-k}}{3}} - \frac{1}{\hbar z - \epsilon_q + \epsilon_{q-k}} - \frac{\hbar^2 k^2}{2m} \frac{2}{\left(\hbar z - \frac{\epsilon_{q+k} - \epsilon_{q-k}}{2}\right)^2} \right\} \Rightarrow \\
[\chi_0^{(4,4)}(\mathbf{k}, z)]_7 &= + \left(\frac{m}{\hbar^2}\right)^3 \frac{1}{18k^6} \int \frac{d^3q}{(2\pi)^3} 2f_0(\mathbf{q}) \left\{ \frac{3}{\hbar z - \frac{\epsilon_{q+2k} - \epsilon_{q-k}}{3}} - \frac{3}{\hbar z - \epsilon_q + \epsilon_{q-k}} - \frac{6\epsilon_{\mathbf{k}}}{\left(\hbar z - \frac{\epsilon_{q+k} - \epsilon_{q-k}}{2}\right)^2} \right\} \Rightarrow \\
[\chi_0^{(4,4)}(\mathbf{k}, z)]_7 &= + \left(\frac{m}{\hbar^2}\right)^3 \frac{1}{18k^6} \int \frac{d^3q}{(2\pi)^3} 2f_0(\mathbf{q}) \left\{ \frac{9}{3\hbar z - \epsilon_{q+2k} + \epsilon_{q-k}} - \frac{3}{\hbar z - \epsilon_q + \epsilon_{q-k}} - \frac{24\epsilon_{\mathbf{k}}}{(2\hbar z - \epsilon_{q+k} + \epsilon_{q-k})^2} \right\}.
\end{aligned}$$

The *eighth contribution* is characterized by two simple poles and one double pole. This becomes apparrent from the algebraic identity  $(\epsilon_{\mathbf{q}+3\mathbf{k}} - \epsilon_{\mathbf{q}-\mathbf{k}})/4 = (\epsilon_{\mathbf{q}+2\mathbf{k}} - \epsilon_{\mathbf{q}})/2$ . We first identify and calculate the coefficients  $a, b, c$ .

$$\begin{aligned}
\left[\chi_0^{(4,4)}(\mathbf{k}, z)\right]_8 &= - \int \frac{d^3q}{(2\pi)^3} \frac{2f_0(\mathbf{q})}{(4\hbar z - \epsilon_{\mathbf{q}+3\mathbf{k}} + \epsilon_{\mathbf{q}-\mathbf{k}})(3\hbar z - \epsilon_{\mathbf{q}+3\mathbf{k}} + \epsilon_{\mathbf{q}})(2\hbar z - \epsilon_{\mathbf{q}+2\mathbf{k}} + \epsilon_{\mathbf{q}})(\hbar z - \epsilon_{\mathbf{q}+\mathbf{k}} + \epsilon_{\mathbf{q}})} \Rightarrow \\
\left[\chi_0^{(4,4)}(\mathbf{k}, z)\right]_8 &= - \int \frac{d^3q}{(2\pi)^3} \frac{f_0(\mathbf{q})}{12} \frac{1}{\left[\hbar z - \frac{\epsilon_{\mathbf{q}+3\mathbf{k}} - \epsilon_{\mathbf{q}-\mathbf{k}}}{4}\right] \left[\hbar z - \frac{\epsilon_{\mathbf{q}+3\mathbf{k}} - \epsilon_{\mathbf{q}}}{3}\right] \left[\hbar z - \frac{\epsilon_{\mathbf{q}+2\mathbf{k}} - \epsilon_{\mathbf{q}}}{2}\right] [\hbar z - (\epsilon_{\mathbf{q}+\mathbf{k}} - \epsilon_{\mathbf{q}})]} \Rightarrow \\
\left[\chi_0^{(4,4)}(\mathbf{k}, z)\right]_8 &= - \int \frac{d^3q}{(2\pi)^3} \frac{f_0(\mathbf{q})}{12} \frac{1}{\left[\hbar z - \frac{\epsilon_{\mathbf{q}+2\mathbf{k}} - \epsilon_{\mathbf{q}}}{2}\right] \left[\hbar z - \frac{\epsilon_{\mathbf{q}+3\mathbf{k}} - \epsilon_{\mathbf{q}}}{3}\right] \left[\hbar z - \frac{\epsilon_{\mathbf{q}+2\mathbf{k}} - \epsilon_{\mathbf{q}}}{2}\right] [\hbar z - (\epsilon_{\mathbf{q}+\mathbf{k}} - \epsilon_{\mathbf{q}})]} \Rightarrow \\
\left[\chi_0^{(4,4)}(\mathbf{k}, z)\right]_8 &= - \int \frac{d^3q}{(2\pi)^3} \frac{f_0(\mathbf{q})}{12} \frac{1}{\left[\hbar z - \frac{\epsilon_{\mathbf{q}+3\mathbf{k}} - \epsilon_{\mathbf{q}}}{3}\right] [\hbar z - (\epsilon_{\mathbf{q}+\mathbf{k}} - \epsilon_{\mathbf{q}})] \left[\hbar z - \frac{\epsilon_{\mathbf{q}+2\mathbf{k}} - \epsilon_{\mathbf{q}}}{2}\right]^2} \Rightarrow \\
a = \frac{\epsilon_{\mathbf{q}+3\mathbf{k}} - \epsilon_{\mathbf{q}}}{3} &= \frac{\hbar^2}{2m} \frac{(\mathbf{q} + 3\mathbf{k})^2 - q^2}{3} = \frac{\hbar^2}{2m} \frac{9k^2 + 6\mathbf{q} \cdot \mathbf{k}}{3} = \frac{\hbar^2}{2m} (3k^2 + 2\mathbf{q} \cdot \mathbf{k}) , \\
b = \epsilon_{\mathbf{q}+\mathbf{k}} - \epsilon_{\mathbf{q}} &= \frac{\hbar^2}{2m} [(\mathbf{q} + \mathbf{k})^2 - q^2] = \frac{\hbar^2}{2m} (k^2 + 2\mathbf{q} \cdot \mathbf{k}) , \\
c = \frac{\epsilon_{\mathbf{q}+2\mathbf{k}} - \epsilon_{\mathbf{q}}}{2} &= \frac{\hbar^2}{2m} \frac{(\mathbf{q} + 2\mathbf{k})^2 - q^2}{2} = \frac{\hbar^2}{2m} \frac{4k^2 + 4\mathbf{q} \cdot \mathbf{k}}{2} = \frac{\hbar^2}{2m} (2k^2 + 2\mathbf{q} \cdot \mathbf{k}) .
\end{aligned}$$

Then, we compute all the relevant differences between these three coefficients. Note that the  $q^2$  and  $\mathbf{q} \cdot \mathbf{k}$  terms vanish.

$$\begin{aligned}
a - b &= \frac{\hbar^2}{2m} (3k^2 + 2\mathbf{q} \cdot \mathbf{k} - k^2 - 2\mathbf{q} \cdot \mathbf{k}) = \frac{\hbar^2}{2m} (3k^2 - k^2) = \frac{\hbar^2}{2m} (2k^2) , \\
a - c &= \frac{\hbar^2}{2m} (3k^2 + 2\mathbf{q} \cdot \mathbf{k} - 2k^2 - 2\mathbf{q} \cdot \mathbf{k}) = \frac{\hbar^2}{2m} (k^2) , \\
b - c &= \frac{\hbar^2}{2m} (k^2 + 2\mathbf{q} \cdot \mathbf{k} - 2k^2 - 2\mathbf{q} \cdot \mathbf{k}) = -\frac{\hbar^2}{2m} (k^2) , \\
a + b - 2c &= \frac{\hbar^2}{2m} (3k^2 + 2\mathbf{q} \cdot \mathbf{k} + k^2 + 2\mathbf{q} \cdot \mathbf{k} - 4k^2 - 4\mathbf{q} \cdot \mathbf{k}) = \frac{\hbar^2}{2m} (3k^2 + k^2 - 4k^2) = 0 .
\end{aligned}$$

Afterwards, we compute all the algebraic combinations that are present in the partial fraction decomposition.

$$\begin{aligned}
(a - b)(a - c)^2 &= + \left(\frac{\hbar^2}{2m}\right)^3 (2k^2) (k^2)^2 = + \left(\frac{\hbar^2}{2m}\right)^3 (2k^6) , \\
(a - b)(b - c)^2 &= + \left(\frac{\hbar^2}{2m}\right)^3 (2k^2) (k^2)^2 = + \left(\frac{\hbar^2}{2m}\right)^3 (2k^6) , \\
(a - c)^2(b - c)^2 &= + \left(\frac{\hbar^2}{2m}\right)^4 (k^2)^2 (k^2)^2 = + \left(\frac{\hbar^2}{2m}\right)^4 (k^8) , \\
(a - c)(b - c) &= - \left(\frac{\hbar^2}{2m}\right)^2 (k^2) (k^2) = - \left(\frac{\hbar^2}{2m}\right)^2 (k^4) = - \frac{1}{2k^2} \frac{2m}{\hbar^2} \left(\frac{\hbar^2}{2m}\right)^3 (2k^6) .
\end{aligned}$$

Finally, we substitute and perform some algebra. We also introduce the compact notation  $\epsilon_{\mathbf{k}} = (\hbar^2 k^2)/(2m)$ .

$$\begin{aligned}
\left[\chi_0^{(4,4)}(\mathbf{k}, z)\right]_8 &= - \int \frac{d^3q}{(2\pi)^3} \left(\frac{2m}{\hbar^2}\right)^3 \frac{f_0(\mathbf{q})}{12} \frac{1}{2k^6} \left\{ \frac{1}{\hbar z - \frac{\epsilon_{\mathbf{q}+3\mathbf{k}} - \epsilon_{\mathbf{q}}}{3}} - \frac{1}{\hbar z - \epsilon_{\mathbf{q}+\mathbf{k}} + \epsilon_{\mathbf{q}}} - \frac{\hbar^2 k^2}{2m} \frac{2}{\left(\hbar z - \frac{\epsilon_{\mathbf{q}+2\mathbf{k}} - \epsilon_{\mathbf{q}}}{2}\right)^2} \right\} \Rightarrow \\
\left[\chi_0^{(4,4)}(\mathbf{k}, z)\right]_8 &= - \left(\frac{m}{\hbar^2}\right)^3 \frac{1}{18k^6} \int \frac{d^3q}{(2\pi)^3} 2f_0(\mathbf{q}) \left\{ \frac{3}{\hbar z - \frac{\epsilon_{\mathbf{q}+3\mathbf{k}} - \epsilon_{\mathbf{q}}}{3}} - \frac{3}{\hbar z - \epsilon_{\mathbf{q}+\mathbf{k}} + \epsilon_{\mathbf{q}}} - \frac{6\epsilon_{\mathbf{k}}}{\left(\hbar z - \frac{\epsilon_{\mathbf{q}+2\mathbf{k}} - \epsilon_{\mathbf{q}}}{2}\right)^2} \right\} \Rightarrow \\
\left[\chi_0^{(4,4)}(\mathbf{k}, z)\right]_8 &= - \left(\frac{m}{\hbar^2}\right)^3 \frac{1}{18k^6} \int \frac{d^3q}{(2\pi)^3} 2f_0(\mathbf{q}) \left\{ \frac{9}{3\hbar z - \epsilon_{\mathbf{q}+3\mathbf{k}} + \epsilon_{\mathbf{q}}} - \frac{3}{\hbar z - \epsilon_{\mathbf{q}+\mathbf{k}} + \epsilon_{\mathbf{q}}} - \frac{24\epsilon_{\mathbf{k}}}{(2\hbar z - \epsilon_{\mathbf{q}+2\mathbf{k}} + \epsilon_{\mathbf{q}})^2} \right\} .
\end{aligned}$$

The *ninth contribution* is characterized by two simple poles and one double pole. This becomes apparrent from the algebraic identity  $(\epsilon_{\mathbf{q}+\mathbf{k}} - \epsilon_{\mathbf{q}-3\mathbf{k}})/4 = (\epsilon_{\mathbf{q}} - \epsilon_{\mathbf{q}-2\mathbf{k}})/2$ . We first identify and calculate the coefficients  $a, b, c$ .

$$\begin{aligned}
\left[\chi_0^{(4,4)}(\mathbf{k}, z)\right]_9 &= - \int \frac{d^3q}{(2\pi)^3} \frac{2f_0(\mathbf{q})}{(4\hbar z - \epsilon_{\mathbf{q}+\mathbf{k}} + \epsilon_{\mathbf{q}-3\mathbf{k}})(3\hbar z - \epsilon_{\mathbf{q}} + \epsilon_{\mathbf{q}-3\mathbf{k}})(2\hbar z - \epsilon_{\mathbf{q}} + \epsilon_{\mathbf{q}-2\mathbf{k}})(\hbar z - \epsilon_{\mathbf{q}} + \epsilon_{\mathbf{q}-\mathbf{k}})} \Rightarrow \\
\left[\chi_0^{(4,4)}(\mathbf{k}, z)\right]_9 &= - \int \frac{d^3q}{(2\pi)^3} \frac{f_0(\mathbf{q})}{12} \frac{1}{\left[\hbar z - \frac{\epsilon_{\mathbf{q}+\mathbf{k}} - \epsilon_{\mathbf{q}-3\mathbf{k}}}{4}\right] \left[\hbar z - \frac{\epsilon_{\mathbf{q}} - \epsilon_{\mathbf{q}-3\mathbf{k}}}{3}\right] \left[\hbar z - \frac{\epsilon_{\mathbf{q}} - \epsilon_{\mathbf{q}-2\mathbf{k}}}{2}\right] [\hbar z - (\epsilon_{\mathbf{q}} - \epsilon_{\mathbf{q}-\mathbf{k}})]} \Rightarrow \\
\left[\chi_0^{(4,4)}(\mathbf{k}, z)\right]_9 &= - \int \frac{d^3q}{(2\pi)^3} \frac{f_0(\mathbf{q})}{12} \frac{1}{\left[\hbar z - \frac{\epsilon_{\mathbf{q}} - \epsilon_{\mathbf{q}-2\mathbf{k}}}{2}\right] \left[\hbar z - \frac{\epsilon_{\mathbf{q}} - \epsilon_{\mathbf{q}-3\mathbf{k}}}{3}\right] \left[\hbar z - \frac{\epsilon_{\mathbf{q}} - \epsilon_{\mathbf{q}-2\mathbf{k}}}{2}\right] [\hbar z - (\epsilon_{\mathbf{q}} - \epsilon_{\mathbf{q}-\mathbf{k}})]} \Rightarrow \\
\left[\chi_0^{(4,4)}(\mathbf{k}, z)\right]_9 &= - \int \frac{d^3q}{(2\pi)^3} \frac{f_0(\mathbf{q})}{12} \frac{1}{\left[\hbar z - \frac{\epsilon_{\mathbf{q}} - \epsilon_{\mathbf{q}-3\mathbf{k}}}{3}\right] [\hbar z - (\epsilon_{\mathbf{q}} - \epsilon_{\mathbf{q}-\mathbf{k}})] \left[\hbar z - \frac{\epsilon_{\mathbf{q}} - \epsilon_{\mathbf{q}-2\mathbf{k}}}{2}\right]^2} \Rightarrow \\
a = \frac{\epsilon_{\mathbf{q}} - \epsilon_{\mathbf{q}-3\mathbf{k}}}{3} &= \frac{\hbar^2}{2m} \frac{q^2 - (\mathbf{q} - 3\mathbf{k})^2}{3} = \frac{\hbar^2}{2m} \frac{-9k^2 + 6\mathbf{q} \cdot \mathbf{k}}{3} = \frac{\hbar^2}{2m} (-3k^2 + 2\mathbf{q} \cdot \mathbf{k}), \\
b = \epsilon_{\mathbf{q}} - \epsilon_{\mathbf{q}-\mathbf{k}} &= \frac{\hbar^2}{2m} [q^2 - (\mathbf{q} - \mathbf{k})^2] = \frac{\hbar^2}{2m} (-k^2 + 2\mathbf{q} \cdot \mathbf{k}), \\
c = \frac{\epsilon_{\mathbf{q}} - \epsilon_{\mathbf{q}-2\mathbf{k}}}{2} &= \frac{\hbar^2}{2m} \frac{q^2 - (\mathbf{q} - 2\mathbf{k})^2}{2} = \frac{\hbar^2}{2m} \frac{-4k^2 + 4\mathbf{q} \cdot \mathbf{k}}{2} = \frac{\hbar^2}{2m} (-2k^2 + 2\mathbf{q} \cdot \mathbf{k}).
\end{aligned}$$

Then, we compute all the relevant differences between these three coefficients. Note that the  $q^2$  and  $\mathbf{q} \cdot \mathbf{k}$  terms vanish.

$$\begin{aligned}
a - b &= \frac{\hbar^2}{2m} (-3k^2 + 2\mathbf{q} \cdot \mathbf{k} + k^2 - 2\mathbf{q} \cdot \mathbf{k}) = \frac{\hbar^2}{2m} (-3k^2 + k^2) = -\frac{\hbar^2}{2m} (2k^2), \\
a - c &= \frac{\hbar^2}{2m} (-3k^2 + 2\mathbf{q} \cdot \mathbf{k} + 2k^2 - 2\mathbf{q} \cdot \mathbf{k}) = \frac{\hbar^2}{2m} (-3k^2 + 2k^2) = -\frac{\hbar^2}{2m} (k^2), \\
b - c &= \frac{\hbar^2}{2m} (-k^2 + 2\mathbf{q} \cdot \mathbf{k} + 2k^2 - 2\mathbf{q} \cdot \mathbf{k}) = \frac{\hbar^2}{2m} (-k^2 + 2k^2) = +\frac{\hbar^2}{2m} (k^2), \\
a + b - 2c &= \frac{\hbar^2}{2m} (-3k^2 + 2\mathbf{q} \cdot \mathbf{k} - k^2 + 2\mathbf{q} \cdot \mathbf{k} + 4k^2 - 4\mathbf{q} \cdot \mathbf{k}) = \frac{\hbar^2}{2m} (-3k^2 - k^2 + 4k^2) = 0.
\end{aligned}$$

Afterwards, we compute all the algebraic combinations that are present in the partial fraction decomposition.

$$\begin{aligned}
(a - b)(a - c)^2 &= - \left(\frac{\hbar^2}{2m}\right)^3 (2k^2) (k^2)^2 = - \left(\frac{\hbar^2}{2m}\right)^3 (2k^6), \\
(a - b)(b - c)^2 &= - \left(\frac{\hbar^2}{2m}\right)^3 (2k^2) (k^2)^2 = - \left(\frac{\hbar^2}{2m}\right)^3 (2k^6), \\
(a - c)^2(b - c)^2 &= + \left(\frac{\hbar^2}{2m}\right)^4 (k^2)^2 (k^2)^2 = + \left(\frac{\hbar^2}{2m}\right)^4 (k^8), \\
(a - c)(b - c) &= - \left(\frac{\hbar^2}{2m}\right)^2 (k^2) (k^2) = - \left(\frac{\hbar^2}{2m}\right)^2 (k^4) = - \frac{1}{2k^2} \frac{2m}{\hbar^2} \left(\frac{\hbar^2}{2m}\right)^3 (2k^6).
\end{aligned}$$

Finally, we substitute and perform some algebra. We also introduce the compact notation  $\epsilon_{\mathbf{k}} = (\hbar^2 k^2)/(2m)$ .

$$\begin{aligned}
\left[\chi_0^{(4,4)}(\mathbf{k}, z)\right]_9 &= + \int \frac{d^3q}{(2\pi)^3} \left(\frac{2m}{\hbar^2}\right)^3 \frac{f_0(\mathbf{q})}{12} \frac{1}{2k^6} \left\{ \frac{1}{\hbar z - \frac{\epsilon_{\mathbf{q}} - \epsilon_{\mathbf{q}-3\mathbf{k}}}{3}} - \frac{1}{\hbar z - \epsilon_{\mathbf{q}} + \epsilon_{\mathbf{q}-\mathbf{k}}} + \frac{\hbar^2 k^2}{2m} \frac{2}{\left(\hbar z - \frac{\epsilon_{\mathbf{q}} - \epsilon_{\mathbf{q}-2\mathbf{k}}}{2}\right)^2} \right\} \Rightarrow \\
\left[\chi_0^{(4,4)}(\mathbf{k}, z)\right]_9 &= + \left(\frac{m}{\hbar^2}\right)^3 \frac{1}{18k^6} \int \frac{d^3q}{(2\pi)^3} 2f_0(\mathbf{q}) \left\{ \frac{3}{\hbar z - \frac{\epsilon_{\mathbf{q}} - \epsilon_{\mathbf{q}-3\mathbf{k}}}{3}} - \frac{3}{\hbar z - \epsilon_{\mathbf{q}} + \epsilon_{\mathbf{q}-\mathbf{k}}} + \frac{6\epsilon_{\mathbf{k}}}{\left(\hbar z - \frac{\epsilon_{\mathbf{q}} - \epsilon_{\mathbf{q}-2\mathbf{k}}}{2}\right)^2} \right\} \Rightarrow \\
\left[\chi_0^{(4,4)}(\mathbf{k}, z)\right]_9 &= + \left(\frac{m}{\hbar^2}\right)^3 \frac{1}{18k^6} \int \frac{d^3q}{(2\pi)^3} 2f_0(\mathbf{q}) \left\{ \frac{9}{3\hbar z - \epsilon_{\mathbf{q}} + \epsilon_{\mathbf{q}-3\mathbf{k}}} - \frac{3}{\hbar z - \epsilon_{\mathbf{q}} + \epsilon_{\mathbf{q}-\mathbf{k}}} + \frac{24\epsilon_{\mathbf{k}}}{(2\hbar z - \epsilon_{\mathbf{q}} + \epsilon_{\mathbf{q}-2\mathbf{k}})^2} \right\}.
\end{aligned}$$

The *tenth contribution* is characterized by two simple poles and one double pole. This becomes apparrent from the algebraic identity  $(\epsilon_{\mathbf{q}+2\mathbf{k}} - \epsilon_{\mathbf{q}-2\mathbf{k}})/4 = (\epsilon_{\mathbf{q}+\mathbf{k}} - \epsilon_{\mathbf{q}-\mathbf{k}})/2$ . We first identify and calculate the coefficients  $a, b, c$ .

$$\begin{aligned}
\left[\chi_0^{(4,4)}(\mathbf{k}, z)\right]_{10} &= + \int \frac{d^3q}{(2\pi)^3} \frac{2f_0(\mathbf{q})}{(4\hbar z - \epsilon_{\mathbf{q}+2\mathbf{k}} + \epsilon_{\mathbf{q}-2\mathbf{k}})(3\hbar z - \epsilon_{\mathbf{q}+\mathbf{k}} + \epsilon_{\mathbf{q}-2\mathbf{k}})(2\hbar z - \epsilon_{\mathbf{q}+\mathbf{k}} + \epsilon_{\mathbf{q}-\mathbf{k}})(\hbar z - \epsilon_{\mathbf{q}+\mathbf{k}} + \epsilon_{\mathbf{q}})} \Rightarrow \\
\left[\chi_0^{(4,4)}(\mathbf{k}, z)\right]_{10} &= + \int \frac{d^3q}{(2\pi)^3} \frac{f_0(\mathbf{q})}{12} \frac{1}{\left[\hbar z - \frac{\epsilon_{\mathbf{q}+2\mathbf{k}} - \epsilon_{\mathbf{q}-2\mathbf{k}}}{4}\right] \left[\hbar z - \frac{\epsilon_{\mathbf{q}+\mathbf{k}} - \epsilon_{\mathbf{q}-2\mathbf{k}}}{3}\right] \left[\hbar z - \frac{\epsilon_{\mathbf{q}+\mathbf{k}} - \epsilon_{\mathbf{q}-\mathbf{k}}}{2}\right] [\hbar z - (\epsilon_{\mathbf{q}+\mathbf{k}} - \epsilon_{\mathbf{q}})]} \Rightarrow \\
\left[\chi_0^{(4,4)}(\mathbf{k}, z)\right]_{10} &= + \int \frac{d^3q}{(2\pi)^3} \frac{f_0(\mathbf{q})}{12} \frac{1}{\left[\hbar z - \frac{\epsilon_{\mathbf{q}+\mathbf{k}} - \epsilon_{\mathbf{q}-\mathbf{k}}}{2}\right] \left[\hbar z - \frac{\epsilon_{\mathbf{q}+\mathbf{k}} - \epsilon_{\mathbf{q}-2\mathbf{k}}}{3}\right] \left[\hbar z - \frac{\epsilon_{\mathbf{q}+\mathbf{k}} - \epsilon_{\mathbf{q}-\mathbf{k}}}{2}\right] [\hbar z - (\epsilon_{\mathbf{q}+\mathbf{k}} - \epsilon_{\mathbf{q}})]} \Rightarrow \\
\left[\chi_0^{(4,4)}(\mathbf{k}, z)\right]_{10} &= + \int \frac{d^3q}{(2\pi)^3} \frac{f_0(\mathbf{q})}{12} \frac{1}{\left[\hbar z - \frac{\epsilon_{\mathbf{q}+\mathbf{k}} - \epsilon_{\mathbf{q}-2\mathbf{k}}}{3}\right] [\hbar z - (\epsilon_{\mathbf{q}+\mathbf{k}} - \epsilon_{\mathbf{q}})] \left[\hbar z - \frac{\epsilon_{\mathbf{q}+\mathbf{k}} - \epsilon_{\mathbf{q}-\mathbf{k}}}{2}\right]^2} \Rightarrow \\
a = \frac{\epsilon_{\mathbf{q}+\mathbf{k}} - \epsilon_{\mathbf{q}-2\mathbf{k}}}{3} &= \frac{\hbar^2}{2m} \frac{(\mathbf{q} + \mathbf{k})^2 - (\mathbf{q} - 2\mathbf{k})^2}{3} = \frac{\hbar^2}{2m} \frac{k^2 + 2\mathbf{q} \cdot \mathbf{k} - 4k^2 + 4\mathbf{q} \cdot \mathbf{k}}{3} = \frac{\hbar^2}{2m} \frac{-3k^2 + 6\mathbf{q} \cdot \mathbf{k}}{3} = \frac{\hbar^2}{2m} (-k^2 + 2\mathbf{q} \cdot \mathbf{k}), \\
b = \epsilon_{\mathbf{q}+\mathbf{k}} - \epsilon_{\mathbf{q}} &= \frac{\hbar^2}{2m} [(\mathbf{q} + \mathbf{k})^2 - q^2] = \frac{\hbar^2}{2m} (k^2 + 2\mathbf{q} \cdot \mathbf{k}), \\
c = \frac{\epsilon_{\mathbf{q}+\mathbf{k}} - \epsilon_{\mathbf{q}-\mathbf{k}}}{2} &= \frac{\hbar^2}{2m} \frac{(\mathbf{q} + \mathbf{k})^2 - (\mathbf{q} - \mathbf{k})^2}{2} = \frac{\hbar^2}{2m} \frac{k^2 + 2\mathbf{q} \cdot \mathbf{k} - k^2 + 2\mathbf{q} \cdot \mathbf{k}}{2} = \frac{\hbar^2}{2m} \frac{4\mathbf{q} \cdot \mathbf{k}}{2} = \frac{\hbar^2}{2m} (2\mathbf{q} \cdot \mathbf{k}).
\end{aligned}$$

Then, we compute all the relevant differences between these three coefficients. Note that the  $q^2$  and  $\mathbf{q} \cdot \mathbf{k}$  terms vanish.

$$\begin{aligned}
a - b &= \frac{\hbar^2}{2m} (-k^2 + 2\mathbf{q} \cdot \mathbf{k} - k^2 - 2\mathbf{q} \cdot \mathbf{k}) = -\frac{\hbar^2}{2m} (2k^2), \\
a - c &= \frac{\hbar^2}{2m} (-k^2 + 2\mathbf{q} \cdot \mathbf{k} - 2\mathbf{q} \cdot \mathbf{k}) = -\frac{\hbar^2}{2m} (k^2), \\
b - c &= \frac{\hbar^2}{2m} (k^2 + 2\mathbf{q} \cdot \mathbf{k} - 2\mathbf{q} \cdot \mathbf{k}) = +\frac{\hbar^2}{2m} (k^2), \\
a + b - 2c &= \frac{\hbar^2}{2m} (-k^2 + 2\mathbf{q} \cdot \mathbf{k} + k^2 + 2\mathbf{q} \cdot \mathbf{k} - 4\mathbf{q} \cdot \mathbf{k}) = \frac{\hbar^2}{2m} (k^2 - k^2) = 0.
\end{aligned}$$

Afterwards, we compute all the algebraic combinations that are present in the partial fraction decomposition.

$$\begin{aligned}
(a - b)(a - c)^2 &= -\left(\frac{\hbar^2}{2m}\right)^3 (2k^2) (k^2)^2 = -\left(\frac{\hbar^2}{2m}\right)^3 (2k^6), \\
(a - b)(b - c)^2 &= -\left(\frac{\hbar^2}{2m}\right)^3 (2k^2) (k^2)^2 = -\left(\frac{\hbar^2}{2m}\right)^3 (2k^6), \\
(a - c)^2(b - c)^2 &= +\left(\frac{\hbar^2}{2m}\right)^4 (k^2)^2 (k^2)^2 = +\left(\frac{\hbar^2}{2m}\right)^4 (k^8), \\
(a - c)(b - c) &= -\left(\frac{\hbar^2}{2m}\right)^2 (k^2) (k^2) = -\left(\frac{\hbar^2}{2m}\right)^2 (k^4) = -\frac{1}{2k^2} \frac{2m}{\hbar^2} \left(\frac{\hbar^2}{2m}\right)^3 (2k^6).
\end{aligned}$$

Finally, we substitute and perform some algebra. We also introduce the compact notation  $\epsilon_{\mathbf{k}} = (\hbar^2 k^2)/(2m)$ .

$$\begin{aligned}
\left[\chi_0^{(4,4)}(\mathbf{k}, z)\right]_{10} &= - \int \frac{d^3q}{(2\pi)^3} \left(\frac{2m}{\hbar^2}\right)^3 \frac{f_0(\mathbf{q})}{12} \frac{1}{2k^6} \left\{ \frac{1}{\hbar z - \frac{\epsilon_{\mathbf{q}+\mathbf{k}} - \epsilon_{\mathbf{q}-2\mathbf{k}}}{3}} - \frac{1}{\hbar z - \epsilon_{\mathbf{q}+\mathbf{k}} + \epsilon_{\mathbf{q}}} + \frac{\hbar^2 k^2}{2m} \frac{2}{\left(\hbar z - \frac{\epsilon_{\mathbf{q}+\mathbf{k}} - \epsilon_{\mathbf{q}-\mathbf{k}}}{2}\right)^2} \right\} \Rightarrow \\
\left[\chi_0^{(4,4)}(\mathbf{k}, z)\right]_{10} &= -\left(\frac{m}{\hbar^2}\right)^3 \frac{1}{18k^6} \int \frac{d^3q}{(2\pi)^3} 2f_0(\mathbf{q}) \left\{ \frac{3}{\hbar z - \frac{\epsilon_{\mathbf{q}+\mathbf{k}} - \epsilon_{\mathbf{q}-2\mathbf{k}}}{3}} - \frac{3}{\hbar z - \epsilon_{\mathbf{q}+\mathbf{k}} + \epsilon_{\mathbf{q}}} + \frac{6\epsilon_{\mathbf{k}}}{\left(\hbar z - \frac{\epsilon_{\mathbf{q}+\mathbf{k}} - \epsilon_{\mathbf{q}-\mathbf{k}}}{2}\right)^2} \right\} \Rightarrow \\
\left[\chi_0^{(4,4)}(\mathbf{k}, z)\right]_{10} &= -\left(\frac{m}{\hbar^2}\right)^3 \frac{1}{18k^6} \int \frac{d^3q}{(2\pi)^3} 2f_0(\mathbf{q}) \left\{ \frac{9}{3\hbar z - \epsilon_{\mathbf{q}+\mathbf{k}} + \epsilon_{\mathbf{q}-2\mathbf{k}}} - \frac{3}{\hbar z - \epsilon_{\mathbf{q}+\mathbf{k}} + \epsilon_{\mathbf{q}}} + \frac{24\epsilon_{\mathbf{k}}}{(2\hbar z - \epsilon_{\mathbf{q}+\mathbf{k}} + \epsilon_{\mathbf{q}-\mathbf{k}})^2} \right\}.
\end{aligned}$$

The *eleventh contribution* is characterized by two double poles. This becomes apparrent from the algebraic identities  $(\epsilon_{\mathbf{q}+2\mathbf{k}} - \epsilon_{\mathbf{q}-2\mathbf{k}})/4 = (\epsilon_{\mathbf{q}+\mathbf{k}} - \epsilon_{\mathbf{q}-\mathbf{k}})/2$ ,  $(\epsilon_{\mathbf{q}+\mathbf{k}} - \epsilon_{\mathbf{q}-2\mathbf{k}})/3 = \epsilon_{\mathbf{q}} - \epsilon_{\mathbf{q}-\mathbf{k}}$ . We identify and calculate the coefficients  $a, b$ .

$$\begin{aligned}
[\chi_0^{(4,4)}(\mathbf{k}, z)]_{11} &= + \int \frac{d^3 q}{(2\pi)^3} \frac{2f_0(\mathbf{q})}{(4\hbar z - \epsilon_{\mathbf{q}+2\mathbf{k}} + \epsilon_{\mathbf{q}-2\mathbf{k}})(3\hbar z - \epsilon_{\mathbf{q}+\mathbf{k}} + \epsilon_{\mathbf{q}-2\mathbf{k}})(2\hbar z - \epsilon_{\mathbf{q}+\mathbf{k}} + \epsilon_{\mathbf{q}-\mathbf{k}})(\hbar z - \epsilon_{\mathbf{q}} + \epsilon_{\mathbf{q}-\mathbf{k}})} \Rightarrow \\
[\chi_0^{(4,4)}(\mathbf{k}, z)]_{11} &= + \int \frac{d^3 q}{(2\pi)^3} \frac{f_0(\mathbf{q})}{12} \frac{1}{\left[\hbar z - \frac{\epsilon_{\mathbf{q}+2\mathbf{k}} - \epsilon_{\mathbf{q}-2\mathbf{k}}}{4}\right] \left[\hbar z - \frac{\epsilon_{\mathbf{q}+\mathbf{k}} - \epsilon_{\mathbf{q}-2\mathbf{k}}}{3}\right] \left[\hbar z - \frac{\epsilon_{\mathbf{q}+\mathbf{k}} - \epsilon_{\mathbf{q}-\mathbf{k}}}{2}\right] [\hbar z - (\epsilon_{\mathbf{q}} - \epsilon_{\mathbf{q}-\mathbf{k}})]} \Rightarrow \\
[\chi_0^{(4,4)}(\mathbf{k}, z)]_{11} &= + \int \frac{d^3 q}{(2\pi)^3} \frac{f_0(\mathbf{q})}{12} \frac{1}{\left[\hbar z - \frac{\epsilon_{\mathbf{q}+\mathbf{k}} - \epsilon_{\mathbf{q}-\mathbf{k}}}{2}\right] [\hbar z - (\epsilon_{\mathbf{q}} - \epsilon_{\mathbf{q}-\mathbf{k}})] \left[\hbar z - \frac{\epsilon_{\mathbf{q}+\mathbf{k}} - \epsilon_{\mathbf{q}-\mathbf{k}}}{2}\right] [\hbar z - (\epsilon_{\mathbf{q}} - \epsilon_{\mathbf{q}-\mathbf{k}})]} \Rightarrow \\
[\chi_0^{(4,4)}(\mathbf{k}, z)]_{11} &= + \int \frac{d^3 q}{(2\pi)^3} \frac{f_0(\mathbf{q})}{12} \frac{1}{\left[\hbar z - \frac{\epsilon_{\mathbf{q}+\mathbf{k}} - \epsilon_{\mathbf{q}-\mathbf{k}}}{2}\right]^2 [\hbar z - (\epsilon_{\mathbf{q}} - \epsilon_{\mathbf{q}-\mathbf{k}})]^2} \Rightarrow \\
a = \frac{\epsilon_{\mathbf{q}+\mathbf{k}} - \epsilon_{\mathbf{q}-\mathbf{k}}}{2} &= \frac{\hbar^2}{2m} \frac{(\mathbf{q} + \mathbf{k})^2 - (\mathbf{q} - \mathbf{k})^2}{2} = \frac{\hbar^2}{2m} \frac{k^2 + 2\mathbf{q} \cdot \mathbf{k} - k^2 + 2\mathbf{q} \cdot \mathbf{k}}{2} = \frac{\hbar^2}{2m} \frac{4\mathbf{q} \cdot \mathbf{k}}{2} = \frac{\hbar^2}{2m} (2\mathbf{q} \cdot \mathbf{k}) \\
b = \epsilon_{\mathbf{q}} - \epsilon_{\mathbf{q}-\mathbf{k}} &= \frac{\hbar^2}{2m} [q^2 - (\mathbf{q} - \mathbf{k})^2] = \frac{\hbar^2}{2m} (-k^2 + 2\mathbf{q} \cdot \mathbf{k}) .
\end{aligned}$$

Then, we compute all the difference between the two coefficients, as well as the difference's square and cube. Note that the  $q^2$  and  $\mathbf{q} \cdot \mathbf{k}$  terms vanish.

$$\begin{aligned}
(a - b) &= \frac{\hbar^2}{2m} (2\mathbf{q} \cdot \mathbf{k} + k^2 - 2\mathbf{q} \cdot \mathbf{k}) = \frac{\hbar^2}{2m} (k^2) , \\
(a - b)^2 &= \left(\frac{\hbar^2}{2m}\right)^2 (k^4) , \\
(a - b)^3 &= \left(\frac{\hbar^2}{2m}\right)^3 (k^6) .
\end{aligned}$$

Finally, we substitute the above in the contribution and also perform some straightforward algebra. We introduce the compact notation  $\epsilon_{\mathbf{k}} = (\hbar^2 k^2)/(2m)$  for brevity.

$$\begin{aligned}
[\chi_0^{(4,4)}(\mathbf{k}, z)]_{11} &= + \int \frac{d^3 q}{(2\pi)^3} \left(\frac{2m}{\hbar^2}\right)^3 \frac{f_0(\mathbf{q})}{12k^6} \left\{ \frac{2}{\hbar z - \epsilon_{\mathbf{q}} + \epsilon_{\mathbf{q}-\mathbf{k}}} - \frac{2}{\hbar z - \frac{\epsilon_{\mathbf{q}+\mathbf{k}} - \epsilon_{\mathbf{q}-\mathbf{k}}}{2}} + \frac{\hbar^2 k^2}{2m} \frac{1}{(\hbar z - \epsilon_{\mathbf{q}} + \epsilon_{\mathbf{q}-\mathbf{k}})^2} + \frac{\hbar^2 k^2}{2m} \frac{1}{\left(\hbar z - \frac{\epsilon_{\mathbf{q}+\mathbf{k}} - \epsilon_{\mathbf{q}-\mathbf{k}}}{2}\right)^2} \right\} \\
[\chi_0^{(4,4)}(\mathbf{k}, z)]_{11} &= + \int \frac{d^3 q}{(2\pi)^3} \left(\frac{2m}{\hbar^2}\right)^3 \frac{f_0(\mathbf{q})}{12k^6} \left\{ \frac{2}{\hbar z - \epsilon_{\mathbf{q}} + \epsilon_{\mathbf{q}-\mathbf{k}}} - \frac{2}{\hbar z - \frac{\epsilon_{\mathbf{q}+\mathbf{k}} - \epsilon_{\mathbf{q}-\mathbf{k}}}{2}} + \frac{\epsilon_{\mathbf{k}}}{(\hbar z - \epsilon_{\mathbf{q}} + \epsilon_{\mathbf{q}-\mathbf{k}})^2} + \frac{\epsilon_{\mathbf{k}}}{\left(\hbar z - \frac{\epsilon_{\mathbf{q}+\mathbf{k}} - \epsilon_{\mathbf{q}-\mathbf{k}}}{2}\right)^2} \right\} \\
[\chi_0^{(4,4)}(\mathbf{k}, z)]_{11} &= + \int \frac{d^3 q}{(2\pi)^3} \left(\frac{m}{\hbar^2}\right)^3 \frac{8f_0(\mathbf{q})}{12k^6} \left\{ \frac{2}{\hbar z - \epsilon_{\mathbf{q}} + \epsilon_{\mathbf{q}-\mathbf{k}}} - \frac{2}{\hbar z - \frac{\epsilon_{\mathbf{q}+\mathbf{k}} - \epsilon_{\mathbf{q}-\mathbf{k}}}{2}} + \frac{\epsilon_{\mathbf{k}}}{(\hbar z - \epsilon_{\mathbf{q}} + \epsilon_{\mathbf{q}-\mathbf{k}})^2} + \frac{\epsilon_{\mathbf{k}}}{\left(\hbar z - \frac{\epsilon_{\mathbf{q}+\mathbf{k}} - \epsilon_{\mathbf{q}-\mathbf{k}}}{2}\right)^2} \right\} \\
[\chi_0^{(4,4)}(\mathbf{k}, z)]_{11} &= + \int \frac{d^3 q}{(2\pi)^3} \left(\frac{m}{\hbar^2}\right)^3 \frac{2f_0(\mathbf{q})}{3k^6} \left\{ \frac{2}{\hbar z - \epsilon_{\mathbf{q}} + \epsilon_{\mathbf{q}-\mathbf{k}}} - \frac{2}{\hbar z - \frac{\epsilon_{\mathbf{q}+\mathbf{k}} - \epsilon_{\mathbf{q}-\mathbf{k}}}{2}} + \frac{\epsilon_{\mathbf{k}}}{(\hbar z - \epsilon_{\mathbf{q}} + \epsilon_{\mathbf{q}-\mathbf{k}})^2} + \frac{\epsilon_{\mathbf{k}}}{\left(\hbar z - \frac{\epsilon_{\mathbf{q}+\mathbf{k}} - \epsilon_{\mathbf{q}-\mathbf{k}}}{2}\right)^2} \right\} \\
[\chi_0^{(4,4)}(\mathbf{k}, z)]_{11} &= + \left(\frac{m}{\hbar^2}\right)^3 \frac{1}{3k^6} \int \frac{d^3 q}{(2\pi)^3} 2f_0(\mathbf{q}) \left\{ \frac{2}{\hbar z - \epsilon_{\mathbf{q}} + \epsilon_{\mathbf{q}-\mathbf{k}}} - \frac{2}{\hbar z - \frac{\epsilon_{\mathbf{q}+\mathbf{k}} - \epsilon_{\mathbf{q}-\mathbf{k}}}{2}} + \frac{\epsilon_{\mathbf{k}}}{(\hbar z - \epsilon_{\mathbf{q}} + \epsilon_{\mathbf{q}-\mathbf{k}})^2} + \frac{\epsilon_{\mathbf{k}}}{\left(\hbar z - \frac{\epsilon_{\mathbf{q}+\mathbf{k}} - \epsilon_{\mathbf{q}-\mathbf{k}}}{2}\right)^2} \right\} \\
[\chi_0^{(4,4)}(\mathbf{k}, z)]_{11} &= + \left(\frac{m}{\hbar^2}\right)^3 \frac{1}{18k^6} \int \frac{d^3 q}{(2\pi)^3} 2f_0(\mathbf{q}) \left\{ \frac{12}{\hbar z - \epsilon_{\mathbf{q}} + \epsilon_{\mathbf{q}-\mathbf{k}}} - \frac{24}{2\hbar z - \epsilon_{\mathbf{q}+\mathbf{k}} + \epsilon_{\mathbf{q}-\mathbf{k}}} + \frac{6\epsilon_{\mathbf{k}}}{(\hbar z - \epsilon_{\mathbf{q}} + \epsilon_{\mathbf{q}-\mathbf{k}})^2} + \frac{24\epsilon_{\mathbf{k}}}{(2\hbar z - \epsilon_{\mathbf{q}+\mathbf{k}} + \epsilon_{\mathbf{q}-\mathbf{k}})^2} \right\}
\end{aligned}$$



The *twelfth contribution* is characterized by two double poles. This becomes apparrent from the algebraic identities  $(\epsilon_{\mathbf{q}+3\mathbf{k}} - \epsilon_{\mathbf{q}-\mathbf{k}})/4 = (\epsilon_{\mathbf{q}+2\mathbf{k}} - \epsilon_{\mathbf{q}})/2$ ,  $(\epsilon_{\mathbf{q}+2\mathbf{k}} - \epsilon_{\mathbf{q}-\mathbf{k}})/3 = \epsilon_{\mathbf{q}+\mathbf{k}} - \epsilon_{\mathbf{q}}$ . We identify and calculate the coefficients  $a, b$ .

$$\begin{aligned}
\left[\chi_0^{(4,4)}(\mathbf{k}, z)\right]_{12} &= - \int \frac{d^3q}{(2\pi)^3} \frac{2f_0(\mathbf{q})}{(4\hbar z - \epsilon_{\mathbf{q}+3\mathbf{k}} + \epsilon_{\mathbf{q}-\mathbf{k}})(3\hbar z - \epsilon_{\mathbf{q}+2\mathbf{k}} + \epsilon_{\mathbf{q}-\mathbf{k}})(2\hbar z - \epsilon_{\mathbf{q}+2\mathbf{k}} + \epsilon_{\mathbf{q}})(\hbar z - \epsilon_{\mathbf{q}+\mathbf{k}} + \epsilon_{\mathbf{q}})} \Rightarrow \\
\left[\chi_0^{(4,4)}(\mathbf{k}, z)\right]_{12} &= - \int \frac{d^3q}{(2\pi)^3} \frac{f_0(\mathbf{q})}{12} \frac{1}{\left[\hbar z - \frac{\epsilon_{\mathbf{q}+3\mathbf{k}} - \epsilon_{\mathbf{q}-\mathbf{k}}}{4}\right] \left[\hbar z - \frac{\epsilon_{\mathbf{q}+2\mathbf{k}} - \epsilon_{\mathbf{q}-\mathbf{k}}}{3}\right] \left[\hbar z - \frac{\epsilon_{\mathbf{q}+2\mathbf{k}} - \epsilon_{\mathbf{q}}}{2}\right] [\hbar z - (\epsilon_{\mathbf{q}+\mathbf{k}} - \epsilon_{\mathbf{q}})]} \Rightarrow \\
\left[\chi_0^{(4,4)}(\mathbf{k}, z)\right]_{12} &= - \int \frac{d^3q}{(2\pi)^3} \frac{f_0(\mathbf{q})}{12} \frac{1}{\left[\hbar z - \frac{\epsilon_{\mathbf{q}+2\mathbf{k}} - \epsilon_{\mathbf{q}}}{2}\right] [\hbar z - (\epsilon_{\mathbf{q}+\mathbf{k}} - \epsilon_{\mathbf{q}})] \left[\hbar z - \frac{\epsilon_{\mathbf{q}+2\mathbf{k}} - \epsilon_{\mathbf{q}}}{2}\right] [\hbar z - (\epsilon_{\mathbf{q}+\mathbf{k}} - \epsilon_{\mathbf{q}})]} \Rightarrow \\
\left[\chi_0^{(4,4)}(\mathbf{k}, z)\right]_{12} &= - \int \frac{d^3q}{(2\pi)^3} \frac{f_0(\mathbf{q})}{12} \frac{1}{[\hbar z - (\epsilon_{\mathbf{q}+\mathbf{k}} - \epsilon_{\mathbf{q}})]^2 \left[\hbar z - \frac{\epsilon_{\mathbf{q}+2\mathbf{k}} - \epsilon_{\mathbf{q}}}{2}\right]^2} \Rightarrow \\
a = \frac{\epsilon_{\mathbf{q}+2\mathbf{k}} - \epsilon_{\mathbf{q}}}{2} &= \frac{\hbar^2}{2m} \frac{(\mathbf{q} + 2\mathbf{k})^2 - q^2}{2} = \frac{\hbar^2}{2m} \frac{4k^2 + 4\mathbf{q} \cdot \mathbf{k}}{2} = \frac{\hbar^2}{2m} (2k^2 + 2\mathbf{q} \cdot \mathbf{k}) , \\
b = \epsilon_{\mathbf{q}+\mathbf{k}} - \epsilon_{\mathbf{q}} &= \frac{\hbar^2}{2m} [(\mathbf{q} + \mathbf{k})^2 - q^2] = \frac{\hbar^2}{2m} (k^2 + 2\mathbf{q} \cdot \mathbf{k}) .
\end{aligned}$$

Then, we compute all the difference between the two coefficients, as well as the difference's square and cube. Note that the  $q^2$  and  $\mathbf{q} \cdot \mathbf{k}$  terms vanish.

$$\begin{aligned}
(a - b) &= \frac{\hbar^2}{2m} (2k^2 + 2\mathbf{q} \cdot \mathbf{k} - k^2 - 2\mathbf{q} \cdot \mathbf{k}) = \frac{\hbar^2}{2m} (2k^2 - k^2) = \frac{\hbar^2}{2m} (k^2) , \\
(a - b)^2 &= \left(\frac{\hbar^2}{2m}\right)^2 (k^4) , \\
(a - b)^3 &= \left(\frac{\hbar^2}{2m}\right)^3 (k^6) .
\end{aligned}$$

Finally, we substitute the above in the contribution and also perform some straightforward algebra. We introduce the compact notation  $\epsilon_{\mathbf{k}} = (\hbar^2 k^2)/(2m)$  for brevity.

$$\begin{aligned}
\left[\chi_0^{(4,4)}(\mathbf{k}, z)\right]_{12} &= - \int \frac{d^3q}{(2\pi)^3} \left(\frac{2m}{\hbar^2}\right)^3 \frac{f_0(\mathbf{q})}{12k^6} \left\{ \frac{2}{\hbar z - \epsilon_{\mathbf{q}+\mathbf{k}} + \epsilon_{\mathbf{q}}} - \frac{2}{\hbar z - \frac{\epsilon_{\mathbf{q}+2\mathbf{k}} - \epsilon_{\mathbf{q}}}{2}} + \frac{\hbar^2 k^2}{2m} \frac{1}{(\hbar z - \epsilon_{\mathbf{q}+\mathbf{k}} + \epsilon_{\mathbf{q}})^2} + \frac{\hbar^2 k^2}{2m} \frac{1}{\left(\hbar z - \frac{\epsilon_{\mathbf{q}+2\mathbf{k}} - \epsilon_{\mathbf{q}}}{2}\right)^2} \right\} = \\
\left[\chi_0^{(4,4)}(\mathbf{k}, z)\right]_{12} &= - \int \frac{d^3q}{(2\pi)^3} \left(\frac{2m}{\hbar^2}\right)^3 \frac{f_0(\mathbf{q})}{12k^6} \left\{ \frac{2}{\hbar z - \epsilon_{\mathbf{q}+\mathbf{k}} + \epsilon_{\mathbf{q}}} - \frac{2}{\hbar z - \frac{\epsilon_{\mathbf{q}+2\mathbf{k}} - \epsilon_{\mathbf{q}}}{2}} + \frac{\epsilon_{\mathbf{k}}}{(\hbar z - \epsilon_{\mathbf{q}+\mathbf{k}} + \epsilon_{\mathbf{q}})^2} + \frac{\epsilon_{\mathbf{k}}}{\left(\hbar z - \frac{\epsilon_{\mathbf{q}+2\mathbf{k}} - \epsilon_{\mathbf{q}}}{2}\right)^2} \right\} = \\
\left[\chi_0^{(4,4)}(\mathbf{k}, z)\right]_{12} &= - \int \frac{d^3q}{(2\pi)^3} \left(\frac{m}{\hbar^2}\right)^3 \frac{8f_0(\mathbf{q})}{12k^6} \left\{ \frac{2}{\hbar z - \epsilon_{\mathbf{q}+\mathbf{k}} + \epsilon_{\mathbf{q}}} - \frac{2}{\hbar z - \frac{\epsilon_{\mathbf{q}+2\mathbf{k}} - \epsilon_{\mathbf{q}}}{2}} + \frac{\epsilon_{\mathbf{k}}}{(\hbar z - \epsilon_{\mathbf{q}+\mathbf{k}} + \epsilon_{\mathbf{q}})^2} + \frac{\epsilon_{\mathbf{k}}}{\left(\hbar z - \frac{\epsilon_{\mathbf{q}+2\mathbf{k}} - \epsilon_{\mathbf{q}}}{2}\right)^2} \right\} = \\
\left[\chi_0^{(4,4)}(\mathbf{k}, z)\right]_{12} &= - \int \frac{d^3q}{(2\pi)^3} \left(\frac{m}{\hbar^2}\right)^3 \frac{2f_0(\mathbf{q})}{3k^6} \left\{ \frac{2}{\hbar z - \epsilon_{\mathbf{q}+\mathbf{k}} + \epsilon_{\mathbf{q}}} - \frac{2}{\hbar z - \frac{\epsilon_{\mathbf{q}+2\mathbf{k}} - \epsilon_{\mathbf{q}}}{2}} + \frac{\epsilon_{\mathbf{k}}}{(\hbar z - \epsilon_{\mathbf{q}+\mathbf{k}} + \epsilon_{\mathbf{q}})^2} + \frac{\epsilon_{\mathbf{k}}}{\left(\hbar z - \frac{\epsilon_{\mathbf{q}+2\mathbf{k}} - \epsilon_{\mathbf{q}}}{2}\right)^2} \right\} = \\
\left[\chi_0^{(4,4)}(\mathbf{k}, z)\right]_{12} &= - \left(\frac{m}{\hbar^2}\right)^3 \frac{1}{3k^6} \int \frac{d^3q}{(2\pi)^3} 2f_0(\mathbf{q}) \left\{ \frac{2}{\hbar z - \epsilon_{\mathbf{q}+\mathbf{k}} + \epsilon_{\mathbf{q}}} - \frac{2}{\hbar z - \frac{\epsilon_{\mathbf{q}+2\mathbf{k}} - \epsilon_{\mathbf{q}}}{2}} + \frac{\epsilon_{\mathbf{k}}}{(\hbar z - \epsilon_{\mathbf{q}+\mathbf{k}} + \epsilon_{\mathbf{q}})^2} + \frac{\epsilon_{\mathbf{k}}}{\left(\hbar z - \frac{\epsilon_{\mathbf{q}+2\mathbf{k}} - \epsilon_{\mathbf{q}}}{2}\right)^2} \right\} = \\
\left[\chi_0^{(4,4)}(\mathbf{k}, z)\right]_{12} &= - \left(\frac{m}{\hbar^2}\right)^3 \frac{1}{18k^6} \int \frac{d^3q}{(2\pi)^3} 2f_0(\mathbf{q}) \left\{ \frac{12}{\hbar z - \epsilon_{\mathbf{q}+\mathbf{k}} + \epsilon_{\mathbf{q}}} - \frac{24}{2\hbar z - \epsilon_{\mathbf{q}+2\mathbf{k}} + \epsilon_{\mathbf{q}}} + \frac{6\epsilon_{\mathbf{k}}}{(\hbar z - \epsilon_{\mathbf{q}+\mathbf{k}} + \epsilon_{\mathbf{q}})^2} + \frac{24\epsilon_{\mathbf{k}}}{(2\hbar z - \epsilon_{\mathbf{q}+2\mathbf{k}} + \epsilon_{\mathbf{q}})^2} \right\} =
\end{aligned}$$

The *thirteenth contribution* is characterized by two simple poles and one double pole. This becomes apparant from the algebraic identity  $(\epsilon_{\mathbf{q}+\mathbf{k}} - \epsilon_{\mathbf{q}-2\mathbf{k}})/3 = \epsilon_{\mathbf{q}} - \epsilon_{\mathbf{q}-\mathbf{k}}$ . We first identify and calculate the coefficients  $a, b, c$ .

$$\begin{aligned}
\left[\chi_0^{(4,4)}(\mathbf{k}, z)\right]_{13} &= + \int \frac{d^3q}{(2\pi)^3} \frac{2f_0(\mathbf{q})}{(4\hbar z - \epsilon_{\mathbf{q}+2\mathbf{k}} + \epsilon_{\mathbf{q}-2\mathbf{k}})(3\hbar z - \epsilon_{\mathbf{q}+\mathbf{k}} + \epsilon_{\mathbf{q}-2\mathbf{k}})(2\hbar z - \epsilon_{\mathbf{q}} + \epsilon_{\mathbf{q}-2\mathbf{k}})(\hbar z - \epsilon_{\mathbf{q}} + \epsilon_{\mathbf{q}-\mathbf{k}})} \Rightarrow \\
\left[\chi_0^{(4,4)}(\mathbf{k}, z)\right]_{13} &= + \int \frac{d^3q}{(2\pi)^3} \frac{f_0(\mathbf{q})}{12} \frac{1}{\left[\hbar z - \frac{\epsilon_{\mathbf{q}+2\mathbf{k}} - \epsilon_{\mathbf{q}-2\mathbf{k}}}{4}\right] \left[\hbar z - \frac{\epsilon_{\mathbf{q}+\mathbf{k}} - \epsilon_{\mathbf{q}-2\mathbf{k}}}{3}\right] \left[\hbar z - \frac{\epsilon_{\mathbf{q}} - \epsilon_{\mathbf{q}-2\mathbf{k}}}{2}\right] [\hbar z - (\epsilon_{\mathbf{q}} - \epsilon_{\mathbf{q}-\mathbf{k}})]} \Rightarrow \\
\left[\chi_0^{(4,4)}(\mathbf{k}, z)\right]_{13} &= + \int \frac{d^3q}{(2\pi)^3} \frac{f_0(\mathbf{q})}{12} \frac{1}{\left[\hbar z - \frac{\epsilon_{\mathbf{q}+2\mathbf{k}} - \epsilon_{\mathbf{q}-2\mathbf{k}}}{4}\right] [\hbar z - (\epsilon_{\mathbf{q}} - \epsilon_{\mathbf{q}-\mathbf{k}})] \left[\hbar z - \frac{\epsilon_{\mathbf{q}} - \epsilon_{\mathbf{q}-2\mathbf{k}}}{2}\right] [\hbar z - (\epsilon_{\mathbf{q}} - \epsilon_{\mathbf{q}-\mathbf{k}})]} \Rightarrow \\
\left[\chi_0^{(4,4)}(\mathbf{k}, z)\right]_{13} &= + \int \frac{d^3q}{(2\pi)^3} \frac{f_0(\mathbf{q})}{12} \frac{1}{\left[\hbar z - \frac{\epsilon_{\mathbf{q}+2\mathbf{k}} - \epsilon_{\mathbf{q}-2\mathbf{k}}}{4}\right] \left[\hbar z - \frac{\epsilon_{\mathbf{q}} - \epsilon_{\mathbf{q}-2\mathbf{k}}}{2}\right] [\hbar z - (\epsilon_{\mathbf{q}} - \epsilon_{\mathbf{q}-\mathbf{k}})]^2} \Rightarrow \\
a = \frac{\epsilon_{\mathbf{q}+2\mathbf{k}} - \epsilon_{\mathbf{q}-2\mathbf{k}}}{4} &= \frac{\hbar^2}{2m} \frac{(\mathbf{q} + 2\mathbf{k})^2 - (\mathbf{q} - 2\mathbf{k})^2}{4} = \frac{\hbar^2}{2m} \frac{4k^2 + 4\mathbf{q} \cdot \mathbf{k} - 4k^2 + 4\mathbf{q} \cdot \mathbf{k}}{4} = \frac{\hbar^2}{2m} \frac{8\mathbf{q} \cdot \mathbf{k}}{4} = \frac{\hbar^2}{2m} (2\mathbf{q} \cdot \mathbf{k}) , \\
b = \frac{\epsilon_{\mathbf{q}} - \epsilon_{\mathbf{q}-2\mathbf{k}}}{2} &= \frac{\hbar^2}{2m} \frac{q^2 - (\mathbf{q} - 2\mathbf{k})^2}{2} = \frac{\hbar^2}{2m} \frac{-4k^2 + 4\mathbf{q} \cdot \mathbf{k}}{2} = \frac{\hbar^2}{2m} (-2k^2 + 2\mathbf{q} \cdot \mathbf{k}) , \\
c = \epsilon_{\mathbf{q}} - \epsilon_{\mathbf{q}-\mathbf{k}} &= \frac{\hbar^2}{2m} [q^2 - (\mathbf{q} - \mathbf{k})^2] = \frac{\hbar^2}{2m} (-k^2 + 2\mathbf{q} \cdot \mathbf{k}) .
\end{aligned}$$

Then, we compute all the relevant differences between these three coefficients. Note that the  $q^2$  and  $\mathbf{q} \cdot \mathbf{k}$  terms vanish.

$$\begin{aligned}
a - b &= \frac{\hbar^2}{2m} (2\mathbf{q} \cdot \mathbf{k} + 2k^2 - 2\mathbf{q} \cdot \mathbf{k}) = \frac{\hbar^2}{2m} (2k^2) , \\
a - c &= \frac{\hbar^2}{2m} (2\mathbf{q} \cdot \mathbf{k} + k^2 - 2\mathbf{q} \cdot \mathbf{k}) = \frac{\hbar^2}{2m} (k^2) , \\
b - c &= \frac{\hbar^2}{2m} (-2k^2 + 2\mathbf{q} \cdot \mathbf{k} + k^2 - 2\mathbf{q} \cdot \mathbf{k}) = \frac{\hbar^2}{2m} (-2k^2 + k^2) = -\frac{\hbar^2}{2m} (k^2) , \\
a + b - 2c &= \frac{\hbar^2}{2m} (2\mathbf{q} \cdot \mathbf{k} - 2k^2 + 2\mathbf{q} \cdot \mathbf{k} + 2k^2 - 4\mathbf{q} \cdot \mathbf{k}) = \frac{\hbar^2}{2m} (-2k^2 + 2k^2) = 0 .
\end{aligned}$$

Afterwards, we compute all the algebraic combinations that are present in the partial fraction decomposition.

$$\begin{aligned}
(a - b)(a - c)^2 &= + \left(\frac{\hbar^2}{2m}\right)^3 (2k^2) (k^2)^2 = + \left(\frac{\hbar^2}{2m}\right)^3 (2k^6) , \\
(a - b)(b - c)^2 &= + \left(\frac{\hbar^2}{2m}\right)^3 (2k^2) (k^2)^2 = + \left(\frac{\hbar^2}{2m}\right)^3 (2k^6) , \\
(a - c)^2(b - c)^2 &= + \left(\frac{\hbar^2}{2m}\right)^4 (k^2)^2 (k^2)^2 = + \left(\frac{\hbar^2}{2m}\right)^4 (k^8) , \\
(a - c)(b - c) &= - \left(\frac{\hbar^2}{2m}\right)^2 (k^2) (k^2) = - \left(\frac{\hbar^2}{2m}\right)^2 (k^4) = - \frac{1}{2k^2} \frac{2m}{\hbar^2} \left(\frac{\hbar^2}{2m}\right)^3 (2k^6) .
\end{aligned}$$

Finally, we substitute and perform some algebra. We also introduce the compact notation  $\epsilon_{\mathbf{k}} = (\hbar^2 k^2)/(2m)$ .

$$\begin{aligned}
\left[\chi_0^{(4,4)}(\mathbf{k}, z)\right]_{13} &= + \int \frac{d^3q}{(2\pi)^3} \left(\frac{2m}{\hbar^2}\right)^3 \frac{f_0(\mathbf{q})}{12} \frac{1}{2k^6} \left\{ \frac{1}{\hbar z - \frac{\epsilon_{\mathbf{q}+2\mathbf{k}} - \epsilon_{\mathbf{q}-2\mathbf{k}}}{4}} - \frac{1}{\hbar z - \frac{\epsilon_{\mathbf{q}} - \epsilon_{\mathbf{q}-2\mathbf{k}}}{2}} - \frac{\hbar^2 k^2}{2m} \frac{2}{(\hbar z - \epsilon_{\mathbf{q}} + \epsilon_{\mathbf{q}-\mathbf{k}})^2} \right\} \Rightarrow \\
\left[\chi_0^{(4,4)}(\mathbf{k}, z)\right]_{13} &= + \int \frac{d^3q}{(2\pi)^3} \left(\frac{2m}{\hbar^2}\right)^3 \frac{f_0(\mathbf{q})}{12} \frac{1}{2k^6} \left\{ \frac{1}{\hbar z - \frac{\epsilon_{\mathbf{q}+2\mathbf{k}} - \epsilon_{\mathbf{q}-2\mathbf{k}}}{4}} - \frac{1}{\hbar z - \frac{\epsilon_{\mathbf{q}} - \epsilon_{\mathbf{q}-2\mathbf{k}}}{2}} - \frac{2\epsilon_{\mathbf{k}}}{(\hbar z - \epsilon_{\mathbf{q}} + \epsilon_{\mathbf{q}-\mathbf{k}})^2} \right\} \Rightarrow \\
\left[\chi_0^{(4,4)}(\mathbf{k}, z)\right]_{13} &= + \left(\frac{m}{\hbar^2}\right)^3 \frac{1}{18k^6} \int \frac{d^3q}{(2\pi)^3} 2f_0(\mathbf{q}) \left\{ \frac{3}{\hbar z - \frac{\epsilon_{\mathbf{q}+2\mathbf{k}} - \epsilon_{\mathbf{q}-2\mathbf{k}}}{4}} - \frac{3}{\hbar z - \frac{\epsilon_{\mathbf{q}} - \epsilon_{\mathbf{q}-2\mathbf{k}}}{2}} - \frac{6\epsilon_{\mathbf{k}}}{(\hbar z - \epsilon_{\mathbf{q}} + \epsilon_{\mathbf{q}-\mathbf{k}})^2} \right\} \Rightarrow \\
\left[\chi_0^{(4,4)}(\mathbf{k}, z)\right]_{13} &= + \left(\frac{m}{\hbar^2}\right)^3 \frac{1}{18k^6} \int \frac{d^3q}{(2\pi)^3} 2f_0(\mathbf{q}) \left\{ \frac{12}{4\hbar z - \epsilon_{\mathbf{q}+2\mathbf{k}} + \epsilon_{\mathbf{q}-2\mathbf{k}}} - \frac{6}{2\hbar z - \epsilon_{\mathbf{q}} + \epsilon_{\mathbf{q}-2\mathbf{k}}} - \frac{6\epsilon_{\mathbf{k}}}{(\hbar z - \epsilon_{\mathbf{q}} + \epsilon_{\mathbf{q}-\mathbf{k}})^2} \right\} .
\end{aligned}$$

The *fourteenth contribution* is characterized by two simple poles and one double pole. This becomes apparant from the algebraic identity  $(\epsilon_{q+2k} - \epsilon_{q-k})/3 = \epsilon_{q+k} - \epsilon_q$ . We first identify and calculate the coefficients  $a, b, c$ .

$$\begin{aligned}
\left[\chi_0^{(4,4)}(\mathbf{k}, z)\right]_{14} &= - \int \frac{d^3q}{(2\pi)^3} \frac{2f_0(\mathbf{q})}{(4\hbar z - \epsilon_{q+3k} + \epsilon_{q-k})(3\hbar z - \epsilon_{q+2k} + \epsilon_{q-k})(2\hbar z - \epsilon_{q+k} + \epsilon_{q-k})(\hbar z - \epsilon_{q+k} + \epsilon_q)} \Rightarrow \\
\left[\chi_0^{(4,4)}(\mathbf{k}, z)\right]_{14} &= - \int \frac{d^3q}{(2\pi)^3} \frac{f_0(\mathbf{q})}{12} \frac{1}{\left[\hbar z - \frac{\epsilon_{q+3k} - \epsilon_{q-k}}{4}\right] \left[\hbar z - \frac{\epsilon_{q+2k} - \epsilon_{q-k}}{3}\right] \left[\hbar z - \frac{\epsilon_{q+k} - \epsilon_q}{2}\right] [\hbar z - (\epsilon_{q+k} - \epsilon_q)]} \Rightarrow \\
\left[\chi_0^{(4,4)}(\mathbf{k}, z)\right]_{14} &= - \int \frac{d^3q}{(2\pi)^3} \frac{f_0(\mathbf{q})}{12} \frac{1}{\left[\hbar z - \frac{\epsilon_{q+3k} - \epsilon_{q-k}}{4}\right] [\hbar z - (\epsilon_{q+k} - \epsilon_q)] \left[\hbar z - \frac{\epsilon_{q+k} - \epsilon_q}{2}\right] [\hbar z - (\epsilon_{q+k} - \epsilon_q)]} \Rightarrow \\
\left[\chi_0^{(4,4)}(\mathbf{k}, z)\right]_{14} &= - \int \frac{d^3q}{(2\pi)^3} \frac{f_0(\mathbf{q})}{12} \frac{1}{\left[\hbar z - \frac{\epsilon_{q+3k} - \epsilon_{q-k}}{4}\right] \left[\hbar z - \frac{\epsilon_{q+k} - \epsilon_q}{2}\right] [\hbar z - (\epsilon_{q+k} - \epsilon_q)]^2} \Rightarrow \\
a = \frac{\epsilon_{q+3k} - \epsilon_{q-k}}{4} &= \frac{\hbar^2}{2m} \frac{(\mathbf{q} + 3\mathbf{k})^2 - (\mathbf{q} - \mathbf{k})^2}{4} = \frac{\hbar^2}{2m} \frac{9k^2 + 6\mathbf{q} \cdot \mathbf{k} - k^2 + 2\mathbf{q} \cdot \mathbf{k}}{4} = \frac{\hbar^2}{2m} \frac{8k^2 + 8\mathbf{q} \cdot \mathbf{k}}{4} = \frac{\hbar^2}{2m} (2k^2 + 2\mathbf{q} \cdot \mathbf{k}) , \\
b = \frac{\epsilon_{q+k} - \epsilon_{q-k}}{2} &= \frac{\hbar^2}{2m} \frac{(\mathbf{q} + \mathbf{k})^2 - (\mathbf{q} - \mathbf{k})^2}{2} = \frac{\hbar^2}{2m} \frac{k^2 + 2\mathbf{q} \cdot \mathbf{k} - k^2 + 2\mathbf{q} \cdot \mathbf{k}}{2} = \frac{\hbar^2}{2m} \frac{4\mathbf{q} \cdot \mathbf{k}}{2} = \frac{\hbar^2}{2m} (2\mathbf{q} \cdot \mathbf{k}) , \\
c = \epsilon_{q+k} - \epsilon_q &= \frac{\hbar^2}{2m} [(\mathbf{q} + \mathbf{k})^2 - q^2] = \frac{\hbar^2}{2m} (k^2 + 2\mathbf{q} \cdot \mathbf{k}) .
\end{aligned}$$

Then, we compute all the relevant differences between these three coefficients. Note that the  $q^2$  and  $\mathbf{q} \cdot \mathbf{k}$  terms vanish.

$$\begin{aligned}
a - b &= \frac{\hbar^2}{2m} (2k^2 + 2\mathbf{q} \cdot \mathbf{k} - 2\mathbf{q} \cdot \mathbf{k}) = \frac{\hbar^2}{2m} (2k^2) , \\
a - c &= \frac{\hbar^2}{2m} (2k^2 + 2\mathbf{q} \cdot \mathbf{k} - k^2 - 2\mathbf{q} \cdot \mathbf{k}) = \frac{\hbar^2}{2m} (k^2) , \\
b - c &= \frac{\hbar^2}{2m} (2\mathbf{q} \cdot \mathbf{k} - k^2 - 2\mathbf{q} \cdot \mathbf{k}) = -\frac{\hbar^2}{2m} (k^2) , \\
a + b - 2c &= \frac{\hbar^2}{2m} (2k^2 + 2\mathbf{q} \cdot \mathbf{k} + 2\mathbf{q} \cdot \mathbf{k} - 2k^2 - 4\mathbf{q} \cdot \mathbf{k}) = \frac{\hbar^2}{2m} (2k^2 - 2k^2) = 0 .
\end{aligned}$$

Afterwards, we compute all the algebraic combinations that are present in the partial fraction decomposition.

$$\begin{aligned}
(a - b)(a - c)^2 &= + \left(\frac{\hbar^2}{2m}\right)^3 (2k^2) (k^2)^2 = + \left(\frac{\hbar^2}{2m}\right)^3 (2k^6) , \\
(a - b)(b - c)^2 &= + \left(\frac{\hbar^2}{2m}\right)^3 (2k^2) (k^2)^2 = + \left(\frac{\hbar^2}{2m}\right)^3 (2k^6) , \\
(a - c)^2(b - c)^2 &= + \left(\frac{\hbar^2}{2m}\right)^4 (k^2)^2 (k^2)^2 = + \left(\frac{\hbar^2}{2m}\right)^4 (k^8) , \\
(a - c)(b - c) &= - \left(\frac{\hbar^2}{2m}\right)^2 (k^2) (k^2) = - \left(\frac{\hbar^2}{2m}\right)^2 (k^4) = - \frac{1}{2k^2} \frac{2m}{\hbar^2} \left(\frac{\hbar^2}{2m}\right)^3 (2k^6) .
\end{aligned}$$

Finally, we substitute and perform some algebra. We also introduce the compact notation  $\epsilon_k = (\hbar^2 k^2)/(2m)$ .

$$\begin{aligned}
\left[\chi_0^{(4,4)}(\mathbf{k}, z)\right]_{14} &= - \int \frac{d^3q}{(2\pi)^3} \left(\frac{2m}{\hbar^2}\right)^3 \frac{f_0(\mathbf{q})}{12} \frac{1}{2k^6} \left\{ \frac{1}{\hbar z - \frac{\epsilon_{q+3k} - \epsilon_{q-k}}{4}} - \frac{1}{\hbar z - \frac{\epsilon_{q+k} - \epsilon_q}{2}} - \frac{\hbar^2 k^2}{2m} \frac{2}{(\hbar z - \epsilon_{q+k} + \epsilon_q)^2} \right\} \Rightarrow \\
\left[\chi_0^{(4,4)}(\mathbf{k}, z)\right]_{14} &= - \int \frac{d^3q}{(2\pi)^3} \left(\frac{2m}{\hbar^2}\right)^3 \frac{f_0(\mathbf{q})}{12} \frac{1}{2k^6} \left\{ \frac{1}{\hbar z - \frac{\epsilon_{q+3k} - \epsilon_{q-k}}{4}} - \frac{1}{\hbar z - \frac{\epsilon_{q+k} - \epsilon_q}{2}} - \frac{2\epsilon_k}{(\hbar z - \epsilon_{q+k} + \epsilon_q)^2} \right\} \Rightarrow \\
\left[\chi_0^{(4,4)}(\mathbf{k}, z)\right]_{14} &= - \left(\frac{m}{\hbar^2}\right)^3 \frac{1}{18k^6} \int \frac{d^3q}{(2\pi)^3} 2f_0(\mathbf{q}) \left\{ \frac{3}{\hbar z - \frac{\epsilon_{q+3k} - \epsilon_{q-k}}{4}} - \frac{3}{\hbar z - \frac{\epsilon_{q+k} - \epsilon_q}{2}} - \frac{6\epsilon_k}{(\hbar z - \epsilon_{q+k} + \epsilon_q)^2} \right\} \Rightarrow \\
\left[\chi_0^{(4,4)}(\mathbf{k}, z)\right]_{14} &= - \left(\frac{m}{\hbar^2}\right)^3 \frac{1}{18k^6} \int \frac{d^3q}{(2\pi)^3} 2f_0(\mathbf{q}) \left\{ \frac{12}{4\hbar z - \epsilon_{q+3k} + \epsilon_{q-k}} - \frac{6}{2\hbar z - \epsilon_{q+k} + \epsilon_{q-k}} - \frac{6\epsilon_k}{(\hbar z - \epsilon_{q+k} + \epsilon_q)^2} \right\} .
\end{aligned}$$

The *fifteenth contribution* is characterized by four simple poles. We first identify and calculate the coefficients  $a, b, c, d$ .

$$\begin{aligned}
\left[\chi_0^{(4,4)}(\mathbf{k}, z)\right]_{15} &= - \int \frac{d^3q}{(2\pi)^3} \frac{2f_0(\mathbf{q})}{(4\hbar z - \epsilon_{\mathbf{q}+3\mathbf{k}} + \epsilon_{\mathbf{q}-\mathbf{k}})(3\hbar z - \epsilon_{\mathbf{q}+2\mathbf{k}} + \epsilon_{\mathbf{q}-\mathbf{k}})(2\hbar z - \epsilon_{\mathbf{q}+\mathbf{k}} + \epsilon_{\mathbf{q}-\mathbf{k}})(\hbar z - \epsilon_{\mathbf{q}} + \epsilon_{\mathbf{q}-\mathbf{k}})} \Rightarrow \\
\left[\chi_0^{(4,4)}(\mathbf{k}, z)\right]_{15} &= - \int \frac{d^3q}{(2\pi)^3} \frac{f_0(\mathbf{q})}{12} \frac{1}{\left[\hbar z - \frac{\epsilon_{\mathbf{q}+3\mathbf{k}} - \epsilon_{\mathbf{q}-\mathbf{k}}}{4}\right] \left[\hbar z - \frac{\epsilon_{\mathbf{q}+2\mathbf{k}} - \epsilon_{\mathbf{q}-\mathbf{k}}}{3}\right] \left[\hbar z - \frac{\epsilon_{\mathbf{q}+\mathbf{k}} - \epsilon_{\mathbf{q}-\mathbf{k}}}{2}\right] [\hbar z - (\epsilon_{\mathbf{q}} - \epsilon_{\mathbf{q}-\mathbf{k}})]} \Rightarrow \\
a = \frac{\epsilon_{\mathbf{q}+3\mathbf{k}} - \epsilon_{\mathbf{q}-\mathbf{k}}}{4} &= \frac{\hbar^2}{2m} \frac{(\mathbf{q} + 3\mathbf{k})^2 - (\mathbf{q} - \mathbf{k})^2}{4} = \frac{\hbar^2}{2m} \frac{9k^2 + 6\mathbf{q} \cdot \mathbf{k} - k^2 + 2\mathbf{q} \cdot \mathbf{k}}{4} = \frac{\hbar^2}{2m} \frac{8k^2 + 8\mathbf{q} \cdot \mathbf{k}}{4} = \frac{\hbar^2}{2m} (2k^2 + 2\mathbf{q} \cdot \mathbf{k}) , \\
b = \frac{\epsilon_{\mathbf{q}+2\mathbf{k}} - \epsilon_{\mathbf{q}-\mathbf{k}}}{3} &= \frac{\hbar^2}{2m} \frac{(\mathbf{q} + 2\mathbf{k})^2 - (\mathbf{q} - \mathbf{k})^2}{3} = \frac{\hbar^2}{2m} \frac{4k^2 + 4\mathbf{q} \cdot \mathbf{k} - k^2 + 2\mathbf{q} \cdot \mathbf{k}}{3} = \frac{\hbar^2}{2m} \frac{3k^2 + 6\mathbf{q} \cdot \mathbf{k}}{3} = \frac{\hbar^2}{2m} (k^2 + 2\mathbf{q} \cdot \mathbf{k}) , \\
c = \frac{\epsilon_{\mathbf{q}+\mathbf{k}} - \epsilon_{\mathbf{q}-\mathbf{k}}}{2} &= \frac{\hbar^2}{2m} \frac{(\mathbf{q} + \mathbf{k})^2 - (\mathbf{q} - \mathbf{k})^2}{2} = \frac{\hbar^2}{2m} \frac{k^2 + 2\mathbf{q} \cdot \mathbf{k} - k^2 + 2\mathbf{q} \cdot \mathbf{k}}{2} = \frac{\hbar^2}{2m} \frac{4\mathbf{q} \cdot \mathbf{k}}{2} = \frac{\hbar^2}{2m} (2\mathbf{q} \cdot \mathbf{k}) , \\
d = \epsilon_{\mathbf{q}} - \epsilon_{\mathbf{q}-\mathbf{k}} &= \frac{\hbar^2}{2m} [q^2 - (\mathbf{q} - \mathbf{k})^2] = \frac{\hbar^2}{2m} (-k^2 + 2\mathbf{q} \cdot \mathbf{k}) .
\end{aligned}$$

Then, we compute all the possible differences between these four coefficients. Note that  $q^2$  and  $\mathbf{q} \cdot \mathbf{k}$  terms vanish.

$$\begin{aligned}
a - b &= \frac{\hbar^2}{2m} (2k^2 + 2\mathbf{q} \cdot \mathbf{k} - k^2 - 2\mathbf{q} \cdot \mathbf{k}) = \frac{\hbar^2}{2m} (2k^2 - k^2) = \frac{\hbar^2}{2m} (k^2) , \\
b - c &= \frac{\hbar^2}{2m} (k^2 + 2\mathbf{q} \cdot \mathbf{k} - 2\mathbf{q} \cdot \mathbf{k}) = \frac{\hbar^2}{2m} (k^2) , \\
c - d &= \frac{\hbar^2}{2m} (2\mathbf{q} \cdot \mathbf{k} + k^2 - 2\mathbf{q} \cdot \mathbf{k}) = \frac{\hbar^2}{2m} (k^2) , \\
a - c &= \frac{\hbar^2}{2m} (2k^2 + 2\mathbf{q} \cdot \mathbf{k} - 2\mathbf{q} \cdot \mathbf{k}) = \frac{\hbar^2}{2m} (2k^2) , \\
a - d &= \frac{\hbar^2}{2m} (2k^2 + 2\mathbf{q} \cdot \mathbf{k} + k^2 - 2\mathbf{q} \cdot \mathbf{k}) = \frac{\hbar^2}{2m} (2k^2 + k^2) = \frac{\hbar^2}{2m} (3k^2) , \\
b - d &= \frac{\hbar^2}{2m} (k^2 + 2\mathbf{q} \cdot \mathbf{k} + k^2 - 2\mathbf{q} \cdot \mathbf{k}) = \frac{\hbar^2}{2m} (k^2 + k^2) = \frac{\hbar^2}{2m} (2k^2) .
\end{aligned}$$

Afterwards, we compute all the triple difference combinations that are present in the partial fraction decomposition.

$$\begin{aligned}
(a - b)(a - c)(a - d) &= \frac{\hbar^2}{2m} (k^2) \frac{\hbar^2}{2m} (2k^2) \frac{\hbar^2}{2m} (3k^2) = \left(\frac{\hbar^2}{2m}\right)^3 (k^2)(2k^2)(3k^2) = \left(\frac{\hbar^2}{2m}\right)^3 (6k^6) , \\
(a - b)(b - c)(b - d) &= \frac{\hbar^2}{2m} (k^2) \frac{\hbar^2}{2m} (k^2) \frac{\hbar^2}{2m} (2k^2) = \left(\frac{\hbar^2}{2m}\right)^3 (k^2)(k^2)(2k^2) = \left(\frac{\hbar^2}{2m}\right)^3 (2k^6) , \\
(a - c)(b - c)(c - d) &= \frac{\hbar^2}{2m} (2k^2) \frac{\hbar^2}{2m} (k^2) \frac{\hbar^2}{2m} (k^2) = \left(\frac{\hbar^2}{2m}\right)^3 (2k^2)(k^2)(k^2) = \left(\frac{\hbar^2}{2m}\right)^3 (2k^6) , \\
(a - d)(b - d)(c - d) &= \frac{\hbar^2}{2m} (3k^2) \frac{\hbar^2}{2m} (2k^2) \frac{\hbar^2}{2m} (k^2) = \left(\frac{\hbar^2}{2m}\right)^3 (3k^2)(2k^2)(k^2) = \left(\frac{\hbar^2}{2m}\right)^3 (6k^6) .
\end{aligned}$$

Finally, we substitute the above in the contribution and perform some straightforward algebra.

$$\begin{aligned}
\left[\chi_0^{(4,4)}(\mathbf{k}, z)\right]_{15} &= - \int \frac{d^3q}{(2\pi)^3} \left(\frac{2m}{\hbar^2}\right)^3 \frac{f_0(\mathbf{q})}{12} \frac{1}{6k^6} \left[ \frac{1}{\hbar z - \frac{\epsilon_{\mathbf{q}+3\mathbf{k}} - \epsilon_{\mathbf{q}-\mathbf{k}}}{4}} - \frac{3}{\hbar z - \frac{\epsilon_{\mathbf{q}+2\mathbf{k}} - \epsilon_{\mathbf{q}-\mathbf{k}}}{3}} + \frac{3}{\hbar z - \frac{\epsilon_{\mathbf{q}+\mathbf{k}} - \epsilon_{\mathbf{q}-\mathbf{k}}}{2}} - \frac{1}{\hbar z - \epsilon_{\mathbf{q}} + \epsilon_{\mathbf{q}-\mathbf{k}}} \right] = \\
\left[\chi_0^{(4,4)}(\mathbf{k}, z)\right]_{15} &= - \int \frac{d^3q}{(2\pi)^3} \left(\frac{m}{\hbar^2}\right)^3 \frac{2f_0(\mathbf{q})}{18} \frac{1}{k^6} \left[ \frac{1}{\hbar z - \frac{\epsilon_{\mathbf{q}+3\mathbf{k}} - \epsilon_{\mathbf{q}-\mathbf{k}}}{4}} - \frac{3}{\hbar z - \frac{\epsilon_{\mathbf{q}+2\mathbf{k}} - \epsilon_{\mathbf{q}-\mathbf{k}}}{3}} + \frac{3}{\hbar z - \frac{\epsilon_{\mathbf{q}+\mathbf{k}} - \epsilon_{\mathbf{q}-\mathbf{k}}}{2}} - \frac{1}{\hbar z - \epsilon_{\mathbf{q}} + \epsilon_{\mathbf{q}-\mathbf{k}}} \right] = \\
\left[\chi_0^{(4,4)}(\mathbf{k}, z)\right]_{15} &= - \left(\frac{m}{\hbar^2}\right)^3 \frac{1}{18k^6} \int \frac{d^3q}{(2\pi)^3} 2f_0(\mathbf{q}) \left[ \frac{1}{\hbar z - \frac{\epsilon_{\mathbf{q}+3\mathbf{k}} - \epsilon_{\mathbf{q}-\mathbf{k}}}{4}} - \frac{3}{\hbar z - \frac{\epsilon_{\mathbf{q}+2\mathbf{k}} - \epsilon_{\mathbf{q}-\mathbf{k}}}{3}} + \frac{3}{\hbar z - \frac{\epsilon_{\mathbf{q}+\mathbf{k}} - \epsilon_{\mathbf{q}-\mathbf{k}}}{2}} - \frac{1}{\hbar z - \epsilon_{\mathbf{q}} + \epsilon_{\mathbf{q}-\mathbf{k}}} \right] \\
\left[\chi_0^{(4,4)}(\mathbf{k}, z)\right]_{15} &= - \left(\frac{m}{\hbar^2}\right)^3 \frac{1}{18k^6} \int \frac{d^3q}{(2\pi)^3} 2f_0(\mathbf{q}) \left[ \frac{4}{4\hbar z - \epsilon_{\mathbf{q}+3\mathbf{k}} + \epsilon_{\mathbf{q}-\mathbf{k}}} - \frac{9}{3\hbar z - \epsilon_{\mathbf{q}+2\mathbf{k}} + \epsilon_{\mathbf{q}-\mathbf{k}}} + \frac{6}{2\hbar z - \epsilon_{\mathbf{q}+\mathbf{k}} + \epsilon_{\mathbf{q}-\mathbf{k}}} - \frac{1}{\hbar z - \epsilon_{\mathbf{q}} + \epsilon_{\mathbf{q}-\mathbf{k}}} \right]
\end{aligned}$$

The *sixteenth contribution* is characterized by four simple poles. We first identify and calculate the coefficients  $a, b, c, d$ .

$$\begin{aligned}
\left[\chi_0^{(4,4)}(\mathbf{k}, z)\right]_{16} &= + \int \frac{d^3 q}{(2\pi)^3} \frac{2f_0(\mathbf{q})}{(4\hbar z - \epsilon_{\mathbf{q}+4\mathbf{k}} + \epsilon_{\mathbf{q}})(3\hbar z - \epsilon_{\mathbf{q}+3\mathbf{k}} + \epsilon_{\mathbf{q}})(2\hbar z - \epsilon_{\mathbf{q}+2\mathbf{k}} + \epsilon_{\mathbf{q}})(\hbar z - \epsilon_{\mathbf{q}+\mathbf{k}} + \epsilon_{\mathbf{q}})} \Rightarrow \\
\left[\chi_0^{(4,4)}(\mathbf{k}, z)\right]_{16} &= + \int \frac{d^3 q}{(2\pi)^3} \frac{f_0(\mathbf{q})}{12} \frac{1}{\left[\hbar z - \frac{\epsilon_{\mathbf{q}+4\mathbf{k}} - \epsilon_{\mathbf{q}}}{4}\right] \left[\hbar z - \frac{\epsilon_{\mathbf{q}+3\mathbf{k}} - \epsilon_{\mathbf{q}}}{3}\right] \left[\hbar z - \frac{\epsilon_{\mathbf{q}+2\mathbf{k}} - \epsilon_{\mathbf{q}}}{2}\right] [\hbar z - (\epsilon_{\mathbf{q}+\mathbf{k}} - \epsilon_{\mathbf{q}})]} \Rightarrow \\
a = \frac{\epsilon_{\mathbf{q}+4\mathbf{k}} - \epsilon_{\mathbf{q}}}{4} &= \frac{\hbar^2}{2m} \frac{(\mathbf{q} + 4\mathbf{k})^2 - q^2}{4} = \frac{\hbar^2}{2m} \frac{16k^2 + 8\mathbf{q} \cdot \mathbf{k}}{4} = \frac{\hbar^2}{2m} (4k^2 + 2\mathbf{q} \cdot \mathbf{k}), \\
b = \frac{\epsilon_{\mathbf{q}+3\mathbf{k}} - \epsilon_{\mathbf{q}}}{3} &= \frac{\hbar^2}{2m} \frac{(\mathbf{q} + 3\mathbf{k})^2 - q^2}{3} = \frac{\hbar^2}{2m} \frac{9k^2 + 6\mathbf{q} \cdot \mathbf{k}}{3} = \frac{\hbar^2}{2m} (3k^2 + 2\mathbf{q} \cdot \mathbf{k}), \\
c = \frac{\epsilon_{\mathbf{q}+2\mathbf{k}} - \epsilon_{\mathbf{q}}}{2} &= \frac{\hbar^2}{2m} \frac{(\mathbf{q} + 2\mathbf{k})^2 - q^2}{2} = \frac{\hbar^2}{2m} \frac{4k^2 + 4\mathbf{q} \cdot \mathbf{k}}{2} = \frac{\hbar^2}{2m} (2k^2 + 2\mathbf{q} \cdot \mathbf{k}), \\
d = \epsilon_{\mathbf{q}+\mathbf{k}} - \epsilon_{\mathbf{q}} &= \frac{\hbar^2}{2m} [(\mathbf{q} + \mathbf{k})^2 - q^2] = \frac{\hbar^2}{2m} (k^2 + 2\mathbf{q} \cdot \mathbf{k}).
\end{aligned}$$

Then, we compute all the possible differences between these four coefficients. Note that  $q^2$  and  $\mathbf{q} \cdot \mathbf{k}$  terms vanish.

$$\begin{aligned}
a - b &= \frac{\hbar^2}{2m} (4k^2 + 2\mathbf{q} \cdot \mathbf{k} - 3k^2 - 2\mathbf{q} \cdot \mathbf{k}) = \frac{\hbar^2}{2m} (4k^2 - 3k^2) = \frac{\hbar^2}{2m} (k^2), \\
b - c &= \frac{\hbar^2}{2m} (3k^2 + 2\mathbf{q} \cdot \mathbf{k} - 2k^2 - 2\mathbf{q} \cdot \mathbf{k}) = \frac{\hbar^2}{2m} (3k^2 - 2k^2) = \frac{\hbar^2}{2m} (k^2), \\
c - d &= \frac{\hbar^2}{2m} (2k^2 + 2\mathbf{q} \cdot \mathbf{k} - k^2 - 2\mathbf{q} \cdot \mathbf{k}) = \frac{\hbar^2}{2m} (2k^2 - k^2) = \frac{\hbar^2}{2m} (k^2), \\
a - c &= \frac{\hbar^2}{2m} (4k^2 + 2\mathbf{q} \cdot \mathbf{k} - 2k^2 - 2\mathbf{q} \cdot \mathbf{k}) = \frac{\hbar^2}{2m} (4k^2 - 2k^2) = \frac{\hbar^2}{2m} (2k^2), \\
a - d &= \frac{\hbar^2}{2m} (4k^2 + 2\mathbf{q} \cdot \mathbf{k} - k^2 - 2\mathbf{q} \cdot \mathbf{k}) = \frac{\hbar^2}{2m} (4k^2 - k^2) = \frac{\hbar^2}{2m} (3k^2), \\
b - d &= \frac{\hbar^2}{2m} (3k^2 + 2\mathbf{q} \cdot \mathbf{k} - k^2 - 2\mathbf{q} \cdot \mathbf{k}) = \frac{\hbar^2}{2m} (3k^2 - k^2) = \frac{\hbar^2}{2m} (2k^2).
\end{aligned}$$

Afterwards, we compute all the triple difference combinations that are present in the partial fraction decomposition.

$$\begin{aligned}
(a - b)(a - c)(a - d) &= \frac{\hbar^2}{2m} (k^2) \frac{\hbar^2}{2m} (2k^2) \frac{\hbar^2}{2m} (3k^2) = \left(\frac{\hbar^2}{2m}\right)^3 (k^2)(2k^2)(3k^2) = \left(\frac{\hbar^2}{2m}\right)^3 (6k^6), \\
(a - b)(b - c)(b - d) &= \frac{\hbar^2}{2m} (k^2) \frac{\hbar^2}{2m} (k^2) \frac{\hbar^2}{2m} (2k^2) = \left(\frac{\hbar^2}{2m}\right)^3 (k^2)(k^2)(2k^2) = \left(\frac{\hbar^2}{2m}\right)^3 (2k^6), \\
(a - c)(b - c)(c - d) &= \frac{\hbar^2}{2m} (2k^2) \frac{\hbar^2}{2m} (k^2) \frac{\hbar^2}{2m} (k^2) = \left(\frac{\hbar^2}{2m}\right)^3 (2k^2)(k^2)(k^2) = \left(\frac{\hbar^2}{2m}\right)^3 (2k^6), \\
(a - d)(b - d)(c - d) &= \frac{\hbar^2}{2m} (3k^2) \frac{\hbar^2}{2m} (2k^2) \frac{\hbar^2}{2m} (k^2) = \left(\frac{\hbar^2}{2m}\right)^3 (3k^2)(2k^2)(k^2) = \left(\frac{\hbar^2}{2m}\right)^3 (6k^6).
\end{aligned}$$

Finally, we substitute the above in the contribution and perform some straightforward algebra.

$$\begin{aligned}
\left[\chi_0^{(4,4)}(\mathbf{k}, z)\right]_{16} &= + \int \frac{d^3 q}{(2\pi)^3} \left(\frac{2m}{\hbar^2}\right)^3 \frac{f_0(\mathbf{q})}{12} \frac{1}{6k^6} \left[ \frac{1}{\hbar z - \frac{\epsilon_{\mathbf{q}+4\mathbf{k}} - \epsilon_{\mathbf{q}}}{4}} - \frac{3}{\hbar z - \frac{\epsilon_{\mathbf{q}+3\mathbf{k}} - \epsilon_{\mathbf{q}}}{3}} + \frac{3}{\hbar z - \frac{\epsilon_{\mathbf{q}+2\mathbf{k}} - \epsilon_{\mathbf{q}}}{2}} - \frac{1}{\hbar z - \epsilon_{\mathbf{q}+\mathbf{k}} + \epsilon_{\mathbf{q}}} \right] \Rightarrow \\
\left[\chi_0^{(4,4)}(\mathbf{k}, z)\right]_{16} &= + \int \frac{d^3 q}{(2\pi)^3} \left(\frac{m}{\hbar^2}\right)^3 \frac{2f_0(\mathbf{q})}{18} \frac{1}{k^6} \left[ \frac{1}{\hbar z - \frac{\epsilon_{\mathbf{q}+4\mathbf{k}} - \epsilon_{\mathbf{q}}}{4}} - \frac{3}{\hbar z - \frac{\epsilon_{\mathbf{q}+3\mathbf{k}} - \epsilon_{\mathbf{q}}}{3}} + \frac{3}{\hbar z - \frac{\epsilon_{\mathbf{q}+2\mathbf{k}} - \epsilon_{\mathbf{q}}}{2}} - \frac{1}{\hbar z - \epsilon_{\mathbf{q}+\mathbf{k}} + \epsilon_{\mathbf{q}}} \right] \Rightarrow \\
\left[\chi_0^{(4,4)}(\mathbf{k}, z)\right]_{16} &= + \left(\frac{m}{\hbar^2}\right)^3 \frac{1}{18k^6} \int \frac{d^3 q}{(2\pi)^3} 2f_0(\mathbf{q}) \left[ \frac{1}{\hbar z - \frac{\epsilon_{\mathbf{q}+4\mathbf{k}} - \epsilon_{\mathbf{q}}}{4}} - \frac{3}{\hbar z - \frac{\epsilon_{\mathbf{q}+3\mathbf{k}} - \epsilon_{\mathbf{q}}}{3}} + \frac{3}{\hbar z - \frac{\epsilon_{\mathbf{q}+2\mathbf{k}} - \epsilon_{\mathbf{q}}}{2}} - \frac{1}{\hbar z - \epsilon_{\mathbf{q}+\mathbf{k}} + \epsilon_{\mathbf{q}}} \right] \Rightarrow \\
\left[\chi_0^{(4,4)}(\mathbf{k}, z)\right]_{16} &= + \left(\frac{m}{\hbar^2}\right)^3 \frac{1}{18k^6} \int \frac{d^3 q}{(2\pi)^3} 2f_0(\mathbf{q}) \left[ \frac{4}{4\hbar z - \epsilon_{\mathbf{q}+4\mathbf{k}} + \epsilon_{\mathbf{q}}} - \frac{9}{3\hbar z - \epsilon_{\mathbf{q}+3\mathbf{k}} + \epsilon_{\mathbf{q}}} + \frac{6}{2\hbar z - \epsilon_{\mathbf{q}+2\mathbf{k}} + \epsilon_{\mathbf{q}}} - \frac{1}{\hbar z - \epsilon_{\mathbf{q}+\mathbf{k}} + \epsilon_{\mathbf{q}}} \right]
\end{aligned}$$

We now simply combine the sixteen distinct contributions

[illegible]

We isolate the common factor and obtain

[illegible]

All terms that contain  $\epsilon_{\mathbf{k}}$  cancel each other. The remaining terms are grouped according to the  $\hbar z$  harmonic of the denominator. Some straightforward algebra is carried out.

$$\begin{aligned} \chi_0^{(4,4)}(\mathbf{k}, z) &= \left(\frac{m}{\hbar^2}\right)^3 \frac{1}{18k^6} \int \frac{d^3q}{(2\pi)^3} 2f_0(q) \\ &\left\{ -\frac{4}{4\hbar z - \epsilon_q + \epsilon_{q-4\mathbf{k}}} + \frac{9}{3\hbar z - \epsilon_q + \epsilon_{q-3\mathbf{k}}} - \frac{6}{2\hbar z - \epsilon_q + \epsilon_{q-2\mathbf{k}}} + \frac{1}{\hbar z - \epsilon_q + \epsilon_{q-\mathbf{k}}} + \frac{4}{4\hbar z - \epsilon_{q+\mathbf{k}} + \epsilon_{q-3\mathbf{k}}} \right. \\ &- \frac{9}{3\hbar z - \epsilon_{q+\mathbf{k}} + \epsilon_{q-2\mathbf{k}}} + \frac{6}{2\hbar z - \epsilon_{q+\mathbf{k}} + \epsilon_{q-\mathbf{k}}} - \frac{1}{\hbar z - \epsilon_{q+\mathbf{k}} + \epsilon_q} + \frac{12}{4\hbar z - \epsilon_{q+\mathbf{k}} + \epsilon_{q-3\mathbf{k}}} - \frac{6}{2\hbar z - \epsilon_{q+\mathbf{k}} + \epsilon_{q-\mathbf{k}}} \\ &- \frac{12}{4\hbar z - \epsilon_{q+2\mathbf{k}} + \epsilon_{q-2\mathbf{k}}} + \frac{6}{2\hbar z - \epsilon_{q+2\mathbf{k}} + \epsilon_q} + \frac{12}{\hbar z - \epsilon_q + \epsilon_{q-\mathbf{k}}} - \frac{24}{2\hbar z - \epsilon_q + \epsilon_{q-2\mathbf{k}}} - \frac{12}{\hbar z - \epsilon_{q+\mathbf{k}} + \epsilon_q} \\ &+ \frac{24}{2\hbar z - \epsilon_{q+\mathbf{k}} + \epsilon_{q-\mathbf{k}}} + \frac{9}{3\hbar z - \epsilon_{q+2\mathbf{k}} + \epsilon_{q-\mathbf{k}}} - \frac{\hbar z - \epsilon_q + \epsilon_{q-\mathbf{k}}}{3} - \frac{3\hbar z - \epsilon_{q+3\mathbf{k}} + \epsilon_q}{9} - \frac{2\hbar z - \epsilon_{q+\mathbf{k}} + \epsilon_{q-\mathbf{k}}}{3} \\ &+ \frac{\hbar z - \epsilon_{q+\mathbf{k}} + \epsilon_q}{12} + \frac{3\hbar z - \epsilon_q + \epsilon_{q-3\mathbf{k}}}{9} - \frac{\hbar z - \epsilon_q + \epsilon_{q-\mathbf{k}}}{3} - \frac{3\hbar z - \epsilon_{q+\mathbf{k}} + \epsilon_{q-2\mathbf{k}}}{9} + \frac{\hbar z - \epsilon_{q+\mathbf{k}} + \epsilon_q}{3} \\ &+ \frac{\hbar z - \epsilon_q + \epsilon_{q-\mathbf{k}}}{12} - \frac{2\hbar z - \epsilon_{q+\mathbf{k}} + \epsilon_{q-\mathbf{k}}}{24} - \frac{\hbar z - \epsilon_{q+\mathbf{k}} + \epsilon_q}{12} + \frac{2\hbar z - \epsilon_{q+2\mathbf{k}} + \epsilon_q}{24} + \frac{4\hbar z - \epsilon_{q+2\mathbf{k}} + \epsilon_{q-2\mathbf{k}}}{12} \\ &- \frac{2\hbar z - \epsilon_q + \epsilon_{q-2\mathbf{k}}}{6} - \frac{4\hbar z - \epsilon_{q+3\mathbf{k}} + \epsilon_{q-\mathbf{k}}}{12} + \frac{2\hbar z - \epsilon_{q+\mathbf{k}} + \epsilon_{q-\mathbf{k}}}{6} - \frac{4\hbar z - \epsilon_{q+3\mathbf{k}} + \epsilon_{q-\mathbf{k}}}{4} + \frac{3\hbar z - \epsilon_{q+2\mathbf{k}} + \epsilon_{q-\mathbf{k}}}{9} \\ &+ \frac{1}{\hbar z - \epsilon_q + \epsilon_{q-\mathbf{k}}} + \frac{4}{4\hbar z - \epsilon_{q+4\mathbf{k}} + \epsilon_q} - \frac{9}{3\hbar z - \epsilon_{q+3\mathbf{k}} + \epsilon_q} + \frac{6}{2\hbar z - \epsilon_{q+2\mathbf{k}} + \epsilon_q} - \frac{1}{\hbar z - \epsilon_{q+\mathbf{k}} + \epsilon_q} \Big\} \Rightarrow \\ \chi_0^{(4,4)}(\mathbf{k}, z) &= \left(\frac{m}{\hbar^2}\right)^3 \frac{1}{18k^6} \int \frac{d^3q}{(2\pi)^3} 2f_0(q) \\ &\left\{ -\frac{4}{4\hbar z - \epsilon_q + \epsilon_{q-4\mathbf{k}}} + \frac{4}{4\hbar z - \epsilon_{q+\mathbf{k}} + \epsilon_{q-3\mathbf{k}}} + \frac{12}{4\hbar z - \epsilon_{q+\mathbf{k}} + \epsilon_{q-3\mathbf{k}}} - \frac{12}{4\hbar z - \epsilon_{q+2\mathbf{k}} + \epsilon_{q-2\mathbf{k}}} + \frac{12}{4\hbar z - \epsilon_{q+2\mathbf{k}} + \epsilon_{q-2\mathbf{k}}} \right. \\ &- \frac{4\hbar z - \epsilon_{q+3\mathbf{k}} + \epsilon_{q-\mathbf{k}}}{9} - \frac{4\hbar z - \epsilon_{q+3\mathbf{k}} + \epsilon_{q-\mathbf{k}}}{9} + \frac{4\hbar z - \epsilon_{q+4\mathbf{k}} + \epsilon_q}{9} + \frac{3\hbar z - \epsilon_q + \epsilon_{q-3\mathbf{k}}}{9} - \frac{3\hbar z - \epsilon_{q+\mathbf{k}} + \epsilon_{q-2\mathbf{k}}}{9} \\ &+ \frac{3\hbar z - \epsilon_{q+2\mathbf{k}} + \epsilon_{q-\mathbf{k}}}{9} - \frac{3\hbar z - \epsilon_{q+3\mathbf{k}} + \epsilon_q}{6} + \frac{3\hbar z - \epsilon_q + \epsilon_{q-3\mathbf{k}}}{6} - \frac{3\hbar z - \epsilon_{q+\mathbf{k}} + \epsilon_{q-2\mathbf{k}}}{6} + \frac{3\hbar z - \epsilon_{q+2\mathbf{k}} + \epsilon_{q-\mathbf{k}}}{6} \\ &- \frac{3\hbar z - \epsilon_{q+3\mathbf{k}} + \epsilon_q}{24} - \frac{2\hbar z - \epsilon_q + \epsilon_{q-2\mathbf{k}}}{24} + \frac{2\hbar z - \epsilon_{q+\mathbf{k}} + \epsilon_{q-\mathbf{k}}}{6} - \frac{2\hbar z - \epsilon_{q+\mathbf{k}} + \epsilon_{q-\mathbf{k}}}{24} + \frac{2\hbar z - \epsilon_{q+2\mathbf{k}} + \epsilon_q}{24} \\ &- \frac{2\hbar z - \epsilon_q + \epsilon_{q-2\mathbf{k}}}{6} + \frac{2\hbar z - \epsilon_{q+\mathbf{k}} + \epsilon_{q-\mathbf{k}}}{6} - \frac{2\hbar z - \epsilon_{q+\mathbf{k}} + \epsilon_{q-\mathbf{k}}}{6} - \frac{2\hbar z - \epsilon_{q+\mathbf{k}} + \epsilon_{q-\mathbf{k}}}{24} + \frac{2\hbar z - \epsilon_{q+2\mathbf{k}} + \epsilon_q}{24} \\ &- \frac{2\hbar z - \epsilon_q + \epsilon_{q-2\mathbf{k}}}{12} + \frac{2\hbar z - \epsilon_{q+\mathbf{k}} + \epsilon_{q-\mathbf{k}}}{12} + \frac{2\hbar z - \epsilon_{q+2\mathbf{k}} + \epsilon_q}{3} + \frac{\hbar z - \epsilon_q + \epsilon_{q-\mathbf{k}}}{3} - \frac{\hbar z - \epsilon_{q+\mathbf{k}} + \epsilon_q}{3} \\ &+ \frac{\hbar z - \epsilon_q + \epsilon_{q-\mathbf{k}}}{3} - \frac{\hbar z - \epsilon_{q+\mathbf{k}} + \epsilon_q}{12} - \frac{\hbar z - \epsilon_q + \epsilon_{q-\mathbf{k}}}{12} + \frac{\hbar z - \epsilon_{q+\mathbf{k}} + \epsilon_q}{3} - \frac{\hbar z - \epsilon_q + \epsilon_{q-\mathbf{k}}}{3} \\ &+ \frac{3}{\hbar z - \epsilon_{q+\mathbf{k}} + \epsilon_q} + \frac{12}{\hbar z - \epsilon_q + \epsilon_{q-\mathbf{k}}} - \frac{12}{\hbar z - \epsilon_{q+\mathbf{k}} + \epsilon_q} + \frac{1}{\hbar z - \epsilon_q + \epsilon_{q-\mathbf{k}}} - \frac{1}{\hbar z - \epsilon_{q+\mathbf{k}} + \epsilon_q} \Big\} \Rightarrow \\ \chi_0^{(4,4)}(\mathbf{k}, z) &= \left(\frac{m}{\hbar^2}\right)^3 \frac{1}{18k^6} \int \frac{d^3q}{(2\pi)^3} 2f_0(q) \\ &\left\{ +\frac{4}{4\hbar z - \epsilon_{q+4\mathbf{k}} + \epsilon_q} - \frac{4}{4\hbar z - \epsilon_q + \epsilon_{q-4\mathbf{k}}} + \frac{16}{4\hbar z - \epsilon_{q+\mathbf{k}} + \epsilon_{q-3\mathbf{k}}} - \frac{16}{4\hbar z - \epsilon_{q+3\mathbf{k}} + \epsilon_{q-\mathbf{k}}} + \frac{18}{3\hbar z - \epsilon_q + \epsilon_{q-3\mathbf{k}}} \right. \\ &- \frac{18}{3\hbar z - \epsilon_{q+3\mathbf{k}} + \epsilon_q} + \frac{3\hbar z - \epsilon_{q+2\mathbf{k}} + \epsilon_{q-\mathbf{k}}}{18} - \frac{3\hbar z - \epsilon_{q+\mathbf{k}} + \epsilon_{q-2\mathbf{k}}}{18} + \frac{36}{2\hbar z - \epsilon_{q+2\mathbf{k}} + \epsilon_q} - \frac{36}{2\hbar z - \epsilon_q + \epsilon_{q-2\mathbf{k}}} \\ &+ \frac{20}{\hbar z - \epsilon_q + \epsilon_{q-\mathbf{k}}} - \frac{20}{\hbar z - \epsilon_{q+\mathbf{k}} + \epsilon_q} \Big\} \Rightarrow \end{aligned}$$



The four algebraic identities  $(\epsilon_{q+3k} - \epsilon_{q-k})/4 = (\epsilon_{q+2k} - \epsilon_q)/2$ ,  $(\epsilon_{q+k} - \epsilon_{q-3k})/4 = (\epsilon_q - \epsilon_{q-2k})/2$ ,  $(\epsilon_{q+2k} - \epsilon_{q-k})/3 = \epsilon_{q+k} - \epsilon_q$ ,  $(\epsilon_{q+k} - \epsilon_{q-2k})/3 = \epsilon_q - \epsilon_{q-k}$  are employed in order to further simplify the final result.

$$\begin{aligned}
\chi_0^{(4,4)}(\mathbf{k}, z) &= \left(\frac{m}{\hbar^2}\right)^3 \frac{1}{18k^6} \int \frac{d^3q}{(2\pi)^3} 2f_0(\mathbf{q}) \\
&\left\{ + \frac{4}{4\hbar z - \epsilon_{q+4k} + \epsilon_q} - \frac{4}{4\hbar z - \epsilon_q + \epsilon_{q-4k}} - \frac{18}{3\hbar z - \epsilon_{q+3k} + \epsilon_q} + \frac{18}{3\hbar z - \epsilon_q + \epsilon_{q-3k}} \right. \\
&+ \frac{4}{2\hbar z - \epsilon_{q+2k} + \epsilon_q} - \frac{4}{2\hbar z - \epsilon_q + \epsilon_{q-2k}} - \frac{20}{\hbar z - \epsilon_{q+k} + \epsilon_q} + \frac{20}{\hbar z - \epsilon_q + \epsilon_{q-k}} \\
&\left. + \frac{16}{4\hbar z - \epsilon_{q+k} + \epsilon_{q-3k}} - \frac{16}{4\hbar z - \epsilon_{q+3k} + \epsilon_{q-k}} + \frac{18}{3\hbar z - \epsilon_{q+2k} + \epsilon_{q-k}} - \frac{18}{3\hbar z - \epsilon_{q+k} + \epsilon_{q-2k}} \right\} \Rightarrow \\
\chi_0^{(4,4)}(\mathbf{k}, z) &= \left(\frac{m}{\hbar^2}\right)^3 \frac{1}{18k^6} \int \frac{d^3q}{(2\pi)^3} 2f_0(\mathbf{q}) \\
&\left\{ + \frac{4}{4\hbar z - \epsilon_{q+4k} + \epsilon_q} - \frac{4}{4\hbar z - \epsilon_q + \epsilon_{q-4k}} - \frac{18}{3\hbar z - \epsilon_{q+3k} + \epsilon_q} + \frac{18}{3\hbar z - \epsilon_q + \epsilon_{q-3k}} \right. \\
&+ \frac{4}{2\hbar z - \epsilon_{q+2k} + \epsilon_q} - \frac{4}{2\hbar z - \epsilon_q + \epsilon_{q-2k}} - \frac{20}{\hbar z - \epsilon_{q+k} + \epsilon_q} + \frac{20}{\hbar z - \epsilon_q + \epsilon_{q-k}} \\
&\left. + \frac{4}{\hbar z - \frac{\epsilon_{q+k} - \epsilon_{q-3k}}{4}} - \frac{4}{\hbar z - \frac{\epsilon_{q+3k} - \epsilon_{q-k}}{4}} + \frac{6}{\hbar z - \frac{\epsilon_{q+2k} - \epsilon_{q-k}}{3}} - \frac{6}{\hbar z - \frac{\epsilon_{q+k} - \epsilon_{q-2k}}{3}} \right\} \Rightarrow \\
\chi_0^{(4,4)}(\mathbf{k}, z) &= \left(\frac{m}{\hbar^2}\right)^3 \frac{1}{18k^6} \int \frac{d^3q}{(2\pi)^3} 2f_0(\mathbf{q}) \\
&\left\{ + \frac{4}{4\hbar z - \epsilon_{q+4k} + \epsilon_q} - \frac{4}{4\hbar z - \epsilon_q + \epsilon_{q-4k}} - \frac{18}{3\hbar z - \epsilon_{q+3k} + \epsilon_q} + \frac{18}{3\hbar z - \epsilon_q + \epsilon_{q-3k}} \right. \\
&+ \frac{4}{2\hbar z - \epsilon_{q+2k} + \epsilon_q} - \frac{4}{2\hbar z - \epsilon_q + \epsilon_{q-2k}} - \frac{20}{\hbar z - \epsilon_{q+k} + \epsilon_q} + \frac{20}{\hbar z - \epsilon_q + \epsilon_{q-k}} \\
&\left. + \frac{4}{\hbar z - \frac{\epsilon_q - \epsilon_{q-2k}}{2}} - \frac{4}{\hbar z - \frac{\epsilon_{q+2k} - \epsilon_q}{2}} + \frac{6}{\hbar z - \epsilon_{q+k} + \epsilon_q} - \frac{6}{\hbar z - \epsilon_q + \epsilon_{q-k}} \right\} \Rightarrow \\
\chi_0^{(4,4)}(\mathbf{k}, z) &= \left(\frac{m}{\hbar^2}\right)^3 \frac{1}{18k^6} \int \frac{d^3q}{(2\pi)^3} 2f_0(\mathbf{q}) \\
&\left\{ + \frac{4}{4\hbar z - \epsilon_{q+4k} + \epsilon_q} - \frac{4}{4\hbar z - \epsilon_q + \epsilon_{q-4k}} - \frac{18}{3\hbar z - \epsilon_{q+3k} + \epsilon_q} + \frac{18}{3\hbar z - \epsilon_q + \epsilon_{q-3k}} \right. \\
&+ \frac{4}{2\hbar z - \epsilon_{q+2k} + \epsilon_q} - \frac{4}{2\hbar z - \epsilon_q + \epsilon_{q-2k}} - \frac{20}{\hbar z - \epsilon_{q+k} + \epsilon_q} + \frac{20}{\hbar z - \epsilon_q + \epsilon_{q-k}} \\
&\left. + \frac{8}{2\hbar z - \epsilon_q + \epsilon_{q-2k}} - \frac{8}{2\hbar z - \epsilon_{q+2k} + \epsilon_q} + \frac{6}{\hbar z - \epsilon_{q+k} + \epsilon_q} - \frac{6}{\hbar z - \epsilon_q + \epsilon_{q-k}} \right\} \Rightarrow \\
\chi_0^{(4,4)}(\mathbf{k}, z) &= \left(\frac{m}{\hbar^2}\right)^3 \frac{1}{18k^6} \int \frac{d^3q}{(2\pi)^3} 2f_0(\mathbf{q}) \\
&\left\{ + \frac{4}{4\hbar z - \epsilon_{q+4k} + \epsilon_q} - \frac{4}{4\hbar z - \epsilon_q + \epsilon_{q-4k}} - \frac{18}{3\hbar z - \epsilon_{q+3k} + \epsilon_q} + \frac{18}{3\hbar z - \epsilon_q + \epsilon_{q-3k}} \right. \\
&+ \frac{28}{2\hbar z - \epsilon_{q+2k} + \epsilon_q} - \frac{28}{2\hbar z - \epsilon_q + \epsilon_{q-2k}} - \frac{14}{\hbar z - \epsilon_{q+k} + \epsilon_q} + \frac{14}{\hbar z - \epsilon_q + \epsilon_{q-k}} \left. \right\} \Rightarrow
\end{aligned}$$

One ends up with eight unique terms that can be expressed as an algebraic combination of four ideal Lindhard first order density responses, that are evaluated at different multiple wavenumber and complex frequency arguments. In particular, the ideal Lindhard density responses of interest are

$$\begin{aligned}\chi_0(\mathbf{k}, z) &= \int \frac{d^3q}{(2\pi)^3} 2f_0(\mathbf{q}) \left[ \frac{1}{\hbar z - \epsilon_{\mathbf{q}+\mathbf{k}} + \epsilon_{\mathbf{q}}} - \frac{1}{\hbar z - \epsilon_{\mathbf{q}} + \epsilon_{\mathbf{q}-\mathbf{k}}} \right], \\ \chi_0(2\mathbf{k}, 2z) &= \int \frac{d^3q}{(2\pi)^3} 2f_0(\mathbf{q}) \left[ \frac{1}{\hbar(2z) - \epsilon_{\mathbf{q}+2\mathbf{k}} + \epsilon_{\mathbf{q}}} - \frac{1}{\hbar(2z) - \epsilon_{\mathbf{q}} + \epsilon_{\mathbf{q}-2\mathbf{k}}} \right], \\ \chi_0(3\mathbf{k}, 3z) &= \int \frac{d^3q}{(2\pi)^3} 2f_0(\mathbf{q}) \left[ \frac{1}{\hbar(3z) - \epsilon_{\mathbf{q}+3\mathbf{k}} + \epsilon_{\mathbf{q}}} - \frac{1}{\hbar(3z) - \epsilon_{\mathbf{q}} + \epsilon_{\mathbf{q}-3\mathbf{k}}} \right], \\ \chi_0(4\mathbf{k}, 4z) &= \int \frac{d^3q}{(2\pi)^3} 2f_0(\mathbf{q}) \left[ \frac{1}{\hbar(4z) - \epsilon_{\mathbf{q}+4\mathbf{k}} + \epsilon_{\mathbf{q}}} - \frac{1}{\hbar(4z) - \epsilon_{\mathbf{q}} + \epsilon_{\mathbf{q}-4\mathbf{k}}} \right].\end{aligned}$$

Ultimately, a fourth order Mikhailov-type recursion relation emerges that expresses the symmetric fourth order ideal density response in terms of the first order ideal density response.

$$\begin{aligned}\chi_0^{(4,4)}(\mathbf{k}, z) &= + \left(\frac{m}{\hbar^2}\right)^3 \frac{1}{18k^6} \int \frac{d^3q}{(2\pi)^3} 2f_0(\mathbf{q}) \left[ \frac{4}{4\hbar z - \epsilon_{\mathbf{q}+4\mathbf{k}} + \epsilon_{\mathbf{q}}} - \frac{4}{4\hbar z - \epsilon_{\mathbf{q}} + \epsilon_{\mathbf{q}-4\mathbf{k}}} \right] \\ &\quad - \left(\frac{m}{\hbar^2}\right)^3 \frac{1}{18k^6} \int \frac{d^3q}{(2\pi)^3} 2f_0(\mathbf{q}) \left[ \frac{18}{3\hbar z - \epsilon_{\mathbf{q}+3\mathbf{k}} + \epsilon_{\mathbf{q}}} - \frac{18}{3\hbar z - \epsilon_{\mathbf{q}} + \epsilon_{\mathbf{q}-3\mathbf{k}}} \right] \\ &\quad + \left(\frac{m}{\hbar^2}\right)^3 \frac{1}{18k^6} \int \frac{d^3q}{(2\pi)^3} 2f_0(\mathbf{q}) \left[ \frac{28}{2\hbar z - \epsilon_{\mathbf{q}+2\mathbf{k}} + \epsilon_{\mathbf{q}}} - \frac{28}{2\hbar z - \epsilon_{\mathbf{q}} + \epsilon_{\mathbf{q}-2\mathbf{k}}} \right] \\ &\quad - \left(\frac{m}{\hbar^2}\right)^3 \frac{1}{18k^6} \int \frac{d^3q}{(2\pi)^3} 2f_0(\mathbf{q}) \left[ \frac{14}{\hbar z - \epsilon_{\mathbf{q}+\mathbf{k}} + \epsilon_{\mathbf{q}}} - \frac{14}{\hbar z - \epsilon_{\mathbf{q}} + \epsilon_{\mathbf{q}-\mathbf{k}}} \right] \Rightarrow \\ \chi_0^{(4,4)}(\mathbf{k}, z) &= + \left(\frac{m}{\hbar^2}\right)^3 \frac{1}{18k^6} 4 \int \frac{d^3q}{(2\pi)^3} 2f_0(\mathbf{q}) \left[ \frac{1}{4\hbar z - \epsilon_{\mathbf{q}+4\mathbf{k}} + \epsilon_{\mathbf{q}}} - \frac{1}{4\hbar z - \epsilon_{\mathbf{q}} + \epsilon_{\mathbf{q}-4\mathbf{k}}} \right] \\ &\quad - \left(\frac{m}{\hbar^2}\right)^3 \frac{1}{18k^6} 18 \int \frac{d^3q}{(2\pi)^3} 2f_0(\mathbf{q}) \left[ \frac{1}{3\hbar z - \epsilon_{\mathbf{q}+3\mathbf{k}} + \epsilon_{\mathbf{q}}} - \frac{1}{3\hbar z - \epsilon_{\mathbf{q}} + \epsilon_{\mathbf{q}-3\mathbf{k}}} \right] \\ &\quad + \left(\frac{m}{\hbar^2}\right)^3 \frac{1}{18k^6} 28 \int \frac{d^3q}{(2\pi)^3} 2f_0(\mathbf{q}) \left[ \frac{1}{2\hbar z - \epsilon_{\mathbf{q}+2\mathbf{k}} + \epsilon_{\mathbf{q}}} - \frac{1}{2\hbar z - \epsilon_{\mathbf{q}} + \epsilon_{\mathbf{q}-2\mathbf{k}}} \right] \\ &\quad - \left(\frac{m}{\hbar^2}\right)^3 \frac{1}{18k^6} 14 \int \frac{d^3q}{(2\pi)^3} 2f_0(\mathbf{q}) \left[ \frac{1}{\hbar z - \epsilon_{\mathbf{q}+\mathbf{k}} + \epsilon_{\mathbf{q}}} - \frac{1}{\hbar z - \epsilon_{\mathbf{q}} + \epsilon_{\mathbf{q}-\mathbf{k}}} \right] \Rightarrow \\ \chi_0^{(4,4)}(\mathbf{k}, z) &= + \left(\frac{m}{\hbar^2}\right)^3 \frac{1}{18k^6} 4 \int \frac{d^3q}{(2\pi)^3} 2f_0(\mathbf{q}) \left[ \frac{1}{\hbar(4z) - \epsilon_{\mathbf{q}+4\mathbf{k}} + \epsilon_{\mathbf{q}}} - \frac{1}{\hbar(4z) - \epsilon_{\mathbf{q}} + \epsilon_{\mathbf{q}-4\mathbf{k}}} \right] \\ &\quad - \left(\frac{m}{\hbar^2}\right)^3 \frac{1}{18k^6} 18 \int \frac{d^3q}{(2\pi)^3} 2f_0(\mathbf{q}) \left[ \frac{1}{\hbar(3z) - \epsilon_{\mathbf{q}+3\mathbf{k}} + \epsilon_{\mathbf{q}}} - \frac{1}{\hbar(3z) - \epsilon_{\mathbf{q}} + \epsilon_{\mathbf{q}-3\mathbf{k}}} \right] \\ &\quad + \left(\frac{m}{\hbar^2}\right)^3 \frac{1}{18k^6} 28 \int \frac{d^3q}{(2\pi)^3} 2f_0(\mathbf{q}) \left[ \frac{1}{\hbar(2z) - \epsilon_{\mathbf{q}+2\mathbf{k}} + \epsilon_{\mathbf{q}}} - \frac{1}{\hbar(2z) - \epsilon_{\mathbf{q}} + \epsilon_{\mathbf{q}-2\mathbf{k}}} \right] \\ &\quad - \left(\frac{m}{\hbar^2}\right)^3 \frac{1}{18k^6} 14 \int \frac{d^3q}{(2\pi)^3} 2f_0(\mathbf{q}) \left[ \frac{1}{\hbar z - \epsilon_{\mathbf{q}+\mathbf{k}} + \epsilon_{\mathbf{q}}} - \frac{1}{\hbar z - \epsilon_{\mathbf{q}} + \epsilon_{\mathbf{q}-\mathbf{k}}} \right] \Rightarrow \\ \chi_0^{(4,4)}(\mathbf{k}, z) &= + \left(\frac{m}{\hbar^2}\right)^3 \frac{1}{18k^6} 4\chi_0(4\mathbf{k}, 4z) - \left(\frac{m}{\hbar^2}\right)^3 \frac{1}{18k^6} 18\chi_0(3\mathbf{k}, 3z) + \left(\frac{m}{\hbar^2}\right)^3 \frac{1}{18k^6} 28\chi_0(2\mathbf{k}, 2z) - \left(\frac{m}{\hbar^2}\right)^3 \frac{1}{18k^6} 14\chi_0(\mathbf{k}, z) \Rightarrow \\ \chi_0^{(4,4)}(\mathbf{k}, z) &= + \left(\frac{m}{\hbar^2}\right)^3 \frac{1}{18k^6} [4\chi_0(4\mathbf{k}, 4z) - 18\chi_0(3\mathbf{k}, 3z) + 28\chi_0(2\mathbf{k}, 2z) - 14\chi_0(\mathbf{k}, z)].\end{aligned}$$

Overall, we end up with the compact recursion relation

$$\chi_0^{(4,4)}(\mathbf{k}, z) = + \left(\frac{m}{\hbar^2}\right)^3 \frac{1}{18k^6} [4\chi_0(4\mathbf{k}, 4z) - 18\chi_0(3\mathbf{k}, 3z) + 28\chi_0(2\mathbf{k}, 2z) - 14\chi_0(\mathbf{k}, z)].$$

**The normalized compact form of the symmetric expression.** From the definition of the fourth order ideal density response as the fourth order functional derivative of the density with respect to the external potential energy, it is evident that the proper normalization is achieved by dividing with  $1/(n\beta^4)$ . In addition from the definition of the first order ideal density response as the first order functional derivative of the density with respect to the external potential energy, it is evident that the proper normalization of the Lindhard response is achieved by dividing with  $1/(n\beta)$ . The calculation proceeds with the introduction of the dimensionless complex frequency  $z = (T/\hbar)Z$  as well as of the dimensionless wavenumber  $k = k_F x$ . The utilization of the Fermi energy definition  $E_F = \hbar^2 k_F^2 / (2m)$  and the introduction of the degeneracy temperature definition  $\Theta = T/E_F$  ultimately lead to

$$\begin{aligned}
\chi_0^{(4,4)}(\mathbf{k}, z) &= + \left( \frac{m}{\hbar^2} \right)^3 \frac{1}{18k^6} [4\chi_0(4\mathbf{k}, 4z) - 18\chi_0(3\mathbf{k}, 3z) + 28\chi_0(2\mathbf{k}, 2z) - 14\chi_0(\mathbf{k}, z)] \Rightarrow \\
\frac{\chi_0^{(4,4)}(\mathbf{k}, z)}{n\beta^4} &= + \frac{1}{n\beta^4} \left( \frac{m}{\hbar^2} \right)^3 \frac{1}{18k^6} [4\chi_0(4\mathbf{k}, 4z) - 18\chi_0(3\mathbf{k}, 3z) + 28\chi_0(2\mathbf{k}, 2z) - 14\chi_0(\mathbf{k}, z)] \Rightarrow \\
\frac{\chi_0^{(4,4)}(\mathbf{k}, z)}{n\beta^4} &= + \left( \frac{m}{\hbar^2} \right)^3 \frac{T^3}{18k^6} \left[ 4 \frac{\chi_0(4\mathbf{k}, 4z)}{n\beta} - 18 \frac{\chi_0(3\mathbf{k}, 3z)}{n\beta} + 28 \frac{\chi_0(2\mathbf{k}, 2z)}{n\beta} - 14 \frac{\chi_0(\mathbf{k}, z)}{n\beta} \right] \Rightarrow \\
\frac{\chi_0^{(4,4)}(\mathbf{x}, Z)}{n\beta^4} &= + \left( \frac{m}{\hbar^2} \right)^3 \frac{T^3}{18k_F^6 x^6} \left[ 4 \frac{\chi_0(4\mathbf{x}, 4Z)}{n\beta} - 18 \frac{\chi_0(3\mathbf{x}, 3Z)}{n\beta} + 28 \frac{\chi_0(2\mathbf{x}, 2Z)}{n\beta} - 14 \frac{\chi_0(\mathbf{x}, Z)}{n\beta} \right] \Rightarrow \\
\frac{\chi_0^{(4,4)}(\mathbf{x}, Z)}{n\beta^4} &= + \left( \frac{2m}{\hbar^2 k_F^2} \right)^3 \frac{1}{2^3} \frac{T^3}{18x^6} \left[ 4 \frac{\chi_0(4\mathbf{x}, 4Z)}{n\beta} - 18 \frac{\chi_0(3\mathbf{x}, 3Z)}{n\beta} + 28 \frac{\chi_0(2\mathbf{x}, 2Z)}{n\beta} - 14 \frac{\chi_0(\mathbf{x}, Z)}{n\beta} \right] \Rightarrow \\
\frac{\chi_0^{(4,4)}(\mathbf{x}, Z)}{n\beta^4} &= + \frac{T^3}{[\hbar^2 k_F^2 / (2m)]^3} \frac{1}{2^3} \frac{1}{18x^6} \left[ 4 \frac{\chi_0(4\mathbf{x}, 4Z)}{n\beta} - 18 \frac{\chi_0(3\mathbf{x}, 3Z)}{n\beta} + 28 \frac{\chi_0(2\mathbf{x}, 2Z)}{n\beta} - 14 \frac{\chi_0(\mathbf{x}, Z)}{n\beta} \right] \Rightarrow \\
\frac{\chi_0^{(4,4)}(\mathbf{x}, Z)}{n\beta^4} &= + \frac{T^3}{E_F^3} \frac{1}{2^3} \frac{1}{18x^6} \left[ 4 \frac{\chi_0(4\mathbf{x}, 4Z)}{n\beta} - 18 \frac{\chi_0(3\mathbf{x}, 3Z)}{n\beta} + 28 \frac{\chi_0(2\mathbf{x}, 2Z)}{n\beta} - 14 \frac{\chi_0(\mathbf{x}, Z)}{n\beta} \right] \Rightarrow \\
\frac{\chi_0^{(4,4)}(\mathbf{x}, Z)}{n\beta^4} &= + \frac{1}{2^3} \frac{1}{18} \frac{\Theta^3}{x^6} \left[ 4 \frac{\chi_0(4\mathbf{x}, 4Z)}{n\beta} - 18 \frac{\chi_0(3\mathbf{x}, 3Z)}{n\beta} + 28 \frac{\chi_0(2\mathbf{x}, 2Z)}{n\beta} - 14 \frac{\chi_0(\mathbf{x}, Z)}{n\beta} \right] \Rightarrow \\
\frac{\chi_0^{(4,4)}(\mathbf{x}, Z)}{n\beta^4} &= + \frac{1}{144} \frac{\Theta^3}{x^6} \left[ 4 \frac{\chi_0(4\mathbf{x}, 4Z)}{n\beta} - 18 \frac{\chi_0(3\mathbf{x}, 3Z)}{n\beta} + 28 \frac{\chi_0(2\mathbf{x}, 2Z)}{n\beta} - 14 \frac{\chi_0(\mathbf{x}, Z)}{n\beta} \right] \Rightarrow \\
\frac{\chi_0^{(4,4)}(\mathbf{x}, Z)}{n\beta^4} &= + \frac{1}{2 \times 4} \frac{1}{2 \times 3 \times 3} \frac{\Theta^3}{x^6} \left[ 4 \frac{\chi_0(4\mathbf{x}, 4Z)}{n\beta} - 18 \frac{\chi_0(3\mathbf{x}, 3Z)}{n\beta} + 28 \frac{\chi_0(2\mathbf{x}, 2Z)}{n\beta} - 14 \frac{\chi_0(\mathbf{x}, Z)}{n\beta} \right] \Rightarrow \\
\frac{\chi_0^{(4,4)}(\mathbf{x}, Z)}{n\beta^4} &= + \frac{1}{2 \times 3} \frac{1}{2 \times 3 \times 4} \frac{\Theta^3}{x^6} \left[ 4 \frac{\chi_0(4\mathbf{x}, 4Z)}{n\beta} - 18 \frac{\chi_0(3\mathbf{x}, 3Z)}{n\beta} + 28 \frac{\chi_0(2\mathbf{x}, 2Z)}{n\beta} - 14 \frac{\chi_0(\mathbf{x}, Z)}{n\beta} \right] \Rightarrow \\
\frac{\chi_0^{(4,4)}(\mathbf{x}, Z)}{n\beta^4} &= + \frac{1}{3!} \frac{1}{4!} \frac{\Theta^3}{x^6} \left[ 4 \frac{\chi_0(4\mathbf{x}, 4Z)}{n\beta} - 18 \frac{\chi_0(3\mathbf{x}, 3Z)}{n\beta} + 28 \frac{\chi_0(2\mathbf{x}, 2Z)}{n\beta} - 14 \frac{\chi_0(\mathbf{x}, Z)}{n\beta} \right].
\end{aligned}$$

In the final steps, the numerical pre-factors were decomposed into products that were later expressed as factorials with respect to the order of the ideal density response. Ultimately, one has

$$\frac{\chi_0^{(4,4)}(\mathbf{x}, Z)}{n\beta^4} = + \frac{1}{(4-1)!} \frac{1}{4!} \frac{\Theta^3}{x^6} \left[ 4 \frac{\chi_0(4\mathbf{x}, 4Z)}{n\beta} - 18 \frac{\chi_0(3\mathbf{x}, 3Z)}{n\beta} + 28 \frac{\chi_0(2\mathbf{x}, 2Z)}{n\beta} - 14 \frac{\chi_0(\mathbf{x}, Z)}{n\beta} \right].$$

The static limit simply reads as

$$\frac{\chi_0^{(4,4)}(\mathbf{x})}{n\beta^4} = + \frac{1}{(4-1)!} \frac{1}{4!} \frac{\Theta^3}{x^6} \left[ 4 \frac{\chi_0(4\mathbf{x})}{n\beta} - 18 \frac{\chi_0(3\mathbf{x})}{n\beta} + 28 \frac{\chi_0(2\mathbf{x})}{n\beta} - 14 \frac{\chi_0(\mathbf{x})}{n\beta} \right].$$

**The long wavelength limit of the static normalized symmetric expression.** The long-wavelength limit of the static fourth order ideal density response at the fourth harmonic should converge. Given the  $1/x^6$  pre-factor and the even parity, this implies that the first three terms of the small argument expansion of the ideal quantic density response should cancel out exactly, otherwise the long-wavelength limit of the static case would diverge. We first write down the first four terms of the small argument expansion of the ideal Lindhard density response for the arguments  $4x, 3x, 2x, x$ .

$$\begin{aligned}\frac{\chi_0(x)}{n\beta} &\simeq -\frac{3}{2}\Theta \int_0^\infty dy f_0(y; \Theta) \left[ 1 + \frac{1}{12} \left(\frac{x}{y}\right)^2 + \frac{1}{5} \frac{1}{16} \left(\frac{x}{y}\right)^4 + \frac{1}{7} \frac{1}{64} \left(\frac{x}{y}\right)^6 \right], \\ \frac{\chi_0(2x)}{n\beta} &\simeq -\frac{3}{2}\Theta \int_0^\infty dy f_0(y; \Theta) \left[ 1 + \frac{1}{3} \left(\frac{x}{y}\right)^2 + \frac{1}{5} \left(\frac{x}{y}\right)^4 + \frac{1}{7} \left(\frac{x}{y}\right)^6 \right], \\ \frac{\chi_0(3x)}{n\beta} &\simeq -\frac{3}{2}\Theta \int_0^\infty dy f_0(y; \Theta) \left[ 1 + \frac{3}{4} \left(\frac{x}{y}\right)^2 + \frac{1}{5} \frac{81}{16} \left(\frac{x}{y}\right)^4 + \frac{1}{7} \frac{729}{64} \left(\frac{x}{y}\right)^6 \right], \\ \frac{\chi_0(4x)}{n\beta} &\simeq -\frac{3}{2}\Theta \int_0^\infty dy f_0(y; \Theta) \left[ 1 + \frac{4}{3} \left(\frac{x}{y}\right)^2 + \frac{16}{5} \left(\frac{x}{y}\right)^4 + \frac{64}{7} \left(\frac{x}{y}\right)^6 \right].\end{aligned}$$

Then, we substitute the above in the static limit of the normalized compact form of the fourth order ideal density response at the fourth harmonic

$$\begin{aligned}\frac{\chi_0^{(4,4)}(x)}{n\beta^4} &= +\frac{1}{3!} \frac{1}{4!} \frac{\Theta^3}{x^6} \left[ 4 \frac{\chi_0(4x)}{n\beta} - 18 \frac{\chi_0(3x)}{n\beta} + 28 \frac{\chi_0(2x)}{n\beta} - 14 \frac{\chi_0(x)}{n\beta} \right] \Rightarrow \\ \frac{\chi_0^{(4,4)}(x)}{n\beta^4} &= -\frac{1}{3!} \frac{1}{4!} \frac{\Theta^3}{x^6} \left\{ 4 \frac{3}{2} \Theta \int_0^\infty dy f_0(y; \Theta) \left[ 1 + \frac{4}{3} \left(\frac{x}{y}\right)^2 + \frac{16}{5} \left(\frac{x}{y}\right)^4 + \frac{64}{7} \left(\frac{x}{y}\right)^6 \right] \right. \\ &\quad - 18 \frac{3}{2} \Theta \int_0^\infty dy f_0(y; \Theta) \left[ 1 + \frac{3}{4} \left(\frac{x}{y}\right)^2 + \frac{1}{5} \frac{81}{16} \left(\frac{x}{y}\right)^4 + \frac{1}{7} \frac{729}{64} \left(\frac{x}{y}\right)^6 \right] \\ &\quad + 28 \frac{3}{2} \Theta \int_0^\infty dy f_0(y; \Theta) \left[ 1 + \frac{1}{3} \left(\frac{x}{y}\right)^2 + \frac{1}{5} \left(\frac{x}{y}\right)^4 + \frac{1}{7} \left(\frac{x}{y}\right)^6 \right] \\ &\quad \left. - 14 \frac{3}{2} \Theta \int_0^\infty dy f_0(y; \Theta) \left[ 1 + \frac{1}{12} \left(\frac{x}{y}\right)^2 + \frac{1}{5} \frac{1}{16} \left(\frac{x}{y}\right)^4 + \frac{1}{7} \frac{1}{64} \left(\frac{x}{y}\right)^6 \right] \right\} \Rightarrow \\ \frac{\chi_0^{(4,4)}(x)}{n\beta^4} &= -\frac{1}{3!} \frac{1}{4!} \frac{\Theta^3}{x^6} \left\{ \frac{3}{2} \Theta \int_0^\infty dy f_0(y; \Theta) \left[ 4 + 4 \frac{4}{3} \left(\frac{x}{y}\right)^2 + 4 \frac{16}{5} \left(\frac{x}{y}\right)^4 + 4 \frac{64}{7} \left(\frac{x}{y}\right)^6 \right] \right. \\ &\quad + \frac{3}{2} \Theta \int_0^\infty dy f_0(y; \Theta) \left[ -18 - 18 \frac{3}{4} \left(\frac{x}{y}\right)^2 - 18 \frac{1}{5} \frac{81}{16} \left(\frac{x}{y}\right)^4 - 18 \frac{1}{7} \frac{729}{64} \left(\frac{x}{y}\right)^6 \right] \\ &\quad + \frac{3}{2} \Theta \int_0^\infty dy f_0(y; \Theta) \left[ 28 + 28 \frac{1}{3} \left(\frac{x}{y}\right)^2 + 28 \frac{1}{5} \left(\frac{x}{y}\right)^4 + 28 \frac{1}{7} \left(\frac{x}{y}\right)^6 \right] \\ &\quad \left. + \frac{3}{2} \Theta \int_0^\infty dy f_0(y; \Theta) \left[ -14 - 14 \frac{1}{12} \left(\frac{x}{y}\right)^2 - 14 \frac{1}{5} \frac{1}{16} \left(\frac{x}{y}\right)^4 - 14 \frac{1}{7} \frac{1}{64} \left(\frac{x}{y}\right)^6 \right] \right\} \Rightarrow \\ \frac{\chi_0^{(4,4)}(x)}{n\beta^4} &= -\frac{1}{3!} \frac{1}{4!} \frac{\Theta^3}{x^6} \frac{3}{2} \Theta \int_0^\infty dy f_0(y; \Theta) \left[ 4 + 4 \frac{4}{3} \left(\frac{x}{y}\right)^2 + 4 \frac{16}{5} \left(\frac{x}{y}\right)^4 + 4 \frac{64}{7} \left(\frac{x}{y}\right)^6 \right. \\ &\quad - 18 - 18 \frac{3}{4} \left(\frac{x}{y}\right)^2 - 18 \frac{1}{5} \frac{81}{16} \left(\frac{x}{y}\right)^4 - 18 \frac{1}{7} \frac{729}{64} \left(\frac{x}{y}\right)^6 \\ &\quad + 28 + 28 \frac{1}{3} \left(\frac{x}{y}\right)^2 + 28 \frac{1}{5} \left(\frac{x}{y}\right)^4 + 28 \frac{1}{7} \left(\frac{x}{y}\right)^6 \\ &\quad \left. - 14 - 14 \frac{1}{12} \left(\frac{x}{y}\right)^2 - 14 \frac{1}{5} \frac{1}{16} \left(\frac{x}{y}\right)^4 - 14 \frac{1}{7} \frac{1}{64} \left(\frac{x}{y}\right)^6 \right].\end{aligned}$$

We simply re-organize the terms in ascending powers of  $x/y$ . It is straightforward to prove that the first three terms,  $\propto (x/y)^0, (x/y)^2, (x/y)^4$ , cancel out exactly. The leading order term is  $\mathcal{O}[(x/y)^6]$  and leads to finite contribution at the long-wavelength limit,  $\mathcal{O}(y^{-6})$ , after the removal of the  $1/x^6$  pre-factor. It is rather apparent that the remaining improper integral is indeed convergent.

$$\begin{aligned}
\frac{\chi_0^{(4,4)}(\mathbf{x})}{n\beta^4} &= -\frac{1}{3!} \frac{1}{4!} \frac{3}{2} \frac{\Theta^4}{x^6} \int_0^\infty dy f_0(y; \Theta) \left[ 4 + 4\frac{4}{3} \left(\frac{x}{y}\right)^2 + 4\frac{16}{5} \left(\frac{x}{y}\right)^4 + 4\frac{64}{7} \left(\frac{x}{y}\right)^6 \right. \\
&\quad - 18 - 18\frac{3}{4} \left(\frac{x}{y}\right)^2 - 18\frac{1}{5} \frac{81}{16} \left(\frac{x}{y}\right)^4 - 18\frac{1}{7} \frac{729}{64} \left(\frac{x}{y}\right)^6 \\
&\quad + 28 + 28\frac{1}{3} \left(\frac{x}{y}\right)^2 + 28\frac{1}{5} \left(\frac{x}{y}\right)^4 + 28\frac{1}{7} \left(\frac{x}{y}\right)^6 \\
&\quad \left. - 14 - 14\frac{1}{12} \left(\frac{x}{y}\right)^2 - 14\frac{1}{5} \frac{1}{16} \left(\frac{x}{y}\right)^4 - 14\frac{1}{7} \frac{1}{64} \left(\frac{x}{y}\right)^6 \right] \Rightarrow \\
\frac{\chi_0^{(4,4)}(\mathbf{x})}{n\beta^4} &= -\frac{1}{3!} \frac{1}{4!} \frac{3}{2} \frac{\Theta^4}{x^6} \int_0^\infty dy f_0(y; \Theta) \left[ 4 - 18 + 28 - 14 + 4\frac{4}{3} \left(\frac{x}{y}\right)^2 - 18\frac{3}{4} \left(\frac{x}{y}\right)^2 + 28\frac{1}{3} \left(\frac{x}{y}\right)^2 - 14\frac{1}{12} \left(\frac{x}{y}\right)^2 \right. \\
&\quad + 4\frac{16}{5} \left(\frac{x}{y}\right)^4 - 18\frac{1}{5} \frac{81}{16} \left(\frac{x}{y}\right)^4 + 28\frac{1}{5} \left(\frac{x}{y}\right)^4 - 14\frac{1}{5} \frac{1}{16} \left(\frac{x}{y}\right)^4 \\
&\quad \left. + 4\frac{64}{7} \left(\frac{x}{y}\right)^6 - 18\frac{1}{7} \frac{729}{64} \left(\frac{x}{y}\right)^6 + 28\frac{1}{7} \left(\frac{x}{y}\right)^6 - 14\frac{1}{7} \frac{1}{64} \left(\frac{x}{y}\right)^6 \right] \Rightarrow \\
\frac{\chi_0^{(4,4)}(\mathbf{x})}{n\beta^4} &= -\frac{1}{3!} \frac{1}{4!} \frac{3}{2} \frac{\Theta^4}{x^6} \int_0^\infty dy f_0(y; \Theta) \left[ (4 - 18 + 28 - 14) + \left(4\frac{4}{3} - 18\frac{3}{4} + 28\frac{1}{3} - 14\frac{1}{12}\right) \left(\frac{x}{y}\right)^2 \right. \\
&\quad + \left(4\frac{16}{5} - 18\frac{1}{5} \frac{81}{16} + 28\frac{1}{5} - 14\frac{1}{5} \frac{1}{16}\right) \left(\frac{x}{y}\right)^4 + \left(4\frac{64}{7} - 18\frac{1}{7} \frac{729}{64} + 28\frac{1}{7} - 14\frac{1}{7} \frac{1}{64}\right) \left(\frac{x}{y}\right)^6 \left. \right] \Rightarrow \\
\frac{\chi_0^{(4,4)}(\mathbf{x})}{n\beta^4} &= -\frac{1}{3!} \frac{1}{4!} \frac{3}{2} \frac{\Theta^4}{x^6} \int_0^\infty dy f_0(y; \Theta) \left[ (32 - 32) + \frac{16 \times 4 - 54 \times 3 + 28 \times 4 - 14}{12} \left(\frac{x}{y}\right)^2 \right. \\
&\quad + \frac{4 \times 16^2 - 18 \times 81 + 28 \times 16 - 14}{80} \left(\frac{x}{y}\right)^4 + \frac{4 \times 64^2 - 18 \times 729 + 28 \times 64 - 14}{448} \left(\frac{x}{y}\right)^6 \left. \right] \Rightarrow \\
\frac{\chi_0^{(4,4)}(\mathbf{x})}{n\beta^4} &= -\frac{1}{3!} \frac{1}{4!} \frac{3}{2} \frac{\Theta^4}{x^6} \int_0^\infty dy f_0(y; \Theta) \left[ (32 - 32) + \frac{64 - 162 + 112 - 14}{12} \left(\frac{x}{y}\right)^2 \right. \\
&\quad + \frac{1024 - 1458 + 448 - 14}{80} \left(\frac{x}{y}\right)^4 + \frac{16384 - 13122 + 1792 - 14}{448} \left(\frac{x}{y}\right)^6 \left. \right] \Rightarrow \\
\frac{\chi_0^{(4,4)}(\mathbf{x})}{n\beta^4} &= -\frac{1}{3!} \frac{1}{4!} \frac{3}{2} \frac{\Theta^4}{x^6} \int_0^\infty dy f_0(y; \Theta) \left[ (32 - 32) + \frac{176 - 176}{12} \left(\frac{x}{y}\right)^2 + \frac{1472 - 1472}{80} \left(\frac{x}{y}\right)^4 + \frac{5040}{448} \left(\frac{x}{y}\right)^6 \right] \Rightarrow \\
\frac{\chi_0^{(4,4)}(\mathbf{x})}{n\beta^4} &= -\frac{1}{3!} \frac{1}{4!} \frac{3}{2} \frac{\Theta^4}{x^6} \int_0^\infty dy f_0(y; \Theta) \frac{720}{64} \left(\frac{x}{y}\right)^6 \Rightarrow \\
\frac{\chi_0^{(4,4)}(\mathbf{x})}{n\beta^4} &= -\frac{1}{3!} \frac{1}{4!} \frac{3}{2} \frac{45}{4} \frac{\Theta^4}{x^6} \int_0^\infty dy f_0(y; \Theta) \left(\frac{x}{y}\right)^6 \Rightarrow \\
\frac{\chi_0^{(4,4)}(\mathbf{x})}{n\beta^4} &= -\frac{1}{2 \times 3} \frac{1}{2 \times 3 \times 4} \frac{3 \times 5 \times 9}{2 \times 4} \frac{\Theta^4}{x^6} \int_0^\infty dy f_0(y; \Theta) \left(\frac{x}{y}\right)^6 \Rightarrow \\
\frac{\chi_0^{(4,4)}(\mathbf{x})}{n\beta^4} &= -\frac{15}{128} \frac{\Theta^4}{x^6} \int_0^\infty dy f_0(y; \Theta) \left(\frac{x}{y}\right)^6 \Rightarrow \\
\frac{\chi_0^{(4,4)}(\mathbf{x})}{n\beta^4} &= -\frac{15}{128} \Theta^4 \int_0^\infty dy \frac{f_0(y; \Theta)}{y^6}.
\end{aligned}$$



[illegible]

[illegible]



[illegible]





[illegible]







[illegible]





[illegible]

Note that  $\mathcal{W}_{\mathbf{k}_1, z_1; \mathbf{k}_2, z_2; \mathbf{k}_3, z_3; \mathbf{k}_4, z_4; \mathbf{k}_5, z_5}^{(5), 0}$  is separated in four terms (split in two pages),

[illegible]

[illegible]





[illegible]

[illegible]



[illegible]



[illegible]













[illegible]







[illegible]



**The compact form of the symmetric expression.** The calculation proceeds with the separate evaluation of each of the 32 contributing integrals that have been labelled as  $\left[\chi_0^{(5,5)}(\mathbf{k}, z)\right]_1, \left[\chi_0^{(5,5)}(\mathbf{k}, z)\right]_2, \left[\chi_0^{(5,5)}(\mathbf{k}, z)\right]_3, \left[\chi_0^{(5,5)}(\mathbf{k}, z)\right]_4, \left[\chi_0^{(5,5)}(\mathbf{k}, z)\right]_5, \left[\chi_0^{(5,5)}(\mathbf{k}, z)\right]_6, \left[\chi_0^{(5,5)}(\mathbf{k}, z)\right]_7, \left[\chi_0^{(5,5)}(\mathbf{k}, z)\right]_8, \left[\chi_0^{(5,5)}(\mathbf{k}, z)\right]_9, \left[\chi_0^{(5,5)}(\mathbf{k}, z)\right]_{10}, \left[\chi_0^{(5,5)}(\mathbf{k}, z)\right]_{11}, \left[\chi_0^{(5,5)}(\mathbf{k}, z)\right]_{12}, \left[\chi_0^{(5,5)}(\mathbf{k}, z)\right]_{13}, \left[\chi_0^{(5,5)}(\mathbf{k}, z)\right]_{14}, \left[\chi_0^{(5,5)}(\mathbf{k}, z)\right]_{15}, \left[\chi_0^{(5,5)}(\mathbf{k}, z)\right]_{16}, \left[\chi_0^{(5,5)}(\mathbf{k}, z)\right]_{17}, \left[\chi_0^{(5,5)}(\mathbf{k}, z)\right]_{18}, \left[\chi_0^{(5,5)}(\mathbf{k}, z)\right]_{19}, \left[\chi_0^{(5,5)}(\mathbf{k}, z)\right]_{20}, \left[\chi_0^{(5,5)}(\mathbf{k}, z)\right]_{21}, \left[\chi_0^{(5,5)}(\mathbf{k}, z)\right]_{22}, \left[\chi_0^{(5,5)}(\mathbf{k}, z)\right]_{23}, \left[\chi_0^{(5,5)}(\mathbf{k}, z)\right]_{24}, \left[\chi_0^{(5,5)}(\mathbf{k}, z)\right]_{25}, \left[\chi_0^{(5,5)}(\mathbf{k}, z)\right]_{26}, \left[\chi_0^{(5,5)}(\mathbf{k}, z)\right]_{27}, \left[\chi_0^{(5,5)}(\mathbf{k}, z)\right]_{28}, \left[\chi_0^{(5,5)}(\mathbf{k}, z)\right]_{29}, \left[\chi_0^{(5,5)}(\mathbf{k}, z)\right]_{30}, \left[\chi_0^{(5,5)}(\mathbf{k}, z)\right]_{31}, \left[\chi_0^{(5,5)}(\mathbf{k}, z)\right]_{32}$ . The calculation is based on splitting the integrands into simple fractions and is facilitated by the fact that the multiplication coefficient of the decomposition always turns out to be independent of the integration variable  $q$ . For the purposes of the partial fraction decomposition, it is convenient to consider the fractions as functions of the variable  $\hbar z$ . The fractions of the integrands within the contributions  $\left[\chi_0^{(5,5)}(\mathbf{k}, z)\right]_1, \left[\chi_0^{(5,5)}(\mathbf{k}, z)\right]_2, \left[\chi_0^{(5,5)}(\mathbf{k}, z)\right]_{31}, \left[\chi_0^{(5,5)}(\mathbf{k}, z)\right]_{32}$ , have **five simple real poles**. It is straightforward to demonstrate by solving the emerging  $5 \times 5$  set of equations that their partial fraction decomposition follows

$$\frac{1}{(x-a)(x-b)(x-c)(x-d)(x-e)} = \frac{1}{(a-b)(a-c)(a-d)(a-e)(x-a)} - \frac{1}{(a-b)(b-c)(b-d)(b-e)(x-b)} + \frac{1}{(a-c)(b-c)(c-d)(c-e)(x-c)} - \frac{1}{(a-d)(b-d)(c-d)(d-e)(x-d)} + \frac{1}{(a-e)(b-e)(c-e)(d-e)(x-e)}.$$

The fractions of the integrands within the contributions  $\left[\chi_0^{(5,5)}(\mathbf{k}, z)\right]_3, \left[\chi_0^{(5,5)}(\mathbf{k}, z)\right]_4, \left[\chi_0^{(5,5)}(\mathbf{k}, z)\right]_{15}, \left[\chi_0^{(5,5)}(\mathbf{k}, z)\right]_{16}, \left[\chi_0^{(5,5)}(\mathbf{k}, z)\right]_{17}, \left[\chi_0^{(5,5)}(\mathbf{k}, z)\right]_{18}, \left[\chi_0^{(5,5)}(\mathbf{k}, z)\right]_{29}$ , have **three simple real poles and one double real pole**. This only becomes apparent when utilizing the algebraic identity  $(\epsilon_{q+k} - \epsilon_{q-2k})/3 = \epsilon_q - \epsilon_{q-k}$  for  $\left[\chi_0^{(5,5)}(\mathbf{k}, z)\right]_{30}$ , the algebraic identity  $(\epsilon_{q+2k} - \epsilon_{q-k})/3 = \epsilon_{q+k} - \epsilon_q$  for  $\left[\chi_0^{(5,5)}(\mathbf{k}, z)\right]_4$ , the algebraic identity  $(\epsilon_{q+3k} - \epsilon_{q-2k})/5 = (\epsilon_{q+2k} - \epsilon_{q-k})/3$  for  $\left[\chi_0^{(5,5)}(\mathbf{k}, z)\right]_{15}$ , the algebraic identity  $(\epsilon_{q+4k} - \epsilon_{q-k})/5 = (\epsilon_{q+3k} - \epsilon_{q-2k})/3$  for  $\left[\chi_0^{(5,5)}(\mathbf{k}, z)\right]_{16}$ , the algebraic identity  $(\epsilon_{q+k} - \epsilon_{q-4k})/5 = (\epsilon_q - \epsilon_{q-3k})/3$  for  $\left[\chi_0^{(5,5)}(\mathbf{k}, z)\right]_{17}$ , the algebraic identity  $(\epsilon_{q+2k} - \epsilon_{q-3k})/5 = (\epsilon_{q+k} - \epsilon_{q-2k})/3$  for  $\left[\chi_0^{(5,5)}(\mathbf{k}, z)\right]_{18}$ , the algebraic identity  $(\epsilon_{q+k} - \epsilon_{q-2k})/3 = \epsilon_q - \epsilon_{q-k}$  for  $\left[\chi_0^{(5,5)}(\mathbf{k}, z)\right]_{29}$  and the algebraic identity  $(\epsilon_{q+2k} - \epsilon_{q-k})/3 = \epsilon_{q+k} - \epsilon_q$  for  $\left[\chi_0^{(5,5)}(\mathbf{k}, z)\right]_{30}$ . It is straightforward to demonstrate by solving the emerging  $5 \times 5$  set of equations that their partial fraction decomposition follows

$$\frac{1}{(x-a)(x-b)(x-c)(x-d)^2} = \frac{1}{(a-b)(a-c)(a-d)^2(x-a)} - \frac{1}{(a-b)(b-c)(b-d)^2(x-b)} + \frac{1}{(a-c)(b-c)(c-d)^2(x-c)} - \frac{1}{(a-d)(b-d)(c-d)^2(x-d)} - \frac{1}{(a-d)^2(b-d)^2(c-d)^2(x-d)^2}.$$

The fractions of the integrands within the contributions  $\left[\chi_0^{(5,5)}(\mathbf{k}, z)\right]_{13}, \left[\chi_0^{(5,5)}(\mathbf{k}, z)\right]_{14}, \left[\chi_0^{(5,5)}(\mathbf{k}, z)\right]_{19}, \left[\chi_0^{(5,5)}(\mathbf{k}, z)\right]_{20}$ , have **two simple real poles and one triple real pole**. This only becomes apparent when utilizing the algebraic identity  $(\epsilon_{q+2k} - \epsilon_{q-3k})/5 = (\epsilon_{q+k} - \epsilon_{q-2k})/3 = \epsilon_q - \epsilon_{q-k}$  for  $\left[\chi_0^{(5,5)}(\mathbf{k}, z)\right]_{13}$ , the algebraic identity  $(\epsilon_{q+3k} - \epsilon_{q-2k})/5 = (\epsilon_{q+2k} - \epsilon_{q-k})/3$  for  $\left[\chi_0^{(5,5)}(\mathbf{k}, z)\right]_{14}$ , the algebraic identity  $(\epsilon_{q+2k} - \epsilon_{q-k})/3 = \epsilon_{q+k} - \epsilon_q$  for  $\left[\chi_0^{(5,5)}(\mathbf{k}, z)\right]_{19}$ , and the algebraic identity  $(\epsilon_{q+3k} - \epsilon_{q-2k})/5 = (\epsilon_{q+2k} - \epsilon_{q-k})/3 = (\epsilon_{q+k} - \epsilon_{q-2k})/3 = \epsilon_q - \epsilon_{q-k}$  for  $\left[\chi_0^{(5,5)}(\mathbf{k}, z)\right]_{20}$ , and the algebraic identity  $(\epsilon_{q+2k} - \epsilon_{q-k})/3 = \epsilon_{q+k} - \epsilon_q$  for  $\left[\chi_0^{(5,5)}(\mathbf{k}, z)\right]_{20}$ . It is straightforward to demonstrate by solving the emerging  $5 \times 5$  set of equations that their partial fraction decomposition follows

$$\frac{1}{(x-a)(x-b)(x-c)^3} = \frac{1}{(a-b)(a-c)^3(x-a)} - \frac{1}{(a-b)(b-c)^3(x-b)} + \frac{1}{(a-c)(b-c)^3(x-c)} - \frac{1}{(a-c)^2(b-c)^2(x-c)^2} + \frac{1}{(a-c)^3(b-c)^3(x-c)^3}.$$

It is worth pointing out that for all the four latter contributions we have  $a + b - 2c = 0$  and, thus, this leads to

$$\frac{1}{(x-a)(x-b)(x-c)^3} = \frac{1}{(a-b)(a-c)^3(x-a)} - \frac{1}{(a-b)(b-c)^3(x-b)} + \frac{(a-b)^2 + 3(a-c)(b-c)}{(a-c)^3(b-c)^3(x-c)} \\ + \frac{(a-c)(b-c)(x-c)^3}{1}.$$

The fractions of the integrands within the contributions  $\left[\chi_0^{(5,5)}(\mathbf{k}, z)\right]_5$ ,  $\left[\chi_0^{(5,5)}(\mathbf{k}, z)\right]_7$ ,  $\left[\chi_0^{(5,5)}(\mathbf{k}, z)\right]_8$ ,  $\left[\chi_0^{(5,5)}(\mathbf{k}, z)\right]_9$ ,  $\left[\chi_0^{(5,5)}(\mathbf{k}, z)\right]_{10}$ ,  $\left[\chi_0^{(5,5)}(\mathbf{k}, z)\right]_{23}$ ,  $\left[\chi_0^{(5,5)}(\mathbf{k}, z)\right]_{24}$ ,  $\left[\chi_0^{(5,5)}(\mathbf{k}, z)\right]_{25}$ ,  $\left[\chi_0^{(5,5)}(\mathbf{k}, z)\right]_{26}$ ,  $\left[\chi_0^{(5,5)}(\mathbf{k}, z)\right]_{27}$ ,  $\left[\chi_0^{(5,5)}(\mathbf{k}, z)\right]_{28}$ , have **one simple real pole and two double real poles**. This only becomes apparent when utilizing the algebraic identities  $(\epsilon_q + \mathbf{k} - \epsilon_{q-3\mathbf{k}})/4 = (\epsilon_q - \epsilon_{q-2\mathbf{k}})/2$ ,  $(\epsilon_q + \mathbf{k} - \epsilon_{q-2\mathbf{k}})/3 = \epsilon_q - \epsilon_{q-\mathbf{k}}$  for  $\left[\chi_0^{(5,5)}(\mathbf{k}, z)\right]_5$ , the algebraic identities  $(\epsilon_q + 2\mathbf{k} - \epsilon_{q-2\mathbf{k}})/4 = (\epsilon_q + \mathbf{k} - \epsilon_{q-\mathbf{k}})/2$ ,  $(\epsilon_q + 2\mathbf{k} - \epsilon_{q-3\mathbf{k}})/5 = \epsilon_q - \epsilon_{q-\mathbf{k}}$  for  $\left[\chi_0^{(5,5)}(\mathbf{k}, z)\right]_7$ , the algebraic identities  $(\epsilon_q + \mathbf{k} - \epsilon_{q-\mathbf{k}})/4 = (\epsilon_q + 2\mathbf{k} - \epsilon_{q-2\mathbf{k}})/5 = \epsilon_q - \epsilon_{q-\mathbf{k}}$  for  $\left[\chi_0^{(5,5)}(\mathbf{k}, z)\right]_8$ , the algebraic identities  $(\epsilon_q + \mathbf{k} - \epsilon_{q-3\mathbf{k}})/4 = (\epsilon_q - \epsilon_{q-2\mathbf{k}})/2$ ,  $(\epsilon_q + 2\mathbf{k} - \epsilon_{q-3\mathbf{k}})/5 = (\epsilon_q + \mathbf{k} - \epsilon_{q-2\mathbf{k}})/3$  for  $\left[\chi_0^{(5,5)}(\mathbf{k}, z)\right]_{10}$ , the algebraic identities  $(\epsilon_q + 2\mathbf{k} - \epsilon_{q-2\mathbf{k}})/4 = (\epsilon_q + \mathbf{k} - \epsilon_{q-\mathbf{k}})/2$ , the algebraic identities  $(\epsilon_q + 3\mathbf{k} - \epsilon_{q-\mathbf{k}})/4 = (\epsilon_q + 2\mathbf{k} - \epsilon_{q-2\mathbf{k}})/5 = (\epsilon_q + \mathbf{k} - \epsilon_{q-\mathbf{k}})/2$ , the algebraic identities  $(\epsilon_q + 3\mathbf{k} - \epsilon_{q-2\mathbf{k}})/5 = \epsilon_q - \epsilon_{q-\mathbf{k}}$  for  $\left[\chi_0^{(5,5)}(\mathbf{k}, z)\right]_{23}$ , the algebraic identities  $(\epsilon_q + 2\mathbf{k} - \epsilon_{q-2\mathbf{k}})/4 = (\epsilon_q + \mathbf{k} - \epsilon_{q-\mathbf{k}})/2$ , the algebraic identities  $(\epsilon_q + 2\mathbf{k} - \epsilon_{q-2\mathbf{k}})/5 = \epsilon_q - \epsilon_{q-\mathbf{k}}$  for  $\left[\chi_0^{(5,5)}(\mathbf{k}, z)\right]_{24}$ , the algebraic identities  $(\epsilon_q + \mathbf{k} - \epsilon_{q-2\mathbf{k}})/4 = (\epsilon_q + 2\mathbf{k} - \epsilon_{q-2\mathbf{k}})/5 = \epsilon_q - \epsilon_{q-\mathbf{k}}$  for  $\left[\chi_0^{(5,5)}(\mathbf{k}, z)\right]_{25}$ , the algebraic identities  $(\epsilon_q + 2\mathbf{k} - \epsilon_{q-2\mathbf{k}})/4 = (\epsilon_q + \mathbf{k} - \epsilon_{q-\mathbf{k}})/2$ ,  $(\epsilon_q + 3\mathbf{k} - \epsilon_{q-2\mathbf{k}})/5 = \epsilon_q - \epsilon_{q-\mathbf{k}}$  for  $\left[\chi_0^{(5,5)}(\mathbf{k}, z)\right]_{26}$ , the algebraic identities  $(\epsilon_q + 2\mathbf{k} - \epsilon_{q-2\mathbf{k}})/4 = (\epsilon_q + \mathbf{k} - \epsilon_{q-\mathbf{k}})/2$ ,  $(\epsilon_q + 3\mathbf{k} - \epsilon_{q-2\mathbf{k}})/5 = (\epsilon_q + 2\mathbf{k} - \epsilon_{q-2\mathbf{k}})/3 = \epsilon_q - \epsilon_{q-\mathbf{k}}$  for  $\left[\chi_0^{(5,5)}(\mathbf{k}, z)\right]_{27}$ , the algebraic identities  $(\epsilon_q + 3\mathbf{k} - \epsilon_{q-\mathbf{k}})/4 = (\epsilon_q + 2\mathbf{k} - \epsilon_{q-2\mathbf{k}})/5 = (\epsilon_q + \mathbf{k} - \epsilon_{q-\mathbf{k}})/2$ ,  $(\epsilon_q + 2\mathbf{k} - \epsilon_{q-2\mathbf{k}})/3 = \epsilon_q - \epsilon_{q-\mathbf{k}}$  for  $\left[\chi_0^{(5,5)}(\mathbf{k}, z)\right]_{28}$ . It is straightforward to demonstrate by solving the emerging  $5 \times 5$  set of equations that their partial fraction decomposition follows

$$\frac{1}{(x-a)(x-b)^2(x-c)^2} = \frac{1}{(a-b)^2(a-c)^2(x-a)} + \frac{2a-3b+c}{(a-b)^2(b-c)^3(x-b)} - \frac{2a+b-3c}{(a-c)^2(b-c)^3(x-c)} \\ - \frac{(a-b)(b-c)^2(x-b)^2}{(a-b)^2(b-c)^2(x-c)^2}.$$

The fractions of the integrands within the contributions  $\left[\chi_0^{(5,5)}(\mathbf{k}, z)\right]_{11}$ ,  $\left[\chi_0^{(5,5)}(\mathbf{k}, z)\right]_{12}$ ,  $\left[\chi_0^{(5,5)}(\mathbf{k}, z)\right]_{21}$ ,  $\left[\chi_0^{(5,5)}(\mathbf{k}, z)\right]_{22}$ , have **one double real pole and one triple real pole**. This only becomes apparent when utilizing the algebraic identities  $(\epsilon_q + 2\mathbf{k} - \epsilon_{q-2\mathbf{k}})/4 = (\epsilon_q + \mathbf{k} - \epsilon_{q-\mathbf{k}})/2$ ,  $(\epsilon_q + 2\mathbf{k} - \epsilon_{q-3\mathbf{k}})/5 = (\epsilon_q + \mathbf{k} - \epsilon_{q-2\mathbf{k}})/3 = \epsilon_q - \epsilon_{q-\mathbf{k}}$  for  $\left[\chi_0^{(5,5)}(\mathbf{k}, z)\right]_{11}$ , the algebraic identities  $(\epsilon_q + 3\mathbf{k} - \epsilon_{q-\mathbf{k}})/4 = (\epsilon_q + 2\mathbf{k} - \epsilon_{q-2\mathbf{k}})/5 = (\epsilon_q + \mathbf{k} - \epsilon_{q-\mathbf{k}})/2$ , the algebraic identities  $(\epsilon_q + 2\mathbf{k} - \epsilon_{q-2\mathbf{k}})/4 = (\epsilon_q + \mathbf{k} - \epsilon_{q-\mathbf{k}})/2$ ,  $(\epsilon_q + 3\mathbf{k} - \epsilon_{q-2\mathbf{k}})/5 = (\epsilon_q + 2\mathbf{k} - \epsilon_{q-2\mathbf{k}})/3 = \epsilon_q - \epsilon_{q-\mathbf{k}}$  for  $\left[\chi_0^{(5,5)}(\mathbf{k}, z)\right]_{12}$ , the algebraic identities  $(\epsilon_q + 2\mathbf{k} - \epsilon_{q-2\mathbf{k}})/4 = (\epsilon_q + \mathbf{k} - \epsilon_{q-\mathbf{k}})/2$ , the algebraic identities  $(\epsilon_q + 2\mathbf{k} - \epsilon_{q-2\mathbf{k}})/5 = (\epsilon_q + \mathbf{k} - \epsilon_{q-\mathbf{k}})/2$ ,  $(\epsilon_q + 3\mathbf{k} - \epsilon_{q-2\mathbf{k}})/5 = (\epsilon_q + 2\mathbf{k} - \epsilon_{q-2\mathbf{k}})/3 = \epsilon_q - \epsilon_{q-\mathbf{k}}$  for  $\left[\chi_0^{(5,5)}(\mathbf{k}, z)\right]_{21}$ , the algebraic identities  $(\epsilon_q + 2\mathbf{k} - \epsilon_{q-2\mathbf{k}})/4 = (\epsilon_q + \mathbf{k} - \epsilon_{q-\mathbf{k}})/2$ ,  $(\epsilon_q + 3\mathbf{k} - \epsilon_{q-2\mathbf{k}})/5 = (\epsilon_q + 2\mathbf{k} - \epsilon_{q-2\mathbf{k}})/3 = \epsilon_q - \epsilon_{q-\mathbf{k}}$  for  $\left[\chi_0^{(5,5)}(\mathbf{k}, z)\right]_{22}$ . It is straightforward to demonstrate by solving the emerging  $5 \times 5$  set of equations that their partial fraction decomposition follows

$$\frac{1}{(x-a)^2(x-b)^3} = -\frac{3}{(a-b)^4(x-a)} + \frac{3}{(a-b)^4(x-b)} + \frac{1}{(a-b)^3(x-a)^2} + \frac{2}{(a-b)^3(x-b)^2} \\ + \frac{(a-b)^2(x-b)^3}{(a-b)^2(x-b)^3}.$$

Given the above, there are  $4 \times 5 = 20$  terms from the first group of contributions,  $8 \times 5 = 40$  terms from the second group of contributions,  $4 \times 4 = 16$  terms from the third group of contributions,  $12 \times 5 = 60$  terms from the fourth group of contributions and  $4 \times 5 = 20$  terms from the fifth group of contributions. These translate to  $20 + 40 + 16 + 60 + 20 = 156$  terms that constitute the ideal fifth order density response  $\chi_0^{(5,5)}(\mathbf{k}, z)$ .



The *first contribution* is characterized by five simple poles. We first identify and calculate the coefficients  $a, b, c, d, e$ .

$$\begin{aligned}
\left[ \chi_0^{(5,5)}(\mathbf{k}, z) \right]_1 &= - \int \frac{d^3 q}{(2\pi)^3} \frac{2f_0(\mathbf{q})}{(5\hbar z - \epsilon_q + \epsilon_{q-5\mathbf{k}})(4\hbar z - \epsilon_q + \epsilon_{q-4\mathbf{k}})(3\hbar z - \epsilon_q + \epsilon_{q-3\mathbf{k}})(2\hbar z - \epsilon_q + \epsilon_{q-2\mathbf{k}})(\hbar z - \epsilon_q + \epsilon_{q-\mathbf{k}})} \Rightarrow \\
\left[ \chi_0^{(5,5)}(\mathbf{k}, z) \right]_1 &= - \int \frac{d^3 q}{(2\pi)^3} \frac{f_0(\mathbf{q})}{60} \frac{1}{\left[ \hbar z - \frac{\epsilon_q - \epsilon_{q-5\mathbf{k}}}{5} \right] \left[ \hbar z - \frac{\epsilon_q - \epsilon_{q-4\mathbf{k}}}{4} \right] \left[ \hbar z - \frac{\epsilon_q - \epsilon_{q-3\mathbf{k}}}{3} \right] \left[ \hbar z - \frac{\epsilon_q - \epsilon_{q-2\mathbf{k}}}{2} \right] \left[ \hbar z - (\epsilon_q - \epsilon_{q-\mathbf{k}}) \right]} \Rightarrow \\
a &= \frac{\epsilon_q - \epsilon_{q-5\mathbf{k}}}{5} = \frac{\hbar^2}{2m} \frac{q^2 - (\mathbf{q} - 5\mathbf{k})^2}{5} = \frac{\hbar^2}{2m} \frac{-25k^2 + 10\mathbf{q} \cdot \mathbf{k}}{5} = \frac{\hbar^2}{2m} (-5k^2 + 2\mathbf{q} \cdot \mathbf{k}), \\
b &= \frac{\epsilon_q - \epsilon_{q-4\mathbf{k}}}{4} = \frac{\hbar^2}{2m} \frac{q^2 - (\mathbf{q} - 4\mathbf{k})^2}{4} = \frac{\hbar^2}{2m} \frac{-16k^2 + 8\mathbf{q} \cdot \mathbf{k}}{4} = \frac{\hbar^2}{2m} (-4k^2 + 2\mathbf{q} \cdot \mathbf{k}), \\
c &= \frac{\epsilon_q - \epsilon_{q-3\mathbf{k}}}{3} = \frac{\hbar^2}{2m} \frac{q^2 - (\mathbf{q} - 3\mathbf{k})^2}{3} = \frac{\hbar^2}{2m} \frac{-9k^2 + 6\mathbf{q} \cdot \mathbf{k}}{3} = \frac{\hbar^2}{2m} (-3k^2 + 2\mathbf{q} \cdot \mathbf{k}), \\
d &= \frac{\epsilon_q - \epsilon_{q-2\mathbf{k}}}{2} = \frac{\hbar^2}{2m} \frac{q^2 - (\mathbf{q} - 2\mathbf{k})^2}{2} = \frac{\hbar^2}{2m} \frac{-4k^2 + 4\mathbf{q} \cdot \mathbf{k}}{2} = \frac{\hbar^2}{2m} (-2k^2 + 2\mathbf{q} \cdot \mathbf{k}), \\
e &= \epsilon_q - \epsilon_{q-\mathbf{k}} = \frac{\hbar^2}{2m} [q^2 - (\mathbf{q} - \mathbf{k})^2] = \frac{\hbar^2}{2m} (-k^2 + 2\mathbf{q} \cdot \mathbf{k}).
\end{aligned}$$

Then, we compute all the possible differences between these four coefficients. Note that  $q^2$  and  $\mathbf{q} \cdot \mathbf{k}$  terms vanish.

$$\begin{aligned}
a - b &= \frac{\hbar^2}{2m} (-5k^2 + 2\mathbf{q} \cdot \mathbf{k} + 4k^2 - 2\mathbf{q} \cdot \mathbf{k}) = \frac{\hbar^2}{2m} (-5k^2 + 4k^2) = \frac{\hbar^2}{2m} (-k^2), & b - c &= \frac{\hbar^2}{2m} (-4k^2 + 2\mathbf{q} \cdot \mathbf{k} + 3k^2 - 2\mathbf{q} \cdot \mathbf{k}) = \frac{\hbar^2}{2m} (-4k^2 + 3k^2) = \frac{\hbar^2}{2m} (-k^2), \\
c - d &= \frac{\hbar^2}{2m} (-3k^2 + 2\mathbf{q} \cdot \mathbf{k} + 2k^2 - 2\mathbf{q} \cdot \mathbf{k}) = \frac{\hbar^2}{2m} (-3k^2 + 2k^2) = \frac{\hbar^2}{2m} (-k^2), & d - e &= \frac{\hbar^2}{2m} (-2k^2 + 2\mathbf{q} \cdot \mathbf{k} + k^2 - 2\mathbf{q} \cdot \mathbf{k}) = \frac{\hbar^2}{2m} (-2k^2 + k^2) = \frac{\hbar^2}{2m} (-k^2), \\
a - c &= \frac{\hbar^2}{2m} (-5k^2 + 2\mathbf{q} \cdot \mathbf{k} + 3k^2 - 2\mathbf{q} \cdot \mathbf{k}) = \frac{\hbar^2}{2m} (-5k^2 + 3k^2) = \frac{\hbar^2}{2m} (-2k^2), & b - d &= \frac{\hbar^2}{2m} (-4k^2 + 2\mathbf{q} \cdot \mathbf{k} + 2k^2 - 2\mathbf{q} \cdot \mathbf{k}) = \frac{\hbar^2}{2m} (-4k^2 + 2k^2) = \frac{\hbar^2}{2m} (-2k^2), \\
c - e &= \frac{\hbar^2}{2m} (-3k^2 + 2\mathbf{q} \cdot \mathbf{k} + k^2 - 2\mathbf{q} \cdot \mathbf{k}) = \frac{\hbar^2}{2m} (-3k^2 + k^2) = \frac{\hbar^2}{2m} (-2k^2), & a - d &= \frac{\hbar^2}{2m} (-5k^2 + 2\mathbf{q} \cdot \mathbf{k} + 2k^2 - 2\mathbf{q} \cdot \mathbf{k}) = \frac{\hbar^2}{2m} (-5k^2 + 2k^2) = \frac{\hbar^2}{2m} (-3k^2), \\
b - e &= \frac{\hbar^2}{2m} (-4k^2 + 2\mathbf{q} \cdot \mathbf{k} + k^2 - 2\mathbf{q} \cdot \mathbf{k}) = \frac{\hbar^2}{2m} (-4k^2 + k^2) = \frac{\hbar^2}{2m} (-3k^2), & a - e &= \frac{\hbar^2}{2m} (-5k^2 + 2\mathbf{q} \cdot \mathbf{k} + k^2 - 2\mathbf{q} \cdot \mathbf{k}) = \frac{\hbar^2}{2m} (-5k^2 + k^2) = \frac{\hbar^2}{2m} (-4k^2),
\end{aligned}$$

Afterwards, we compute all the triple difference combinations that are present in the partial fraction decomposition.

$$\begin{aligned}
(a-b)(a-c)(a-d)(a-e) &= \frac{\hbar^2}{2m} (-k^2) \frac{\hbar^2}{2m} (-2k^2) \frac{\hbar^2}{2m} (-3k^2) \frac{\hbar^2}{2m} (-4k^2) = \left( \frac{\hbar^2}{2m} \right)^4 (24k^8), & (a-b)(b-c)(b-d)(b-e) &= \frac{\hbar^2}{2m} (-k^2) \frac{\hbar^2}{2m} (-k^2) \frac{\hbar^2}{2m} (-2k^2) \frac{\hbar^2}{2m} (-3k^2) = \left( \frac{\hbar^2}{2m} \right)^4 (6k^8), \\
(a-c)(b-c)(c-d)(c-e) &= \frac{\hbar^2}{2m} (-2k^2) \frac{\hbar^2}{2m} (-k^2) \frac{\hbar^2}{2m} (-k^2) \frac{\hbar^2}{2m} (-2k^2) = \left( \frac{\hbar^2}{2m} \right)^4 (4k^8), & (a-d)(b-d)(c-d)(d-e) &= \frac{\hbar^2}{2m} (-3k^2) \frac{\hbar^2}{2m} (-2k^2) \frac{\hbar^2}{2m} (-k^2) = \left( \frac{\hbar^2}{2m} \right)^4 (6k^8), \\
(a-e)(b-e)(c-e)(d-e) &= \frac{\hbar^2}{2m} (-4k^2) \frac{\hbar^2}{2m} (-3k^2) \frac{\hbar^2}{2m} (-2k^2) \frac{\hbar^2}{2m} (-k^2) = \left( \frac{\hbar^2}{2m} \right)^4 (24k^8).
\end{aligned}$$

Finally, we substitute the above in the contribution and perform some straightforward algebra.

$$\begin{aligned}
\left[ \chi_0^{(5,5)}(\mathbf{k}, z) \right]_1 &= - \int \frac{d^3 q}{(2\pi)^3} \left( \frac{2m}{\hbar^2} \right)^4 \frac{1}{24k^8} \frac{1}{60} \frac{f_0(\mathbf{q})}{\left[ \hbar z - \frac{\epsilon_q - \epsilon_{q-5\mathbf{k}}}{5} \right] \left[ \hbar z - \frac{\epsilon_q - \epsilon_{q-4\mathbf{k}}}{4} \right] \left[ \hbar z - \frac{\epsilon_q - \epsilon_{q-3\mathbf{k}}}{3} \right] \left[ \hbar z - \frac{\epsilon_q - \epsilon_{q-2\mathbf{k}}}{2} \right] \left[ \hbar z - \epsilon_q + \epsilon_{q-\mathbf{k}} \right]} \Rightarrow \\
\left[ \chi_0^{(5,5)}(\mathbf{k}, z) \right]_1 &= - \left( \frac{m}{\hbar^2} \right)^4 \frac{1}{180k^8} \int \frac{d^3 q}{(2\pi)^3} \frac{2f_0(\mathbf{q})}{\left[ \hbar z - \frac{\epsilon_q - \epsilon_{q-5\mathbf{k}}}{5} \right] \left[ \hbar z - \frac{\epsilon_q - \epsilon_{q-4\mathbf{k}}}{4} \right] \left[ \hbar z - \frac{\epsilon_q - \epsilon_{q-3\mathbf{k}}}{3} \right] \left[ \hbar z - \frac{\epsilon_q - \epsilon_{q-2\mathbf{k}}}{2} \right] \left[ \hbar z - \epsilon_q + \epsilon_{q-\mathbf{k}} \right]} \Rightarrow \\
\left[ \chi_0^{(5,5)}(\mathbf{k}, z) \right]_1 &= - \left( \frac{m}{\hbar^2} \right)^4 \frac{1}{180k^8} \int \frac{d^3 q}{(2\pi)^3} \frac{2f_0(\mathbf{q})}{\left[ 5\hbar z - \epsilon_q + \epsilon_{q-5\mathbf{k}} \right] \left[ 4\hbar z - \epsilon_q + \epsilon_{q-4\mathbf{k}} \right] \left[ 3\hbar z - \epsilon_q + \epsilon_{q-3\mathbf{k}} \right] \left[ 2\hbar z - \epsilon_q + \epsilon_{q-2\mathbf{k}} \right] \left[ \hbar z - \epsilon_q + \epsilon_{q-\mathbf{k}} \right]}.
\end{aligned}$$

The *second contribution* is characterized by five simple poles. We first identify and calculate the coefficients  $a, b, c, d, e$ .

$$\begin{aligned}
\left[ \chi_0^{(5,5)}(\mathbf{k}, z) \right]_2 &= + \int \frac{d^3 q}{(2\pi)^3} \frac{2f_0(\mathbf{q})}{(5\hbar z - \epsilon_{\mathbf{q}+\mathbf{k}} + \epsilon_{\mathbf{q}-4\mathbf{k}})(4\hbar z - \epsilon_{\mathbf{q}+\mathbf{k}} + \epsilon_{\mathbf{q}-3\mathbf{k}})(3\hbar z - \epsilon_{\mathbf{q}+\mathbf{k}} + \epsilon_{\mathbf{q}-2\mathbf{k}})(2\hbar z - \epsilon_{\mathbf{q}+\mathbf{k}} + \epsilon_{\mathbf{q}-\mathbf{k}})(\hbar z - \epsilon_{\mathbf{q}+\mathbf{k}} + \epsilon_{\mathbf{q}})} \\
\left[ \chi_0^{(5,5)}(\mathbf{k}, z) \right]_2 &= + \int \frac{d^3 q}{(2\pi)^3} \frac{f_0(\mathbf{q})}{60} \left[ \hbar z - \frac{\epsilon_{\mathbf{q}+\mathbf{k}} - \epsilon_{\mathbf{q}-4\mathbf{k}}}{5} \right] \left[ \hbar z - \frac{\epsilon_{\mathbf{q}+\mathbf{k}} - \epsilon_{\mathbf{q}-3\mathbf{k}}}{4} \right] \left[ \hbar z - \frac{\epsilon_{\mathbf{q}+\mathbf{k}} - \epsilon_{\mathbf{q}-2\mathbf{k}}}{3} \right] \left[ \hbar z - \frac{\epsilon_{\mathbf{q}+\mathbf{k}} - \epsilon_{\mathbf{q}-\mathbf{k}}}{2} \right] \\
a &= \frac{\epsilon_{\mathbf{q}+\mathbf{k}} - \epsilon_{\mathbf{q}-4\mathbf{k}}}{5} = \frac{\hbar^2}{2m} \frac{(q+\mathbf{k})^2 - (q-4\mathbf{k})^2}{5} = \frac{\hbar^2}{2m} \frac{k^2 + 2\mathbf{q} \cdot \mathbf{k} - 16k^2 + 8\mathbf{q} \cdot \mathbf{k}}{5} = \frac{\hbar^2}{2m} \frac{-15k^2 + 10\mathbf{q} \cdot \mathbf{k}}{5} = \frac{\hbar^2}{2m} (-3k^2 + 2\mathbf{q} \cdot \mathbf{k}), \\
b &= \frac{\epsilon_{\mathbf{q}+\mathbf{k}} - \epsilon_{\mathbf{q}-3\mathbf{k}}}{4} = \frac{\hbar^2}{2m} \frac{(q+\mathbf{k})^2 - (q-3\mathbf{k})^2}{4} = \frac{\hbar^2}{2m} \frac{k^2 + 2\mathbf{q} \cdot \mathbf{k} - 9k^2 + 6\mathbf{q} \cdot \mathbf{k}}{4} = \frac{\hbar^2}{2m} \frac{-8k^2 + 8\mathbf{q} \cdot \mathbf{k}}{4} = \frac{\hbar^2}{2m} (-2k^2 + 2\mathbf{q} \cdot \mathbf{k}), \\
c &= \frac{\epsilon_{\mathbf{q}+\mathbf{k}} - \epsilon_{\mathbf{q}-2\mathbf{k}}}{3} = \frac{\hbar^2}{2m} \frac{(q+\mathbf{k})^2 - (q-2\mathbf{k})^2}{3} = \frac{\hbar^2}{2m} \frac{k^2 + 2\mathbf{q} \cdot \mathbf{k} - 4k^2 + 4\mathbf{q} \cdot \mathbf{k}}{3} = \frac{\hbar^2}{2m} \frac{-3k^2 + 6\mathbf{q} \cdot \mathbf{k}}{3} = \frac{\hbar^2}{2m} (-k^2 + 2\mathbf{q} \cdot \mathbf{k}), \\
d &= \frac{\epsilon_{\mathbf{q}+\mathbf{k}} - \epsilon_{\mathbf{q}-\mathbf{k}}}{2} = \frac{\hbar^2}{2m} \frac{(q+\mathbf{k})^2 - (q-\mathbf{k})^2}{2} = \frac{\hbar^2}{2m} \frac{k^2 + 2\mathbf{q} \cdot \mathbf{k} - k^2 + 2\mathbf{q} \cdot \mathbf{k}}{2} = \frac{\hbar^2}{2m} \frac{4\mathbf{q} \cdot \mathbf{k}}{2} = \frac{\hbar^2}{2m} (2\mathbf{q} \cdot \mathbf{k}), \\
e &= \epsilon_{\mathbf{q}+\mathbf{k}} - \epsilon_{\mathbf{q}} = \frac{\hbar^2}{2m} [(q+\mathbf{k})^2 - q^2] = \frac{\hbar^2}{2m} (k^2 + 2\mathbf{q} \cdot \mathbf{k}).
\end{aligned}$$

Then, we compute all the possible differences between these four coefficients. Note that  $q^2$  and  $\mathbf{q} \cdot \mathbf{k}$  terms vanish.

$$\begin{aligned}
a - b &= \frac{\hbar^2}{2m} (-3k^2 + 2\mathbf{q} \cdot \mathbf{k} + 2k^2 - 2\mathbf{q} \cdot \mathbf{k}) = \frac{\hbar^2}{2m} (-3k^2 + 2k^2) = \frac{\hbar^2}{2m} (-k^2), & b - c &= \frac{\hbar^2}{2m} (-2k^2 + 2\mathbf{q} \cdot \mathbf{k} + k^2 - 2\mathbf{q} \cdot \mathbf{k}) = \frac{\hbar^2}{2m} (-2k^2 + k^2) = \frac{\hbar^2}{2m} (-k^2), \\
c - d &= \frac{\hbar^2}{2m} (-k^2 + 2\mathbf{q} \cdot \mathbf{k} - 2\mathbf{q} \cdot \mathbf{k}) = \frac{\hbar^2}{2m} (-k^2) = \frac{\hbar^2}{2m} (-k^2), & d - e &= \frac{\hbar^2}{2m} (2\mathbf{q} \cdot \mathbf{k} - k^2 - 2\mathbf{q} \cdot \mathbf{k}) = \frac{\hbar^2}{2m} (-k^2) = \frac{\hbar^2}{2m} (-k^2), \\
a - c &= \frac{\hbar^2}{2m} (-3k^2 + 2\mathbf{q} \cdot \mathbf{k} + k^2 - 2\mathbf{q} \cdot \mathbf{k}) = \frac{\hbar^2}{2m} (-3k^2 + k^2) = \frac{\hbar^2}{2m} (-2k^2), & b - d &= \frac{\hbar^2}{2m} (-2k^2 + 2\mathbf{q} \cdot \mathbf{k} - 2\mathbf{q} \cdot \mathbf{k}) = \frac{\hbar^2}{2m} (-2k^2) = \frac{\hbar^2}{2m} (-2k^2), \\
c - e &= \frac{\hbar^2}{2m} (-k^2 + 2\mathbf{q} \cdot \mathbf{k} - k^2 - 2\mathbf{q} \cdot \mathbf{k}) = \frac{\hbar^2}{2m} (-k^2 - k^2) = \frac{\hbar^2}{2m} (-2k^2), & a - d &= \frac{\hbar^2}{2m} (-3k^2 + 2\mathbf{q} \cdot \mathbf{k} - 2\mathbf{q} \cdot \mathbf{k}) = \frac{\hbar^2}{2m} (-3k^2) = \frac{\hbar^2}{2m} (-3k^2), \\
b - e &= \frac{\hbar^2}{2m} (-2k^2 + 2\mathbf{q} \cdot \mathbf{k} - k^2 - 2\mathbf{q} \cdot \mathbf{k}) = \frac{\hbar^2}{2m} (-2k^2 - k^2) = \frac{\hbar^2}{2m} (-3k^2), & a - e &= \frac{\hbar^2}{2m} (-3k^2 + 2\mathbf{q} \cdot \mathbf{k} - k^2 - 2\mathbf{q} \cdot \mathbf{k}) = \frac{\hbar^2}{2m} (-3k^2 - k^2) = \frac{\hbar^2}{2m} (-4k^2),
\end{aligned}$$

Afterwards, we compute all the triple difference combinations that are present in the partial fraction decomposition.

$$\begin{aligned}
(a-b)(a-c)(a-d)(a-e) &= \frac{\hbar^2}{2m} (-k^2) \frac{\hbar^2}{2m} (-2k^2) \frac{\hbar^2}{2m} (-3k^2) \frac{\hbar^2}{2m} (-4k^2) = \left( \frac{\hbar^2}{2m} \right)^4 (24k^8), & (a-b)(b-c)(b-d)(b-e) &= \frac{\hbar^2}{2m} (-k^2) \frac{\hbar^2}{2m} (-k^2) \frac{\hbar^2}{2m} (-2k^2) \frac{\hbar^2}{2m} (-3k^2) = \left( \frac{\hbar^2}{2m} \right)^4 (6k^8), \\
(a-c)(b-c)(c-d)(c-e) &= \frac{\hbar^2}{2m} (-2k^2) \frac{\hbar^2}{2m} (-k^2) \frac{\hbar^2}{2m} (-k^2) \frac{\hbar^2}{2m} (-2k^2) = \left( \frac{\hbar^2}{2m} \right)^4 (4k^8), & (a-d)(b-d)(c-d)(d-e) &= \frac{\hbar^2}{2m} (-3k^2) \frac{\hbar^2}{2m} (-2k^2) \frac{\hbar^2}{2m} (-k^2) = \left( \frac{\hbar^2}{2m} \right)^4 (6k^8), \\
(a-e)(b-e)(c-e)(d-e) &= \frac{\hbar^2}{2m} (-4k^2) \frac{\hbar^2}{2m} (-3k^2) \frac{\hbar^2}{2m} (-2k^2) \frac{\hbar^2}{2m} (-k^2) = \left( \frac{\hbar^2}{2m} \right)^4 (24k^8).
\end{aligned}$$

Finally, we substitute the above in the contribution and perform some straightforward algebra.

$$\begin{aligned}
\left[ \chi_0^{(5,5)}(\mathbf{k}, z) \right]_2 &= + \int \frac{d^3 q}{(2\pi)^3} \left( \frac{2m}{\hbar^2} \right)^4 \frac{1}{24k^8} \frac{f_0(\mathbf{q})}{60} \left[ \frac{1}{\hbar z - \frac{\epsilon_{\mathbf{q}+\mathbf{k}} - \epsilon_{\mathbf{q}-4\mathbf{k}}}{5}} - \frac{4}{\hbar z - \frac{\epsilon_{\mathbf{q}+\mathbf{k}} - \epsilon_{\mathbf{q}-3\mathbf{k}}}{4}} + \frac{6}{\hbar z - \frac{\epsilon_{\mathbf{q}+\mathbf{k}} - \epsilon_{\mathbf{q}-2\mathbf{k}}}{3}} - \frac{4}{\hbar z - \frac{\epsilon_{\mathbf{q}+\mathbf{k}} - \epsilon_{\mathbf{q}-\mathbf{k}}}{2}} + \frac{1}{\hbar z - \epsilon_{\mathbf{q}+\mathbf{k}} + \epsilon_{\mathbf{q}}} \right] \\
\left[ \chi_0^{(5,5)}(\mathbf{k}, z) \right]_2 &= + \left( \frac{m}{\hbar^2} \right)^4 \frac{1}{180k^8} \int \frac{d^3 q}{(2\pi)^3} \frac{2f_0(\mathbf{q})}{60} \left[ \frac{1}{\hbar z - \frac{\epsilon_{\mathbf{q}+\mathbf{k}} - \epsilon_{\mathbf{q}-4\mathbf{k}}}{5}} - \frac{4}{\hbar z - \frac{\epsilon_{\mathbf{q}+\mathbf{k}} - \epsilon_{\mathbf{q}-3\mathbf{k}}}{4}} + \frac{6}{\hbar z - \frac{\epsilon_{\mathbf{q}+\mathbf{k}} - \epsilon_{\mathbf{q}-2\mathbf{k}}}{3}} - \frac{4}{\hbar z - \frac{\epsilon_{\mathbf{q}+\mathbf{k}} - \epsilon_{\mathbf{q}-\mathbf{k}}}{2}} + \frac{1}{\hbar z - \epsilon_{\mathbf{q}+\mathbf{k}} + \epsilon_{\mathbf{q}}} \right] \\
\left[ \chi_0^{(5,5)}(\mathbf{k}, z) \right]_2 &= + \left( \frac{m}{\hbar^2} \right)^4 \frac{1}{180k^8} \int \frac{d^3 q}{(2\pi)^3} \frac{2f_0(\mathbf{q})}{60} \left[ \frac{1}{5\hbar z - \epsilon_{\mathbf{q}+\mathbf{k}} + \epsilon_{\mathbf{q}-4\mathbf{k}}} - \frac{4}{4\hbar z - \epsilon_{\mathbf{q}+\mathbf{k}} + \epsilon_{\mathbf{q}-3\mathbf{k}}} + \frac{6}{3\hbar z - \epsilon_{\mathbf{q}+\mathbf{k}} + \epsilon_{\mathbf{q}-2\mathbf{k}}} - \frac{4}{2\hbar z - \epsilon_{\mathbf{q}+\mathbf{k}} + \epsilon_{\mathbf{q}-\mathbf{k}}} + \frac{1}{\hbar z - \epsilon_{\mathbf{q}+\mathbf{k}} + \epsilon_{\mathbf{q}}} \right].
\end{aligned}$$

The *third contribution* is characterized by three simple poles and one double pole. This becomes apparent from the algebraic identity  $(\epsilon_q + k - \epsilon_{q-2k})/3 = (\epsilon_q - \epsilon_{q-k})$ . We first identify and calculate the coefficients  $a, b, c, d$ .

$$\begin{aligned}
\left[ \chi_0^{(5,5)}(\mathbf{k}, z) \right]_3 &= + \int \frac{d^3 q}{(2\pi)^3} \frac{2 f_0(\mathbf{q})}{(5\hbar z - \epsilon_{q+k} + \epsilon_{q-4k})(4\hbar z - \epsilon_{q+k} + \epsilon_{q-3k})(3\hbar z - \epsilon_{q+k} + \epsilon_{q-2k})(2\hbar z - \epsilon_{q+k} + \epsilon_{q-k})(\hbar z - \epsilon_q + \epsilon_{q-k})} \Rightarrow \\
\left[ \chi_0^{(5,5)}(\mathbf{k}, z) \right]_3 &= + \int \frac{d^3 q}{(2\pi)^3} \frac{f_0(\mathbf{q})}{60} \left[ \hbar z - \frac{\epsilon_{q+k} - \epsilon_{q-4k}}{5} \right] \left[ \hbar z - \frac{\epsilon_{q+k} - \epsilon_{q-3k}}{4} \right] \left[ \hbar z - \frac{\epsilon_{q+k} - \epsilon_{q-2k}}{3} \right] \left[ \hbar z - \frac{\epsilon_{q+k} - \epsilon_{q-k}}{2} \right] \Rightarrow \\
\left[ \chi_0^{(5,5)}(\mathbf{k}, z) \right]_3 &= + \int \frac{d^3 q}{(2\pi)^3} \frac{f_0(\mathbf{q})}{60} \left[ \hbar z - \frac{\epsilon_{q+k} - \epsilon_{q-4k}}{5} \right] \left[ \hbar z - \frac{\epsilon_{q+k} - \epsilon_{q-3k}}{4} \right] \left[ \hbar z - \frac{\epsilon_{q+k} - \epsilon_{q-2k}}{3} \right] \left[ \hbar z - \frac{\epsilon_{q+k} - \epsilon_{q-k}}{2} \right] \Rightarrow \\
\left[ \chi_0^{(5,5)}(\mathbf{k}, z) \right]_3 &= + \int \frac{d^3 q}{(2\pi)^3} \frac{f_0(\mathbf{q})}{60} \left[ \hbar z - \frac{\epsilon_{q+k} - \epsilon_{q-4k}}{5} \right] \left[ \hbar z - \frac{\epsilon_{q+k} - \epsilon_{q-3k}}{4} \right] \left[ \hbar z - \frac{\epsilon_{q+k} - \epsilon_{q-2k}}{3} \right] \left[ \hbar z - \frac{\epsilon_{q+k} - \epsilon_{q-k}}{2} \right] \Rightarrow \\
a &= \frac{\epsilon_{q+k} - \epsilon_{q-4k}}{5} = \frac{\hbar^2}{2m} \frac{(q+k)^2 - (q-4k)^2}{5} = \frac{\hbar^2}{2m} \frac{k^2 + 2q \cdot k - 16k^2 + 8q \cdot k}{5} = \frac{\hbar^2}{2m} \frac{k^2 - 15k^2 + 10q \cdot k}{5} = \frac{\hbar^2}{2m} \frac{(-3k^2 + 2q \cdot k)}{5} \\
b &= \frac{\epsilon_{q+k} - \epsilon_{q-3k}}{4} = \frac{\hbar^2}{2m} \frac{(q+k)^2 - (q-3k)^2}{4} = \frac{\hbar^2}{2m} \frac{k^2 + 2q \cdot k - 9k^2 + 6q \cdot k}{4} = \frac{\hbar^2}{2m} \frac{k^2 - 8k^2 + 8q \cdot k}{4} = \frac{\hbar^2}{2m} \frac{(-2k^2 + 2q \cdot k)}{4} \\
c &= \frac{\epsilon_{q+k} - \epsilon_{q-k}}{2} = \frac{\hbar^2}{2m} \frac{(q+k)^2 - (q-k)^2}{2} = \frac{\hbar^2}{2m} \frac{k^2 + 2q \cdot k - k^2 + 2q \cdot k}{2} = \frac{\hbar^2}{2m} \frac{4q \cdot k}{2} = \frac{\hbar^2}{2m} (2q \cdot k) \\
d &= (\epsilon_q - \epsilon_{q-k}) = \frac{\hbar^2}{2m} [q^2 - (q-k)^2] = \frac{\hbar^2}{2m} (-k^2 + 2q \cdot k).
\end{aligned}$$

Then, we compute all the relevant algebraic combinations between the coefficients. Note that  $q^2$  and  $q \cdot k$  terms vanish.

$$\begin{aligned}
a - b &= \frac{\hbar^2}{2m} \frac{(-3k^2 + 2q \cdot k + 2k^2 - 2q \cdot k)}{5} = \frac{\hbar^2}{2m} \frac{(-3k^2 + 2k^2)}{5} = \frac{\hbar^2}{2m} \frac{(-k^2)}{5}, \quad b - c = \frac{\hbar^2}{2m} \frac{(-2k^2 + 2q \cdot k - 2q \cdot k)}{4} = \frac{\hbar^2}{2m} \frac{(-2k^2)}{4} \\
c - d &= \frac{\hbar^2}{2m} \frac{(2q \cdot k + k^2 - 2q \cdot k)}{2} = \frac{\hbar^2}{2m} \frac{(-3k^2 + 2q \cdot k - 2q \cdot k)}{2} = \frac{\hbar^2}{2m} \frac{(-3k^2)}{2} \\
b - d &= \frac{\hbar^2}{2m} \frac{(-2k^2 + 2q \cdot k + k^2 - 2q \cdot k)}{2} = \frac{\hbar^2}{2m} \frac{(-2k^2 + k^2)}{2} = \frac{\hbar^2}{2m} \frac{(-k^2)}{2}, \quad a - d = \frac{\hbar^2}{2m} \frac{(-3k^2 + 2q \cdot k + k^2 - 2q \cdot k)}{2} = \frac{\hbar^2}{2m} \frac{(-3k^2 + k^2)}{2} = \frac{\hbar^2}{2m} \frac{(-2k^2)}{2}.
\end{aligned}$$

Afterwards, we compute all the combinations that are present in the partial fraction decomposition.

$$\begin{aligned}
(a-b)(a-c)(a-d)^2 &= \left( \frac{\hbar^2}{2m} \right)^4 \frac{(-k^2)^4}{(-3k^2)(4k^4)} = \left( \frac{\hbar^2}{2m} \right)^4 \frac{(12k^8)}{(12k^8)}, \quad (a-b)(b-c)(b-d)^2 = \left( \frac{\hbar^2}{2m} \right)^4 \frac{(-k^2)^4}{(-2k^2)(-2k^2)} = \left( \frac{\hbar^2}{2m} \right)^4 \frac{(2k^8)}{(2k^8)}, \\
(a-c)(b-c)(c-d)^2 &= \left( \frac{\hbar^2}{2m} \right)^4 \frac{(-3k^2)^4}{(-2k^2)(-2k^2)} = \left( \frac{\hbar^2}{2m} \right)^4 \frac{(6k^8)}{(6k^8)}, \quad (a-d)(b-d)(c-d) = \left( \frac{\hbar^2}{2m} \right)^3 \frac{(-2k^2)^3}{(-2k^2)(-k^2)} = \left( \frac{\hbar^2}{2m} \right)^3 \frac{(2k^6)}{(2k^6)}, \\
(a-d)^2(b-d)^2(c-d)^2 &= \left( \frac{\hbar^2}{2m} \right)^6 \frac{(4k^{12})}{(a-b)(b-c) + (a-d)^2 + (b-d)^2 + (c-d)^2 - (a-c)^2} = \left( \frac{\hbar^2}{2m} \right)^2 \frac{(2k^4 + 4k^4 + k^4 - 9k^4)}{(2m)} = \left( \frac{\hbar^2}{2m} \right)^2 \frac{(-k^4)}{(-k^4)}.
\end{aligned}$$

Finally, we substitute and perform some straightforward algebra. We also introduce the compact notation  $\epsilon_k = (\hbar^2 k^2)/(2m)$ .

$$\begin{aligned}
\left[ \chi_0^{(5,5)}(\mathbf{k}, z) \right]_3 &= + \int \frac{d^3 q}{(2\pi)^3} \frac{2m}{\left( \frac{\hbar^2}{2m} \right)^4} \frac{1}{12k^8} \frac{f_0(\mathbf{q})}{60} \left[ \frac{1}{\hbar z - \frac{\epsilon_{q+k} - \epsilon_{q-4k}}{5}} - \frac{6}{\hbar z - \frac{\epsilon_{q+k} - \epsilon_{q-3k}}{4}} + \frac{2}{\hbar z - \frac{\epsilon_{q+k} - \epsilon_{q-2k}}{3}} + \frac{3}{\hbar z - \epsilon_q + \epsilon_{q-k}} - \frac{\hbar^2}{2m} \frac{6k^2}{(\hbar z - \epsilon_q + \epsilon_{q-k})^2} \right] \Rightarrow \\
\left[ \chi_0^{(5,5)}(\mathbf{k}, z) \right]_3 &= + \left( \frac{m}{\hbar^2} \right)^4 \frac{1}{90k^8} \int \frac{d^3 q}{(2\pi)^3} \frac{2f_0(\mathbf{q})}{60} \left[ \frac{1}{\hbar z - \frac{\epsilon_{q+k} - \epsilon_{q-4k}}{5}} - \frac{6}{\hbar z - \frac{\epsilon_{q+k} - \epsilon_{q-3k}}{4}} + \frac{2}{\hbar z - \frac{\epsilon_{q+k} - \epsilon_{q-2k}}{3}} + \frac{3}{\hbar z - \epsilon_q + \epsilon_{q-k}} - \frac{6\epsilon_k}{(\hbar z - \epsilon_q + \epsilon_{q-k})^2} \right] \Rightarrow \\
\left[ \chi_0^{(5,5)}(\mathbf{k}, z) \right]_3 &= + \left( \frac{m}{\hbar^2} \right)^4 \frac{1}{180k^8} \int \frac{d^3 q}{(2\pi)^3} \frac{2f_0(\mathbf{q})}{60} \left[ \frac{10}{5\hbar z - \epsilon_q + \epsilon_{q-k} + \epsilon_{q-4k}} - \frac{48}{4\hbar z - \epsilon_q + \epsilon_{q-k} + \epsilon_{q-3k}} + \frac{8}{2\hbar z - \epsilon_q + \epsilon_{q-k} + \epsilon_{q-k}} + \frac{6}{\hbar z - \epsilon_q + \epsilon_{q-k}} - \frac{12\epsilon_k}{(\hbar z - \epsilon_q + \epsilon_{q-k})^2} \right].
\end{aligned}$$

The *fourth contribution* is characterized by three simple poles and one double pole. This becomes apparent from the algebraic identity  $(\epsilon_q + 2k - \epsilon_q - k)/3 = (\epsilon_q + k - \epsilon_q)$ . We first identify and calculate the coefficients  $a, b, c, d$ .

$$\begin{aligned}
\left[ \chi_0^{(5,5)}(\mathbf{k}, z) \right]_4 &= - \int \frac{d^3 q}{(2\pi)^3} \frac{2 f_0(q)}{(5hz - \epsilon_q + 2k + \epsilon_q - 3k) (4hz - \epsilon_q + 2k + \epsilon_q - 2k) (3hz - \epsilon_q + 2k + \epsilon_q - k) (hz - \epsilon_q + k + \epsilon_q)} \Rightarrow \\
\left[ \chi_0^{(5,5)}(\mathbf{k}, z) \right]_4 &= - \int \frac{d^3 q}{(2\pi)^3} \frac{f_0(q)}{60} \left[ \overline{hz - \frac{\epsilon_q + 2k - \epsilon_q - 3k}{5}} \right]_4 \left[ \overline{hz - \frac{\epsilon_q + 2k - \epsilon_q - 2k}{4}} \right]_4 \left[ \overline{hz - \frac{\epsilon_q + 2k - \epsilon_q - k}{3}} \right]_4 \left[ \overline{hz - (\epsilon_q + k - \epsilon_q)} \right]_4 \Rightarrow \\
\left[ \chi_0^{(5,5)}(\mathbf{k}, z) \right]_4 &= - \int \frac{d^3 q}{(2\pi)^3} \frac{f_0(q)}{60} \left[ \overline{hz - \frac{\epsilon_q + 2k - \epsilon_q - 3k}{5}} \right]_4 \left[ \overline{hz - \frac{\epsilon_q + 2k - \epsilon_q - 2k}{4}} \right]_4 \left[ \overline{hz - (\epsilon_q + k - \epsilon_q)} \right]_4 \left[ \overline{hz - (\epsilon_q + k - \epsilon_q)} \right]_4 \Rightarrow \\
\left[ \chi_0^{(5,5)}(\mathbf{k}, z) \right]_4 &= - \int \frac{d^3 q}{(2\pi)^3} \frac{f_0(q)}{60} \left[ \overline{hz - \frac{\epsilon_q + 2k - \epsilon_q - 3k}{5}} \right]_4 \left[ \overline{hz - \frac{\epsilon_q + 2k - \epsilon_q - 2k}{4}} \right]_4 \left[ \overline{hz - (\epsilon_q + k - \epsilon_q)} \right]_4 \left[ \overline{hz - (\epsilon_q + k - \epsilon_q)} \right]_4 \Rightarrow \\
a &= \frac{\epsilon_q + 2k - \epsilon_q - 3k}{5} = \frac{\hbar^2}{2m} \frac{(q + 2k)^2 - (q - 3k)^2}{5} = \frac{\hbar^2}{2m} \frac{4k^2 + 4q \cdot k - 9k^2 + 6q \cdot k}{5} = \frac{\hbar^2}{2m} \frac{-5k^2 + 10q \cdot k}{5} = \frac{\hbar^2}{2m} (-k^2 + 2q \cdot k) \\
b &= \frac{\epsilon_q + 2k - \epsilon_q - 2k}{4} = \frac{\hbar^2}{2m} \frac{(q + 2k)^2 - (q - 2k)^2}{4} = \frac{\hbar^2}{2m} \frac{4k^2 + 4q \cdot k - 4k^2 + 4q \cdot k}{4} = \frac{\hbar^2}{2m} \frac{8q \cdot k}{4} = \frac{\hbar^2}{2m} (2q \cdot k) \\
c &= \frac{\epsilon_q + 2k - \epsilon_q}{2} = \frac{\hbar^2}{2m} \frac{(q + 2k)^2 - q^2}{2} = \frac{\hbar^2}{2m} \frac{4k^2 + 4q \cdot k}{2} = \frac{\hbar^2}{2m} (2k^2 + 2q \cdot k) \\
d &= (\epsilon_q + k - \epsilon_q) = \frac{\hbar^2}{2m} [(q + k)^2 - q^2] = \frac{\hbar^2}{2m} (k^2 + 2q \cdot k).
\end{aligned}$$

Then, we compute all the relevant algebraic combinations between the coefficients. Note that  $q^2$  and  $q \cdot k$  terms vanish.

$$\begin{aligned}
a - b &= \frac{\hbar^2}{2m} (-k^2 + 2q \cdot k - 2q \cdot k) = \frac{\hbar^2}{2m} (-k^2), \quad b - c = \frac{\hbar^2}{2m} (2q \cdot k - 2k^2 - 2q \cdot k) = \frac{\hbar^2}{2m} (-2k^2) \\
c - d &= \frac{\hbar^2}{2m} (2k^2 + 2q \cdot k - k^2 - 2q \cdot k) = \frac{\hbar^2}{2m} (k^2), \quad a - c = \frac{\hbar^2}{2m} (-k^2 + 2q \cdot k - 2k^2 - 2q \cdot k) = \frac{\hbar^2}{2m} (-3k^2) \\
b - d &= \frac{\hbar^2}{2m} (2q \cdot k - k^2 - 2q \cdot k) = \frac{\hbar^2}{2m} (-k^2), \quad a - d = \frac{\hbar^2}{2m} (-k^2 + 2q \cdot k - k^2 - 2q \cdot k) = \frac{\hbar^2}{2m} (-2k^2).
\end{aligned}$$

Afterwards, we compute all the combinations that are present in the partial fraction decomposition.

$$\begin{aligned}
(a - b)(a - c)(a - d)^2 &= \left( \frac{\hbar^2}{2m} \right)^4 (-k^2)^2 (-3k^2) (4k^4) = \left( \frac{\hbar^2}{2m} \right)^4 (12k^8), \quad (a - b)(b - c)(b - d)^2 = \left( \frac{\hbar^2}{2m} \right)^4 (-k^2)^2 (-2k^2) (k^4) = \left( \frac{\hbar^2}{2m} \right)^4 (2k^8), \\
(a - c)(b - c)(c - d)^2 &= \left( \frac{\hbar^2}{2m} \right)^4 (-3k^2)^2 (-2k^2) (k^4) = \left( \frac{\hbar^2}{2m} \right)^4 (6k^8), \quad (a - d)(b - d)(c - d)^2 = \left( \frac{\hbar^2}{2m} \right)^3 (-2k^2)^2 (-k^2) (k^2) = \left( \frac{\hbar^2}{2m} \right)^3 (2k^6), \\
(a - d)^2(b - d)^2(c - d)^2 &= \left( \frac{\hbar^2}{2m} \right)^6 (4k^{12}), \quad (a - b)(b - c) + (a - d)^2 + (b - d)^2 + (c - d)^2 = \left( \frac{\hbar^2}{2m} \right)^2 (2k^4 + 4k^4 + k^4 - 9k^4) = \left( \frac{\hbar^2}{2m} \right)^2 (-k^4).
\end{aligned}$$

Finally, we substitute and perform some straightforward algebra. We also introduce the compact notation  $\epsilon_k = (\hbar^2 k^2)/(2m)$ .

$$\begin{aligned}
\left[ \chi_0^{(5,5)}(\mathbf{k}, z) \right]_4 &= - \int \frac{d^3 q}{(2\pi)^3} \left( \frac{2m}{\hbar^2} \right)^4 \frac{1}{12k^8} \frac{f_0(q)}{60} \left[ \overline{hz - \frac{\epsilon_q + 2k - \epsilon_q - 3k}{5}} - \frac{6}{hz - \frac{\epsilon_q + 2k - \epsilon_q - 2k}{4}} + \frac{2}{hz - \frac{\epsilon_q + 2k - \epsilon_q - k}{3}} + \frac{3}{hz - (\epsilon_q + k + \epsilon_q)} - \frac{6k^2}{2m(hz - \epsilon_q + k + \epsilon_q)} \right] \Rightarrow \\
\left[ \chi_0^{(5,5)}(\mathbf{k}, z) \right]_4 &= - \left( \frac{m}{\hbar^2} \right)^4 \frac{1}{90k^8} \int \frac{d^3 q}{(2\pi)^3} \frac{2f_0(q)}{60} \left[ \overline{hz - \frac{\epsilon_q + 2k - \epsilon_q - 3k}{5}} - \frac{6}{hz - \frac{\epsilon_q + 2k - \epsilon_q - 2k}{4}} + \frac{2}{hz - \frac{\epsilon_q + 2k - \epsilon_q - k}{3}} + \frac{3}{hz - (\epsilon_q + k + \epsilon_q)} - \frac{6\epsilon_k}{(hz - \epsilon_q + k + \epsilon_q)^2} \right] \Rightarrow \\
\left[ \chi_0^{(5,5)}(\mathbf{k}, z) \right]_4 &= - \left( \frac{m}{\hbar^2} \right)^4 \frac{1}{180k^8} \int \frac{d^3 q}{(2\pi)^3} \frac{2f_0(q)}{60} \left[ \overline{5hz - \epsilon_q + 2k + \epsilon_q - 3k} - \frac{48}{4hz - \epsilon_q + 2k + \epsilon_q - 2k} + \frac{8}{2hz - \epsilon_q + 2k + \epsilon_q} + \frac{6}{(hz - \epsilon_q + k + \epsilon_q)} - \frac{12\epsilon_k}{(hz - \epsilon_q + k + \epsilon_q)^2} \right].
\end{aligned}$$

The *fifth contribution* is characterized by one simple pole and two double poles. This becomes apparent from the algebraic identities  $(\epsilon_q + \mathbf{k} - \epsilon_{q-3\mathbf{k}})/4 = (\epsilon_q - \epsilon_{q-2\mathbf{k}})/2$  and  $(\epsilon_q + \mathbf{k} - \epsilon_{q-2\mathbf{k}})/3 = (\epsilon_q - \epsilon_{q-\mathbf{k}})$ . We first identify and calculate the coefficients  $a, b, c$ .

$$\begin{aligned}
\left[ \chi_0^{(5,5)}(\mathbf{k}, z) \right]_5 &= + \int \frac{d^3 q}{(2\pi)^3} \frac{5\hbar z - \epsilon_q + \mathbf{k} + \epsilon_{q-4\mathbf{k}}}{(2\pi)^3} \frac{2f_0(\mathbf{q})}{60} \frac{(3\hbar z - \epsilon_q + \mathbf{k} + \epsilon_{q-3\mathbf{k}})(2\hbar z - \epsilon_q + \epsilon_{q-2\mathbf{k}})(\hbar z - \epsilon_q + \epsilon_{q-\mathbf{k}})}{60} \Rightarrow \\
\left[ \chi_0^{(5,5)}(\mathbf{k}, z) \right]_5 &= + \int \frac{d^3 q}{(2\pi)^3} \frac{f_0(\mathbf{q})}{60} \frac{1}{\left[ \hbar z - \frac{\epsilon_q + \mathbf{k} - \epsilon_{q-4\mathbf{k}}}{5} \right] \left[ \hbar z - \frac{\epsilon_q + \mathbf{k} - \epsilon_{q-3\mathbf{k}}}{4} \right] \left[ \hbar z - \frac{\epsilon_q + \mathbf{k} - \epsilon_{q-2\mathbf{k}}}{3} \right] \left[ \hbar z - (\epsilon_q - \epsilon_{q-\mathbf{k}}) \right]} \Rightarrow \\
\left[ \chi_0^{(5,5)}(\mathbf{k}, z) \right]_5 &= + \int \frac{d^3 q}{(2\pi)^3} \frac{f_0(\mathbf{q})}{60} \frac{1}{\left[ \hbar z - \frac{\epsilon_q + \mathbf{k} - \epsilon_{q-4\mathbf{k}}}{5} \right] \left[ \hbar z - \frac{\epsilon_q - \epsilon_{q-2\mathbf{k}}}{2} \right]^2 \left[ \hbar z - (\epsilon_q - \epsilon_{q-\mathbf{k}}) \right]^2} \Rightarrow \\
a = \frac{\epsilon_q + \mathbf{k} - \epsilon_{q-4\mathbf{k}}}{5} &= \frac{\hbar^2}{2m} \frac{(q + \mathbf{k})^2 - (q - 4\mathbf{k})^2}{2} = \frac{2m}{5} \frac{\hbar^2}{2} \frac{k^2 + 2\mathbf{q} \cdot \mathbf{k} - 16k^2 + 8\mathbf{q} \cdot \mathbf{k} - 15k^2 + 10\mathbf{q} \cdot \mathbf{k}}{5} = \frac{\hbar^2}{2m} (-3k^2 + 2\mathbf{q} \cdot \mathbf{k}) \\
b = \frac{\epsilon_q - \epsilon_{q-2\mathbf{k}}}{2} &= \frac{\hbar^2}{2m} \frac{q^2 - (q - 2\mathbf{k})^2}{2} = \frac{2m}{2} \frac{\hbar^2}{2} \frac{-4k^2 + 4\mathbf{q} \cdot \mathbf{k}}{2} = \frac{\hbar^2}{2m} (-2k^2 + 2\mathbf{q} \cdot \mathbf{k}) \\
c = \epsilon_q - \epsilon_{q-\mathbf{k}} &= \frac{\hbar^2}{2m} [q^2 - (q - \mathbf{k})^2] = \frac{\hbar^2}{2m} (-k^2 + 2\mathbf{q} \cdot \mathbf{k}).
\end{aligned}$$

Then, we compute all the relevant algebraic combinations between these three coefficients. Note that  $q^2$  and  $\mathbf{q} \cdot \mathbf{k}$  terms vanish.

$$\begin{aligned}
a - b &= \frac{\hbar^2}{2m} (-3k^2 + 2\mathbf{q} \cdot \mathbf{k} + 2k^2 - 2\mathbf{q} \cdot \mathbf{k}) = \frac{\hbar^2}{2m} (-k^2), \quad b - c = \frac{\hbar^2}{2m} (-2k^2 + 2\mathbf{q} \cdot \mathbf{k} + k^2 - 2\mathbf{q} \cdot \mathbf{k}) = \frac{\hbar^2}{2m} (-2k^2 + k^2) = \frac{\hbar^2}{2m} (-k^2), \\
a - c &= \frac{\hbar^2}{2m} (-3k^2 + 2\mathbf{q} \cdot \mathbf{k} + k^2 - 2\mathbf{q} \cdot \mathbf{k}) = \frac{\hbar^2}{2m} (-3k^2 + k^2) = \frac{\hbar^2}{2m} (-2k^2), \quad 2a - 3b + c = \frac{\hbar^2}{2m} (-6k^2 + 4\mathbf{q} \cdot \mathbf{k} + 6k^2 - 6\mathbf{q} \cdot \mathbf{k} - k^2 + 2\mathbf{q} \cdot \mathbf{k}) = \frac{\hbar^2}{2m} (-6k^2 + 6k^2 - k^2) = \frac{\hbar^2}{2m} (-k^2), \\
2a + b - 3c &= \frac{\hbar^2}{2m} (-6k^2 + 4\mathbf{q} \cdot \mathbf{k} - 2k^2 + 2\mathbf{q} \cdot \mathbf{k} + 3k^2 - 6\mathbf{q} \cdot \mathbf{k}) = \frac{\hbar^2}{2m} (-5k^2).
\end{aligned}$$

Afterwards, we compute all the combinations that are present in the partial fraction decomposition.

$$\begin{aligned}
(a - b)^2(a - c)^2 &= \left( \frac{\hbar^2}{2m} \right)^2 (k^4) \left( \frac{\hbar^2}{2m} \right)^2 (4k^4) = \left( \frac{\hbar^2}{2m} \right)^4 (4k^8), \quad (a - b)^2(b - c)^3 = \left( \frac{\hbar^2}{2m} \right)^2 (k^4) \left( \frac{\hbar^2}{2m} \right)^3 (-k^6) = \left( \frac{\hbar^2}{2m} \right)^5 (-k^{10}), \\
(a - c)^2(b - c)^3 &= \left( \frac{\hbar^2}{2m} \right)^2 (4k^4) \left( \frac{\hbar^2}{2m} \right)^3 (-k^6) = \left( \frac{\hbar^2}{2m} \right)^5 (-4k^{10}), \quad (a - b)(b - c)^2 = \frac{\hbar^2}{2m} (-k^2) \left( \frac{\hbar^2}{2m} \right)^2 (k^4) = \left( \frac{\hbar^2}{2m} \right)^3 (-k^6), \\
(a - c)(b - c)^2 &= \frac{\hbar^2}{2m} (-2k^2) \left( \frac{\hbar^2}{2m} \right)^2 (k^4) = \left( \frac{\hbar^2}{2m} \right)^3 (-2k^6).
\end{aligned}$$

Finally, we substitute and perform some straightforward algebra. We also introduce the compact notation  $\epsilon_{\mathbf{k}} = (\hbar^2 k^2)/(2m)$ .

$$\begin{aligned}
\left[ \chi_0^{(5,5)}(\mathbf{k}, z) \right]_5 &= + \int \frac{d^3 q}{(2\pi)^3} \left( \frac{2m}{\hbar^2} \right)^4 \frac{1}{4k^8} \frac{f_0(\mathbf{q})}{60} \left[ \frac{1}{\hbar z - \frac{\epsilon_q + \mathbf{k} - \epsilon_{q-4\mathbf{k}}}{5}} + \frac{4}{\hbar z - \frac{\epsilon_q - \epsilon_{q-2\mathbf{k}}}{2}} - \frac{5}{\hbar z - \epsilon_q + \epsilon_{q-\mathbf{k}}} + \frac{\hbar^2}{2m} \frac{4k^2}{\left( \hbar z - \frac{\epsilon_q - \epsilon_{q-2\mathbf{k}}}{2} \right)^2} + \frac{\hbar^2}{2m} \frac{2k^2}{(\hbar z - \epsilon_q + \epsilon_{q-\mathbf{k}})^2} \right] \Rightarrow \\
\left[ \chi_0^{(5,5)}(\mathbf{k}, z) \right]_5 &= + \int \frac{d^3 q}{(2\pi)^3} \left( \frac{m}{\hbar^2} \right)^4 \frac{1}{k^8} \frac{2f_0(\mathbf{q})}{30} \left[ \frac{1}{\hbar z - \frac{\epsilon_q + \mathbf{k} - \epsilon_{q-4\mathbf{k}}}{5}} + \frac{4}{\hbar z - \frac{\epsilon_q - \epsilon_{q-2\mathbf{k}}}{2}} - \frac{5}{\hbar z - \epsilon_q + \epsilon_{q-\mathbf{k}}} + \frac{4\epsilon_{\mathbf{k}}}{\left( \hbar z - \frac{\epsilon_q - \epsilon_{q-2\mathbf{k}}}{2} \right)^2} + \frac{2\epsilon_{\mathbf{k}}}{(\hbar z - \epsilon_q + \epsilon_{q-\mathbf{k}})^2} \right] \Rightarrow \\
\left[ \chi_0^{(5,5)}(\mathbf{k}, z) \right]_5 &= + \left( \frac{m}{\hbar^2} \right)^4 \frac{1}{30k^8} \int \frac{d^3 q}{(2\pi)^3} \frac{2f_0(\mathbf{q})}{8} \left[ \frac{1}{\hbar z - \frac{\epsilon_q + \mathbf{k} - \epsilon_{q-4\mathbf{k}}}{5}} + \frac{4}{\hbar z - \frac{\epsilon_q - \epsilon_{q-2\mathbf{k}}}{2}} - \frac{5}{\hbar z - \epsilon_q + \epsilon_{q-\mathbf{k}}} + \frac{4\epsilon_{\mathbf{k}}}{\left( \hbar z - \frac{\epsilon_q - \epsilon_{q-2\mathbf{k}}}{2} \right)^2} + \frac{2\epsilon_{\mathbf{k}}}{(\hbar z - \epsilon_q + \epsilon_{q-\mathbf{k}})^2} \right] \Rightarrow \\
\left[ \chi_0^{(5,5)}(\mathbf{k}, z) \right]_5 &= + \left( \frac{m}{\hbar^2} \right)^4 \frac{1}{180k^8} \int \frac{d^3 q}{(2\pi)^3} \frac{2f_0(\mathbf{q})}{8} \left[ \frac{30}{5\hbar z - \epsilon_q + \mathbf{k} + \epsilon_{q-4\mathbf{k}}} + \frac{48}{2\hbar z - \epsilon_q + \epsilon_{q-2\mathbf{k}}} - \frac{30}{\hbar z - \epsilon_q + \epsilon_{q-\mathbf{k}}} + \frac{96\epsilon_{\mathbf{k}}}{(2\hbar z - \epsilon_q + \epsilon_{q-2\mathbf{k}})^2} + \frac{12\epsilon_{\mathbf{k}}}{(\hbar z - \epsilon_q + \epsilon_{q-\mathbf{k}})^2} \right].
\end{aligned}$$

The *sixth contribution* is characterized by one simple pole and two double poles. This becomes apparent from the algebraic identities  $(\epsilon_q + 2k - \epsilon_q - 2k)/4 = (\epsilon_q + k - \epsilon_q - k)/2$  and  $(\epsilon_q + 2k - \epsilon_q - k)/3 = (\epsilon_q + k - \epsilon_q)$ . We first identify and calculate the coefficients  $a, b, c$ .

$$\begin{aligned}
[\chi_0^{(5,5)}(\mathbf{k}, z)]_6 &= - \int \frac{d^3 q}{(2\pi)^3} \frac{(5\hbar z - \epsilon_q + 2k + \epsilon_q - 3k)(4\hbar z - \epsilon_q + 2k + \epsilon_q - 2k)(3\hbar z - \epsilon_q + 2k + \epsilon_q - k)(2\hbar z - \epsilon_q + k + \epsilon_q - k)(\hbar z - \epsilon_q + k + \epsilon_q)}{2f_0(\mathbf{q})} \Rightarrow \\
[\chi_0^{(5,5)}(\mathbf{k}, z)]_6 &= - \int \frac{d^3 q}{(2\pi)^3} \frac{f_0(\mathbf{q})}{60} \frac{1}{\left[\hbar z - \frac{\epsilon_q + 2k - \epsilon_q - 3k}{5}\right] \left[\hbar z - \frac{\epsilon_q + 2k - \epsilon_q - 2k}{4}\right] \left[\hbar z - \frac{\epsilon_q + 2k - \epsilon_q - k}{3}\right] \left[\hbar z - (\epsilon_q + k - \epsilon_q)\right]} \Rightarrow \\
[\chi_0^{(5,5)}(\mathbf{k}, z)]_6 &= - \int \frac{d^3 q}{(2\pi)^3} \frac{f_0(\mathbf{q})}{60} \frac{1}{\left[\hbar z - \frac{\epsilon_q + 2k - \epsilon_q - 3k}{5}\right] \left[\hbar z - \frac{\epsilon_q + k - \epsilon_q - k}{2}\right]^2 \left[\hbar z - (\epsilon_q + k - \epsilon_q)\right]^2} \Rightarrow \\
a &= \frac{\epsilon_q + 2k - \epsilon_q - 3k}{5} = \frac{\hbar^2}{2m} \frac{(q + 2k)^2 - (q - 3k)^2}{(q - 3k)^2} = \frac{\hbar^2}{2m} \frac{4q \cdot k - 9k^2 + 6q \cdot k}{4k^2 + 4q \cdot k - 9k^2 + 10q \cdot k} = \frac{\hbar^2}{2m} \frac{-5k^2 + 10q \cdot k}{-k^2 + 2q \cdot k} \\
b &= \frac{\epsilon_q + k - \epsilon_q - k}{2} = \frac{\hbar^2}{2m} \frac{(q + k)^2 - (q - k)^2}{k^2} = \frac{\hbar^2}{2m} \frac{k^2 + 2q \cdot k - k^2 + 2q \cdot k}{k^2} = \frac{\hbar^2}{2m} \frac{4q \cdot k}{2q \cdot k} \\
c &= \epsilon_q + k - \epsilon_q = \frac{\hbar^2}{2m} [(q + k)^2 - q^2] = \frac{\hbar^2}{2m} (k^2 + 2q \cdot k).
\end{aligned}$$

Then, we compute all the relevant algebraic combinations between these three coefficients. Note that  $q^2$  and  $q \cdot k$  terms vanish.

$$\begin{aligned}
a - b &= \frac{\hbar^2}{2m} (-k^2 + 2q \cdot k - 2q \cdot k) = \frac{\hbar^2}{2m} (-k^2), \quad b - c = \frac{\hbar^2}{2m} (2q \cdot k - k^2 - 2q \cdot k) = \frac{\hbar^2}{2m} (-k^2), \\
a - c &= \frac{\hbar^2}{2m} (-k^2 + 2q \cdot k - k^2 - 2q \cdot k) = \frac{\hbar^2}{2m} (-k^2 - k^2) = \frac{\hbar^2}{2m} (-2k^2), \quad 2a - 3b + c = \frac{\hbar^2}{2m} (-2k^2 + 4q \cdot k - 6q \cdot k + k^2 + 2q \cdot k) = \frac{\hbar^2}{2m} (-2k^2 + k^2) = \frac{\hbar^2}{2m} (-k^2), \\
2a + b - 3c &= \frac{\hbar^2}{2m} (-2k^2 + 4q \cdot k + 2q \cdot k - 3k^2 - 6q \cdot k) = \frac{\hbar^2}{2m} (-2k^2 - 3k^2) = \frac{\hbar^2}{2m} (-5k^2).
\end{aligned}$$

Afterwards, we compute all the combinations that are present in the partial fraction decomposition.

$$\begin{aligned}
(a - b)^2(a - c)^2 &= \left(\frac{\hbar^2}{2m}\right)^2 (k^4) \left(\frac{\hbar^2}{2m}\right)^2 (4k^4) = \left(\frac{\hbar^2}{2m}\right)^4 (4k^8), \quad (a - b)^2(b - c)^3 = \left(\frac{\hbar^2}{2m}\right)^2 (k^4) \left(\frac{\hbar^2}{2m}\right)^3 (-k^6) = \left(\frac{\hbar^2}{2m}\right)^5 (-k^{10}), \\
(a - c)^2(b - c)^3 &= \left(\frac{\hbar^2}{2m}\right)^2 (4k^4) \left(\frac{\hbar^2}{2m}\right)^3 (-k^6) = \left(\frac{\hbar^2}{2m}\right)^5 (-4k^{10}), \quad (a - b)(b - c)^2 = \frac{\hbar^2}{2m} (-k^2) \left(\frac{\hbar^2}{2m}\right)^2 (k^4) = \left(\frac{\hbar^2}{2m}\right)^3 (-k^6), \\
(a - c)(b - c)^2 &= \frac{\hbar^2}{2m} (-2k^2) \left(\frac{\hbar^2}{2m}\right)^2 (k^4) = \left(\frac{\hbar^2}{2m}\right)^3 (-2k^6).
\end{aligned}$$

Finally, we substitute and perform some straightforward algebra. We also introduce the compact notation  $\epsilon_k = (\hbar^2 k^2)/(2m)$ .

$$\begin{aligned}
[\chi_0^{(5,5)}(\mathbf{k}, z)]_6 &= - \int \frac{d^3 q}{(2\pi)^3} \left(\frac{2m}{\hbar^2}\right)^4 \frac{1}{4k^8} \frac{f_0(\mathbf{q})}{60} \left[ \frac{1}{\hbar z - \frac{\epsilon_q + 2k - \epsilon_q - 3k}{5}} + \frac{4}{\hbar z - \frac{\epsilon_q + k - \epsilon_q - k}{2}} - \frac{5}{\hbar z - \epsilon_q + k + \epsilon_q} + \frac{\hbar^2}{2m} \frac{4k^2}{\left(\hbar z - \frac{\epsilon_q + k - \epsilon_q - k}{2}\right)^2} + \frac{\hbar^2}{2m} \frac{2k^2}{(\hbar z - \epsilon_q + k + \epsilon_q)^2} \right] \Rightarrow \\
[\chi_0^{(5,5)}(\mathbf{k}, z)]_6 &= - \int \frac{d^3 q}{(2\pi)^3} \left(\frac{m}{\hbar^2}\right)^4 \frac{1}{k^8} \frac{2f_0(\mathbf{q})}{30} \left[ \frac{1}{\hbar z - \frac{\epsilon_q + 2k - \epsilon_q - 3k}{5}} + \frac{4}{\hbar z - \frac{\epsilon_q + k - \epsilon_q - k}{2}} - \frac{5}{\hbar z - \epsilon_q + k + \epsilon_q} + \frac{4\epsilon_k}{\left(\hbar z - \frac{\epsilon_q + k - \epsilon_q - k}{2}\right)^2} + \frac{2\epsilon_k}{(\hbar z - \epsilon_q + k + \epsilon_q)^2} \right] \Rightarrow \\
[\chi_0^{(5,5)}(\mathbf{k}, z)]_6 &= - \left(\frac{m}{\hbar^2}\right)^4 \frac{1}{30k^8} \int \frac{d^3 q}{(2\pi)^3} \frac{2f_0(\mathbf{q})}{k^8} \left[ \frac{1}{\hbar z - \frac{\epsilon_q + 2k - \epsilon_q - 3k}{5}} + \frac{4}{\hbar z - \frac{\epsilon_q + k - \epsilon_q - k}{2}} - \frac{5}{\hbar z - \epsilon_q + k + \epsilon_q} + \frac{4\epsilon_k}{\left(\hbar z - \frac{\epsilon_q + k - \epsilon_q - k}{2}\right)^2} + \frac{2\epsilon_k}{(\hbar z - \epsilon_q + k + \epsilon_q)^2} \right] \Rightarrow \\
[\chi_0^{(5,5)}(\mathbf{k}, z)]_6 &= - \left(\frac{m}{\hbar^2}\right)^4 \frac{1}{180k^8} \int \frac{d^3 q}{(2\pi)^3} \frac{2f_0(\mathbf{q})}{k^8} \left[ \frac{30}{5\hbar z - \epsilon_q + 2k + \epsilon_q - 3k} + \frac{48}{2\hbar z - \epsilon_q + k + \epsilon_q - k} - \frac{30}{\hbar z - \epsilon_q + k + \epsilon_q} + \frac{96\epsilon_k}{(2\hbar z - \epsilon_q + k + \epsilon_q - k)^2} + \frac{12\epsilon_k}{(\hbar z - \epsilon_q + k + \epsilon_q)^2} \right].
\end{aligned}$$

The *seventh contribution* is characterized by one simple pole and two double poles. This becomes apparent from the algebraic identities  $(\epsilon_q + 2\mathbf{k} - \epsilon_q - 3\mathbf{k})/5 = (\epsilon_q - \epsilon_q - \mathbf{k})$  and  $(\epsilon_q + 2\mathbf{k} - \epsilon_q - 2\mathbf{k})/4 = (\epsilon_q + \mathbf{k} - \epsilon_q - \mathbf{k})/2$ . We first identify and calculate the coefficients  $a, b, c$ .

$$\begin{aligned}
[\chi_0^{(5,5)}(\mathbf{k}, z)]_7 &= - \int \frac{d^3 q}{(2\pi)^3} \frac{(5\hbar z - \epsilon_q + 2\mathbf{k} + \epsilon_q - 3\mathbf{k})}{(2\pi)^3} \frac{4\hbar z - \epsilon_q + 2\mathbf{k} + \epsilon_q - 2\mathbf{k}}{(2\pi)^3} \frac{(3\hbar z - \epsilon_q + 2\mathbf{k} + \epsilon_q - \mathbf{k})}{(2\pi)^3} \frac{(2\hbar z - \epsilon_q + \mathbf{k} + \epsilon_q - \mathbf{k})}{(2\pi)^3} \frac{2f_0(\mathbf{q})}{(2\pi)^3} \Rightarrow \\
[\chi_0^{(5,5)}(\mathbf{k}, z)]_7 &= - \int \frac{d^3 q}{(2\pi)^3} \frac{f_0(\mathbf{q})}{60} \frac{1}{60} \left[ \hbar z - \frac{\epsilon_q + 2\mathbf{k} - \epsilon_q - 3\mathbf{k}}{5} \right] \left[ \hbar z - \frac{\epsilon_q + 2\mathbf{k} - \epsilon_q - 2\mathbf{k}}{4} \right] \left[ \hbar z - \frac{\epsilon_q + 2\mathbf{k} - \epsilon_q - \mathbf{k}}{3} \right] \left[ \hbar z - (\epsilon_q - \epsilon_q - \mathbf{k}) \right] \Rightarrow \\
[\chi_0^{(5,5)}(\mathbf{k}, z)]_7 &= - \int \frac{d^3 q}{(2\pi)^3} \frac{f_0(\mathbf{q})}{60} \frac{1}{60} \left[ \hbar z - \frac{\epsilon_q + 2\mathbf{k} - \epsilon_q - \mathbf{k}}{3} \right] \left[ \hbar z - \frac{\epsilon_q + 2\mathbf{k} - \epsilon_q - \mathbf{k}}{2} \right]^2 \left[ \hbar z - (\epsilon_q - \epsilon_q - \mathbf{k}) \right]^2 \Rightarrow \\
a &= \frac{\epsilon_q + 2\mathbf{k} - \epsilon_q - \mathbf{k}}{3} = \frac{\hbar^2}{2m} \frac{(q + 2\mathbf{k})^2 - (q - \mathbf{k})^2}{(q - \mathbf{k})^2} = \frac{\hbar^2}{2m} \frac{4q \cdot \mathbf{k} - k^2 + 2q \cdot \mathbf{k}}{k^2} = \frac{\hbar^2}{2m} \frac{3k^2 + 6q \cdot \mathbf{k}}{3} = \frac{\hbar^2}{2m} (k^2 + 2q \cdot \mathbf{k}) \\
b &= \frac{\epsilon_q + \mathbf{k} - \epsilon_q - \mathbf{k}}{2} = \frac{\hbar^2}{2m} \frac{(q + \mathbf{k})^2 - (q - \mathbf{k})^2}{(q - \mathbf{k})^2} = \frac{\hbar^2}{2m} \frac{k^2 + 2q \cdot \mathbf{k} - k^2 + 2q \cdot \mathbf{k}}{k^2} = \frac{\hbar^2}{2m} \frac{4q \cdot \mathbf{k}}{2} = \frac{\hbar^2}{2m} (2q \cdot \mathbf{k}) \\
c &= \epsilon_q - \epsilon_q - \mathbf{k} = \frac{\hbar^2}{2m} [q^2 - (q - \mathbf{k})^2] = \frac{\hbar^2}{2m} (-k^2 + 2q \cdot \mathbf{k}) .
\end{aligned}$$

Then, we compute all the relevant algebraic combinations between these three coefficients. Note that  $q^2$  and  $q \cdot \mathbf{k}$  terms vanish.

$$\begin{aligned}
a - b &= \frac{\hbar^2}{2m} (k^2 + 2q \cdot \mathbf{k} - 2q \cdot \mathbf{k}) = \frac{\hbar^2}{2m} (k^2) , \quad b - c = \frac{\hbar^2}{2m} (2q \cdot \mathbf{k} + k^2 - 2q \cdot \mathbf{k}) = \frac{\hbar^2}{2m} (k^2) , \\
a - c &= \frac{\hbar^2}{2m} (k^2 + 2q \cdot \mathbf{k} + k^2 - 2q \cdot \mathbf{k}) = \frac{\hbar^2}{2m} (k^2 + k^2) = \frac{\hbar^2}{2m} (2k^2) , \quad 2a - 3b + c = \frac{\hbar^2}{2m} (2k^2 + 4q \cdot \mathbf{k} - k^2 + 2q \cdot \mathbf{k}) = \frac{\hbar^2}{2m} (2k^2 - k^2) = \frac{\hbar^2}{2m} (k^2) , \\
2a + b - 3c &= \frac{\hbar^2}{2m} (2k^2 + 4q \cdot \mathbf{k} + 2q \cdot \mathbf{k} + 3k^2 - 6q \cdot \mathbf{k}) = \frac{\hbar^2}{2m} (2k^2 + 3k^2) = \frac{\hbar^2}{2m} (5k^2) .
\end{aligned}$$

Afterwards, we compute all the combinations that are present in the partial fraction decomposition.

$$\begin{aligned}
(a - b)^2 (a - c)^2 &= \left( \frac{\hbar^2}{2m} \right)^2 (k^4) \left( \frac{\hbar^2}{2m} \right)^2 (4k^8) = \left( \frac{\hbar^2}{2m} \right)^4 (4k^8) , \quad (a - b)^2 (b - c)^3 = \left( \frac{\hbar^2}{2m} \right)^2 (k^4) \left( \frac{\hbar^2}{2m} \right)^3 (k^6) = \left( \frac{\hbar^2}{2m} \right)^5 (k^{10}) , \\
(a - c)^2 (b - c)^3 &= \left( \frac{\hbar^2}{2m} \right)^2 (4k^4) \left( \frac{\hbar^2}{2m} \right)^3 (k^6) = \left( \frac{\hbar^2}{2m} \right)^5 (4k^{10}) , \quad (a - b)(b - c)^2 = \frac{\hbar^2}{2m} (k^2) \left( \frac{\hbar^2}{2m} \right)^2 (k^4) = \left( \frac{\hbar^2}{2m} \right)^3 (k^6) , \\
(a - c)(b - c)^2 &= \frac{\hbar^2}{2m} (2k^2) \left( \frac{\hbar^2}{2m} \right)^2 (k^4) = \left( \frac{\hbar^2}{2m} \right)^3 (2k^6) .
\end{aligned}$$

Finally, we substitute and perform some straightforward algebra. We also introduce the compact notation  $\epsilon_{\mathbf{k}} = (\hbar^2 k^2)/(2m)$ .

$$\begin{aligned}
[\chi_0^{(5,5)}(\mathbf{k}, z)]_7 &= - \int \frac{d^3 q}{(2\pi)^3} \left( \frac{2m}{\hbar^2} \right)^4 \frac{1}{4k^8} \frac{f_0(\mathbf{q})}{60} \left[ \frac{1}{\hbar z - \frac{\epsilon_q + 2\mathbf{k} - \epsilon_q - \mathbf{k}}{3}} + \frac{4}{\hbar z - \frac{\epsilon_q + \mathbf{k} - \epsilon_q - \mathbf{k}}{2}} - \frac{5}{\hbar z - \epsilon_q + \epsilon_q - \mathbf{k}} - \frac{\hbar^2}{2m} \frac{4k^2}{\left( \hbar z - \frac{\epsilon_q + \mathbf{k} - \epsilon_q - \mathbf{k}}{2} \right)^2} - \frac{\hbar^2}{2m} \frac{2k^2}{(\hbar z - \epsilon_q + \epsilon_q - \mathbf{k})^2} \right] \Rightarrow \\
[\chi_0^{(5,5)}(\mathbf{k}, z)]_7 &= - \int \frac{d^3 q}{(2\pi)^3} \left( \frac{2m}{\hbar^2} \right)^4 \frac{1}{4k^8} \frac{f_0(\mathbf{q})}{60} \left[ \frac{1}{\hbar z - \frac{\epsilon_q + 2\mathbf{k} - \epsilon_q - \mathbf{k}}{3}} + \frac{4}{\hbar z - \frac{\epsilon_q + \mathbf{k} - \epsilon_q - \mathbf{k}}{2}} - \frac{5}{\hbar z - \epsilon_q + \epsilon_q - \mathbf{k}} - \frac{4\epsilon_{\mathbf{k}}}{\left( \hbar z - \frac{\epsilon_q + \mathbf{k} - \epsilon_q - \mathbf{k}}{2} \right)^2} - \frac{2\epsilon_{\mathbf{k}}}{(\hbar z - \epsilon_q + \epsilon_q - \mathbf{k})^2} \right] \Rightarrow \\
[\chi_0^{(5,5)}(\mathbf{k}, z)]_7 &= - \left( \frac{m}{\hbar^2} \right)^4 \frac{1}{30k^8} \int \frac{d^3 q}{(2\pi)^3} \frac{2f_0(\mathbf{q})}{60} \left[ \frac{1}{\hbar z - \frac{\epsilon_q + 2\mathbf{k} - \epsilon_q - \mathbf{k}}{3}} + \frac{4}{\hbar z - \frac{\epsilon_q + \mathbf{k} - \epsilon_q - \mathbf{k}}{2}} - \frac{5}{\hbar z - \epsilon_q + \epsilon_q - \mathbf{k}} - \frac{4\epsilon_{\mathbf{k}}}{\left( \hbar z - \frac{\epsilon_q + \mathbf{k} - \epsilon_q - \mathbf{k}}{2} \right)^2} - \frac{2\epsilon_{\mathbf{k}}}{(\hbar z - \epsilon_q + \epsilon_q - \mathbf{k})^2} \right] \Rightarrow \\
[\chi_0^{(5,5)}(\mathbf{k}, z)]_7 &= - \left( \frac{m}{\hbar^2} \right)^4 \frac{1}{180k^8} \int \frac{d^3 q}{(2\pi)^3} \frac{2f_0(\mathbf{q})}{60} \left[ \frac{18}{3\hbar z - \epsilon_q + 2\mathbf{k} + \epsilon_q - \mathbf{k}} + \frac{48}{2\hbar z - \epsilon_q + \mathbf{k} + \epsilon_q - \mathbf{k}} - \frac{30}{\hbar z - \epsilon_q + \epsilon_q - \mathbf{k}} - \frac{96\epsilon_{\mathbf{k}}}{(2\hbar z - \epsilon_q + \epsilon_q - \mathbf{k})^2} - \frac{12\epsilon_{\mathbf{k}}}{(\hbar z - \epsilon_q + \epsilon_q - \mathbf{k})^2} \right] .
\end{aligned}$$

The *eighth contribution* is characterized by one simple pole and two double poles. This becomes apparent from the algebraic identities  $(\epsilon_q + 3k - \epsilon_q - 2k)/5 = (\epsilon_q + k - \epsilon_q)$  and  $(\epsilon_q + 3k - \epsilon_q - k)/4 = (\epsilon_q + 2k - \epsilon_q)/2$ . We first identify and calculate the coefficients  $a, b, c$ .

$$\begin{aligned}
\left[ \chi_0^{(5,5)}(\mathbf{k}, z) \right]_8 &= + \int \frac{d^3 q}{(2\pi)^3} \frac{2f_0(\mathbf{q})}{(5\hbar z - \epsilon_q + 3k + \epsilon_q - 2k)(4\hbar z - \epsilon_q + 3k + \epsilon_q - k)(3\hbar z - \epsilon_q + 3k + \epsilon_q)(2\hbar z - \epsilon_q + 2k + \epsilon_q)(\hbar z - \epsilon_q + k + \epsilon_q)} \\
\left[ \chi_0^{(5,5)}(\mathbf{k}, z) \right]_8 &= + \int \frac{d^3 q}{(2\pi)^3} \frac{f_0(\mathbf{q})}{60} \frac{1}{\left[ \hbar z - \frac{\epsilon_q + 3k - \epsilon_q - 2k}{5} \right] \left[ \hbar z - \frac{\epsilon_q + 3k - \epsilon_q - k}{4} \right] \left[ \hbar z - \frac{\epsilon_q + 3k - \epsilon_q}{3} \right] \left[ \hbar z - (\epsilon_q + k - \epsilon_q) \right]} \\
\left[ \chi_0^{(5,5)}(\mathbf{k}, z) \right]_8 &= + \int \frac{d^3 q}{(2\pi)^3} \frac{f_0(\mathbf{q})}{60} \frac{1}{\left[ \hbar z - \frac{\epsilon_q + 3k - \epsilon_q}{3} \right] \left[ \hbar z - \frac{\epsilon_q + 2k - \epsilon_q}{2} \right]^2 \left[ \hbar z - (\epsilon_q + k - \epsilon_q) \right]^2} \\
a &= \frac{\epsilon_q + 3k - \epsilon_q}{3} = \frac{\hbar^2}{2m} \frac{(q + 3k)^2 - q^2}{3} = \frac{\hbar^2}{2m} \frac{9k^2 + 6\mathbf{q} \cdot \mathbf{k}}{3} = \frac{\hbar^2}{2m} (3k^2 + 2\mathbf{q} \cdot \mathbf{k}) \\
b &= \frac{\epsilon_q + 2k - \epsilon_q}{2} = \frac{\hbar^2}{2m} \frac{(q + 2k)^2 - q^2}{2} = \frac{\hbar^2}{2m} \frac{4k^2 + 4\mathbf{q} \cdot \mathbf{k}}{2} = \frac{\hbar^2}{2m} (2k^2 + 2\mathbf{q} \cdot \mathbf{k}) \\
c &= \epsilon_q + k - \epsilon_q = \frac{\hbar^2}{2m} [(q + k)^2 - q^2] = \frac{\hbar^2}{2m} (k^2 + 2\mathbf{q} \cdot \mathbf{k}) .
\end{aligned}$$

Then, we compute all the relevant algebraic combinations between these three coefficients. Note that  $q^2$  and  $\mathbf{q} \cdot \mathbf{k}$  terms vanish.

$$\begin{aligned}
a - b &= \frac{\hbar^2}{2m} (3k^2 + 2\mathbf{q} \cdot \mathbf{k} - 2k^2 - 2\mathbf{q} \cdot \mathbf{k}) = \frac{\hbar^2}{2m} (3k^2 - 2k^2) = \frac{\hbar^2}{2m} (k^2) , \quad b - c = \frac{\hbar^2}{2m} (2k^2 + 2\mathbf{q} \cdot \mathbf{k} - k^2 - 2\mathbf{q} \cdot \mathbf{k}) = \frac{\hbar^2}{2m} (2k^2 - k^2) = \frac{\hbar^2}{2m} (k^2) , \\
a - c &= \frac{\hbar^2}{2m} (3k^2 + 2\mathbf{q} \cdot \mathbf{k} - k^2 - 2\mathbf{q} \cdot \mathbf{k}) = \frac{\hbar^2}{2m} (3k^2 - k^2) = \frac{\hbar^2}{2m} (2k^2) , \quad 2a - 3b + c = \frac{\hbar^2}{2m} (6k^2 + 4\mathbf{q} \cdot \mathbf{k} - 6k^2 - 6\mathbf{q} \cdot \mathbf{k} + k^2 + 2\mathbf{q} \cdot \mathbf{k}) = \frac{\hbar^2}{2m} (6k^2 - 6k^2 + k^2) = \frac{\hbar^2}{2m} (k^2) , \\
2a + b - 3c &= \frac{\hbar^2}{2m} (6k^2 + 4\mathbf{q} \cdot \mathbf{k} + 2k^2 + 2\mathbf{q} \cdot \mathbf{k} - 3k^2 - 6\mathbf{q} \cdot \mathbf{k}) = \frac{\hbar^2}{2m} (6k^2 - 3k^2 + 2k^2) = \frac{\hbar^2}{2m} (5k^2) .
\end{aligned}$$

Afterwards, we compute all the combinations that are present in the partial fraction decomposition.

$$\begin{aligned}
(a - b)^2 (a - c)^2 &= \left( \frac{\hbar^2}{2m} \right)^2 (k^4) \left( \frac{\hbar^2}{2m} \right)^2 (4k^8) = \left( \frac{\hbar^2}{2m} \right)^4 (4k^8) , \quad (a - b)^2 (b - c)^3 = \left( \frac{\hbar^2}{2m} \right)^2 (k^4) \left( \frac{\hbar^2}{2m} \right)^3 (k^{10}) = \left( \frac{\hbar^2}{2m} \right)^5 (k^{10}) , \\
(a - c)^2 (b - c)^3 &= \left( \frac{\hbar^2}{2m} \right)^2 (4k^4) \left( \frac{\hbar^2}{2m} \right)^3 (k^6) = \left( \frac{\hbar^2}{2m} \right)^5 (4k^{10}) , \quad (a - b)(b - c)^2 = \frac{\hbar^2}{2m} (k^2) \left( \frac{\hbar^2}{2m} \right)^2 (k^4) = \left( \frac{\hbar^2}{2m} \right)^3 (k^6) , \\
(a - c)(b - c)^2 &= \frac{\hbar^2}{2m} (2k^2) \left( \frac{\hbar^2}{2m} \right)^2 (k^4) = \left( \frac{\hbar^2}{2m} \right)^3 (2k^6) .
\end{aligned}$$

Finally, we substitute and perform some straightforward algebra. We also introduce the compact notation  $\epsilon_k = (\hbar^2 k^2)/(2m)$ .

$$\begin{aligned}
\left[ \chi_0^{(5,5)}(\mathbf{k}, z) \right]_8 &= + \int \frac{d^3 q}{(2\pi)^3} \frac{(2m)^4}{\left( \frac{\hbar^2}{2m} \right)^3} \frac{1}{4k^8} \frac{1}{60} \left[ \frac{1}{\hbar z - \frac{\epsilon_q + 3k - \epsilon_q}{3}} + \frac{4}{\hbar z - \frac{\epsilon_q + 2k - \epsilon_q}{2}} - \frac{5}{\hbar z - \epsilon_q + k - \epsilon_q} - \frac{\hbar^2}{2m} \frac{4k^2}{\left( \hbar z - \frac{\epsilon_q + 2k - \epsilon_q}{2} \right)^2} - \frac{\hbar^2}{2m} \frac{2k^2}{(\hbar z - \epsilon_q + k + \epsilon_q)^2} \right] \\
\left[ \chi_0^{(5,5)}(\mathbf{k}, z) \right]_8 &= + \int \frac{d^3 q}{(2\pi)^3} \frac{(2m)^4}{\left( \frac{\hbar^2}{2m} \right)^3} \frac{1}{4k^8} \frac{1}{60} \left[ \frac{1}{\hbar z - \frac{\epsilon_q + 3k - \epsilon_q}{3}} + \frac{4}{\hbar z - \frac{\epsilon_q + 2k - \epsilon_q}{2}} - \frac{5}{\hbar z - \epsilon_q + k - \epsilon_q} - \frac{4\epsilon_k}{\left( \hbar z - \frac{\epsilon_q + 2k - \epsilon_q}{2} \right)^2} - \frac{2\epsilon_k}{(\hbar z - \epsilon_q + k + \epsilon_q)^2} \right] \\
\left[ \chi_0^{(5,5)}(\mathbf{k}, z) \right]_8 &= + \left( \frac{m}{\hbar^2} \right)^4 \frac{1}{30k^8} \int \frac{d^3 q}{(2\pi)^3} \frac{2f_0(\mathbf{q})}{60} \left[ \frac{1}{\hbar z - \frac{\epsilon_q + 3k - \epsilon_q}{3}} + \frac{4}{\hbar z - \frac{\epsilon_q + 2k - \epsilon_q}{2}} - \frac{5}{\hbar z - \epsilon_q + k - \epsilon_q} - \frac{4\epsilon_k}{\left( \hbar z - \frac{\epsilon_q + 2k - \epsilon_q}{2} \right)^2} - \frac{2\epsilon_k}{(\hbar z - \epsilon_q + k + \epsilon_q)^2} \right] \\
\left[ \chi_0^{(5,5)}(\mathbf{k}, z) \right]_8 &= + \left( \frac{m}{\hbar^2} \right)^4 \frac{1}{180k^8} \int \frac{d^3 q}{(2\pi)^3} \frac{2f_0(\mathbf{q})}{60} \left[ \frac{18}{3\hbar z - \epsilon_q + 3k + \epsilon_q} + \frac{48}{2\hbar z - \epsilon_q + 2k + \epsilon_q} - \frac{30}{\hbar z - \epsilon_q + k - \epsilon_q} - \frac{96\epsilon_k}{(2\hbar z - \epsilon_q + 2k + \epsilon_q)^2} - \frac{12\epsilon_k}{(\hbar z - \epsilon_q + k + \epsilon_q)^2} \right]
\end{aligned}$$



The *ninth contribution* is characterized by one simple pole and two double poles. This becomes apparent from the algebraic identities  $(\epsilon_{\mathbf{q}+\mathbf{k}} - \epsilon_{\mathbf{q}-4\mathbf{k}})/5 = (\epsilon_{\mathbf{q}} - \epsilon_{\mathbf{q}-3\mathbf{k}})/3$  and  $(\epsilon_{\mathbf{q}+\mathbf{k}} - \epsilon_{\mathbf{q}-3\mathbf{k}})/4 = (\epsilon_{\mathbf{q}} - \epsilon_{\mathbf{q}-2\mathbf{k}})/2$ . We first identify and calculate the coefficients  $a, b, c$ .

$$\begin{aligned}
\left[\chi_0^{(5,5)}(\mathbf{k}, z)\right]_9 &= + \int \frac{d^3 q}{(2\pi)^3} \frac{5\hbar z - \epsilon_{\mathbf{q}+\mathbf{k}} + \epsilon_{\mathbf{q}-4\mathbf{k}}}{60} \frac{2f_0(\mathbf{q})}{(2\pi)^3} \frac{f_0(\mathbf{q})}{60} \frac{(3\hbar z - \epsilon_{\mathbf{q}} + \epsilon_{\mathbf{q}-3\mathbf{k}})(2\hbar z - \epsilon_{\mathbf{q}} + \epsilon_{\mathbf{q}-2\mathbf{k}})(\hbar z - \epsilon_{\mathbf{q}} + \epsilon_{\mathbf{q}-\mathbf{k}})}{(2\pi)^3} \\
\left[\chi_0^{(5,5)}(\mathbf{k}, z)\right]_9 &= + \int \frac{d^3 q}{(2\pi)^3} \frac{f_0(\mathbf{q})}{60} \frac{1}{60} \left[ \hbar z - \frac{\epsilon_{\mathbf{q}+\mathbf{k}} - \epsilon_{\mathbf{q}-4\mathbf{k}}}{5} \right] \left[ \hbar z - \frac{\epsilon_{\mathbf{q}-\epsilon_{\mathbf{q}-3\mathbf{k}}}}{4} \right] \left[ \hbar z - \frac{\epsilon_{\mathbf{q}} - \epsilon_{\mathbf{q}-2\mathbf{k}}}{2} \right] \left[ \hbar z - (\epsilon_{\mathbf{q}} - \epsilon_{\mathbf{q}-\mathbf{k}}) \right] \\
\left[\chi_0^{(5,5)}(\mathbf{k}, z)\right]_9 &= + \int \frac{d^3 q}{(2\pi)^3} \frac{f_0(\mathbf{q})}{60} \frac{1}{60} \left[ \hbar z - (\epsilon_{\mathbf{q}} - \epsilon_{\mathbf{q}-\mathbf{k}}) \right] \left[ \hbar z - \frac{\epsilon_{\mathbf{q}} - \epsilon_{\mathbf{q}-2\mathbf{k}}}{2} \right]^2 \left[ \hbar z - \frac{\epsilon_{\mathbf{q}} - \epsilon_{\mathbf{q}-3\mathbf{k}}}{3} \right]^2 \\
a = \epsilon_{\mathbf{q}} - \epsilon_{\mathbf{q}-\mathbf{k}} &= \frac{\hbar^2}{2m} [q^2 - (\mathbf{q} - \mathbf{k})^2] = \frac{\hbar^2}{2m} (-k^2 + 2\mathbf{q} \cdot \mathbf{k}) \\
b = \frac{\epsilon_{\mathbf{q}} - \epsilon_{\mathbf{q}-2\mathbf{k}}}{2} &= \frac{\hbar^2}{2m} \frac{q^2 - (\mathbf{q} - 2\mathbf{k})^2}{2} = \frac{\hbar^2}{2m} \frac{\hbar^2 - 4k^2 + 4\mathbf{q} \cdot \mathbf{k}}{2} = \frac{\hbar^2}{2m} (-2k^2 + 2\mathbf{q} \cdot \mathbf{k}) \\
c = \frac{\epsilon_{\mathbf{q}} - \epsilon_{\mathbf{q}-3\mathbf{k}}}{3} &= \frac{\hbar^2}{2m} \frac{q^2 - (\mathbf{q} - 3\mathbf{k})^2}{3} = \frac{\hbar^2}{2m} \frac{\hbar^2 - 9k^2 + 6\mathbf{q} \cdot \mathbf{k}}{3} = \frac{\hbar^2}{2m} (-3k^2 + 2\mathbf{q} \cdot \mathbf{k}) .
\end{aligned}$$

Then, we compute all the relevant algebraic combinations between these three coefficients. Note that  $q^2$  and  $\mathbf{q} \cdot \mathbf{k}$  terms vanish.

$$\begin{aligned}
a - b &= \frac{\hbar^2}{2m} (-k^2 + 2\mathbf{q} \cdot \mathbf{k} + 2k^2 - 2\mathbf{q} \cdot \mathbf{k}) = \frac{\hbar^2}{2m} (2k^2 - k^2) = \frac{\hbar^2}{2m} (k^2) , \quad b - c = \frac{\hbar^2}{2m} (-2k^2 + 2\mathbf{q} \cdot \mathbf{k} + 3k^2 - 2\mathbf{q} \cdot \mathbf{k}) = \frac{\hbar^2}{2m} (3k^2 - 2k^2) = \frac{\hbar^2}{2m} (k^2) , \\
a - c &= \frac{\hbar^2}{2m} (-k^2 + 2\mathbf{q} \cdot \mathbf{k} + 3k^2 - 2\mathbf{q} \cdot \mathbf{k}) = \frac{\hbar^2}{2m} (3k^2 - k^2) = \frac{\hbar^2}{2m} (2k^2) , \quad 2a - 3b + c = \frac{\hbar^2}{2m} (-2k^2 + 4\mathbf{q} \cdot \mathbf{k} + 6k^2 - 6\mathbf{q} \cdot \mathbf{k} + 3k^2 + 2\mathbf{q} \cdot \mathbf{k}) = \frac{\hbar^2}{2m} (6k^2 - 3k^2 - 2k^2) = \frac{\hbar^2}{2m} (k^2) , \\
2a + b - 3c &= \frac{\hbar^2}{2m} (-2k^2 + 4\mathbf{q} \cdot \mathbf{k} - 2k^2 + 2\mathbf{q} \cdot \mathbf{k} + 9k^2 - 6\mathbf{q} \cdot \mathbf{k}) = \frac{\hbar^2}{2m} (9k^2 - 2k^2 - 2k^2) = \frac{\hbar^2}{2m} (5k^2) .
\end{aligned}$$

Afterwards, we compute all the combinations that are present in the partial fraction decomposition.

$$\begin{aligned}
(a-b)^2(a-c)^2 &= \left(\frac{\hbar^2}{2m}\right)^2 (k^4) \left(\frac{\hbar^2}{2m}\right)^2 (4k^8) = \left(\frac{\hbar^2}{2m}\right)^4 (4k^8) , \quad (a-b)^2(b-c)^3 = \left(\frac{\hbar^2}{2m}\right)^2 (k^4) \left(\frac{\hbar^2}{2m}\right)^3 (k^6) = \left(\frac{\hbar^2}{2m}\right)^5 (k^{10}) , \\
(a-c)^2(b-c)^3 &= \left(\frac{\hbar^2}{2m}\right)^2 (4k^4) \left(\frac{\hbar^2}{2m}\right)^3 (k^6) = \left(\frac{\hbar^2}{2m}\right)^5 (4k^{10}) , \quad (a-b)(b-c)^2 = \frac{\hbar^2}{2m} (k^2) \left(\frac{\hbar^2}{2m}\right)^2 (k^4) = \left(\frac{\hbar^2}{2m}\right)^3 (k^6) , \\
(a-c)(b-c)^2 &= \frac{\hbar^2}{2m} (2k^2) \left(\frac{\hbar^2}{2m}\right)^2 (k^4) = \left(\frac{\hbar^2}{2m}\right)^3 (2k^6) .
\end{aligned}$$

Finally, we substitute and perform some straightforward algebra. We also introduce the compact notation  $\epsilon_{\mathbf{k}} = (\hbar^2 k^2)/(2m)$ .

$$\begin{aligned}
\left[\chi_0^{(5,5)}(\mathbf{k}, z)\right]_9 &= + \int \frac{d^3 q}{(2\pi)^3} \left(\frac{2m}{\hbar^2}\right)^4 \frac{1}{4k^8} \frac{f_0(\mathbf{q})}{60} \left[ \frac{1}{\hbar z - \epsilon_{\mathbf{q}} + \epsilon_{\mathbf{q}-\mathbf{k}}} + \frac{4}{\hbar z - \frac{\epsilon_{\mathbf{q}} - \epsilon_{\mathbf{q}-2\mathbf{k}}}{2}} - \frac{4}{\hbar z - \frac{\epsilon_{\mathbf{q}} - \epsilon_{\mathbf{q}-3\mathbf{k}}}{3}} - \frac{\hbar^2}{2m} \frac{4k^2}{\left(\hbar z - \frac{\epsilon_{\mathbf{q}} - \epsilon_{\mathbf{q}-2\mathbf{k}}}{2}\right)^2} - \frac{\hbar^2}{2m} \frac{2k^2}{\left(\hbar z - \frac{\epsilon_{\mathbf{q}} - \epsilon_{\mathbf{q}-3\mathbf{k}}}{3}\right)^2} \right] \\
\left[\chi_0^{(5,5)}(\mathbf{k}, z)\right]_9 &= + \int \frac{d^3 q}{(2\pi)^3} \left(\frac{2m}{\hbar^2}\right)^4 \frac{1}{4k^8} \frac{f_0(\mathbf{q})}{60} \left[ \frac{1}{\hbar z - \epsilon_{\mathbf{q}} + \epsilon_{\mathbf{q}-\mathbf{k}}} + \frac{4}{\hbar z - \frac{\epsilon_{\mathbf{q}} - \epsilon_{\mathbf{q}-2\mathbf{k}}}{2}} - \frac{5}{\hbar z - \frac{\epsilon_{\mathbf{q}} - \epsilon_{\mathbf{q}-3\mathbf{k}}}{3}} - \frac{4\epsilon_{\mathbf{k}}}{\left(\hbar z - \frac{\epsilon_{\mathbf{q}} - \epsilon_{\mathbf{q}-2\mathbf{k}}}{2}\right)^2} - \frac{2\epsilon_{\mathbf{k}}}{\left(\hbar z - \frac{\epsilon_{\mathbf{q}} - \epsilon_{\mathbf{q}-3\mathbf{k}}}{3}\right)^2} \right] \\
\left[\chi_0^{(5,5)}(\mathbf{k}, z)\right]_9 &= + \left(\frac{m}{\hbar^2}\right)^4 \frac{1}{30k^8} \int \frac{d^3 q}{(2\pi)^3} 2f_0(\mathbf{q}) \left[ \frac{1}{\hbar z - \epsilon_{\mathbf{q}} + \epsilon_{\mathbf{q}-\mathbf{k}}} + \frac{4}{\hbar z - \frac{\epsilon_{\mathbf{q}} - \epsilon_{\mathbf{q}-2\mathbf{k}}}{2}} - \frac{5}{\hbar z - \frac{\epsilon_{\mathbf{q}} - \epsilon_{\mathbf{q}-3\mathbf{k}}}{3}} - \frac{4\epsilon_{\mathbf{k}}}{\left(\hbar z - \frac{\epsilon_{\mathbf{q}} - \epsilon_{\mathbf{q}-2\mathbf{k}}}{2}\right)^2} - \frac{2\epsilon_{\mathbf{k}}}{\left(\hbar z - \frac{\epsilon_{\mathbf{q}} - \epsilon_{\mathbf{q}-3\mathbf{k}}}{3}\right)^2} \right] \\
\left[\chi_0^{(5,5)}(\mathbf{k}, z)\right]_9 &= + \left(\frac{m}{\hbar^2}\right)^4 \frac{1}{180k^8} \int \frac{d^3 q}{(2\pi)^3} 2f_0(\mathbf{q}) \left[ \frac{6}{\hbar z - \epsilon_{\mathbf{q}} + \epsilon_{\mathbf{q}-\mathbf{k}}} + \frac{48}{2\hbar z - \epsilon_{\mathbf{q}} + \epsilon_{\mathbf{q}-2\mathbf{k}}} - \frac{90}{3\hbar z - \epsilon_{\mathbf{q}} + \epsilon_{\mathbf{q}-3\mathbf{k}}} - \frac{96\epsilon_{\mathbf{k}}}{(2\hbar z - \epsilon_{\mathbf{q}} + \epsilon_{\mathbf{q}-2\mathbf{k}})^2} - \frac{108\epsilon_{\mathbf{k}}}{(3\hbar z - \epsilon_{\mathbf{q}} + \epsilon_{\mathbf{q}-3\mathbf{k}})^2} \right] .
\end{aligned}$$

$$\begin{aligned}
\left[\chi_0^{(5,5)}(\mathbf{k}, z)\right]_{10} &= - \int \frac{d^3 q}{(2\pi)^3} \left(\frac{2m}{\hbar^2}\right)^4 \frac{1}{4k^8} \frac{f_0(\mathbf{q})}{60} \Rightarrow \left[ \frac{1}{\hbar z - \epsilon_{\mathbf{q}+\mathbf{k}} + \epsilon_{\mathbf{q}}} + \frac{4}{\hbar z - \frac{\epsilon_{\mathbf{q}+\mathbf{k}} - \epsilon_{\mathbf{q}-\mathbf{k}}}{2}} - \frac{5}{\hbar z - \frac{\epsilon_{\mathbf{q}+\mathbf{k}} - \epsilon_{\mathbf{q}-2\mathbf{k}}}{3}} - \frac{h^2}{2m \left(\hbar z - \frac{\epsilon_{\mathbf{q}+\mathbf{k}} - \epsilon_{\mathbf{q}-\mathbf{k}}}{2}\right)^2} - \frac{h^2}{2m \left(\hbar z - \frac{\epsilon_{\mathbf{q}+\mathbf{k}} - \epsilon_{\mathbf{q}-2\mathbf{k}}}{3}\right)^2} \right] \Rightarrow \\
\left[\chi_0^{(5,5)}(\mathbf{k}, z)\right]_{10} &= - \int \frac{d^3 q}{(2\pi)^3} \left(\frac{2m}{\hbar^2}\right)^4 \frac{1}{4k^8} \frac{f_0(\mathbf{q})}{60} \Rightarrow \left[ \frac{1}{\hbar z - \epsilon_{\mathbf{q}+\mathbf{k}} + \epsilon_{\mathbf{q}}} + \frac{4}{\hbar z - \frac{\epsilon_{\mathbf{q}+\mathbf{k}} - \epsilon_{\mathbf{q}-\mathbf{k}}}{2}} - \frac{5}{\hbar z - \frac{\epsilon_{\mathbf{q}+\mathbf{k}} - \epsilon_{\mathbf{q}-2\mathbf{k}}}{3}} - \frac{4\epsilon_{\mathbf{k}}}{\left(\hbar z - \frac{\epsilon_{\mathbf{q}+\mathbf{k}} - \epsilon_{\mathbf{q}-\mathbf{k}}}{2}\right)^2} - \frac{2\epsilon_{\mathbf{k}}}{\left(\hbar z - \frac{\epsilon_{\mathbf{q}+\mathbf{k}} - \epsilon_{\mathbf{q}-2\mathbf{k}}}{3}\right)^2} \right] \Rightarrow \\
\left[\chi_0^{(5,5)}(\mathbf{k}, z)\right]_{10} &= - \left(\frac{m}{\hbar^2}\right)^4 \frac{1}{30k^8} \frac{1}{(2\pi)^3} \int \frac{d^3 q}{(2\pi)^3} \frac{2f_0(\mathbf{q})}{60} \Rightarrow \left[ \frac{1}{\hbar z - \epsilon_{\mathbf{q}+\mathbf{k}} + \epsilon_{\mathbf{q}}} + \frac{4}{\hbar z - \frac{\epsilon_{\mathbf{q}+\mathbf{k}} - \epsilon_{\mathbf{q}-\mathbf{k}}}{2}} - \frac{5}{\hbar z - \frac{\epsilon_{\mathbf{q}+\mathbf{k}} - \epsilon_{\mathbf{q}-2\mathbf{k}}}{3}} - \frac{4\epsilon_{\mathbf{k}}}{\left(\hbar z - \frac{\epsilon_{\mathbf{q}+\mathbf{k}} - \epsilon_{\mathbf{q}-\mathbf{k}}}{2}\right)^2} - \frac{2\epsilon_{\mathbf{k}}}{\left(\hbar z - \frac{\epsilon_{\mathbf{q}+\mathbf{k}} - \epsilon_{\mathbf{q}-2\mathbf{k}}}{3}\right)^2} \right] \Rightarrow \\
\left[\chi_0^{(5,5)}(\mathbf{k}, z)\right]_{10} &= - \left(\frac{m}{\hbar^2}\right)^4 \frac{1}{180k^8} \frac{1}{(2\pi)^3} \int \frac{d^3 q}{(2\pi)^3} \frac{2f_0(\mathbf{q})}{60} \Rightarrow \left[ \frac{6}{\hbar z - \epsilon_{\mathbf{q}+\mathbf{k}} + \epsilon_{\mathbf{q}}} + \frac{48}{2\hbar z - \epsilon_{\mathbf{q}+\mathbf{k}} + \epsilon_{\mathbf{q}-\mathbf{k}}} - \frac{90}{3\hbar z - \epsilon_{\mathbf{q}+\mathbf{k}} + \epsilon_{\mathbf{q}-2\mathbf{k}}} - \frac{96\epsilon_{\mathbf{k}}}{(2\hbar z - \epsilon_{\mathbf{q}+\mathbf{k}} + \epsilon_{\mathbf{q}-\mathbf{k}})^2} - \frac{108\epsilon_{\mathbf{k}}}{(3\hbar z - \epsilon_{\mathbf{q}+\mathbf{k}} + \epsilon_{\mathbf{q}-2\mathbf{k}})^2} \right] \Rightarrow
\end{aligned}$$

The *eleventh contribution* is characterized by one double pole and one triple pole. This becomes apparent from the algebraic identities  $(\epsilon_{q+2k} - \epsilon_{q-2k})/4 = (\epsilon_{q+k} - \epsilon_{q-k})/2$  and  $(\epsilon_{q+2k} - \epsilon_{q-2k})/5 = (\epsilon_{q+k} - \epsilon_{q-k})/3 = (\epsilon_q - \epsilon_{q-k})$ . We first identify and calculate the coefficients  $a, b$ .

$$\begin{aligned}
[\chi_0^{(5,5)}(\mathbf{k}, z)]_{11} &= - \int \frac{d^3 q}{(2\pi)^3} \frac{2f_0(\mathbf{q})}{(5\hbar z - \epsilon_{q+2k} + \epsilon_{q-3k})(4\hbar z - \epsilon_{q+2k} + \epsilon_{q-2k})(3\hbar z - \epsilon_{q+k} + \epsilon_{q-k})(2\hbar z - \epsilon_q + \epsilon_{q-k})} \Rightarrow \\
[\chi_0^{(5,5)}(\mathbf{k}, z)]_{11} &= - \int \frac{d^3 q}{(2\pi)^3} \frac{f_0(\mathbf{q})}{60} \frac{1}{\left[\hbar z - \frac{\epsilon_{q+2k} - \epsilon_{q-3k}}{5}\right] \left[\hbar z - \frac{\epsilon_{q+2k} - \epsilon_{q-2k}}{4}\right] \left[\hbar z - \frac{\epsilon_{q+k} - \epsilon_{q-k}}{3}\right] \left[\hbar z - (\epsilon_q - \epsilon_{q-k})\right]} \Rightarrow \\
[\chi_0^{(5,5)}(\mathbf{k}, z)]_{11} &= - \int \frac{d^3 q}{(2\pi)^3} \frac{f_0(\mathbf{q})}{60} \frac{1}{\left[\hbar z - (\epsilon_q - \epsilon_{q-k})\right] \left[\hbar z - \frac{\epsilon_{q+k} - \epsilon_{q-k}}{2}\right] \left[\hbar z - (\epsilon_q - \epsilon_{q-k})\right] \left[\hbar z - (\epsilon_q - \epsilon_{q-k})\right]} \Rightarrow \\
[\chi_0^{(5,5)}(\mathbf{k}, z)]_{11} &= - \int \frac{d^3 q}{(2\pi)^3} \frac{f_0(\mathbf{q})}{60} \frac{1}{\left[\hbar z - \frac{\epsilon_{q+k} - \epsilon_{q-k}}{2}\right]^2 \left[\hbar z - (\epsilon_q - \epsilon_{q-k})\right]^3} \Rightarrow \\
a = \frac{\epsilon_{q+k} - \epsilon_{q-k}}{2} &= \frac{\hbar^2}{2m} \frac{(q+k)^2 - (q-k)^2}{2} = \frac{\hbar^2}{2m} \frac{k^2 + 2\mathbf{q} \cdot \mathbf{k} - k^2 + 2\mathbf{q} \cdot \mathbf{k}}{2} = \frac{\hbar^2}{2m} \frac{4\mathbf{q} \cdot \mathbf{k}}{2} = \frac{\hbar^2}{2m} (2\mathbf{q} \cdot \mathbf{k}) \\
b = (\epsilon_q - \epsilon_{q-k}) &= \frac{\hbar^2}{2m} [q^2 - (q-k)^2] = \frac{\hbar^2}{2m} (-k^2 + 2\mathbf{q} \cdot \mathbf{k}).
\end{aligned}$$

Then, we compute all the relevant algebraic combinations between the coefficients. Note that  $q^2$  and  $\mathbf{q} \cdot \mathbf{k}$  terms vanish.

$$\begin{aligned}
a - b &= \frac{\hbar^2}{2m} (2\mathbf{q} \cdot \mathbf{k} + k^2 - 2\mathbf{q} \cdot \mathbf{k}) = \frac{\hbar^2}{2m} (k^2), \\
(a - b)^3 &= \left(\frac{\hbar^2}{2m}\right)^3 (k^6), \\
(a - b)^4 &= \left(\frac{\hbar^2}{2m}\right)^4 (k^8), \\
(a - b)^2 &= \left(\frac{\hbar^2}{2m}\right)^2 (k^4).
\end{aligned}$$

Finally, we substitute and perform some straightforward algebra. We also introduce the compact notation  $\epsilon_k = (\hbar^2 k^2)/(2m)$ .

$$\begin{aligned}
[\chi_0^{(5,5)}(\mathbf{k}, z)]_{11} &= - \int \frac{d^3 q}{(2\pi)^3} \frac{(2m)^4}{\hbar^2} \frac{1}{k^8} \frac{f_0(\mathbf{q})}{60} \left[ - \frac{3}{\hbar z - \frac{\epsilon_{q+k} - \epsilon_{q-k}}{2}} + \frac{3}{\hbar z - \epsilon_q + \epsilon_{q-k}} + \frac{\hbar^2}{2m} \frac{k^2}{\left(\hbar z - \frac{\epsilon_{q+k} - \epsilon_{q-k}}{2}\right)^2} + \frac{\hbar^2}{2m} \frac{2k^2}{(\hbar z - \epsilon_q + \epsilon_{q-k})^2} + \left(\frac{\hbar^2}{2m}\right)^2 \frac{k^4}{(\hbar z - \epsilon_q + \epsilon_{q-k})^3} \right] \Rightarrow \\
[\chi_0^{(5,5)}(\mathbf{k}, z)]_{11} &= - \int \frac{d^3 q}{(2\pi)^3} \frac{(2m)^4}{\hbar^2} \frac{1}{k^8} \frac{f_0(\mathbf{q})}{60} \left[ - \frac{3}{\hbar z - \frac{\epsilon_{q+k} - \epsilon_{q-k}}{2}} + \frac{3}{\hbar z - \epsilon_q + \epsilon_{q-k}} + \frac{\epsilon_k}{\left(\hbar z - \frac{\epsilon_{q+k} - \epsilon_{q-k}}{2}\right)^2} + \frac{2\epsilon_k}{(\hbar z - \epsilon_q + \epsilon_{q-k})^2} + \frac{\epsilon_k^2}{(\hbar z - \epsilon_q + \epsilon_{q-k})^3} \right] \Rightarrow \\
[\chi_0^{(5,5)}(\mathbf{k}, z)]_{11} &= - \int \frac{d^3 q}{(2\pi)^3} \frac{(m)^4}{\hbar^2} \frac{16}{4k^8} \frac{f_0(\mathbf{q})}{60} \left[ - \frac{12}{\hbar z - \frac{\epsilon_{q+k} - \epsilon_{q-k}}{2}} + \frac{12}{\hbar z - \epsilon_q + \epsilon_{q-k}} + \frac{4\epsilon_k}{\left(\hbar z - \frac{\epsilon_{q+k} - \epsilon_{q-k}}{2}\right)^2} + \frac{8\epsilon_k}{(\hbar z - \epsilon_q + \epsilon_{q-k})^2} + \frac{4\epsilon_k^2}{(\hbar z - \epsilon_q + \epsilon_{q-k})^3} \right] \Rightarrow \\
[\chi_0^{(5,5)}(\mathbf{k}, z)]_{11} &= - \int \frac{d^3 q}{(2\pi)^3} \frac{(m)^4}{\hbar^2} \frac{2f_0(\mathbf{q})}{30} \left[ - \frac{12}{\hbar z - \frac{\epsilon_{q+k} - \epsilon_{q-k}}{2}} + \frac{12}{\hbar z - \epsilon_q + \epsilon_{q-k}} + \frac{4\epsilon_k}{\left(\hbar z - \frac{\epsilon_{q+k} - \epsilon_{q-k}}{2}\right)^2} + \frac{8\epsilon_k}{(\hbar z - \epsilon_q + \epsilon_{q-k})^2} + \frac{4\epsilon_k^2}{(\hbar z - \epsilon_q + \epsilon_{q-k})^3} \right] \Rightarrow \\
[\chi_0^{(5,5)}(\mathbf{k}, z)]_{11} &= - \left(\frac{m}{\hbar^2}\right)^4 \frac{1}{30k^8} \int \frac{d^3 q}{(2\pi)^3} \frac{2f_0(\mathbf{q})}{60} \left[ - \frac{12}{\hbar z - \frac{\epsilon_{q+k} - \epsilon_{q-k}}{2}} + \frac{12}{\hbar z - \epsilon_q + \epsilon_{q-k}} + \frac{4\epsilon_k}{\left(\hbar z - \frac{\epsilon_{q+k} - \epsilon_{q-k}}{2}\right)^2} + \frac{8\epsilon_k}{(\hbar z - \epsilon_q + \epsilon_{q-k})^2} + \frac{4\epsilon_k^2}{(\hbar z - \epsilon_q + \epsilon_{q-k})^3} \right] \Rightarrow \\
[\chi_0^{(5,5)}(\mathbf{k}, z)]_{11} &= - \left(\frac{m}{\hbar^2}\right)^4 \frac{1}{180k^8} \int \frac{d^3 q}{(2\pi)^3} \frac{2f_0(\mathbf{q})}{60} \left[ - \frac{144}{2\hbar z - \epsilon_{q+k} + \epsilon_{q-k}} + \frac{72}{\hbar z - \epsilon_q + \epsilon_{q-k}} + \frac{96\epsilon_k}{(2\hbar z - \epsilon_{q+k} + \epsilon_{q-k})^2} + \frac{48\epsilon_k}{(\hbar z - \epsilon_q + \epsilon_{q-k})^2} + \frac{24\epsilon_k^2}{(\hbar z - \epsilon_q + \epsilon_{q-k})^3} \right].
\end{aligned}$$

The *twelfth contribution* is characterized by one double pole and one triple pole. This becomes apparent from the algebraic identities  $(\epsilon_q + 3k - \epsilon_q - k)/4 = (\epsilon_q + 2k - \epsilon_q)/2$  and  $(\epsilon_q + 3k - \epsilon_q - 2k)/5 = (\epsilon_q + 2k - \epsilon_q - k)/3 = (\epsilon_q + k - \epsilon_q)$ . We first identify and calculate the coefficients  $a, b$ .

$$\begin{aligned}
\left[ \chi_0^{(5,5)}(\mathbf{k}, z) \right]_{12} &= + \int \frac{d^3 q}{(2\pi)^3} \frac{2f_0(\mathbf{q})}{(5\hbar z - \epsilon_q + 3k + \epsilon_q - 2k)(4\hbar z - \epsilon_q + 3k + \epsilon_q - k)(3\hbar z - \epsilon_q + 2k + \epsilon_q)(\hbar z - \epsilon_q + k + \epsilon_q)} \Rightarrow \\
\left[ \chi_0^{(5,5)}(\mathbf{k}, z) \right]_{12} &= + \int \frac{d^3 q}{(2\pi)^3} \frac{f_0(\mathbf{q})}{60} \frac{1}{\left[ \hbar z - \frac{\epsilon_q + 3k - \epsilon_q - k}{4} \right] \left[ \hbar z - \frac{\epsilon_q + 2k - \epsilon_q - k}{3} \right] \left[ \hbar z - (\epsilon_q + k - \epsilon_q) \right]} \Rightarrow \\
\left[ \chi_0^{(5,5)}(\mathbf{k}, z) \right]_{12} &= + \int \frac{d^3 q}{(2\pi)^3} \frac{f_0(\mathbf{q})}{60} \frac{1}{\left[ \hbar z - (\epsilon_q + k - \epsilon_q) \right] \left[ \hbar z - \frac{\epsilon_q + 2k - \epsilon_q}{2} \right] \left[ \hbar z - (\epsilon_q + k - \epsilon_q) \right]} \Rightarrow \\
\left[ \chi_0^{(5,5)}(\mathbf{k}, z) \right]_{12} &= + \int \frac{d^3 q}{(2\pi)^3} \frac{f_0(\mathbf{q})}{60} \frac{1}{\left[ \hbar z - \frac{\epsilon_q + 2k - \epsilon_q}{2} \right]^2 \left[ \hbar z - (\epsilon_q + k - \epsilon_q) \right]^3} \Rightarrow \\
a = \frac{\epsilon_q + 2k - \epsilon_q}{2} &= \frac{\hbar^2}{2m} \frac{(q + 2k)^2 - q^2}{4k^2 + 4q \cdot k} = \frac{\hbar^2}{2m} (2k^2 + 2q \cdot k) \\
b = (\epsilon_q + k - \epsilon_q) &= \frac{\hbar^2}{2m} [(q + k)^2 - q^2] = \frac{\hbar^2}{2m} (k^2 + 2q \cdot k).
\end{aligned}$$

Then, we compute all the relevant algebraic combinations between the coefficients. Note that  $q^2$  and  $q \cdot k$  terms vanish.

$$\begin{aligned}
a - b &= \frac{\hbar^2}{2m} (2k^2 + 2q \cdot k - k^2 - 2q \cdot k) = \frac{\hbar^2}{2m} (2k^2 - k^2) = \frac{\hbar^2}{2m} (k^2), \\
(a - b)^3 &= \left( \frac{\hbar^2}{2m} \right)^3 (k^6), \\
(a - b)^2 &= \left( \frac{\hbar^2}{2m} \right)^2 (k^4), \\
(a - b)^4 &= \left( \frac{\hbar^2}{2m} \right)^4 (k^8).
\end{aligned}$$

Finally, we substitute and perform some straightforward algebra. We also introduce the compact notation  $\epsilon_k = (\hbar^2 k^2)/(2m)$ .

$$\begin{aligned}
\left[ \chi_0^{(5,5)}(\mathbf{k}, z) \right]_{12} &= + \int \frac{d^3 q}{(2\pi)^3} \frac{\left( \frac{2m}{\hbar^2} \right)^4}{k^8} \frac{1}{60} \frac{f_0(\mathbf{q})}{\hbar z - \frac{\epsilon_q + 2k - \epsilon_q}{2}} + \frac{3}{\hbar z - \epsilon_q + k + \epsilon_q} + \frac{\hbar^2}{2m} \frac{k^2}{\left( \hbar z - \frac{\epsilon_q + 2k - \epsilon_q}{2} \right)^2} + \frac{\hbar^2}{2m} \frac{2k^2}{(\hbar z - \epsilon_q + k + \epsilon_q)^2} + \left( \frac{\hbar^2}{2m} \right)^2 \frac{k^4}{(\hbar z - \epsilon_q + k + \epsilon_q)^3} \Rightarrow \\
\left[ \chi_0^{(5,5)}(\mathbf{k}, z) \right]_{12} &= + \int \frac{d^3 q}{(2\pi)^3} \frac{\left( \frac{2m}{\hbar^2} \right)^4}{k^8} \frac{1}{60} \frac{f_0(\mathbf{q})}{\hbar z - \frac{\epsilon_q + 2k - \epsilon_q}{2}} + \frac{3}{\hbar z - \epsilon_q + k + \epsilon_q} + \frac{\epsilon_k}{\left( \hbar z - \frac{\epsilon_q + 2k - \epsilon_q}{2} \right)^2} + \frac{2\epsilon_k}{(\hbar z - \epsilon_q + k + \epsilon_q)^2} + \frac{\epsilon_k^2}{(\hbar z - \epsilon_q + k + \epsilon_q)^3} \Rightarrow \\
\left[ \chi_0^{(5,5)}(\mathbf{k}, z) \right]_{12} &= + \int \frac{d^3 q}{(2\pi)^3} \frac{\left( \frac{m}{\hbar^2} \right)^4}{4k^8} \frac{16}{60} \frac{f_0(\mathbf{q})}{\hbar z - \frac{\epsilon_q + 2k - \epsilon_q}{2}} + \frac{12}{\hbar z - \epsilon_q + k + \epsilon_q} + \frac{4\epsilon_k}{\left( \hbar z - \frac{\epsilon_q + 2k - \epsilon_q}{2} \right)^2} + \frac{8\epsilon_k}{(\hbar z - \epsilon_q + k + \epsilon_q)^2} + \frac{4\epsilon_k^2}{(\hbar z - \epsilon_q + k + \epsilon_q)^3} \Rightarrow \\
\left[ \chi_0^{(5,5)}(\mathbf{k}, z) \right]_{12} &= + \int \frac{d^3 q}{(2\pi)^3} \frac{\left( \frac{m}{\hbar^2} \right)^4}{k^8} \frac{1}{30} \frac{2f_0(\mathbf{q})}{\hbar z - \frac{\epsilon_q + 2k - \epsilon_q}{2}} + \frac{12}{\hbar z - \epsilon_q + k + \epsilon_q} + \frac{4\epsilon_k}{\left( \hbar z - \frac{\epsilon_q + 2k - \epsilon_q}{2} \right)^2} + \frac{8\epsilon_k}{(\hbar z - \epsilon_q + k + \epsilon_q)^2} + \frac{4\epsilon_k^2}{(\hbar z - \epsilon_q + k + \epsilon_q)^3} \Rightarrow \\
\left[ \chi_0^{(5,5)}(\mathbf{k}, z) \right]_{12} &= + \left( \frac{m}{\hbar^2} \right)^4 \frac{1}{30k^8} \int \frac{d^3 q}{(2\pi)^3} \frac{2f_0(\mathbf{q})}{\hbar z - \frac{\epsilon_q + 2k - \epsilon_q}{2}} + \frac{12}{\hbar z - \epsilon_q + k + \epsilon_q} + \frac{4\epsilon_k}{\left( \hbar z - \frac{\epsilon_q + 2k - \epsilon_q}{2} \right)^2} + \frac{8\epsilon_k}{(\hbar z - \epsilon_q + k + \epsilon_q)^2} + \frac{4\epsilon_k^2}{(\hbar z - \epsilon_q + k + \epsilon_q)^3} \Rightarrow \\
\left[ \chi_0^{(5,5)}(\mathbf{k}, z) \right]_{12} &= + \left( \frac{m}{\hbar^2} \right)^4 \frac{1}{180k^8} \int \frac{d^3 q}{(2\pi)^3} \frac{2f_0(\mathbf{q})}{\hbar z - \epsilon_q + 2k + \epsilon_q} + \frac{144}{2\hbar z - \epsilon_q + 2k + \epsilon_q} + \frac{72}{\hbar z - \epsilon_q + k + \epsilon_q} + \frac{96\epsilon_k}{(2\hbar z - \epsilon_q + 2k + \epsilon_q)^2} + \frac{48\epsilon_k}{(\hbar z - \epsilon_q + k + \epsilon_q)^2} + \frac{24\epsilon_k^2}{(\hbar z - \epsilon_q + k + \epsilon_q)^3}.
\end{aligned}$$

The *thirteenth contribution* is characterized by two simple poles and one triple pole. This becomes apparent from the algebraic identity  $(\epsilon_q + 2\mathbf{k} - \epsilon_{q-3\mathbf{k}})/5 = (\epsilon_q + \mathbf{k} - \epsilon_{q-2\mathbf{k}})/3 = (\epsilon_q - \epsilon_{q-\mathbf{k}})$ . We first identify and calculate the coefficients  $a, b, c$ .

$$\begin{aligned}
[\chi_0^{(5,5)}(\mathbf{k}, z)]_{13} &= - \int \frac{d^3 q}{(2\pi)^3} \frac{(5\hbar z - \epsilon_{q+2\mathbf{k}} + \epsilon_{q-3\mathbf{k}})(4\hbar z - \epsilon_{q+2\mathbf{k}} + \epsilon_{q-2\mathbf{k}})(3\hbar z - \epsilon_{q+\mathbf{k}} + \epsilon_{q-2\mathbf{k}})(2\hbar z - \epsilon_q + \epsilon_{q-2\mathbf{k}})(\hbar z - \epsilon_q + \epsilon_{q-\mathbf{k}})}{2f_0(\mathbf{q})} \Rightarrow \\
[\chi_0^{(5,5)}(\mathbf{k}, z)]_{13} &= - \int \frac{d^3 q}{(2\pi)^3} \frac{f_0(\mathbf{q})}{60} \frac{1}{\left[\hbar z - \frac{\epsilon_q - \epsilon_{q-2\mathbf{k}}}{2}\right] \left[\hbar z - \frac{\epsilon_q + \mathbf{k} - \epsilon_{q-2\mathbf{k}}}{3}\right] \left[\hbar z - (\epsilon_q - \epsilon_{q-\mathbf{k}})\right]} \Rightarrow \\
[\chi_0^{(5,5)}(\mathbf{k}, z)]_{13} &= - \int \frac{d^3 q}{(2\pi)^3} \frac{f_0(\mathbf{q})}{60} \frac{1}{\left[\hbar z - \frac{\epsilon_q - \epsilon_{q-\mathbf{k}}}{2}\right] \left[\hbar z - \frac{\epsilon_q + 2\mathbf{k} - \epsilon_{q-2\mathbf{k}}}{4}\right] \left[\hbar z - (\epsilon_q - \epsilon_{q-\mathbf{k}})\right]} \Rightarrow \\
[\chi_0^{(5,5)}(\mathbf{k}, z)]_{13} &= - \int \frac{d^3 q}{(2\pi)^3} \frac{f_0(\mathbf{q})}{60} \frac{1}{\left[\hbar z - \frac{\epsilon_q - \epsilon_{q-2\mathbf{k}}}{2}\right] \left[\hbar z - \frac{\epsilon_q + 2\mathbf{k} - \epsilon_{q-2\mathbf{k}}}{4}\right] \left[\hbar z - (\epsilon_q - \epsilon_{q-\mathbf{k}})\right]^3} \Rightarrow \\
a &= \frac{\epsilon_q - \epsilon_{q-2\mathbf{k}}}{2} = \frac{\hbar^2}{2m} \frac{q^2 - (q-2\mathbf{k})^2}{2} = \frac{\hbar^2}{2m} \frac{-4k^2 + 4\mathbf{q} \cdot \mathbf{k}}{2} = \frac{\hbar^2}{2m} (-2k^2 + 2\mathbf{q} \cdot \mathbf{k}) \\
b &= \frac{\epsilon_{q+2\mathbf{k}} - \epsilon_{q-2\mathbf{k}}}{4} = \frac{\hbar^2}{2m} \frac{(q+2\mathbf{k})^2 - (q-2\mathbf{k})^2}{4} = \frac{\hbar^2}{2m} \frac{4k^2 + 4\mathbf{q} \cdot \mathbf{k}}{4} = \frac{\hbar^2}{2m} \frac{8\mathbf{q} \cdot \mathbf{k}}{4} = \frac{\hbar^2}{2m} (2\mathbf{q} \cdot \mathbf{k}) \\
c &= (\epsilon_q - \epsilon_{q-\mathbf{k}}) = \frac{\hbar^2}{2m} [q^2 - (\mathbf{q} - \mathbf{k})^2] = \frac{\hbar^2}{2m} (-k^2 + 2\mathbf{q} \cdot \mathbf{k}).
\end{aligned}$$

Then, we compute all the relevant algebraic combinations between the coefficients. Note that  $q^2$  and  $\mathbf{q} \cdot \mathbf{k}$  terms vanish.

$$\begin{aligned}
a - b &= \frac{\hbar^2}{2m} (-2k^2 + 2\mathbf{q} \cdot \mathbf{k} - 2\mathbf{q} \cdot \mathbf{k}) = \frac{\hbar^2}{2m} (-2k^2), \quad b - c = \frac{\hbar^2}{2m} (2\mathbf{q} \cdot \mathbf{k} + k^2 - 2\mathbf{q} \cdot \mathbf{k}) = \frac{\hbar^2}{2m} (k^2) \\
a - c &= \frac{\hbar^2}{2m} (-2k^2 + 2\mathbf{q} \cdot \mathbf{k} + k^2 - 2\mathbf{q} \cdot \mathbf{k}) = \frac{\hbar^2}{2m} (-2k^2 + k^2) = \frac{\hbar^2}{2m} (-k^2), \quad a + b - 2c = \frac{\hbar^2}{2m} (-2k^2 + 2\mathbf{q} \cdot \mathbf{k} + 2\mathbf{q} \cdot \mathbf{k} + 2k^2 - 4\mathbf{q} \cdot \mathbf{k}) = \frac{\hbar^2}{2m} (-2k^2 + 2k^2) = 0.
\end{aligned}$$

Afterwards, we compute all the combinations that are present in the partial fraction decomposition.

$$\begin{aligned}
(a-b)(a-c)^3 &= \left(\frac{\hbar^2}{2m}\right)^4 (-2k^2)^4 (-k^6) = \left(\frac{\hbar^2}{2m}\right)^4 (2k^8), \quad (a-b)(b-c)^3 = \left(\frac{\hbar^2}{2m}\right)^4 (-2k^2)^4 (k^6) = \left(\frac{\hbar^2}{2m}\right)^4 (-2k^8), \\
(a-c)(b-c)^2 &= \left(\frac{\hbar^2}{2m}\right)^2 (-k^2)^2 (k^2) = \left(\frac{\hbar^2}{2m}\right)^2 (-k^4), \quad (a-c)^2(b-c)^2 = \left(\frac{\hbar^2}{2m}\right)^4 (k^8), \\
(a-c)^3(b-c)^3 &= \left(\frac{\hbar^2}{2m}\right)^6 (-k^{12}), \quad (a-b)^2 + 3(a-c)(b-c) = \left(\frac{\hbar^2}{2m}\right)^2 (4k^4 - 3k^4) = \left(\frac{\hbar^2}{2m}\right)^2 (k^4).
\end{aligned}$$

Finally, we substitute and perform some straightforward algebra. We also introduce the compact notation  $\epsilon_{\mathbf{k}} = (\hbar^2 k^2)/(2m)$ .

$$\begin{aligned}
[\chi_0^{(5,5)}(\mathbf{k}, z)]_{13} &= - \int \frac{d^3 q}{(2\pi)^3} \left(\frac{2m}{\hbar^2}\right)^4 \frac{1}{2k^8} \frac{1}{60} \frac{f_0(\mathbf{q})}{\left[\hbar z - \frac{\epsilon_q - \epsilon_{q-2\mathbf{k}}}{2}\right] \left[\hbar z - \frac{\epsilon_q + 2\mathbf{k} - \epsilon_{q-2\mathbf{k}}}{4}\right] - \frac{2}{\hbar z - \epsilon_q + \epsilon_{q-\mathbf{k}}} - \left(\frac{\hbar^2}{2m}\right)^2 \frac{2k^4}{(\hbar z - \epsilon_q + \epsilon_{q-\mathbf{k}})^3}} \Rightarrow \\
[\chi_0^{(5,5)}(\mathbf{k}, z)]_{13} &= - \left(\frac{m}{\hbar^2}\right)^4 \frac{1}{15k^8} \int \frac{d^3 q}{(2\pi)^3} \frac{2f_0(\mathbf{q})}{\left[\hbar z - \frac{\epsilon_q - \epsilon_{q-2\mathbf{k}}}{2}\right] \left[\hbar z - \frac{\epsilon_q + 2\mathbf{k} - \epsilon_{q-2\mathbf{k}}}{4}\right] - \frac{2}{\hbar z - \epsilon_q + \epsilon_{q-\mathbf{k}}} - \frac{2\epsilon_{\mathbf{k}}^2}{(\hbar z - \epsilon_q + \epsilon_{q-\mathbf{k}})^3}} \Rightarrow \\
[\chi_0^{(5,5)}(\mathbf{k}, z)]_{13} &= - \left(\frac{m}{\hbar^2}\right)^4 \frac{1}{180k^8} \int \frac{d^3 q}{(2\pi)^3} \frac{2f_0(\mathbf{q})}{\left[\frac{2\hbar z - \epsilon_q + \epsilon_{q-2\mathbf{k}}}{4\hbar z - \epsilon_q + \epsilon_{q-2\mathbf{k}}} + \frac{48}{\hbar z - \epsilon_q + \epsilon_{q-2\mathbf{k}}} - \frac{24}{\hbar z - \epsilon_q + \epsilon_{q-\mathbf{k}}} - \frac{24\epsilon_{\mathbf{k}}^2}{(\hbar z - \epsilon_q + \epsilon_{q-\mathbf{k}})^3}\right]}.
\end{aligned}$$

The *fourteenth contribution* is characterized by two simple poles and one triple pole. This becomes apparent from the algebraic identity  $(\epsilon_{\mathbf{q}+3\mathbf{k}} - \epsilon_{\mathbf{q}-2\mathbf{k}})/5 = (\epsilon_{\mathbf{q}+2\mathbf{k}} - \epsilon_{\mathbf{q}-\mathbf{k}})/3 = -(\epsilon_{\mathbf{q}+\mathbf{k}} - \epsilon_{\mathbf{q}})$ . We first identify and calculate the coefficients  $a, b, c$ .

$$\begin{aligned}
[\chi_0^{(5,5)}(\mathbf{k}, z)]_{14} &= + \int \frac{d^3q}{(2\pi)^3} \frac{2f_0(\mathbf{q})}{(5\hbar z - \epsilon_{\mathbf{q}+3\mathbf{k}} + \epsilon_{\mathbf{q}-2\mathbf{k}})(4\hbar z - \epsilon_{\mathbf{q}+3\mathbf{k}} + \epsilon_{\mathbf{q}-\mathbf{k}})(3\hbar z - \epsilon_{\mathbf{q}+2\mathbf{k}} + \epsilon_{\mathbf{q}-\mathbf{k}})(2\hbar z - \epsilon_{\mathbf{q}+\mathbf{k}} + \epsilon_{\mathbf{q}-\mathbf{k}})(\hbar z - \epsilon_{\mathbf{q}+\mathbf{k}} + \epsilon_{\mathbf{q}})} \\
[\chi_0^{(5,5)}(\mathbf{k}, z)]_{14} &= + \int \frac{d^3q}{(2\pi)^3} \frac{f_0(\mathbf{q})}{60} \left[ \hbar z - \frac{\epsilon_{\mathbf{q}+3\mathbf{k}} - \epsilon_{\mathbf{q}-2\mathbf{k}}}{5} \right] \left[ \hbar z - \frac{\epsilon_{\mathbf{q}+2\mathbf{k}} - \epsilon_{\mathbf{q}-\mathbf{k}}}{3} \right] \left[ \hbar z - \frac{\epsilon_{\mathbf{q}+\mathbf{k}} - \epsilon_{\mathbf{q}-\mathbf{k}}}{2} \right] \left[ \hbar z - (\epsilon_{\mathbf{q}+\mathbf{k}} - \epsilon_{\mathbf{q}}) \right] \\
[\chi_0^{(5,5)}(\mathbf{k}, z)]_{14} &= + \int \frac{d^3q}{(2\pi)^3} \frac{f_0(\mathbf{q})}{60} \left[ \hbar z - (\epsilon_{\mathbf{q}+\mathbf{k}} - \epsilon_{\mathbf{q}}) \right] \left[ \hbar z - \frac{\epsilon_{\mathbf{q}+3\mathbf{k}} - \epsilon_{\mathbf{q}-\mathbf{k}}}{4} \right] \left[ \hbar z - \frac{\epsilon_{\mathbf{q}+\mathbf{k}} - \epsilon_{\mathbf{q}-\mathbf{k}}}{2} \right] \left[ \hbar z - (\epsilon_{\mathbf{q}+\mathbf{k}} - \epsilon_{\mathbf{q}}) \right] \\
[\chi_0^{(5,5)}(\mathbf{k}, z)]_{14} &= + \int \frac{d^3q}{(2\pi)^3} \frac{f_0(\mathbf{q})}{60} \left[ \hbar z - \frac{\epsilon_{\mathbf{q}+\mathbf{k}} - \epsilon_{\mathbf{q}-\mathbf{k}}}{2} \right] \left[ \hbar z - \frac{\epsilon_{\mathbf{q}+3\mathbf{k}} - \epsilon_{\mathbf{q}-\mathbf{k}}}{4} \right] \left[ \hbar z - (\epsilon_{\mathbf{q}+\mathbf{k}} - \epsilon_{\mathbf{q}}) \right] \left[ \hbar z - (\epsilon_{\mathbf{q}+\mathbf{k}} - \epsilon_{\mathbf{q}}) \right] \\
a &= \frac{\epsilon_{\mathbf{q}+\mathbf{k}} - \epsilon_{\mathbf{q}-\mathbf{k}}}{2} \frac{\hbar^2 (\mathbf{q} + \mathbf{k})^2 - (\mathbf{q} - \mathbf{k})^2}{2m} = \frac{\hbar^2 k^2 + 2\mathbf{q} \cdot \mathbf{k} - k^2 + 2\mathbf{q} \cdot \mathbf{k}}{2m} = \frac{\hbar^2 4\mathbf{q} \cdot \mathbf{k}}{2m} = \frac{\hbar^2 (2\mathbf{q} \cdot \mathbf{k})}{2m} \\
b &= \frac{\epsilon_{\mathbf{q}+3\mathbf{k}} - \epsilon_{\mathbf{q}-\mathbf{k}}}{4} \frac{\hbar^2 (\mathbf{q} + 3\mathbf{k})^2 - (\mathbf{q} - \mathbf{k})^2}{2m} = \frac{\hbar^2 9k^2 + 6\mathbf{q} \cdot \mathbf{k} - k^2 + 2\mathbf{q} \cdot \mathbf{k}}{2m} = \frac{\hbar^2 8k^2 + 8\mathbf{q} \cdot \mathbf{k}}{2m} = \frac{\hbar^2 (2k^2 + 2\mathbf{q} \cdot \mathbf{k})}{2m} \\
c &= (\epsilon_{\mathbf{q}+\mathbf{k}} - \epsilon_{\mathbf{q}}) = \frac{\hbar^2}{2m} [(\mathbf{q} + \mathbf{k})^2 - q^2] = \frac{\hbar^2}{2m} (k^2 + 2\mathbf{q} \cdot \mathbf{k}).
\end{aligned}$$

Then, we compute all the relevant algebraic combinations between the coefficients. Note that  $q^2$  and  $\mathbf{q} \cdot \mathbf{k}$  terms vanish.

$$\begin{aligned}
a - b &= \frac{\hbar^2}{2m} (2\mathbf{q} \cdot \mathbf{k} - 2k^2 - 2\mathbf{q} \cdot \mathbf{k}) = \frac{\hbar^2}{2m} (-2k^2), \quad b - c = \frac{\hbar^2}{2m} (2k^2 + 2\mathbf{q} \cdot \mathbf{k} - k^2 - 2\mathbf{q} \cdot \mathbf{k}) = \frac{\hbar^2}{2m} (k^2) \\
a - c &= \frac{\hbar^2}{2m} (2\mathbf{q} \cdot \mathbf{k} - k^2 - 2\mathbf{q} \cdot \mathbf{k}) = \frac{\hbar^2}{2m} (-k^2), \quad a + b - 2c = \frac{\hbar^2}{2m} (2\mathbf{q} \cdot \mathbf{k} + 2k^2 + 2\mathbf{q} \cdot \mathbf{k} - 2k^2 - 4\mathbf{q} \cdot \mathbf{k}) = \frac{\hbar^2}{2m} (-2k^2 + 2k^2) = 0.
\end{aligned}$$

Afterwards, we compute all the combinations that are present in the partial fraction decomposition.

$$\begin{aligned}
(a-b)(a-c)^3 &= \left(\frac{\hbar^2}{2m}\right)^4 (-2k^2)^4 (-k^6) = \left(\frac{\hbar^2}{2m}\right)^4 (2k^8), \quad (a-b)(b-c)^3 = \left(\frac{\hbar^2}{2m}\right)^4 (-2k^2)^4 (k^6) = \left(\frac{\hbar^2}{2m}\right)^4 (-2k^8), \\
(a-c)(b-c)^2 &= \left(\frac{\hbar^2}{2m}\right)^2 (-k^2)^2 (k^2) = \left(\frac{\hbar^2}{2m}\right)^2 (-k^4), \quad (a-c)^2(b-c)^2 = \left(\frac{\hbar^2}{2m}\right)^4 (k^8), \\
(a-c)^3(b-c)^3 &= \left(\frac{\hbar^2}{2m}\right)^6 (-k^{12}), \quad (a-b)^2 + 3(a-c)(b-c) = \left(\frac{\hbar^2}{2m}\right)^2 (4k^4 - 3k^4) = \left(\frac{\hbar^2}{2m}\right)^2 (k^4).
\end{aligned}$$

Finally, we substitute and perform some straightforward algebra. We also introduce the compact notation  $\epsilon_{\mathbf{k}} = (\hbar^2 k^2)/(2m)$ .

$$\begin{aligned}
[\chi_0^{(5,5)}(\mathbf{k}, z)]_{14} &= + \int \frac{d^3q}{(2\pi)^3} \left(\frac{2m}{\hbar^2}\right)^4 \frac{f_0(\mathbf{q})}{60} \frac{1}{2k^8} + \frac{1}{\hbar z - \frac{\epsilon_{\mathbf{q}+\mathbf{k}} - \epsilon_{\mathbf{q}-\mathbf{k}}}{2}} + \frac{1}{\hbar z - \frac{\epsilon_{\mathbf{q}+3\mathbf{k}} - \epsilon_{\mathbf{q}-\mathbf{k}}}{4}} - \frac{2}{\hbar z - \epsilon_{\mathbf{q}+\mathbf{k}} + \epsilon_{\mathbf{q}}} - \left(\frac{\hbar^2}{2m}\right)^2 \frac{2k^4}{(\hbar z - \epsilon_{\mathbf{q}+\mathbf{k}} + \epsilon_{\mathbf{q}})^3} \Rightarrow \\
[\chi_0^{(5,5)}(\mathbf{k}, z)]_{14} &= + \left(\frac{m}{\hbar^2}\right)^4 \frac{1}{15k^8} \int \frac{d^3q}{(2\pi)^3} \frac{2f_0(\mathbf{q})}{(2\pi)^3} + \frac{1}{\hbar z - \frac{\epsilon_{\mathbf{q}+\mathbf{k}} - \epsilon_{\mathbf{q}-\mathbf{k}}}{2}} + \frac{1}{\hbar z - \frac{\epsilon_{\mathbf{q}+3\mathbf{k}} - \epsilon_{\mathbf{q}-\mathbf{k}}}{4}} - \frac{2}{\hbar z - \epsilon_{\mathbf{q}+\mathbf{k}} + \epsilon_{\mathbf{q}}} - \frac{2\epsilon_{\mathbf{k}}^2}{(\hbar z - \epsilon_{\mathbf{q}+\mathbf{k}} + \epsilon_{\mathbf{q}})^3} \Rightarrow \\
[\chi_0^{(5,5)}(\mathbf{k}, z)]_{14} &= + \left(\frac{m}{\hbar^2}\right)^4 \frac{1}{180k^8} \int \frac{d^3q}{(2\pi)^3} \frac{2f_0(\mathbf{q})}{(2\pi)^3} + \frac{24}{2\hbar z - \epsilon_{\mathbf{q}+\mathbf{k}} + \epsilon_{\mathbf{q}-\mathbf{k}}} + \frac{48}{4\hbar z - \epsilon_{\mathbf{q}+3\mathbf{k}} + \epsilon_{\mathbf{q}-\mathbf{k}}} - \frac{24}{\hbar z - \epsilon_{\mathbf{q}+\mathbf{k}} + \epsilon_{\mathbf{q}}} - \frac{24\epsilon_{\mathbf{k}}^2}{(\hbar z - \epsilon_{\mathbf{q}+\mathbf{k}} + \epsilon_{\mathbf{q}})^3}.
\end{aligned}$$

The *fifteenth contribution* is characterized by three simple poles and one double pole. This becomes apparent from the algebraic identity  $(\epsilon_q + 3k - \epsilon_{q-2k})/5 = (\epsilon_q + 2k - \epsilon_{q-k})/3$ . We first identify and calculate the coefficients  $a, b, c, d$ .

$$\begin{aligned}
\left[ \chi_0^{(5,5)}(\mathbf{k}, z) \right]_{15} &= + \int \frac{d^3 q}{(2\pi)^3} \frac{2f_0(\mathbf{q})}{(5\hbar z - \epsilon_q + 3k + \epsilon_{q-2k})(4\hbar z - \epsilon_q + 3k + \epsilon_{q-k})(3\hbar z - \epsilon_q + 2k + \epsilon_{q-k})(2\hbar z - \epsilon_q + k + \epsilon_{q-k})(\hbar z - \epsilon_q - k)} \Rightarrow \\
\left[ \chi_0^{(5,5)}(\mathbf{k}, z) \right]_{15} &= + \int \frac{d^3 q}{(2\pi)^3} \frac{f_0(\mathbf{q})}{60} \left[ \hbar z - \frac{\epsilon_q + 3k - \epsilon_{q-2k}}{5} \right] \left[ \hbar z - \frac{\epsilon_q + 2k - \epsilon_{q-k}}{3} \right] \left[ \hbar z - \frac{\epsilon_q + k - \epsilon_{q-k}}{2} \right] \left[ \hbar z - (\epsilon_q - k) \right] \Rightarrow \\
\left[ \chi_0^{(5,5)}(\mathbf{k}, z) \right]_{15} &= + \int \frac{d^3 q}{(2\pi)^3} \frac{f_0(\mathbf{q})}{60} \left[ \hbar z - \frac{\epsilon_q + 2k - \epsilon_{q-k}}{3} \right] \left[ \hbar z - \frac{\epsilon_q + 3k - \epsilon_{q-k}}{4} \right] \left[ \hbar z - \frac{\epsilon_q + 2k - \epsilon_{q-k}}{2} \right] \left[ \hbar z - (\epsilon_q - k) \right] \Rightarrow \\
\left[ \chi_0^{(5,5)}(\mathbf{k}, z) \right]_{15} &= + \int \frac{d^3 q}{(2\pi)^3} \frac{f_0(\mathbf{q})}{60} \left[ \hbar z - \frac{\epsilon_q + 2k - \epsilon_{q-k}}{3} \right] \left[ \hbar z - \frac{\epsilon_q + 3k - \epsilon_{q-k}}{4} \right] \left[ \hbar z - \frac{\epsilon_q + 2k - \epsilon_{q-k}}{2} \right] \left[ \hbar z - (\epsilon_q - k) \right] \Rightarrow \\
\left[ \chi_0^{(5,5)}(\mathbf{k}, z) \right]_{15} &= + \int \frac{d^3 q}{(2\pi)^3} \frac{f_0(\mathbf{q})}{60} \left[ \hbar z - (\epsilon_q - k) \right] \left[ \hbar z - \frac{\epsilon_q + k - \epsilon_{q-k}}{2} \right] \left[ \hbar z - \frac{\epsilon_q + 3k - \epsilon_{q-k}}{4} \right] \left[ \hbar z - \frac{\epsilon_q + 2k - \epsilon_{q-k}}{3} \right]^2 \Rightarrow \\
a = (\epsilon_q - \epsilon_{q-k}) &= \frac{\hbar^2}{2m} [q^2 - (q-k)^2] = \frac{\hbar^2}{2m} (-k^2 + 2\mathbf{q} \cdot \mathbf{k}) \\
b = \frac{\epsilon_q + k - \epsilon_{q-k}}{2} &= \frac{\hbar^2}{2m} \frac{2}{(q+k)^2 - (q-k)^2} = \frac{\hbar^2}{2m} \frac{2}{k^2 + 2\mathbf{q} \cdot \mathbf{k} - k^2 + 2\mathbf{q} \cdot \mathbf{k}} = \frac{\hbar^2}{2m} \frac{4\mathbf{q} \cdot \mathbf{k}}{2} = \frac{\hbar^2}{2m} (2\mathbf{q} \cdot \mathbf{k}) \\
c = \frac{\epsilon_q + 3k - \epsilon_{q-k}}{4} &= \frac{\hbar^2}{2m} \frac{4}{(q+3k)^2 - (q-k)^2} = \frac{\hbar^2}{2m} \frac{4}{9k^2 + 6\mathbf{q} \cdot \mathbf{k} - k^2 + 2\mathbf{q} \cdot \mathbf{k}} = \frac{\hbar^2}{2m} \frac{8k^2 + 8\mathbf{q} \cdot \mathbf{k}}{4} = \frac{\hbar^2}{2m} (2k^2 + 2\mathbf{q} \cdot \mathbf{k}) \\
d = \frac{\epsilon_q + 2k - \epsilon_{q-k}}{3} &= \frac{\hbar^2}{2m} \frac{3}{(q+2k)^2 - (q-k)^2} = \frac{\hbar^2}{2m} \frac{3}{4k^2 + 4\mathbf{q} \cdot \mathbf{k} - k^2 + 2\mathbf{q} \cdot \mathbf{k}} = \frac{\hbar^2}{2m} \frac{3k^2 + 6\mathbf{q} \cdot \mathbf{k}}{5} = \frac{\hbar^2}{2m} (k^2 + 2\mathbf{q} \cdot \mathbf{k}).
\end{aligned}$$

Then, we compute all the relevant algebraic combinations between the coefficients. Note that  $q^2$  and  $\mathbf{q} \cdot \mathbf{k}$  terms vanish.

$$\begin{aligned}
a - b &= \frac{\hbar^2}{2m} (-k^2 + 2\mathbf{q} \cdot \mathbf{k} - 2\mathbf{q} \cdot \mathbf{k}) = \frac{\hbar^2}{2m} (-k^2), \quad b - c = \frac{\hbar^2}{2m} (2\mathbf{q} \cdot \mathbf{k} - 2k^2 - 2\mathbf{q} \cdot \mathbf{k}) = \frac{\hbar^2}{2m} (-2k^2) \\
c - d &= \frac{\hbar^2}{2m} (2k^2 + 2\mathbf{q} \cdot \mathbf{k} - k^2 - 2\mathbf{q} \cdot \mathbf{k}) = \frac{\hbar^2}{2m} (k^2), \quad a - c = \frac{\hbar^2}{2m} (-k^2 + 2\mathbf{q} \cdot \mathbf{k} - 2k^2 - 2\mathbf{q} \cdot \mathbf{k}) = \frac{\hbar^2}{2m} (-3k^2) \\
b - d &= \frac{\hbar^2}{2m} (2\mathbf{q} \cdot \mathbf{k} - k^2 - 2\mathbf{q} \cdot \mathbf{k}) = \frac{\hbar^2}{2m} (-k^2), \quad a - d = \frac{\hbar^2}{2m} (-k^2 + 2\mathbf{q} \cdot \mathbf{k} - k^2 - 2\mathbf{q} \cdot \mathbf{k}) = \frac{\hbar^2}{2m} (-2k^2).
\end{aligned}$$

Afterwards, we compute all the combinations that are present in the partial fraction decomposition.

$$\begin{aligned}
(a-b)(a-c)(a-d)^2 &= \left( \frac{\hbar^2}{2m} \right)^4 (-k^2) (-3k^2) (4k^4) = \left( \frac{\hbar^2}{2m} \right)^4 (12k^8), \quad (a-b)(b-c)(b-d)^2 = \left( \frac{\hbar^2}{2m} \right)^4 (-k^2) (-2k^2) (k^4) = \left( \frac{\hbar^2}{2m} \right)^4 (2k^8), \\
(a-c)(b-c)(c-d)^2 &= \left( \frac{\hbar^2}{2m} \right)^4 (-3k^2) (-2k^2) (k^4) = \left( \frac{\hbar^2}{2m} \right)^4 (6k^8), \quad (a-d)(b-d)(c-d) = \left( \frac{\hbar^2}{2m} \right)^3 (-2k^2) (-k^2) (k^2) = \left( \frac{\hbar^2}{2m} \right)^3 (2k^6), \\
(a-d)^2(b-d)^2(c-d)^2 &= \left( \frac{\hbar^2}{2m} \right)^6 (4k^{12}), \quad (a-b)(b-c) + (a-d)^2 + (b-d)^2 + (c-d)^2 = \left( \frac{\hbar^2}{2m} \right)^2 (2k^4 + 4k^4 + k^4 - 9k^4) = \left( \frac{\hbar^2}{2m} \right)^2 (-k^4).
\end{aligned}$$

Finally, we substitute and perform some straightforward algebra. We also introduce the compact notation  $\epsilon_k = (\hbar^2 k^2)/(2m)$ .

$$\begin{aligned}
\left[ \chi_0^{(5,5)}(\mathbf{k}, z) \right]_{15} &= + \int \frac{d^3 q}{(2\pi)^3} \frac{(2m)^4}{(\hbar^2)^2} \frac{1}{12k^8} \frac{f_0(\mathbf{q})}{60} \left[ \frac{1}{\hbar z - \epsilon_q - \epsilon_{q-k}} - \frac{6}{\hbar z - \epsilon_q - k} + \frac{2}{\hbar z - \frac{\epsilon_q + k - \epsilon_{q-k}}{2}} + \frac{3}{\hbar z - \frac{\epsilon_q + 2k - \epsilon_{q-k}}{3}} - \frac{h^2}{2m} \frac{6k^2}{\left( \hbar z - \frac{\epsilon_q + 2k - \epsilon_{q-k}}{3} \right)^2} \right] \Rightarrow \\
\left[ \chi_0^{(5,5)}(\mathbf{k}, z) \right]_{15} &= + \left( \frac{m}{\hbar^2} \right)^4 \frac{1}{90k^8} \int \frac{d^3 q}{(2\pi)^3} \frac{2f_0(\mathbf{q})}{60} \left[ \frac{1}{\hbar z - \epsilon_q - \epsilon_{q-k}} - \frac{6}{\hbar z - \frac{\epsilon_q + k - \epsilon_{q-k}}{2}} + \frac{2}{\hbar z - \frac{\epsilon_q + 3k - \epsilon_{q-k}}{4}} + \frac{3}{\hbar z - \frac{\epsilon_q + 2k - \epsilon_{q-k}}{3}} - \frac{6\epsilon_k}{\left( \hbar z - \frac{\epsilon_q + 2k - \epsilon_{q-k}}{3} \right)^2} \right] \Rightarrow \\
\left[ \chi_0^{(5,5)}(\mathbf{k}, z) \right]_{15} &= + \left( \frac{m}{\hbar^2} \right)^4 \frac{1}{180k^8} \int \frac{d^3 q}{(2\pi)^3} \frac{2f_0(\mathbf{q})}{60} \left[ \frac{2}{\hbar z - \epsilon_q - \epsilon_{q-k}} - \frac{24}{2\hbar z - \epsilon_q + k + \epsilon_{q-k}} + \frac{16}{4\hbar z - \epsilon_q + 3k + \epsilon_{q-k}} + \frac{18}{3\hbar z - \epsilon_q + 2k + \epsilon_{q-k}} - \frac{108\epsilon_k}{(3\hbar z - \epsilon_q + 2k + \epsilon_{q-k})^2} \right].
\end{aligned}$$

The *sixteenth contribution* is characterized by three simple poles and one double pole. This becomes apparent from the algebraic identity  $(\epsilon_q + 4k - \epsilon_q - k)/5 = (\epsilon_q + 3k - \epsilon_q)/3$ . We first identify and calculate the coefficients  $a, b, c, d$ .

$$\begin{aligned}
[\chi_0^{(5,5)}(\mathbf{k}, z)]_{16} &= - \int \frac{d^3 q}{(2\pi)^3} \frac{5\hbar z - \epsilon_q + 4k + \epsilon_q - k}{(2\pi)^3} \frac{2f_0(\mathbf{q})}{(3\hbar z - \epsilon_q + 3k + \epsilon_q) (2\hbar z - \epsilon_q + 2k + \epsilon_q) (\hbar z - \epsilon_q + k + \epsilon_q)} \Rightarrow \\
[\chi_0^{(5,5)}(\mathbf{k}, z)]_{16} &= - \int \frac{d^3 q}{(2\pi)^3} \frac{f_0(\mathbf{q})}{60} \frac{1}{\left[\hbar z - \frac{\epsilon_q + 4k - \epsilon_q - k}{5}\right] \left[\hbar z - \frac{\epsilon_q + 4k - \epsilon_q}{4}\right] \left[\hbar z - \frac{\epsilon_q + 3k - \epsilon_q}{3}\right] \left[\hbar z - \frac{\epsilon_q + 2k - \epsilon_q}{2}\right] \left[\hbar z - (\epsilon_q + k - \epsilon_q)\right]} \Rightarrow \\
[\chi_0^{(5,5)}(\mathbf{k}, z)]_{16} &= - \int \frac{d^3 q}{(2\pi)^3} \frac{f_0(\mathbf{q})}{60} \frac{1}{\left[\hbar z - \frac{\epsilon_q + 3k - \epsilon_q}{3}\right] \left[\hbar z - \frac{\epsilon_q + 4k - \epsilon_q}{4}\right] \left[\hbar z - \frac{\epsilon_q + 2k - \epsilon_q}{2}\right] \left[\hbar z - (\epsilon_q + k - \epsilon_q)\right]} \Rightarrow \\
[\chi_0^{(5,5)}(\mathbf{k}, z)]_{16} &= - \int \frac{d^3 q}{(2\pi)^3} \frac{f_0(\mathbf{q})}{60} \frac{1}{\left[\hbar z - (\epsilon_q + k - \epsilon_q)\right] \left[\hbar z - \frac{\epsilon_q + 2k - \epsilon_q}{2}\right] \left[\hbar z - \frac{\epsilon_q + 4k - \epsilon_q}{4}\right] \left[\hbar z - \frac{\epsilon_q + 3k - \epsilon_q}{3}\right]} \Rightarrow \\
a = (\epsilon_q + k - \epsilon_q) &= \frac{\hbar^2}{2m} [(q + k)^2 - q^2] = \frac{\hbar^2}{2m} (k^2 + 2q \cdot k) \\
b = \frac{\epsilon_q + 2k - \epsilon_q}{2} &= \frac{\hbar^2}{2m} \frac{(q + 2k)^2 - q^2}{2} = \frac{\hbar^2}{2m} \frac{4k^2 + 4q \cdot k}{2} = \frac{\hbar^2}{2m} (2k^2 + 2q \cdot k) \\
c = \frac{\epsilon_q + 4k - \epsilon_q}{4} &= \frac{\hbar^2}{2m} \frac{(q + 4k)^2 - q^2}{4} = \frac{\hbar^2}{2m} \frac{16k^2 + 8q \cdot k}{4} = \frac{\hbar^2}{2m} (4k^2 + 2q \cdot k) \\
d = \frac{\epsilon_q + 3k - \epsilon_q}{3} &= \frac{\hbar^2}{2m} \frac{(q + 3k)^2 - q^2}{3} = \frac{\hbar^2}{2m} \frac{9k^2 + 6q \cdot k}{3} = \frac{\hbar^2}{2m} (3k^2 + 2q \cdot k).
\end{aligned}$$

Then, we compute all the relevant algebraic combinations between the coefficients. Note that  $q^2$  and  $q \cdot k$  terms vanish.

$$\begin{aligned}
a - b &= \frac{\hbar^2}{2m} (k^2 + 2q \cdot k - 2k^2 - 2q \cdot k) = \frac{\hbar^2}{2m} (-k^2), \quad b - c = \frac{\hbar^2}{2m} (2k^2 + 2q \cdot k - 4k^2 - 2q \cdot k) = \frac{\hbar^2}{2m} (-2k^2) \\
c - d &= \frac{\hbar^2}{2m} (4k^2 + 2q \cdot k - 3k^2 - 2q \cdot k) = \frac{\hbar^2}{2m} (k^2), \quad a - c = \frac{\hbar^2}{2m} (k^2 + 2q \cdot k - 4k^2 - 2q \cdot k) = \frac{\hbar^2}{2m} (-3k^2) \\
b - d &= \frac{\hbar^2}{2m} (2k^2 + 2q \cdot k - 3k^2 - 2q \cdot k) = \frac{\hbar^2}{2m} (-k^2), \quad a - d = \frac{\hbar^2}{2m} (k^2 + 2q \cdot k - 3k^2 - 2q \cdot k) = \frac{\hbar^2}{2m} (-2k^2).
\end{aligned}$$

Afterwards, we compute all the combinations that are present in the partial fraction decomposition.

$$\begin{aligned}
(a - b)(a - c)(a - d)^2 &= \left(\frac{\hbar^2}{2m}\right)^4 (-k^2)^2 (-3k^2) (4k^4) = \left(\frac{\hbar^2}{2m}\right)^4 (12k^8), \quad (a - b)(b - c)(b - d)^2 = \left(\frac{\hbar^2}{2m}\right)^4 (-k^2)^2 (-2k^2) (k^4) = \left(\frac{\hbar^2}{2m}\right)^4 (2k^8), \\
(a - c)(b - c)(c - d)^2 &= \left(\frac{\hbar^2}{2m}\right)^4 (-3k^2)^2 (-2k^2) (k^4) = \left(\frac{\hbar^2}{2m}\right)^4 (6k^8), \quad (a - d)(b - d)(c - d) = \left(\frac{\hbar^2}{2m}\right)^3 (-2k^2)^2 (-k^2) (k^2) = \left(\frac{\hbar^2}{2m}\right)^3 (2k^6), \\
(a - d)^2(b - d)^2(c - d)^2 &= \left(\frac{\hbar^2}{2m}\right)^6 (4k^{12}), \quad (a - b)(b - c) + (a - d)^2 + (b - d)^2 + (c - d)^2 = \left(\frac{\hbar^2}{2m}\right)^2 (2k^4 + 4k^4 + k^4 - 9k^4) = \left(\frac{\hbar^2}{2m}\right)^2 (-k^4).
\end{aligned}$$

Finally, we substitute and perform some straightforward algebra. We also introduce the compact notation  $\epsilon_k = (\hbar^2 k^2)/(2m)$ .

$$\begin{aligned}
[\chi_0^{(5,5)}(\mathbf{k}, z)]_{16} &= - \int \frac{d^3 q}{(2\pi)^3} \frac{(2m)^4}{(\hbar^2)^2} \frac{1}{12k^8} \frac{f_0(\mathbf{q})}{60} \left[ \frac{1}{\hbar z - \epsilon_q + k + \epsilon_q} - \frac{6}{\hbar z - \epsilon_q + 2k - \epsilon_q} + \frac{2}{\hbar z - \frac{\epsilon_q + 4k - \epsilon_q}{4}} + \frac{3}{\hbar z - \frac{\epsilon_q + 3k - \epsilon_q}{3}} - \frac{\hbar^2}{2m} \frac{6k^2}{\left(\hbar z - \frac{\epsilon_q + 3k - \epsilon_q}{3}\right)^2} \right] \Rightarrow \\
[\chi_0^{(5,5)}(\mathbf{k}, z)]_{16} &= - \left(\frac{m}{\hbar^2}\right)^4 \frac{1}{90k^8} \int \frac{d^3 q}{(2\pi)^3} \frac{2f_0(\mathbf{q})}{60} \left[ \frac{1}{\hbar z - \epsilon_q + k + \epsilon_q} - \frac{6}{\hbar z - \frac{\epsilon_q + 2k - \epsilon_q}{2}} + \frac{2}{\hbar z - \frac{\epsilon_q + 4k - \epsilon_q}{4}} + \frac{3}{\hbar z - \frac{\epsilon_q + 3k - \epsilon_q}{3}} - \frac{6\epsilon_k}{\left(\hbar z - \frac{\epsilon_q + 3k - \epsilon_q}{3}\right)^2} \right] \Rightarrow \\
[\chi_0^{(5,5)}(\mathbf{k}, z)]_{16} &= - \left(\frac{m}{\hbar^2}\right)^4 \frac{1}{180k^8} \int \frac{d^3 q}{(2\pi)^3} \frac{2f_0(\mathbf{q})}{60} \left[ \frac{2}{\hbar z - \epsilon_q + k + \epsilon_q} - \frac{24}{2\hbar z - \epsilon_q + 2k + \epsilon_q} + \frac{16}{4\hbar z - \epsilon_q + 4k + \epsilon_q} + \frac{18}{3\hbar z - \epsilon_q + 3k + \epsilon_q} - \frac{108\epsilon_k}{\left(3\hbar z - \epsilon_q + 3k + \epsilon_q\right)^2} \right].
\end{aligned}$$



The *seventeenth contribution* is characterized by three simple poles and one double pole. This becomes apparent from the algebraic identity  $(\epsilon_q + \mathbf{k} - \epsilon_{q-4\mathbf{k}})/5 = (\epsilon_q - \epsilon_{q-3\mathbf{k}})/3$ . We first identify and calculate the coefficients  $a, b, c, d$ .

$$\begin{aligned}
\left[ \chi_0^{(5,5)}(\mathbf{k}, z) \right]_{17} &= + \int \frac{d^3 q}{(2\pi)^3} \frac{5\hbar z - \epsilon_{q+\mathbf{k}} + \epsilon_{q-4\mathbf{k}}}{(2\pi)^3} \frac{(4\hbar z - \epsilon_q + \epsilon_{q-4\mathbf{k}})(3\hbar z - \epsilon_q + \epsilon_{q-3\mathbf{k}})(2\hbar z - \epsilon_q + \epsilon_{q-2\mathbf{k}})(\hbar z - \epsilon_q + \epsilon_{q-\mathbf{k}})}{2f_0(\mathbf{q})} \Rightarrow \\
\left[ \chi_0^{(5,5)}(\mathbf{k}, z) \right]_{17} &= + \int \frac{d^3 q}{(2\pi)^3} \frac{f_0(\mathbf{q})}{60} \frac{1}{\left[ \hbar z - \frac{\epsilon_q - \epsilon_{q-4\mathbf{k}}}{5} \right] \left[ \hbar z - \frac{\epsilon_q - \epsilon_{q-4\mathbf{k}}}{4} \right] \left[ \hbar z - \frac{\epsilon_q - \epsilon_{q-3\mathbf{k}}}{3} \right] \left[ \hbar z - \frac{\epsilon_q - \epsilon_{q-2\mathbf{k}}}{2} \right] \left[ \hbar z - (\epsilon_q - \epsilon_{q-\mathbf{k}}) \right]} \Rightarrow \\
\left[ \chi_0^{(5,5)}(\mathbf{k}, z) \right]_{17} &= + \int \frac{d^3 q}{(2\pi)^3} \frac{f_0(\mathbf{q})}{60} \frac{1}{\left[ \hbar z - \frac{\epsilon_q - \epsilon_{q-3\mathbf{k}}}{3} \right] \left[ \hbar z - \frac{\epsilon_q - \epsilon_{q-4\mathbf{k}}}{4} \right] \left[ \hbar z - \frac{\epsilon_q - \epsilon_{q-2\mathbf{k}}}{2} \right] \left[ \hbar z - (\epsilon_q - \epsilon_{q-\mathbf{k}}) \right]} \Rightarrow \\
\left[ \chi_0^{(5,5)}(\mathbf{k}, z) \right]_{17} &= + \int \frac{d^3 q}{(2\pi)^3} \frac{f_0(\mathbf{q})}{60} \frac{1}{\left[ \hbar z - (\epsilon_q - \epsilon_{q-\mathbf{k}}) \right] \left[ \hbar z - \frac{\epsilon_q - \epsilon_{q-2\mathbf{k}}}{2} \right] \left[ \hbar z - \frac{\epsilon_q - \epsilon_{q-4\mathbf{k}}}{4} \right] \left[ \hbar z - \frac{\epsilon_q - \epsilon_{q-3\mathbf{k}}}{3} \right]} \Rightarrow \\
a = (\epsilon_q - \epsilon_{q-\mathbf{k}}) &= \frac{\hbar^2}{2m} [q^2 - (q - \mathbf{k})^2] = \frac{\hbar^2}{2m} (-k^2 + 2\mathbf{q} \cdot \mathbf{k}) \\
b = \frac{\epsilon_q - \epsilon_{q-2\mathbf{k}}}{2} &= \frac{\hbar^2}{2m} \frac{q^2 - (q - 2\mathbf{k})^2}{2} = \frac{\hbar^2}{2m} \frac{-4k^2 + 4\mathbf{q} \cdot \mathbf{k}}{2} = \frac{\hbar^2}{2m} (-2k^2 + 2\mathbf{q} \cdot \mathbf{k}) \\
c = \frac{\epsilon_q - \epsilon_{q-4\mathbf{k}}}{4} &= \frac{\hbar^2}{2m} \frac{q^2 - (q - 4\mathbf{k})^2}{4} = \frac{\hbar^2}{2m} \frac{-16k^2 + 8\mathbf{q} \cdot \mathbf{k}}{4} = \frac{\hbar^2}{2m} (-4k^2 + 2\mathbf{q} \cdot \mathbf{k}) \\
d = \frac{\epsilon_q - \epsilon_{q-3\mathbf{k}}}{3} &= \frac{\hbar^2}{2m} \frac{q^2 - (q - 3\mathbf{k})^2}{3} = \frac{\hbar^2}{2m} \frac{-9k^2 + 6\mathbf{q} \cdot \mathbf{k}}{3} = \frac{\hbar^2}{2m} (-3k^2 + 2\mathbf{q} \cdot \mathbf{k}).
\end{aligned}$$

Then, we compute all the relevant algebraic combinations between the coefficients. Note that  $q^2$  and  $\mathbf{q} \cdot \mathbf{k}$  terms vanish.

$$\begin{aligned}
a - b &= \frac{\hbar^2}{2m} (-k^2 + 2\mathbf{q} \cdot \mathbf{k} + 2k^2 - 2\mathbf{q} \cdot \mathbf{k}) = \frac{\hbar^2}{2m} (+k^2), \quad b - c = \frac{\hbar^2}{2m} (-2k^2 + 2\mathbf{q} \cdot \mathbf{k} + 4k^2 - 2\mathbf{q} \cdot \mathbf{k}) = \frac{\hbar^2}{2m} (2k^2) \\
c - d &= \frac{\hbar^2}{2m} (-4k^2 + 2\mathbf{q} \cdot \mathbf{k} + 3k^2 - 2\mathbf{q} \cdot \mathbf{k}) = \frac{\hbar^2}{2m} (-k^2), \quad a - c = \frac{\hbar^2}{2m} (-k^2 + 2\mathbf{q} \cdot \mathbf{k} + 4k^2 - 2\mathbf{q} \cdot \mathbf{k}) = \frac{\hbar^2}{2m} (3k^2) \\
b - d &= \frac{\hbar^2}{2m} (-2k^2 + 2\mathbf{q} \cdot \mathbf{k} + 3k^2 - 2\mathbf{q} \cdot \mathbf{k}) = \frac{\hbar^2}{2m} (+k^2), \quad a - d = \frac{\hbar^2}{2m} (-k^2 + 2\mathbf{q} \cdot \mathbf{k} + 3k^2 - 2\mathbf{q} \cdot \mathbf{k}) = \frac{\hbar^2}{2m} (-k^2 + 3k^2) = \frac{\hbar^2}{2m} (2k^2).
\end{aligned}$$

Afterwards, we compute all the combinations that are present in the partial fraction decomposition.

$$\begin{aligned}
(a - b)(a - c)(a - d)^2 &= \left( \frac{\hbar^2}{2m} \right)^4 (k^2)^4 (3k^2)^4 (4k^4)^4 = \left( \frac{\hbar^2}{2m} \right)^4 (k^2)^4 (b - c)(b - d)^2 = \left( \frac{\hbar^2}{2m} \right)^4 (k^2)^4 (2k^2)^4 (k^4)^4 = \left( \frac{\hbar^2}{2m} \right)^4 (2k^8)^4, \\
(a - c)(b - c)(c - d)^2 &= \left( \frac{\hbar^2}{2m} \right)^4 (3k^2)^4 (2k^2)^4 (k^4)^4 = \left( \frac{\hbar^2}{2m} \right)^4 (6k^8)^4, \quad (a - d)(b - d)(c - d) = \left( \frac{\hbar^2}{2m} \right)^3 (2k^2)^3 (k^2)^3 (-k^2)^3 = \left( \frac{\hbar^2}{2m} \right)^3 (-2k^6)^3, \\
(a - d)^2(b - d)^2(c - d)^2 &= \left( \frac{\hbar^2}{2m} \right)^6 (4k^{12})^6, \quad (a - b)(b - c) + (a - d)^2 + (b - d)^2 + (c - d)^2 = \left( \frac{\hbar^2}{2m} \right)^2 (2k^4 + 4k^4 + k^4 + k^4 - 9k^4) = \left( \frac{\hbar^2}{2m} \right)^2 (-k^4)^2.
\end{aligned}$$

Finally, we substitute and perform some straightforward algebra. We also introduce the compact notation  $\epsilon_{\mathbf{k}} = (\hbar^2 k^2)/(2m)$ .

$$\begin{aligned}
\left[ \chi_0^{(5,5)}(\mathbf{k}, z) \right]_{17} &= + \int \frac{d^3 q}{(2\pi)^3} \frac{(2m)^4}{(\hbar^2)^2} \frac{1}{12k^8} \frac{f_0(\mathbf{q})}{60} \left[ \frac{1}{\hbar z - \epsilon_q + \epsilon_{q-\mathbf{k}}} - \frac{6}{\hbar z - \frac{\epsilon_q - \epsilon_{q-2\mathbf{k}}}{2}} + \frac{2}{\hbar z - \frac{\epsilon_q - \epsilon_{q-4\mathbf{k}}}{4}} + \frac{3}{\hbar z - \frac{\epsilon_q - \epsilon_{q-3\mathbf{k}}}{3}} + \frac{\hbar^2}{2m} \frac{6k^2}{\left( \hbar z - \frac{\epsilon_q - \epsilon_{q-3\mathbf{k}}}{3} \right)^2} \right] \Rightarrow \\
\left[ \chi_0^{(5,5)}(\mathbf{k}, z) \right]_{17} &= + \left( \frac{m}{\hbar^2} \right)^4 \frac{1}{90k^8} \int \frac{d^3 q}{(2\pi)^3} \frac{2f_0(\mathbf{q})}{60} \left[ \frac{1}{\hbar z - \epsilon_q + \epsilon_{q-\mathbf{k}}} - \frac{6}{\hbar z - \frac{\epsilon_q - \epsilon_{q-2\mathbf{k}}}{2}} + \frac{2}{\hbar z - \frac{\epsilon_q - \epsilon_{q-4\mathbf{k}}}{4}} + \frac{3}{\hbar z - \frac{\epsilon_q - \epsilon_{q-3\mathbf{k}}}{3}} + \frac{6\epsilon_{\mathbf{k}}}{\left( \hbar z - \frac{\epsilon_q - \epsilon_{q-3\mathbf{k}}}{3} \right)^2} \right] \Rightarrow \\
\left[ \chi_0^{(5,5)}(\mathbf{k}, z) \right]_{17} &= + \left( \frac{m}{\hbar^2} \right)^4 \frac{1}{180k^8} \int \frac{d^3 q}{(2\pi)^3} \frac{2f_0(\mathbf{q})}{60} \left[ \frac{2}{\hbar z - \epsilon_q + \epsilon_{q-\mathbf{k}}} - \frac{24}{2\hbar z - \epsilon_q + \epsilon_{q-2\mathbf{k}}} + \frac{16}{4\hbar z - \epsilon_q + \epsilon_{q-4\mathbf{k}}} + \frac{18}{3\hbar z - \epsilon_q + \epsilon_{q-3\mathbf{k}}} + \frac{108\epsilon_{\mathbf{k}}}{\left( \hbar z - \frac{\epsilon_q - \epsilon_{q-3\mathbf{k}}}{3} \right)^2} \right].
\end{aligned}$$

The *eighteenth contribution* is characterized by three simple poles and one double pole. This becomes apparent from the algebraic identity  $(\epsilon_{q+2k} - \epsilon_{q-3k})/5 = (\epsilon_{q+k} - \epsilon_{q-2k})/3$ . We first identify and calculate the coefficients  $a, b, c, d$ .

$$\begin{aligned}
[\chi_0^{(5,5)}(\mathbf{k}, z)]_{18} &= - \int \frac{d^3 q}{(2\pi)^3} \frac{2f_0(\mathbf{q})}{(5\hbar z - \epsilon_{q+2k} + \epsilon_{q-3k})(4\hbar z - \epsilon_{q+k} + \epsilon_{q-2k})(2\hbar z - \epsilon_{q+k} + \epsilon_{q-k})(\hbar z - \epsilon_{q+k} + \epsilon_q)} \Rightarrow \\
[\chi_0^{(5,5)}(\mathbf{k}, z)]_{18} &= - \int \frac{d^3 q}{(2\pi)^3} \frac{f_0(\mathbf{q})}{60} \left[ \hbar z - \frac{\epsilon_{q+2k} - \epsilon_{q-3k}}{5} \right] \left[ \hbar z - \frac{\epsilon_{q+k} - \epsilon_{q-2k}}{3} \right] \left[ \hbar z - \frac{\epsilon_{q+k} - \epsilon_{q-k}}{2} \right] [\hbar z - (\epsilon_{q+k} - \epsilon_q)] \Rightarrow \\
[\chi_0^{(5,5)}(\mathbf{k}, z)]_{18} &= - \int \frac{d^3 q}{(2\pi)^3} \frac{f_0(\mathbf{q})}{60} \left[ \hbar z - \frac{\epsilon_{q+k} - \epsilon_{q-2k}}{3} \right] \left[ \hbar z - \frac{\epsilon_{q+k} - \epsilon_{q-3k}}{4} \right] \left[ \hbar z - \frac{\epsilon_{q+k} - \epsilon_{q-k}}{2} \right] [\hbar z - (\epsilon_{q+k} - \epsilon_q)] \Rightarrow \\
[\chi_0^{(5,5)}(\mathbf{k}, z)]_{18} &= - \int \frac{d^3 q}{(2\pi)^3} \frac{f_0(\mathbf{q})}{60} \left[ \hbar z - \frac{\epsilon_{q+k} - \epsilon_{q-2k}}{3} \right] \left[ \hbar z - \frac{\epsilon_{q+k} - \epsilon_{q-3k}}{4} \right] \left[ \hbar z - \frac{\epsilon_{q+k} - \epsilon_{q-k}}{2} \right] [\hbar z - (\epsilon_{q+k} - \epsilon_q)] \Rightarrow \\
[\chi_0^{(5,5)}(\mathbf{k}, z)]_{18} &= - \int \frac{d^3 q}{(2\pi)^3} \frac{f_0(\mathbf{q})}{60} \left[ \hbar z - (\epsilon_{q+k} - \epsilon_q) \right] \left[ \hbar z - \frac{\epsilon_{q+k} - \epsilon_{q-k}}{2} \right] \left[ \hbar z - \frac{\epsilon_{q+k} - \epsilon_{q-3k}}{4} \right] \left[ \hbar z - \frac{\epsilon_{q+k} - \epsilon_{q-2k}}{3} \right] \Rightarrow \\
a = (\epsilon_{q+k} - \epsilon_q) &= \frac{\hbar^2}{2m} [(q+k)^2 - q^2] = \frac{\hbar^2}{2m} (k^2 + 2\mathbf{q} \cdot \mathbf{k}) \\
b = \frac{\epsilon_{q+k} - \epsilon_{q-k}}{2} &= \frac{\hbar^2}{2m} \frac{2}{(q+k)^2 - (q-k)^2} = \frac{\hbar^2}{2m} \frac{2}{k^2 + 2\mathbf{q} \cdot \mathbf{k} - k^2 + 2\mathbf{q} \cdot \mathbf{k}} = \frac{\hbar^2}{2m} \frac{2}{2\mathbf{q} \cdot \mathbf{k}} = \frac{\hbar^2}{2m} (2\mathbf{q} \cdot \mathbf{k}) \\
c = \frac{\epsilon_{q+k} - \epsilon_{q-3k}}{4} &= \frac{\hbar^2}{2m} \frac{4}{(q+k)^2 - (q-3k)^2} = \frac{\hbar^2}{2m} \frac{4}{k^2 + 6\mathbf{q} \cdot \mathbf{k} + k^2 + 2\mathbf{q} \cdot \mathbf{k}} = \frac{\hbar^2}{2m} \frac{4}{-9k^2 + 8\mathbf{q} \cdot \mathbf{k}} = \frac{\hbar^2}{2m} \frac{4}{-2k^2 + 2\mathbf{q} \cdot \mathbf{k}} \\
d = \frac{\epsilon_{q+k} - \epsilon_{q-2k}}{3} &= \frac{\hbar^2}{2m} \frac{3}{(q-k)^2 - (q-2k)^2} = \frac{\hbar^2}{2m} \frac{3}{k^2 + 4\mathbf{q} \cdot \mathbf{k} + k^2 + 2\mathbf{q} \cdot \mathbf{k}} = \frac{\hbar^2}{2m} \frac{3}{-3k^2 + 6\mathbf{q} \cdot \mathbf{k}} = \frac{\hbar^2}{2m} \frac{3}{-k^2 + 2\mathbf{q} \cdot \mathbf{k}}.
\end{aligned}$$

Then, we compute all the relevant algebraic combinations between the coefficients. Note that  $q^2$  and  $\mathbf{q} \cdot \mathbf{k}$  terms vanish.

$$\begin{aligned}
a - b &= \frac{\hbar^2}{2m} (k^2 + 2\mathbf{q} \cdot \mathbf{k} - 2\mathbf{q} \cdot \mathbf{k}) = \frac{\hbar^2}{2m} (k^2), \quad b - c = \frac{\hbar^2}{2m} (2\mathbf{q} \cdot \mathbf{k} + 2k^2 - 2\mathbf{q} \cdot \mathbf{k}) = \frac{\hbar^2}{2m} (2k^2) \\
c - d &= \frac{\hbar^2}{2m} (-2k^2 + 2\mathbf{q} \cdot \mathbf{k} + k^2 - 2\mathbf{q} \cdot \mathbf{k}) = \frac{\hbar^2}{2m} (-k^2), \quad a - c = \frac{\hbar^2}{2m} (k^2 + 2\mathbf{q} \cdot \mathbf{k} + 2k^2 - 2\mathbf{q} \cdot \mathbf{k}) = \frac{\hbar^2}{2m} (3k^2) \\
b - d &= \frac{\hbar^2}{2m} (2\mathbf{q} \cdot \mathbf{k} + k^2 - 2\mathbf{q} \cdot \mathbf{k}) = \frac{\hbar^2}{2m} (k^2), \quad a - d = \frac{\hbar^2}{2m} (k^2 + 2\mathbf{q} \cdot \mathbf{k} + k^2 - 2\mathbf{q} \cdot \mathbf{k}) = \frac{\hbar^2}{2m} (2k^2).
\end{aligned}$$

Afterwards, we compute all the combinations that are present in the partial fraction decomposition.

$$\begin{aligned}
(a-b)(a-c)(a-d)^2 &= \left(\frac{\hbar^2}{2m}\right)^4 (k^2)^4 (3k^2)^4 (4k^4)^4 = \left(\frac{\hbar^2}{2m}\right)^4 (12k^8)^4, \quad (a-b)(b-c)(b-d)^2 = \left(\frac{\hbar^2}{2m}\right)^4 (k^2)^4 (2k^2)^4 (k^4)^4 = \left(\frac{\hbar^2}{2m}\right)^4 (2k^8)^4, \\
(a-c)(b-c)(c-d)^2 &= \left(\frac{\hbar^2}{2m}\right)^4 (3k^2)^4 (2k^2)^4 (k^4)^4 = \left(\frac{\hbar^2}{2m}\right)^4 (6k^8)^4, \quad (a-d)(b-d)(c-d) = \left(\frac{\hbar^2}{2m}\right)^3 (2k^2)^3 (k^2)^3 (-k^2)^3 = \left(\frac{\hbar^2}{2m}\right)^3 (-2k^6)^3, \\
(a-d)^2(b-d)^2(c-d)^2 &= \left(\frac{\hbar^2}{2m}\right)^6 (4k^{12})^6, \quad (a-b)(b-c) + (a-d)^2 + (b-d)^2 + (c-d)^2 = \left(\frac{\hbar^2}{2m}\right)^2 (2k^4 + 4k^4 + k^4 - 9k^4) = \left(\frac{\hbar^2}{2m}\right)^2 (-k^4).
\end{aligned}$$

Finally, we substitute and perform some straightforward algebra. We also introduce the compact notation  $\epsilon_k = (\hbar^2 k^2)/(2m)$ .

$$\begin{aligned}
[\chi_0^{(5,5)}(\mathbf{k}, z)]_{18} &= - \int \frac{d^3 q}{(2\pi)^3} \frac{(2m)^4}{(\hbar^2)^3} \frac{1}{12k^8} \frac{f_0(\mathbf{q})}{60} \left[ \frac{1}{\hbar z - \epsilon_{q+k} + \epsilon_q} - \frac{6}{\hbar z - \frac{\epsilon_{q+k} - \epsilon_{q-k}}{2}} + \frac{2}{\hbar z - \frac{\epsilon_{q+k} - \epsilon_{q-3k}}{4}} + \frac{3}{\hbar z - \frac{\epsilon_{q+k} - \epsilon_{q-2k}}{3}} + \frac{\hbar^2}{2m} \frac{6k^2}{(\hbar z - \frac{\epsilon_{q+k} - \epsilon_{q-2k}}{3})^2} \right] \Rightarrow \\
[\chi_0^{(5,5)}(\mathbf{k}, z)]_{18} &= - \left(\frac{m}{\hbar^2}\right)^4 \frac{1}{90k^8} \int \frac{d^3 q}{(2\pi)^3} \frac{2f_0(\mathbf{q})}{60} \left[ \frac{1}{\hbar z - \epsilon_{q+k} + \epsilon_q} - \frac{6}{\hbar z - \frac{\epsilon_{q+k} - \epsilon_{q-k}}{2}} + \frac{2}{\hbar z - \frac{\epsilon_{q+k} - \epsilon_{q-3k}}{4}} + \frac{3}{\hbar z - \frac{\epsilon_{q+k} - \epsilon_{q-2k}}{3}} + \frac{6\epsilon_k}{(\hbar z - \frac{\epsilon_{q+k} - \epsilon_{q-2k}}{3})^2} \right] \Rightarrow \\
[\chi_0^{(5,5)}(\mathbf{k}, z)]_{18} &= - \left(\frac{m}{\hbar^2}\right)^4 \frac{1}{180k^8} \int \frac{d^3 q}{(2\pi)^3} \frac{2f_0(\mathbf{q})}{60} \left[ \frac{2}{\hbar z - \epsilon_{q+k} + \epsilon_q} - \frac{24}{2\hbar z - \epsilon_{q+k} + \epsilon_{q-k}} + \frac{16}{4\hbar z - \epsilon_{q+k} + \epsilon_{q-3k}} + \frac{18}{3\hbar z - \epsilon_{q+k} + \epsilon_{q-2k}} + \frac{108\epsilon_k}{(3\hbar z - \epsilon_{q+k} + \epsilon_{q-2k})^2} \right].
\end{aligned}$$

The *nineteenth contribution* is characterized by two simple poles and one triple pole. This becomes apparent from the algebraic identity  $(\epsilon_q + 2\mathbf{k} - \epsilon_{q-3\mathbf{k}})/5 = (\epsilon_q + \mathbf{k} - \epsilon_{q-2\mathbf{k}})/3 = (\epsilon_q - \epsilon_{q-\mathbf{k}})$ . We first identify and calculate the coefficients  $a, b, c$ .

$$\begin{aligned}
[\chi_0^{(5,5)}(\mathbf{k}, z)]_{19} &= - \int \frac{d^3 q}{(2\pi)^3} \frac{5\hbar z - \epsilon_{q+2\mathbf{k}} + \epsilon_{q-3\mathbf{k}}}{(4\hbar z - \epsilon_{q+\mathbf{k}} + \epsilon_{q-3\mathbf{k}})} \frac{2f_0(\mathbf{q})}{(3\hbar z - \epsilon_{q+\mathbf{k}} + \epsilon_{q-2\mathbf{k}})} \frac{(\hbar z - \epsilon_q + \epsilon_{q-\mathbf{k}})}{(2\hbar z - \epsilon_q + \epsilon_{q-\mathbf{k}})} \Rightarrow \\
[\chi_0^{(5,5)}(\mathbf{k}, z)]_{19} &= - \int \frac{d^3 q}{(2\pi)^3} \frac{f_0(\mathbf{q})}{60} \frac{1}{\left[\hbar z - \frac{\epsilon_{q+2\mathbf{k}} - \epsilon_{q-3\mathbf{k}}}{5}\right] \left[\hbar z - \frac{\epsilon_{q+\mathbf{k}} - \epsilon_{q-3\mathbf{k}}}{4}\right] \left[\hbar z - \frac{\epsilon_{q+\mathbf{k}} - \epsilon_{q-2\mathbf{k}}}{3}\right] \left[\hbar z - (\epsilon_q - \epsilon_{q-\mathbf{k}})\right]} \Rightarrow \\
[\chi_0^{(5,5)}(\mathbf{k}, z)]_{19} &= - \int \frac{d^3 q}{(2\pi)^3} \frac{f_0(\mathbf{q})}{60} \frac{1}{\left[\hbar z - (\epsilon_q - \epsilon_{q-\mathbf{k}})\right] \left[\hbar z - \frac{\epsilon_{q+\mathbf{k}} - \epsilon_{q-3\mathbf{k}}}{4}\right] \left[\hbar z - \frac{\epsilon_{q+\mathbf{k}} - \epsilon_{q-\mathbf{k}}}{2}\right] \left[\hbar z - (\epsilon_q - \epsilon_{q-\mathbf{k}})\right]} \Rightarrow \\
[\chi_0^{(5,5)}(\mathbf{k}, z)]_{19} &= - \int \frac{d^3 q}{(2\pi)^3} \frac{f_0(\mathbf{q})}{60} \frac{1}{\left[\hbar z - \frac{\epsilon_{q+\mathbf{k}} - \epsilon_{q-\mathbf{k}}}{2}\right] \left[\hbar z - \frac{\epsilon_{q+\mathbf{k}} - \epsilon_{q-3\mathbf{k}}}{4}\right] \left[\hbar z - (\epsilon_q - \epsilon_{q-\mathbf{k}})\right]^3} \Rightarrow \\
a &= \frac{\epsilon_{q+\mathbf{k}} - \epsilon_{q-\mathbf{k}}}{2} \frac{\hbar^2 (\mathbf{q} + \mathbf{k})^2 - (\mathbf{q} - \mathbf{k})^2}{\hbar^2 (\mathbf{q} + \mathbf{k})^2 - (\mathbf{q} - 3\mathbf{k})^2} = \frac{2}{2m} \frac{\hbar^2 k^2 + 2\mathbf{q} \cdot \mathbf{k} - k^2 + 2\mathbf{q} \cdot \mathbf{k}}{\hbar^2 k^2 + 2\mathbf{q} \cdot \mathbf{k} - k^2 + 2\mathbf{q} \cdot \mathbf{k}} = \frac{\hbar^2}{2m} \frac{4\mathbf{q} \cdot \mathbf{k}}{2} = \frac{\hbar^2}{2m} (2\mathbf{q} \cdot \mathbf{k}) \\
b &= \frac{\epsilon_{q+\mathbf{k}} - \epsilon_{q-3\mathbf{k}}}{4} \frac{\hbar^2 (\mathbf{q} + \mathbf{k})^2 - (\mathbf{q} - 3\mathbf{k})^2}{\hbar^2 k^2 + 2\mathbf{q} \cdot \mathbf{k} - 9k^2 + 6\mathbf{q} \cdot \mathbf{k}} = \frac{2}{2m} \frac{\hbar^2 k^2 + 2\mathbf{q} \cdot \mathbf{k} - 9k^2 + 6\mathbf{q} \cdot \mathbf{k}}{\hbar^2 k^2 + 2\mathbf{q} \cdot \mathbf{k} - 9k^2 + 6\mathbf{q} \cdot \mathbf{k}} = \frac{\hbar^2}{2m} \frac{-2k^2 + 2\mathbf{q} \cdot \mathbf{k}}{4} \\
c &= (\epsilon_q - \epsilon_{q-\mathbf{k}}) = \frac{\hbar^2}{2m} [q^2 - (\mathbf{q} - \mathbf{k})^2] = \frac{\hbar^2}{2m} (-k^2 + 2\mathbf{q} \cdot \mathbf{k}).
\end{aligned}$$

Then, we compute all the relevant algebraic combinations between the coefficients. Note that  $q^2$  and  $\mathbf{q} \cdot \mathbf{k}$  terms vanish.

$$\begin{aligned}
a - b &= \frac{\hbar^2}{2m} (2\mathbf{q} \cdot \mathbf{k} + 2k^2 - 2\mathbf{q} \cdot \mathbf{k}) = \frac{\hbar^2}{2m} (2k^2), \quad b - c = \frac{\hbar^2}{2m} (-2k^2 + 2\mathbf{q} \cdot \mathbf{k} + k^2 - 2\mathbf{q} \cdot \mathbf{k}) = \frac{\hbar^2}{2m} (-k^2) \\
a - c &= \frac{\hbar^2}{2m} (2\mathbf{q} \cdot \mathbf{k} + k^2 - 2\mathbf{q} \cdot \mathbf{k}) = \frac{\hbar^2}{2m} (k^2), \quad a + b - 2c = \frac{\hbar^2}{2m} (2\mathbf{q} \cdot \mathbf{k} - 2k^2 + 2\mathbf{q} \cdot \mathbf{k} + 2k^2 - 4\mathbf{q} \cdot \mathbf{k}) = \frac{\hbar^2}{2m} (-2k^2 + 2\mathbf{q} \cdot \mathbf{k}) = 0.
\end{aligned}$$

Afterwards, we compute all the combinations that are present in the partial fraction decomposition.

$$\begin{aligned}
(a - b)(a - c)^3 &= \left(\frac{\hbar^2}{2m}\right)^4 (2k^2)^2 (k^6) = \left(\frac{\hbar^2}{2m}\right)^4 (2k^8), \quad (a - b)(b - c)^3 = \left(\frac{\hbar^2}{2m}\right)^4 (2k^2)^2 (-k^6) = \left(\frac{\hbar^2}{2m}\right)^4 (-2k^8), \\
(a - c)(b - c) &= \left(\frac{\hbar^2}{2m}\right)^2 (k^2)^2 (-k^2) = \left(\frac{\hbar^2}{2m}\right)^2 (-k^4), \quad (a - c)^2 (b - c)^2 = \left(\frac{\hbar^2}{2m}\right)^4 (k^8), \\
(a - c)^3 (b - c)^3 &= \left(\frac{\hbar^2}{2m}\right)^6 (-k^{12}), \quad (a - b)^2 + 3(a - c)(b - c) = \left(\frac{\hbar^2}{2m}\right)^2 (4k^4 - 3k^4) = \left(\frac{\hbar^2}{2m}\right)^2 (k^4).
\end{aligned}$$

Finally, we substitute and perform some straightforward algebra. We also introduce the compact notation  $\epsilon_{\mathbf{k}} = (\hbar^2 k^2)/(2m)$ .

$$\begin{aligned}
[\chi_0^{(5,5)}(\mathbf{k}, z)]_{19} &= - \int \frac{d^3 q}{(2\pi)^3} \frac{(2m)^4}{\hbar^2} \frac{1}{60} \frac{f_0(\mathbf{q})}{\left[\hbar z - \frac{\epsilon_{q+\mathbf{k}} - \epsilon_{q-\mathbf{k}}}{2}\right] \left[\hbar z - \frac{\epsilon_{q+\mathbf{k}} - \epsilon_{q-3\mathbf{k}}}{4}\right] \left[\hbar z - \epsilon_q + \epsilon_{q-\mathbf{k}}\right] \left[\hbar z - \epsilon_q + \epsilon_{q-\mathbf{k}}\right]^3} \Rightarrow \\
[\chi_0^{(5,5)}(\mathbf{k}, z)]_{19} &= - \left(\frac{m}{\hbar^2}\right)^4 \frac{1}{15k^8} \int \frac{d^3 q}{(2\pi)^3} \frac{2f_0(\mathbf{q})}{\left[\hbar z - \frac{\epsilon_{q+\mathbf{k}} - \epsilon_{q-\mathbf{k}}}{2}\right] \left[\hbar z - \frac{\epsilon_{q+\mathbf{k}} - \epsilon_{q-3\mathbf{k}}}{4}\right] \left[\hbar z - \epsilon_q + \epsilon_{q-\mathbf{k}}\right] \left[\hbar z - \epsilon_q + \epsilon_{q-\mathbf{k}}\right]^3} \Rightarrow \\
[\chi_0^{(5,5)}(\mathbf{k}, z)]_{19} &= - \left(\frac{m}{\hbar^2}\right)^4 \frac{1}{180k^8} \int \frac{d^3 q}{(2\pi)^3} \frac{2f_0(\mathbf{q})}{\left[\hbar z - \epsilon_q + \epsilon_{q-\mathbf{k}} + \epsilon_{q-\mathbf{k}}\right] \left[\hbar z - \epsilon_q + \epsilon_{q-\mathbf{k}} + \epsilon_{q-3\mathbf{k}}\right] \left[\hbar z - \epsilon_q + \epsilon_{q-\mathbf{k}}\right] \left[\hbar z - \epsilon_q + \epsilon_{q-\mathbf{k}}\right]^3}.
\end{aligned}$$

The *twentyeth contribution* is characterized by two simple poles and one triple pole. This becomes apparent from the algebraic identity  $(\epsilon_{\mathbf{q}+3\mathbf{k}} - \epsilon_{\mathbf{q}-2\mathbf{k}})/5 = (\epsilon_{\mathbf{q}+2\mathbf{k}} - \epsilon_{\mathbf{q}-\mathbf{k}})/3 = (\epsilon_{\mathbf{q}+\mathbf{k}} - \epsilon_{\mathbf{q}})$ . We first identify and calculate the coefficients  $a, b, c$ .

$$\begin{aligned}
[\chi_0^{(5,5)}(\mathbf{k}, z)]_{20} &= + \int \frac{d^3q}{(2\pi)^3} \frac{2f_0(\mathbf{q})}{(5\hbar z - \epsilon_{\mathbf{q}+3\mathbf{k}} + \epsilon_{\mathbf{q}-2\mathbf{k}})(4\hbar z - \epsilon_{\mathbf{q}+3\mathbf{k}} + \epsilon_{\mathbf{q}-\mathbf{k}})(3\hbar z - \epsilon_{\mathbf{q}+2\mathbf{k}} + \epsilon_{\mathbf{q}-\mathbf{k}})(2\hbar z - \epsilon_{\mathbf{q}+\mathbf{k}} + \epsilon_{\mathbf{q}-\mathbf{k}})(\hbar z - \epsilon_{\mathbf{q}+\mathbf{k}} + \epsilon_{\mathbf{q}})} \Rightarrow \\
[\chi_0^{(5,5)}(\mathbf{k}, z)]_{20} &= + \int \frac{d^3q}{(2\pi)^3} \frac{f_0(\mathbf{q})}{60} \left[ \hbar z - \frac{\epsilon_{\mathbf{q}+3\mathbf{k}} - \epsilon_{\mathbf{q}-2\mathbf{k}}}{5} \right] \left[ \hbar z - \frac{\epsilon_{\mathbf{q}+3\mathbf{k}} - \epsilon_{\mathbf{q}-\mathbf{k}}}{4} \right] \left[ \hbar z - \frac{\epsilon_{\mathbf{q}+2\mathbf{k}} - \epsilon_{\mathbf{q}-\mathbf{k}}}{3} \right] \left[ \hbar z - \frac{\epsilon_{\mathbf{q}+\mathbf{k}} - \epsilon_{\mathbf{q}-\mathbf{k}}}{2} \right] \left[ \hbar z - (\epsilon_{\mathbf{q}+\mathbf{k}} - \epsilon_{\mathbf{q}}) \right] \Rightarrow \\
[\chi_0^{(5,5)}(\mathbf{k}, z)]_{20} &= + \int \frac{d^3q}{(2\pi)^3} \frac{f_0(\mathbf{q})}{60} \left[ \hbar z - (\epsilon_{\mathbf{q}+\mathbf{k}} - \epsilon_{\mathbf{q}}) \right] \left[ \hbar z - \frac{\epsilon_{\mathbf{q}+3\mathbf{k}} - \epsilon_{\mathbf{q}-\mathbf{k}}}{4} \right] \left[ \hbar z - (\epsilon_{\mathbf{q}+\mathbf{k}} - \epsilon_{\mathbf{q}}) \right] \left[ \hbar z - \frac{\epsilon_{\mathbf{q}+\mathbf{k}} - \epsilon_{\mathbf{q}-\mathbf{k}}}{2} \right] \left[ \hbar z - (\epsilon_{\mathbf{q}+\mathbf{k}} - \epsilon_{\mathbf{q}}) \right] \Rightarrow \\
[\chi_0^{(5,5)}(\mathbf{k}, z)]_{20} &= + \int \frac{d^3q}{(2\pi)^3} \frac{f_0(\mathbf{q})}{60} \left[ \hbar z - \frac{\epsilon_{\mathbf{q}+\mathbf{k}} - \epsilon_{\mathbf{q}-\mathbf{k}}}{2} \right] \left[ \hbar z - \frac{\epsilon_{\mathbf{q}+3\mathbf{k}} - \epsilon_{\mathbf{q}-\mathbf{k}}}{4} \right] \left[ \hbar z - (\epsilon_{\mathbf{q}+\mathbf{k}} - \epsilon_{\mathbf{q}}) \right]^3 \Rightarrow \\
a &= \frac{\epsilon_{\mathbf{q}+2\mathbf{k}} - \epsilon_{\mathbf{q}}}{2} = \frac{\hbar^2}{2m} \frac{(\mathbf{q} + 2\mathbf{k})^2 - q^2}{2} = \frac{\hbar^2}{2m} \frac{4k^2 + 4\mathbf{q} \cdot \mathbf{k}}{2} = \frac{\hbar^2}{2m} (2k^2 + 2\mathbf{q} \cdot \mathbf{k}) \\
b &= \frac{\epsilon_{\mathbf{q}+2\mathbf{k}} - \epsilon_{\mathbf{q}-2\mathbf{k}}}{4} = \frac{\hbar^2}{2m} \frac{(\mathbf{q} + 2\mathbf{k})^2 - (\mathbf{q} - 2\mathbf{k})^2}{4} = \frac{\hbar^2}{2m} \frac{4k^2 + 4\mathbf{q} \cdot \mathbf{k} - 4k^2 + 4\mathbf{q} \cdot \mathbf{k}}{4} = \frac{\hbar^2}{2m} \frac{8\mathbf{q} \cdot \mathbf{k}}{4} = \frac{\hbar^2}{2m} (2\mathbf{q} \cdot \mathbf{k}) \\
c &= (\epsilon_{\mathbf{q}+\mathbf{k}} - \epsilon_{\mathbf{q}}) = \frac{\hbar^2}{2m} [(\mathbf{q} + \mathbf{k})^2 - q^2] = \frac{\hbar^2}{2m} (k^2 + 2\mathbf{q} \cdot \mathbf{k}).
\end{aligned}$$

Then, we compute all the relevant algebraic combinations between the coefficients. Note that  $q^2$  and  $\mathbf{q} \cdot \mathbf{k}$  terms vanish.

$$\begin{aligned}
a - b &= \frac{\hbar^2}{2m} (2k^2 + 2\mathbf{q} \cdot \mathbf{k} - 2\mathbf{q} \cdot \mathbf{k}) = \frac{\hbar^2}{2m} (2k^2), \quad b - c = \frac{\hbar^2}{2m} (2\mathbf{q} \cdot \mathbf{k} - k^2 - 2\mathbf{q} \cdot \mathbf{k}) = \frac{\hbar^2}{2m} (-k^2) \\
a - c &= \frac{\hbar^2}{2m} (2k^2 + 2\mathbf{q} \cdot \mathbf{k} - k^2 - 2\mathbf{q} \cdot \mathbf{k}) = \frac{\hbar^2}{2m} (k^2), \quad a + b - 2c = \frac{\hbar^2}{2m} (2k^2 + 2\mathbf{q} \cdot \mathbf{k} + 2\mathbf{q} \cdot \mathbf{k} - 2k^2 - 4\mathbf{q} \cdot \mathbf{k}) = \frac{\hbar^2}{2m} (2k^2 - 2k^2) = 0.
\end{aligned}$$

Afterwards, we compute all the combinations that are present in the partial fraction decomposition.

$$\begin{aligned}
(a - b)(a - c)^3 &= \left( \frac{\hbar^2}{2m} \right)^4 (2k^2)(k^6) = \left( \frac{\hbar^2}{2m} \right)^4 (2k^8), \quad (a - b)(b - c)^3 = \left( \frac{\hbar^2}{2m} \right)^4 (2k^2)(-k^6) = \left( \frac{\hbar^2}{2m} \right)^4 (-2k^8), \\
(a - c)(b - c)^2 &= \left( \frac{\hbar^2}{2m} \right)^2 (k^2)(-k^2) = \left( \frac{\hbar^2}{2m} \right)^2 (-k^4), \quad (a - c)^2(b - c)^2 = \left( \frac{\hbar^2}{2m} \right)^4 (k^8), \\
(a - c)^3(b - c)^3 &= \left( \frac{\hbar^2}{2m} \right)^6 (-k^{12}), \quad (a - b)^2 + 3(a - c)(b - c) = \left( \frac{\hbar^2}{2m} \right)^2 (4k^4 - 3k^4) = \left( \frac{\hbar^2}{2m} \right)^2 (k^4).
\end{aligned}$$

Finally, we substitute and perform some straightforward algebra. We also introduce the compact notation  $\epsilon_{\mathbf{k}} = (\hbar^2 k^2)/(2m)$ .

$$\begin{aligned}
[\chi_0^{(5,5)}(\mathbf{k}, z)]_{20} &= + \int \frac{d^3q}{(2\pi)^3} \left( \frac{2m}{\hbar^2} \right)^4 \frac{f_0(\mathbf{q})}{60} \frac{1}{2k^8} \left[ \frac{1}{\hbar z - \frac{\epsilon_{\mathbf{q}+\mathbf{k}} - \epsilon_{\mathbf{q}-\mathbf{k}}}{2}} + \frac{1}{\hbar z - \frac{\epsilon_{\mathbf{q}+3\mathbf{k}} - \epsilon_{\mathbf{q}-\mathbf{k}}}{4}} - \frac{2}{\hbar z - \epsilon_{\mathbf{q}+\mathbf{k}} + \epsilon_{\mathbf{q}}} - \left( \frac{\hbar^2}{2m} \right)^2 \frac{2k^4}{(\hbar z - \epsilon_{\mathbf{q}+\mathbf{k}} + \epsilon_{\mathbf{q}})^3} \right] \Rightarrow \\
[\chi_0^{(5,5)}(\mathbf{k}, z)]_{20} &= + \left( \frac{m}{\hbar^2} \right)^4 \frac{1}{15k^8} \int \frac{d^3q}{(2\pi)^3} \frac{2f_0(\mathbf{q})}{(2\pi)^3} \left[ \frac{1}{\hbar z - \frac{\epsilon_{\mathbf{q}+\mathbf{k}} - \epsilon_{\mathbf{q}-\mathbf{k}}}{2}} + \frac{1}{\hbar z - \frac{\epsilon_{\mathbf{q}+3\mathbf{k}} - \epsilon_{\mathbf{q}-\mathbf{k}}}{4}} - \frac{2}{\hbar z - \epsilon_{\mathbf{q}+\mathbf{k}} + \epsilon_{\mathbf{q}}} - \frac{2c_k^2}{(\hbar z - \epsilon_{\mathbf{q}+\mathbf{k}} + \epsilon_{\mathbf{q}})^3} \right] \Rightarrow \\
[\chi_0^{(5,5)}(\mathbf{k}, z)]_{20} &= + \left( \frac{m}{\hbar^2} \right)^4 \frac{1}{180k^8} \int \frac{d^3q}{(2\pi)^3} \frac{2f_0(\mathbf{q})}{(2\pi)^3} \left[ \frac{24}{2\hbar z - \epsilon_{\mathbf{q}+\mathbf{k}} + \epsilon_{\mathbf{q}-\mathbf{k}}} + \frac{48}{4\hbar z - \epsilon_{\mathbf{q}+3\mathbf{k}} + \epsilon_{\mathbf{q}-\mathbf{k}}} - \frac{24}{\hbar z - \epsilon_{\mathbf{q}+\mathbf{k}} + \epsilon_{\mathbf{q}}} - \frac{24c_k^2}{(\hbar z - \epsilon_{\mathbf{q}+\mathbf{k}} + \epsilon_{\mathbf{q}})^3} \right].
\end{aligned}$$

The *twenty-first contribution* is characterized by one double pole and one triple pole. This becomes apparent from the algebraic identities  $(\epsilon_q + \mathbf{k} - \epsilon_{q-3\mathbf{k}})/4 = (\epsilon_q - \epsilon_{q-2\mathbf{k}})/2$  and  $(\epsilon_q + 2\mathbf{k} - \epsilon_{q-3\mathbf{k}})/5 = (\epsilon_q + \mathbf{k} - \epsilon_{q-2\mathbf{k}})/3 = (\epsilon_q - \epsilon_{q-\mathbf{k}})$ . We first identify and calculate the coefficients  $a, b$ .

$$\begin{aligned}
[\chi_0^{(5,5)}(\mathbf{k}, z)]_{21} &= - \int \frac{d^3 q}{(2\pi)^3} \frac{2f_0(\mathbf{q})}{(5\hbar z - \epsilon_q + 2\mathbf{k} + \epsilon_{q-3\mathbf{k}})(4\hbar z - \epsilon_q + \mathbf{k} + \epsilon_{q-2\mathbf{k}})(2\hbar z - \epsilon_q + \epsilon_{q-2\mathbf{k}})(\hbar z - \epsilon_q + \epsilon_{q-\mathbf{k}})} \\
[\chi_0^{(5,5)}(\mathbf{k}, z)]_{21} &= - \int \frac{d^3 q}{(2\pi)^3} \frac{f_0(\mathbf{q})}{60} \frac{1}{\left[\hbar z - \frac{\epsilon_q + 2\mathbf{k} - \epsilon_{q-3\mathbf{k}}}{5}\right] \left[\hbar z - \frac{\epsilon_q + \mathbf{k} - \epsilon_{q-2\mathbf{k}}}{4}\right] \left[\hbar z - \frac{\epsilon_q - \epsilon_{q-2\mathbf{k}}}{3}\right] \left[\hbar z - (\epsilon_q - \epsilon_{q-\mathbf{k}})\right]} \\
[\chi_0^{(5,5)}(\mathbf{k}, z)]_{21} &= - \int \frac{d^3 q}{(2\pi)^3} \frac{f_0(\mathbf{q})}{60} \frac{1}{\left[\hbar z - (\epsilon_q - \epsilon_{q-\mathbf{k}})\right] \left[\hbar z - \frac{\epsilon_q - \epsilon_{q-2\mathbf{k}}}{2}\right] \left[\hbar z - (\epsilon_q - \epsilon_{q-2\mathbf{k}})\right] \left[\hbar z - (\epsilon_q - \epsilon_{q-\mathbf{k}})\right]} \\
[\chi_0^{(5,5)}(\mathbf{k}, z)]_{21} &= - \int \frac{d^3 q}{(2\pi)^3} \frac{f_0(\mathbf{q})}{60} \frac{1}{\left[\hbar z - \frac{\epsilon_q - \epsilon_{q-2\mathbf{k}}}{2}\right]^2 \left[\hbar z - (\epsilon_q - \epsilon_{q-\mathbf{k}})\right]^3} \\
a = \frac{\epsilon_q - \epsilon_{q-2\mathbf{k}}}{2} &= \frac{\hbar^2}{2m} \frac{q^2 - (\mathbf{q} - 2\mathbf{k})^2}{2} = \frac{\hbar^2}{2m} \frac{-4k^2 + 4\mathbf{q} \cdot \mathbf{k}}{2} = \frac{\hbar^2}{2m} (-2k^2 + 2\mathbf{q} \cdot \mathbf{k}) \\
b = (\epsilon_q - \epsilon_{q-\mathbf{k}}) &= \frac{\hbar^2}{2m} [q^2 - (\mathbf{q} - \mathbf{k})^2] = \frac{\hbar^2}{2m} (-k^2 + 2\mathbf{q} \cdot \mathbf{k}) .
\end{aligned}$$

Then, we compute all the relevant algebraic combinations between the coefficients. Note that  $q^2$  and  $\mathbf{q} \cdot \mathbf{k}$  terms vanish.

$$\begin{aligned}
a - b &= \frac{\hbar^2}{2m} (-2k^2 + 2\mathbf{q} \cdot \mathbf{k} + k^2 - 2\mathbf{q} \cdot \mathbf{k}) = \frac{\hbar^2}{2m} (-2k^2 + k^2) = -\frac{\hbar^2}{2m} (k^2) , \\
(a - b)^3 &= -\left(\frac{\hbar^2}{2m}\right)^3 (k^6) , \\
(a - b)^2 &= +\left(\frac{\hbar^2}{2m}\right)^2 (k^4) \\
(a - b)^4 &= +\left(\frac{\hbar^2}{2m}\right)^4 (k^8) .
\end{aligned}$$

Finally, we substitute and perform some straightforward algebra. We also introduce the compact notation  $\epsilon_{\mathbf{k}} = (\hbar^2 k^2)/(2m)$ .

$$\begin{aligned}
[\chi_0^{(5,5)}(\mathbf{k}, z)]_{21} &= - \int \frac{d^3 q}{(2\pi)^3} \left( \frac{2m}{\hbar^2} \right)^4 \frac{1}{k^8} \frac{f_0(\mathbf{q})}{60} \left[ -\frac{3}{\hbar z - \frac{\epsilon_q - \epsilon_{q-2\mathbf{k}}}{2}} + \frac{3}{\hbar z - \epsilon_q + \epsilon_{q-\mathbf{k}}} - \frac{\hbar^2}{2m} \frac{k^2}{\left(\hbar z - \frac{\epsilon_q - \epsilon_{q-2\mathbf{k}}}{2}\right)^2} - \frac{\hbar^2}{2m} \frac{2k^2}{(\hbar z - \epsilon_q + \epsilon_{q-\mathbf{k}})^2} + \left(\frac{\hbar^2}{2m}\right)^2 \frac{k^4}{(\hbar z - \epsilon_q + \epsilon_{q-\mathbf{k}})^3} \right] \\
[\chi_0^{(5,5)}(\mathbf{k}, z)]_{21} &= - \int \frac{d^3 q}{(2\pi)^3} \left( \frac{2m}{\hbar^2} \right)^4 \frac{1}{k^8} \frac{f_0(\mathbf{q})}{60} \left[ -\frac{3}{\hbar z - \frac{\epsilon_q - \epsilon_{q-2\mathbf{k}}}{2}} + \frac{3}{\hbar z - \epsilon_q + \epsilon_{q-\mathbf{k}}} - \frac{\epsilon_{\mathbf{k}}}{\left(\hbar z - \frac{\epsilon_q - \epsilon_{q-2\mathbf{k}}}{2}\right)^2} - \frac{2\epsilon_{\mathbf{k}}}{(\hbar z - \epsilon_q + \epsilon_{q-\mathbf{k}})^2} + \frac{\epsilon_{\mathbf{k}}^2}{(\hbar z - \epsilon_q + \epsilon_{q-\mathbf{k}})^3} \right] \\
[\chi_0^{(5,5)}(\mathbf{k}, z)]_{21} &= - \int \frac{d^3 q}{(2\pi)^3} \left( \frac{m}{\hbar^2} \right)^4 \frac{16}{4k^8} \frac{f_0(\mathbf{q})}{60} \left[ -\frac{12}{\hbar z - \frac{\epsilon_q - \epsilon_{q-2\mathbf{k}}}{2}} + \frac{12}{\hbar z - \epsilon_q + \epsilon_{q-\mathbf{k}}} - \frac{4\epsilon_{\mathbf{k}}}{\left(\hbar z - \frac{\epsilon_q - \epsilon_{q-2\mathbf{k}}}{2}\right)^2} - \frac{8\epsilon_{\mathbf{k}}}{(\hbar z - \epsilon_q + \epsilon_{q-\mathbf{k}})^2} + \frac{4\epsilon_{\mathbf{k}}^2}{(\hbar z - \epsilon_q + \epsilon_{q-\mathbf{k}})^3} \right] \\
[\chi_0^{(5,5)}(\mathbf{k}, z)]_{21} &= - \int \frac{d^3 q}{(2\pi)^3} \left( \frac{m}{\hbar^2} \right)^4 \frac{1}{k^8} \frac{2f_0(\mathbf{q})}{30} \left[ -\frac{12}{\hbar z - \frac{\epsilon_q - \epsilon_{q-2\mathbf{k}}}{2}} + \frac{12}{\hbar z - \epsilon_q + \epsilon_{q-\mathbf{k}}} - \frac{4\epsilon_{\mathbf{k}}}{\left(\hbar z - \frac{\epsilon_q - \epsilon_{q-2\mathbf{k}}}{2}\right)^2} - \frac{8\epsilon_{\mathbf{k}}}{(\hbar z - \epsilon_q + \epsilon_{q-\mathbf{k}})^2} + \frac{4\epsilon_{\mathbf{k}}^2}{(\hbar z - \epsilon_q + \epsilon_{q-\mathbf{k}})^3} \right] \\
[\chi_0^{(5,5)}(\mathbf{k}, z)]_{21} &= - \left( \frac{m}{\hbar^2} \right)^4 \frac{1}{30k^8} \int \frac{d^3 q}{(2\pi)^3} \frac{2f_0(\mathbf{q})}{60} \left[ -\frac{12}{\hbar z - \frac{\epsilon_q - \epsilon_{q-2\mathbf{k}}}{2}} + \frac{12}{\hbar z - \epsilon_q + \epsilon_{q-\mathbf{k}}} - \frac{4\epsilon_{\mathbf{k}}}{\left(\hbar z - \frac{\epsilon_q - \epsilon_{q-2\mathbf{k}}}{2}\right)^2} - \frac{8\epsilon_{\mathbf{k}}}{(\hbar z - \epsilon_q + \epsilon_{q-\mathbf{k}})^2} + \frac{4\epsilon_{\mathbf{k}}^2}{(\hbar z - \epsilon_q + \epsilon_{q-\mathbf{k}})^3} \right] \\
[\chi_0^{(5,5)}(\mathbf{k}, z)]_{21} &= - \left( \frac{m}{\hbar^2} \right)^4 \frac{1}{180k^8} \int \frac{d^3 q}{(2\pi)^3} \frac{2f_0(\mathbf{q})}{60} \left[ -\frac{144}{2\hbar z - \epsilon_q + \epsilon_{q-2\mathbf{k}}} + \frac{72}{\hbar z - \epsilon_q + \epsilon_{q-\mathbf{k}}} - \frac{96\epsilon_{\mathbf{k}}}{(2\hbar z - \epsilon_q + \epsilon_{q-2\mathbf{k}})^2} - \frac{48\epsilon_{\mathbf{k}}}{(\hbar z - \epsilon_q + \epsilon_{q-\mathbf{k}})^2} + \frac{24\epsilon_{\mathbf{k}}^2}{(\hbar z - \epsilon_q + \epsilon_{q-\mathbf{k}})^3} \right] .
\end{aligned}$$

The *twenty-second contribution* is characterized by one double pole and one triple pole. This becomes apparent from the algebraic identities  $(\epsilon_{q+2k} - \epsilon_{q-2k})/4 = (\epsilon_{q+k} - \epsilon_{q-k})/2$  and  $(\epsilon_{q+3k} - \epsilon_{q-2k})/5 = (\epsilon_{q+k} - \epsilon_q)$ . We first identify and calculate the coefficients  $a, b$ .

$$\begin{aligned}
[\chi_0^{(5,5)}(\mathbf{k}, z)]_{22} &= + \int \frac{d^3 q}{(2\pi)^3} \frac{2f_0(\mathbf{q})}{(5\hbar z - \epsilon_{q+3k} + \epsilon_{q-2k})(4\hbar z - \epsilon_{q+2k} + \epsilon_{q-2k})(3\hbar z - \epsilon_{q+2k} + \epsilon_{q-k})(2\hbar z - \epsilon_{q+k} + \epsilon_{q-k})(\hbar z - \epsilon_{q+k} + \epsilon_q)} \Rightarrow \\
[\chi_0^{(5,5)}(\mathbf{k}, z)]_{22} &= + \int \frac{d^3 q}{(2\pi)^3} \frac{f_0(\mathbf{q})}{60} \frac{1}{\left[\hbar z - \frac{\epsilon_{q+3k} - \epsilon_{q-2k}}{5}\right] \left[\hbar z - \frac{\epsilon_{q+2k} - \epsilon_{q-2k}}{4}\right] \left[\hbar z - \frac{\epsilon_{q+k} - \epsilon_{q-k}}{3}\right] \left[\hbar z - \frac{\epsilon_{q+k} - \epsilon_q}{2}\right] [\hbar z - (\epsilon_{q+k} - \epsilon_q)]} \Rightarrow \\
[\chi_0^{(5,5)}(\mathbf{k}, z)]_{22} &= + \int \frac{d^3 q}{(2\pi)^3} \frac{f_0(\mathbf{q})}{60} \frac{1}{\left[\hbar z - (\epsilon_{q+k} - \epsilon_q)\right] \left[\hbar z - \frac{\epsilon_{q+k} - \epsilon_{q-k}}{2}\right] \left[\hbar z - (\epsilon_{q+k} - \epsilon_q)\right] \left[\hbar z - \frac{\epsilon_{q+k} - \epsilon_{q-k}}{2}\right] [\hbar z - (\epsilon_{q+k} - \epsilon_q)]} \Rightarrow \\
[\chi_0^{(5,5)}(\mathbf{k}, z)]_{22} &= + \int \frac{d^3 q}{(2\pi)^3} \frac{f_0(\mathbf{q})}{60} \frac{1}{\left[\hbar z - \frac{\epsilon_{q+k} - \epsilon_{q-k}}{2}\right]^2 [\hbar z - (\epsilon_{q+k} - \epsilon_q)]^3} \Rightarrow \\
a = \frac{\epsilon_{q+k} - \epsilon_{q-k}}{2} &= \frac{\hbar^2}{2m} \frac{(q + \mathbf{k})^2 - (q - \mathbf{k})^2}{2} = \frac{\hbar^2}{2m} \frac{k^2 + 2\mathbf{q} \cdot \mathbf{k} - k^2 + 2\mathbf{q} \cdot \mathbf{k}}{2} = \frac{\hbar^2}{2m} \frac{4\mathbf{q} \cdot \mathbf{k}}{2} = \frac{\hbar^2}{2m} (2\mathbf{q} \cdot \mathbf{k}) \\
b = (\epsilon_{q+k} - \epsilon_q) &= \frac{\hbar^2}{2m} [(q + \mathbf{k})^2 - q^2] = \frac{\hbar^2}{2m} (k^2 + 2\mathbf{q} \cdot \mathbf{k}) .
\end{aligned}$$

Then, we compute all the relevant algebraic combinations between the coefficients. Note that  $q^2$  and  $\mathbf{q} \cdot \mathbf{k}$  terms vanish.

$$\begin{aligned}
a - b &= \frac{\hbar^2}{2m} (2\mathbf{q} \cdot \mathbf{k} - k^2 - 2\mathbf{q} \cdot \mathbf{k}) = -\frac{\hbar^2}{2m} (k^2) , \\
(a - b)^3 &= -\left(\frac{\hbar^2}{2m}\right)^3 (k^6) , \\
(a - b)^2 &= +\left(\frac{\hbar^2}{2m}\right)^2 (k^4) \\
(a - b)^4 &= +\left(\frac{\hbar^2}{2m}\right)^4 (k^8) .
\end{aligned}$$

Finally, we substitute and perform some straightforward algebra. We also introduce the compact notation  $\epsilon_k = (\hbar^2 k^2)/(2m)$ .

$$\begin{aligned}
[\chi_0^{(5,5)}(\mathbf{k}, z)]_{22} &= + \int \frac{d^3 q}{(2\pi)^3} \frac{(2m)^4}{\hbar^2} \frac{1}{k^8} \frac{f_0(\mathbf{q})}{60} \left[ -\frac{3}{\hbar z - \frac{\epsilon_{q+k} - \epsilon_{q-k}}{2}} + \frac{3}{\hbar z - \epsilon_{q+k} + \epsilon_q} - \frac{\hbar^2}{2m} \frac{k^2}{\left(\hbar z - \frac{\epsilon_{q+k} - \epsilon_{q-k}}{2}\right)^2} - \frac{\hbar^2}{2m} \frac{2k^2}{(\hbar z - \epsilon_{q+k} + \epsilon_q)^2} + \left(\frac{\hbar^2}{2m}\right)^2 \frac{k^4}{(\hbar z - \epsilon_{q+k} + \epsilon_q)^3} \right] \Rightarrow \\
[\chi_0^{(5,5)}(\mathbf{k}, z)]_{22} &= + \int \frac{d^3 q}{(2\pi)^3} \frac{(2m)^4}{\hbar^2} \frac{1}{k^8} \frac{f_0(\mathbf{q})}{60} \left[ -\frac{3}{\hbar z - \frac{\epsilon_{q+k} - \epsilon_{q-k}}{2}} + \frac{3}{\hbar z - \epsilon_{q+k} + \epsilon_q} - \frac{\epsilon_k}{\left(\hbar z - \frac{\epsilon_{q+k} - \epsilon_{q-k}}{2}\right)^2} - \frac{2\epsilon_k}{(\hbar z - \epsilon_{q+k} + \epsilon_q)^2} + \frac{\epsilon_k^2}{(\hbar z - \epsilon_{q+k} + \epsilon_q)^3} \right] \Rightarrow \\
[\chi_0^{(5,5)}(\mathbf{k}, z)]_{22} &= + \int \frac{d^3 q}{(2\pi)^3} \frac{(m)^4}{\hbar^2} \frac{16}{4k^8} \frac{f_0(\mathbf{q})}{60} \left[ -\frac{12}{\hbar z - \frac{\epsilon_{q+k} - \epsilon_{q-k}}{2}} + \frac{12}{\hbar z - \epsilon_{q+k} + \epsilon_q} - \frac{4\epsilon_k}{\left(\hbar z - \frac{\epsilon_{q+k} - \epsilon_{q-k}}{2}\right)^2} - \frac{8\epsilon_k}{(\hbar z - \epsilon_{q+k} + \epsilon_q)^2} + \frac{4\epsilon_k^2}{(\hbar z - \epsilon_{q+k} + \epsilon_q)^3} \right] \Rightarrow \\
[\chi_0^{(5,5)}(\mathbf{k}, z)]_{22} &= + \int \frac{d^3 q}{(2\pi)^3} \frac{(m)^4}{\hbar^2} \frac{2f_0(\mathbf{q})}{k^8} \frac{1}{30} \left[ -\frac{12}{\hbar z - \frac{\epsilon_{q+k} - \epsilon_{q-k}}{2}} + \frac{12}{\hbar z - \epsilon_{q+k} + \epsilon_q} - \frac{4\epsilon_k}{\left(\hbar z - \frac{\epsilon_{q+k} - \epsilon_{q-k}}{2}\right)^2} - \frac{8\epsilon_k}{(\hbar z - \epsilon_{q+k} + \epsilon_q)^2} + \frac{4\epsilon_k^2}{(\hbar z - \epsilon_{q+k} + \epsilon_q)^3} \right] \Rightarrow \\
[\chi_0^{(5,5)}(\mathbf{k}, z)]_{22} &= + \left(\frac{m}{\hbar^2}\right)^4 \frac{1}{30k^8} \int \frac{d^3 q}{(2\pi)^3} \frac{2f_0(\mathbf{q})}{60} \left[ -\frac{12}{\hbar z - \frac{\epsilon_{q+k} - \epsilon_{q-k}}{2}} + \frac{12}{\hbar z - \epsilon_{q+k} + \epsilon_q} - \frac{4\epsilon_k}{\left(\hbar z - \frac{\epsilon_{q+k} - \epsilon_{q-k}}{2}\right)^2} - \frac{8\epsilon_k}{(\hbar z - \epsilon_{q+k} + \epsilon_q)^2} + \frac{4\epsilon_k^2}{(\hbar z - \epsilon_{q+k} + \epsilon_q)^3} \right] \Rightarrow \\
[\chi_0^{(5,5)}(\mathbf{k}, z)]_{22} &= + \left(\frac{m}{\hbar^2}\right)^4 \frac{1}{180k^8} \int \frac{d^3 q}{(2\pi)^3} \frac{2f_0(\mathbf{q})}{60} \left[ -\frac{144}{2\hbar z - \epsilon_{q+k} + \epsilon_{q-k}} + \frac{72}{\hbar z - \epsilon_{q+k} + \epsilon_q} - \frac{96\epsilon_k}{(2\hbar z - \epsilon_{q+k} + \epsilon_{q-k})^2} - \frac{48\epsilon_k}{(\hbar z - \epsilon_{q+k} + \epsilon_q)^2} + \frac{24\epsilon_k^2}{(\hbar z - \epsilon_{q+k} + \epsilon_q)^3} \right] .
\end{aligned}$$

The *twenty-third contribution* is characterized by one simple pole and two double poles. This becomes apparent from the algebraic identities  $(\epsilon_q + 3k - \epsilon_{q-2k})/5 = (\epsilon_q + 2k - \epsilon_{q-k})/3$  and  $(\epsilon_q + 2k - \epsilon_{q-2k})/4 = (\epsilon_q + k - \epsilon_{q-k})/2$ . We first identify and calculate the coefficients  $a, b, c$ .

$$\begin{aligned}
[\chi_0^{(5,5)}(\mathbf{k}, z)]_{23} &= + \int \frac{d^3 q}{(2\pi)^3} \frac{5\hbar z - \epsilon_q + 3k + \epsilon_{q-2k}}{(2\pi)^3} \frac{2f_0(\mathbf{q})}{(2\pi)^3} \frac{(3\hbar z - \epsilon_q + 2k + \epsilon_{q-k})(2\hbar z - \epsilon_q + k + \epsilon_{q-k})(\hbar z - \epsilon_q + \epsilon_{q-k})}{(2\pi)^3} \Rightarrow \\
[\chi_0^{(5,5)}(\mathbf{k}, z)]_{23} &= + \int \frac{d^3 q}{(2\pi)^3} \frac{f_0(\mathbf{q})}{60} \frac{1}{\left[\hbar z - \frac{\epsilon_q + 3k - \epsilon_{q-2k}}{5}\right] \left[\hbar z - \frac{\epsilon_q + 2k - \epsilon_{q-k}}{4}\right] \left[\hbar z - \frac{\epsilon_q + k - \epsilon_{q-k}}{3}\right] \left[\hbar z - (\epsilon_q - \epsilon_{q-k})\right]} \Rightarrow \\
[\chi_0^{(5,5)}(\mathbf{k}, z)]_{23} &= + \int \frac{d^3 q}{(2\pi)^3} \frac{f_0(\mathbf{q})}{60} \frac{1}{\left[\hbar z - (\epsilon_q - \epsilon_{q-k})\right] \left[\hbar z - \frac{\epsilon_q + k - \epsilon_{q-k}}{2}\right]^2 \left[\hbar z - \frac{\epsilon_q + 2k - \epsilon_{q-k}}{3}\right]} \Rightarrow \\
a = \epsilon_q - \epsilon_{q-k} &= \frac{\hbar^2}{2m} [q^2 - (q - \mathbf{k})^2] = \frac{\hbar^2}{2m} (-k^2 + 2\mathbf{q} \cdot \mathbf{k}) \\
b = \frac{\epsilon_q + k - \epsilon_{q-k}}{2} &= \frac{\hbar^2}{2m} \frac{(q + \mathbf{k})^2 - (q - \mathbf{k})^2}{2} = \frac{\hbar^2}{2m} \frac{k^2 + 2\mathbf{q} \cdot \mathbf{k} - k^2 + 2\mathbf{q} \cdot \mathbf{k}}{2} = \frac{\hbar^2}{2m} \frac{4\mathbf{q} \cdot \mathbf{k}}{2} = \frac{\hbar^2}{2m} (2\mathbf{q} \cdot \mathbf{k}) \\
c = \frac{\epsilon_q + 2k - \epsilon_{q-k}}{3} &= \frac{\hbar^2}{2m} \frac{(q + 2\mathbf{k})^2 - (q - \mathbf{k})^2}{3} = \frac{\hbar^2}{2m} \frac{4k^2 + 4\mathbf{q} \cdot \mathbf{k} - k^2 + 2\mathbf{q} \cdot \mathbf{k}}{3} = \frac{\hbar^2}{2m} \frac{3k^2 + 6\mathbf{q} \cdot \mathbf{k}}{3} = \frac{\hbar^2}{2m} (k^2 + 2\mathbf{q} \cdot \mathbf{k}).
\end{aligned}$$

Then, we compute all the relevant algebraic combinations between these three coefficients. Note that  $q^2$  and  $\mathbf{q} \cdot \mathbf{k}$  terms vanish.

$$\begin{aligned}
a - b &= \frac{\hbar^2}{2m} (-k^2 + 2\mathbf{q} \cdot \mathbf{k} - 2\mathbf{q} \cdot \mathbf{k}) = \frac{\hbar^2}{2m} (-k^2), \quad b - c = \frac{\hbar^2}{2m} (2\mathbf{q} \cdot \mathbf{k} - k^2 - 2\mathbf{q} \cdot \mathbf{k}) = \frac{\hbar^2}{2m} (-k^2), \\
a - c &= \frac{\hbar^2}{2m} (-k^2 + 2\mathbf{q} \cdot \mathbf{k} - k^2 - 2\mathbf{q} \cdot \mathbf{k}) = \frac{\hbar^2}{2m} (-k^2 - k^2) = \frac{\hbar^2}{2m} (-2k^2), \quad 2a - 3b + c = \frac{\hbar^2}{2m} (-2k^2 + 4\mathbf{q} \cdot \mathbf{k} - 6\mathbf{q} \cdot \mathbf{k} + k^2 + 2\mathbf{q} \cdot \mathbf{k}) = \frac{\hbar^2}{2m} (-2k^2 + k^2) = \frac{\hbar^2}{2m} (-k^2), \\
2a + b - 3c &= \frac{\hbar^2}{2m} (-2k^2 + 4\mathbf{q} \cdot \mathbf{k} + 2\mathbf{q} \cdot \mathbf{k} - 3k^2 - 6\mathbf{q} \cdot \mathbf{k}) = \frac{\hbar^2}{2m} (-3k^2 - 2k^2) = \frac{\hbar^2}{2m} (-5k^2).
\end{aligned}$$

Afterwards, we compute all the combinations that are present in the partial fraction decomposition.

$$\begin{aligned}
(a-b)^2(a-c)^2 &= \left(\frac{\hbar^2}{2m}\right)^2 (k^4) \left(\frac{\hbar^2}{2m}\right)^2 (4k^4) = \left(\frac{\hbar^2}{2m}\right)^4 (4k^8), \quad (a-b)^2(b-c)^3 = \left(\frac{\hbar^2}{2m}\right)^2 (k^4) \left(\frac{\hbar^2}{2m}\right)^3 (-k^6) = \left(\frac{\hbar^2}{2m}\right)^5 (-k^{10}), \\
(a-c)^2(b-c)^3 &= \left(\frac{\hbar^2}{2m}\right)^2 (4k^4) \left(\frac{\hbar^2}{2m}\right)^3 (-k^6) = \left(\frac{\hbar^2}{2m}\right)^5 (-4k^{10}), \quad (a-b)(b-c)^2 = \frac{\hbar^2}{2m} (-k^2) \left(\frac{\hbar^2}{2m}\right)^2 (k^4) = \left(\frac{\hbar^2}{2m}\right)^3 (-k^6), \\
(a-c)(b-c)^2 &= \frac{\hbar^2}{2m} (-2k^2) \left(\frac{\hbar^2}{2m}\right)^2 (k^4) = \left(\frac{\hbar^2}{2m}\right)^3 (-2k^6).
\end{aligned}$$

Finally, we substitute and perform some straightforward algebra. We also introduce the compact notation  $\epsilon_{\mathbf{k}} = (\hbar^2 k^2)/(2m)$ .

$$\begin{aligned}
[\chi_0^{(5,5)}(\mathbf{k}, z)]_{23} &= + \int \frac{d^3 q}{(2\pi)^3} \frac{(2m)^4}{\left(\frac{\hbar^2}{2m}\right)^3} \frac{1}{4k^8} \frac{f_0(\mathbf{q})}{60} \left[ \frac{1}{\hbar z - \epsilon_q + \epsilon_{q-k}} + \frac{4}{\hbar z - \frac{\epsilon_q + k - \epsilon_{q-k}}{2}} - \frac{5}{\hbar z - \frac{\epsilon_q + 2k - \epsilon_{q-k}}{3}} + \frac{\hbar^2}{2m} \frac{4k^2}{\left(\hbar z - \frac{\epsilon_q + k - \epsilon_{q-k}}{2}\right)^2} + \frac{\hbar^2}{2m} \frac{2k^2}{\left(\hbar z - \frac{\epsilon_q + 2k - \epsilon_{q-k}}{3}\right)^2} \right] \Rightarrow \\
[\chi_0^{(5,5)}(\mathbf{k}, z)]_{23} &= + \int \frac{d^3 q}{(2\pi)^3} \frac{(2m)^4}{\left(\frac{\hbar^2}{2m}\right)^3} \frac{1}{4k^8} \frac{f_0(\mathbf{q})}{60} \left[ \frac{1}{\hbar z - \epsilon_q + \epsilon_{q-k}} + \frac{4}{\hbar z - \frac{\epsilon_q + k - \epsilon_{q-k}}{2}} - \frac{5}{\hbar z - \frac{\epsilon_q + 2k - \epsilon_{q-k}}{3}} + \frac{4\epsilon_{\mathbf{k}}}{\left(\hbar z - \frac{\epsilon_q + k - \epsilon_{q-k}}{2}\right)^2} + \frac{2\epsilon_{\mathbf{k}}}{\left(\hbar z - \frac{\epsilon_q + 2k - \epsilon_{q-k}}{3}\right)^2} \right] \Rightarrow \\
[\chi_0^{(5,5)}(\mathbf{k}, z)]_{23} &= + \left(\frac{m}{\hbar^2}\right)^4 \frac{1}{30k^8} \int \frac{d^3 q}{(2\pi)^3} \frac{2f_0(\mathbf{q})}{60} \left[ \frac{1}{\hbar z - \epsilon_q + \epsilon_{q-k}} + \frac{4}{\hbar z - \frac{\epsilon_q + k - \epsilon_{q-k}}{2}} - \frac{5}{\hbar z - \frac{\epsilon_q + 2k - \epsilon_{q-k}}{3}} + \frac{4\epsilon_{\mathbf{k}}}{\left(\hbar z - \frac{\epsilon_q + k - \epsilon_{q-k}}{2}\right)^2} + \frac{2\epsilon_{\mathbf{k}}}{\left(\hbar z - \frac{\epsilon_q + 2k - \epsilon_{q-k}}{3}\right)^2} \right] \Rightarrow \\
[\chi_0^{(5,5)}(\mathbf{k}, z)]_{23} &= + \left(\frac{m}{\hbar^2}\right)^4 \frac{1}{180k^8} \int \frac{d^3 q}{(2\pi)^3} \frac{2f_0(\mathbf{q})}{60} \left[ \frac{6}{\hbar z - \epsilon_q + \epsilon_{q-k}} + \frac{48}{2\hbar z - \epsilon_q + k + \epsilon_{q-k}} - \frac{90}{3\hbar z - \epsilon_q + 2k + \epsilon_{q-k}} + \frac{96\epsilon_{\mathbf{k}}}{(2\hbar z - \epsilon_q + k + \epsilon_{q-k})^2} + \frac{108\epsilon_{\mathbf{k}}}{(3\hbar z - \epsilon_q + 2k + \epsilon_{q-k})^2} \right].
\end{aligned}$$

The *twenty-fourth contribution* is characterized by one simple pole and two double poles. This becomes apparent from the algebraic identities  $(\epsilon_q + 4\mathbf{k} - \epsilon_q - \mathbf{k})/5 = (\epsilon_q + 3\mathbf{k} - \epsilon_q)/3$  and  $(\epsilon_q + 3\mathbf{k} - \epsilon_q - \mathbf{k})/4 = (\epsilon_q + 2\mathbf{k} - \epsilon_q)/2$ . We first identify and calculate the coefficients  $a, b, c$ .

$$\begin{aligned}
\left[ \chi_0^{(5,5)}(\mathbf{k}, z) \right]_{24} &= - \int \frac{d^3 q}{(2\pi)^3} \frac{2f_0(\mathbf{q})}{(5\hbar z - \epsilon_q + 4\mathbf{k} + \epsilon_q - \mathbf{k})(4\hbar z - \epsilon_q + 3\mathbf{k} + \epsilon_q)(2\hbar z - \epsilon_q + 2\mathbf{k} + \epsilon_q)(\hbar z - \epsilon_q + \mathbf{k} + \epsilon_q)} \Rightarrow \\
\left[ \chi_0^{(5,5)}(\mathbf{k}, z) \right]_{24} &= - \int \frac{d^3 q}{(2\pi)^3} \frac{f_0(\mathbf{q})}{60} \frac{1}{\left[ \hbar z - \frac{\epsilon_q + 4\mathbf{k} - \epsilon_q - \mathbf{k}}{5} \right] \left[ \hbar z - \frac{\epsilon_q + 3\mathbf{k} - \epsilon_q}{4} \right] \left[ \hbar z - \frac{\epsilon_q + 2\mathbf{k} - \epsilon_q}{2} \right] \left[ \hbar z - (\epsilon_q + \mathbf{k} - \epsilon_q) \right]} \Rightarrow \\
\left[ \chi_0^{(5,5)}(\mathbf{k}, z) \right]_{24} &= - \int \frac{d^3 q}{(2\pi)^3} \frac{f_0(\mathbf{q})}{60} \frac{1}{\left[ \hbar z - (\epsilon_q + \mathbf{k} - \epsilon_q) \right] \left[ \hbar z - \frac{\epsilon_q + 2\mathbf{k} - \epsilon_q}{2} \right]^2 \left[ \hbar z - \frac{\epsilon_q + 3\mathbf{k} - \epsilon_q}{3} \right]} \Rightarrow \\
a = \epsilon_q + \mathbf{k} - \epsilon_q &= \frac{\hbar^2}{2m} [(q + \mathbf{k})^2 - q^2] = \frac{\hbar^2}{2m} (k^2 + 2\mathbf{q} \cdot \mathbf{k}) \\
b = \frac{\epsilon_q + 2\mathbf{k} - \epsilon_q}{2} &= \frac{\hbar^2}{2m} \frac{(q + 2\mathbf{k})^2 - q^2}{2} = \frac{\hbar^2}{2m} \frac{4k^2 + 4\mathbf{q} \cdot \mathbf{k}}{2} = \frac{\hbar^2}{2m} (2k^2 + 2\mathbf{q} \cdot \mathbf{k}) \\
c = \frac{\epsilon_q + 3\mathbf{k} - \epsilon_q}{3} &= \frac{\hbar^2}{2m} \frac{(q + 3\mathbf{k})^2 - q^2}{3} = \frac{\hbar^2}{2m} \frac{9k^2 + 6\mathbf{q} \cdot \mathbf{k}}{3} = \frac{\hbar^2}{2m} (3k^2 + 2\mathbf{q} \cdot \mathbf{k}).
\end{aligned}$$

Then, we compute all the relevant algebraic combinations between these three coefficients. Note that  $q^2$  and  $\mathbf{q} \cdot \mathbf{k}$  terms vanish.

$$\begin{aligned}
a - b &= \frac{\hbar^2}{2m} (k^2 + 2\mathbf{q} \cdot \mathbf{k} - 2k^2 - 2\mathbf{q} \cdot \mathbf{k}) = \frac{\hbar^2}{2m} (-2k^2 + k^2) = \frac{\hbar^2}{2m} (-k^2), \quad b - c = \frac{\hbar^2}{2m} (2k^2 + 2\mathbf{q} \cdot \mathbf{k} - 3k^2 - 2\mathbf{q} \cdot \mathbf{k}) = \frac{\hbar^2}{2m} (2k^2 - 3k^2) = \frac{\hbar^2}{2m} (-k^2), \\
a - c &= \frac{\hbar^2}{2m} (k^2 + 2\mathbf{q} \cdot \mathbf{k} - 3k^2 - 2\mathbf{q} \cdot \mathbf{k}) = \frac{\hbar^2}{2m} (-3k^2 + k^2) = \frac{\hbar^2}{2m} (-2k^2), \quad 2a - 3b + c = \frac{\hbar^2}{2m} (2k^2 + 4\mathbf{q} \cdot \mathbf{k} - 6k^2 - 6\mathbf{q} \cdot \mathbf{k} + 3k^2 + 2\mathbf{q} \cdot \mathbf{k}) = \frac{\hbar^2}{2m} (2k^2 - 6k^2 + 3k^2) = \frac{\hbar^2}{2m} (-k^2), \\
2a + b - 3c &= \frac{\hbar^2}{2m} (2k^2 + 4\mathbf{q} \cdot \mathbf{k} + 2k^2 + 2\mathbf{q} \cdot \mathbf{k} - 9k^2 - 6\mathbf{q} \cdot \mathbf{k}) = \frac{\hbar^2}{2m} (-9k^2 + 2k^2 + 2k^2) = \frac{\hbar^2}{2m} (-5k^2).
\end{aligned}$$

Afterwards, we compute all the combinations that are present in the partial fraction decomposition.

$$\begin{aligned}
(a - b)^2(a - c)^2 &= \left( \frac{\hbar^2}{2m} \right)^2 (k^4) \left( \frac{\hbar^2}{2m} \right)^2 (4k^4) = \left( \frac{\hbar^2}{2m} \right)^4 (4k^8), \quad (a - b)^2(b - c)^3 = \left( \frac{\hbar^2}{2m} \right)^2 (k^4) \left( \frac{\hbar^2}{2m} \right)^3 (-k^6) = \left( \frac{\hbar^2}{2m} \right)^5 (-k^{10}), \\
(a - c)^2(b - c)^3 &= \left( \frac{\hbar^2}{2m} \right)^2 (4k^4) \left( \frac{\hbar^2}{2m} \right)^3 (-k^6) = \left( \frac{\hbar^2}{2m} \right)^5 (-4k^{10}), \quad (a - b)(b - c)^2 = \frac{\hbar^2}{2m} (-k^2) \left( \frac{\hbar^2}{2m} \right)^2 (k^4) = \left( \frac{\hbar^2}{2m} \right)^3 (-k^6), \\
(a - c)(b - c)^2 &= \frac{\hbar^2}{2m} (-2k^2) \left( \frac{\hbar^2}{2m} \right)^2 (k^4) = \left( \frac{\hbar^2}{2m} \right)^3 (-2k^6).
\end{aligned}$$

Finally, we substitute and perform some straightforward algebra. We also introduce the compact notation  $\epsilon_{\mathbf{k}} = (\hbar^2 k^2)/(2m)$ .

$$\begin{aligned}
\left[ \chi_0^{(5,5)}(\mathbf{k}, z) \right]_{24} &= - \int \frac{d^3 q}{(2\pi)^3} \frac{(2m)^4}{(\hbar^2)^4} \frac{1}{4k^8} \frac{f_0(\mathbf{q})}{60} \left[ \frac{1}{\hbar z - \epsilon_q + \mathbf{k} + \epsilon_q} + \frac{4}{\hbar z - \frac{\epsilon_q + 2\mathbf{k} - \epsilon_q}{2}} - \frac{4}{\hbar z - \frac{\epsilon_q + 3\mathbf{k} - \epsilon_q}{3}} + \frac{\hbar^2}{2m} \frac{4k^2}{\left( \hbar z - \frac{\epsilon_q + 2\mathbf{k} - \epsilon_q}{2} \right)^2} + \frac{\hbar^2}{2m} \frac{2k^2}{\left( \hbar z - \frac{\epsilon_q + 3\mathbf{k} - \epsilon_q}{3} \right)^2} \right] \Rightarrow \\
\left[ \chi_0^{(5,5)}(\mathbf{k}, z) \right]_{24} &= - \int \frac{d^3 q}{(2\pi)^3} \frac{(2m)^4}{(\hbar^2)^4} \frac{1}{4k^8} \frac{f_0(\mathbf{q})}{60} \left[ \frac{1}{\hbar z - \epsilon_q + \mathbf{k} + \epsilon_q} + \frac{4}{\hbar z - \frac{\epsilon_q + 2\mathbf{k} - \epsilon_q}{2}} - \frac{5}{\hbar z - \frac{\epsilon_q + 3\mathbf{k} - \epsilon_q}{3}} + \frac{4\epsilon_{\mathbf{k}}}{\left( \hbar z - \frac{\epsilon_q + 2\mathbf{k} - \epsilon_q}{2} \right)^2} + \frac{2\epsilon_{\mathbf{k}}}{\left( \hbar z - \frac{\epsilon_q + 3\mathbf{k} - \epsilon_q}{3} \right)^2} \right] \Rightarrow \\
\left[ \chi_0^{(5,5)}(\mathbf{k}, z) \right]_{24} &= - \left( \frac{m}{\hbar^2} \right)^4 \frac{1}{30k^8} \int \frac{d^3 q}{(2\pi)^3} \frac{2f_0(\mathbf{q})}{24} \left[ \frac{1}{\hbar z - \epsilon_q + \mathbf{k} + \epsilon_q} + \frac{4}{\hbar z - \frac{\epsilon_q + 2\mathbf{k} - \epsilon_q}{2}} - \frac{5}{\hbar z - \frac{\epsilon_q + 3\mathbf{k} - \epsilon_q}{3}} + \frac{4\epsilon_{\mathbf{k}}}{\left( \hbar z - \frac{\epsilon_q + 2\mathbf{k} - \epsilon_q}{2} \right)^2} + \frac{2\epsilon_{\mathbf{k}}}{\left( \hbar z - \frac{\epsilon_q + 3\mathbf{k} - \epsilon_q}{3} \right)^2} \right] \Rightarrow \\
\left[ \chi_0^{(5,5)}(\mathbf{k}, z) \right]_{24} &= - \left( \frac{m}{\hbar^2} \right)^4 \frac{1}{180k^8} \int \frac{d^3 q}{(2\pi)^3} \frac{2f_0(\mathbf{q})}{24} \left[ \frac{6}{\hbar z - \epsilon_q + \mathbf{k} + \epsilon_q} + \frac{48}{2\hbar z - \epsilon_q + 2\mathbf{k} + \epsilon_q} - \frac{90}{3\hbar z - \epsilon_q + 3\mathbf{k} + \epsilon_q} + \frac{96\epsilon_{\mathbf{k}}}{\left( 2\hbar z - \epsilon_q + 2\mathbf{k} + \epsilon_q \right)^2} + \frac{108\epsilon_{\mathbf{k}}}{\left( 3\hbar z - \epsilon_q + 3\mathbf{k} + \epsilon_q \right)^2} \right].
\end{aligned}$$



The *twenty-fifth contribution* is characterized by one simple pole and two double poles. This becomes apparent from the algebraic identities  $(\epsilon_q + 2\mathbf{k} - \epsilon_q - 3\mathbf{k})/5 = (\epsilon_q - \epsilon_q - \mathbf{k})$  and  $(\epsilon_q + \mathbf{k} - \epsilon_q - 3\mathbf{k})/4 = (\epsilon_q - \epsilon_q - 2\mathbf{k})/2$ . We first identify and calculate the coefficients  $a, b, c$ .

$$\begin{aligned}
[\chi_0^{(5,5)}(\mathbf{k}, z)]_{25} &= - \int \frac{d^3 q}{(2\pi)^3} \frac{5\hbar z - \epsilon_q + 2\mathbf{k} + \epsilon_q - 3\mathbf{k}}{(2\pi)^3} \frac{4\hbar z - \epsilon_q + \mathbf{k} + \epsilon_q - 3\mathbf{k}}{(2\pi)^3} \frac{2\hbar z - \epsilon_q + \epsilon_q - 2\mathbf{k}}{(2\pi)^3} \frac{2f_0(\mathbf{q})}{(2\pi)^3} \Rightarrow \\
[\chi_0^{(5,5)}(\mathbf{k}, z)]_{25} &= - \int \frac{d^3 q}{(2\pi)^3} \frac{f_0(\mathbf{q})}{60} \frac{1}{60} \left[ \hbar z - \frac{\epsilon_q + 2\mathbf{k} - \epsilon_q - 3\mathbf{k}}{5} \right] \left[ \hbar z - \frac{\epsilon_q + \mathbf{k} - \epsilon_q - 3\mathbf{k}}{4} \right] \left[ \hbar z - \frac{\epsilon_q - \epsilon_q - 2\mathbf{k}}{2} \right] \left[ \hbar z - (\epsilon_q - \epsilon_q - \mathbf{k}) \right] \Rightarrow \\
[\chi_0^{(5,5)}(\mathbf{k}, z)]_{25} &= - \int \frac{d^3 q}{(2\pi)^3} \frac{f_0(\mathbf{q})}{60} \frac{1}{60} \left[ \hbar z - \frac{\epsilon_q - \epsilon_q - 3\mathbf{k}}{3} \right] \left[ \hbar z - \frac{\epsilon_q - \epsilon_q - 2\mathbf{k}}{2} \right] \left[ \hbar z - (\epsilon_q - \epsilon_q - \mathbf{k}) \right]^2 \Rightarrow \\
a &= \frac{\epsilon_q - \epsilon_q - 3\mathbf{k}}{3} = \frac{\hbar^2}{2m} \frac{q^2 - (\mathbf{q} - 3\mathbf{k})^2}{3} = \frac{\hbar^2}{2m} \frac{-9k^2 + 6\mathbf{q} \cdot \mathbf{k}}{3} = \frac{\hbar^2}{2m} (-3k^2 + 2\mathbf{q} \cdot \mathbf{k}) \\
b &= \frac{\epsilon_q - \epsilon_q - 2\mathbf{k}}{2} = \frac{\hbar^2}{2m} \frac{q^2 - (\mathbf{q} - 2\mathbf{k})^2}{2} = \frac{\hbar^2}{2m} \frac{-4k^2 + 4\mathbf{q} \cdot \mathbf{k}}{2} = \frac{\hbar^2}{2m} (-2k^2 + 2\mathbf{q} \cdot \mathbf{k}) \\
c &= \epsilon_q - \epsilon_q - \mathbf{k} = \frac{\hbar^2}{2m} [q^2 - (\mathbf{q} - \mathbf{k})^2] = \frac{\hbar^2}{2m} (-k^2 + 2\mathbf{q} \cdot \mathbf{k}).
\end{aligned}$$

Then, we compute all the relevant algebraic combinations between these three coefficients. Note that  $q^2$  and  $\mathbf{q} \cdot \mathbf{k}$  terms vanish.

$$\begin{aligned}
a - b &= \frac{\hbar^2}{2m} (-3k^2 + 2\mathbf{q} \cdot \mathbf{k} + 2k^2 - 2\mathbf{q} \cdot \mathbf{k}) = \frac{\hbar^2}{2m} (-3k^2 + 2k^2) = \frac{\hbar^2}{2m} (-k^2), \quad b - c = \frac{\hbar^2}{2m} (-2k^2 + 2\mathbf{q} \cdot \mathbf{k} + k^2 - 2\mathbf{q} \cdot \mathbf{k}) = \frac{\hbar^2}{2m} (-2k^2 + k^2) = \frac{\hbar^2}{2m} (-k^2), \\
a - c &= \frac{\hbar^2}{2m} (-3k^2 + 2\mathbf{q} \cdot \mathbf{k} + k^2 - 2\mathbf{q} \cdot \mathbf{k}) = \frac{\hbar^2}{2m} (-3k^2 + k^2) = \frac{\hbar^2}{2m} (-2k^2), \quad 2a - 3b + c = \frac{\hbar^2}{2m} (-6k^2 + 4\mathbf{q} \cdot \mathbf{k} + 6k^2 - 6\mathbf{q} \cdot \mathbf{k} - k^2 + 2\mathbf{q} \cdot \mathbf{k}) = \frac{\hbar^2}{2m} (6k^2 - 6k^2 - k^2) = \frac{\hbar^2}{2m} (-k^2), \\
2a + b - 3c &= \frac{\hbar^2}{2m} (-6k^2 + 4\mathbf{q} \cdot \mathbf{k} - 2k^2 + 2\mathbf{q} \cdot \mathbf{k} + 3k^2 - 6\mathbf{q} \cdot \mathbf{k}) = \frac{\hbar^2}{2m} (-6k^2 - 2k^2 + 3k^2) = \frac{\hbar^2}{2m} (-5k^2).
\end{aligned}$$

Afterwards, we compute all the combinations that are present in the partial fraction decomposition.

$$\begin{aligned}
(a-b)^2(a-c)^2 &= \left( \frac{\hbar^2}{2m} \right)^2 (k^4) \left( \frac{\hbar^2}{2m} \right)^2 (4k^4) = \left( \frac{\hbar^2}{2m} \right)^4 (4k^8), \quad (a-b)^2(b-c)^3 = \left( \frac{\hbar^2}{2m} \right)^2 (k^4) \left( \frac{\hbar^2}{2m} \right)^3 (-k^6) = \left( \frac{\hbar^2}{2m} \right)^5 (-k^{10}), \\
(a-c)^2(b-c)^3 &= \left( \frac{\hbar^2}{2m} \right)^2 (4k^4) \left( \frac{\hbar^2}{2m} \right)^3 (-k^6) = \left( \frac{\hbar^2}{2m} \right)^5 (-4k^{10}), \quad (a-b)(b-c)^2 = \frac{\hbar^2}{2m} (-k^2) \left( \frac{\hbar^2}{2m} \right)^2 (k^4) = \left( \frac{\hbar^2}{2m} \right)^3 (-k^6), \\
(a-c)(b-c)^2 &= \frac{\hbar^2}{2m} (-2k^2) \left( \frac{\hbar^2}{2m} \right)^2 (k^4) = \left( \frac{\hbar^2}{2m} \right)^3 (-2k^6).
\end{aligned}$$

Finally, we substitute and perform some straightforward algebra. We also introduce the compact notation  $\epsilon_{\mathbf{k}} = (\hbar^2 k^2)/(2m)$ .

$$\begin{aligned}
[\chi_0^{(5,5)}(\mathbf{k}, z)]_{25} &= - \int \frac{d^3 q}{(2\pi)^3} \frac{(2m)^4}{(\hbar^2)^3} \frac{1}{4k^8} \frac{f_0(\mathbf{q})}{60} \left[ \frac{1}{\hbar z - \frac{\epsilon_q - \epsilon_q - 3\mathbf{k}}{3}} + \frac{4}{\hbar z - \frac{\epsilon_q - \epsilon_q - 2\mathbf{k}}{2}} - \frac{5}{\hbar z - \epsilon_q + \epsilon_q - \mathbf{k}} + \frac{\hbar^2}{2m} \frac{4k^2}{\left( \hbar z - \frac{\epsilon_q - \epsilon_q - 2\mathbf{k}}{2} \right)^2} + \frac{\hbar^2}{2m} \frac{2k^2}{(\hbar z - \epsilon_q + \epsilon_q - \mathbf{k})^2} \right] \Rightarrow \\
[\chi_0^{(5,5)}(\mathbf{k}, z)]_{25} &= - \int \frac{d^3 q}{(2\pi)^3} \frac{(2m)^4}{(\hbar^2)^3} \frac{1}{4k^8} \frac{f_0(\mathbf{q})}{60} \left[ \frac{1}{\hbar z - \frac{\epsilon_q - \epsilon_q - 3\mathbf{k}}{3}} + \frac{4}{\hbar z - \frac{\epsilon_q - \epsilon_q - 2\mathbf{k}}{2}} - \frac{5}{\hbar z - \epsilon_q + \epsilon_q - \mathbf{k}} + \frac{4\epsilon_{\mathbf{k}}}{\left( \hbar z - \frac{\epsilon_q - \epsilon_q - 2\mathbf{k}}{2} \right)^2} + \frac{2\epsilon_{\mathbf{k}}}{(\hbar z - \epsilon_q + \epsilon_q - \mathbf{k})^2} \right] \Rightarrow \\
[\chi_0^{(5,5)}(\mathbf{k}, z)]_{25} &= - \left( \frac{m}{\hbar^2} \right)^4 \frac{1}{30k^8} \int \frac{d^3 q}{(2\pi)^3} \frac{2f_0(\mathbf{q})}{60} \left[ \frac{1}{\hbar z - \frac{\epsilon_q - \epsilon_q - 3\mathbf{k}}{3}} + \frac{4}{\hbar z - \frac{\epsilon_q - \epsilon_q - 2\mathbf{k}}{2}} - \frac{5}{\hbar z - \epsilon_q + \epsilon_q - \mathbf{k}} + \frac{4\epsilon_{\mathbf{k}}}{\left( \hbar z - \frac{\epsilon_q - \epsilon_q - 2\mathbf{k}}{2} \right)^2} + \frac{2\epsilon_{\mathbf{k}}}{(\hbar z - \epsilon_q + \epsilon_q - \mathbf{k})^2} \right] \Rightarrow \\
[\chi_0^{(5,5)}(\mathbf{k}, z)]_{25} &= - \left( \frac{m}{\hbar^2} \right)^4 \frac{1}{180k^8} \int \frac{d^3 q}{(2\pi)^3} \frac{2f_0(\mathbf{q})}{60} \left[ \frac{18}{3\hbar z - \epsilon_q + \epsilon_q - 3\mathbf{k}} + \frac{48}{2\hbar z - \epsilon_q + \epsilon_q - 2\mathbf{k}} - \frac{30}{\hbar z - \epsilon_q + \epsilon_q - \mathbf{k}} + \frac{96\epsilon_{\mathbf{k}}}{(2\hbar z - \epsilon_q + \epsilon_q - 2\mathbf{k})^2} + \frac{12\epsilon_{\mathbf{k}}}{(\hbar z - \epsilon_q + \epsilon_q - \mathbf{k})^2} \right].
\end{aligned}$$

The *twenty-sixth contribution* is characterized by one simple pole and two double poles. This becomes apparent from the algebraic identities  $(\epsilon_q + 3k - \epsilon_{q-2k})/5 = (\epsilon_q + k - \epsilon_q)$  and  $(\epsilon_q + 2k - \epsilon_{q-2k})/4 = (\epsilon_q + k - \epsilon_{q-k})/2$ . We first identify and calculate the coefficients  $a, b, c$ .

$$\begin{aligned}
[\chi_0^{(5,5)}(\mathbf{k}, z)]_{26} &= + \int \frac{d^3 q}{(2\pi)^3} \frac{2f_0(\mathbf{q})}{(5\hbar z - \epsilon_q + 3k + \epsilon_{q-2k})(4\hbar z - \epsilon_q + 2k + \epsilon_{q-2k})(3\hbar z - \epsilon_q + k + \epsilon_{q-2k})(2\hbar z - \epsilon_q + k + \epsilon_q)(\hbar z - \epsilon_q + k + \epsilon_q)} \Rightarrow \\
[\chi_0^{(5,5)}(\mathbf{k}, z)]_{26} &= + \int \frac{d^3 q}{(2\pi)^3} \frac{f_0(\mathbf{q})}{60} \frac{1}{\left[\hbar z - \frac{\epsilon_q + 3k - \epsilon_{q-2k}}{5}\right] \left[\hbar z - \frac{\epsilon_q + 2k - \epsilon_{q-2k}}{4}\right] \left[\hbar z - \frac{\epsilon_q + k - \epsilon_{q-2k}}{3}\right] \left[\hbar z - (\epsilon_q + k - \epsilon_q)\right]} \Rightarrow \\
[\chi_0^{(5,5)}(\mathbf{k}, z)]_{26} &= + \int \frac{d^3 q}{(2\pi)^3} \frac{f_0(\mathbf{q})}{60} \frac{1}{\left[\hbar z - \frac{\epsilon_q + k - \epsilon_{q-2k}}{3}\right] \left[\hbar z - \frac{\epsilon_q + k - \epsilon_{q-k}}{2}\right]^2 \left[\hbar z - (\epsilon_q + k - \epsilon_q)\right]^2} \Rightarrow \\
a &= \frac{\epsilon_q + k - \epsilon_{q-2k}}{3} = \frac{\hbar^2}{2m} \frac{(q + k)^2 - (q - 2k)^2}{3} = \frac{\hbar^2}{2m} \frac{k^2 + 2q \cdot k - k^2 + 4q \cdot k}{3} = \frac{\hbar^2}{2m} \frac{-3k^2 + 6q \cdot k}{3} = \frac{\hbar^2}{2m} (-k^2 + 2q \cdot k) \\
b &= \frac{\epsilon_q + k - \epsilon_{q-k}}{2} = \frac{\hbar^2}{2m} \frac{(q + k)^2 - (q - k)^2}{2} = \frac{\hbar^2}{2m} \frac{k^2 + 2q \cdot k - k^2 + 2q \cdot k}{2} = \frac{\hbar^2}{2m} \frac{4q \cdot k}{2} = \frac{\hbar^2}{2m} (2q \cdot k) \\
c &= \epsilon_q + k - \epsilon_q = \frac{\hbar^2}{2m} [(q + k)^2 - q^2] = \frac{\hbar^2}{2m} (k^2 + 2q \cdot k).
\end{aligned}$$

Then, we compute all the relevant algebraic combinations between these three coefficients. Note that  $q^2$  and  $q \cdot k$  terms vanish.

$$\begin{aligned}
a - b &= \frac{\hbar^2}{2m} (-k^2 + 2q \cdot k - 2q \cdot k) = \frac{\hbar^2}{2m} (-k^2), \quad b - c = \frac{\hbar^2}{2m} (2q \cdot k - k^2 - 2q \cdot k) = \frac{\hbar^2}{2m} (-k^2), \\
a - c &= \frac{\hbar^2}{2m} (-k^2 + 2q \cdot k - k^2 - 2q \cdot k) = \frac{\hbar^2}{2m} (-2k^2), \quad 2a - 3b + c = \frac{\hbar^2}{2m} (-2k^2 + 4q \cdot k - 6q \cdot k + k^2 + 2q \cdot k) = \frac{\hbar^2}{2m} (-2k^2 + k^2) = \frac{\hbar^2}{2m} (-k^2), \\
2a + b - 3c &= \frac{\hbar^2}{2m} (-2k^2 + 4q \cdot k + 2q \cdot k - 3k^2 - 6q \cdot k) = \frac{\hbar^2}{2m} (-2k^2 - 3k^2) = \frac{\hbar^2}{2m} (-5k^2).
\end{aligned}$$

Afterwards, we compute all the combinations that are present in the partial fraction decomposition.

$$\begin{aligned}
(a - b)^2(a - c)^2 &= \left(\frac{\hbar^2}{2m}\right)^2 (k^4) \left(\frac{\hbar^2}{2m}\right)^2 (4k^4) = \left(\frac{\hbar^2}{2m}\right)^4 (4k^8), \quad (a - b)^2(b - c)^3 = \left(\frac{\hbar^2}{2m}\right)^2 (k^4) \left(\frac{\hbar^2}{2m}\right)^3 (-k^6) = \left(\frac{\hbar^2}{2m}\right)^5 (-k^{10}), \\
(a - c)^2(b - c)^3 &= \left(\frac{\hbar^2}{2m}\right)^2 (4k^4) \left(\frac{\hbar^2}{2m}\right)^3 (-k^6) = \left(\frac{\hbar^2}{2m}\right)^5 (-4k^{10}), \quad (a - b)(b - c)^2 = \frac{\hbar^2}{2m} (-k^2) \left(\frac{\hbar^2}{2m}\right)^2 (k^4) = \left(\frac{\hbar^2}{2m}\right)^3 (-k^6), \\
(a - c)(b - c)^2 &= \frac{\hbar^2}{2m} (-2k^2) \left(\frac{\hbar^2}{2m}\right)^2 (k^4) = \left(\frac{\hbar^2}{2m}\right)^3 (-2k^6).
\end{aligned}$$

Finally, we substitute and perform some straightforward algebra. We also introduce the compact notation  $\epsilon_k = (\hbar^2 k^2)/(2m)$ .

$$\begin{aligned}
[\chi_0^{(5,5)}(\mathbf{k}, z)]_{26} &= + \int \frac{d^3 q}{(2\pi)^3} \left(\frac{2m}{\hbar^2}\right)^4 \frac{1}{4k^8} \frac{f_0(\mathbf{q})}{60} \left[ \frac{1}{\hbar z - \frac{\epsilon_q + k - \epsilon_{q-2k}}{3}} + \frac{4}{\hbar z - \frac{\epsilon_q + k - \epsilon_{q-k}}{2}} - \frac{5}{\hbar z - \epsilon_q + k + \epsilon_q} + \frac{\hbar^2}{2m} \frac{4k^2}{\left(\hbar z - \frac{\epsilon_q + k - \epsilon_{q-k}}{2}\right)^2} + \frac{\hbar^2}{2m} \frac{2k^2}{(\hbar z - \epsilon_q + k + \epsilon_q)^2} \right] \Rightarrow \\
[\chi_0^{(5,5)}(\mathbf{k}, z)]_{26} &= + \int \frac{d^3 q}{(2\pi)^3} \left(\frac{2m}{\hbar^2}\right)^4 \frac{1}{4k^8} \frac{f_0(\mathbf{q})}{60} \left[ \frac{1}{\hbar z - \frac{\epsilon_q + k - \epsilon_{q-2k}}{3}} + \frac{4}{\hbar z - \frac{\epsilon_q + k - \epsilon_{q-k}}{2}} - \frac{5}{\hbar z - \epsilon_q + k + \epsilon_q} + \frac{4\epsilon_k}{\left(\hbar z - \frac{\epsilon_q + k - \epsilon_{q-k}}{2}\right)^2} + \frac{2\epsilon_k}{(\hbar z - \epsilon_q + k + \epsilon_q)^2} \right] \Rightarrow \\
[\chi_0^{(5,5)}(\mathbf{k}, z)]_{26} &= + \left(\frac{m}{\hbar^2}\right)^4 \frac{1}{30k^8} \int \frac{d^3 q}{(2\pi)^3} \frac{2f_0(\mathbf{q})}{60} \left[ \frac{1}{\hbar z - \frac{\epsilon_q + k - \epsilon_{q-2k}}{3}} + \frac{4}{\hbar z - \frac{\epsilon_q + k - \epsilon_{q-k}}{2}} - \frac{5}{\hbar z - \epsilon_q + k + \epsilon_q} + \frac{4\epsilon_k}{\left(\hbar z - \frac{\epsilon_q + k - \epsilon_{q-k}}{2}\right)^2} + \frac{2\epsilon_k}{(\hbar z - \epsilon_q + k + \epsilon_q)^2} \right] \Rightarrow \\
[\chi_0^{(5,5)}(\mathbf{k}, z)]_{26} &= + \left(\frac{m}{\hbar^2}\right)^4 \frac{1}{180k^8} \int \frac{d^3 q}{(2\pi)^3} \frac{2f_0(\mathbf{q})}{60} \left[ \frac{18}{3\hbar z - \epsilon_q + k + \epsilon_{q-2k}} + \frac{48}{2\hbar z - \epsilon_q + k + \epsilon_{q-k}} - \frac{30}{\hbar z - \epsilon_q + k + \epsilon_q} + \frac{96\epsilon_k}{(2\hbar z - \epsilon_q + k + \epsilon_{q-k})^2} + \frac{12\epsilon_k}{(\hbar z - \epsilon_q + k + \epsilon_q)^2} \right].
\end{aligned}$$

The *twenty-seventh contribution* is characterized by one simple pole and two double poles. This becomes apparent from the algebraic identities  $(\epsilon_q + 2k - \epsilon_q - 2k)/4 = (\epsilon_q + k - \epsilon_q - k)/2$  and  $(\epsilon_q + k - \epsilon_q - 2k)/3 = (\epsilon_q - \epsilon_q - k)$ . We first identify and calculate the coefficients  $a, b, c$ .

$$\begin{aligned}
\left[ \chi_0^{(5,5)}(\mathbf{k}, z) \right]_{27} &= + \int \frac{d^3 q}{(2\pi)^3} \frac{5\hbar z - \epsilon_q + 3k + \epsilon_q - 2k}{(2\pi)^3} \frac{4\hbar z - \epsilon_q + 2k + \epsilon_q - 2k}{(2\pi)^3} \frac{2f_0(\mathbf{q})}{(2\pi)^3} \frac{(2\hbar z - \epsilon_q + k + \epsilon_q - k)(\hbar z - \epsilon_q + \epsilon_q - k)}{(2\pi)^3} \Rightarrow \\
\left[ \chi_0^{(5,5)}(\mathbf{k}, z) \right]_{27} &= + \int \frac{d^3 q}{(2\pi)^3} \frac{f_0(\mathbf{q})}{60} \frac{1}{\left[ \hbar z - \frac{\epsilon_q + 3k - \epsilon_q - 2k}{5} \right] \left[ \hbar z - \frac{\epsilon_q + 2k - \epsilon_q - 2k}{4} \right] \left[ \hbar z - \frac{\epsilon_q + k - \epsilon_q - k}{3} \right] \left[ \hbar z - (\epsilon_q - \epsilon_q - k) \right]} \Rightarrow \\
\left[ \chi_0^{(5,5)}(\mathbf{k}, z) \right]_{27} &= + \int \frac{d^3 q}{(2\pi)^3} \frac{f_0(\mathbf{q})}{60} \frac{1}{\left[ \hbar z - \frac{\epsilon_q + 3k - \epsilon_q - 2k}{5} \right] \left[ \hbar z - \frac{\epsilon_q + k - \epsilon_q - k}{2} \right] \left[ \hbar z - (\epsilon_q - \epsilon_q - k) \right]^2} \Rightarrow \\
a &= \frac{\epsilon_q + 3k - \epsilon_q - 2k}{5} = \frac{\hbar^2}{2m} \frac{(q + 3k)^2 - (q - 2k)^2}{5} = \frac{\hbar^2}{2m} \frac{9k^2 + 6q \cdot k - 4k^2 + 4q \cdot k - \hbar^2 5k^2 + 10q \cdot k}{5} = \frac{\hbar^2}{2m} (k^2 + 2q \cdot k) \\
b &= \frac{\epsilon_q + k - \epsilon_q - k}{2} = \frac{\hbar^2}{2m} \frac{(q + k)^2 - (q - k)^2}{2} = \frac{\hbar^2}{2m} \frac{k^2 + 2q \cdot k - k^2 + 2q \cdot k - \hbar^2 4q \cdot k}{2} = \frac{\hbar^2}{2m} \frac{2q \cdot k}{2} = \frac{\hbar^2}{2m} (2q \cdot k) \\
c &= \epsilon_q - \epsilon_q - k = \frac{\hbar^2}{2m} [q^2 - (q - k)^2] = \frac{\hbar^2}{2m} (-k^2 + 2q \cdot k)
\end{aligned}$$

Then, we compute all the relevant algebraic combinations between these three coefficients. Note that  $q^2$  and  $q \cdot k$  terms vanish.

$$\begin{aligned}
a - b &= \frac{\hbar^2}{2m} (k^2 + 2q \cdot k - 2q \cdot k) = \frac{\hbar^2}{2m} (k^2), \quad b - c = \frac{\hbar^2}{2m} (2q \cdot k + k^2 - 2q \cdot k) = \frac{\hbar^2}{2m} (k^2), \\
a - c &= \frac{\hbar^2}{2m} (k^2 + 2q \cdot k + k^2 - 2q \cdot k) = \frac{\hbar^2}{2m} (k^2 + k^2) = \frac{\hbar^2}{2m} (2k^2), \quad 2a - 3b + c = \frac{\hbar^2}{2m} (2k^2 + 4q \cdot k - k^2 + 2q \cdot k) = \frac{\hbar^2}{2m} (2k^2 - k^2) = \frac{\hbar^2}{2m} (k^2), \\
2a + b - 3c &= \frac{\hbar^2}{2m} (2k^2 + 4q \cdot k + 2q \cdot k + 3k^2 - 6q \cdot k) = \frac{\hbar^2}{2m} (2k^2 + 3k^2) = \frac{\hbar^2}{2m} (5k^2).
\end{aligned}$$

Afterwards, we compute all the combinations that are present in the partial fraction decomposition.

$$\begin{aligned}
(a - b)^2 (a - c)^2 &= \left( \frac{\hbar^2}{2m} \right)^2 (k^4) \left( \frac{\hbar^2}{2m} \right)^2 (4k^8) = \left( \frac{\hbar^2}{2m} \right)^4 (4k^8), \quad (a - b)^2 (b - c)^3 = \left( \frac{\hbar^2}{2m} \right)^2 (k^4) \left( \frac{\hbar^2}{2m} \right)^3 (k^6) = \left( \frac{\hbar^2}{2m} \right)^5 (k^{10}), \\
(a - c)^2 (b - c)^3 &= \left( \frac{\hbar^2}{2m} \right)^2 (4k^4) \left( \frac{\hbar^2}{2m} \right)^3 (k^6) = \left( \frac{\hbar^2}{2m} \right)^5 (4k^{10}), \quad (a - b)(b - c)^2 = \frac{\hbar^2}{2m} (k^2) \left( \frac{\hbar^2}{2m} \right)^2 (k^4) = \left( \frac{\hbar^2}{2m} \right)^3 (k^6), \\
(a - c)(b - c)^2 &= \frac{\hbar^2}{2m} (2k^2) \left( \frac{\hbar^2}{2m} \right)^2 (k^4) = \left( \frac{\hbar^2}{2m} \right)^3 (2k^6).
\end{aligned}$$

Finally, we substitute and perform some straightforward algebra. We also introduce the compact notation  $\epsilon_k = (\hbar^2 k^2)/(2m)$ .

$$\begin{aligned}
\left[ \chi_0^{(5,5)}(\mathbf{k}, z) \right]_{27} &= + \int \frac{d^3 q}{(2\pi)^3} \left( \frac{2m}{\hbar^2} \right)^4 \frac{1}{4k^8} \frac{f_0(\mathbf{q})}{60} \left[ \frac{1}{\hbar z - \frac{\epsilon_q + 3k - \epsilon_q - 2k}{5}} + \frac{4}{\hbar z - \frac{\epsilon_q + k - \epsilon_q - k}{2}} - \frac{5}{\hbar z - \epsilon_q + \epsilon_q - k} - \frac{\hbar^2}{2m} \frac{4k^2}{\left( \hbar z - \frac{\epsilon_q + k - \epsilon_q - k}{2} \right)^2} - \frac{\hbar^2}{2m} \frac{2k^2}{(\hbar z - \epsilon_q + \epsilon_q - k)^2} \right] \Rightarrow \\
\left[ \chi_0^{(5,5)}(\mathbf{k}, z) \right]_{27} &= + \int \frac{d^3 q}{(2\pi)^3} \left( \frac{2m}{\hbar^2} \right)^4 \frac{1}{4k^8} \frac{f_0(\mathbf{q})}{60} \left[ \frac{1}{\hbar z - \frac{\epsilon_q + 3k - \epsilon_q - 2k}{5}} + \frac{4}{\hbar z - \frac{\epsilon_q + k - \epsilon_q - k}{2}} - \frac{5}{\hbar z - \epsilon_q + \epsilon_q - k} - \frac{4\epsilon_k}{\left( \hbar z - \frac{\epsilon_q + k - \epsilon_q - k}{2} \right)^2} - \frac{2\epsilon_k}{(\hbar z - \epsilon_q + \epsilon_q - k)^2} \right] \Rightarrow \\
\left[ \chi_0^{(5,5)}(\mathbf{k}, z) \right]_{27} &= + \left( \frac{m}{\hbar^2} \right)^4 \frac{1}{30k^8} \int \frac{d^3 q}{(2\pi)^3} \frac{2f_0(\mathbf{q})}{60} \left[ \frac{1}{\hbar z - \frac{\epsilon_q + 3k - \epsilon_q - 2k}{5}} + \frac{4}{\hbar z - \frac{\epsilon_q + k - \epsilon_q - k}{2}} - \frac{5}{\hbar z - \epsilon_q + \epsilon_q - k} - \frac{4\epsilon_k}{\left( \hbar z - \frac{\epsilon_q + k - \epsilon_q - k}{2} \right)^2} - \frac{2\epsilon_k}{(\hbar z - \epsilon_q + \epsilon_q - k)^2} \right] \Rightarrow \\
\left[ \chi_0^{(5,5)}(\mathbf{k}, z) \right]_{27} &= + \left( \frac{m}{\hbar^2} \right)^4 \frac{1}{180k^8} \int \frac{d^3 q}{(2\pi)^3} \frac{2f_0(\mathbf{q})}{60} \left[ \frac{30}{5\hbar z - \epsilon_q + 3k + \epsilon_q - 2k} + \frac{48}{2\hbar z - \epsilon_q + k + \epsilon_q - k} - \frac{30}{\hbar z - \epsilon_q + \epsilon_q - k} - \frac{96\epsilon_k}{(2\hbar z - \epsilon_q + k + \epsilon_q - k)^2} - \frac{12\epsilon_k}{(\hbar z - \epsilon_q + \epsilon_q - k)^2} \right].
\end{aligned}$$

The *twenty-eighth contribution* is characterized by one simple pole and two double poles. This becomes apparent from the algebraic identities  $(\epsilon_q + 3k - \epsilon_q - k)/4 = (\epsilon_q + 2k - \epsilon_q)/2$  and  $(\epsilon_q + 2k - \epsilon_q - k)/3 = (\epsilon_q + k - \epsilon_q)$ . We first identify and calculate the coefficients  $a, b, c$ .

$$\begin{aligned}
\left[ \chi_0^{(5,5)}(\mathbf{k}, z) \right]_{28} &= - \int \frac{d^3 q}{(2\pi)^3} \frac{5\hbar z - \epsilon_q + 4k + \epsilon_q - k}{(2\pi)^3} \frac{2f_0(\mathbf{q})}{(3\hbar z - \epsilon_q + 2k + \epsilon_q - k) (2\hbar z - \epsilon_q + 2k + \epsilon_q) (\hbar z - \epsilon_q + k + \epsilon_q)} \Rightarrow \\
\left[ \chi_0^{(5,5)}(\mathbf{k}, z) \right]_{28} &= - \int \frac{d^3 q}{(2\pi)^3} \frac{f_0(\mathbf{q})}{60} \frac{1}{\left[ \hbar z - \frac{\epsilon_q + 4k - \epsilon_q - k}{5} \right] \left[ \hbar z - \frac{\epsilon_q + 3k - \epsilon_q - k}{4} \right] \left[ \hbar z - \frac{\epsilon_q + 2k - \epsilon_q - k}{3} \right] \left[ \hbar z - (\epsilon_q + k - \epsilon_q) \right]} \Rightarrow \\
\left[ \chi_0^{(5,5)}(\mathbf{k}, z) \right]_{28} &= - \int \frac{d^3 q}{(2\pi)^3} \frac{f_0(\mathbf{q})}{60} \frac{1}{\left[ \hbar z - \frac{\epsilon_q + 4k - \epsilon_q - k}{5} \right] \left[ \hbar z - \frac{\epsilon_q + 2k - \epsilon_q - k}{2} \right] \left[ \hbar z - (\epsilon_q + k - \epsilon_q) \right]^2} \Rightarrow \\
a &= \frac{\epsilon_q + 4k - \epsilon_q - k}{5} = \frac{\hbar^2}{2m} \frac{(q + 4k)^2 - (q - k)^2}{2} = \frac{\hbar^2}{2m} \frac{16k^2 + 8q \cdot k - k^2 + 2q \cdot k}{2} = \frac{\hbar^2}{2m} \frac{15k^2 + 10q \cdot k}{5} = \frac{\hbar^2}{2m} \frac{(3k^2 + 2q \cdot k)}{5} \\
b &= \frac{\epsilon_q + 2k - \epsilon_q}{2} = \frac{\hbar^2}{2m} \frac{(q + 2k)^2 - q^2}{2} = \frac{\hbar^2}{2m} \frac{4k^2 + 4q \cdot k}{2} = \frac{\hbar^2}{2m} (2k^2 + 2q \cdot k) \\
c &= \epsilon_q + k - \epsilon_q = \frac{\hbar^2}{2m} [(q + k)^2 - q^2] = \frac{\hbar^2}{2m} (k^2 + 2q \cdot k)
\end{aligned}$$

Then, we compute all the relevant algebraic combinations between these three coefficients. Note that  $q^2$  and  $q \cdot k$  terms vanish.

$$\begin{aligned}
a - b &= \frac{\hbar^2}{2m} (3k^2 + 2q \cdot k - 2k^2 - 2q \cdot k) = \frac{\hbar^2}{2m} (3k^2 - 2k^2) = \frac{\hbar^2}{2m} (k^2), \quad b - c = \frac{\hbar^2}{2m} (2k^2 + 2q \cdot k - k^2 - 2q \cdot k) = \frac{\hbar^2}{2m} (2k^2 - k^2) = \frac{\hbar^2}{2m} (k^2), \\
a - c &= \frac{\hbar^2}{2m} (3k^2 + 2q \cdot k - k^2 - 2q \cdot k) = \frac{\hbar^2}{2m} (3k^2 - k^2) = \frac{\hbar^2}{2m} (2k^2), \quad 2a - 3b + c = \frac{\hbar^2}{2m} (6k^2 + 4q \cdot k - 6k^2 - 6q \cdot k + k^2 + 2q \cdot k) = \frac{\hbar^2}{2m} (6k^2 - 6k^2 + k^2) = \frac{\hbar^2}{2m} (k^2), \\
2a + b - 3c &= \frac{\hbar^2}{2m} (6k^2 + 4q \cdot k + 2k^2 + 2q \cdot k - 3k^2 - 6q \cdot k) = \frac{\hbar^2}{2m} (6k^2 + 2k^2 - 3k^2) = \frac{\hbar^2}{2m} (5k^2).
\end{aligned}$$

Afterwards, we compute all the combinations that are present in the partial fraction decomposition.

$$\begin{aligned}
(a - b)^2 (a - c)^2 &= \left( \frac{\hbar^2}{2m} \right)^2 (k^4) \left( \frac{\hbar^2}{2m} \right)^2 (4k^8) = \left( \frac{\hbar^2}{2m} \right)^4 (4k^8), \quad (a - b)^2 (b - c)^3 = \left( \frac{\hbar^2}{2m} \right)^2 (k^4) \left( \frac{\hbar^2}{2m} \right)^3 (k^6) = \left( \frac{\hbar^2}{2m} \right)^5 (k^{10}), \\
(a - c)^2 (b - c)^3 &= \left( \frac{\hbar^2}{2m} \right)^2 (4k^4) \left( \frac{\hbar^2}{2m} \right)^3 (k^6) = \left( \frac{\hbar^2}{2m} \right)^5 (4k^{10}), \quad (a - b)(b - c)^2 = \frac{\hbar^2}{2m} (k^2) \left( \frac{\hbar^2}{2m} \right)^2 (k^4) = \left( \frac{\hbar^2}{2m} \right)^3 (k^6), \\
(a - c)(b - c)^2 &= \frac{\hbar^2}{2m} (2k^2) \left( \frac{\hbar^2}{2m} \right)^2 (k^4) = \left( \frac{\hbar^2}{2m} \right)^3 (2k^6).
\end{aligned}$$

Finally, we substitute and perform some straightforward algebra. We also introduce the compact notation  $\epsilon_k = (\hbar^2 k^2)/(2m)$ .

$$\begin{aligned}
\left[ \chi_0^{(5,5)}(\mathbf{k}, z) \right]_{28} &= - \int \frac{d^3 q}{(2\pi)^3} \left( \frac{2m}{\hbar^2} \right)^4 \frac{1}{4k^8} \frac{f_0(\mathbf{q})}{60} \left[ \frac{1}{\hbar z - \frac{\epsilon_q + 4k - \epsilon_q - k}{5}} + \frac{4}{\hbar z - \frac{\epsilon_q + 2k - \epsilon_q}{2}} - \frac{5}{\hbar z - \epsilon_q + k + \epsilon_q} - \frac{\hbar^2}{2m} \frac{4k^2}{\left( \hbar z - \frac{\epsilon_q + 2k - \epsilon_q}{2} \right)^2} - \frac{\hbar^2}{2m} \frac{2k^2}{(\hbar z - \epsilon_q + k + \epsilon_q)^2} \right] \Rightarrow \\
\left[ \chi_0^{(5,5)}(\mathbf{k}, z) \right]_{28} &= - \int \frac{d^3 q}{(2\pi)^3} \left( \frac{2m}{\hbar^2} \right)^4 \frac{1}{4k^8} \frac{f_0(\mathbf{q})}{60} \left[ \frac{1}{\hbar z - \frac{\epsilon_q + 4k - \epsilon_q - k}{5}} + \frac{4}{\hbar z - \frac{\epsilon_q + 2k - \epsilon_q}{2}} - \frac{5}{\hbar z - \epsilon_q + k + \epsilon_q} - \frac{4\epsilon_k}{\left( \hbar z - \frac{\epsilon_q + 2k - \epsilon_q}{2} \right)^2} - \frac{2\epsilon_k}{(\hbar z - \epsilon_q + k + \epsilon_q)^2} \right] \Rightarrow \\
\left[ \chi_0^{(5,5)}(\mathbf{k}, z) \right]_{28} &= - \left( \frac{m}{\hbar^2} \right)^4 \frac{1}{30k^8} \int \frac{d^3 q}{(2\pi)^3} 2f_0(\mathbf{q}) \left[ \frac{1}{\hbar z - \frac{\epsilon_q + 4k - \epsilon_q - k}{5}} + \frac{4}{\hbar z - \frac{\epsilon_q + 2k - \epsilon_q}{2}} - \frac{5}{\hbar z - \epsilon_q + k + \epsilon_q} - \frac{4\epsilon_k}{\left( \hbar z - \frac{\epsilon_q + 2k - \epsilon_q}{2} \right)^2} - \frac{2\epsilon_k}{(\hbar z - \epsilon_q + k + \epsilon_q)^2} \right] \Rightarrow \\
\left[ \chi_0^{(5,5)}(\mathbf{k}, z) \right]_{28} &= - \left( \frac{m}{\hbar^2} \right)^4 \frac{1}{180k^8} \int \frac{d^3 q}{(2\pi)^3} 2f_0(\mathbf{q}) \left[ \frac{30}{5\hbar z - \epsilon_q + 4k + \epsilon_q - k} + \frac{48}{2\hbar z - \epsilon_q + 2k + \epsilon_q} - \frac{30}{\hbar z - \epsilon_q + k + \epsilon_q} - \frac{96\epsilon_k}{(2\hbar z - \epsilon_q + 2k + \epsilon_q)^2} - \frac{12\epsilon_k}{(\hbar z - \epsilon_q + k + \epsilon_q)^2} \right].
\end{aligned}$$

The *twenty-ninth contribution* is characterized by three simple poles and one double pole. This becomes apparent from the algebraic identity  $(\epsilon_q + \mathbf{k} - \epsilon_{q-2\mathbf{k}})/3 = (\epsilon_q - \epsilon_{q-\mathbf{k}})$ . We first identify and calculate the coefficients  $a, b, c, d$ .

$$\begin{aligned}
\left[ \chi_0^{(5,5)}(\mathbf{k}, z) \right]_{29} &= + \int \frac{d^3 q}{(2\pi)^3} \frac{(5\hbar z - \epsilon_{q+3\mathbf{k}} + \epsilon_{q-2\mathbf{k}})(4\hbar z - \epsilon_{q+2\mathbf{k}} + \epsilon_{q-2\mathbf{k}})(3\hbar z - \epsilon_{q+\mathbf{k}} + \epsilon_{q-2\mathbf{k}})(2\hbar z - \epsilon_q + \epsilon_{q-\mathbf{k}})}{2f_0(\mathbf{q})} \Rightarrow \\
\left[ \chi_0^{(5,5)}(\mathbf{k}, z) \right]_{29} &= + \int \frac{d^3 q}{(2\pi)^3} \frac{f_0(\mathbf{q})}{60} \left[ \hbar z - \frac{\epsilon_{q+3\mathbf{k}} - \epsilon_{q-2\mathbf{k}}}{5} \right] \left[ \hbar z - \frac{\epsilon_{q+2\mathbf{k}} - \epsilon_{q-2\mathbf{k}}}{4} \right] \left[ \hbar z - \frac{\epsilon_{q+\mathbf{k}} - \epsilon_{q-2\mathbf{k}}}{3} \right] \left[ \hbar z - (\epsilon_q - \epsilon_{q-\mathbf{k}}) \right] \Rightarrow \\
\left[ \chi_0^{(5,5)}(\mathbf{k}, z) \right]_{29} &= + \int \frac{d^3 q}{(2\pi)^3} \frac{f_0(\mathbf{q})}{60} \left[ \hbar z - \frac{\epsilon_{q+3\mathbf{k}} - \epsilon_{q-2\mathbf{k}}}{5} \right] \left[ \hbar z - \frac{\epsilon_{q+2\mathbf{k}} - \epsilon_{q-2\mathbf{k}}}{4} \right] \left[ \hbar z - (\epsilon_q - \epsilon_{q-\mathbf{k}}) \right] \left[ \hbar z - (\epsilon_q - \epsilon_{q-\mathbf{k}}) \right] \Rightarrow \\
\left[ \chi_0^{(5,5)}(\mathbf{k}, z) \right]_{29} &= + \int \frac{d^3 q}{(2\pi)^3} \frac{f_0(\mathbf{q})}{60} \left[ \hbar z - \frac{\epsilon_{q+3\mathbf{k}} - \epsilon_{q-2\mathbf{k}}}{5} \right] \left[ \hbar z - \frac{\epsilon_{q+2\mathbf{k}} - \epsilon_{q-2\mathbf{k}}}{4} \right] \left[ \hbar z - (\epsilon_q - \epsilon_{q-\mathbf{k}}) \right] \left[ \hbar z - (\epsilon_q - \epsilon_{q-\mathbf{k}}) \right] \Rightarrow \\
a &= \frac{\epsilon_{q+3\mathbf{k}} - \epsilon_{q-2\mathbf{k}}}{5} = \frac{\hbar^2}{2m} \frac{(q+3\mathbf{k})^2 - (q-2\mathbf{k})^2}{5} = \frac{\hbar^2}{2m} \frac{9k^2 + 6\mathbf{q} \cdot \mathbf{k} - 4k^2 + 4\mathbf{q} \cdot \mathbf{k}}{5} = \frac{\hbar^2}{2m} \frac{5k^2 + 10\mathbf{q} \cdot \mathbf{k}}{5} = \frac{\hbar^2}{2m} (k^2 + 2\mathbf{q} \cdot \mathbf{k}) \\
b &= \frac{\epsilon_{q+2\mathbf{k}} - \epsilon_{q-2\mathbf{k}}}{4} = \frac{\hbar^2}{2m} \frac{(q+2\mathbf{k})^2 - (q-2\mathbf{k})^2}{4} = \frac{\hbar^2}{2m} \frac{4k^2 + 4\mathbf{q} \cdot \mathbf{k} - 4k^2 + 4\mathbf{q} \cdot \mathbf{k}}{4} = \frac{\hbar^2}{2m} \frac{8\mathbf{q} \cdot \mathbf{k}}{4} = \frac{\hbar^2}{2m} (2\mathbf{q} \cdot \mathbf{k}) \\
c &= \frac{\epsilon_q - \epsilon_{q-2\mathbf{k}}}{2} = \frac{\hbar^2}{2m} \frac{q^2 - (q-2\mathbf{k})^2}{2} = \frac{\hbar^2}{2m} \frac{-4k^2 + 4\mathbf{q} \cdot \mathbf{k}}{2} = \frac{\hbar^2}{2m} (-2k^2 + 2\mathbf{q} \cdot \mathbf{k}) \\
d &= (\epsilon_q - \epsilon_{q-\mathbf{k}}) = \frac{\hbar^2}{2m} [q^2 - (\mathbf{q} - \mathbf{k})^2] = \frac{\hbar^2}{2m} (-k^2 + 2\mathbf{q} \cdot \mathbf{k}) .
\end{aligned}$$

Then, we compute all the relevant algebraic combinations between the coefficients. Note that  $q^2$  and  $\mathbf{q} \cdot \mathbf{k}$  terms vanish.

$$\begin{aligned}
a - b &= \frac{\hbar^2}{2m} (k^2 + 2\mathbf{q} \cdot \mathbf{k} - 2\mathbf{q} \cdot \mathbf{k}) = \frac{\hbar^2}{2m} (k^2) , \quad b - c = \frac{\hbar^2}{2m} (2\mathbf{q} \cdot \mathbf{k} + 2k^2 - 2\mathbf{q} \cdot \mathbf{k}) = \frac{\hbar^2}{2m} (2k^2) \\
c - d &= \frac{\hbar^2}{2m} (-2k^2 + 2\mathbf{q} \cdot \mathbf{k} + k^2 - 2\mathbf{q} \cdot \mathbf{k}) = \frac{\hbar^2}{2m} (-k^2) , \quad a - c = \frac{\hbar^2}{2m} (k^2 + 2\mathbf{q} \cdot \mathbf{k} + 2k^2 - 2\mathbf{q} \cdot \mathbf{k}) = \frac{\hbar^2}{2m} (3k^2) \\
b - d &= \frac{\hbar^2}{2m} (2\mathbf{q} \cdot \mathbf{k} + k^2 - 2\mathbf{q} \cdot \mathbf{k}) = \frac{\hbar^2}{2m} (k^2) , \quad a - d = \frac{\hbar^2}{2m} (k^2 + 2\mathbf{q} \cdot \mathbf{k} + k^2 - 2\mathbf{q} \cdot \mathbf{k}) = \frac{\hbar^2}{2m} (2k^2) .
\end{aligned}$$

Afterwards, we compute all the combinations that are present in the partial fraction decomposition.

$$\begin{aligned}
(a-b)(a-c)(a-d)^2 &= \left( \frac{\hbar^2}{2m} \right)^4 (k^2)^2 (3k^2) (4k^4) = \left( \frac{\hbar^2}{2m} \right)^4 (12k^8) , \quad (a-b)(b-c)(b-d)^2 = \left( \frac{\hbar^2}{2m} \right)^4 (k^2)^2 (2k^2) (k^4) = \left( \frac{\hbar^2}{2m} \right)^4 (2k^8) , \\
(a-c)(b-c)(c-d)^2 &= \left( \frac{\hbar^2}{2m} \right)^4 (3k^2)^2 (2k^2) (k^4) = \left( \frac{\hbar^2}{2m} \right)^4 (6k^8) , \quad (a-d)(b-d)(c-d) = \left( \frac{\hbar^2}{2m} \right)^3 (2k^2)^2 (k^2) (-k^2) = \left( \frac{\hbar^2}{2m} \right)^3 (-2k^6) , \\
(a-d)^2(b-d)^2(c-d)^2 &= \left( \frac{\hbar^2}{2m} \right)^6 (4k^{12}) , \quad (a-b)(b-c) + (a-d)^2 + (b-d)^2 + (c-d)^2 = \left( \frac{\hbar^2}{2m} \right)^2 (2k^4 + 4k^4 + k^4 - 9k^4) = \left( \frac{\hbar^2}{2m} \right)^2 (-k^4) .
\end{aligned}$$

Finally, we substitute and perform some straightforward algebra. We also introduce the compact notation  $\epsilon_{\mathbf{k}} = (\hbar^2 k^2)/(2m)$ .

$$\begin{aligned}
\left[ \chi_0^{(5,5)}(\mathbf{k}, z) \right]_{29} &= + \int \frac{d^3 q}{(2\pi)^3} \frac{(2m)^4}{\hbar^2} \frac{1}{12k^8} \frac{f_0(\mathbf{q})}{60} \left[ \frac{1}{\hbar z - \frac{\epsilon_{q+3\mathbf{k}} - \epsilon_{q-2\mathbf{k}}}{5}} - \frac{6}{\hbar z - \frac{\epsilon_{q+2\mathbf{k}} - \epsilon_{q-2\mathbf{k}}}{4}} + \frac{2}{\hbar z - \frac{\epsilon_{q+\mathbf{k}} - \epsilon_{q-2\mathbf{k}}}{3}} + \frac{3}{\hbar z - \epsilon_q + \epsilon_{q-\mathbf{k}}} + \frac{\hbar^2}{2m} \frac{6k^2}{(\hbar z - \epsilon_q + \epsilon_{q-\mathbf{k}})^2} \right] \Rightarrow \\
\left[ \chi_0^{(5,5)}(\mathbf{k}, z) \right]_{29} &= + \left( \frac{m}{\hbar^2} \right)^4 \frac{1}{90k^8} \int \frac{d^3 q}{(2\pi)^3} \frac{2f_0(\mathbf{q})}{60} \left[ \frac{1}{\hbar z - \frac{\epsilon_{q+3\mathbf{k}} - \epsilon_{q-2\mathbf{k}}}{5}} - \frac{6}{\hbar z - \frac{\epsilon_{q+2\mathbf{k}} - \epsilon_{q-2\mathbf{k}}}{4}} + \frac{2}{\hbar z - \frac{\epsilon_{q+\mathbf{k}} - \epsilon_{q-2\mathbf{k}}}{3}} + \frac{3}{\hbar z - \epsilon_q + \epsilon_{q-\mathbf{k}}} + \frac{6\epsilon_{\mathbf{k}}}{(\hbar z - \epsilon_q + \epsilon_{q-\mathbf{k}})^2} \right] \Rightarrow \\
\left[ \chi_0^{(5,5)}(\mathbf{k}, z) \right]_{29} &= + \left( \frac{m}{\hbar^2} \right)^4 \frac{1}{180k^8} \int \frac{d^3 q}{(2\pi)^3} \frac{2f_0(\mathbf{q})}{60} \left[ \frac{10}{5\hbar z - \epsilon_{q+3\mathbf{k}} + \epsilon_{q-2\mathbf{k}}} - \frac{48}{4\hbar z - \epsilon_{q+2\mathbf{k}} + \epsilon_{q-2\mathbf{k}}} + \frac{8}{2\hbar z - \epsilon_q + \epsilon_{q-\mathbf{k}}} + \frac{6}{\hbar z - \epsilon_q + \epsilon_{q-\mathbf{k}}} + \frac{12\epsilon_{\mathbf{k}}}{(\hbar z - \epsilon_q + \epsilon_{q-\mathbf{k}})^2} \right] .
\end{aligned}$$

The *thirtieth contribution* is characterized by three simple poles and one double pole. This becomes apparent from the algebraic identity  $(\epsilon_q + 2k - \epsilon_q - k)/3 = (\epsilon_q + k - \epsilon_q)$ . We first identify and calculate the coefficients  $a, b, c, d$ .

$$\begin{aligned}
\left[ \chi_0^{(5,5)}(\mathbf{k}, z) \right]_{30} &= - \int \frac{d^3 q}{(2\pi)^3} \frac{2f_0(\mathbf{q})}{(5hz - \epsilon_q + 4k + \epsilon_q - k)(4hz - \epsilon_q + 3k + \epsilon_q - k)(3hz - \epsilon_q + 2k + \epsilon_q - k)(2hz - \epsilon_q + k + \epsilon_q - k)(hz - \epsilon_q + k + \epsilon_q)} \\
\left[ \chi_0^{(5,5)}(\mathbf{k}, z) \right]_{30} &= - \int \frac{d^3 q}{(2\pi)^3} \frac{f_0(\mathbf{q})}{60} \left[ \frac{hz - \frac{\epsilon_q + 4k - \epsilon_q - k}{5}}{hz - \frac{\epsilon_q + 3k - \epsilon_q - k}{4}} \right] \left[ \frac{hz - \frac{\epsilon_q + 2k - \epsilon_q - k}{3}}{hz - \frac{\epsilon_q + k - \epsilon_q - k}{2}} \right] \left[ \frac{hz - (\epsilon_q + k - \epsilon_q)}{hz - (\epsilon_q + k - \epsilon_q)} \right] \\
\left[ \chi_0^{(5,5)}(\mathbf{k}, z) \right]_{30} &= - \int \frac{d^3 q}{(2\pi)^3} \frac{f_0(\mathbf{q})}{60} \left[ \frac{hz - \frac{\epsilon_q + 4k - \epsilon_q - k}{5}}{hz - \frac{\epsilon_q + 3k - \epsilon_q - k}{4}} \right] \left[ \frac{hz - (\epsilon_q + k - \epsilon_q)}{hz - (\epsilon_q + k - \epsilon_q)} \right] \left[ \frac{hz - (\epsilon_q + k - \epsilon_q)}{hz - (\epsilon_q + k - \epsilon_q)} \right] \\
\left[ \chi_0^{(5,5)}(\mathbf{k}, z) \right]_{30} &= - \int \frac{d^3 q}{(2\pi)^3} \frac{f_0(\mathbf{q})}{60} \left[ \frac{hz - \frac{\epsilon_q + 4k - \epsilon_q - k}{5}}{hz - \frac{\epsilon_q + 3k - \epsilon_q - k}{4}} \right] \left[ \frac{hz - \frac{\epsilon_q + 3k - \epsilon_q - k}{4}}{hz - (\epsilon_q + k - \epsilon_q)} \right] \left[ \frac{hz - (\epsilon_q + k - \epsilon_q)}{hz - (\epsilon_q + k - \epsilon_q)} \right]^2 \\
a &= \frac{\epsilon_q + 4k - \epsilon_q - k}{5} = \frac{h^2}{2m} \frac{(q + 4k)^2 - (q - k)^2}{16k^2 + 8q \cdot k - k^2 + 2q \cdot k} = \frac{h^2}{2m} \frac{15k^2 + 10q \cdot k}{5} = \frac{h^2}{2m} (3k^2 + 2q \cdot k) \\
b &= \frac{\epsilon_q + 3k - \epsilon_q - k}{4} = \frac{h^2}{2m} \frac{(q + 3k)^2 - (q - k)^2}{9k^2 + 6q \cdot k - k^2 + 2q \cdot k} = \frac{h^2}{2m} \frac{8k^2 + 8q \cdot k}{4} = \frac{h^2}{2m} (2k^2 + 2q \cdot k) \\
c &= \frac{\epsilon_q + k - \epsilon_q - k}{2} = \frac{h^2}{2m} \frac{(q + k)^2 - (q - k)^2}{k^2 + 2q \cdot k - k^2 + 2q \cdot k} = \frac{h^2}{2m} \frac{2}{2} = \frac{h^2}{2m} (2q \cdot k) \\
d &= (\epsilon_q + k - \epsilon_q) = \frac{h^2}{2m} [(q + k)^2 - q^2] = \frac{h^2}{2m} (k^2 + 2q \cdot k).
\end{aligned}$$

Then, we compute all the relevant algebraic combinations between the coefficients. Note that  $q^2$  and  $q \cdot k$  terms vanish.

$$\begin{aligned}
a - b &= \frac{h^2}{2m} (3k^2 + 2q \cdot k - 2k^2 - 2q \cdot k) = \frac{h^2}{2m} (k^2), \quad b - c = \frac{h^2}{2m} (2k^2 + 2q \cdot k - 2q \cdot k) = \frac{h^2}{2m} (2k^2) \\
c - d &= \frac{h^2}{2m} (2q \cdot k - k^2 - 2q \cdot k) = \frac{h^2}{2m} (-k^2), \quad a - c = \frac{h^2}{2m} (3k^2 + 2q \cdot k - 2q \cdot k) = \frac{h^2}{2m} (3k^2) \\
b - d &= \frac{h^2}{2m} (2k^2 + 2q \cdot k - k^2 - 2q \cdot k) = \frac{h^2}{2m} (k^2), \quad a - d = \frac{h^2}{2m} (3k^2 + 2q \cdot k - k^2 - 2q \cdot k) = \frac{h^2}{2m} (3k^2 - k^2) = \frac{h^2}{2m} (2k^2).
\end{aligned}$$

Afterwards, we compute all the combinations that are present in the partial fraction decomposition.

$$\begin{aligned}
(a - b)(a - c)(a - d)^2 &= \left( \frac{h^2}{2m} \right)^4 (k^2)^2 (3k^2) (4k^4) = \left( \frac{h^2}{2m} \right)^4 (12k^8), \quad (a - b)(b - c)(b - d)^2 = \left( \frac{h^2}{2m} \right)^4 (k^2)^2 (2k^2) (k^4) = \left( \frac{h^2}{2m} \right)^4 (2k^8), \\
(a - c)(b - c)(c - d)^2 &= \left( \frac{h^2}{2m} \right)^4 (3k^2)^2 (2k^2) (k^4) = \left( \frac{h^2}{2m} \right)^4 (6k^8), \quad (a - d)(b - d)(c - d) = \left( \frac{h^2}{2m} \right)^3 (2k^2)^2 (k^2) (-k^2) = \left( \frac{h^2}{2m} \right)^3 (-2k^6), \\
(a - d)^2(b - d)^2(c - d)^2 &= \left( \frac{h^2}{2m} \right)^6 (4k^{12}), \quad (a - b)(b - c) + (a - d)^2 + (b - d)^2 + (c - d)^2 = \left( \frac{h^2}{2m} \right)^2 (2k^4 + 4k^4 + k^4 + k^4 - 9k^4) = \left( \frac{h^2}{2m} \right)^2 (-k^4).
\end{aligned}$$

Finally, we substitute and perform some straightforward algebra. We also introduce the compact notation  $\epsilon_k = (h^2 k^2)/(2m)$ .

$$\begin{aligned}
\left[ \chi_0^{(5,5)}(\mathbf{k}, z) \right]_{30} &= - \int \frac{d^3 q}{(2\pi)^3} \left( \frac{2m}{h^2} \right)^4 \frac{1}{12k^8} \frac{f_0(\mathbf{q})}{60} \left[ \frac{1}{hz - \frac{\epsilon_q + 4k - \epsilon_q - k}{5}} - \frac{6}{hz - \frac{\epsilon_q + 3k - \epsilon_q - k}{4}} + \frac{2}{hz - \frac{\epsilon_q + k - \epsilon_q - k}{2}} + \frac{3}{hz - \epsilon_q + k + \epsilon_q} + \frac{h^2}{2m} \frac{6k^2}{(hz - \epsilon_q + k + \epsilon_q)^2} \right] \\
\left[ \chi_0^{(5,5)}(\mathbf{k}, z) \right]_{30} &= - \left( \frac{m}{h^2} \right)^4 \frac{1}{90k^8} \int \frac{d^3 q}{(2\pi)^3} \frac{2f_0(\mathbf{q})}{60} \left[ \frac{1}{hz - \frac{\epsilon_q + 4k - \epsilon_q - k}{5}} - \frac{6}{hz - \frac{\epsilon_q + 3k - \epsilon_q - k}{4}} + \frac{2}{hz - \frac{\epsilon_q + k - \epsilon_q - k}{2}} + \frac{3}{hz - \epsilon_q + k + \epsilon_q} + \frac{6\epsilon_k}{(hz - \epsilon_q + k + \epsilon_q)^2} \right] \\
\left[ \chi_0^{(5,5)}(\mathbf{k}, z) \right]_{30} &= - \left( \frac{m}{h^2} \right)^4 \frac{1}{180k^8} \int \frac{d^3 q}{(2\pi)^3} \frac{2f_0(\mathbf{q})}{60} \left[ \frac{10}{5hz - \epsilon_q + 4k + \epsilon_q - k} - \frac{48}{4hz - \epsilon_q + 3k + \epsilon_q - k} + \frac{8}{2hz - \epsilon_q + k + \epsilon_q - k} + \frac{6}{hz - \epsilon_q + k + \epsilon_q} + \frac{12\epsilon_k}{(hz - \epsilon_q + k + \epsilon_q)^2} \right].
\end{aligned}$$

The *thirty-first contribution* is characterized by five simple poles. We first identify and calculate the coefficients  $a, b, c, d, e$ .

$$\begin{aligned}
\left[ \chi_0^{(5,5)}(\mathbf{k}, z) \right]_{31} &= - \int \frac{d^3 q}{(2\pi)^3} \frac{2f_0(\mathbf{q})}{(5\hbar z - \epsilon_q + 4\mathbf{k} + \epsilon_q - \mathbf{k}) (4\hbar z - \epsilon_q + 3\mathbf{k} + \epsilon_q - \mathbf{k}) (3\hbar z - \epsilon_q + 2\mathbf{k} + \epsilon_q - \mathbf{k}) (2\hbar z - \epsilon_q + \mathbf{k} + \epsilon_q - \mathbf{k}) (\hbar z - \epsilon_q + \epsilon_q - \mathbf{k})} \Rightarrow \\
\left[ \chi_0^{(5,5)}(\mathbf{k}, z) \right]_{31} &= - \int \frac{d^3 q}{(2\pi)^3} \frac{f_0(\mathbf{q})}{60} \frac{1}{\left[ \hbar z - \frac{\epsilon_q + 4\mathbf{k} - \epsilon_q - \mathbf{k}}{5} \right] \left[ \hbar z - \frac{\epsilon_q + 3\mathbf{k} - \epsilon_q - \mathbf{k}}{4} \right] \left[ \hbar z - \frac{\epsilon_q + 2\mathbf{k} - \epsilon_q - \mathbf{k}}{3} \right] \left[ \hbar z - \frac{\epsilon_q + \mathbf{k} - \epsilon_q - \mathbf{k}}{2} \right]} \Rightarrow \\
a &= \frac{\epsilon_q + 4\mathbf{k} - \epsilon_q - \mathbf{k}}{5} = \frac{\hbar^2}{2m} \frac{(q + 4k)^2 - (q - k)^2}{2m} = \frac{\hbar^2}{2m} \frac{16k^2 + 8q \cdot k - k^2 + 2q \cdot k}{2m} = \frac{\hbar^2}{2m} \frac{15k^2 + 10q \cdot k}{2m} = \frac{\hbar^2}{2m} (3k^2 + 2q \cdot k), \\
b &= \frac{\epsilon_q + 3\mathbf{k} - \epsilon_q - \mathbf{k}}{4} = \frac{\hbar^2}{2m} \frac{(q + 3k)^2 - (q - k)^2}{2m} = \frac{\hbar^2}{2m} \frac{9k^2 + 6q \cdot k - k^2 + 2q \cdot k}{2m} = \frac{\hbar^2}{2m} \frac{8k^2 + 8q \cdot k}{2m} = \frac{\hbar^2}{2m} (2k^2 + 2q \cdot k), \\
c &= \frac{\epsilon_q + 2\mathbf{k} - \epsilon_q - \mathbf{k}}{3} = \frac{\hbar^2}{2m} \frac{(q + 2k)^2 - (q - k)^2}{2m} = \frac{\hbar^2}{2m} \frac{4k^2 + 4q \cdot k - k^2 + 2q \cdot k}{2m} = \frac{\hbar^2}{2m} \frac{3k^2 + 6q \cdot k}{2m} = \frac{\hbar^2}{2m} (k^2 + 2q \cdot k), \\
d &= \frac{\epsilon_q + \mathbf{k} - \epsilon_q - \mathbf{k}}{2} = \frac{\hbar^2}{2m} \frac{(q + k)^2 - (q - k)^2}{2m} = \frac{\hbar^2}{2m} \frac{k^2 + 2q \cdot k - k^2 + 2q \cdot k}{2m} = \frac{\hbar^2}{2m} \frac{4q \cdot k}{2m} = \frac{\hbar^2}{2m} (2q \cdot k), \\
e &= \epsilon_q - \epsilon_q - \mathbf{k} = \frac{\hbar^2}{2m} [q^2 - (q - k)^2] = \frac{\hbar^2}{2m} (-k^2 + 2q \cdot k).
\end{aligned}$$

Then, we compute all the possible differences between these four coefficients. Note that  $q^2$  and  $q \cdot k$  terms vanish.

$$\begin{aligned}
a - b &= \frac{\hbar^2}{2m} (3k^2 + 2q \cdot k - 2k^2 - 2q \cdot k) = \frac{\hbar^2}{2m} (3k^2 - 2k^2) = \frac{\hbar^2}{2m} (k^2), & b - c &= \frac{\hbar^2}{2m} (2k^2 + 2q \cdot k - k^2 - 2q \cdot k) = \frac{\hbar^2}{2m} (2k^2 - k^2) = \frac{\hbar^2}{2m} (k^2), \\
c - d &= \frac{\hbar^2}{2m} (k^2 + 2q \cdot k - 2q \cdot k) = \frac{\hbar^2}{2m} (k^2) = \frac{\hbar^2}{2m} (k^2), & d - e &= \frac{\hbar^2}{2m} (2q \cdot k + k^2 - 2q \cdot k) = \frac{\hbar^2}{2m} (k^2) = \frac{\hbar^2}{2m} (k^2), \\
a - c &= \frac{\hbar^2}{2m} (3k^2 + 2q \cdot k - k^2 - 2q \cdot k) = \frac{\hbar^2}{2m} (3k^2 - k^2) = \frac{\hbar^2}{2m} (2k^2), & b - d &= \frac{\hbar^2}{2m} (2k^2 + 2q \cdot k - 2q \cdot k) = \frac{\hbar^2}{2m} (2k^2) = \frac{\hbar^2}{2m} (2k^2), \\
c - e &= \frac{\hbar^2}{2m} (k^2 + 2q \cdot k + k^2 - 2q \cdot k) = \frac{\hbar^2}{2m} (k^2 + k^2) = \frac{\hbar^2}{2m} (2k^2), & a - d &= \frac{\hbar^2}{2m} (3k^2 + 2q \cdot k - 2q \cdot k) = \frac{\hbar^2}{2m} (3k^2) = \frac{\hbar^2}{2m} (3k^2), \\
b - e &= \frac{\hbar^2}{2m} (2k^2 + 2q \cdot k + k^2 - 2q \cdot k) = \frac{\hbar^2}{2m} (2k^2 + k^2) = \frac{\hbar^2}{2m} (3k^2), & a - e &= \frac{\hbar^2}{2m} (3k^2 + 2q \cdot k + k^2 - 2q \cdot k) = \frac{\hbar^2}{2m} (3k^2 + k^2) = \frac{\hbar^2}{2m} (4k^2),
\end{aligned}$$

Afterwards, we compute all the triple difference combinations that are present in the partial fraction decomposition.

$$\begin{aligned}
(a - b)(a - c)(a - d)(a - e) &= \frac{\hbar^2}{2m} (k^2) \frac{\hbar^2}{2m} (2k^2) \frac{\hbar^2}{2m} (3k^2) \frac{\hbar^2}{2m} (4k^2) = \left( \frac{\hbar^2}{2m} \right)^4 (24k^8), & (a - b)(b - c)(b - d)(b - e) &= \frac{\hbar^2}{2m} (k^2) \frac{\hbar^2}{2m} (k^2) \frac{\hbar^2}{2m} (2k^2) \frac{\hbar^2}{2m} (3k^2) = \left( \frac{\hbar^2}{2m} \right)^4 (6k^8), \\
(a - c)(b - c)(c - d)(c - e) &= \frac{\hbar^2}{2m} (2k^2) \frac{\hbar^2}{2m} (2k^2) \frac{\hbar^2}{2m} (k^2) \frac{\hbar^2}{2m} (2k^2) = \left( \frac{\hbar^2}{2m} \right)^4 (4k^8), & (a - d)(b - d)(c - d)(d - e) &= \frac{\hbar^2}{2m} (3k^2) \frac{\hbar^2}{2m} (2k^2) \frac{\hbar^2}{2m} (k^2) = \left( \frac{\hbar^2}{2m} \right)^4 (6k^8), \\
(a - e)(b - e)(c - e)(d - e) &= \frac{\hbar^2}{2m} (4k^2) \frac{\hbar^2}{2m} (3k^2) \frac{\hbar^2}{2m} (2k^2) \frac{\hbar^2}{2m} (k^2) = \left( \frac{\hbar^2}{2m} \right)^4 (24k^8).
\end{aligned}$$

Finally, we substitute the above in the contribution and perform some straightforward algebra.

$$\begin{aligned}
\left[ \chi_0^{(5,5)}(\mathbf{k}, z) \right]_{31} &= - \int \frac{d^3 q}{(2\pi)^3} \left( \frac{2m}{\hbar^2} \right)^4 \frac{1}{24k^8} \frac{1}{60} f_0(\mathbf{q}) \left[ \frac{1}{\hbar z - \frac{\epsilon_q + 4\mathbf{k} - \epsilon_q - \mathbf{k}}{5}} - \frac{4}{\hbar z - \frac{\epsilon_q + 3\mathbf{k} - \epsilon_q - \mathbf{k}}{4}} + \frac{6}{\hbar z - \frac{\epsilon_q + 2\mathbf{k} - \epsilon_q - \mathbf{k}}{3}} - \frac{4}{\hbar z - \frac{\epsilon_q + \mathbf{k} - \epsilon_q - \mathbf{k}}{2}} + \frac{1}{\hbar z - \epsilon_q + \epsilon_q - \mathbf{k}} \right] \Rightarrow \\
\left[ \chi_0^{(5,5)}(\mathbf{k}, z) \right]_{31} &= - \left( \frac{m}{\hbar^2} \right)^4 \frac{1}{180k^8} \int \frac{d^3 q}{(2\pi)^3} \frac{2f_0(\mathbf{q})}{60} \left[ \frac{1}{\hbar z - \frac{\epsilon_q + 4\mathbf{k} - \epsilon_q - \mathbf{k}}{5}} - \frac{4}{\hbar z - \frac{\epsilon_q + 3\mathbf{k} - \epsilon_q - \mathbf{k}}{4}} + \frac{6}{\hbar z - \frac{\epsilon_q + 2\mathbf{k} - \epsilon_q - \mathbf{k}}{3}} - \frac{4}{\hbar z - \frac{\epsilon_q + \mathbf{k} - \epsilon_q - \mathbf{k}}{2}} + \frac{1}{\hbar z - \epsilon_q + \epsilon_q - \mathbf{k}} \right] \Rightarrow \\
\left[ \chi_0^{(5,5)}(\mathbf{k}, z) \right]_{31} &= - \left( \frac{m}{\hbar^2} \right)^4 \frac{1}{180k^8} \int \frac{d^3 q}{(2\pi)^3} \frac{2f_0(\mathbf{q})}{60} \left[ \frac{5\hbar z - \epsilon_q + 4\mathbf{k} + \epsilon_q - \mathbf{k}}{5} - \frac{16}{4\hbar z - \epsilon_q + 3\mathbf{k} + \epsilon_q - \mathbf{k}} + \frac{18}{3\hbar z - \epsilon_q + 2\mathbf{k} + \epsilon_q - \mathbf{k}} - \frac{8}{2\hbar z - \epsilon_q + \mathbf{k} + \epsilon_q - \mathbf{k}} + \frac{1}{\hbar z - \epsilon_q + \epsilon_q - \mathbf{k}} \right].
\end{aligned}$$

The *thirty-second contribution* is characterized by five simple poles. We first identify and calculate the coefficients  $a, b, c, d, e$ .

$$\begin{aligned}
\left[ \chi_0^{(5,5)}(\mathbf{k}, z) \right]_{32} &= + \int \frac{d^3 q}{(2\pi)^3} \frac{2f_0(\mathbf{q})}{(5\hbar z - \epsilon_q + 5\mathbf{k} + \epsilon_q)(4\hbar z - \epsilon_q + 4\mathbf{k} + \epsilon_q)(3\hbar z - \epsilon_q + 3\mathbf{k} + \epsilon_q)(2\hbar z - \epsilon_q + 2\mathbf{k} + \epsilon_q)(\hbar z - \epsilon_q + \mathbf{k} + \epsilon_q)} \Rightarrow \\
\left[ \chi_0^{(5,5)}(\mathbf{k}, z) \right]_{32} &= + \int \frac{d^3 q}{(2\pi)^3} \frac{f_0(\mathbf{q})}{60} \frac{1}{\left[ \hbar z - \frac{\epsilon_q + 5\mathbf{k} - \epsilon_q}{5} \right] \left[ \hbar z - \frac{\epsilon_q + 4\mathbf{k} - \epsilon_q}{4} \right] \left[ \hbar z - \frac{\epsilon_q + 3\mathbf{k} - \epsilon_q}{3} \right] \left[ \hbar z - \frac{\epsilon_q + 2\mathbf{k} - \epsilon_q}{2} \right] \left[ \hbar z - (\epsilon_q + \mathbf{k} - \epsilon_q) \right]} \Rightarrow \\
a &= \frac{\epsilon_q + 5\mathbf{k} - \epsilon_q}{5} = \frac{\hbar^2}{2m} \frac{(q + 5\mathbf{k})^2 - q^2}{5} = \frac{\hbar^2}{2m} \frac{25k^2 + 10\mathbf{q} \cdot \mathbf{k}}{5} = \frac{\hbar^2}{2m} (5k^2 + 2\mathbf{q} \cdot \mathbf{k}), \\
b &= \frac{\epsilon_q + 4\mathbf{k} - \epsilon_q}{4} = \frac{\hbar^2}{2m} \frac{(q + 4\mathbf{k})^2 - q^2}{4} = \frac{\hbar^2}{2m} \frac{16k^2 + 8\mathbf{q} \cdot \mathbf{k}}{4} = \frac{\hbar^2}{2m} (4k^2 + 2\mathbf{q} \cdot \mathbf{k}), \\
c &= \frac{\epsilon_q + 3\mathbf{k} - \epsilon_q}{3} = \frac{\hbar^2}{2m} \frac{(q + 3\mathbf{k})^2 - q^2}{3} = \frac{\hbar^2}{2m} \frac{9k^2 + 6\mathbf{q} \cdot \mathbf{k}}{3} = \frac{\hbar^2}{2m} (3k^2 + 2\mathbf{q} \cdot \mathbf{k}), \\
d &= \frac{\epsilon_q + 2\mathbf{k} - \epsilon_q}{2} = \frac{\hbar^2}{2m} \frac{(q + 2\mathbf{k})^2 - q^2}{2} = \frac{\hbar^2}{2m} \frac{4k^2 + 4\mathbf{q} \cdot \mathbf{k}}{2} = \frac{\hbar^2}{2m} (2k^2 + 2\mathbf{q} \cdot \mathbf{k}), \\
e &= \epsilon_q + \mathbf{k} - \epsilon_q = \frac{\hbar^2}{2m} [(q - \mathbf{k})^2 - q^2] = \frac{\hbar^2}{2m} (k^2 + 2\mathbf{q} \cdot \mathbf{k}).
\end{aligned}$$

Then, we compute all the possible differences between these four coefficients. Note that  $q^2$  and  $\mathbf{q} \cdot \mathbf{k}$  terms vanish.

$$\begin{aligned}
a - b &= \frac{\hbar^2}{2m} (5k^2 + 2\mathbf{q} \cdot \mathbf{k} - 4k^2 - 2\mathbf{q} \cdot \mathbf{k}) = \frac{\hbar^2}{2m} (5k^2 - 4k^2) = \frac{\hbar^2}{2m} (k^2), & b - c &= \frac{\hbar^2}{2m} (4k^2 + 2\mathbf{q} \cdot \mathbf{k} - 3k^2 - 2\mathbf{q} \cdot \mathbf{k}) = \frac{\hbar^2}{2m} (4k^2 - 3k^2) = \frac{\hbar^2}{2m} (k^2), \\
c - d &= \frac{\hbar^2}{2m} (3k^2 + 2\mathbf{q} \cdot \mathbf{k} - 2k^2 - 2\mathbf{q} \cdot \mathbf{k}) = \frac{\hbar^2}{2m} (3k^2 - 2k^2) = \frac{\hbar^2}{2m} (k^2), & d - e &= \frac{\hbar^2}{2m} (2k^2 + 2\mathbf{q} \cdot \mathbf{k} - k^2 - 2\mathbf{q} \cdot \mathbf{k}) = \frac{\hbar^2}{2m} (2k^2 - k^2) = \frac{\hbar^2}{2m} (k^2), \\
a - c &= \frac{\hbar^2}{2m} (5k^2 + 2\mathbf{q} \cdot \mathbf{k} - 3k^2 - 2\mathbf{q} \cdot \mathbf{k}) = \frac{\hbar^2}{2m} (5k^2 - 3k^2) = \frac{\hbar^2}{2m} (2k^2), & b - d &= \frac{\hbar^2}{2m} (4k^2 + 2\mathbf{q} \cdot \mathbf{k} - 2k^2 - 2\mathbf{q} \cdot \mathbf{k}) = \frac{\hbar^2}{2m} (4k^2 - 2k^2) = \frac{\hbar^2}{2m} (2k^2), \\
c - e &= \frac{\hbar^2}{2m} (3k^2 + 2\mathbf{q} \cdot \mathbf{k} - k^2 - 2\mathbf{q} \cdot \mathbf{k}) = \frac{\hbar^2}{2m} (3k^2 - k^2) = \frac{\hbar^2}{2m} (2k^2), & a - d &= \frac{\hbar^2}{2m} (5k^2 + 2\mathbf{q} \cdot \mathbf{k} - 2k^2 - 2\mathbf{q} \cdot \mathbf{k}) = \frac{\hbar^2}{2m} (5k^2 - 2k^2) = \frac{\hbar^2}{2m} (3k^2), \\
b - e &= \frac{\hbar^2}{2m} (4k^2 + 2\mathbf{q} \cdot \mathbf{k} - k^2 - 2\mathbf{q} \cdot \mathbf{k}) = \frac{\hbar^2}{2m} (4k^2 - k^2) = \frac{\hbar^2}{2m} (3k^2), & a - e &= \frac{\hbar^2}{2m} (5k^2 + 2\mathbf{q} \cdot \mathbf{k} - k^2 - 2\mathbf{q} \cdot \mathbf{k}) = \frac{\hbar^2}{2m} (5k^2 - k^2) = \frac{\hbar^2}{2m} (4k^2),
\end{aligned}$$

Afterwards, we compute all the triple difference combinations that are present in the partial fraction decomposition.

$$\begin{aligned}
(a - b)(a - c)(a - d)(a - e) &= \frac{\hbar^2}{2m} (k^2) \frac{\hbar^2}{2m} (2k^2) \frac{\hbar^2}{2m} (3k^2) \frac{\hbar^2}{2m} (4k^2) = \left( \frac{\hbar^2}{2m} \right)^4 (24k^8), & (a - b)(b - c)(b - d)(b - e) &= \frac{\hbar^2}{2m} (k^2) \frac{\hbar^2}{2m} (k^2) \frac{\hbar^2}{2m} (2k^2) \frac{\hbar^2}{2m} (3k^2) = \left( \frac{\hbar^2}{2m} \right)^4 (6k^8), \\
(a - c)(b - c)(c - d)(c - e) &= \frac{\hbar^2}{2m} (2k^2) \frac{\hbar^2}{2m} (k^2) \frac{\hbar^2}{2m} (2k^2) \frac{\hbar^2}{2m} (2k^2) = \left( \frac{\hbar^2}{2m} \right)^4 (4k^8), & (a - d)(b - d)(c - d)(d - e) &= \frac{\hbar^2}{2m} (3k^2) \frac{\hbar^2}{2m} (2k^2) \frac{\hbar^2}{2m} (k^2) = \left( \frac{\hbar^2}{2m} \right)^4 (6k^8), \\
(a - e)(b - e)(c - e)(d - e) &= \frac{\hbar^2}{2m} (4k^2) \frac{\hbar^2}{2m} (3k^2) \frac{\hbar^2}{2m} (2k^2) \frac{\hbar^2}{2m} (k^2) = \left( \frac{\hbar^2}{2m} \right)^4 (24k^8).
\end{aligned}$$

Finally, we substitute the above in the contribution and perform some straightforward algebra.

$$\begin{aligned}
\left[ \chi_0^{(5,5)}(\mathbf{k}, z) \right]_{32} &= + \int \frac{d^3 q}{(2\pi)^3} \left( \frac{2m}{\hbar^2} \right)^4 \frac{1}{24k^8} \frac{1}{60} f_0(\mathbf{q}) \left[ \frac{1}{\hbar z - \frac{\epsilon_q + 5\mathbf{k} - \epsilon_q}{5}} - \frac{4}{\hbar z - \frac{\epsilon_q + 4\mathbf{k} - \epsilon_q}{4}} + \frac{6}{\hbar z - \frac{\epsilon_q + 3\mathbf{k} - \epsilon_q}{3}} - \frac{4}{\hbar z - \frac{\epsilon_q + 2\mathbf{k} - \epsilon_q}{2}} + \frac{1}{\hbar z - \epsilon_q + \mathbf{k} + \epsilon_q} \right] \Rightarrow \\
\left[ \chi_0^{(5,5)}(\mathbf{k}, z) \right]_{32} &= + \left( \frac{m}{\hbar^2} \right)^4 \frac{1}{180k^8} \int \frac{d^3 q}{(2\pi)^3} \frac{2f_0(\mathbf{q})}{5} \left[ \frac{1}{\hbar z - \frac{\epsilon_q + 5\mathbf{k} - \epsilon_q}{5}} - \frac{4}{\hbar z - \frac{\epsilon_q + 4\mathbf{k} - \epsilon_q}{4}} + \frac{6}{\hbar z - \frac{\epsilon_q + 3\mathbf{k} - \epsilon_q}{3}} - \frac{4}{\hbar z - \frac{\epsilon_q + 2\mathbf{k} - \epsilon_q}{2}} + \frac{1}{\hbar z - \epsilon_q + \mathbf{k} + \epsilon_q} \right] \Rightarrow \\
\left[ \chi_0^{(5,5)}(\mathbf{k}, z) \right]_{32} &= + \left( \frac{m}{\hbar^2} \right)^4 \frac{1}{180k^8} \int \frac{d^3 q}{(2\pi)^3} \frac{2f_0(\mathbf{q})}{5} \left[ 5\hbar z - \epsilon_q + 5\mathbf{k} + \epsilon_q - \frac{4\hbar z - \epsilon_q + 4\mathbf{k} + \epsilon_q}{4} + \frac{3\hbar z - \epsilon_q + 3\mathbf{k} + \epsilon_q}{3} - \frac{2\hbar z - \epsilon_q + 2\mathbf{k} + \epsilon_q}{2} + \frac{1}{\hbar z - \epsilon_q + \mathbf{k} + \epsilon_q} \right].
\end{aligned}$$



$$\begin{aligned} \chi_0^{(5,5)}(\mathbf{k}, z) = & -\left(\frac{m}{\hbar^2}\right)^4 \frac{1}{180k^8} \int \frac{d^3q}{(2\pi)^3} \frac{2f_0(q)}{(2\pi)^3} \left[ \frac{5}{5\hbar z - \epsilon_q + \epsilon_{q-5k}} - \frac{16}{4\hbar z - \epsilon_q + \epsilon_{q-4k}} + \frac{18}{3\hbar z - \epsilon_q + \epsilon_{q-3k}} - \frac{8}{2\hbar z - \epsilon_q + \epsilon_{q-2k}} + \frac{1}{\hbar z - \epsilon_q + \epsilon_{q-k}} \right] \\ & + \left(\frac{m}{\hbar^2}\right)^4 \frac{1}{180k^8} \int \frac{d^3q}{(2\pi)^3} \frac{2f_0(q)}{(2\pi)^3} \left[ \frac{5}{5\hbar z - \epsilon_{q+k} + \epsilon_{q-4k}} - \frac{16}{4\hbar z - \epsilon_{q+k} + \epsilon_{q-3k}} + \frac{18}{3\hbar z - \epsilon_{q+k} + \epsilon_{q-2k}} - \frac{8}{2\hbar z - \epsilon_{q+k} + \epsilon_{q-k}} + \frac{1}{\hbar z - \epsilon_{q+k} + \epsilon_q} \right] \\ & + \left(\frac{m}{\hbar^2}\right)^4 \frac{1}{180k^8} \int \frac{d^3q}{(2\pi)^3} \frac{2f_0(q)}{(2\pi)^3} \left[ \frac{10}{5\hbar z - \epsilon_{q+k} + \epsilon_{q-4k}} - \frac{48}{4\hbar z - \epsilon_{q+k} + \epsilon_{q-3k}} + \frac{8}{2\hbar z - \epsilon_{q+k} + \epsilon_{q-2k}} + \frac{6}{\hbar z - \epsilon_{q+k} + \epsilon_{q-k}} - \frac{12\epsilon_k}{(\hbar z - \epsilon_q + \epsilon_{q-k})^2} \right] \\ & - \left(\frac{m}{\hbar^2}\right)^4 \frac{1}{180k^8} \int \frac{d^3q}{(2\pi)^3} \frac{2f_0(q)}{(2\pi)^3} \left[ \frac{10}{5\hbar z - \epsilon_{q+2k} + \epsilon_{q-3k}} - \frac{48}{4\hbar z - \epsilon_{q+2k} + \epsilon_{q-2k}} + \frac{8}{2\hbar z - \epsilon_{q+2k} + \epsilon_q} + \frac{6}{(\hbar z - \epsilon_{q+k} + \epsilon_q)} - \frac{12\epsilon_k}{(\hbar z - \epsilon_{q+k} + \epsilon_q)^2} \right] \\ & + \left(\frac{m}{\hbar^2}\right)^4 \frac{1}{180k^8} \int \frac{d^3q}{(2\pi)^3} \frac{2f_0(q)}{(2\pi)^3} \left[ \frac{30}{5\hbar z - \epsilon_{q+k} + \epsilon_{q-4k}} + \frac{2\hbar z - \epsilon_q + \epsilon_{q-2k}}{48} - \frac{\hbar z - \epsilon_q + \epsilon_{q-k}}{30} + \frac{96\epsilon_k}{(2\hbar z - \epsilon_q + \epsilon_{q-2k})^2} + \frac{12\epsilon_k}{(\hbar z - \epsilon_q + \epsilon_{q-k})^2} \right] \\ & - \left(\frac{m}{\hbar^2}\right)^4 \frac{1}{180k^8} \int \frac{d^3q}{(2\pi)^3} \frac{2f_0(q)}{(2\pi)^3} \left[ \frac{30}{5\hbar z - \epsilon_{q+2k} + \epsilon_{q-3k}} + \frac{2\hbar z - \epsilon_{q+k} + \epsilon_{q-k}}{48} - \frac{\hbar z - \epsilon_{q+k} + \epsilon_q}{30} + \frac{96\epsilon_k}{(2\hbar z - \epsilon_{q+k} + \epsilon_q)^2} + \frac{12\epsilon_k}{(\hbar z - \epsilon_{q+k} + \epsilon_q)^2} \right] \\ & - \left(\frac{m}{\hbar^2}\right)^4 \frac{1}{180k^8} \int \frac{d^3q}{(2\pi)^3} \frac{2f_0(q)}{(2\pi)^3} \left[ \frac{18}{3\hbar z - \epsilon_{q+2k} + \epsilon_{q-k}} + \frac{2\hbar z - \epsilon_{q+k} + \epsilon_{q-k}}{48} - \frac{\hbar z - \epsilon_q + \epsilon_{q-k}}{30} - \frac{96\epsilon_k}{(2\hbar z - \epsilon_{q+k} + \epsilon_{q-k})^2} - \frac{12\epsilon_k}{(\hbar z - \epsilon_q + \epsilon_{q-k})^2} \right] \\ & + \left(\frac{m}{\hbar^2}\right)^4 \frac{1}{180k^8} \int \frac{d^3q}{(2\pi)^3} \frac{2f_0(q)}{(2\pi)^3} \left[ \frac{18}{3\hbar z - \epsilon_{q+3k} + \epsilon_q} + \frac{2\hbar z - \epsilon_{q+2k} + \epsilon_q}{48} - \frac{\hbar z - \epsilon_{q+k} - \epsilon_q}{30} - \frac{(2\hbar z - \epsilon_{q+2k} + \epsilon_q)^2}{(\hbar z - \epsilon_{q+k} + \epsilon_q)^2} - \frac{12\epsilon_k}{(\hbar z - \epsilon_{q+k} + \epsilon_q)^2} \right] \\ & + \left(\frac{m}{\hbar^2}\right)^4 \frac{1}{180k^8} \int \frac{d^3q}{(2\pi)^3} \frac{2f_0(q)}{(2\pi)^3} \left[ \frac{6}{\hbar z - \epsilon_q + \epsilon_{q-k}} + \frac{2\hbar z - \epsilon_q + \epsilon_{q-2k}}{48} - \frac{3\hbar z - \epsilon_q + \epsilon_{q-3k}}{90} - \frac{96\epsilon_k}{(2\hbar z - \epsilon_q + \epsilon_{q-2k})^2} - \frac{108\epsilon_k}{(3\hbar z - \epsilon_q + \epsilon_{q-3k})^2} \right] \\ & - \left(\frac{m}{\hbar^2}\right)^4 \frac{1}{180k^8} \int \frac{d^3q}{(2\pi)^3} \frac{2f_0(q)}{(2\pi)^3} \left[ \frac{6}{\hbar z - \epsilon_{q+k} + \epsilon_q} + \frac{2\hbar z - \epsilon_{q+k} + \epsilon_{q-k}}{48} - \frac{3\hbar z - \epsilon_{q+k} + \epsilon_{q-2k}}{90} - \frac{96\epsilon_k}{(2\hbar z - \epsilon_{q+k} + \epsilon_{q-k})^2} - \frac{108\epsilon_k}{(3\hbar z - \epsilon_{q+k} + \epsilon_{q-2k})^2} \right] \\ & - \left(\frac{m}{\hbar^2}\right)^4 \frac{1}{180k^8} \int \frac{d^3q}{(2\pi)^3} \frac{2f_0(q)}{(2\pi)^3} \left[ \frac{144}{-2\hbar z - \epsilon_{q+k} + \epsilon_{q-k}} + \frac{\hbar z - \epsilon_q + \epsilon_{q-k}}{72} + \frac{96\epsilon_k}{(2\hbar z - \epsilon_{q+k} + \epsilon_{q-k})^2} + \frac{48\epsilon_k}{(\hbar z - \epsilon_q + \epsilon_{q-k})^2} + \frac{24\epsilon_k^2}{(\hbar z - \epsilon_q + \epsilon_{q-k})^3} \right] \\ & + \left(\frac{m}{\hbar^2}\right)^4 \frac{1}{180k^8} \int \frac{d^3q}{(2\pi)^3} \frac{2f_0(q)}{(2\pi)^3} \left[ \frac{144}{-2\hbar z - \epsilon_{q+2k} + \epsilon_q} + \frac{\hbar z - \epsilon_{q+k} + \epsilon_q}{72} + \frac{96\epsilon_k}{(2\hbar z - \epsilon_{q+2k} + \epsilon_q)^2} + \frac{48\epsilon_k}{(\hbar z - \epsilon_{q+k} + \epsilon_q)^2} + \frac{24\epsilon_k^2}{(\hbar z - \epsilon_{q+k} + \epsilon_q)^3} \right] \\ & - \left(\frac{m}{\hbar^2}\right)^4 \frac{1}{180k^8} \int \frac{d^3q}{(2\pi)^3} \frac{2f_0(q)}{(2\pi)^3} \left[ \frac{24}{2\hbar z - \epsilon_q + \epsilon_{q-2k}} + \frac{4\hbar z - \epsilon_{q+2k} + \epsilon_{q-2k}}{48} - \frac{\hbar z - \epsilon_q + \epsilon_{q-k}}{24} - \frac{24\epsilon_k^2}{(\hbar z - \epsilon_q + \epsilon_{q-k})^3} \right] \\ & + \left(\frac{m}{\hbar^2}\right)^4 \frac{1}{180k^8} \int \frac{d^3q}{(2\pi)^3} \frac{2f_0(q)}{(2\pi)^3} \left[ \frac{24}{2\hbar z - \epsilon_{q+k} + \epsilon_{q-k}} + \frac{4\hbar z - \epsilon_{q+3k} + \epsilon_{q-k}}{48} - \frac{\hbar z - \epsilon_{q+k} + \epsilon_q}{24} - \frac{24\epsilon_k^2}{(\hbar z - \epsilon_{q+k} + \epsilon_q)^3} \right] \\ & + \left(\frac{m}{\hbar^2}\right)^4 \frac{1}{180k^8} \int \frac{d^3q}{(2\pi)^3} \frac{2f_0(q)}{(2\pi)^3} \left[ \frac{2}{\hbar z - \epsilon_q - \epsilon_{q-k}} - \frac{24}{2\hbar z - \epsilon_{q+k} + \epsilon_{q-k}} + \frac{16}{4\hbar z - \epsilon_{q+3k} + \epsilon_{q-k}} + \frac{18}{3\hbar z - \epsilon_{q+2k} + \epsilon_{q-k}} - \frac{108\epsilon_k}{(3\hbar z - \epsilon_{q+2k} + \epsilon_{q-k})^2} \right] \\ & - \left(\frac{m}{\hbar^2}\right)^4 \frac{1}{180k^8} \int \frac{d^3q}{(2\pi)^3} \frac{2f_0(q)}{(2\pi)^3} \left[ \frac{2}{\hbar z - \epsilon_{q+k} + \epsilon_q} - \frac{24}{2\hbar z - \epsilon_{q+2k} + \epsilon_q} + \frac{16}{4\hbar z - \epsilon_{q+4k} + \epsilon_q} + \frac{18}{3\hbar z - \epsilon_{q+3k} + \epsilon_q} - \frac{108\epsilon_k}{(3\hbar z - \epsilon_{q+3k} + \epsilon_q)^2} \right] \end{aligned}$$



[illegible]



[illegible]

The fractions that contain  $\epsilon_k$  in the nominator lead to non-Lindhard like responses. Fortunately, all these forty-eight terms cancel out each other paving the way for a Mikhailov-type recursion relation. The  $\epsilon_k$  cancellations ultimately leave

$$\begin{aligned}
\chi_0^{(5,5)}(\mathbf{k}, z) = & + \left( \frac{m}{\hbar^2} \right)^4 \frac{1}{180k^8} \int \frac{d^3q}{(2\pi)^3} 2f_0(\mathbf{q}) \\
& \left[ -\frac{5}{16} + \frac{4\hbar z - \epsilon_q + \epsilon_{q-5k}}{16} + \frac{18}{16} - \frac{3\hbar z - \epsilon_q + \epsilon_{q-4k}}{18} + \frac{8}{10} - \frac{2\hbar z - \epsilon_q + \epsilon_{q-2k}}{48} - \frac{1}{8} + \frac{5}{8} - \frac{\hbar z - \epsilon_q + \epsilon_{q-k}}{8} + \frac{5\hbar z - \epsilon_q + \epsilon_{q-4k}}{8} + \frac{\epsilon_{q-k} + \epsilon_{q-4k}}{6} \right. \\
& - \frac{4\hbar z - \epsilon_q + \epsilon_{q-3k}}{10} + \frac{3\hbar z - \epsilon_q + \epsilon_{q-2k}}{18} + \frac{5\hbar z - \epsilon_q + \epsilon_{q-k}}{48} - \frac{4\hbar z - \epsilon_q + \epsilon_{q-4k}}{8} + \frac{2\hbar z - \epsilon_q + \epsilon_{q-2k}}{6} + \frac{\hbar z - \epsilon_q + \epsilon_{q-k}}{8} + \frac{\hbar z - \epsilon_q + \epsilon_{q-4k}}{6} \\
& - \frac{5\hbar z - \epsilon_q + \epsilon_{q-3k}}{30} + \frac{4\hbar z - \epsilon_q + \epsilon_{q-2k}}{48} - \frac{2\hbar z - \epsilon_q + \epsilon_{q-k}}{30} - \frac{\hbar z - \epsilon_q + \epsilon_{q-4k}}{6} - \frac{2\hbar z - \epsilon_q + \epsilon_{q-2k}}{48} + \frac{\hbar z - \epsilon_q + \epsilon_{q-k}}{8} + \frac{\hbar z - \epsilon_q + \epsilon_{q-4k}}{6} \\
& + \frac{5\hbar z - \epsilon_q + \epsilon_{q-4k}}{144} + \frac{2\hbar z - \epsilon_q + \epsilon_{q-2k}}{72} - \frac{\hbar z - \epsilon_q + \epsilon_{q-k}}{18} - \frac{5\hbar z - \epsilon_q + \epsilon_{q-4k}}{48} - \frac{2\hbar z - \epsilon_q + \epsilon_{q-2k}}{30} + \frac{\hbar z - \epsilon_q + \epsilon_{q-k}}{6} + \frac{\hbar z - \epsilon_q + \epsilon_{q-4k}}{18} \\
& - \frac{2\hbar z - \epsilon_q + \epsilon_{q-2k}}{48} + \frac{\hbar z - \epsilon_q + \epsilon_{q-k}}{30} - \frac{3\hbar z - \epsilon_q + \epsilon_{q-4k}}{144} - \frac{2\hbar z - \epsilon_q + \epsilon_{q-2k}}{72} - \frac{\hbar z - \epsilon_q + \epsilon_{q-k}}{18} + \frac{5\hbar z - \epsilon_q + \epsilon_{q-4k}}{48} - \frac{2\hbar z - \epsilon_q + \epsilon_{q-2k}}{30} + \frac{\hbar z - \epsilon_q + \epsilon_{q-k}}{6} \\
& + \frac{2\hbar z - \epsilon_q + \epsilon_{q-2k}}{90} - \frac{\hbar z - \epsilon_q + \epsilon_{q-k}}{6} + \frac{2\hbar z - \epsilon_q + \epsilon_{q-4k}}{48} - \frac{\hbar z - \epsilon_q + \epsilon_{q-2k}}{90} + \frac{\hbar z - \epsilon_q + \epsilon_{q-k}}{24} + \frac{2\hbar z - \epsilon_q + \epsilon_{q-2k}}{48} \\
& - \frac{3\hbar z - \epsilon_q + \epsilon_{q-3k}}{24} - \frac{\hbar z - \epsilon_q + \epsilon_{q-k}}{24} + \frac{2\hbar z - \epsilon_q + \epsilon_{q-2k}}{48} - \frac{3\hbar z - \epsilon_q + \epsilon_{q-4k}}{24} + \frac{2\hbar z - \epsilon_q + \epsilon_{q-2k}}{24} - \frac{4\hbar z - \epsilon_q + \epsilon_{q-4k}}{24} + \frac{\hbar z - \epsilon_q + \epsilon_{q-k}}{24} \\
& + \frac{\hbar z - \epsilon_q + \epsilon_{q-k}}{16} + \frac{2\hbar z - \epsilon_q + \epsilon_{q-2k}}{18} + \frac{4\hbar z - \epsilon_q + \epsilon_{q-4k}}{18} - \frac{\hbar z - \epsilon_q + \epsilon_{q-k}}{18} + \frac{2\hbar z - \epsilon_q + \epsilon_{q-2k}}{18} - \frac{4\hbar z - \epsilon_q + \epsilon_{q-4k}}{18} + \frac{\hbar z - \epsilon_q + \epsilon_{q-k}}{18} \\
& + \frac{4\hbar z - \epsilon_q + \epsilon_{q-3k}}{2} + \frac{3\hbar z - \epsilon_q + \epsilon_{q-2k}}{24} + \frac{\hbar z - \epsilon_q + \epsilon_{q-k}}{16} + \frac{2\hbar z - \epsilon_q + \epsilon_{q-2k}}{18} + \frac{4\hbar z - \epsilon_q + \epsilon_{q-4k}}{18} - \frac{\hbar z - \epsilon_q + \epsilon_{q-k}}{18} + \frac{2\hbar z - \epsilon_q + \epsilon_{q-2k}}{18} - \frac{4\hbar z - \epsilon_q + \epsilon_{q-4k}}{18} + \frac{\hbar z - \epsilon_q + \epsilon_{q-k}}{18} \\
& + \frac{\hbar z - \epsilon_q + \epsilon_{q-k}}{16} - \frac{2\hbar z - \epsilon_q + \epsilon_{q-2k}}{18} + \frac{4\hbar z - \epsilon_q + \epsilon_{q-4k}}{18} - \frac{\hbar z - \epsilon_q + \epsilon_{q-k}}{18} + \frac{2\hbar z - \epsilon_q + \epsilon_{q-2k}}{18} - \frac{4\hbar z - \epsilon_q + \epsilon_{q-4k}}{18} + \frac{\hbar z - \epsilon_q + \epsilon_{q-k}}{18} \\
& - \frac{4\hbar z - \epsilon_q + \epsilon_{q-3k}}{48} - \frac{3\hbar z - \epsilon_q + \epsilon_{q-2k}}{24} - \frac{2\hbar z - \epsilon_q + \epsilon_{q-k}}{144} - \frac{4\hbar z - \epsilon_q + \epsilon_{q-4k}}{72} + \frac{\hbar z - \epsilon_q + \epsilon_{q-k}}{90} + \frac{2\hbar z - \epsilon_q + \epsilon_{q-2k}}{144} - \frac{4\hbar z - \epsilon_q + \epsilon_{q-4k}}{72} + \frac{\hbar z - \epsilon_q + \epsilon_{q-k}}{48} \\
& + \frac{4\hbar z - \epsilon_q + \epsilon_{q-3k}}{90} - \frac{\hbar z - \epsilon_q + \epsilon_{q-k}}{6} + \frac{2\hbar z - \epsilon_q + \epsilon_{q-2k}}{48} - \frac{\hbar z - \epsilon_q + \epsilon_{q-4k}}{90} + \frac{\hbar z - \epsilon_q + \epsilon_{q-k}}{144} + \frac{2\hbar z - \epsilon_q + \epsilon_{q-2k}}{144} - \frac{4\hbar z - \epsilon_q + \epsilon_{q-4k}}{144} + \frac{\hbar z - \epsilon_q + \epsilon_{q-k}}{72} \\
& - \frac{3\hbar z - \epsilon_q + \epsilon_{q-k}}{18} - \frac{2\hbar z - \epsilon_q + \epsilon_{q-2k}}{48} + \frac{\hbar z - \epsilon_q + \epsilon_{q-k}}{30} + \frac{3\hbar z - \epsilon_q + \epsilon_{q-4k}}{18} - \frac{2\hbar z - \epsilon_q + \epsilon_{q-2k}}{48} + \frac{\hbar z - \epsilon_q + \epsilon_{q-k}}{6} + \frac{2\hbar z - \epsilon_q + \epsilon_{q-2k}}{30} - \frac{4\hbar z - \epsilon_q + \epsilon_{q-4k}}{30} + \frac{\hbar z - \epsilon_q + \epsilon_{q-k}}{30} \\
& + \frac{5\hbar z - \epsilon_q + \epsilon_{q-2k}}{8} + \frac{2\hbar z - \epsilon_q + \epsilon_{q-k}}{1} + \frac{\hbar z - \epsilon_q + \epsilon_{q-4k}}{10} - \frac{4\hbar z - \epsilon_q + \epsilon_{q-2k}}{48} + \frac{5\hbar z - \epsilon_q + \epsilon_{q-4k}}{48} - \frac{2\hbar z - \epsilon_q + \epsilon_{q-k}}{8} + \frac{2\hbar z - \epsilon_q + \epsilon_{q-2k}}{8} + \frac{\hbar z - \epsilon_q + \epsilon_{q-k}}{6} \\
& - \frac{2\hbar z - \epsilon_q + \epsilon_{q-2k}}{10} + \frac{\hbar z - \epsilon_q + \epsilon_{q-k}}{48} + \frac{5\hbar z - \epsilon_q + \epsilon_{q-4k}}{48} - \frac{4\hbar z - \epsilon_q + \epsilon_{q-2k}}{8} + \frac{2\hbar z - \epsilon_q + \epsilon_{q-k}}{6} + \frac{2\hbar z - \epsilon_q + \epsilon_{q-2k}}{5} + \frac{\hbar z - \epsilon_q + \epsilon_{q-k}}{16} \\
& - \frac{5\hbar z - \epsilon_q + \epsilon_{q-4k}}{18} + \frac{4\hbar z - \epsilon_q + \epsilon_{q-3k}}{8} + \frac{2\hbar z - \epsilon_q + \epsilon_{q-k}}{24} - \frac{\hbar z - \epsilon_q + \epsilon_{q-4k}}{5} + \frac{5\hbar z - \epsilon_q + \epsilon_{q-4k}}{16} - \frac{4\hbar z - \epsilon_q + \epsilon_{q-k}}{18} + \frac{4\hbar z - \epsilon_q + \epsilon_{q-4k}}{18} + \frac{\hbar z - \epsilon_q + \epsilon_{q-k}}{18} \\
& - \frac{3\hbar z - \epsilon_q + \epsilon_{q-2k}}{18} + \frac{2\hbar z - \epsilon_q + \epsilon_{q-k}}{8} - \frac{\hbar z - \epsilon_q + \epsilon_{q-4k}}{1} + \frac{5\hbar z - \epsilon_q + \epsilon_{q-4k}}{5} - \frac{4\hbar z - \epsilon_q + \epsilon_{q-k}}{16} + \frac{3\hbar z - \epsilon_q + \epsilon_{q-4k}}{18} + \frac{4\hbar z - \epsilon_q + \epsilon_{q-k}}{18} \Rightarrow
\end{aligned}$$

The remaining terms are grouped according to the  $\hbar z$  harmonic of the denominator. There are twelve  $5\hbar z$  terms, sixteen  $4\hbar z$  terms, sixteen  $3\hbar z$  terms, thirty two  $2\hbar z$  terms and thirty two  $\hbar z$  terms. This sorting out leads to

$$\begin{aligned}
\chi_0^{(5,5)}(\mathbf{k}, z) = & + \left( \frac{m}{\hbar^2} \right)^4 \frac{1}{180k^8} \int \frac{d^3q}{(2\pi)^3} 2f_0(\mathbf{q}) \\
& \left[ \begin{aligned}
& - \frac{5}{5} \frac{5\hbar z - \epsilon_q + \epsilon_{q-5k}}{30} + \frac{5\hbar z - \epsilon_q + \epsilon_{q-4k}}{10} + \frac{5\hbar z - \epsilon_q + \epsilon_{q-3k}}{5} + \frac{5\hbar z - \epsilon_q + \epsilon_{q-2k}}{30} + \frac{5\hbar z - \epsilon_q + \epsilon_{q-k}}{10} \\
& - \frac{5\hbar z - \epsilon_q + \epsilon_{q-4k}}{16} + \frac{5\hbar z - \epsilon_q + \epsilon_{q-3k}}{16} + \frac{5\hbar z - \epsilon_q + \epsilon_{q-2k}}{48} + \frac{5\hbar z - \epsilon_q + \epsilon_{q-k}}{48} + \frac{5\hbar z - \epsilon_q + \epsilon_{q-3k}}{48} + \frac{5\hbar z - \epsilon_q + \epsilon_{q-2k}}{48} \\
& + \frac{4\hbar z - \epsilon_q + \epsilon_{q-4k}}{16} + \frac{4\hbar z - \epsilon_q + \epsilon_{q-3k}}{16} + \frac{4\hbar z - \epsilon_q + \epsilon_{q-2k}}{48} + \frac{4\hbar z - \epsilon_q + \epsilon_{q-k}}{48} + \frac{4\hbar z - \epsilon_q + \epsilon_{q-3k}}{48} + \frac{4\hbar z - \epsilon_q + \epsilon_{q-2k}}{48} \\
& + \frac{4\hbar z - \epsilon_q + \epsilon_{q-3k}}{48} + \frac{4\hbar z - \epsilon_q + \epsilon_{q-2k}}{48} + \frac{4\hbar z - \epsilon_q + \epsilon_{q-k}}{16} + \frac{4\hbar z - \epsilon_q + \epsilon_{q-3k}}{16} + \frac{4\hbar z - \epsilon_q + \epsilon_{q-2k}}{16} + \frac{4\hbar z - \epsilon_q + \epsilon_{q-k}}{16} \\
& - \frac{4\hbar z - \epsilon_q + \epsilon_{q-2k}}{18} + \frac{4\hbar z - \epsilon_q + \epsilon_{q-3k}}{18} + \frac{4\hbar z - \epsilon_q + \epsilon_{q-k}}{90} + \frac{4\hbar z - \epsilon_q + \epsilon_{q-3k}}{90} + \frac{4\hbar z - \epsilon_q + \epsilon_{q-2k}}{90} + \frac{4\hbar z - \epsilon_q + \epsilon_{q-k}}{90} \\
& - \frac{3\hbar z - \epsilon_q + \epsilon_{q-2k}}{18} + \frac{3\hbar z - \epsilon_q + \epsilon_{q-3k}}{18} + \frac{3\hbar z - \epsilon_q + \epsilon_{q-k}}{90} + \frac{3\hbar z - \epsilon_q + \epsilon_{q-3k}}{90} + \frac{3\hbar z - \epsilon_q + \epsilon_{q-2k}}{90} + \frac{3\hbar z - \epsilon_q + \epsilon_{q-k}}{90} \\
& + \frac{3\hbar z - \epsilon_q + \epsilon_{q-3k}}{18} + \frac{3\hbar z - \epsilon_q + \epsilon_{q-2k}}{18} + \frac{3\hbar z - \epsilon_q + \epsilon_{q-k}}{8} + \frac{3\hbar z - \epsilon_q + \epsilon_{q-3k}}{8} + \frac{3\hbar z - \epsilon_q + \epsilon_{q-2k}}{8} + \frac{3\hbar z - \epsilon_q + \epsilon_{q-k}}{8} \\
& - \frac{3\hbar z - \epsilon_q + \epsilon_{q-2k}}{48} + \frac{3\hbar z - \epsilon_q + \epsilon_{q-3k}}{48} + \frac{3\hbar z - \epsilon_q + \epsilon_{q-k}}{144} + \frac{3\hbar z - \epsilon_q + \epsilon_{q-3k}}{144} + \frac{3\hbar z - \epsilon_q + \epsilon_{q-2k}}{144} + \frac{3\hbar z - \epsilon_q + \epsilon_{q-k}}{144} \\
& + \frac{2\hbar z - \epsilon_q + \epsilon_{q-2k}}{48} + \frac{2\hbar z - \epsilon_q + \epsilon_{q-3k}}{48} + \frac{2\hbar z - \epsilon_q + \epsilon_{q-k}}{24} + \frac{2\hbar z - \epsilon_q + \epsilon_{q-3k}}{24} + \frac{2\hbar z - \epsilon_q + \epsilon_{q-2k}}{24} + \frac{2\hbar z - \epsilon_q + \epsilon_{q-k}}{24} \\
& + \frac{2\hbar z - \epsilon_q + \epsilon_{q-2k}}{24} + \frac{2\hbar z - \epsilon_q + \epsilon_{q-3k}}{24} + \frac{2\hbar z - \epsilon_q + \epsilon_{q-k}}{24} + \frac{2\hbar z - \epsilon_q + \epsilon_{q-3k}}{24} + \frac{2\hbar z - \epsilon_q + \epsilon_{q-2k}}{24} + \frac{2\hbar z - \epsilon_q + \epsilon_{q-k}}{24} \\
& - \frac{2\hbar z - \epsilon_q + \epsilon_{q-2k}}{48} + \frac{2\hbar z - \epsilon_q + \epsilon_{q-3k}}{48} + \frac{2\hbar z - \epsilon_q + \epsilon_{q-k}}{48} + \frac{2\hbar z - \epsilon_q + \epsilon_{q-3k}}{48} + \frac{2\hbar z - \epsilon_q + \epsilon_{q-2k}}{48} + \frac{2\hbar z - \epsilon_q + \epsilon_{q-k}}{48} \\
& - \frac{2\hbar z - \epsilon_q + \epsilon_{q-2k}}{8} + \frac{2\hbar z - \epsilon_q + \epsilon_{q-3k}}{8} + \frac{2\hbar z - \epsilon_q + \epsilon_{q-k}}{8} + \frac{2\hbar z - \epsilon_q + \epsilon_{q-3k}}{8} + \frac{2\hbar z - \epsilon_q + \epsilon_{q-2k}}{8} + \frac{2\hbar z - \epsilon_q + \epsilon_{q-k}}{8} \\
& - \frac{2\hbar z - \epsilon_q + \epsilon_{q-2k}}{6} + \frac{2\hbar z - \epsilon_q + \epsilon_{q-3k}}{30} + \frac{2\hbar z - \epsilon_q + \epsilon_{q-k}}{30} + \frac{2\hbar z - \epsilon_q + \epsilon_{q-3k}}{30} + \frac{2\hbar z - \epsilon_q + \epsilon_{q-2k}}{30} + \frac{2\hbar z - \epsilon_q + \epsilon_{q-k}}{30} \\
& - \frac{\hbar z - \epsilon_q + \epsilon_q}{30} + \frac{\hbar z - \epsilon_q + \epsilon_q}{72} + \frac{\hbar z - \epsilon_q + \epsilon_q}{6} + \frac{\hbar z - \epsilon_q + \epsilon_q}{6} + \frac{\hbar z - \epsilon_q + \epsilon_q}{24} + \frac{\hbar z - \epsilon_q + \epsilon_q}{24} \\
& - \frac{\hbar z - \epsilon_q + \epsilon_q}{2} + \frac{\hbar z - \epsilon_q + \epsilon_q}{2} + \frac{\hbar z - \epsilon_q + \epsilon_q}{2} + \frac{\hbar z - \epsilon_q + \epsilon_q}{2} + \frac{\hbar z - \epsilon_q + \epsilon_q}{24} + \frac{\hbar z - \epsilon_q + \epsilon_q}{24} \\
& + \frac{\hbar z - \epsilon_q + \epsilon_q}{72} + \frac{\hbar z - \epsilon_q + \epsilon_q}{6} + \frac{\hbar z - \epsilon_q + \epsilon_q}{6} + \frac{\hbar z - \epsilon_q + \epsilon_q}{72} + \frac{\hbar z - \epsilon_q + \epsilon_q}{30} + \frac{\hbar z - \epsilon_q + \epsilon_q}{30} \\
& - \frac{\hbar z - \epsilon_q + \epsilon_q}{30} + \frac{\hbar z - \epsilon_q + \epsilon_q}{30} + \frac{\hbar z - \epsilon_q + \epsilon_q}{1} + \frac{\hbar z - \epsilon_q + \epsilon_q}{6} + \frac{\hbar z - \epsilon_q + \epsilon_q}{6} + \frac{\hbar z - \epsilon_q + \epsilon_q}{1} \\
& - \frac{\hbar z - \epsilon_q + \epsilon_q}{30} + \frac{\hbar z - \epsilon_q + \epsilon_q}{30} + \frac{\hbar z - \epsilon_q + \epsilon_q}{1} + \frac{\hbar z - \epsilon_q + \epsilon_q}{6} + \frac{\hbar z - \epsilon_q + \epsilon_q}{6} + \frac{\hbar z - \epsilon_q + \epsilon_q}{1} \Rightarrow
\end{aligned} \right]
\end{aligned}$$

The Lindhard-like responses are isolated and  $176 = 128 + 48$  is employed for the seemingly unpaired three responses. The algebraic identities  $(\epsilon_{q+2k} - \epsilon_{q-2k})/2 = (\epsilon_{q+k} - \epsilon_{q-k}) = 4q \cdot k$  and  $(\epsilon_{q+3k} - \epsilon_{q-k})/2 = (\epsilon_{q+2k} - \epsilon_q) = 4k^2 + 4q \cdot k$  yield

$$\begin{aligned}
& \chi_0^{(5,5)}(\mathbf{k}, z) = + \left( \frac{m}{\hbar^2} \right)^4 \frac{1}{180k^8} \int \frac{d^3q}{(2\pi)^3} 2f_0(\mathbf{q}) \left[ + \frac{5}{5\hbar z - \epsilon_q + 5k} + \epsilon_q - \frac{5}{5\hbar z - \epsilon_q + 5k} + \frac{45}{5\hbar z - \epsilon_q + 4k} + \epsilon_q - k - \frac{40}{5\hbar z - \epsilon_q + 3k} + \epsilon_q - 2k \right. \\
& + \frac{32}{4\hbar z - \epsilon_q + \epsilon_{q-4k}} - \frac{4\hbar z - \epsilon_q + 4k + \epsilon_q}{108} + \frac{4\hbar z - \epsilon_q + 3k + \epsilon_q - 3k}{108} + \frac{4\hbar z - \epsilon_q + 2k + \epsilon_q - 2k}{160} \\
& + \frac{3\hbar z - \epsilon_q + 3k + \epsilon_q}{24} - \frac{3\hbar z - \epsilon_q + 2k + \epsilon_q - k}{108} + \frac{3\hbar z - \epsilon_q + k + \epsilon_q - 2k}{70} + \frac{2\hbar z - \epsilon_q + 2k + \epsilon_q}{160} \\
& + \left. \frac{2\hbar z - \epsilon_q + k + \epsilon_q - k}{24} - \frac{2\hbar z - \epsilon_q + 2k + \epsilon_q}{70} + \frac{\hbar z - \epsilon_q + \epsilon_q - k}{70} + \frac{\hbar z - \epsilon_q + k + \epsilon_q}{70} \right] \Rightarrow \\
& \chi_0^{(5,5)}(\mathbf{k}, z) = + \left( \frac{m}{\hbar^2} \right)^4 \frac{1}{180k^8} \int \frac{d^3q}{(2\pi)^3} 2f_0(\mathbf{q}) \left[ + \frac{5}{5\hbar z - \epsilon_q + 5k} + \epsilon_q - \frac{5}{5\hbar z - \epsilon_q + 5k} + \frac{32}{4\hbar z - \epsilon_q + 4k} + \epsilon_q - \frac{32}{4\hbar z - \epsilon_q + 4k} + \frac{108}{3\hbar z - \epsilon_q + 3k} \right. \\
& - \frac{160}{2\hbar z - \epsilon_q + 2k} + \frac{2\hbar z - \epsilon_q + \epsilon_{q-2k}}{40} + \frac{\hbar z - \epsilon_q + \epsilon_q - k}{128} + \frac{\hbar z - \epsilon_q + \epsilon_q - k}{128} + \frac{5\hbar z - \epsilon_q + 4k + \epsilon_q - k}{108} \\
& - \frac{5\hbar z - \epsilon_q + 2k + \epsilon_{q-3k}}{108} + \frac{5\hbar z - \epsilon_q + 3k + \epsilon_{q-2k}}{48} + \frac{4\hbar z - \epsilon_q + k + \epsilon_q - k}{24} + \frac{3\hbar z - \epsilon_q + 2k + \epsilon_q - k}{24} \Rightarrow \\
& + \frac{3\hbar z - \epsilon_q + k + \epsilon_q - 2k}{48} - \frac{4\hbar z - \epsilon_q + 2k + \epsilon_q - 2k}{48} + \frac{2\hbar z - \epsilon_q + k + \epsilon_q - k}{24} + \frac{2\hbar z - \epsilon_q + 2k + \epsilon_q}{24} \Rightarrow \\
& \chi_0^{(5,5)}(\mathbf{k}, z) = + \left( \frac{m}{\hbar^2} \right)^4 \frac{1}{180k^8} \int \frac{d^3q}{(2\pi)^3} 2f_0(\mathbf{q}) \left[ + \frac{5}{5\hbar z - \epsilon_q + 5k} + \epsilon_q - \frac{5}{5\hbar z - \epsilon_q + 5k} + \frac{32}{4\hbar z - \epsilon_q + 4k} + \epsilon_q - \frac{32}{4\hbar z - \epsilon_q + 4k} + \frac{108}{3\hbar z - \epsilon_q + 3k} \right. \\
& - \frac{160}{2\hbar z - \epsilon_q + 2k} + \frac{2\hbar z - \epsilon_q + \epsilon_{q-2k}}{40} + \frac{\hbar z - \epsilon_q + \epsilon_q - k}{128} + \frac{\hbar z - \epsilon_q + \epsilon_q - k}{128} + \frac{5\hbar z - \epsilon_q + 4k + \epsilon_q - k}{108} \\
& - \frac{5\hbar z - \epsilon_q + 2k + \epsilon_{q-3k}}{108} + \frac{5\hbar z - \epsilon_q + 3k + \epsilon_{q-2k}}{48} + \frac{4\hbar z - \epsilon_q + k + \epsilon_q - k}{24} + \frac{3\hbar z - \epsilon_q + 2k + \epsilon_q - k}{24} \Rightarrow \\
& - \frac{2\hbar z - \epsilon_q + k + \epsilon_q - 2k}{48} + \frac{2\hbar z - \epsilon_q + 2k + \epsilon_q - 2k}{48} + \frac{2\hbar z - \epsilon_q + k + \epsilon_q - k}{24} + \frac{2\hbar z - \epsilon_q + 2k + \epsilon_q}{24} \Rightarrow \\
& - \frac{2\hbar z - \epsilon_q + 2k + \epsilon_q}{40} + \frac{2\hbar z - \epsilon_q + \epsilon_{q-2k}}{40} + \frac{\hbar z - \epsilon_q + \epsilon_q - k}{128} + \frac{\hbar z - \epsilon_q + \epsilon_q - k}{128} + \frac{5\hbar z - \epsilon_q + 4k + \epsilon_q - k}{108} \\
& - \frac{5\hbar z - \epsilon_q + 2k + \epsilon_{q-3k}}{108} + \frac{5\hbar z - \epsilon_q + 3k + \epsilon_{q-2k}}{48} + \frac{4\hbar z - \epsilon_q + k + \epsilon_q - k}{24} + \frac{3\hbar z - \epsilon_q + 2k + \epsilon_q - k}{24} \Rightarrow \\
& - \frac{2\hbar z - \epsilon_q + k + \epsilon_q - 2k}{48} + \frac{2\hbar z - \epsilon_q + 2k + \epsilon_q - 2k}{48} + \frac{2\hbar z - \epsilon_q + k + \epsilon_q - k}{24} + \frac{2\hbar z - \epsilon_q + 2k + \epsilon_q}{24} \Rightarrow \\
& \chi_0^{(5,5)}(\mathbf{k}, z) = + \left( \frac{m}{\hbar^2} \right)^4 \frac{1}{180k^8} \int \frac{d^3q}{(2\pi)^3} 2f_0(\mathbf{q}) \left[ + \frac{5}{5\hbar z - \epsilon_q + 5k} + \epsilon_q - \frac{5}{5\hbar z - \epsilon_q + 5k} + \frac{32}{4\hbar z - \epsilon_q + 4k} + \epsilon_q - \frac{32}{4\hbar z - \epsilon_q + 4k} + \frac{108}{3\hbar z - \epsilon_q + 3k} \right. \\
& - \frac{160}{2\hbar z - \epsilon_q + 2k} + \frac{2\hbar z - \epsilon_q + \epsilon_{q-2k}}{40} + \frac{\hbar z - \epsilon_q + \epsilon_q - k}{128} + \frac{\hbar z - \epsilon_q + \epsilon_q - k}{128} + \frac{5\hbar z - \epsilon_q + 4k + \epsilon_q - k}{108} \\
& - \frac{5\hbar z - \epsilon_q + 2k + \epsilon_{q-3k}}{108} + \frac{5\hbar z - \epsilon_q + 3k + \epsilon_{q-2k}}{48} + \frac{4\hbar z - \epsilon_q + k + \epsilon_q - k}{24} + \frac{3\hbar z - \epsilon_q + 2k + \epsilon_q - k}{24} \Rightarrow \\
& - \frac{2\hbar z - \epsilon_q + k + \epsilon_q - 2k}{48} + \frac{2\hbar z - \epsilon_q + 2k + \epsilon_q - 2k}{48} + \frac{2\hbar z - \epsilon_q + k + \epsilon_q - k}{24} + \frac{2\hbar z - \epsilon_q + 2k + \epsilon_q}{24} \Rightarrow \\
& - \frac{2\hbar z - \epsilon_q + 2k + \epsilon_q}{40} + \frac{2\hbar z - \epsilon_q + \epsilon_{q-2k}}{40} + \frac{\hbar z - \epsilon_q + \epsilon_q - k}{128} + \frac{\hbar z - \epsilon_q + \epsilon_q - k}{128} + \frac{5\hbar z - \epsilon_q + 4k + \epsilon_q - k}{108} \\
& - \frac{5\hbar z - \epsilon_q + 2k + \epsilon_{q-3k}}{108} + \frac{5\hbar z - \epsilon_q + 3k + \epsilon_{q-2k}}{48} + \frac{4\hbar z - \epsilon_q + k + \epsilon_q - k}{24} + \frac{3\hbar z - \epsilon_q + 2k + \epsilon_q - k}{24} \Rightarrow \\
& - \frac{2\hbar z - \epsilon_q + k + \epsilon_q - 2k}{48} + \frac{2\hbar z - \epsilon_q + 2k + \epsilon_q - 2k}{48} + \frac{2\hbar z - \epsilon_q + k + \epsilon_q - k}{24} + \frac{2\hbar z - \epsilon_q + 2k + \epsilon_q}{24} \Rightarrow
\end{aligned}$$



[illegible]

Some straightforward algebra is carried out.

$$\begin{aligned} \chi_0^{(5,5)}(\mathbf{k}, z) = & + \left( \frac{m}{\hbar^2} \right)^4 \frac{1}{180k^8} \int \frac{d^3q}{(2\pi)^3} 2f_0(\mathbf{q}) \left[ + \frac{5}{5\hbar z - \epsilon_q + 5k} - \frac{5}{5\hbar z - \epsilon_q + \epsilon_q - 5k} - \frac{32}{4\hbar z - \epsilon_q + \epsilon_q} + \frac{32}{4\hbar z - \epsilon_q + \epsilon_q - 4k} \right. \\ & \left. + \frac{81}{3\hbar z - \epsilon_q + 3k} - \frac{81}{3\hbar z - \epsilon_q + \epsilon_q - 3k} - \frac{96}{2\hbar z - \epsilon_q + 2k} + \frac{96}{2\hbar z - \epsilon_q + \epsilon_q - 2k} + \frac{42}{\hbar z - \epsilon_q + k} - \frac{42}{\hbar z - \epsilon_q + \epsilon_q - k} \right]. \end{aligned}$$

One ends up with ten unique terms that can be expressed as an algebraic combination of five ideal Lindhard first order density responses, that are evaluated at different multiple wavenumber and complex frequency arguments. In particular, the ideal Lindhard density responses of interest are

$$\begin{aligned} \chi_0(\mathbf{k}, z) &= \int \frac{d^3q}{(2\pi)^3} 2f_0(\mathbf{q}) \left[ \frac{1}{\hbar z - \epsilon_q + k} - \frac{1}{\hbar z - \epsilon_q + \epsilon_q - k} \right], \\ \chi_0(2\mathbf{k}, 2z) &= \int \frac{d^3q}{(2\pi)^3} 2f_0(\mathbf{q}) \left[ \frac{1}{\hbar(2z) - \epsilon_q + 2k} - \frac{1}{\hbar(2z) - \epsilon_q + \epsilon_q - 2k} \right], \\ \chi_0(3\mathbf{k}, 3z) &= \int \frac{d^3q}{(2\pi)^3} 2f_0(\mathbf{q}) \left[ \frac{1}{\hbar(3z) - \epsilon_q + 3k} - \frac{1}{\hbar(3z) - \epsilon_q + \epsilon_q - 3k} \right], \\ \chi_0(4\mathbf{k}, 4z) &= \int \frac{d^3q}{(2\pi)^3} 2f_0(\mathbf{q}) \left[ \frac{1}{\hbar(4z) - \epsilon_q + 4k} - \frac{1}{\hbar(4z) - \epsilon_q + \epsilon_q - 4k} \right], \\ \chi_0(5\mathbf{k}, 5z) &= \int \frac{d^3q}{(2\pi)^3} 2f_0(\mathbf{q}) \left[ \frac{1}{\hbar(5z) - \epsilon_q + 5k} - \frac{1}{\hbar(5z) - \epsilon_q + \epsilon_q - 5k} \right]. \end{aligned}$$

Ultimately, a fifth order recursion relation emerges that expresses the symmetric fifth order ideal density response in terms of the first order ideal density response.

$$\begin{aligned} \chi_0^{(5,5)}(\mathbf{k}, z) = & + \left( \frac{m}{\hbar^2} \right)^4 \frac{1}{180k^8} (+5) \int \frac{d^3q}{(2\pi)^3} 2f_0(\mathbf{q}) \left[ \frac{1}{5\hbar z - \epsilon_q + 5k} - \frac{1}{5\hbar z - \epsilon_q + \epsilon_q - 5k} \right] \\ & + \left( \frac{m}{\hbar^2} \right)^4 \frac{1}{180k^8} (-32) \int \frac{d^3q}{(2\pi)^3} 2f_0(\mathbf{q}) \left[ \frac{1}{4\hbar z - \epsilon_q + 4k} - \frac{1}{4\hbar z - \epsilon_q + \epsilon_q - 4k} \right] \\ & + \left( \frac{m}{\hbar^2} \right)^4 \frac{1}{180k^8} (+81) \int \frac{d^3q}{(2\pi)^3} 2f_0(\mathbf{q}) \left[ \frac{1}{3\hbar z - \epsilon_q + 3k} - \frac{1}{3\hbar z - \epsilon_q + \epsilon_q - 3k} \right] \\ & + \left( \frac{m}{\hbar^2} \right)^4 \frac{1}{180k^8} (-96) \int \frac{d^3q}{(2\pi)^3} 2f_0(\mathbf{q}) \left[ \frac{1}{2\hbar z - \epsilon_q + 2k} - \frac{1}{2\hbar z - \epsilon_q + \epsilon_q - 2k} \right] \\ & + \left( \frac{m}{\hbar^2} \right)^4 \frac{1}{180k^8} (+42) \int \frac{d^3q}{(2\pi)^3} 2f_0(\mathbf{q}) \left[ \frac{1}{\hbar z - \epsilon_q + k} - \frac{1}{\hbar z - \epsilon_q + \epsilon_q - k} \right] \Rightarrow \\ \chi_0^{(5,5)}(\mathbf{k}, z) = & + \left( \frac{m}{\hbar^2} \right)^4 \frac{1}{180k^8} [5\chi_0(5\mathbf{k}, 5z) - 32\chi_0(4\mathbf{k}, 4z) + 81\chi_0(3\mathbf{k}, 3z) - 96\chi_0(2\mathbf{k}, 2z) + 42\chi_0(\mathbf{k}, z)]. \end{aligned}$$

Overall, we end up with the compact recursion relation

$$\chi_0^{(5,5)}(\mathbf{k}, z) = + \left( \frac{m}{\hbar^2} \right)^4 \frac{1}{180k^8} [5\chi_0(5\mathbf{k}, 5z) - 32\chi_0(4\mathbf{k}, 4z) + 81\chi_0(3\mathbf{k}, 3z) - 96\chi_0(2\mathbf{k}, 2z) + 42\chi_0(\mathbf{k}, z)].$$

**The normalized compact form of the symmetric expression.** From the definition of the fifth order ideal density response as the fifth order functional derivative of the density with respect to the external potential energy, it is evident that the proper normalization is achieved by dividing with  $1/(n\beta^5)$ . In addition from the definition of the first order ideal density response as the first order functional derivative of the density with respect to the external potential energy, it is evident that the proper normalization of the Lindhard response is achieved by dividing with  $1/(n\beta)$ . The calculation proceeds with the introduction of the dimensionless complex frequency  $z = (T/\hbar)Z$  as well as of the dimensionless wavenumber  $k = k_F x$ . The utilization of the Fermi energy definition  $E_F = \hbar^2 k_F^2 / (2m)$  and the introduction of the degeneracy temperature definition  $\Theta = T/E_F$  ultimately lead to

$$\begin{aligned}
\chi_0^{(5,5)}(\mathbf{k}, z) &= + \left( \frac{m}{\hbar^2} \right)^4 \frac{1}{180k^8} [5\chi_0(5\mathbf{k}, 5z) - 32\chi_0(4\mathbf{k}, 4z) + 81\chi_0(3\mathbf{k}, 3z) - 96\chi_0(2\mathbf{k}, 2z) + 42\chi_0(\mathbf{k}, z)] \Rightarrow \\
\frac{\chi_0^{(5,5)}(\mathbf{k}, z)}{n\beta^5} &= + \frac{1}{n\beta^5} \left( \frac{m}{\hbar^2} \right)^4 \frac{1}{180k^8} [5\chi_0(5\mathbf{k}, 5z) - 32\chi_0(4\mathbf{k}, 4z) + 81\chi_0(3\mathbf{k}, 3z) - 96\chi_0(2\mathbf{k}, 2z) + 42\chi_0(\mathbf{k}, z)] \Rightarrow \\
\frac{\chi_0^{(5,5)}(\mathbf{k}, z)}{n\beta^5} &= + \left( \frac{m}{\hbar^2} \right)^4 \frac{T^4}{180k^8} \left[ 5 \frac{\chi_0(5\mathbf{k}, 5z)}{n\beta} - 32 \frac{\chi_0(4\mathbf{k}, 4z)}{n\beta} + 81 \frac{\chi_0(3\mathbf{k}, 3z)}{n\beta} - 96 \frac{\chi_0(2\mathbf{k}, 2z)}{n\beta} + 42 \frac{\chi_0(\mathbf{k}, z)}{n\beta} \right] \Rightarrow \\
\frac{\chi_0^{(5,5)}(\mathbf{x}, Z)}{n\beta^5} &= + \left( \frac{m}{\hbar^2} \right)^4 \frac{T^4}{180k_F^8 x^8} \left[ 5 \frac{\chi_0(5\mathbf{x}, 5Z)}{n\beta} - 32 \frac{\chi_0(4\mathbf{x}, 4Z)}{n\beta} + 81 \frac{\chi_0(3\mathbf{x}, 3Z)}{n\beta} - 96 \frac{\chi_0(2\mathbf{x}, 2Z)}{n\beta} + 42 \frac{\chi_0(\mathbf{x}, Z)}{n\beta} \right] \Rightarrow \\
\frac{\chi_0^{(5,5)}(\mathbf{x}, Z)}{n\beta^5} &= + \left( \frac{2m}{\hbar^2 k_F^2} \right)^4 \frac{1}{2^4} \frac{T^4}{180x^8} \left[ 5 \frac{\chi_0(5\mathbf{x}, 5Z)}{n\beta} - 32 \frac{\chi_0(4\mathbf{x}, 4Z)}{n\beta} + 81 \frac{\chi_0(3\mathbf{x}, 3Z)}{n\beta} - 96 \frac{\chi_0(2\mathbf{x}, 2Z)}{n\beta} + 42 \frac{\chi_0(\mathbf{x}, Z)}{n\beta} \right] \Rightarrow \\
\frac{\chi_0^{(5,5)}(\mathbf{x}, Z)}{n\beta^5} &= + \frac{T^4}{[ \hbar^2 k_F^2 / (2m) ]^4} \frac{1}{2^4} \frac{1}{180x^8} \left[ 5 \frac{\chi_0(5\mathbf{x}, 5Z)}{n\beta} - 32 \frac{\chi_0(4\mathbf{x}, 4Z)}{n\beta} + 81 \frac{\chi_0(3\mathbf{x}, 3Z)}{n\beta} - 96 \frac{\chi_0(2\mathbf{x}, 2Z)}{n\beta} + 42 \frac{\chi_0(\mathbf{x}, Z)}{n\beta} \right] \Rightarrow \\
\frac{\chi_0^{(5,5)}(\mathbf{x}, Z)}{n\beta^5} &= + \frac{T^4}{E_F^4} \frac{1}{2^4} \frac{1}{180x^8} \left[ 5 \frac{\chi_0(5\mathbf{x}, 5Z)}{n\beta} - 32 \frac{\chi_0(4\mathbf{x}, 4Z)}{n\beta} + 81 \frac{\chi_0(3\mathbf{x}, 3Z)}{n\beta} - 96 \frac{\chi_0(2\mathbf{x}, 2Z)}{n\beta} + 42 \frac{\chi_0(\mathbf{x}, Z)}{n\beta} \right] \Rightarrow \\
\frac{\chi_0^{(5,5)}(\mathbf{x}, Z)}{n\beta^5} &= + \frac{1}{2^4} \frac{1}{180} \frac{\Theta^4}{x^8} \left[ 5 \frac{\chi_0(5\mathbf{x}, 5Z)}{n\beta} - 32 \frac{\chi_0(4\mathbf{x}, 4Z)}{n\beta} + 81 \frac{\chi_0(3\mathbf{x}, 3Z)}{n\beta} - 96 \frac{\chi_0(2\mathbf{x}, 2Z)}{n\beta} + 42 \frac{\chi_0(\mathbf{x}, Z)}{n\beta} \right] \Rightarrow \\
\frac{\chi_0^{(5,5)}(\mathbf{x}, Z)}{n\beta^5} &= + \frac{1}{2 \times 2 \times 4} \frac{1}{3 \times 3 \times 4 \times 5} \frac{\Theta^4}{x^8} \left[ 5 \frac{\chi_0(5\mathbf{x}, 5Z)}{n\beta} - 32 \frac{\chi_0(4\mathbf{x}, 4Z)}{n\beta} + 81 \frac{\chi_0(3\mathbf{x}, 3Z)}{n\beta} - 96 \frac{\chi_0(2\mathbf{x}, 2Z)}{n\beta} + 42 \frac{\chi_0(\mathbf{x}, Z)}{n\beta} \right] \Rightarrow \\
\frac{\chi_0^{(5,5)}(\mathbf{x}, Z)}{n\beta^5} &= + \frac{1}{2 \times 3 \times 4} \frac{1}{2 \times 3 \times 4 \times 5} \frac{\Theta^4}{x^8} \left[ 5 \frac{\chi_0(5\mathbf{x}, 5Z)}{n\beta} - 32 \frac{\chi_0(4\mathbf{x}, 4Z)}{n\beta} + 81 \frac{\chi_0(3\mathbf{x}, 3Z)}{n\beta} - 96 \frac{\chi_0(2\mathbf{x}, 2Z)}{n\beta} + 42 \frac{\chi_0(\mathbf{x}, Z)}{n\beta} \right] \Rightarrow \\
\frac{\chi_0^{(5,5)}(\mathbf{x}, Z)}{n\beta^5} &= + \frac{1}{4!5!} \frac{\Theta^4}{x^8} \left[ 5 \frac{\chi_0(5\mathbf{x}, 5Z)}{n\beta} - 32 \frac{\chi_0(4\mathbf{x}, 4Z)}{n\beta} + 81 \frac{\chi_0(3\mathbf{x}, 3Z)}{n\beta} - 96 \frac{\chi_0(2\mathbf{x}, 2Z)}{n\beta} + 42 \frac{\chi_0(\mathbf{x}, Z)}{n\beta} \right].
\end{aligned}$$

In the final steps, the numerical pre-factors were decomposed into products that were later expressed as factorials with respect to the order of the ideal density response. Ultimately, one has

$$\frac{\chi_0^{(5,5)}(\mathbf{x}, Z)}{n\beta^5} = + \frac{1}{(5-1)!5!} \frac{\Theta^4}{x^8} \left[ 5 \frac{\chi_0(5\mathbf{x}, 5Z)}{n\beta} - 32 \frac{\chi_0(4\mathbf{x}, 4Z)}{n\beta} + 81 \frac{\chi_0(3\mathbf{x}, 3Z)}{n\beta} - 96 \frac{\chi_0(2\mathbf{x}, 2Z)}{n\beta} + 42 \frac{\chi_0(\mathbf{x}, Z)}{n\beta} \right].$$

**The long wavelength limit of the static normalized symmetric expression.** The long-wavelength limit of the static fifth order ideal density response at the fifth harmonic should converge. Given the  $1/x^8$  pre-factor and the even parity, this implies that the first four terms of the small argument expansion of the ideal quintic density response should cancel out exactly, otherwise the long-wavelength limit of the static case would diverge. We first write down the first five terms of the small argument expansion of the ideal Lindhard density response for the arguments  $5\mathbf{x}$ ,  $4\mathbf{x}$ ,  $3\mathbf{x}$ ,  $2\mathbf{x}$ ,  $\mathbf{x}$ .

$$\begin{aligned}\frac{\chi_0(\mathbf{x})}{n\beta} &\simeq -\frac{3}{2}\Theta \int_0^\infty dy f_0(y; \Theta) \left[ 1 + \frac{1}{12} \left(\frac{x}{y}\right)^2 + \frac{1}{5} \frac{1}{16} \left(\frac{x}{y}\right)^4 + \frac{1}{7} \frac{1}{64} \left(\frac{x}{y}\right)^6 + \frac{1}{9} \frac{1}{256} \left(\frac{x}{y}\right)^8 \right], \\ \frac{\chi_0(2\mathbf{x})}{n\beta} &\simeq -\frac{3}{2}\Theta \int_0^\infty dy f_0(y; \Theta) \left[ 1 + \frac{1}{3} \left(\frac{x}{y}\right)^2 + \frac{1}{5} \left(\frac{x}{y}\right)^4 + \frac{1}{7} \left(\frac{x}{y}\right)^6 + \frac{1}{9} \left(\frac{x}{y}\right)^8 \right], \\ \frac{\chi_0(3\mathbf{x})}{n\beta} &\simeq -\frac{3}{2}\Theta \int_0^\infty dy f_0(y; \Theta) \left[ 1 + \frac{3}{4} \left(\frac{x}{y}\right)^2 + \frac{1}{5} \frac{1}{16} \left(\frac{x}{y}\right)^4 + \frac{1}{7} \frac{1}{64} \left(\frac{x}{y}\right)^6 + \frac{1}{9} \frac{1}{256} \left(\frac{x}{y}\right)^8 \right], \\ \frac{\chi_0(4\mathbf{x})}{n\beta} &\simeq -\frac{3}{2}\Theta \int_0^\infty dy f_0(y; \Theta) \left[ 1 + \frac{4}{3} \left(\frac{x}{y}\right)^2 + \frac{16}{5} \left(\frac{x}{y}\right)^4 + \frac{64}{7} \left(\frac{x}{y}\right)^6 + \frac{256}{9} \left(\frac{x}{y}\right)^8 \right], \\ \frac{\chi_0(5\mathbf{x})}{n\beta} &\simeq -\frac{3}{2}\Theta \int_0^\infty dy f_0(y; \Theta) \left[ 1 + \frac{25}{12} \left(\frac{x}{y}\right)^2 + \frac{125}{16} \left(\frac{x}{y}\right)^4 + \frac{1}{7} \frac{15625}{64} \left(\frac{x}{y}\right)^6 + \frac{1}{9} \frac{390625}{256} \left(\frac{x}{y}\right)^8 \right],\end{aligned}$$

We then substitute in the static limit of the normalized compact form of the fifth order ideal density response at the fifth harmonic

$$\begin{aligned}\frac{\chi_0^{(5,5)}(\mathbf{x}, Z)}{n\beta^5} &= +\frac{1}{(5-1)!5!} \frac{\Theta^4}{x^8} \left[ \frac{5\chi_0(5\mathbf{x}, 5Z)}{n\beta} - 32 \frac{\chi_0(4\mathbf{x}, 4Z)}{n\beta} + 81 \frac{\chi_0(3\mathbf{x}, 3Z)}{n\beta} - 96 \frac{\chi_0(2\mathbf{x}, 2Z)}{n\beta} + 42 \frac{\chi_0(\mathbf{x}, Z)}{n\beta} \right] \Rightarrow \\ \frac{\chi_0^{(5,5)}(\mathbf{x})}{n\beta^5} &= +\frac{1}{(5-1)!5!} \frac{\Theta^4}{x^8} \left[ \frac{5\chi_0(5\mathbf{x})}{n\beta} - 32 \frac{\chi_0(4\mathbf{x})}{n\beta} + 81 \frac{\chi_0(3\mathbf{x})}{n\beta} - 96 \frac{\chi_0(2\mathbf{x})}{n\beta} + 42 \frac{\chi_0(\mathbf{x})}{n\beta} \right] \Rightarrow \\ \frac{\chi_0^{(5,5)}(\mathbf{x})}{n\beta^5} &= -\frac{1}{(5-1)!5!} \frac{\Theta^4}{x^8} \left\{ \frac{5}{2} \Theta \int_0^\infty dy f_0(y; \Theta) \left[ 1 + \frac{25}{12} \left(\frac{x}{y}\right)^2 + \frac{125}{16} \left(\frac{x}{y}\right)^4 + \frac{1}{7} \frac{15625}{64} \left(\frac{x}{y}\right)^6 + \frac{1}{9} \frac{390625}{256} \left(\frac{x}{y}\right)^8 \right] \right. \\ &\quad - 32 \frac{3}{2} \Theta \int_0^\infty dy f_0(y; \Theta) \left[ 1 + \frac{4}{3} \left(\frac{x}{y}\right)^2 + \frac{16}{5} \left(\frac{x}{y}\right)^4 + \frac{64}{7} \left(\frac{x}{y}\right)^6 + \frac{256}{9} \left(\frac{x}{y}\right)^8 \right] \\ &\quad + 81 \frac{3}{2} \Theta \int_0^\infty dy f_0(y; \Theta) \left[ 1 + \frac{3}{4} \left(\frac{x}{y}\right)^2 + \frac{1}{5} \frac{1}{16} \left(\frac{x}{y}\right)^4 + \frac{1}{7} \frac{1}{64} \left(\frac{x}{y}\right)^6 + \frac{1}{9} \frac{1}{256} \left(\frac{x}{y}\right)^8 \right] \\ &\quad - 96 \frac{3}{2} \Theta \int_0^\infty dy f_0(y; \Theta) \left[ 1 + \frac{1}{3} \left(\frac{x}{y}\right)^2 + \frac{1}{5} \left(\frac{x}{y}\right)^4 + \frac{1}{7} \left(\frac{x}{y}\right)^6 + \frac{1}{9} \left(\frac{x}{y}\right)^8 \right] \\ &\quad \left. + 42 \frac{3}{2} \Theta \int_0^\infty dy f_0(y; \Theta) \left[ 1 + \frac{1}{12} \left(\frac{x}{y}\right)^2 + \frac{1}{5} \frac{1}{16} \left(\frac{x}{y}\right)^4 + \frac{1}{7} \frac{1}{64} \left(\frac{x}{y}\right)^6 + \frac{1}{9} \frac{1}{256} \left(\frac{x}{y}\right)^8 \right] \right\} \Rightarrow \\ \frac{\chi_0^{(5,5)}(\mathbf{x})}{n\beta^5} &= -\frac{1}{(5-1)!5!} \frac{\Theta^4}{2} \frac{\Theta}{x^8} \int_0^\infty dy f_0(y; \Theta) \left[ 5 + \frac{25}{12} \left(\frac{x}{y}\right)^2 + \frac{125}{16} \left(\frac{x}{y}\right)^4 + \frac{1}{7} \frac{15625}{64} \left(\frac{x}{y}\right)^6 + \frac{1}{9} \frac{390625}{256} \left(\frac{x}{y}\right)^8 \right. \\ &\quad - 32 - 32 \frac{4}{3} \left(\frac{x}{y}\right)^2 - 32 \frac{16}{5} \left(\frac{x}{y}\right)^4 - 32 \frac{64}{7} \left(\frac{x}{y}\right)^6 - 32 \frac{256}{9} \left(\frac{x}{y}\right)^8 + 81 + 81 \frac{3}{4} \left(\frac{x}{y}\right)^2 + 81 \frac{1}{5} \frac{1}{16} \left(\frac{x}{y}\right)^4 + 81 \frac{1}{7} \frac{1}{64} \left(\frac{x}{y}\right)^6 + 81 \frac{1}{9} \frac{1}{256} \left(\frac{x}{y}\right)^8 \\ &\quad \left. - 96 - 96 \frac{1}{3} \left(\frac{x}{y}\right)^2 - 96 \frac{1}{5} \left(\frac{x}{y}\right)^4 - 96 \frac{1}{7} \left(\frac{x}{y}\right)^6 - 96 \frac{1}{9} \left(\frac{x}{y}\right)^8 + 42 + 42 \frac{1}{12} \left(\frac{x}{y}\right)^2 + 42 \frac{1}{5} \frac{1}{16} \left(\frac{x}{y}\right)^4 + 42 \frac{1}{7} \frac{1}{64} \left(\frac{x}{y}\right)^6 + 42 \frac{1}{9} \frac{1}{256} \left(\frac{x}{y}\right)^8 \right].\end{aligned}$$

We simply re-organize the terms in ascending powers of  $x/y$ . It is straightforward to prove that the first four terms,  $\propto (x/y)^0, (x/y)^2, (x/y)^4, (x/y)^6$ , cancel out exactly. Thus, the leading order term is  $\mathcal{O}[(x/y)^8]$  and leads to finite contribution at the long-wavelength limit,  $\mathcal{O}(y^{-8})$ , after the removal of the  $1/x^8$  pre-factor. It is rather apparent that the remaining improper integral is indeed convergent.

$$\begin{aligned}
\frac{\chi_0^{(5,5)}(\mathbf{x})}{n\beta^5} &= -\frac{1}{4!5!} \frac{3\Theta^5}{2x^8} \int_0^\infty dy f_0(y; \Theta) \left[ 5 - 32 + 81 - 96 + 42 + 5 \frac{25}{12} \left(\frac{x}{y}\right)^2 - 32 \frac{4}{3} \left(\frac{x}{y}\right)^4 + 81 \frac{3}{4} \left(\frac{x}{y}\right)^6 - 96 \frac{1}{3} \left(\frac{x}{y}\right)^8 + 42 \frac{1}{12} \left(\frac{x}{y}\right)^{10} \right. \\
&\quad + 5 \frac{125}{16} \left(\frac{x}{y}\right)^{12} - 32 \frac{16}{5} \left(\frac{x}{y}\right)^{14} + 81 \frac{1}{5} \frac{81}{16} \left(\frac{x}{y}\right)^{16} - 96 \frac{1}{5} \left(\frac{x}{y}\right)^{18} + 42 \frac{1}{5} \frac{1}{16} \left(\frac{x}{y}\right)^{20} \\
&\quad \left. + \frac{5}{9} \frac{390625}{256} \left(\frac{x}{y}\right)^8 - 32 \frac{256}{9} \left(\frac{x}{y}\right)^{10} + 81 \frac{729}{256} \left(\frac{x}{y}\right)^{12} - 96 \frac{1}{9} \left(\frac{x}{y}\right)^{14} + 42 \frac{1}{9} \frac{1}{256} \left(\frac{x}{y}\right)^{16} \right] \Rightarrow \\
\frac{\chi_0^{(5,5)}(\mathbf{x})}{n\beta^5} &= -\frac{1}{4!5!} \frac{3\Theta^5}{2x^8} \int_0^\infty dy f_0(y; \Theta) \left\{ [5 - 32 + 81 - 96 + 42] + \left[ \frac{25}{12} - 32 \frac{4}{3} + 81 \frac{3}{4} - 96 \frac{1}{3} + 42 \frac{1}{12} \right] \left(\frac{x}{y}\right)^2 + \left[ \frac{125}{16} - 32 \frac{16}{5} + 81 \frac{1}{5} \frac{81}{16} - 96 \frac{1}{5} + 42 \frac{1}{5} \frac{1}{16} \right] \left(\frac{x}{y}\right)^4 \right. \\
&\quad \left. + \left[ \frac{5}{7} \frac{15625}{64} + 81 \frac{1}{7} \frac{729}{64} - 32 \frac{64}{7} - 96 \frac{1}{7} + 42 \frac{1}{7} \frac{1}{64} \right] \left(\frac{x}{y}\right)^6 + \left[ \frac{5}{9} \frac{390625}{256} - 32 \frac{256}{9} + 81 \frac{729}{256} - 96 \frac{1}{9} + 42 \frac{1}{9} \frac{1}{256} \right] \left(\frac{x}{y}\right)^8 \right\} \Rightarrow \\
\frac{\chi_0^{(5,5)}(\mathbf{x})}{n\beta^5} &= -\frac{1}{4!5!} \frac{3\Theta^5}{2x^8} \int_0^\infty dy f_0(y; \Theta) \left\{ (128 - 128) + \frac{125 - 32 \times 16 + 81 \times 9 - 96 \times 4 + 42}{12} \left(\frac{x}{y}\right)^2 + \frac{125 \times 25 - 32 \times 256 + 81 \times 81 - 96 \times 16 + 42}{80} \left(\frac{x}{y}\right)^4 \right. \\
&\quad \left. + \frac{15625 \times 5 + 729 \times 81 - 32 \times 64^2 - 96 \times 64 + 42}{64 \times 7} \left(\frac{x}{y}\right)^6 + \frac{390625 \times 5 - 32 \times 256^2 + 729 \times 81 \times 9 - 256 \times 96 + 42}{256 \times 9} \left(\frac{x}{y}\right)^8 \right\} \Rightarrow \\
\frac{\chi_0^{(5,5)}(\mathbf{x})}{n\beta^5} &= -\frac{1}{4!5!} \frac{3\Theta^5}{2x^8} \int_0^\infty dy f_0(y; \Theta) \left\{ (128 - 128) + \frac{896 - 896}{12} \left(\frac{x}{y}\right)^2 + \frac{9728 - 9728}{80} \left(\frac{x}{y}\right)^4 + \frac{137216 - 137216}{64 \times 7} \left(\frac{x}{y}\right)^6 + \frac{2484608 - 2121728}{256 \times 9} \left(\frac{x}{y}\right)^8 \right\} \Rightarrow \\
\frac{\chi_0^{(5,5)}(\mathbf{x})}{n\beta^5} &= -\frac{1}{4!5!} \frac{3\Theta^5}{2x^8} \int_0^\infty dy f_0(y; \Theta) \frac{2484608 - 2121728}{256 \times 9} \left(\frac{x}{y}\right)^8 \Rightarrow \\
\frac{\chi_0^{(5,5)}(\mathbf{x})}{n\beta^5} &= -\frac{1}{4!5!} \frac{3\Theta^5}{2x^8} \int_0^\infty dy f_0(y; \Theta) \frac{362880}{256 \times 9} \left(\frac{x}{y}\right)^8 \Rightarrow \\
\frac{\chi_0^{(5,5)}(\mathbf{x})}{n\beta^5} &= -\frac{1}{4!5!} \frac{3\Theta^5}{2x^8} \int_0^\infty dy f_0(y; \Theta) \frac{40320}{256} \left(\frac{x}{y}\right)^8 \Rightarrow \\
\frac{\chi_0^{(5,5)}(\mathbf{x})}{n\beta^5} &= -\frac{1}{4!5!} \frac{3\Theta^5}{2x^8} \int_0^\infty dy f_0(y; \Theta) \frac{315}{2} \left(\frac{x}{y}\right)^8 \Rightarrow \\
\frac{\chi_0^{(5,5)}(\mathbf{x})}{n\beta^5} &= -\frac{1}{4!5!} \frac{3 \times 315}{2} \frac{\Theta^5}{2x^8} \int_0^\infty dy f_0(y; \Theta) \left(\frac{x}{y}\right)^8 \Rightarrow \\
\frac{\chi_0^{(5,5)}(\mathbf{x})}{n\beta^5} &= -\frac{1}{2 \times 3 \times 4 \times 2 \times 3 \times 4 \times 5 \times 2} \frac{3 \times 7 \times 5 \times 9 \Theta^5}{2} \int_0^\infty dy \left(\frac{x}{y}\right)^8 f_0(y; \Theta) \Rightarrow \\
\frac{\chi_0^{(5,5)}(\mathbf{x})}{n\beta^5} &= -\frac{21}{256} \Theta^5 \int_0^\infty dy \frac{f_0(y; \Theta)}{y^8}.
\end{aligned}$$

## II. CANONICAL CONJECTURE CALCULATIONS

The brute force quantum kinetic theory calculations lead to compact expressions for the normalized form of the quadratic ideal density response at the second harmonic, the cubic ideal density response at the third harmonic, the quartic ideal density response at the fourth harmonic and the quintic ideal density response at the fifth harmonic,

$$\begin{aligned}\frac{\chi_0^{(2,2)}(\mathbf{x}, Z)}{n\beta^2} &= \frac{1}{(2-1)!} \frac{1}{2!} \frac{\Theta}{x^2} \left[ 2 \frac{\chi_0(2\mathbf{x}, 2Z)}{n\beta} - 2 \frac{\chi_0(\mathbf{x}, Z)}{n\beta} \right], \\ \frac{\chi_0^{(3,3)}(\mathbf{x}, Z)}{n\beta^3} &= \frac{1}{(3-1)!} \frac{1}{3!} \frac{\Theta^2}{x^4} \left[ 3 \frac{\chi_0(3\mathbf{x}, 3Z)}{n\beta} - 8 \frac{\chi_0(2\mathbf{x}, 2Z)}{n\beta} + 5 \frac{\chi_0(\mathbf{x}, Z)}{n\beta} \right], \\ \frac{\chi_0^{(4,4)}(\mathbf{x}, Z)}{n\beta^4} &= \frac{1}{(4-1)!} \frac{1}{4!} \frac{\Theta^3}{x^6} \left[ 4 \frac{\chi_0(4\mathbf{x}, 4Z)}{n\beta} - 18 \frac{\chi_0(3\mathbf{x}, 3Z)}{n\beta} + 28 \frac{\chi_0(2\mathbf{x}, 2Z)}{n\beta} - 14 \frac{\chi_0(\mathbf{x}, Z)}{n\beta} \right], \\ \frac{\chi_0^{(5,5)}(\mathbf{x}, Z)}{n\beta^5} &= \frac{1}{(5-1)!} \frac{1}{5!} \frac{\Theta^4}{x^8} \left[ 5 \frac{\chi_0(5\mathbf{x}, 5Z)}{n\beta} - 32 \frac{\chi_0(4\mathbf{x}, 4Z)}{n\beta} + 81 \frac{\chi_0(3\mathbf{x}, 3Z)}{n\beta} - 96 \frac{\chi_0(2\mathbf{x}, 2Z)}{n\beta} + 42 \frac{\chi_0(\mathbf{x}, Z)}{n\beta} \right].\end{aligned}$$

It has been verified that the first order term of the Taylor expansion of the even quantity in brackets cancels out for the quadratic ideal static density response, that the first plus second order terms of the Taylor expansion of the even quantity in brackets cancel out for the cubic ideal static density response, that the first plus second plus third order terms of the Taylor expansion of the even quantity in brackets cancel out for the quartic ideal static density response, that the first plus second plus third plus fourth order terms of the Taylor expansion of the even quantity in brackets cancel out for the quintic ideal static density response. These constitute an independent confirmation of the veracity of our brute force calculations, since the long-wavelength limit of any high order ideal static density response needs to be well-defined for the UEF to be stable against constant potential energy perturbations. Therefore, the divergent pre-factor requires that a number of coefficients in the Taylor expansion of the bracketed term cancels out. Our main conjecture is that the  $l$ -order ideal density response at the  $l$ -th harmonic can be expressed as linear combination of linear ideal density responses (Lindhard responses) at all harmonics up to  $l$ . We shall refer to this as canonical form.

$$\frac{\chi_0^{(l,l)}(\mathbf{x}, Z)}{n\beta^l} = \sum_{m=1}^l a_m \frac{\chi_0(m\mathbf{x}, mZ)}{n\beta}.$$

The highest harmonic contribution to the canonical form can be proven to have a simple recursive form, which is

$$a_l = \frac{1}{[(l-1)!]^2} \frac{\Theta^{l-1}}{x^{2l-2}}.$$

The factorization of  $1/[(l-1)!l!]\Theta^{l-1}/x^{2l-2}$  is advisable, leading to

$$\frac{\chi_0^{(l,l)}(\mathbf{x}, Z)}{n\beta^l} = + \frac{1}{(l-1)!l!} \frac{\Theta^{l-1}}{x^{2l-2}} \left[ l \frac{\chi_0(l\mathbf{x}, lZ)}{n\beta} + \sum_{m=1}^{l-1} a_m \frac{\chi_0(m\mathbf{x}, mZ)}{n\beta} \right].$$

This factorization ensures that the above defined  $l-1$   $a_m$  coefficients are integers, which constitutes a straightforward check for errors. The unknown  $l-1$   $a_m$  coefficients can be simply calculated from the stability of the quantum system against constant external potential energy perturbations. Recall that the Taylor expansion of the static Lindhard density response reads as

$$\frac{\chi_0(\mathbf{x})}{n\beta} = -\frac{3}{2}\Theta \int_0^\infty dy f_0(y; \Theta) \sum_{\nu=0}^\infty \frac{1}{2\nu+1} \left( \frac{x}{2y} \right)^{2\nu}.$$

This naturally implies that

$$\frac{\chi_0(m\mathbf{x})}{n\beta} = -\frac{3}{2}\Theta \int_0^\infty dy f_0(y; \Theta) \sum_{\nu=0}^\infty \frac{1}{2\nu+1} \left( \frac{mx}{2y} \right)^{2\nu}.$$

Substitution of the Taylor expansion in the canonical conjecture for the static nonlinear response, after numerous interchanges between the series and integral operations as well as the application of the long wavelength limit, yields

$$\begin{aligned}
\frac{\chi_0^{(l,l)}(\mathbf{x})}{n\beta^l} &= \frac{1}{(l-1)!!} \frac{\Theta^{l-1}}{x^{2l-2}} \left[ l \frac{\chi_0(l\mathbf{x})}{n\beta} + \sum_{m=1}^{l-1} a_m \frac{\chi_0(m\mathbf{x})}{n\beta} \right] \Rightarrow \\
\frac{\chi_0^{(l,l)}(\mathbf{x})}{n\beta^l} &= \frac{1}{(l-1)!!} \frac{\Theta^{l-1}}{x^{2l-2}} \left\{ l \left[ -\frac{3}{2} \Theta \int_0^\infty dy f_0(y; \Theta) \sum_{\nu=0}^\infty \frac{1}{2\nu+1} \left( \frac{l\mathbf{x}}{2y} \right)^{2\nu} \right] \right. \\
&\quad \left. + \sum_{m=1}^{l-1} a_m \left[ -\frac{3}{2} \Theta \int_0^\infty dy f_0(y; \Theta) \sum_{\nu=0}^\infty \frac{1}{2\nu+1} \left( \frac{m\mathbf{x}}{2y} \right)^{2\nu} \right] \right\} \Rightarrow \\
\frac{\chi_0^{(l,l)}(\mathbf{x})}{n\beta^l} &= -\frac{1}{(l-1)!!} \frac{\Theta^{l-1}}{x^{2l-2}} \frac{3}{2} \Theta \int_0^\infty dy f_0(y; \Theta) \left\{ l \sum_{\nu=0}^\infty \frac{1}{2\nu+1} \left( \frac{l\mathbf{x}}{2y} \right)^{2\nu} + \sum_{m=1}^{l-1} a_m \sum_{\nu=0}^\infty \frac{1}{2\nu+1} \left( \frac{m\mathbf{x}}{2y} \right)^{2\nu} \right\} \Rightarrow \\
\frac{\chi_0^{(l,l)}(\mathbf{x})}{n\beta^l} &= -\frac{3}{2} \frac{1}{(l-1)!!} \Theta^l \int_0^\infty dy f_0(y; \Theta) \left\{ l \sum_{\nu=0}^\infty \frac{1}{2\nu+1} \left( \frac{l\mathbf{x}}{2y} \right)^{2\nu} \frac{1}{x^{2l-2}} + \sum_{m=1}^{l-1} a_m \sum_{\nu=0}^\infty \frac{1}{2\nu+1} \left( \frac{m\mathbf{x}}{2y} \right)^{2\nu} \frac{1}{x^{2l-2}} \right\} \Rightarrow \\
\frac{\chi_0^{(l,l)}(\mathbf{x})}{n\beta^l} &= -\frac{3}{2} \frac{1}{(l-1)!!} \Theta^l \int_0^\infty dy f_0(y; \Theta) \left\{ l \sum_{\nu=0}^\infty \frac{1}{2\nu+1} \frac{l^{2\nu}}{2^{2\nu}} \frac{x^{2\nu}}{y^{2\nu}} \frac{1}{x^{2l-2}} + \sum_{m=1}^{l-1} a_m \sum_{\nu=0}^\infty \frac{1}{2\nu+1} \frac{m^{2\nu}}{2^{2\nu}} \frac{x^{2\nu}}{y^{2\nu}} \frac{1}{x^{2l-2}} \right\} \Rightarrow \\
\frac{\chi_0^{(l,l)}(\mathbf{x})}{n\beta^l} &= -\frac{3}{2} \frac{1}{(l-1)!!} \Theta^l \sum_{\nu=0}^\infty \int_0^\infty dy f_0(y; \Theta) \left\{ \frac{1}{2\nu+1} \frac{l^{2\nu+1}}{2^{2\nu}} \frac{x^{2\nu-2l+2}}{y^{2\nu}} + \sum_{m=1}^{l-1} \frac{1}{2\nu+1} \frac{a_m m^{2\nu}}{2^{2\nu}} \frac{x^{2\nu-2l+2}}{y^{2\nu}} \right\} \Rightarrow \\
\frac{\chi_0^{(l,l)}(\mathbf{x})}{n\beta^l} &= -\frac{3}{2} \frac{1}{(l-1)!!} \Theta^l \sum_{\nu=0}^\infty \int_0^\infty dy \frac{f_0(y; \Theta)}{y^{2\nu}} \left\{ \frac{1}{2\nu+1} \frac{l^{2\nu+1}}{2^{2\nu}} + \sum_{m=1}^{l-1} \frac{1}{2\nu+1} \frac{a_m m^{2\nu}}{2^{2\nu}} \right\} x^{2\nu-2l+2} \Rightarrow \\
\lim_{x \rightarrow 0} \frac{\chi_0^{(l,l)}(\mathbf{x})}{n\beta^l} &= -\frac{3}{2} \frac{1}{(l-1)!!} \Theta^l \lim_{x \rightarrow 0} \sum_{\nu=0}^\infty \int_0^\infty dy \frac{f_0(y; \Theta)}{y^{2\nu}} \left\{ \frac{1}{2\nu+1} \frac{l^{2\nu+1}}{2^{2\nu}} + \sum_{m=1}^{l-1} \frac{1}{2\nu+1} \frac{a_m m^{2\nu}}{2^{2\nu}} \right\} x^{2\nu-2l+2} \Rightarrow \\
\lim_{x \rightarrow 0} \frac{\chi_0^{(l,l)}(\mathbf{x})}{n\beta^l} &= -\frac{3}{2} \frac{1}{(l-1)!!} \Theta^l \lim_{x \rightarrow 0} \sum_{\nu=0}^{l-1} \int_0^\infty dy \frac{f_0(y; \Theta)}{y^{2\nu}} \left\{ \frac{1}{2\nu+1} \frac{l^{2\nu+1}}{2^{2\nu}} + \sum_{m=1}^{l-1} \frac{1}{2\nu+1} \frac{a_m m^{2\nu}}{2^{2\nu}} \right\} x^{2\nu-2l+2}.
\end{aligned}$$

Note the upper index change of the  $\nu$ -series from infinity to  $l-1$ . The long-wavelength limit converges and becomes

$$\begin{aligned}
\lim_{x \rightarrow 0} \frac{\chi_0^{(l,l)}(\mathbf{x})}{n\beta^l} &= -\frac{3}{2} \frac{1}{(l-1)!!} \Theta^l \delta_{\nu, l-1} \int_0^\infty dy \frac{f_0(y; \Theta)}{y^{2\nu}} \left\{ \frac{1}{2\nu+1} \frac{l^{2\nu+1}}{2^{2\nu}} + \sum_{m=1}^{l-1} \frac{1}{2\nu+1} \frac{a_m m^{2\nu}}{2^{2\nu}} \right\} \lim_{x \rightarrow 0} x^{2\nu-2l+2} \Rightarrow \\
\lim_{x \rightarrow 0} \frac{\chi_0^{(l,l)}(\mathbf{x})}{n\beta^l} &= -\frac{3}{2} \frac{1}{(l-1)!!} \Theta^l \int_0^\infty dy \frac{f_0(y; \Theta)}{y^{2(l-1)}} \left\{ \frac{1}{2(l-1)+1} \frac{l^{2(l-1)+1}}{2^{2(l-1)}} + \sum_{m=1}^{l-1} \frac{1}{2(l-1)+1} \frac{a_m m^{2(l-1)}}{2^{2(l-1)}} \right\} \lim_{x \rightarrow 0} x^{2(l-1)-2l+2} \Rightarrow \\
\lim_{x \rightarrow 0} \frac{\chi_0^{(l,l)}(\mathbf{x})}{n\beta^l} &= -\frac{3}{2} \frac{1}{(l-1)!!} \Theta^l \int_0^\infty dy \frac{f_0(y; \Theta)}{y^{2(l-1)}} \left\{ \frac{1}{2l-2+1} \frac{l^{2l-2+1}}{2^{2l-2}} + \sum_{m=1}^{l-1} \frac{1}{2l-2+1} \frac{a_m m^{2l-2}}{2^{2l-2}} \right\} \lim_{x \rightarrow 0} x^{2l-2-2l+2} \Rightarrow \\
\lim_{x \rightarrow 0} \frac{\chi_0^{(l,l)}(\mathbf{x})}{n\beta^l} &= -\frac{3}{2} \frac{1}{(l-1)!!} \Theta^l \int_0^\infty dy \frac{f_0(y; \Theta)}{y^{2(l-1)}} \left\{ \frac{1}{2l-1} \frac{l^{2l-1}}{2^{2l-2}} + \sum_{m=1}^{l-1} \frac{1}{2l-1} \frac{a_m m^{2l-2}}{2^{2l-2}} \right\} \lim_{x \rightarrow 0} x^0 \Rightarrow \\
\lim_{x \rightarrow 0} \frac{\chi_0^{(l,l)}(\mathbf{x})}{n\beta^l} &= -\frac{3}{2} \frac{1}{(l-1)!!} \Theta^l \left\{ \frac{1}{2l-1} \frac{l^{2l-1}}{2^{2l-2}} + \sum_{m=1}^{l-1} \frac{1}{2l-1} \frac{a_m m^{2l-2}}{2^{2l-2}} \right\} \int_0^\infty dy \frac{f_0(y; \Theta)}{y^{2(l-1)}}.
\end{aligned}$$

provided that all the  $\nu = 0, 1, \dots, l-2$  coefficients vanish. This leads to the  $(l-1) \times (l-1)$  system of linear equations

$$\begin{aligned}
\frac{1}{2\nu+1} \frac{l^{2\nu+1}}{2^{2\nu}} + \sum_{m=1}^{l-1} \frac{1}{2\nu+1} \frac{a_m m^{2\nu}}{2^{2\nu}} &= 0, \text{ for } \nu = 0, 1, \dots, l-2 \Rightarrow \\
\sum_{m=1}^{l-1} a_m m^{2\nu} &= -l^{2\nu+1}, \text{ for } \nu = 0, 1, \dots, l-2.
\end{aligned}$$

which determines the unknown  $l-1$   $a_m$  coefficients of the canonical form.

### A. The sixth-order (sextic) ideal density response at the sixth harmonic

Based on the arbitrary perturbation order methodology that was outlined earlier, the general form of the normalized sextic ideal density response at the sixth harmonic reads as

$$\frac{\chi_0^{(6,6)}(\mathbf{x}, Z)}{n\beta^6} = \frac{1}{(6-1)!6!} \frac{\Theta^5}{x^{10}} \left[ 6 \frac{\chi_0(6\mathbf{x}, 6Z)}{n\beta} + a_5 \frac{\chi_0(5\mathbf{x}, 5Z)}{n\beta} + a_4 \frac{\chi_0(4\mathbf{x}, 4Z)}{n\beta} + a_3 \frac{\chi_0(3\mathbf{x}, 3Z)}{n\beta} + a_2 \frac{\chi_0(2\mathbf{x}, 2Z)}{n\beta} + a_1 \frac{\chi_0(\mathbf{x}, Z)}{n\beta} \right]$$

The key for the determination of the coefficients  $a_5, a_4, a_3, a_2, a_1$  lies in the behavior of the static density responses,

$$\frac{\chi_0^{(6,6)}(\mathbf{x})}{n\beta^6} = \frac{1}{(6-1)!6!} \frac{\Theta^5}{x^{10}} \left[ 6 \frac{\chi_0(6\mathbf{x})}{n\beta} + a_5 \frac{\chi_0(5\mathbf{x})}{n\beta} + a_4 \frac{\chi_0(4\mathbf{x})}{n\beta} + a_3 \frac{\chi_0(3\mathbf{x})}{n\beta} + a_2 \frac{\chi_0(2\mathbf{x})}{n\beta} + a_1 \frac{\chi_0(\mathbf{x})}{n\beta} \right],$$

where

$$\begin{aligned} \frac{\chi_0(\mathbf{x})}{n\beta} &= -\frac{3}{2} \frac{\Theta}{x} \int_0^\infty y f_0(y; \Theta) \ln \left| \frac{x+2y}{x-2y} \right| dy, \\ \frac{\chi_0(2\mathbf{x})}{n\beta} &= -\frac{3}{2} \frac{\Theta}{2x} \int_0^\infty y f_0(y; \Theta) \ln \left| \frac{2x+2y}{2x-2y} \right| dy, \\ \frac{\chi_0(3\mathbf{x})}{n\beta} &= -\frac{3}{2} \frac{\Theta}{3x} \int_0^\infty y f_0(y; \Theta) \ln \left| \frac{3x+2y}{3x-2y} \right| dy, \\ \frac{\chi_0(4\mathbf{x})}{n\beta} &= -\frac{3}{2} \frac{\Theta}{4x} \int_0^\infty y f_0(y; \Theta) \ln \left| \frac{4x+2y}{4x-2y} \right| dy, \\ \frac{\chi_0(5\mathbf{x})}{n\beta} &= -\frac{3}{2} \frac{\Theta}{5x} \int_0^\infty y f_0(y; \Theta) \ln \left| \frac{5x+2y}{5x-2y} \right| dy, \\ \frac{\chi_0(6\mathbf{x})}{n\beta} &= -\frac{3}{2} \frac{\Theta}{6x} \int_0^\infty y f_0(y; \Theta) \ln \left| \frac{6x+2y}{6x-2y} \right| dy. \end{aligned}$$

Given the  $x^{-10}$  pre-factor and the Taylor expansion of the even static Lindhard response  $\chi_0(\mathbf{x})/(n\beta)$ , the first five terms of the Taylor expansion of  $\chi_0^{(6,6)}(\mathbf{x})/(n\beta^6)$  need to cancel out exactly in the long-wavelength limit. Otherwise, the non-interacting UEF would be unstable against constant potential energy perturbations. This constraint yields exactly five linear equations for the determination of the unknown coefficients  $a_5, a_4, a_3, a_2, a_1$ . Let us compute the first five terms in the small argument expansion of the Lindhard density response at the first six harmonics.

$$\begin{aligned} \frac{\chi_0(\mathbf{x})}{n\beta} &\simeq -\frac{3}{2} \Theta \int_0^\infty dy f_0(y; \Theta) \left[ 1 + \frac{1}{3} \frac{1}{4} \left( \frac{x}{y} \right)^2 + \frac{1}{5} \frac{1}{16} \left( \frac{x}{y} \right)^4 + \frac{1}{7} \frac{1}{64} \left( \frac{x}{y} \right)^6 + \frac{1}{9} \frac{1}{256} \left( \frac{x}{y} \right)^8 \right], \\ \frac{\chi_0(2\mathbf{x})}{n\beta} &\simeq -\frac{3}{2} \Theta \int_0^\infty dy f_0(y; \Theta) \left[ 1 + \frac{1}{3} \frac{1}{4} \left( \frac{2x}{y} \right)^2 + \frac{1}{5} \frac{1}{16} \left( \frac{2x}{y} \right)^4 + \frac{1}{7} \frac{1}{64} \left( \frac{2x}{y} \right)^6 + \frac{1}{9} \frac{1}{256} \left( \frac{2x}{y} \right)^8 \right], \\ \frac{\chi_0(3\mathbf{x})}{n\beta} &\simeq -\frac{3}{2} \Theta \int_0^\infty dy f_0(y; \Theta) \left[ 1 + \frac{1}{3} \frac{1}{4} \left( \frac{3x}{y} \right)^2 + \frac{1}{5} \frac{1}{16} \left( \frac{3x}{y} \right)^4 + \frac{1}{7} \frac{1}{64} \left( \frac{3x}{y} \right)^6 + \frac{1}{9} \frac{1}{256} \left( \frac{3x}{y} \right)^8 \right], \\ \frac{\chi_0(4\mathbf{x})}{n\beta} &\simeq -\frac{3}{2} \Theta \int_0^\infty dy f_0(y; \Theta) \left[ 1 + \frac{1}{3} \frac{1}{4} \left( \frac{4x}{y} \right)^2 + \frac{1}{5} \frac{1}{16} \left( \frac{4x}{y} \right)^4 + \frac{1}{7} \frac{1}{64} \left( \frac{4x}{y} \right)^6 + \frac{1}{9} \frac{1}{256} \left( \frac{4x}{y} \right)^8 \right], \\ \frac{\chi_0(5\mathbf{x})}{n\beta} &\simeq -\frac{3}{2} \Theta \int_0^\infty dy f_0(y; \Theta) \left[ 1 + \frac{1}{3} \frac{1}{4} \left( \frac{5x}{y} \right)^2 + \frac{1}{5} \frac{1}{16} \left( \frac{5x}{y} \right)^4 + \frac{1}{7} \frac{1}{64} \left( \frac{5x}{y} \right)^6 + \frac{1}{9} \frac{1}{256} \left( \frac{5x}{y} \right)^8 \right], \\ \frac{\chi_0(6\mathbf{x})}{n\beta} &\simeq -\frac{3}{2} \Theta \int_0^\infty dy f_0(y; \Theta) \left[ 1 + \frac{1}{3} \frac{1}{4} \left( \frac{6x}{y} \right)^2 + \frac{1}{5} \frac{1}{16} \left( \frac{6x}{y} \right)^4 + \frac{1}{7} \frac{1}{64} \left( \frac{6x}{y} \right)^6 + \frac{1}{9} \frac{1}{256} \left( \frac{6x}{y} \right)^8 \right] \Rightarrow \end{aligned}$$



$$\begin{aligned}
\frac{\chi_0(\mathbf{x})}{n\beta} &\simeq -\frac{3}{2}\Theta \int_0^\infty dy f_0(y; \Theta) \left[ 1 + \frac{1}{3} \frac{1}{4} \left(\frac{x}{y}\right)^2 + \frac{1}{5} \frac{1}{16} \left(\frac{x}{y}\right)^4 + \frac{1}{7} \frac{1}{64} \left(\frac{x}{y}\right)^6 + \frac{1}{9} \frac{1}{256} \left(\frac{x}{y}\right)^8 \right], \\
\frac{\chi_0(2\mathbf{x})}{n\beta} &\simeq -\frac{3}{2}\Theta \int_0^\infty dy f_0(y; \Theta) \left[ 1 + \frac{1}{3} \frac{2^2}{4} \left(\frac{x}{y}\right)^2 + \frac{1}{5} \frac{2^4}{16} \left(\frac{x}{y}\right)^4 + \frac{1}{7} \frac{2^6}{64} \left(\frac{x}{y}\right)^6 + \frac{1}{9} \frac{2^8}{256} \left(\frac{x}{y}\right)^8 \right], \\
\frac{\chi_0(3\mathbf{x})}{n\beta} &\simeq -\frac{3}{2}\Theta \int_0^\infty dy f_0(y; \Theta) \left[ 1 + \frac{1}{3} \frac{3^2}{4} \left(\frac{x}{y}\right)^2 + \frac{1}{5} \frac{3^4}{16} \left(\frac{x}{y}\right)^4 + \frac{1}{7} \frac{3^6}{64} \left(\frac{x}{y}\right)^6 + \frac{1}{9} \frac{3^8}{256} \left(\frac{x}{y}\right)^8 \right], \\
\frac{\chi_0(4\mathbf{x})}{n\beta} &\simeq -\frac{3}{2}\Theta \int_0^\infty dy f_0(y; \Theta) \left[ 1 + \frac{1}{3} \frac{4^2}{4} \left(\frac{x}{y}\right)^2 + \frac{1}{5} \frac{4^4}{16} \left(\frac{x}{y}\right)^4 + \frac{1}{7} \frac{4^6}{64} \left(\frac{x}{y}\right)^6 + \frac{1}{9} \frac{4^8}{256} \left(\frac{x}{y}\right)^8 \right], \\
\frac{\chi_0(5\mathbf{x})}{n\beta} &\simeq -\frac{3}{2}\Theta \int_0^\infty dy f_0(y; \Theta) \left[ 1 + \frac{1}{3} \frac{5^2}{4} \left(\frac{x}{y}\right)^2 + \frac{1}{5} \frac{5^4}{16} \left(\frac{x}{y}\right)^4 + \frac{1}{7} \frac{5^6}{64} \left(\frac{x}{y}\right)^6 + \frac{1}{9} \frac{5^8}{256} \left(\frac{x}{y}\right)^8 \right], \\
\frac{\chi_0(6\mathbf{x})}{n\beta} &\simeq -\frac{3}{2}\Theta \int_0^\infty dy f_0(y; \Theta) \left[ 1 + \frac{1}{3} \frac{6^2}{4} \left(\frac{x}{y}\right)^2 + \frac{1}{5} \frac{6^4}{16} \left(\frac{x}{y}\right)^4 + \frac{1}{7} \frac{6^6}{64} \left(\frac{x}{y}\right)^6 + \frac{1}{9} \frac{6^8}{256} \left(\frac{x}{y}\right)^8 \right] \Rightarrow \\
\frac{\chi_0(\mathbf{x})}{n\beta} &\simeq -\frac{3}{2}\Theta \int_0^\infty dy f_0(y; \Theta) \left[ 1 + \frac{1}{12} \left(\frac{x}{y}\right)^2 + \frac{1}{80} \left(\frac{x}{y}\right)^4 + \frac{1}{448} \left(\frac{x}{y}\right)^6 + \frac{1}{2304} \left(\frac{x}{y}\right)^8 \right], \\
\frac{\chi_0(2\mathbf{x})}{n\beta} &\simeq -\frac{3}{2}\Theta \int_0^\infty dy f_0(y; \Theta) \left[ 1 + \frac{1}{3} \left(\frac{x}{y}\right)^2 + \frac{1}{5} \left(\frac{x}{y}\right)^4 + \frac{1}{7} \left(\frac{x}{y}\right)^6 + \frac{1}{9} \left(\frac{x}{y}\right)^8 \right], \\
\frac{\chi_0(3\mathbf{x})}{n\beta} &\simeq -\frac{3}{2}\Theta \int_0^\infty dy f_0(y; \Theta) \left[ 1 + \frac{3}{4} \left(\frac{x}{y}\right)^2 + \frac{81}{80} \left(\frac{x}{y}\right)^4 + \frac{729}{448} \left(\frac{x}{y}\right)^6 + \frac{6561}{2304} \left(\frac{x}{y}\right)^8 \right], \\
\frac{\chi_0(4\mathbf{x})}{n\beta} &\simeq -\frac{3}{2}\Theta \int_0^\infty dy f_0(y; \Theta) \left[ 1 + \frac{4}{3} \left(\frac{x}{y}\right)^2 + \frac{16}{5} \left(\frac{x}{y}\right)^4 + \frac{64}{7} \left(\frac{x}{y}\right)^6 + \frac{256}{9} \left(\frac{x}{y}\right)^8 \right], \\
\frac{\chi_0(5\mathbf{x})}{n\beta} &\simeq -\frac{3}{2}\Theta \int_0^\infty dy f_0(y; \Theta) \left[ 1 + \frac{25}{12} \left(\frac{x}{y}\right)^2 + \frac{125}{16} \left(\frac{x}{y}\right)^4 + \frac{15625}{448} \left(\frac{x}{y}\right)^6 + \frac{390625}{2304} \left(\frac{x}{y}\right)^8 \right], \\
\frac{\chi_0(6\mathbf{x})}{n\beta} &\simeq -\frac{3}{2}\Theta \int_0^\infty dy f_0(y; \Theta) \left[ 1 + 3 \left(\frac{x}{y}\right)^2 + \frac{81}{5} \left(\frac{x}{y}\right)^4 + \frac{729}{7} \left(\frac{x}{y}\right)^6 + 729 \left(\frac{x}{y}\right)^8 \right].
\end{aligned}$$

Substituting in the canonical form, ordering in powers of  $1/x^{10}$ ,  $1/x^8$ ,  $1/x^6$ ,  $1/x^4$ ,  $1/x^2$ , taking the limit  $x \rightarrow 0$  and equating each coefficient with zero (as demanded by the stability requirement) leads to the  $5 \times 5$  system of equations  $Ma = b$  where the  $5 \times 5$  matrix  $M$  is given by

$$\begin{pmatrix}
1 & 1 & 1 & 1 & 1 \\
\frac{25}{12} & \frac{4}{3} & \frac{3}{4} & \frac{1}{3} & \frac{1}{12} \\
\frac{125}{16} & \frac{16}{5} & \frac{81}{80} & \frac{1}{5} & \frac{1}{80} \\
\frac{15625}{448} & \frac{64}{7} & \frac{729}{448} & \frac{1}{7} & \frac{1}{448} \\
\frac{390625}{2304} & \frac{256}{9} & \frac{729}{256} & \frac{1}{9} & \frac{1}{2304}
\end{pmatrix}$$

the 5-dim source vector  $b$  is given by  $b = (-6, -18, -486/5, -4374/7, -4374)$  and the 5-dim unknown vector  $a$  is defined by  $a = (a_5, a_4, a_3, a_2, a_1)$ . The solution is  $(a_5, a_4, a_3, a_2, a_1) = (-50, 176, -330, 330, -132)$ . It should be noted that the unknown coefficients can only be integers, which provides a straightforward way to check for misprints. Thus, the canonical form of the normalized sextic ideal density response at the sixth harmonic reads as

$$\frac{\chi_0^{(6,6)}(\mathbf{x}, Z)}{n\beta^6} = \frac{1}{(6-1)! x^{10}} \left[ 6 \frac{\chi_0(6\mathbf{x}, 6Z)}{n\beta} - 50 \frac{\chi_0(5\mathbf{x}, 5Z)}{n\beta} + 176 \frac{\chi_0(4\mathbf{x}, 4Z)}{n\beta} - 330 \frac{\chi_0(3\mathbf{x}, 3Z)}{n\beta} + 330 \frac{\chi_0(2\mathbf{x}, 2Z)}{n\beta} - 132 \frac{\chi_0(\mathbf{x}, Z)}{n\beta} \right]$$

In order to obtain the long-wavelength limit of the normalized sextic static ideal density response at the sixth harmonic, given the automatic cancellations due to the stability requirement, it suffices to consider the sixth term of the small argument expansion of the Lindhard density response constituents alone. This leads to

$$\begin{aligned}
\frac{\chi_0^{(6,6)}(\mathbf{x})}{n\beta^6} &= \frac{1}{86400} \frac{\Theta^5}{x^{10}} \left[ 6 \frac{\chi_0(6\mathbf{x})}{n\beta} - 50 \frac{\chi_0(5\mathbf{x})}{n\beta} + 176 \frac{\chi_0(4\mathbf{x})}{n\beta} - 330 \frac{\chi_0(3\mathbf{x})}{n\beta} + 330 \frac{\chi_0(2\mathbf{x})}{n\beta} - 132 \frac{\chi_0(\mathbf{x})}{n\beta} \right] \Rightarrow \\
\frac{\chi_0^{(6,6)}(\mathbf{x})}{n\beta^6} &= -\frac{1}{86400} \frac{\Theta^5}{x^{10}} \left\{ 6 \left[ \frac{3}{2} \Theta \int_0^\infty dy f_0(y; \Theta) \frac{1}{11} \frac{1}{1024} \left( \frac{6x}{y} \right)^{10} \right] - 50 \left[ \frac{3}{2} \Theta \int_0^\infty dy f_0(y; \Theta) \frac{1}{11} \frac{1}{1024} \left( \frac{5x}{y} \right)^{10} \right] \right. \\
&\quad + 176 \left[ \frac{3}{2} \Theta \int_0^\infty dy f_0(y; \Theta) \frac{1}{11} \frac{1}{1024} \left( \frac{4x}{y} \right)^{10} \right] - 330 \left[ \frac{3}{2} \Theta \int_0^\infty dy f_0(y; \Theta) \frac{1}{11} \frac{1}{1024} \left( \frac{3x}{y} \right)^{10} \right] \\
&\quad \left. + 330 \left[ \frac{3}{2} \Theta \int_0^\infty dy f_0(y; \Theta) \frac{1}{11} \frac{1}{1024} \left( \frac{2x}{y} \right)^{10} \right] - 132 \left[ \frac{3}{2} \Theta \int_0^\infty dy f_0(y; \Theta) \frac{1}{11} \frac{1}{1024} \left( \frac{x}{y} \right)^{10} \right] \right\} \Rightarrow \\
\frac{\chi_0^{(6,6)}(\mathbf{x})}{n\beta^6} &= -\frac{1}{86400} \frac{\Theta^5}{x^{10}} \frac{3}{2} \Theta \int_0^\infty dy f_0(y; \Theta) \left\{ \frac{6}{11} \frac{1}{1024} \left( \frac{6x}{y} \right)^{10} - \frac{50}{11} \frac{1}{1024} \left( \frac{5x}{y} \right)^{10} + \frac{176}{11} \frac{1}{1024} \left( \frac{4x}{y} \right)^{10} \right. \\
&\quad \left. - \frac{330}{11} \frac{1}{1024} \left( \frac{3x}{y} \right)^{10} + \frac{330}{11} \frac{1}{1024} \left( \frac{2x}{y} \right)^{10} - \frac{132}{11} \frac{1}{1024} \left( \frac{x}{y} \right)^{10} \right\} \Rightarrow \\
\frac{\chi_0^{(6,6)}(\mathbf{x})}{n\beta^6} &= -\frac{1}{86400} \frac{\Theta^5}{x^{10}} \frac{3}{2} \Theta \int_0^\infty dy f_0(y; \Theta) \left\{ \frac{6}{11} \frac{6^{10}}{1024} \left( \frac{x}{y} \right)^{10} - \frac{50}{11} \frac{5^{10}}{1024} \left( \frac{x}{y} \right)^{10} + \frac{176}{11} \frac{4^{10}}{1024} \left( \frac{x}{y} \right)^{10} \right. \\
&\quad \left. - \frac{330}{11} \frac{3^{10}}{1024} \left( \frac{x}{y} \right)^{10} + \frac{330}{11} \frac{2^{10}}{1024} \left( \frac{x}{y} \right)^{10} - \frac{132}{11} \frac{1}{1024} \left( \frac{x}{y} \right)^{10} \right\} \Rightarrow \\
\frac{\chi_0^{(6,6)}(\mathbf{x})}{n\beta^6} &= -\frac{1}{57600} \frac{\Theta^6}{x^{10}} \int_0^\infty dy f_0(y; \Theta) \left\{ \frac{6}{11} \frac{6^{10}}{1024} \left( \frac{x}{y} \right)^{10} - \frac{50}{11} \frac{5^{10}}{1024} \left( \frac{x}{y} \right)^{10} + \frac{176}{11} \frac{4^{10}}{1024} \left( \frac{x}{y} \right)^{10} \right. \\
&\quad \left. - \frac{330}{11} \frac{3^{10}}{1024} \left( \frac{x}{y} \right)^{10} + \frac{330}{11} \frac{2^{10}}{1024} \left( \frac{x}{y} \right)^{10} - \frac{132}{11} \frac{1}{1024} \left( \frac{x}{y} \right)^{10} \right\} \Rightarrow \\
\frac{\chi_0^{(6,6)}(\mathbf{x})}{n\beta^6} &= -\frac{1}{57600} \frac{\Theta^6}{x^{10}} \int_0^\infty dy f_0(y; \Theta) \left\{ \frac{6}{11} \frac{6^{10}}{1024} - \frac{50}{11} \frac{5^{10}}{1024} + \frac{176}{11} \frac{4^{10}}{1024} - \frac{330}{11} \frac{3^{10}}{1024} + \frac{330}{11} \frac{2^{10}}{1024} - \frac{132}{11} \frac{1}{1024} \right\} \left( \frac{x}{y} \right)^{10} \Rightarrow \\
\frac{\chi_0^{(6,6)}(\mathbf{x})}{n\beta^6} &= -\frac{1}{57600} \left\{ \frac{6}{11} \frac{6^{10}}{1024} - \frac{50}{11} \frac{5^{10}}{1024} + \frac{176}{11} \frac{4^{10}}{1024} - \frac{330}{11} \frac{3^{10}}{1024} + \frac{330}{11} \frac{2^{10}}{1024} - \frac{132}{11} \frac{1}{1024} \right\} \frac{\Theta^6}{x^{10}} \int_0^\infty dy f_0(y; \Theta) \frac{x^{10}}{y^{10}} \Rightarrow \\
\frac{\chi_0^{(6,6)}(\mathbf{x})}{n\beta^6} &= -\frac{1}{57600} \left\{ \frac{6^{11}}{11264} - \frac{5^{11} \times 10}{11264} + \frac{4^{10} \times 176}{11264} - \frac{3^{10} \times 330}{11264} + \frac{2^{10} \times 330}{11264} - \frac{132}{11264} \right\} \Theta^6 \int_0^\infty dy \frac{f_0(y; \Theta)}{y^{10}} \Rightarrow \\
\frac{\chi_0^{(6,6)}(\mathbf{x})}{n\beta^6} &= -\frac{1}{57600} \frac{6^{11} - 5^{11} \times 10 + 4^{10} \times 176 - 3^{10} \times 330 + 2^{10} \times 330 - 132}{11264} \Theta^6 \int_0^\infty dy \frac{f_0(y; \Theta)}{y^{10}} \Rightarrow \\
\frac{\chi_0^{(6,6)}(\mathbf{x})}{n\beta^6} &= -\frac{1}{57600} \frac{362797056 - 488281250 + 184549376 - 19486170 + 337920 - 132}{11264} \Theta^6 \int_0^\infty dy \frac{f_0(y; \Theta)}{y^{10}} \Rightarrow \\
\frac{\chi_0^{(6,6)}(\mathbf{x})}{n\beta^6} &= -\frac{1}{57600} \frac{39916800}{11264} \Theta^6 \int_0^\infty dy \frac{f_0(y; \Theta)}{y^{10}} \Rightarrow \\
\frac{\chi_0^{(6,6)}(\mathbf{x})}{n\beta^6} &= -\frac{39916800}{64806400} \Theta^6 \int_0^\infty dy \frac{f_0(y; \Theta)}{y^{10}} \Rightarrow \\
\frac{\chi_0^{(6,6)}(\mathbf{x})}{n\beta^6} &= -\frac{39916800}{633600} \frac{633600}{64806400} \Theta^6 \int_0^\infty dy \frac{f_0(y; \Theta)}{y^{10}} \Rightarrow \\
\frac{\chi_0^{(6,6)}(\mathbf{x})}{n\beta^6} &= -\frac{63}{1024} \Theta^6 \int_0^\infty dy \frac{f_0(y; \Theta)}{y^{10}}.
\end{aligned}$$

### B. The seventh-order (septic) ideal density response

Based on the arbitrary perturbation order methodology that was outlined earlier, the general form of the normalized septic ideal density response at the seventh harmonic reads as

$$\frac{\chi_0^{(7,7)}(\mathbf{x}, Z)}{n\beta^7} = \frac{1}{(7-1)!7! x^{12}} \left[ 7 \frac{\chi_0(7\mathbf{x}, 7Z)}{n\beta} + a_6 \frac{\chi_0(6\mathbf{x}, 6Z)}{n\beta} + a_5 \frac{\chi_0(5\mathbf{x}, 5Z)}{n\beta} + a_4 \frac{\chi_0(4\mathbf{x}, 4Z)}{n\beta} + a_3 \frac{\chi_0(3\mathbf{x}, 3Z)}{n\beta} + a_2 \frac{\chi_0(2\mathbf{x}, 2Z)}{n\beta} \right]$$

The key for the determination of the coefficients  $a_6, a_5, a_4, a_3, a_2, a_1$  lies in the behavior of the static density responses,

$$\frac{\chi_0^{(7,7)}(\mathbf{x})}{n\beta^7} = \frac{1}{(7-1)!7! x^{12}} \left[ 7 \frac{\chi_0(7\mathbf{x})}{n\beta} + a_6 \frac{\chi_0(6\mathbf{x})}{n\beta} + a_5 \frac{\chi_0(5\mathbf{x})}{n\beta} + a_4 \frac{\chi_0(4\mathbf{x})}{n\beta} + a_3 \frac{\chi_0(3\mathbf{x})}{n\beta} + a_2 \frac{\chi_0(2\mathbf{x})}{n\beta} + a_1 \frac{\chi_0(\mathbf{x})}{n\beta} \right],$$

where

$$\begin{aligned} \frac{\chi_0(\mathbf{x})}{n\beta} &= -\frac{3}{2} \frac{\Theta}{x} \int_0^\infty y f_0(y; \Theta) \ln \left| \frac{x+2y}{x-2y} \right| dy, & \frac{\chi_0(2\mathbf{x})}{n\beta} &= -\frac{3}{2} \frac{\Theta}{2x} \int_0^\infty y f_0(y; \Theta) \ln \left| \frac{2x+2y}{2x-2y} \right| dy, \\ \frac{\chi_0(3\mathbf{x})}{n\beta} &= -\frac{3}{2} \frac{\Theta}{3x} \int_0^\infty y f_0(y; \Theta) \ln \left| \frac{3x+2y}{3x-2y} \right| dy, & \frac{\chi_0(4\mathbf{x})}{n\beta} &= -\frac{3}{2} \frac{\Theta}{4x} \int_0^\infty y f_0(y; \Theta) \ln \left| \frac{4x+2y}{4x-2y} \right| dy, \\ \frac{\chi_0(5\mathbf{x})}{n\beta} &= -\frac{3}{2} \frac{\Theta}{5x} \int_0^\infty y f_0(y; \Theta) \ln \left| \frac{5x+2y}{5x-2y} \right| dy, & \frac{\chi_0(6\mathbf{x})}{n\beta} &= -\frac{3}{2} \frac{\Theta}{6x} \int_0^\infty y f_0(y; \Theta) \ln \left| \frac{6x+2y}{6x-2y} \right| dy, \\ \frac{\chi_0(7\mathbf{x})}{n\beta} &= -\frac{3}{2} \frac{\Theta}{7x} \int_0^\infty y f_0(y; \Theta) \ln \left| \frac{7x+2y}{7x-2y} \right| dy. \end{aligned}$$

Given the  $x^{-12}$  pre-factor and the Taylor expansion of the even static Lindhard response  $\chi_0(\mathbf{x})/(n\beta)$ , the first six terms of the Taylor expansion of  $\chi_0^{(7,7)}(\mathbf{x})/(n\beta^7)$  need to cancel out exactly in the long-wavelength limit. Otherwise, the non-interacting UEF would be unstable against constant potential energy perturbations. This constraint yields exactly six linear equations for the determination of the unknown coefficients  $a_6, a_5, a_4, a_3, a_2, a_1$ . Let us compute the first six terms in the small argument expansion of the Lindhard density response at the first seven harmonics. This reads as

$$\begin{aligned} \frac{\chi_0(\mathbf{x})}{n\beta} &\simeq -\frac{3}{2} \Theta \int_0^\infty dy f_0(y; \Theta) \left[ 1 + \frac{1}{3} \frac{1}{4} \left( \frac{x}{y} \right)^2 + \frac{1}{5} \frac{1}{16} \left( \frac{x}{y} \right)^4 + \frac{1}{7} \frac{1}{64} \left( \frac{x}{y} \right)^6 + \frac{1}{9} \frac{1}{256} \left( \frac{x}{y} \right)^8 + \frac{1}{11} \frac{1}{1024} \left( \frac{x}{y} \right)^{10} \right], \\ \frac{\chi_0(2\mathbf{x})}{n\beta} &\simeq -\frac{3}{2} \Theta \int_0^\infty dy f_0(y; \Theta) \left[ 1 + \frac{1}{3} \frac{1}{4} \left( \frac{2x}{y} \right)^2 + \frac{1}{5} \frac{1}{16} \left( \frac{2x}{y} \right)^4 + \frac{1}{7} \frac{1}{64} \left( \frac{2x}{y} \right)^6 + \frac{1}{9} \frac{1}{256} \left( \frac{2x}{y} \right)^8 + \frac{1}{11} \frac{1}{1024} \left( \frac{2x}{y} \right)^{10} \right], \\ \frac{\chi_0(3\mathbf{x})}{n\beta} &\simeq -\frac{3}{2} \Theta \int_0^\infty dy f_0(y; \Theta) \left[ 1 + \frac{1}{3} \frac{1}{4} \left( \frac{3x}{y} \right)^2 + \frac{1}{5} \frac{1}{16} \left( \frac{3x}{y} \right)^4 + \frac{1}{7} \frac{1}{64} \left( \frac{3x}{y} \right)^6 + \frac{1}{9} \frac{1}{256} \left( \frac{3x}{y} \right)^8 + \frac{1}{11} \frac{1}{1024} \left( \frac{3x}{y} \right)^{10} \right], \\ \frac{\chi_0(4\mathbf{x})}{n\beta} &\simeq -\frac{3}{2} \Theta \int_0^\infty dy f_0(y; \Theta) \left[ 1 + \frac{1}{3} \frac{1}{4} \left( \frac{4x}{y} \right)^2 + \frac{1}{5} \frac{1}{16} \left( \frac{4x}{y} \right)^4 + \frac{1}{7} \frac{1}{64} \left( \frac{4x}{y} \right)^6 + \frac{1}{9} \frac{1}{256} \left( \frac{4x}{y} \right)^8 + \frac{1}{11} \frac{1}{1024} \left( \frac{4x}{y} \right)^{10} \right], \\ \frac{\chi_0(5\mathbf{x})}{n\beta} &\simeq -\frac{3}{2} \Theta \int_0^\infty dy f_0(y; \Theta) \left[ 1 + \frac{1}{3} \frac{1}{4} \left( \frac{5x}{y} \right)^2 + \frac{1}{5} \frac{1}{16} \left( \frac{5x}{y} \right)^4 + \frac{1}{7} \frac{1}{64} \left( \frac{5x}{y} \right)^6 + \frac{1}{9} \frac{1}{256} \left( \frac{5x}{y} \right)^8 + \frac{1}{11} \frac{1}{1024} \left( \frac{5x}{y} \right)^{10} \right], \\ \frac{\chi_0(6\mathbf{x})}{n\beta} &\simeq -\frac{3}{2} \Theta \int_0^\infty dy f_0(y; \Theta) \left[ 1 + \frac{1}{3} \frac{1}{4} \left( \frac{6x}{y} \right)^2 + \frac{1}{5} \frac{1}{16} \left( \frac{6x}{y} \right)^4 + \frac{1}{7} \frac{1}{64} \left( \frac{6x}{y} \right)^6 + \frac{1}{9} \frac{1}{256} \left( \frac{6x}{y} \right)^8 + \frac{1}{11} \frac{1}{1024} \left( \frac{6x}{y} \right)^{10} \right], \\ \frac{\chi_0(7\mathbf{x})}{n\beta} &\simeq -\frac{3}{2} \Theta \int_0^\infty dy f_0(y; \Theta) \left[ 1 + \frac{1}{3} \frac{1}{4} \left( \frac{7x}{y} \right)^2 + \frac{1}{5} \frac{1}{16} \left( \frac{7x}{y} \right)^4 + \frac{1}{7} \frac{1}{64} \left( \frac{7x}{y} \right)^6 + \frac{1}{9} \frac{1}{256} \left( \frac{7x}{y} \right)^8 + \frac{1}{11} \frac{1}{1024} \left( \frac{7x}{y} \right)^{10} \right] \Rightarrow \\ \frac{\chi_0(\mathbf{x})}{n\beta} &\simeq -\frac{3}{2} \Theta \int_0^\infty dy f_0(y; \Theta) \left[ 1 + \frac{1}{3} \frac{1}{4} \left( \frac{x}{y} \right)^2 + \frac{1}{5} \frac{1}{16} \left( \frac{x}{y} \right)^4 + \frac{1}{7} \frac{1}{64} \left( \frac{x}{y} \right)^6 + \frac{1}{9} \frac{1}{256} \left( \frac{x}{y} \right)^8 + \frac{1}{11} \frac{1}{1024} \left( \frac{x}{y} \right)^{10} \right], \\ \frac{\chi_0(2\mathbf{x})}{n\beta} &\simeq -\frac{3}{2} \Theta \int_0^\infty dy f_0(y; \Theta) \left[ 1 + \frac{1}{3} \frac{2^2}{4} \left( \frac{x}{y} \right)^2 + \frac{1}{5} \frac{2^4}{16} \left( \frac{x}{y} \right)^4 + \frac{1}{7} \frac{2^6}{64} \left( \frac{x}{y} \right)^6 + \frac{1}{9} \frac{2^8}{256} \left( \frac{x}{y} \right)^8 + \frac{1}{11} \frac{2^{10}}{1024} \left( \frac{x}{y} \right)^{10} \right], \end{aligned}$$

$$\begin{aligned}
\frac{\chi_0(3\mathbf{x})}{n\beta} &\simeq -\frac{3}{2}\Theta \int_0^\infty dy f_0(y; \Theta) \left[ 1 + \frac{1}{3} \frac{3^2}{4} \left(\frac{x}{y}\right)^2 + \frac{1}{5} \frac{3^4}{16} \left(\frac{x}{y}\right)^4 + \frac{1}{7} \frac{3^6}{64} \left(\frac{x}{y}\right)^6 + \frac{1}{9} \frac{3^8}{256} \left(\frac{x}{y}\right)^8 + \frac{1}{11} \frac{3^{10}}{1024} \left(\frac{x}{y}\right)^{10} \right], \\
\frac{\chi_0(4\mathbf{x})}{n\beta} &\simeq -\frac{3}{2}\Theta \int_0^\infty dy f_0(y; \Theta) \left[ 1 + \frac{1}{3} \frac{4^2}{4} \left(\frac{x}{y}\right)^2 + \frac{1}{5} \frac{4^4}{16} \left(\frac{x}{y}\right)^4 + \frac{1}{7} \frac{4^6}{64} \left(\frac{x}{y}\right)^6 + \frac{1}{9} \frac{4^8}{256} \left(\frac{x}{y}\right)^8 + \frac{1}{11} \frac{4^{10}}{1024} \left(\frac{x}{y}\right)^{10} \right], \\
\frac{\chi_0(5\mathbf{x})}{n\beta} &\simeq -\frac{3}{2}\Theta \int_0^\infty dy f_0(y; \Theta) \left[ 1 + \frac{1}{3} \frac{5^2}{4} \left(\frac{x}{y}\right)^2 + \frac{1}{5} \frac{5^4}{16} \left(\frac{x}{y}\right)^4 + \frac{1}{7} \frac{5^6}{64} \left(\frac{x}{y}\right)^6 + \frac{1}{9} \frac{5^8}{256} \left(\frac{x}{y}\right)^8 + \frac{1}{11} \frac{5^{10}}{1024} \left(\frac{x}{y}\right)^{10} \right], \\
\frac{\chi_0(6\mathbf{x})}{n\beta} &\simeq -\frac{3}{2}\Theta \int_0^\infty dy f_0(y; \Theta) \left[ 1 + \frac{1}{3} \frac{6^2}{4} \left(\frac{x}{y}\right)^2 + \frac{1}{5} \frac{6^4}{16} \left(\frac{x}{y}\right)^4 + \frac{1}{7} \frac{6^6}{64} \left(\frac{x}{y}\right)^6 + \frac{1}{9} \frac{6^8}{256} \left(\frac{x}{y}\right)^8 + \frac{1}{11} \frac{6^{10}}{1024} \left(\frac{x}{y}\right)^{10} \right], \\
\frac{\chi_0(7\mathbf{x})}{n\beta} &\simeq -\frac{3}{2}\Theta \int_0^\infty dy f_0(y; \Theta) \left[ 1 + \frac{1}{3} \frac{7^2}{4} \left(\frac{x}{y}\right)^2 + \frac{1}{5} \frac{7^4}{16} \left(\frac{x}{y}\right)^4 + \frac{1}{7} \frac{7^6}{64} \left(\frac{x}{y}\right)^6 + \frac{1}{9} \frac{7^8}{256} \left(\frac{x}{y}\right)^8 + \frac{1}{11} \frac{7^{10}}{1024} \left(\frac{x}{y}\right)^{10} \right] \Rightarrow \\
\frac{\chi_0(\mathbf{x})}{n\beta} &\simeq -\frac{3}{2}\Theta \int_0^\infty dy f_0(y; \Theta) \left[ 1 + \frac{1}{12} \left(\frac{x}{y}\right)^2 + \frac{1}{80} \left(\frac{x}{y}\right)^4 + \frac{1}{448} \left(\frac{x}{y}\right)^6 + \frac{1}{2304} \left(\frac{x}{y}\right)^8 + \frac{1}{11264} \left(\frac{x}{y}\right)^{10} \right], \\
\frac{\chi_0(2\mathbf{x})}{n\beta} &\simeq -\frac{3}{2}\Theta \int_0^\infty dy f_0(y; \Theta) \left[ 1 + \frac{1}{3} \left(\frac{x}{y}\right)^2 + \frac{1}{5} \left(\frac{x}{y}\right)^4 + \frac{1}{7} \left(\frac{x}{y}\right)^6 + \frac{1}{9} \left(\frac{x}{y}\right)^8 + \frac{1}{11} \left(\frac{x}{y}\right)^{10} \right], \\
\frac{\chi_0(3\mathbf{x})}{n\beta} &\simeq -\frac{3}{2}\Theta \int_0^\infty dy f_0(y; \Theta) \left[ 1 + \frac{3}{4} \left(\frac{x}{y}\right)^2 + \frac{81}{80} \left(\frac{x}{y}\right)^4 + \frac{729}{448} \left(\frac{x}{y}\right)^6 + \frac{6561}{2304} \left(\frac{x}{y}\right)^8 + \frac{59049}{11264} \left(\frac{x}{y}\right)^{10} \right], \\
\frac{\chi_0(4\mathbf{x})}{n\beta} &\simeq -\frac{3}{2}\Theta \int_0^\infty dy f_0(y; \Theta) \left[ 1 + \frac{4}{3} \left(\frac{x}{y}\right)^2 + \frac{16}{5} \left(\frac{x}{y}\right)^4 + \frac{64}{7} \left(\frac{x}{y}\right)^6 + \frac{256}{9} \left(\frac{x}{y}\right)^8 + \frac{1024}{11} \left(\frac{x}{y}\right)^{10} \right], \\
\frac{\chi_0(5\mathbf{x})}{n\beta} &\simeq -\frac{3}{2}\Theta \int_0^\infty dy f_0(y; \Theta) \left[ 1 + \frac{25}{12} \left(\frac{x}{y}\right)^2 + \frac{125}{16} \left(\frac{x}{y}\right)^4 + \frac{15625}{448} \left(\frac{x}{y}\right)^6 + \frac{390625}{2304} \left(\frac{x}{y}\right)^8 + \frac{9765625}{11264} \left(\frac{x}{y}\right)^{10} \right], \\
\frac{\chi_0(6\mathbf{x})}{n\beta} &\simeq -\frac{3}{2}\Theta \int_0^\infty dy f_0(y; \Theta) \left[ 1 + 3 \left(\frac{x}{y}\right)^2 + \frac{81}{5} \left(\frac{x}{y}\right)^4 + \frac{729}{7} \left(\frac{x}{y}\right)^6 + 729 \left(\frac{x}{y}\right)^8 + \frac{59049}{11} \left(\frac{x}{y}\right)^{10} \right], \\
\frac{\chi_0(7\mathbf{x})}{n\beta} &\simeq -\frac{3}{2}\Theta \int_0^\infty dy f_0(y; \Theta) \left[ 1 + \frac{49}{12} \left(\frac{x}{y}\right)^2 + \frac{2401}{80} \left(\frac{x}{y}\right)^4 + \frac{16807}{64} \left(\frac{x}{y}\right)^6 + \frac{5764801}{2304} \left(\frac{x}{y}\right)^8 + \frac{282475249}{11264} \left(\frac{x}{y}\right)^{10} \right].
\end{aligned}$$

Substituting in the canonical form, ordering in powers of  $1/x^{12}$ ,  $1/x^{10}$ ,  $1/x^8$ ,  $1/x^6$ ,  $1/x^4$ ,  $1/x^2$ , taking the limit  $x \rightarrow 0$  and equating each coefficient with zero (as demanded by the stability requirement) leads to the  $6 \times 6$  system of equations  $Ma = b$  where the  $6 \times 6$  matrix  $M$  is given by

$$\begin{pmatrix}
1 & \frac{1}{25} & \frac{1}{4} & \frac{1}{3} & \frac{1}{1} & \frac{1}{12} \\
3 & \frac{12}{12} & \frac{3}{3} & \frac{4}{4} & \frac{1}{3} & \frac{1}{12} \\
\frac{81}{5} & \frac{125}{16} & \frac{16}{5} & \frac{81}{80} & \frac{1}{5} & \frac{1}{80} \\
\frac{729}{7} & \frac{15625}{448} & \frac{64}{7} & \frac{729}{448} & \frac{1}{7} & \frac{1}{448} \\
729 & \frac{390625}{2304} & \frac{256}{9} & \frac{729}{256} & \frac{1}{9} & \frac{1}{2304} \\
\frac{59049}{11} & \frac{9765625}{11264} & \frac{1024}{11} & \frac{59049}{11264} & \frac{1}{11} & \frac{1}{11264}
\end{pmatrix}$$

the 6-dim source vector  $b$  is given by  $(-7, -343/12, -16807/80, -117649/64, -40353607/2304, -1977326743/11264)$ , whereas the 6-dim unknown vector  $a$  is defined by  $a = (a_6, a_5, a_4, a_3, a_2, a_1)$ . The solution is  $(a_6, a_5, a_4, a_3, a_2, a_1) = (-72, 325, -832, 1287, -1144, 429)$ . It should be pointed out that the unknown coefficients can only be integers, which constitutes a straightforward way to check for misprints. Therefore, the canonical form of the normalized septic ideal

density response at the seventh harmonic reads as

$$\frac{\chi_0^{(7,7)}(\mathbf{x}, Z)}{n\beta^7} = \frac{1}{(7-1)!7!} \frac{\Theta^6}{x^{12}} \left[ 7 \frac{\chi_0(7\mathbf{x}, 7Z)}{n\beta} - 72 \frac{\chi_0(6\mathbf{x}, 6Z)}{n\beta} + 325 \frac{\chi_0(5\mathbf{x}, 5Z)}{n\beta} - 832 \frac{\chi_0(4\mathbf{x}, 4Z)}{n\beta} + 1287 \frac{\chi_0(3\mathbf{x}, 3Z)}{n\beta} - 1144 \frac{\chi_0(2\mathbf{x}, 2Z)}{n\beta} + 429 \frac{\chi_0(\mathbf{x}, Z)}{n\beta} \right]$$

In order to obtain the long-wavelength limit of the normalized septic static ideal density response at the seventh harmonic, given the automatic cancellations due to the stability requirement, it suffices to consider the seventh term of the small argument expansion of the Lindhard density response constituents alone. This leads to

$$\begin{aligned} \frac{\chi_0^{(7,7)}(\mathbf{x})}{n\beta^7} &= \frac{1}{(7-1)!7!} \frac{\Theta^6}{x^{12}} \left[ 7 \frac{\chi_0(7\mathbf{x})}{n\beta} - 72 \frac{\chi_0(6\mathbf{x})}{n\beta} + 325 \frac{\chi_0(5\mathbf{x})}{n\beta} - 832 \frac{\chi_0(4\mathbf{x})}{n\beta} + 1287 \frac{\chi_0(3\mathbf{x})}{n\beta} - 1144 \frac{\chi_0(2\mathbf{x})}{n\beta} + 429 \frac{\chi_0(\mathbf{x})}{n\beta} \right] \Rightarrow \\ \frac{\chi_0^{(7,7)}(\mathbf{x})}{n\beta^7} &= -\frac{1}{(7-1)!7!} \frac{\Theta^6}{x^{12}} \left\{ 7 \frac{3}{2} \Theta \int_0^\infty dy f_0(y; \Theta) \frac{1}{13} \frac{1}{4096} \left( \frac{7x}{y} \right)^{12} - 72 \frac{3}{2} \Theta \int_0^\infty dy f_0(y; \Theta) \frac{1}{13} \frac{1}{4096} \left( \frac{6x}{y} \right)^{12} \right. \\ &\quad + 325 \frac{3}{2} \Theta \int_0^\infty dy f_0(y; \Theta) \frac{1}{13} \frac{1}{4096} \left( \frac{5x}{y} \right)^{12} - 832 \frac{3}{2} \Theta \int_0^\infty dy f_0(y; \Theta) \frac{1}{13} \frac{1}{4096} \left( \frac{4x}{y} \right)^{12} \\ &\quad + 1287 \frac{3}{2} \Theta \int_0^\infty dy f_0(y; \Theta) \frac{1}{13} \frac{1}{4096} \left( \frac{3x}{y} \right)^{12} - 1144 \frac{3}{2} \Theta \int_0^\infty dy f_0(y; \Theta) \frac{1}{13} \frac{1}{4096} \left( \frac{2x}{y} \right)^{12} \\ &\quad \left. + 429 \frac{3}{2} \Theta \int_0^\infty dy f_0(y; \Theta) \frac{1}{13} \frac{1}{4096} \left( \frac{x}{y} \right)^{12} \right\} \Rightarrow \\ \frac{\chi_0^{(7,7)}(\mathbf{x})}{n\beta^7} &= -\frac{1}{3628800} \frac{\Theta^6}{x^{12}} \frac{3}{2} \Theta \int_0^\infty dy f_0(y; \Theta) \left\{ \frac{7}{13} \frac{7^{12}}{4096} \left( \frac{x}{y} \right)^{12} - \frac{72}{13} \frac{6^{12}}{4096} \left( \frac{x}{y} \right)^{12} + \frac{325}{13} \frac{5^{12}}{4096} \left( \frac{x}{y} \right)^{12} \right. \\ &\quad \left. - \frac{832}{13} \frac{4^{12}}{4096} \left( \frac{x}{y} \right)^{12} + \frac{1287}{13} \frac{3^{12}}{4096} \left( \frac{x}{y} \right)^{12} - \frac{1144}{13} \frac{2^{12}}{4096} \left( \frac{x}{y} \right)^{12} + \frac{429}{13} \frac{1}{4096} \left( \frac{x}{y} \right)^{12} \right\} \Rightarrow \\ \frac{\chi_0^{(7,7)}(\mathbf{x})}{n\beta^7} &= -\frac{1}{2419200} \frac{\Theta^7}{x^{12}} \int_0^\infty dy f_0(y; \Theta) \left\{ \frac{7}{13} \frac{7^{12}}{4096} \left( \frac{x}{y} \right)^{12} - \frac{72}{13} \frac{6^{12}}{4096} \left( \frac{x}{y} \right)^{12} + \frac{325}{13} \frac{5^{12}}{4096} \left( \frac{x}{y} \right)^{12} \right. \\ &\quad \left. - \frac{832}{13} \frac{4^{12}}{4096} \left( \frac{x}{y} \right)^{12} + \frac{1287}{13} \frac{3^{12}}{4096} \left( \frac{x}{y} \right)^{12} - \frac{1144}{13} \frac{2^{12}}{4096} \left( \frac{x}{y} \right)^{12} + \frac{429}{13} \frac{1}{4096} \left( \frac{x}{y} \right)^{12} \right\} \Rightarrow \\ \frac{\chi_0^{(7,7)}(\mathbf{x})}{n\beta^7} &= -\frac{1}{2419200} \frac{\Theta^7}{x^{12}} \int_0^\infty dy f_0(y; \Theta) \left\{ \frac{7^{13}}{53248} \left( \frac{x}{y} \right)^{12} - \frac{72 \times 6^{12}}{53248} \left( \frac{x}{y} \right)^{12} + \frac{325 \times 5^{12}}{53248} \left( \frac{x}{y} \right)^{12} \right. \\ &\quad \left. - \frac{832 \times 4^{12}}{53248} \left( \frac{x}{y} \right)^{12} + \frac{1287 \times 3^{12}}{53248} \left( \frac{x}{y} \right)^{12} - \frac{1144 \times 2^{12}}{53248} \left( \frac{x}{y} \right)^{12} + \frac{429}{53248} \left( \frac{x}{y} \right)^{12} \right\} \Rightarrow \\ \frac{\chi_0^{(7,7)}(\mathbf{x})}{n\beta^7} &= -\frac{1}{2419200} \frac{\Theta^7}{x^{12}} \int_0^\infty dy f_0(y; \Theta) \left\{ \frac{7^{13} - 72 \times 6^{12} + 325 \times 5^{12} - 832 \times 4^{12} + 1287 \times 3^{12} - 1144 \times 2^{12} + 429}{53248} \right\} \left( \frac{x}{y} \right)^{12} \\ \frac{\chi_0^{(7,7)}(\mathbf{x})}{n\beta^7} &= -\frac{1}{2419200} \Theta^7 \left\{ \frac{7^{13} - 72 \times 6^{12} + 325 \times 5^{12} - 832 \times 4^{12} + 1287 \times 3^{12} - 1144 \times 2^{12} + 429}{53248} \right\} \int_0^\infty dy \frac{f_0(y; \Theta)}{x^{12}} \frac{x^{12}}{y^{12}} \Rightarrow \\ \frac{\chi_0^{(7,7)}(\mathbf{x})}{n\beta^7} &= -\frac{1}{2419200} \Theta^7 \left\{ \frac{7^{13} - 72 \times 6^{12} + 325 \times 5^{12} - 832 \times 4^{12} + 1287 \times 3^{12} - 1144 \times 2^{12} + 429}{53248} \right\} \int_0^\infty dy \frac{f_0(y; \Theta)}{y^{12}} \Rightarrow \\ \frac{\chi_0^{(7,7)}(\mathbf{x})}{n\beta^7} &= -\frac{6227020800}{128817561600} \Theta^7 \int_0^\infty dy \frac{f_0(y; \Theta)}{y^{12}} \Rightarrow \\ \frac{\chi_0^{(7,7)}(\mathbf{x})}{n\beta^7} &= -\frac{6227020800}{62899200} \frac{62899200}{128817561600} \Theta^7 \int_0^\infty dy \frac{f_0(y; \Theta)}{y^{12}} \Rightarrow \\ \frac{\chi_0^{(7,7)}(\mathbf{x})}{n\beta^7} &= -\frac{99}{2048} \Theta^7 \int_0^\infty dy \frac{f_0(y; \Theta)}{y^{12}}. \end{aligned}$$

### C. The eighth-order (octic) ideal density response

Based on the arbitrary perturbation order methodology that was outlined earlier, the general form of the normalized octic ideal density response at the eighth harmonic reads as

$$\frac{\chi_0^{(8,8)}(\mathbf{x}, Z)}{n\beta^8} = \frac{1}{(8-1)!8!} \frac{\Theta^7}{x^{14}} \left[ 8 \frac{\chi_0(8\mathbf{x}, 8Z)}{n\beta} + a_7 \frac{\chi_0(7\mathbf{x}, 7Z)}{n\beta} + a_6 \frac{\chi_0(6\mathbf{x}, 6Z)}{n\beta} + a_5 \frac{\chi_0(5\mathbf{x}, 5Z)}{n\beta} + a_4 \frac{\chi_0(4\mathbf{x}, 4Z)}{n\beta} + a_3 \frac{\chi_0(3\mathbf{x}, 3Z)}{n\beta} + a_2 \frac{\chi_0(2\mathbf{x}, 2Z)}{n\beta} + a_1 \frac{\chi_0(\mathbf{x}, Z)}{n\beta} \right] + \dots$$

The key for determination of the coefficients  $a_7, a_6, a_5, a_4, a_3, a_2, a_1$  lies in the behavior of the static density responses,

$$\frac{\chi_0^{(8,8)}(\mathbf{x})}{n\beta^8} = \frac{1}{(8-1)!8!} \frac{\Theta^7}{x^{14}} \left[ 8 \frac{\chi_0(8\mathbf{x})}{n\beta} + a_7 \frac{\chi_0(7\mathbf{x})}{n\beta} + a_6 \frac{\chi_0(6\mathbf{x})}{n\beta} + a_5 \frac{\chi_0(5\mathbf{x})}{n\beta} + a_4 \frac{\chi_0(4\mathbf{x})}{n\beta} + a_3 \frac{\chi_0(3\mathbf{x})}{n\beta} + a_2 \frac{\chi_0(2\mathbf{x})}{n\beta} + a_1 \frac{\chi_0(\mathbf{x})}{n\beta} \right],$$

where

$$\begin{aligned} \frac{\chi_0(\mathbf{x})}{n\beta} &= -\frac{3}{2} \frac{\Theta}{x} \int_0^\infty y f_0(y; \Theta) \ln \left| \frac{x+2y}{x-2y} \right| dy, & \frac{\chi_0(2\mathbf{x})}{n\beta} &= -\frac{3}{2} \frac{\Theta}{2x} \int_0^\infty y f_0(y; \Theta) \ln \left| \frac{2x+2y}{2x-2y} \right| dy, \\ \frac{\chi_0(3\mathbf{x})}{n\beta} &= -\frac{3}{2} \frac{\Theta}{3x} \int_0^\infty y f_0(y; \Theta) \ln \left| \frac{3x+2y}{3x-2y} \right| dy, & \frac{\chi_0(4\mathbf{x})}{n\beta} &= -\frac{3}{2} \frac{\Theta}{4x} \int_0^\infty y f_0(y; \Theta) \ln \left| \frac{4x+2y}{4x-2y} \right| dy, \\ \frac{\chi_0(5\mathbf{x})}{n\beta} &= -\frac{3}{2} \frac{\Theta}{5x} \int_0^\infty y f_0(y; \Theta) \ln \left| \frac{5x+2y}{5x-2y} \right| dy, & \frac{\chi_0(6\mathbf{x})}{n\beta} &= -\frac{3}{2} \frac{\Theta}{6x} \int_0^\infty y f_0(y; \Theta) \ln \left| \frac{6x+2y}{6x-2y} \right| dy, \\ \frac{\chi_0(7\mathbf{x})}{n\beta} &= -\frac{3}{2} \frac{\Theta}{7x} \int_0^\infty y f_0(y; \Theta) \ln \left| \frac{7x+2y}{7x-2y} \right| dy, & \frac{\chi_0(8\mathbf{x})}{n\beta} &= -\frac{3}{2} \frac{\Theta}{8x} \int_0^\infty y f_0(y; \Theta) \ln \left| \frac{8x+2y}{8x-2y} \right| dy. \end{aligned}$$

Given the  $x^{-14}$  pre-factor and the Taylor expansion of the even static Lindhard response  $\chi_0(\mathbf{x})/(n\beta)$ , the first seven terms of the Taylor expansion of  $\chi_0^{(8,8)}(\mathbf{x})/(n\beta^8)$  need to cancel out exactly in the long-wavelength limit. Otherwise, the non-interacting UEF would be unstable against constant potential energy perturbations. This constraint yields exactly seven linear equations for the determination of the unknown coefficients  $a_7, a_6, a_5, a_4, a_3, a_2, a_1$ . Let us compute the first seven terms in the small argument expansion of the Lindhard density response at the first eight harmonics. This reads as

$$\begin{aligned} \frac{\chi_0(\mathbf{x})}{n\beta} &\simeq -\frac{3}{2} \Theta \int_0^\infty dy f_0(y; \Theta) \left[ 1 + \frac{1}{3} \frac{1}{4} \left( \frac{x}{y} \right)^2 + \frac{1}{5} \frac{1}{16} \left( \frac{x}{y} \right)^4 + \frac{1}{7} \frac{1}{64} \left( \frac{x}{y} \right)^6 + \frac{1}{9} \frac{1}{256} \left( \frac{x}{y} \right)^8 + \frac{1}{11} \frac{1}{1024} \left( \frac{x}{y} \right)^{10} + \frac{1}{13} \frac{1}{4096} \left( \frac{x}{y} \right)^{12} \right], \\ \frac{\chi_0(2\mathbf{x})}{n\beta} &\simeq -\frac{3}{2} \Theta \int_0^\infty dy f_0(y; \Theta) \left[ 1 + \frac{1}{3} \frac{1}{4} \left( \frac{2x}{y} \right)^2 + \frac{1}{5} \frac{1}{16} \left( \frac{2x}{y} \right)^4 + \frac{1}{7} \frac{1}{64} \left( \frac{2x}{y} \right)^6 + \frac{1}{9} \frac{1}{256} \left( \frac{2x}{y} \right)^8 + \frac{1}{11} \frac{1}{1024} \left( \frac{2x}{y} \right)^{10} + \frac{1}{13} \frac{1}{4096} \left( \frac{2x}{y} \right)^{12} \right], \\ \frac{\chi_0(3\mathbf{x})}{n\beta} &\simeq -\frac{3}{2} \Theta \int_0^\infty dy f_0(y; \Theta) \left[ 1 + \frac{1}{3} \frac{1}{4} \left( \frac{3x}{y} \right)^2 + \frac{1}{5} \frac{1}{16} \left( \frac{3x}{y} \right)^4 + \frac{1}{7} \frac{1}{64} \left( \frac{3x}{y} \right)^6 + \frac{1}{9} \frac{1}{256} \left( \frac{3x}{y} \right)^8 + \frac{1}{11} \frac{1}{1024} \left( \frac{3x}{y} \right)^{10} + \frac{1}{13} \frac{1}{4096} \left( \frac{3x}{y} \right)^{12} \right], \\ \frac{\chi_0(4\mathbf{x})}{n\beta} &\simeq -\frac{3}{2} \Theta \int_0^\infty dy f_0(y; \Theta) \left[ 1 + \frac{1}{3} \frac{1}{4} \left( \frac{4x}{y} \right)^2 + \frac{1}{5} \frac{1}{16} \left( \frac{4x}{y} \right)^4 + \frac{1}{7} \frac{1}{64} \left( \frac{4x}{y} \right)^6 + \frac{1}{9} \frac{1}{256} \left( \frac{4x}{y} \right)^8 + \frac{1}{11} \frac{1}{1024} \left( \frac{4x}{y} \right)^{10} + \frac{1}{13} \frac{1}{4096} \left( \frac{4x}{y} \right)^{12} \right], \\ \frac{\chi_0(5\mathbf{x})}{n\beta} &\simeq -\frac{3}{2} \Theta \int_0^\infty dy f_0(y; \Theta) \left[ 1 + \frac{1}{3} \frac{1}{4} \left( \frac{5x}{y} \right)^2 + \frac{1}{5} \frac{1}{16} \left( \frac{5x}{y} \right)^4 + \frac{1}{7} \frac{1}{64} \left( \frac{5x}{y} \right)^6 + \frac{1}{9} \frac{1}{256} \left( \frac{5x}{y} \right)^8 + \frac{1}{11} \frac{1}{1024} \left( \frac{5x}{y} \right)^{10} + \frac{1}{13} \frac{1}{4096} \left( \frac{5x}{y} \right)^{12} \right], \\ \frac{\chi_0(6\mathbf{x})}{n\beta} &\simeq -\frac{3}{2} \Theta \int_0^\infty dy f_0(y; \Theta) \left[ 1 + \frac{1}{3} \frac{1}{4} \left( \frac{6x}{y} \right)^2 + \frac{1}{5} \frac{1}{16} \left( \frac{6x}{y} \right)^4 + \frac{1}{7} \frac{1}{64} \left( \frac{6x}{y} \right)^6 + \frac{1}{9} \frac{1}{256} \left( \frac{6x}{y} \right)^8 + \frac{1}{11} \frac{1}{1024} \left( \frac{6x}{y} \right)^{10} + \frac{1}{13} \frac{1}{4096} \left( \frac{6x}{y} \right)^{12} \right], \\ \frac{\chi_0(7\mathbf{x})}{n\beta} &\simeq -\frac{3}{2} \Theta \int_0^\infty dy f_0(y; \Theta) \left[ 1 + \frac{1}{3} \frac{1}{4} \left( \frac{7x}{y} \right)^2 + \frac{1}{5} \frac{1}{16} \left( \frac{7x}{y} \right)^4 + \frac{1}{7} \frac{1}{64} \left( \frac{7x}{y} \right)^6 + \frac{1}{9} \frac{1}{256} \left( \frac{7x}{y} \right)^8 + \frac{1}{11} \frac{1}{1024} \left( \frac{7x}{y} \right)^{10} + \frac{1}{13} \frac{1}{4096} \left( \frac{7x}{y} \right)^{12} \right], \\ \frac{\chi_0(8\mathbf{x})}{n\beta} &\simeq -\frac{3}{2} \Theta \int_0^\infty dy f_0(y; \Theta) \left[ 1 + \frac{1}{3} \frac{1}{4} \left( \frac{8x}{y} \right)^2 + \frac{1}{5} \frac{1}{16} \left( \frac{8x}{y} \right)^4 + \frac{1}{7} \frac{1}{64} \left( \frac{8x}{y} \right)^6 + \frac{1}{9} \frac{1}{256} \left( \frac{8x}{y} \right)^8 + \frac{1}{11} \frac{1}{1024} \left( \frac{8x}{y} \right)^{10} + \frac{1}{13} \frac{1}{4096} \left( \frac{8x}{y} \right)^{12} \right] \Rightarrow \\ \frac{\chi_0(\mathbf{x})}{n\beta} &\simeq -\frac{3}{2} \Theta \int_0^\infty dy f_0(y; \Theta) \left[ 1 + \frac{1}{3} \frac{1}{4} \left( \frac{x}{y} \right)^2 + \frac{1}{5} \frac{1}{16} \left( \frac{x}{y} \right)^4 + \frac{1}{7} \frac{1}{64} \left( \frac{x}{y} \right)^6 + \frac{1}{9} \frac{1}{256} \left( \frac{x}{y} \right)^8 + \frac{1}{11} \frac{1}{1024} \left( \frac{x}{y} \right)^{10} + \frac{1}{13} \frac{1}{4096} \left( \frac{x}{y} \right)^{12} \right], \\ \frac{\chi_0(2\mathbf{x})}{n\beta} &\simeq -\frac{3}{2} \Theta \int_0^\infty dy f_0(y; \Theta) \left[ 1 + \frac{1}{3} \frac{2^2}{4} \left( \frac{x}{y} \right)^2 + \frac{1}{5} \frac{2^4}{16} \left( \frac{x}{y} \right)^4 + \frac{1}{7} \frac{2^6}{64} \left( \frac{x}{y} \right)^6 + \frac{1}{9} \frac{2^8}{256} \left( \frac{x}{y} \right)^8 + \frac{1}{11} \frac{2^{10}}{1024} \left( \frac{x}{y} \right)^{10} + \frac{1}{13} \frac{2^{12}}{4096} \left( \frac{x}{y} \right)^{12} \right], \\ \frac{\chi_0(3\mathbf{x})}{n\beta} &\simeq -\frac{3}{2} \Theta \int_0^\infty dy f_0(y; \Theta) \left[ 1 + \frac{1}{3} \frac{3^2}{4} \left( \frac{x}{y} \right)^2 + \frac{1}{5} \frac{3^4}{16} \left( \frac{x}{y} \right)^4 + \frac{1}{7} \frac{3^6}{64} \left( \frac{x}{y} \right)^6 + \frac{1}{9} \frac{3^8}{256} \left( \frac{x}{y} \right)^8 + \frac{1}{11} \frac{3^{10}}{1024} \left( \frac{x}{y} \right)^{10} + \frac{1}{13} \frac{3^{12}}{4096} \left( \frac{x}{y} \right)^{12} \right], \end{aligned}$$

$$\begin{aligned}
\frac{\chi_0(4\mathbf{x})}{n\beta} &\simeq -\frac{3}{2}\Theta \int_0^\infty dy f_0(y; \Theta) \left[ 1 + \frac{1}{3} \frac{4^2}{4} \left(\frac{x}{y}\right)^2 + \frac{1}{5} \frac{4^4}{16} \left(\frac{x}{y}\right)^4 + \frac{1}{7} \frac{4^6}{64} \left(\frac{x}{y}\right)^6 + \frac{1}{9} \frac{4^8}{256} \left(\frac{x}{y}\right)^8 + \frac{1}{11} \frac{4^{10}}{1024} \left(\frac{x}{y}\right)^{10} + \frac{1}{13} \frac{4^{12}}{4096} \left(\frac{x}{y}\right)^{12} \right], \\
\frac{\chi_0(5\mathbf{x})}{n\beta} &\simeq -\frac{3}{2}\Theta \int_0^\infty dy f_0(y; \Theta) \left[ 1 + \frac{1}{3} \frac{5^2}{4} \left(\frac{x}{y}\right)^2 + \frac{1}{5} \frac{5^4}{16} \left(\frac{x}{y}\right)^4 + \frac{1}{7} \frac{5^6}{64} \left(\frac{x}{y}\right)^6 + \frac{1}{9} \frac{5^8}{256} \left(\frac{x}{y}\right)^8 + \frac{1}{11} \frac{5^{10}}{1024} \left(\frac{x}{y}\right)^{10} + \frac{1}{13} \frac{5^{12}}{4096} \left(\frac{x}{y}\right)^{12} \right], \\
\frac{\chi_0(6\mathbf{x})}{n\beta} &\simeq -\frac{3}{2}\Theta \int_0^\infty dy f_0(y; \Theta) \left[ 1 + \frac{1}{3} \frac{6^2}{4} \left(\frac{x}{y}\right)^2 + \frac{1}{5} \frac{6^4}{16} \left(\frac{x}{y}\right)^4 + \frac{1}{7} \frac{6^6}{64} \left(\frac{x}{y}\right)^6 + \frac{1}{9} \frac{6^8}{256} \left(\frac{x}{y}\right)^8 + \frac{1}{11} \frac{6^{10}}{1024} \left(\frac{x}{y}\right)^{10} + \frac{1}{13} \frac{6^{12}}{4096} \left(\frac{x}{y}\right)^{12} \right], \\
\frac{\chi_0(7\mathbf{x})}{n\beta} &\simeq -\frac{3}{2}\Theta \int_0^\infty dy f_0(y; \Theta) \left[ 1 + \frac{1}{3} \frac{7^2}{4} \left(\frac{x}{y}\right)^2 + \frac{1}{5} \frac{7^4}{16} \left(\frac{x}{y}\right)^4 + \frac{1}{7} \frac{7^6}{64} \left(\frac{x}{y}\right)^6 + \frac{1}{9} \frac{7^8}{256} \left(\frac{x}{y}\right)^8 + \frac{1}{11} \frac{7^{10}}{1024} \left(\frac{x}{y}\right)^{10} + \frac{1}{13} \frac{7^{12}}{4096} \left(\frac{x}{y}\right)^{12} \right], \\
\frac{\chi_0(8\mathbf{x})}{n\beta} &\simeq -\frac{3}{2}\Theta \int_0^\infty dy f_0(y; \Theta) \left[ 1 + \frac{1}{3} \frac{8^2}{4} \left(\frac{x}{y}\right)^2 + \frac{1}{5} \frac{8^4}{16} \left(\frac{x}{y}\right)^4 + \frac{1}{7} \frac{8^6}{64} \left(\frac{x}{y}\right)^6 + \frac{1}{9} \frac{8^8}{256} \left(\frac{x}{y}\right)^8 + \frac{1}{11} \frac{8^{10}}{1024} \left(\frac{x}{y}\right)^{10} + \frac{1}{13} \frac{8^{12}}{4096} \left(\frac{x}{y}\right)^{12} \right] \Rightarrow \\
\frac{\chi_0(\mathbf{x})}{n\beta} &\simeq -\frac{3}{2}\Theta \int_0^\infty dy f_0(y; \Theta) \left[ 1 + \frac{1}{12} \left(\frac{x}{y}\right)^2 + \frac{1}{80} \left(\frac{x}{y}\right)^4 + \frac{1}{448} \left(\frac{x}{y}\right)^6 + \frac{1}{2304} \left(\frac{x}{y}\right)^8 + \frac{1}{11264} \left(\frac{x}{y}\right)^{10} + \frac{1}{53248} \left(\frac{x}{y}\right)^{12} \right], \\
\frac{\chi_0(2\mathbf{x})}{n\beta} &\simeq -\frac{3}{2}\Theta \int_0^\infty dy f_0(y; \Theta) \left[ 1 + \frac{1}{3} \left(\frac{x}{y}\right)^2 + \frac{1}{5} \left(\frac{x}{y}\right)^4 + \frac{1}{7} \left(\frac{x}{y}\right)^6 + \frac{1}{9} \left(\frac{x}{y}\right)^8 + \frac{1}{11} \left(\frac{x}{y}\right)^{10} + \frac{1}{13} \left(\frac{x}{y}\right)^{12} \right], \\
\frac{\chi_0(3\mathbf{x})}{n\beta} &\simeq -\frac{3}{2}\Theta \int_0^\infty dy f_0(y; \Theta) \left[ 1 + \frac{3}{4} \left(\frac{x}{y}\right)^2 + \frac{81}{80} \left(\frac{x}{y}\right)^4 + \frac{729}{448} \left(\frac{x}{y}\right)^6 + \frac{729}{256} \left(\frac{x}{y}\right)^8 + \frac{59049}{11264} \left(\frac{x}{y}\right)^{10} + \frac{531441}{53248} \left(\frac{x}{y}\right)^{12} \right], \\
\frac{\chi_0(4\mathbf{x})}{n\beta} &\simeq -\frac{3}{2}\Theta \int_0^\infty dy f_0(y; \Theta) \left[ 1 + \frac{4}{3} \left(\frac{x}{y}\right)^2 + \frac{16}{5} \left(\frac{x}{y}\right)^4 + \frac{64}{7} \left(\frac{x}{y}\right)^6 + \frac{256}{9} \left(\frac{x}{y}\right)^8 + \frac{1024}{11} \left(\frac{x}{y}\right)^{10} + \frac{4096}{13} \left(\frac{x}{y}\right)^{12} \right], \\
\frac{\chi_0(5\mathbf{x})}{n\beta} &\simeq -\frac{3}{2}\Theta \int_0^\infty dy f_0(y; \Theta) \left[ 1 + \frac{25}{12} \left(\frac{x}{y}\right)^2 + \frac{125}{16} \left(\frac{x}{y}\right)^4 + \frac{15625}{448} \left(\frac{x}{y}\right)^6 + \frac{390625}{2304} \left(\frac{x}{y}\right)^8 + \frac{9765625}{11264} \left(\frac{x}{y}\right)^{10} + \frac{244140625}{53248} \left(\frac{x}{y}\right)^{12} \right], \\
\frac{\chi_0(6\mathbf{x})}{n\beta} &\simeq -\frac{3}{2}\Theta \int_0^\infty dy f_0(y; \Theta) \left[ 1 + 3 \left(\frac{x}{y}\right)^2 + \frac{81}{5} \left(\frac{x}{y}\right)^4 + \frac{729}{7} \left(\frac{x}{y}\right)^6 + 729 \left(\frac{x}{y}\right)^8 + \frac{59049}{11} \left(\frac{x}{y}\right)^{10} + \frac{531441}{13} \left(\frac{x}{y}\right)^{12} \right], \\
\frac{\chi_0(7\mathbf{x})}{n\beta} &\simeq -\frac{3}{2}\Theta \int_0^\infty dy f_0(y; \Theta) \left[ 1 + \frac{49}{12} \left(\frac{x}{y}\right)^2 + \frac{2401}{80} \left(\frac{x}{y}\right)^4 + \frac{16807}{64} \left(\frac{x}{y}\right)^6 + \frac{5764801}{2304} \left(\frac{x}{y}\right)^8 + \frac{282475249}{11264} \left(\frac{x}{y}\right)^{10} + \frac{13841287201}{53248} \left(\frac{x}{y}\right)^{12} \right], \\
\frac{\chi_0(8\mathbf{x})}{n\beta} &\simeq -\frac{3}{2}\Theta \int_0^\infty dy f_0(y; \Theta) \left[ 1 + \frac{16}{3} \left(\frac{x}{y}\right)^2 + \frac{256}{5} \left(\frac{x}{y}\right)^4 + \frac{4096}{7} \left(\frac{x}{y}\right)^6 + \frac{65536}{9} \left(\frac{x}{y}\right)^8 + \frac{1048576}{11} \left(\frac{x}{y}\right)^{10} + \frac{16777216}{13} \left(\frac{x}{y}\right)^{12} \right].
\end{aligned}$$

Substituting in the canonical form, ordering in powers of  $1/x^{14}$ ,  $1/x^{12}$ ,  $1/x^{10}$ ,  $1/x^8$ ,  $1/x^6$ ,  $1/x^4$ ,  $1/x^2$ , taking the limit  $x \rightarrow 0$  and equating each coefficient with zero (as demanded by the stability requirement) leads to the  $7 \times 7$  system of equations  $Ma = b$  where the  $7 \times 7$  matrix  $M$  is given by

$$\begin{pmatrix}
\frac{1}{49} & 1 & \frac{1}{25} & \frac{1}{4} & \frac{1}{3} & \frac{1}{4} & \frac{1}{3} \\
\frac{12}{12} & 3 & \frac{12}{12} & \frac{3}{3} & \frac{4}{4} & \frac{1}{3} & \frac{1}{12} \\
\frac{2401}{80} & \frac{81}{5} & \frac{125}{16} & \frac{16}{5} & \frac{81}{80} & \frac{1}{5} & \frac{1}{80} \\
\frac{16807}{64} & \frac{729}{7} & \frac{15625}{448} & \frac{64}{7} & \frac{729}{448} & \frac{1}{7} & \frac{1}{448} \\
\frac{5764801}{2304} & 729 & \frac{390625}{2304} & \frac{256}{9} & \frac{729}{256} & \frac{1}{9} & \frac{1}{2304} \\
\frac{282475249}{11264} & \frac{59049}{11} & \frac{9765625}{11264} & \frac{1024}{11} & \frac{59049}{11264} & \frac{1}{11} & \frac{1}{11264} \\
\frac{13841287201}{53248} & \frac{531441}{13} & \frac{244140625}{53248} & \frac{4096}{13} & \frac{531441}{53248} & \frac{1}{13} & \frac{1}{53248}
\end{pmatrix}$$

the 7-dim source vector  $b$  is given by  $(-8, -128/3, -2048/5, -32768/7, -524288/9, -8388608/11, -134217728/13)$ , the 7-dim unknown vector  $a$  is defined by  $a = (a_7, a_6, a_5, a_4, a_3, a_2, a_1)$ . The solution is  $(a_7, a_6, a_5, a_4, a_3, a_2, a_1) = (-98, 540, -1750, 3640, -4914, 4004, -1430)$ . The unknown coefficients can only be integers, which is a simple way to check for misprints. The canonical form of the normalized octic ideal density response at the eighth harmonic is

$$\begin{aligned}
\frac{\chi_0^{(8,8)}(\mathbf{x}, Z)}{n\beta^8} &= \frac{1}{(8-1)! x^{14}} \Theta^7 \left[ 8 \frac{\chi_0(8\mathbf{x}, 8Z)}{n\beta} - 98 \frac{\chi_0(7\mathbf{x}, 7Z)}{n\beta} + 540 \frac{\chi_0(6\mathbf{x}, 6Z)}{n\beta} - 1750 \frac{\chi_0(5\mathbf{x}, 5Z)}{n\beta} + 3640 \frac{\chi_0(4\mathbf{x}, 4Z)}{n\beta} - 4914 \frac{\chi_0(3\mathbf{x}, 3Z)}{n\beta} \right. \\
&\quad \left. + 4004 \frac{\chi_0(2\mathbf{x}, 2Z)}{n\beta} - 1430 \frac{\chi_0(\mathbf{x}, Z)}{n\beta} \right],
\end{aligned}$$

In order to obtain the long-wavelength limit of the normalized octic static ideal density response at the eighth harmonic, given the automatic cancellations due to the stability requirement, it suffices to consider the eighth term

of the small argument expansion of the Lindhard density response constituents alone. This leads to

$$\begin{aligned}
\frac{\chi_0^{(8,8)}(\mathbf{x})}{n\beta^8} &= \frac{1}{(8-1)!} \frac{\Theta^7}{x^{14}} \left[ 8 \frac{\chi_0(8\mathbf{x})}{n\beta} - 98 \frac{\chi_0(7\mathbf{x})}{n\beta} + 540 \frac{\chi_0(6\mathbf{x})}{n\beta} - 1750 \frac{\chi_0(5\mathbf{x})}{n\beta} + 3640 \frac{\chi_0(4\mathbf{x})}{n\beta} - 4914 \frac{\chi_0(3\mathbf{x})}{n\beta} + 4004 \frac{\chi_0(2\mathbf{x})}{n\beta} - 1430 \frac{\chi_0(\mathbf{x})}{n\beta} \right] \Rightarrow \\
\frac{\chi_0^{(8,8)}(\mathbf{x})}{n\beta^8} &= -\frac{1}{(8-1)!} \frac{\Theta^7}{x^{14}} \left[ 8 \frac{3}{2} \Theta \int_0^\infty dy f_0(y; \Theta) \frac{1}{15} \frac{1}{16384} \left( \frac{8x}{y} \right)^{14} - 98 \frac{3}{2} \Theta \int_0^\infty dy f_0(y; \Theta) \frac{1}{15} \frac{1}{16384} \left( \frac{7x}{y} \right)^{14} \right. \\
&\quad + 540 \frac{3}{2} \Theta \int_0^\infty dy f_0(y; \Theta) \frac{1}{15} \frac{1}{16384} \left( \frac{6x}{y} \right)^{14} - 1750 \frac{3}{2} \Theta \int_0^\infty dy f_0(y; \Theta) \frac{1}{15} \frac{1}{16384} \left( \frac{5x}{y} \right)^{14} \\
&\quad + 3640 \frac{3}{2} \Theta \int_0^\infty dy f_0(y; \Theta) \frac{1}{15} \frac{1}{16384} \left( \frac{4x}{y} \right)^{14} - 4914 \frac{3}{2} \Theta \int_0^\infty dy f_0(y; \Theta) \frac{1}{15} \frac{1}{16384} \left( \frac{3x}{y} \right)^{14} \\
&\quad \left. + 4004 \frac{3}{2} \Theta \int_0^\infty dy f_0(y; \Theta) \frac{1}{15} \frac{1}{16384} \left( \frac{2x}{y} \right)^{14} - 1430 \frac{3}{2} \Theta \int_0^\infty dy f_0(y; \Theta) \frac{1}{15} \frac{1}{16384} \left( \frac{x}{y} \right)^{14} \right] \Rightarrow \\
\frac{\chi_0^{(8,8)}(\mathbf{x})}{n\beta^8} &= -\frac{1}{203212800} \frac{\Theta^7}{x^{14}} \frac{3}{2} \Theta \int_0^\infty dy f_0(y; \Theta) \left[ 8 \frac{1}{15} \frac{1}{16384} \left( \frac{8x}{y} \right)^{14} - 98 \frac{1}{15} \frac{1}{16384} \left( \frac{7x}{y} \right)^{14} + 540 \frac{1}{15} \frac{1}{16384} \left( \frac{6x}{y} \right)^{14} \right. \\
&\quad \left. - 1750 \frac{1}{15} \frac{1}{16384} \left( \frac{5x}{y} \right)^{14} + 3640 \frac{1}{15} \frac{1}{16384} \left( \frac{4x}{y} \right)^{14} - 4914 \frac{1}{15} \frac{1}{16384} \left( \frac{3x}{y} \right)^{14} + 4004 \frac{1}{15} \frac{1}{16384} \left( \frac{2x}{y} \right)^{14} - 1430 \frac{1}{15} \frac{1}{16384} \left( \frac{x}{y} \right)^{14} \right] \Rightarrow \\
\frac{\chi_0^{(8,8)}(\mathbf{x})}{n\beta^8} &= -\frac{1}{203212800} \frac{\Theta^7}{x^{14}} \frac{3}{2} \Theta \int_0^\infty dy f_0(y; \Theta) \left[ \frac{8}{15} \frac{8^{14}}{16384} \left( \frac{x}{y} \right)^{14} - \frac{98}{15} \frac{7^{14}}{16384} \left( \frac{x}{y} \right)^{14} + \frac{540}{15} \frac{6^{14}}{16384} \left( \frac{x}{y} \right)^{14} \right. \\
&\quad \left. - \frac{1750}{15} \frac{5^{14}}{16384} \left( \frac{x}{y} \right)^{14} + \frac{3640}{15} \frac{4^{14}}{16384} \left( \frac{x}{y} \right)^{14} - \frac{4914}{15} \frac{3^{14}}{16384} \left( \frac{x}{y} \right)^{14} + \frac{4004}{15} \frac{2^{14}}{16384} \left( \frac{x}{y} \right)^{14} - \frac{1430}{15} \frac{1}{16384} \left( \frac{x}{y} \right)^{14} \right] \Rightarrow \\
\frac{\chi_0^{(8,8)}(\mathbf{x})}{n\beta^8} &= -\frac{1}{135475200} \frac{\Theta^8}{x^{14}} \int_0^\infty dy f_0(y; \Theta) \left[ \frac{8}{15} \frac{8^{14}}{16384} \left( \frac{x}{y} \right)^{14} - \frac{98}{15} \frac{7^{14}}{16384} \left( \frac{x}{y} \right)^{14} + \frac{540}{15} \frac{6^{14}}{16384} \left( \frac{x}{y} \right)^{14} \right. \\
&\quad \left. - \frac{1750}{15} \frac{5^{14}}{16384} \left( \frac{x}{y} \right)^{14} + \frac{3640}{15} \frac{4^{14}}{16384} \left( \frac{x}{y} \right)^{14} - \frac{4914}{15} \frac{3^{14}}{16384} \left( \frac{x}{y} \right)^{14} + \frac{4004}{15} \frac{2^{14}}{16384} \left( \frac{x}{y} \right)^{14} - \frac{1430}{15} \frac{1}{16384} \left( \frac{x}{y} \right)^{14} \right] \Rightarrow \\
\frac{\chi_0^{(8,8)}(\mathbf{x})}{n\beta^8} &= -\frac{1}{135475200} \frac{\Theta^8}{x^{14}} \int_0^\infty dy f_0(y; \Theta) \left[ \frac{8}{15} \frac{8^{14}}{16384} - \frac{98}{15} \frac{7^{14}}{16384} + \frac{540}{15} \frac{6^{14}}{16384} - \frac{1750}{15} \frac{5^{14}}{16384} + \frac{3640}{15} \frac{4^{14}}{16384} - \frac{4914}{15} \frac{3^{14}}{16384} \right. \\
&\quad \left. + \frac{4004}{15} \frac{2^{14}}{16384} - \frac{1430}{15} \frac{1}{16384} \right] \left( \frac{x}{y} \right)^{14} \Rightarrow \\
\frac{\chi_0^{(8,8)}(\mathbf{x})}{n\beta^8} &= -\frac{1}{135475200} \Theta^8 \int_0^\infty dy f_0(y; \Theta) \left[ \frac{8}{15} \frac{8^{14}}{16384} - \frac{98}{15} \frac{7^{14}}{16384} + \frac{540}{15} \frac{6^{14}}{16384} - \frac{1750}{15} \frac{5^{14}}{16384} + \frac{3640}{15} \frac{4^{14}}{16384} - \frac{4914}{15} \frac{3^{14}}{16384} \right. \\
&\quad \left. + \frac{4004}{15} \frac{2^{14}}{16384} - \frac{1430}{15} \frac{1}{16384} \right] \frac{1}{x^{14}} \left( \frac{x}{y} \right)^{14} \Rightarrow \\
\frac{\chi_0^{(8,8)}(\mathbf{x})}{n\beta^8} &= -\frac{1}{135475200} \Theta^8 \int_0^\infty dy f_0(y; \Theta) \left[ \frac{8}{15} \frac{8^{14}}{16384} - \frac{98}{15} \frac{7^{14}}{16384} + \frac{540}{15} \frac{6^{14}}{16384} - \frac{1750}{15} \frac{5^{14}}{16384} + \frac{3640}{15} \frac{4^{14}}{16384} - \frac{4914}{15} \frac{3^{14}}{16384} \right. \\
&\quad \left. + \frac{4004}{15} \frac{2^{14}}{16384} - \frac{1430}{15} \frac{1}{16384} \right] \frac{1}{x^{14}} \left( \frac{x}{y} \right)^{14} \Rightarrow \\
\frac{\chi_0^{(8,8)}(\mathbf{x})}{n\beta^8} &= -\frac{1}{135475200} \Theta^8 \int_0^\infty dy \frac{f_0(y; \Theta)}{y^{14}} \frac{8^{15} - 98 \times 7^{14} + 540 \times 6^{14} - 1750 \times 5^{14} + 3640 \times 4^{14} - 4914 \times 3^{14} + 4004 \times 2^{14} - 1430}{245760} \Rightarrow \\
\frac{\chi_0^{(8,8)}(\mathbf{x})}{n\beta^8} &= -\frac{1}{135475200} \frac{8^{15} - 98 \times 7^{14} + 540 \times 6^{14} - 1750 \times 5^{14} + 3640 \times 4^{14} - 4914 \times 3^{14} + 4004 \times 2^{14} - 1430}{245760} \Theta^8 \int_0^\infty dy \frac{f_0(y; \Theta)}{y^{14}} \Rightarrow \\
\frac{\chi_0^{(8,8)}(\mathbf{x})}{n\beta^8} &= -\frac{1307674368000}{135475200} \frac{1}{245760} \Theta^8 \int_0^\infty dy \frac{f_0(y; \Theta)}{y^{14}} \Rightarrow \\
\frac{\chi_0^{(8,8)}(\mathbf{x})}{n\beta^8} &= -\frac{1307674368}{33294385152} \Theta^8 \int_0^\infty dy \frac{f_0(y; \Theta)}{y^{14}} \Rightarrow \\
\frac{\chi_0^{(8,8)}(\mathbf{x})}{n\beta^8} &= -\frac{1307674368}{1016064} \frac{1016064}{33294385152} \Theta^8 \int_0^\infty dy \frac{f_0(y; \Theta)}{y^{14}} \Rightarrow \\
\frac{\chi_0^{(8,8)}(\mathbf{x})}{n\beta^8} &= -\frac{1287}{32768} \Theta^8 \int_0^\infty dy \frac{f_0(y; \Theta)}{y^{14}} .
\end{aligned}$$



### D. The ninth-order (nonic) ideal density response

Based on the arbitrary perturbation order methodology that was outlined earlier, the general form of the normalized nonic ideal density response at the ninth harmonic reads as

$$\frac{\chi_0^{(9,9)}(\mathbf{x}, Z)}{n\beta^9} = \frac{1}{(9-1)!} \frac{\Theta^8}{x^{16}} \left[ 9 \frac{\chi_0(9\mathbf{x}, 9Z)}{n\beta} + a_8 \frac{\chi_0(8\mathbf{x}, 8Z)}{n\beta} + a_7 \frac{\chi_0(7\mathbf{x}, 7Z)}{n\beta} + a_6 \frac{\chi_0(6\mathbf{x}, 6Z)}{n\beta} + a_5 \frac{\chi_0(5\mathbf{x}, 5Z)}{n\beta} + a_4 \frac{\chi_0(4\mathbf{x}, 4Z)}{n\beta} \right. \\ \left. + a_3 \frac{\chi_0(3\mathbf{x}, 3Z)}{n\beta} + a_2 \frac{\chi_0(2\mathbf{x}, 2Z)}{n\beta} + a_1 \frac{\chi_0(\mathbf{x}, Z)}{n\beta} \right],$$

The key for the determination of the coefficients  $a_8, a_7, a_6, a_5, a_4, a_3, a_2, a_1$  lies in the behavior of the static density responses,

$$\frac{\chi_0^{(9,9)}(\mathbf{x})}{n\beta^9} = \frac{1}{(9-1)!} \frac{\Theta^8}{x^{16}} \left[ 9 \frac{\chi_0(9\mathbf{x})}{n\beta} + a_8 \frac{\chi_0(8\mathbf{x})}{n\beta} + a_7 \frac{\chi_0(7\mathbf{x})}{n\beta} + a_6 \frac{\chi_0(6\mathbf{x})}{n\beta} + a_5 \frac{\chi_0(5\mathbf{x})}{n\beta} + a_4 \frac{\chi_0(4\mathbf{x})}{n\beta} \right. \\ \left. + a_3 \frac{\chi_0(3\mathbf{x})}{n\beta} + a_2 \frac{\chi_0(2\mathbf{x})}{n\beta} + a_1 \frac{\chi_0(\mathbf{x})}{n\beta} \right],$$

where

$$\frac{\chi_0(\mathbf{x})}{n\beta} = -\frac{3}{2} \frac{\Theta}{x} \int_0^\infty y f_0(y; \Theta) \ln \left| \frac{x+2y}{x-2y} \right| dy, \quad \frac{\chi_0(2\mathbf{x})}{n\beta} = -\frac{3}{2} \frac{\Theta}{2x} \int_0^\infty y f_0(y; \Theta) \ln \left| \frac{2x+2y}{2x-2y} \right| dy, \quad \frac{\chi_0(3\mathbf{x})}{n\beta} = -\frac{3}{2} \frac{\Theta}{3x} \int_0^\infty y f_0(y; \Theta) \ln \left| \frac{3x+2y}{3x-2y} \right| dy, \\ \frac{\chi_0(4\mathbf{x})}{n\beta} = -\frac{3}{2} \frac{\Theta}{4x} \int_0^\infty y f_0(y; \Theta) \ln \left| \frac{4x+2y}{4x-2y} \right| dy, \quad \frac{\chi_0(5\mathbf{x})}{n\beta} = -\frac{3}{2} \frac{\Theta}{5x} \int_0^\infty y f_0(y; \Theta) \ln \left| \frac{5x+2y}{5x-2y} \right| dy, \quad \frac{\chi_0(6\mathbf{x})}{n\beta} = -\frac{3}{2} \frac{\Theta}{6x} \int_0^\infty y f_0(y; \Theta) \ln \left| \frac{6x+2y}{6x-2y} \right| dy, \\ \frac{\chi_0(7\mathbf{x})}{n\beta} = -\frac{3}{2} \frac{\Theta}{7x} \int_0^\infty y f_0(y; \Theta) \ln \left| \frac{7x+2y}{7x-2y} \right| dy, \quad \frac{\chi_0(8\mathbf{x})}{n\beta} = -\frac{3}{2} \frac{\Theta}{8x} \int_0^\infty y f_0(y; \Theta) \ln \left| \frac{8x+2y}{8x-2y} \right| dy, \quad \frac{\chi_0(9\mathbf{x})}{n\beta} = -\frac{3}{2} \frac{\Theta}{9x} \int_0^\infty y f_0(y; \Theta) \ln \left| \frac{9x+2y}{9x-2y} \right| dy.$$

Given the  $x^{-16}$  pre-factor and the Taylor expansion of the even static Lindhard response  $\chi_0(\mathbf{x})/(n\beta)$ , the first eight terms of the Taylor expansion of  $\chi_0^{(9,9)}(\mathbf{x})/(n\beta^9)$  need to cancel out exactly in the long-wavelength limit. Otherwise, the non-interacting UEF would be unstable against constant potential energy perturbations. This constraint yields exactly eight linear equations for the determination of the unknown coefficients  $a_8, a_7, a_6, a_5, a_4, a_3, a_2, a_1$ . Let us compute the first eight terms in the small argument expansion of the Lindhard density response at the first nine harmonics. This reads as

$$\frac{\chi_0(\mathbf{x})}{n\beta} \simeq -\frac{3}{2} \Theta \int_0^\infty dy f_0(y; \Theta) \left[ 1 + \frac{1}{3} \frac{1}{4} \left( \frac{x}{y} \right)^2 + \frac{1}{5} \frac{1}{16} \left( \frac{x}{y} \right)^4 + \frac{1}{7} \frac{1}{64} \left( \frac{x}{y} \right)^6 + \frac{1}{9} \frac{1}{256} \left( \frac{x}{y} \right)^8 + \frac{1}{11} \frac{1}{1024} \left( \frac{x}{y} \right)^{10} + \frac{1}{13} \frac{1}{4096} \left( \frac{x}{y} \right)^{12} + \frac{1}{15} \frac{1}{16384} \left( \frac{x}{y} \right)^{14} \right], \\ \frac{\chi_0(2\mathbf{x})}{n\beta} \simeq -\frac{3}{2} \Theta \int_0^\infty dy f_0(y; \Theta) \left[ 1 + \frac{1}{3} \frac{1}{4} \left( \frac{2x}{y} \right)^2 + \frac{1}{5} \frac{1}{16} \left( \frac{2x}{y} \right)^4 + \frac{1}{7} \frac{1}{64} \left( \frac{2x}{y} \right)^6 + \frac{1}{9} \frac{1}{256} \left( \frac{2x}{y} \right)^8 + \frac{1}{11} \frac{1}{1024} \left( \frac{2x}{y} \right)^{10} + \frac{1}{13} \frac{1}{4096} \left( \frac{2x}{y} \right)^{12} + \frac{1}{15} \frac{1}{16384} \left( \frac{2x}{y} \right)^{14} \right], \\ \frac{\chi_0(3\mathbf{x})}{n\beta} \simeq -\frac{3}{2} \Theta \int_0^\infty dy f_0(y; \Theta) \left[ 1 + \frac{1}{3} \frac{1}{4} \left( \frac{3x}{y} \right)^2 + \frac{1}{5} \frac{1}{16} \left( \frac{3x}{y} \right)^4 + \frac{1}{7} \frac{1}{64} \left( \frac{3x}{y} \right)^6 + \frac{1}{9} \frac{1}{256} \left( \frac{3x}{y} \right)^8 + \frac{1}{11} \frac{1}{1024} \left( \frac{3x}{y} \right)^{10} + \frac{1}{13} \frac{1}{4096} \left( \frac{3x}{y} \right)^{12} + \frac{1}{15} \frac{1}{16384} \left( \frac{3x}{y} \right)^{14} \right], \\ \frac{\chi_0(4\mathbf{x})}{n\beta} \simeq -\frac{3}{2} \Theta \int_0^\infty dy f_0(y; \Theta) \left[ 1 + \frac{1}{3} \frac{1}{4} \left( \frac{4x}{y} \right)^2 + \frac{1}{5} \frac{1}{16} \left( \frac{4x}{y} \right)^4 + \frac{1}{7} \frac{1}{64} \left( \frac{4x}{y} \right)^6 + \frac{1}{9} \frac{1}{256} \left( \frac{4x}{y} \right)^8 + \frac{1}{11} \frac{1}{1024} \left( \frac{4x}{y} \right)^{10} + \frac{1}{13} \frac{1}{4096} \left( \frac{4x}{y} \right)^{12} + \frac{1}{15} \frac{1}{16384} \left( \frac{4x}{y} \right)^{14} \right], \\ \frac{\chi_0(5\mathbf{x})}{n\beta} \simeq -\frac{3}{2} \Theta \int_0^\infty dy f_0(y; \Theta) \left[ 1 + \frac{1}{3} \frac{1}{4} \left( \frac{5x}{y} \right)^2 + \frac{1}{5} \frac{1}{16} \left( \frac{5x}{y} \right)^4 + \frac{1}{7} \frac{1}{64} \left( \frac{5x}{y} \right)^6 + \frac{1}{9} \frac{1}{256} \left( \frac{5x}{y} \right)^8 + \frac{1}{11} \frac{1}{1024} \left( \frac{5x}{y} \right)^{10} + \frac{1}{13} \frac{1}{4096} \left( \frac{5x}{y} \right)^{12} + \frac{1}{15} \frac{1}{16384} \left( \frac{5x}{y} \right)^{14} \right], \\ \frac{\chi_0(6\mathbf{x})}{n\beta} \simeq -\frac{3}{2} \Theta \int_0^\infty dy f_0(y; \Theta) \left[ 1 + \frac{1}{3} \frac{1}{4} \left( \frac{6x}{y} \right)^2 + \frac{1}{5} \frac{1}{16} \left( \frac{6x}{y} \right)^4 + \frac{1}{7} \frac{1}{64} \left( \frac{6x}{y} \right)^6 + \frac{1}{9} \frac{1}{256} \left( \frac{6x}{y} \right)^8 + \frac{1}{11} \frac{1}{1024} \left( \frac{6x}{y} \right)^{10} + \frac{1}{13} \frac{1}{4096} \left( \frac{6x}{y} \right)^{12} + \frac{1}{15} \frac{1}{16384} \left( \frac{6x}{y} \right)^{14} \right], \\ \frac{\chi_0(7\mathbf{x})}{n\beta} \simeq -\frac{3}{2} \Theta \int_0^\infty dy f_0(y; \Theta) \left[ 1 + \frac{1}{3} \frac{1}{4} \left( \frac{7x}{y} \right)^2 + \frac{1}{5} \frac{1}{16} \left( \frac{7x}{y} \right)^4 + \frac{1}{7} \frac{1}{64} \left( \frac{7x}{y} \right)^6 + \frac{1}{9} \frac{1}{256} \left( \frac{7x}{y} \right)^8 + \frac{1}{11} \frac{1}{1024} \left( \frac{7x}{y} \right)^{10} + \frac{1}{13} \frac{1}{4096} \left( \frac{7x}{y} \right)^{12} + \frac{1}{15} \frac{1}{16384} \left( \frac{7x}{y} \right)^{14} \right], \\ \frac{\chi_0(8\mathbf{x})}{n\beta} \simeq -\frac{3}{2} \Theta \int_0^\infty dy f_0(y; \Theta) \left[ 1 + \frac{1}{3} \frac{1}{4} \left( \frac{8x}{y} \right)^2 + \frac{1}{5} \frac{1}{16} \left( \frac{8x}{y} \right)^4 + \frac{1}{7} \frac{1}{64} \left( \frac{8x}{y} \right)^6 + \frac{1}{9} \frac{1}{256} \left( \frac{8x}{y} \right)^8 + \frac{1}{11} \frac{1}{1024} \left( \frac{8x}{y} \right)^{10} + \frac{1}{13} \frac{1}{4096} \left( \frac{8x}{y} \right)^{12} + \frac{1}{15} \frac{1}{16384} \left( \frac{8x}{y} \right)^{14} \right], \\ \frac{\chi_0(9\mathbf{x})}{n\beta} \simeq -\frac{3}{2} \Theta \int_0^\infty dy f_0(y; \Theta) \left[ 1 + \frac{1}{3} \frac{1}{4} \left( \frac{9x}{y} \right)^2 + \frac{1}{5} \frac{1}{16} \left( \frac{9x}{y} \right)^4 + \frac{1}{7} \frac{1}{64} \left( \frac{9x}{y} \right)^6 + \frac{1}{9} \frac{1}{256} \left( \frac{9x}{y} \right)^8 + \frac{1}{11} \frac{1}{1024} \left( \frac{9x}{y} \right)^{10} + \frac{1}{13} \frac{1}{4096} \left( \frac{9x}{y} \right)^{12} + \frac{1}{15} \frac{1}{16384} \left( \frac{9x}{y} \right)^{14} \right], \\ \frac{\chi_0(\mathbf{x})}{n\beta} \simeq -\frac{3}{2} \Theta \int_0^\infty dy f_0(y; \Theta) \left[ 1 + \frac{1}{3} \frac{1}{4} \left( \frac{x}{y} \right)^2 + \frac{1}{5} \frac{1}{16} \left( \frac{x}{y} \right)^4 + \frac{1}{7} \frac{1}{64} \left( \frac{x}{y} \right)^6 + \frac{1}{9} \frac{1}{256} \left( \frac{x}{y} \right)^8 + \frac{1}{11} \frac{1}{1024} \left( \frac{x}{y} \right)^{10} + \frac{1}{13} \frac{1}{4096} \left( \frac{x}{y} \right)^{12} + \frac{1}{15} \frac{1}{16384} \left( \frac{x}{y} \right)^{14} \right], \\ \frac{\chi_0(2\mathbf{x})}{n\beta} \simeq -\frac{3}{2} \Theta \int_0^\infty dy f_0(y; \Theta) \left[ 1 + \frac{1}{3} \frac{2^2}{4} \left( \frac{x}{y} \right)^2 + \frac{1}{5} \frac{2^4}{16} \left( \frac{x}{y} \right)^4 + \frac{1}{7} \frac{2^6}{64} \left( \frac{x}{y} \right)^6 + \frac{1}{9} \frac{2^8}{256} \left( \frac{x}{y} \right)^8 + \frac{1}{11} \frac{2^{10}}{1024} \left( \frac{x}{y} \right)^{10} + \frac{1}{13} \frac{2^{12}}{4096} \left( \frac{x}{y} \right)^{12} + \frac{1}{15} \frac{2^{14}}{16384} \left( \frac{x}{y} \right)^{14} \right], \\ \frac{\chi_0(3\mathbf{x})}{n\beta} \simeq -\frac{3}{2} \Theta \int_0^\infty dy f_0(y; \Theta) \left[ 1 + \frac{1}{3} \frac{3^2}{4} \left( \frac{x}{y} \right)^2 + \frac{1}{5} \frac{3^4}{16} \left( \frac{x}{y} \right)^4 + \frac{1}{7} \frac{3^6}{64} \left( \frac{x}{y} \right)^6 + \frac{1}{9} \frac{3^8}{256} \left( \frac{x}{y} \right)^8 + \frac{1}{11} \frac{3^{10}}{1024} \left( \frac{x}{y} \right)^{10} + \frac{1}{13} \frac{3^{12}}{4096} \left( \frac{x}{y} \right)^{12} + \frac{1}{15} \frac{3^{14}}{16384} \left( \frac{x}{y} \right)^{14} \right], \\ \frac{\chi_0(4\mathbf{x})}{n\beta} \simeq -\frac{3}{2} \Theta \int_0^\infty dy f_0(y; \Theta) \left[ 1 + \frac{1}{3} \frac{4^2}{4} \left( \frac{x}{y} \right)^2 + \frac{1}{5} \frac{4^4}{16} \left( \frac{x}{y} \right)^4 + \frac{1}{7} \frac{4^6}{64} \left( \frac{x}{y} \right)^6 + \frac{1}{9} \frac{4^8}{256} \left( \frac{x}{y} \right)^8 + \frac{1}{11} \frac{4^{10}}{1024} \left( \frac{x}{y} \right)^{10} + \frac{1}{13} \frac{4^{12}}{4096} \left( \frac{x}{y} \right)^{12} + \frac{1}{15} \frac{4^{14}}{16384} \left( \frac{x}{y} \right)^{14} \right],$$

$$\begin{aligned}
\frac{\chi_0(5\mathbf{x})}{n\beta} &\simeq -\frac{3}{2}\Theta \int_0^\infty dy f_0(y; \Theta) \left[ 1 + \frac{1}{3} \frac{5^2}{4} \left(\frac{x}{y}\right)^2 + \frac{1}{5} \frac{5^4}{16} \left(\frac{x}{y}\right)^4 + \frac{1}{7} \frac{5^6}{64} \left(\frac{x}{y}\right)^6 + \frac{1}{9} \frac{5^8}{256} \left(\frac{x}{y}\right)^8 + \frac{1}{11} \frac{5^{10}}{1024} \left(\frac{x}{y}\right)^{10} + \frac{1}{13} \frac{5^{12}}{4096} \left(\frac{x}{y}\right)^{12} + \frac{1}{15} \frac{5^{14}}{16384} \left(\frac{x}{y}\right)^{14} \right], \\
\frac{\chi_0(6\mathbf{x})}{n\beta} &\simeq -\frac{3}{2}\Theta \int_0^\infty dy f_0(y; \Theta) \left[ 1 + \frac{1}{3} \frac{6^2}{4} \left(\frac{x}{y}\right)^2 + \frac{1}{5} \frac{6^4}{16} \left(\frac{x}{y}\right)^4 + \frac{1}{7} \frac{6^6}{64} \left(\frac{x}{y}\right)^6 + \frac{1}{9} \frac{6^8}{256} \left(\frac{x}{y}\right)^8 + \frac{1}{11} \frac{6^{10}}{1024} \left(\frac{x}{y}\right)^{10} + \frac{1}{13} \frac{6^{12}}{4096} \left(\frac{x}{y}\right)^{12} + \frac{1}{15} \frac{6^{14}}{16384} \left(\frac{x}{y}\right)^{14} \right], \\
\frac{\chi_0(7\mathbf{x})}{n\beta} &\simeq -\frac{3}{2}\Theta \int_0^\infty dy f_0(y; \Theta) \left[ 1 + \frac{1}{3} \frac{7^2}{4} \left(\frac{x}{y}\right)^2 + \frac{1}{5} \frac{7^4}{16} \left(\frac{x}{y}\right)^4 + \frac{1}{7} \frac{7^6}{64} \left(\frac{x}{y}\right)^6 + \frac{1}{9} \frac{7^8}{256} \left(\frac{x}{y}\right)^8 + \frac{1}{11} \frac{7^{10}}{1024} \left(\frac{x}{y}\right)^{10} + \frac{1}{13} \frac{7^{12}}{4096} \left(\frac{x}{y}\right)^{12} + \frac{1}{15} \frac{7^{14}}{16384} \left(\frac{x}{y}\right)^{14} \right], \\
\frac{\chi_0(8\mathbf{x})}{n\beta} &\simeq -\frac{3}{2}\Theta \int_0^\infty dy f_0(y; \Theta) \left[ 1 + \frac{1}{3} \frac{8^2}{4} \left(\frac{x}{y}\right)^2 + \frac{1}{5} \frac{8^4}{16} \left(\frac{x}{y}\right)^4 + \frac{1}{7} \frac{8^6}{64} \left(\frac{x}{y}\right)^6 + \frac{1}{9} \frac{8^8}{256} \left(\frac{x}{y}\right)^8 + \frac{1}{11} \frac{8^{10}}{1024} \left(\frac{x}{y}\right)^{10} + \frac{1}{13} \frac{8^{12}}{4096} \left(\frac{x}{y}\right)^{12} + \frac{1}{15} \frac{8^{14}}{16384} \left(\frac{x}{y}\right)^{14} \right], \\
\frac{\chi_0(9\mathbf{x})}{n\beta} &\simeq -\frac{3}{2}\Theta \int_0^\infty dy f_0(y; \Theta) \left[ 1 + \frac{1}{3} \frac{9^2}{4} \left(\frac{x}{y}\right)^2 + \frac{1}{5} \frac{9^4}{16} \left(\frac{x}{y}\right)^4 + \frac{1}{7} \frac{9^6}{64} \left(\frac{x}{y}\right)^6 + \frac{1}{9} \frac{9^8}{256} \left(\frac{x}{y}\right)^8 + \frac{1}{11} \frac{9^{10}}{1024} \left(\frac{x}{y}\right)^{10} + \frac{1}{13} \frac{9^{12}}{4096} \left(\frac{x}{y}\right)^{12} + \frac{1}{15} \frac{9^{14}}{16384} \left(\frac{x}{y}\right)^{14} \right] \Rightarrow \\
\frac{\chi_0(\mathbf{x})}{n\beta} &\simeq -\frac{3}{2}\Theta \int_0^\infty dy f_0(y; \Theta) \left[ 1 + \frac{1}{12} \left(\frac{x}{y}\right)^2 + \frac{1}{80} \left(\frac{x}{y}\right)^4 + \frac{1}{448} \left(\frac{x}{y}\right)^6 + \frac{1}{2304} \left(\frac{x}{y}\right)^8 + \frac{1}{11264} \left(\frac{x}{y}\right)^{10} + \frac{1}{53248} \left(\frac{x}{y}\right)^{12} + \frac{1}{245760} \left(\frac{x}{y}\right)^{14} \right], \\
\frac{\chi_0(2\mathbf{x})}{n\beta} &\simeq -\frac{3}{2}\Theta \int_0^\infty dy f_0(y; \Theta) \left[ 1 + \frac{1}{3} \left(\frac{x}{y}\right)^2 + \frac{1}{5} \left(\frac{x}{y}\right)^4 + \frac{1}{7} \left(\frac{x}{y}\right)^6 + \frac{1}{9} \left(\frac{x}{y}\right)^8 + \frac{1}{11} \left(\frac{x}{y}\right)^{10} + \frac{1}{13} \left(\frac{x}{y}\right)^{12} + \frac{1}{15} \left(\frac{x}{y}\right)^{14} \right], \\
\frac{\chi_0(3\mathbf{x})}{n\beta} &\simeq -\frac{3}{2}\Theta \int_0^\infty dy f_0(y; \Theta) \left[ 1 + \frac{3}{4} \left(\frac{x}{y}\right)^2 + \frac{81}{80} \left(\frac{x}{y}\right)^4 + \frac{729}{448} \left(\frac{x}{y}\right)^6 + \frac{729}{256} \left(\frac{x}{y}\right)^8 + \frac{59049}{11264} \left(\frac{x}{y}\right)^{10} + \frac{531441}{53248} \left(\frac{x}{y}\right)^{12} + \frac{1594323}{81920} \left(\frac{x}{y}\right)^{14} \right], \\
\frac{\chi_0(4\mathbf{x})}{n\beta} &\simeq -\frac{3}{2}\Theta \int_0^\infty dy f_0(y; \Theta) \left[ 1 + \frac{4}{3} \left(\frac{x}{y}\right)^2 + \frac{16}{5} \left(\frac{x}{y}\right)^4 + \frac{64}{7} \left(\frac{x}{y}\right)^6 + \frac{256}{9} \left(\frac{x}{y}\right)^8 + \frac{1024}{11} \left(\frac{x}{y}\right)^{10} + \frac{4096}{13} \left(\frac{x}{y}\right)^{12} + \frac{16384}{15} \left(\frac{x}{y}\right)^{14} \right], \\
\frac{\chi_0(5\mathbf{x})}{n\beta} &\simeq -\frac{3}{2}\Theta \int_0^\infty dy f_0(y; \Theta) \left[ 1 + \frac{25}{12} \left(\frac{x}{y}\right)^2 + \frac{125}{16} \left(\frac{x}{y}\right)^4 + \frac{15625}{448} \left(\frac{x}{y}\right)^6 + \frac{390625}{2304} \left(\frac{x}{y}\right)^8 + \frac{9765625}{11264} \left(\frac{x}{y}\right)^{10} + \frac{244140625}{53248} \left(\frac{x}{y}\right)^{12} + \frac{1220703125}{49152} \left(\frac{x}{y}\right)^{14} \right], \\
\frac{\chi_0(6\mathbf{x})}{n\beta} &\simeq -\frac{3}{2}\Theta \int_0^\infty dy f_0(y; \Theta) \left[ 1 + 3 \left(\frac{x}{y}\right)^2 + \frac{81}{5} \left(\frac{x}{y}\right)^4 + \frac{729}{7} \left(\frac{x}{y}\right)^6 + 729 \left(\frac{x}{y}\right)^8 + \frac{59049}{11} \left(\frac{x}{y}\right)^{10} + \frac{531441}{13} \left(\frac{x}{y}\right)^{12} + \frac{1594323}{5} \left(\frac{x}{y}\right)^{14} \right], \\
\frac{\chi_0(7\mathbf{x})}{n\beta} &\simeq -\frac{3}{2}\Theta \int_0^\infty dy f_0(y; \Theta) \left[ 1 + \frac{49}{12} \left(\frac{x}{y}\right)^2 + \frac{2401}{80} \left(\frac{x}{y}\right)^4 + \frac{16807}{64} \left(\frac{x}{y}\right)^6 + \frac{5764801}{2304} \left(\frac{x}{y}\right)^8 + \frac{282475249}{11264} \left(\frac{x}{y}\right)^{10} + \frac{13841287201}{53248} \left(\frac{x}{y}\right)^{12} + \frac{678223072}{245760} \left(\frac{x}{y}\right)^{14} \right], \\
\frac{\chi_0(8\mathbf{x})}{n\beta} &\simeq -\frac{3}{2}\Theta \int_0^\infty dy f_0(y; \Theta) \left[ 1 + \frac{16}{3} \left(\frac{x}{y}\right)^2 + \frac{256}{5} \left(\frac{x}{y}\right)^4 + \frac{4096}{7} \left(\frac{x}{y}\right)^6 + \frac{65536}{9} \left(\frac{x}{y}\right)^8 + \frac{1048576}{11} \left(\frac{x}{y}\right)^{10} + \frac{16777216}{13} \left(\frac{x}{y}\right)^{12} + \frac{268435456}{15} \left(\frac{x}{y}\right)^{14} \right], \\
\frac{\chi_0(9\mathbf{x})}{n\beta} &\simeq -\frac{3}{2}\Theta \int_0^\infty dy f_0(y; \Theta) \left[ 1 + \frac{27}{4} \left(\frac{x}{y}\right)^2 + \frac{6561}{80} \left(\frac{x}{y}\right)^4 + \frac{531441}{448} \left(\frac{x}{y}\right)^6 + \frac{4782969}{256} \left(\frac{x}{y}\right)^8 + \frac{3486784401}{11264} \left(\frac{x}{y}\right)^{10} + \frac{282429536481}{53248} \left(\frac{x}{y}\right)^{12} + \frac{762559}{81} \left(\frac{x}{y}\right)^{14} \right]
\end{aligned}$$

Substituting in the canonical form, ordering in powers of  $1/x^{16}$ ,  $1/x^{14}$ ,  $1/x^{12}$ ,  $1/x^{10}$ ,  $1/x^8$ ,  $1/x^6$ ,  $1/x^4$ ,  $1/x^2$ , taking the limit  $x \rightarrow 0$  and equating each coefficient with zero (as demanded by the stability requirement) leads to the  $8 \times 8$  system of equations  $Ma = b$  where the  $8 \times 8$  matrix  $M$  is given by

$$\begin{pmatrix}
\frac{1}{16} & \frac{1}{49} & 1 & \frac{1}{25} & \frac{1}{4} & \frac{1}{3} & \frac{1}{1} & \frac{1}{12} \\
\frac{16}{3} & \frac{49}{12} & 3 & \frac{25}{12} & \frac{4}{3} & \frac{3}{4} & \frac{1}{3} & \frac{1}{12} \\
\frac{256}{5} & \frac{2401}{80} & \frac{81}{5} & \frac{125}{16} & \frac{16}{5} & \frac{81}{80} & \frac{1}{5} & \frac{1}{80} \\
\frac{4096}{7} & \frac{16807}{64} & \frac{729}{7} & \frac{15625}{448} & \frac{64}{7} & \frac{729}{448} & \frac{1}{7} & \frac{1}{448} \\
\frac{65536}{9} & \frac{5764801}{2304} & 729 & \frac{390625}{2304} & \frac{256}{9} & \frac{729}{256} & \frac{1}{9} & \frac{1}{2304} \\
\frac{1048576}{11} & \frac{282475249}{11264} & \frac{59049}{11} & \frac{9765625}{11264} & \frac{1024}{11} & \frac{59049}{11264} & \frac{1}{11} & \frac{1}{11264} \\
\frac{16777216}{13} & \frac{13841287201}{53248} & \frac{531441}{13} & \frac{244140625}{53248} & \frac{4096}{13} & \frac{531441}{53248} & \frac{1}{13} & \frac{1}{53248} \\
\frac{268435456}{15} & \frac{678223072849}{245760} & \frac{1594323}{5} & \frac{1220703125}{49152} & \frac{16384}{15} & \frac{1594323}{81920} & \frac{1}{15} & \frac{1}{245760}
\end{pmatrix}$$

the 8-dim vector  $b$  is  $(-9, -243/4, -59049/80, -4782969/448, -43046721/256, -31381059609/11264, -2541865828329/53248, -68630377364883/81920)$ , the 8-dim unknown vector  $a$  is defined by  $a = (a_8, a_7, a_6, a_5, a_4, a_3, a_2, a_1)$ . The solution is  $(a_8, a_7, a_6, a_5, a_4, a_3, a_2, a_1) = (-128, 833, -3264, 8500, -15232, 18564, -14144, 4862)$ . The unknown coefficients can only be integers, a simple way to check for misprints. The canonical form of the normalized nonic ideal density response at the ninth harmonic is

$$\begin{aligned}
\frac{\chi_0^{(9,9)}(\mathbf{x}, Z)}{n\beta^9} &= \frac{1}{(9-1)! x^{16}} \left[ 9 \frac{\chi_0(9\mathbf{x}, 9Z)}{n\beta} - 128 \frac{\chi_0(8\mathbf{x}, 8Z)}{n\beta} + 833 \frac{\chi_0(7\mathbf{x}, 7Z)}{n\beta} - 3264 \frac{\chi_0(6\mathbf{x}, 6Z)}{n\beta} + 8500 \frac{\chi_0(5\mathbf{x}, 5Z)}{n\beta} - 15232 \frac{\chi_0(4\mathbf{x}, 4Z)}{n\beta} \right. \\
&\quad \left. + 18564 \frac{\chi_0(3\mathbf{x}, 3Z)}{n\beta} - 14144 \frac{\chi_0(2\mathbf{x}, 2Z)}{n\beta} + 4862 \frac{\chi_0(\mathbf{x}, Z)}{n\beta} \right],
\end{aligned}$$

In order to obtain the long-wavelength limit of the normalized nonic static ideal density response at the ninth harmonic, given the automatic cancellations due to the stability requirement, it suffices to consider the ninth term of the small

argument expansion of the Lindhard density response constituents alone. This leads to

$$\begin{aligned}
\frac{\chi_0^{(9,9)}(\mathbf{x})}{n\beta^9} &= \frac{1}{(9-1)!9!} \frac{\Theta^8}{x^{16}} \left[ 9 \frac{\chi_0(9\mathbf{x})}{n\beta} - 128 \frac{\chi_0(8\mathbf{x})}{n\beta} + 833 \frac{\chi_0(7\mathbf{x})}{n\beta} - 3264 \frac{\chi_0(6\mathbf{x})}{n\beta} + 8500 \frac{\chi_0(5\mathbf{x})}{n\beta} - 15232 \frac{\chi_0(4\mathbf{x})}{n\beta} \right. \\
&\quad \left. + 18564 \frac{\chi_0(3\mathbf{x})}{n\beta} - 14144 \frac{\chi_0(2\mathbf{x})}{n\beta} + 4862 \frac{\chi_0(\mathbf{x})}{n\beta} \right] \Rightarrow \\
\frac{\chi_0^{(9,9)}(\mathbf{x})}{n\beta^9} &= -\frac{1}{8!9!} \frac{\Theta^8}{x^{16}} \left[ 9 \frac{3}{2} \Theta \int_0^\infty dy f_0(y; \Theta) \frac{1}{17} \frac{1}{65536} \left( \frac{9x}{y} \right)^{16} \right. \\
&\quad - 128 \frac{3}{2} \Theta \int_0^\infty dy f_0(y; \Theta) \frac{1}{17} \frac{1}{65536} \left( \frac{8x}{y} \right)^{16} + 833 \frac{3}{2} \Theta \int_0^\infty dy f_0(y; \Theta) \frac{1}{17} \frac{1}{65536} \left( \frac{7x}{y} \right)^{16} \\
&\quad - 3264 \frac{3}{2} \Theta \int_0^\infty dy f_0(y; \Theta) \frac{1}{17} \frac{1}{65536} \left( \frac{6x}{y} \right)^{16} + 8500 \frac{3}{2} \Theta \int_0^\infty dy f_0(y; \Theta) \frac{1}{17} \frac{1}{65536} \left( \frac{5x}{y} \right)^{16} \\
&\quad - 15232 \frac{3}{2} \Theta \int_0^\infty dy f_0(y; \Theta) \frac{1}{17} \frac{1}{65536} \left( \frac{4x}{y} \right)^{16} + 18564 \frac{3}{2} \Theta \int_0^\infty dy f_0(y; \Theta) \frac{1}{17} \frac{1}{65536} \left( \frac{3x}{y} \right)^{16} \\
&\quad \left. - 14144 \frac{3}{2} \Theta \int_0^\infty dy f_0(y; \Theta) \frac{1}{17} \frac{1}{65536} \left( \frac{2x}{y} \right)^{16} + 4862 \frac{3}{2} \Theta \int_0^\infty dy f_0(y; \Theta) \frac{1}{17} \frac{1}{65536} \left( \frac{x}{y} \right)^{16} \right] \Rightarrow \\
\frac{\chi_0^{(9,9)}(\mathbf{x})}{n\beta^9} &= -\frac{1}{8!9!} \frac{\Theta^8}{x^{16}} \left[ 9 \frac{3}{2} \Theta \int_0^\infty dy f_0(y; \Theta) \frac{1}{17} \frac{9^{16}}{65536} \left( \frac{x}{y} \right)^{16} \right. \\
&\quad - 128 \frac{3}{2} \Theta \int_0^\infty dy f_0(y; \Theta) \frac{1}{17} \frac{8^{16}}{65536} \left( \frac{x}{y} \right)^{16} + 833 \frac{3}{2} \Theta \int_0^\infty dy f_0(y; \Theta) \frac{1}{17} \frac{7^{16}}{65536} \left( \frac{x}{y} \right)^{16} \\
&\quad - 3264 \frac{3}{2} \Theta \int_0^\infty dy f_0(y; \Theta) \frac{1}{17} \frac{6^{16}}{65536} \left( \frac{x}{y} \right)^{16} + 8500 \frac{3}{2} \Theta \int_0^\infty dy f_0(y; \Theta) \frac{1}{17} \frac{5^{16}}{65536} \left( \frac{x}{y} \right)^{16} \\
&\quad - 15232 \frac{3}{2} \Theta \int_0^\infty dy f_0(y; \Theta) \frac{1}{17} \frac{4^{16}}{65536} \left( \frac{x}{y} \right)^{16} + 18564 \frac{3}{2} \Theta \int_0^\infty dy f_0(y; \Theta) \frac{1}{17} \frac{3^{16}}{65536} \left( \frac{x}{y} \right)^{16} \\
&\quad \left. - 14144 \frac{3}{2} \Theta \int_0^\infty dy f_0(y; \Theta) \frac{1}{17} \frac{2^{16}}{65536} \left( \frac{x}{y} \right)^{16} + 4862 \frac{3}{2} \Theta \int_0^\infty dy f_0(y; \Theta) \frac{1}{17} \frac{1}{65536} \left( \frac{x}{y} \right)^{16} \right] \Rightarrow \\
\frac{\chi_0^{(9,9)}(\mathbf{x})}{n\beta^9} &= -\frac{1}{8!9!} \frac{\Theta^8}{x^{16}} \frac{3}{2} \Theta \int_0^\infty dy f_0(y; \Theta) \left[ 9 \frac{1}{17} \frac{9^{16}}{65536} \left( \frac{x}{y} \right)^{16} - 128 \frac{1}{17} \frac{8^{16}}{65536} \left( \frac{x}{y} \right)^{16} + 833 \frac{1}{17} \frac{7^{16}}{65536} \left( \frac{x}{y} \right)^{16} \right. \\
&\quad - 3264 \frac{1}{17} \frac{6^{16}}{65536} \left( \frac{x}{y} \right)^{16} + 8500 \frac{1}{17} \frac{5^{16}}{65536} \left( \frac{x}{y} \right)^{16} - 15232 \frac{1}{17} \frac{4^{16}}{65536} \left( \frac{x}{y} \right)^{16} \\
&\quad \left. + 18564 \frac{1}{17} \frac{3^{16}}{65536} \left( \frac{x}{y} \right)^{16} - 14144 \frac{1}{17} \frac{2^{16}}{65536} \left( \frac{x}{y} \right)^{16} + 4862 \frac{1}{17} \frac{1}{65536} \left( \frac{x}{y} \right)^{16} \right] \Rightarrow \\
\frac{\chi_0^{(9,9)}(\mathbf{x})}{n\beta^9} &= -\frac{1}{8!9!} \frac{\Theta^8}{x^{16}} \frac{3}{2} \Theta \int_0^\infty dy f_0(y; \Theta) \left[ 9 \frac{1}{17} \frac{9^{16}}{65536} - 128 \frac{1}{17} \frac{8^{16}}{65536} + 833 \frac{1}{17} \frac{7^{16}}{65536} - 3264 \frac{1}{17} \frac{6^{16}}{65536} \right. \\
&\quad \left. + 8500 \frac{1}{17} \frac{5^{16}}{65536} - 15232 \frac{1}{17} \frac{4^{16}}{65536} + 18564 \frac{1}{17} \frac{3^{16}}{65536} - 14144 \frac{1}{17} \frac{2^{16}}{65536} + 4862 \frac{1}{17} \frac{1}{65536} \right] \left( \frac{x}{y} \right)^{16} \Rightarrow \\
\frac{\chi_0^{(9,9)}(\mathbf{x})}{n\beta^9} &= -\frac{3}{2} \frac{1}{8!9!} \Theta^9 \int_0^\infty dy \frac{f_0(y; \Theta)}{y^{16}} \left[ \frac{9^{17}}{1114112} - \frac{128 \times 8^{16}}{1114112} + \frac{833 \times 7^{16}}{1114112} - \frac{3264 \times 6^{16}}{1114112} + \frac{8500 \times 5^{16}}{1114112} \right. \\
&\quad \left. - \frac{15232 \times 4^{16}}{1114112} + \frac{18564 \times 3^{16}}{1114112} - \frac{14144 \times 2^{16}}{1114112} + \frac{4862}{1114112} \right] \Rightarrow \\
\frac{\chi_0^{(9,9)}(\mathbf{x})}{n\beta^9} &= -\frac{355687428096000}{1114112} \frac{1}{9754214400} \Theta^9 \int_0^\infty dy \frac{f_0(y; \Theta)}{y^{16}} \Rightarrow \\
\frac{\chi_0^{(9,9)}(\mathbf{x})}{n\beta^9} &= -\frac{355687428096000}{10867287313612800} \Theta^9 \int_0^\infty dy \frac{f_0(y; \Theta)}{y^{16}} \Rightarrow \\
\frac{\chi_0^{(9,9)}(\mathbf{x})}{n\beta^9} &= -\frac{355687428096000}{165821644800} \frac{165821644800}{10867287313612800} \Theta^9 \int_0^\infty dy \frac{f_0(y; \Theta)}{y^{16}} \Rightarrow \\
\frac{\chi_0^{(9,9)}(\mathbf{x})}{n\beta^9} &= -\frac{2145}{65536} \Theta^9 \int_0^\infty dy \frac{f_0(y; \Theta)}{y^{16}}.
\end{aligned}$$

### E. The tenth-order (decic) ideal density response

Based on the arbitrary perturbation order methodology that was outlined earlier, the general form of the normalized decic ideal density response at the tenth harmonic reads as

$$\frac{\chi_0^{(10,10)}(\mathbf{x}, Z)}{n\beta^{10}} = \frac{1}{(10-1)!10!} \frac{\Theta^9}{x^{18}} \left[ 10 \frac{\chi_0(10\mathbf{x}, 10Z)}{n\beta} + a_9 \frac{\chi_0(9\mathbf{x}, 9Z)}{n\beta} + a_8 \frac{\chi_0(8\mathbf{x}, 8Z)}{n\beta} + a_7 \frac{\chi_0(7\mathbf{x}, 7Z)}{n\beta} + a_6 \frac{\chi_0(6\mathbf{x}, 6Z)}{n\beta} + a_5 \frac{\chi_0(5\mathbf{x}, 5Z)}{n\beta} + a_4 \frac{\chi_0(4\mathbf{x}, 4Z)}{n\beta} \right. \\ \left. + a_3 \frac{\chi_0(3\mathbf{x}, 3Z)}{n\beta} + a_2 \frac{\chi_0(2\mathbf{x}, 2Z)}{n\beta} + a_1 \frac{\chi_0(\mathbf{x}, Z)}{n\beta} \right],$$

The key for the determination of the coefficients  $a_9, a_8, a_7, a_6, a_5, a_4, a_3, a_2, a_1$  lies in the behavior of the static density responses,

$$\frac{\chi_0^{(10,10)}(\mathbf{x})}{n\beta^{10}} = \frac{1}{(10-1)!10!} \frac{\Theta^9}{x^{18}} \left[ 10 \frac{\chi_0(10\mathbf{x})}{n\beta} + a_9 \frac{\chi_0(9\mathbf{x})}{n\beta} + a_8 \frac{\chi_0(8\mathbf{x})}{n\beta} + a_7 \frac{\chi_0(7\mathbf{x})}{n\beta} + a_6 \frac{\chi_0(6\mathbf{x})}{n\beta} + a_5 \frac{\chi_0(5\mathbf{x})}{n\beta} + a_4 \frac{\chi_0(4\mathbf{x})}{n\beta} \right. \\ \left. + a_3 \frac{\chi_0(3\mathbf{x})}{n\beta} + a_2 \frac{\chi_0(2\mathbf{x})}{n\beta} + a_1 \frac{\chi_0(\mathbf{x})}{n\beta} \right],$$

where

$$\begin{aligned} \frac{\chi_0(\mathbf{x})}{n\beta} &= -\frac{3}{2} \frac{\Theta}{x} \int_0^\infty y f_0(y; \Theta) \ln \left| \frac{x+2y}{x-2y} \right| dy, & \frac{\chi_0(2\mathbf{x})}{n\beta} &= -\frac{3}{2} \frac{\Theta}{2x} \int_0^\infty y f_0(y; \Theta) \ln \left| \frac{2x+2y}{2x-2y} \right| dy, \\ \frac{\chi_0(3\mathbf{x})}{n\beta} &= -\frac{3}{2} \frac{\Theta}{3x} \int_0^\infty y f_0(y; \Theta) \ln \left| \frac{3x+2y}{3x-2y} \right| dy, & \frac{\chi_0(4\mathbf{x})}{n\beta} &= -\frac{3}{2} \frac{\Theta}{4x} \int_0^\infty y f_0(y; \Theta) \ln \left| \frac{4x+2y}{4x-2y} \right| dy, \\ \frac{\chi_0(5\mathbf{x})}{n\beta} &= -\frac{3}{2} \frac{\Theta}{5x} \int_0^\infty y f_0(y; \Theta) \ln \left| \frac{5x+2y}{5x-2y} \right| dy, & \frac{\chi_0(6\mathbf{x})}{n\beta} &= -\frac{3}{2} \frac{\Theta}{6x} \int_0^\infty y f_0(y; \Theta) \ln \left| \frac{6x+2y}{6x-2y} \right| dy, \\ \frac{\chi_0(7\mathbf{x})}{n\beta} &= -\frac{3}{2} \frac{\Theta}{7x} \int_0^\infty y f_0(y; \Theta) \ln \left| \frac{7x+2y}{7x-2y} \right| dy, & \frac{\chi_0(8\mathbf{x})}{n\beta} &= -\frac{3}{2} \frac{\Theta}{8x} \int_0^\infty y f_0(y; \Theta) \ln \left| \frac{8x+2y}{8x-2y} \right| dy, \\ \frac{\chi_0(9\mathbf{x})}{n\beta} &= -\frac{3}{2} \frac{\Theta}{9x} \int_0^\infty y f_0(y; \Theta) \ln \left| \frac{9x+2y}{9x-2y} \right| dy, & \frac{\chi_0(10\mathbf{x})}{n\beta} &= -\frac{3}{2} \frac{\Theta}{10x} \int_0^\infty y f_0(y; \Theta) \ln \left| \frac{10x+2y}{10x-2y} \right| dy. \end{aligned}$$

Given the  $x^{-18}$  pre-factor and the Taylor expansion of the even static Lindhard response  $\chi_0(\mathbf{x})/(n\beta)$ , the first nine terms of the Taylor expansion of  $\chi_0^{(10,10)}(\mathbf{x})/(n\beta^{10})$  need to cancel out exactly in the long-wavelength limit. Otherwise, the non-interacting UEF would be unstable against constant potential energy perturbations. This constraint yields exactly nine linear equations for the determination of the unknown coefficients  $a_9, a_8, a_7, a_6, a_5, a_4, a_3, a_2, a_1$ . Let us compute the first nine terms in the small argument expansion of the Lindhard density response at the first ten harmonics. This reads as



$$\begin{aligned}
\frac{\chi_0(\mathbf{x})}{n\beta} &\simeq -\frac{3}{2}\Theta \int_0^\infty dy f_0(y; \Theta) \left[ 1 + \frac{1}{12} \left(\frac{x}{y}\right)^2 + \frac{1}{80} \left(\frac{x}{y}\right)^4 + \frac{1}{448} \left(\frac{x}{y}\right)^6 + \frac{1}{2304} \left(\frac{x}{y}\right)^8 + \frac{1}{11264} \left(\frac{x}{y}\right)^{10} + \frac{1}{53248} \left(\frac{x}{y}\right)^{12} + \frac{1}{245760} \left(\frac{x}{y}\right)^{14} + \frac{1}{1114112} \left(\frac{x}{y}\right)^{16} \right], \\
\frac{\chi_0(2\mathbf{x})}{n\beta} &\simeq -\frac{3}{2}\Theta \int_0^\infty dy f_0(y; \Theta) \left[ 1 + \frac{1}{3} \left(\frac{x}{y}\right)^2 + \frac{1}{5} \left(\frac{x}{y}\right)^4 + \frac{1}{7} \left(\frac{x}{y}\right)^6 + \frac{1}{9} \left(\frac{x}{y}\right)^8 + \frac{1}{11} \left(\frac{x}{y}\right)^{10} + \frac{1}{13} \left(\frac{x}{y}\right)^{12} + \frac{1}{15} \left(\frac{x}{y}\right)^{14} + \frac{1}{17} \left(\frac{x}{y}\right)^{16} \right], \\
\frac{\chi_0(3\mathbf{x})}{n\beta} &\simeq -\frac{3}{2}\Theta \int_0^\infty dy f_0(y; \Theta) \left[ 1 + \frac{2}{3} \left(\frac{x}{y}\right)^2 + \frac{81}{80} \left(\frac{x}{y}\right)^4 + \frac{729}{448} \left(\frac{x}{y}\right)^6 + \frac{729}{256} \left(\frac{x}{y}\right)^8 + \frac{59049}{11264} \left(\frac{x}{y}\right)^{10} + \frac{531441}{53248} \left(\frac{x}{y}\right)^{12} + \frac{1594323}{81920} \left(\frac{x}{y}\right)^{14} + \frac{43046721}{1114112} \left(\frac{x}{y}\right)^{16} \right], \\
\frac{\chi_0(4\mathbf{x})}{n\beta} &\simeq -\frac{3}{2}\Theta \int_0^\infty dy f_0(y; \Theta) \left[ 1 + \frac{4}{3} \left(\frac{x}{y}\right)^2 + \frac{16}{5} \left(\frac{x}{y}\right)^4 + \frac{64}{7} \left(\frac{x}{y}\right)^6 + \frac{256}{9} \left(\frac{x}{y}\right)^8 + \frac{1024}{11} \left(\frac{x}{y}\right)^{10} + \frac{4096}{13} \left(\frac{x}{y}\right)^{12} + \frac{16384}{15} \left(\frac{x}{y}\right)^{14} + \frac{65536}{17} \left(\frac{x}{y}\right)^{16} \right], \\
\frac{\chi_0(5\mathbf{x})}{n\beta} &\simeq -\frac{3}{2}\Theta \int_0^\infty dy f_0(y; \Theta) \left[ 1 + \frac{25}{12} \left(\frac{x}{y}\right)^2 + \frac{125}{16} \left(\frac{x}{y}\right)^4 + \frac{15625}{448} \left(\frac{x}{y}\right)^6 + \frac{390625}{2304} \left(\frac{x}{y}\right)^8 + \frac{9765625}{11264} \left(\frac{x}{y}\right)^{10} + \frac{244140625}{53248} \left(\frac{x}{y}\right)^{12} + \frac{1220703125}{49152} \left(\frac{x}{y}\right)^{14} + \frac{152587890625}{1114112} \left(\frac{x}{y}\right)^{16} \right], \\
\frac{\chi_0(6\mathbf{x})}{n\beta} &\simeq -\frac{3}{2}\Theta \int_0^\infty dy f_0(y; \Theta) \left[ 1 + 3 \left(\frac{x}{y}\right)^2 + \frac{81}{5} \left(\frac{x}{y}\right)^4 + \frac{729}{7} \left(\frac{x}{y}\right)^6 + \frac{729}{11} \left(\frac{x}{y}\right)^8 + \frac{59049}{13} \left(\frac{x}{y}\right)^{10} + \frac{531441}{15} \left(\frac{x}{y}\right)^{12} + \frac{1594323}{17} \left(\frac{x}{y}\right)^{14} + \frac{43046721}{17} \left(\frac{x}{y}\right)^{16} \right], \\
\frac{\chi_0(7\mathbf{x})}{n\beta} &\simeq -\frac{3}{2}\Theta \int_0^\infty dy f_0(y; \Theta) \left[ 1 + \frac{49}{12} \left(\frac{x}{y}\right)^2 + \frac{2401}{80} \left(\frac{x}{y}\right)^4 + \frac{16807}{64} \left(\frac{x}{y}\right)^6 + \frac{5764801}{2304} \left(\frac{x}{y}\right)^8 + \frac{282475249}{11264} \left(\frac{x}{y}\right)^{10} + \frac{13841287201}{53248} \left(\frac{x}{y}\right)^{12} + \frac{678223072849}{245760} \left(\frac{x}{y}\right)^{14} + \frac{33232930569601}{1114112} \left(\frac{x}{y}\right)^{16} \right], \\
\frac{\chi_0(8\mathbf{x})}{n\beta} &\simeq -\frac{3}{2}\Theta \int_0^\infty dy f_0(y; \Theta) \left[ 1 + \frac{16}{3} \left(\frac{x}{y}\right)^2 + \frac{256}{5} \left(\frac{x}{y}\right)^4 + \frac{4096}{7} \left(\frac{x}{y}\right)^6 + \frac{65536}{9} \left(\frac{x}{y}\right)^8 + \frac{1048576}{11} \left(\frac{x}{y}\right)^{10} + \frac{16777216}{13} \left(\frac{x}{y}\right)^{12} + \frac{268435456}{15} \left(\frac{x}{y}\right)^{14} + \frac{4294967296}{17} \left(\frac{x}{y}\right)^{16} \right], \\
\frac{\chi_0(9\mathbf{x})}{n\beta} &\simeq -\frac{3}{2}\Theta \int_0^\infty dy f_0(y; \Theta) \left[ 1 + \frac{27}{4} \left(\frac{x}{y}\right)^2 + \frac{6561}{80} \left(\frac{x}{y}\right)^4 + \frac{531441}{448} \left(\frac{x}{y}\right)^6 + \frac{4782969}{256} \left(\frac{x}{y}\right)^8 + \frac{3486784401}{11264} \left(\frac{x}{y}\right)^{10} + \frac{282429536481}{53248} \left(\frac{x}{y}\right)^{12} + \frac{7625597484987}{81920} \left(\frac{x}{y}\right)^{14} + \frac{1853020188851841}{1114112} \left(\frac{x}{y}\right)^{16} \right], \\
\frac{\chi_0(10\mathbf{x})}{n\beta} &\simeq -\frac{3}{2}\Theta \int_0^\infty dy f_0(y; \Theta) \left[ 1 + \frac{25}{3} \left(\frac{x}{y}\right)^2 + \frac{125}{3} \left(\frac{x}{y}\right)^4 + \frac{15625}{7} \left(\frac{x}{y}\right)^6 + \frac{390625}{9} \left(\frac{x}{y}\right)^8 + \frac{9765625}{11} \left(\frac{x}{y}\right)^{10} + \frac{244140625}{13} \left(\frac{x}{y}\right)^{12} + \frac{1220703125}{3} \left(\frac{x}{y}\right)^{14} + \frac{152587890625}{17} \left(\frac{x}{y}\right)^{16} \right] \Rightarrow
\end{aligned}$$

Substituting in the canonical form, ordering in powers of  $1/x^{18}, 1/x^{16}, 1/x^{14}, 1/x^{12}, 1/x^{10}, 1/x^8, 1/x^6, 1/x^4, 1/x^2$ , taking the limit  $x \rightarrow 0$  and equating each coefficient with zero (as demanded by the stability requirement) leads to the  $9 \times 9$  system of equations  $Ma = b$  where the  $9 \times 9$  matrix  $M$  is given by

$$\begin{pmatrix}
1 & 1 & 1 & 1 & 1 & 1 & 1 & 1 & 1 \\
27 & 16 & 49 & 25 & 4 & 3 & 1 & 1 & 1 \\
4 & 3 & 12 & 12 & 3 & 4 & 3 & 12 & 12 \\
6561 & 256 & 2401 & 81 & 125 & 16 & 81 & 1 & 1 \\
80 & 5 & 80 & 5 & 16 & 5 & 80 & 5 & 80 \\
531441 & 4096 & 16807 & 729 & 15625 & 64 & 729 & 1 & 1 \\
448 & 7 & 64 & 7 & 448 & 7 & 448 & 7 & 448 \\
4782969 & 65536 & 5764801 & 729 & 390625 & 256 & 729 & 1 & 1 \\
256 & 9 & 2304 & 2304 & 2304 & 9 & 256 & 9 & 2304 \\
3486784401 & 1048576 & 282475249 & 59049 & 9765625 & 1024 & 59049 & 1 & 1 \\
11264 & 11 & 11264 & 11 & 11264 & 11 & 11264 & 11 & 11264 \\
282429536481 & 16777216 & 13841287201 & 531441 & 244140625 & 4096 & 531441 & 1 & 1 \\
53248 & 13 & 53248 & 13 & 53248 & 13 & 53248 & 13 & 53248 \\
7625597484987 & 268435456 & 678223072849 & 1594323 & 1220703125 & 16384 & 1594323 & 1 & 1 \\
81920 & 15 & 245760 & 5 & 49152 & 15 & 81920 & 15 & 245760 \\
1853020188851841 & 4294967296 & 33232930569601 & 43046721 & 152587890625 & 65536 & 43046721 & 1 & 1 \\
1114112 & 17 & 1114112 & 17 & 1114112 & 17 & 1114112 & 17 & 1114112
\end{pmatrix}$$

the 9-dim vector  $b$  is given by  $(-10, -250/3, -1250, -156250/7, -3906250/9, -97656250/11, -2441406250/13, -12207031250/3, -1525878906250/17)$ , whereas the 9-dim unknown vector  $a$  is naturally defined by  $a = (a_9, a_8, a_7, a_6, a_5, a_4, a_3, a_2, a_1)$ . The solution is given by  $(a_9, a_8, a_7, a_6, a_5, a_4, a_3, a_2, a_1) = (-162, 1216, -5586, 17442, -38760, 62016, -69768, 50388, -16796)$ . The unknown coefficients can only be integers, which constitutes a straightforward way to check for misprints. The canonical form of the normalized decic ideal density response at the tenth harmonic is

$$\frac{\chi_0^{(10,10)}(\mathbf{x}, Z)}{n\beta^{10}} = \frac{1}{(10-1)!10!} \frac{\Theta^9}{x^{18}} \left[ 10 \frac{\chi_0(10\mathbf{x}, 10Z)}{n\beta} - 162 \frac{\chi_0(9\mathbf{x}, 9Z)}{n\beta} + 1216 \frac{\chi_0(8\mathbf{x}, 8Z)}{n\beta} - 5586 \frac{\chi_0(7\mathbf{x}, 7Z)}{n\beta} + 17442 \frac{\chi_0(6\mathbf{x}, 6Z)}{n\beta} - 38760 \frac{\chi_0(5\mathbf{x}, 5Z)}{n\beta} + 62016 \frac{\chi_0(4\mathbf{x}, 4Z)}{n\beta} - 69768 \frac{\chi_0(3\mathbf{x}, 3Z)}{n\beta} + 50388 \frac{\chi_0(2\mathbf{x}, 2Z)}{n\beta} - 16796 \frac{\chi_0(\mathbf{x}, Z)}{n\beta} \right],$$

In order to obtain the long-wavelength limit of the normalized decic static ideal density response at the tenth harmonic, given the automatic cancellations due to the stability requirement, it suffices to consider the tenth term of the small argument expansion of the Lindhard density response constituents alone. This leads to

$$\begin{aligned} \frac{\chi_0^{(10,10)}(\mathbf{x})}{n\beta^{10}} &= \frac{1}{(10-1)!10!} \frac{\Theta^9}{x^{18}} \left[ 10 \frac{\chi_0(10\mathbf{x})}{n\beta} - 162 \frac{\chi_0(9\mathbf{x})}{n\beta} + 1216 \frac{\chi_0(8\mathbf{x})}{n\beta} - 5586 \frac{\chi_0(7\mathbf{x})}{n\beta} + 17442 \frac{\chi_0(6\mathbf{x})}{n\beta} - 38760 \frac{\chi_0(5\mathbf{x})}{n\beta} + 62016 \frac{\chi_0(4\mathbf{x})}{n\beta} - 69768 \frac{\chi_0(3\mathbf{x})}{n\beta} + 50388 \frac{\chi_0(2\mathbf{x})}{n\beta} - 16796 \frac{\chi_0(\mathbf{x})}{n\beta} \right] \Rightarrow \\ \frac{\chi_0^{(10,10)}(\mathbf{x})}{n\beta^{10}} &= -\frac{1}{(9)!10!} \frac{\Theta^9}{x^{18}} \left\{ 10 \frac{3}{2} \Theta \int_0^\infty dy f_0(y; \Theta) \frac{1}{19} \frac{1}{262144} \left( \frac{10x}{y} \right)^{18} - 162 \frac{3}{2} \Theta \int_0^\infty dy f_0(y; \Theta) \frac{1}{19} \frac{1}{262144} \left( \frac{9x}{y} \right)^{18} + 1216 \frac{3}{2} \Theta \int_0^\infty dy f_0(y; \Theta) \frac{1}{19} \frac{1}{262144} \left( \frac{8x}{y} \right)^{18} \right. \\ &\quad - 5586 \frac{3}{2} \Theta \int_0^\infty dy f_0(y; \Theta) \frac{1}{19} \frac{1}{262144} \left( \frac{7x}{y} \right)^{18} + 17442 \frac{3}{2} \Theta \int_0^\infty dy f_0(y; \Theta) \frac{1}{19} \frac{1}{262144} \left( \frac{6x}{y} \right)^{18} - 38760 \frac{3}{2} \Theta \int_0^\infty dy f_0(y; \Theta) \frac{1}{19} \frac{1}{262144} \left( \frac{5x}{y} \right)^{18} \\ &\quad + 62016 \frac{3}{2} \Theta \int_0^\infty dy f_0(y; \Theta) \frac{1}{19} \frac{1}{262144} \left( \frac{4x}{y} \right)^{18} - 69768 \frac{3}{2} \Theta \int_0^\infty dy f_0(y; \Theta) \frac{1}{19} \frac{1}{262144} \left( \frac{3x}{y} \right)^{18} + 50388 \frac{3}{2} \Theta \int_0^\infty dy f_0(y; \Theta) \frac{1}{19} \frac{1}{262144} \left( \frac{2x}{y} \right)^{18} \\ &\quad \left. - 16796 \frac{3}{2} \Theta \int_0^\infty dy f_0(y; \Theta) \frac{1}{19} \frac{1}{262144} \left( \frac{x}{y} \right)^{18} \right\} \Rightarrow \end{aligned}$$

$$\begin{aligned} \frac{\chi_0^{(10,10)}(\mathbf{x})}{n\beta^{10}} &= -\frac{1}{(9)!10!} \frac{\Theta^9}{x^{18}} \left\{ 10 \frac{3}{2} \Theta \int_0^\infty dy f_0(y; \Theta) \frac{1}{19} \frac{10^{18}}{262144} \left( \frac{x}{y} \right)^{18} - 162 \frac{3}{2} \Theta \int_0^\infty dy f_0(y; \Theta) \frac{1}{19} \frac{9^{18}}{262144} \left( \frac{x}{y} \right)^{18} + 1216 \frac{3}{2} \Theta \int_0^\infty dy f_0(y; \Theta) \frac{1}{19} \frac{8^{18}}{262144} \left( \frac{x}{y} \right)^{18} \right. \\ &\quad - 5586 \frac{3}{2} \Theta \int_0^\infty dy f_0(y; \Theta) \frac{1}{19} \frac{7^{18}}{262144} \left( \frac{x}{y} \right)^{18} + 17442 \frac{3}{2} \Theta \int_0^\infty dy f_0(y; \Theta) \frac{1}{19} \frac{6^{18}}{262144} \left( \frac{x}{y} \right)^{18} - 38760 \frac{3}{2} \Theta \int_0^\infty dy f_0(y; \Theta) \frac{1}{19} \frac{5^{18}}{262144} \left( \frac{x}{y} \right)^{18} \\ &\quad + 62016 \frac{3}{2} \Theta \int_0^\infty dy f_0(y; \Theta) \frac{1}{19} \frac{4^{18}}{262144} \left( \frac{x}{y} \right)^{18} - 69768 \frac{3}{2} \Theta \int_0^\infty dy f_0(y; \Theta) \frac{1}{19} \frac{3^{18}}{262144} \left( \frac{x}{y} \right)^{18} + 50388 \frac{3}{2} \Theta \int_0^\infty dy f_0(y; \Theta) \frac{1}{19} \frac{2^{18}}{262144} \left( \frac{x}{y} \right)^{18} \\ &\quad \left. - 16796 \frac{3}{2} \Theta \int_0^\infty dy f_0(y; \Theta) \frac{1}{19} \frac{1}{262144} \left( \frac{x}{y} \right)^{18} \right\} \Rightarrow \end{aligned}$$

$$\begin{aligned} \frac{\chi_0^{(10,10)}(\mathbf{x})}{n\beta^{10}} &= -\frac{1}{(9)!10!} \frac{\Theta^9}{x^{18}} \frac{3}{2} \Theta \int_0^\infty dy f_0(y; \Theta) \left\{ 10 \frac{1}{19} \frac{10^{18}}{262144} \left( \frac{x}{y} \right)^{18} - 162 \frac{1}{19} \frac{9^{18}}{262144} \left( \frac{x}{y} \right)^{18} + 1216 \frac{1}{19} \frac{8^{18}}{262144} \left( \frac{x}{y} \right)^{18} - 5586 \frac{1}{19} \frac{7^{18}}{262144} \left( \frac{x}{y} \right)^{18} + 17442 \frac{1}{19} \frac{6^{18}}{262144} \left( \frac{x}{y} \right)^{18} \right. \\ &\quad \left. - 38760 \frac{1}{19} \frac{5^{18}}{262144} \left( \frac{x}{y} \right)^{18} + 62016 \frac{1}{19} \frac{4^{18}}{262144} \left( \frac{x}{y} \right)^{18} - 69768 \frac{1}{19} \frac{3^{18}}{262144} \left( \frac{x}{y} \right)^{18} + 50388 \frac{1}{19} \frac{2^{18}}{262144} \left( \frac{x}{y} \right)^{18} - 16796 \frac{1}{19} \frac{1}{262144} \left( \frac{x}{y} \right)^{18} \right\} \Rightarrow \end{aligned}$$

$$\begin{aligned}
\frac{\chi_0^{(10,10)}(x)}{n\beta^{10}} &= -\frac{3}{2} \frac{1}{(9)!10!} \frac{\Theta^{10}}{x^{18}} \int_0^\infty dy f_0(y; \Theta) \left\{ 10 \frac{1}{19} \frac{10^{18}}{262144} \left(\frac{x}{y}\right)^{18} - 162 \frac{1}{19} \frac{9^{18}}{262144} \left(\frac{x}{y}\right)^{18} + 1216 \frac{1}{19} \frac{8^{18}}{262144} \left(\frac{x}{y}\right)^{18} - 5586 \frac{1}{19} \frac{7^{18}}{262144} \left(\frac{x}{y}\right)^{18} + 17442 \frac{1}{19} \frac{6^{18}}{262144} \left(\frac{x}{y}\right)^{18} - 38760 \frac{1}{19} \frac{5^{18}}{262144} \left(\frac{x}{y}\right)^{18} + 62016 \frac{1}{19} \frac{4^{18}}{262144} \left(\frac{x}{y}\right)^{18} - 69768 \frac{1}{19} \frac{3^{18}}{262144} \left(\frac{x}{y}\right)^{18} - 16796 \frac{1}{19} \frac{2^{18}}{262144} \left(\frac{x}{y}\right)^{18} - 16796 \frac{1}{19} \frac{1^{18}}{262144} \left(\frac{x}{y}\right)^{18} \right\} \Rightarrow \\
\frac{\chi_0^{(10,10)}(x)}{n\beta^{10}} &= -\frac{3}{2} \frac{1}{(9)!10!} \frac{\Theta^{10}}{x^{18}} \int_0^\infty dy f_0(y; \Theta) \left\{ 10 \frac{10^{18}}{19 \cdot 262144} - \frac{162 \cdot 9^{18}}{19 \cdot 262144} + \frac{1216 \cdot 8^{18}}{19 \cdot 262144} - \frac{5586 \cdot 7^{18}}{19 \cdot 262144} + \frac{17442 \cdot 6^{18}}{19 \cdot 262144} - \frac{38760 \cdot 5^{18}}{19 \cdot 262144} + \frac{62016 \cdot 4^{18}}{19 \cdot 262144} - \frac{69768 \cdot 3^{18}}{19 \cdot 262144} - \frac{16796 \cdot 2^{18}}{19 \cdot 262144} - \frac{16796 \cdot 1^{18}}{19 \cdot 262144} \right\} \Rightarrow \\
\frac{\chi_0^{(10,10)}(x)}{n\beta^{10}} &= -\frac{3}{2} \frac{1}{(9)!10!} \Theta^{10} \int_0^\infty dy f_0(y; \Theta) \left\{ 10 \frac{10^{18}}{19 \cdot 262144} - \frac{162 \cdot 9^{18}}{19 \cdot 262144} + \frac{1216 \cdot 8^{18}}{19 \cdot 262144} - \frac{5586 \cdot 7^{18}}{19 \cdot 262144} + \frac{17442 \cdot 6^{18}}{19 \cdot 262144} - \frac{38760 \cdot 5^{18}}{19 \cdot 262144} + \frac{62016 \cdot 4^{18}}{19 \cdot 262144} - \frac{69768 \cdot 3^{18}}{19 \cdot 262144} - \frac{16796 \cdot 2^{18}}{19 \cdot 262144} - \frac{16796 \cdot 1^{18}}{19 \cdot 262144} \right\} \Rightarrow \\
\frac{\chi_0^{(10,10)}(x)}{n\beta^{10}} &= -\frac{3}{2} \frac{1}{(9)!10!} \Theta^{10} \int_0^\infty dy f_0(y; \Theta) \left\{ 10 \frac{10^{18}}{19 \cdot 262144} - \frac{162 \cdot 9^{18}}{19 \cdot 262144} + \frac{1216 \cdot 8^{18}}{19 \cdot 262144} - \frac{5586 \cdot 7^{18}}{19 \cdot 262144} + \frac{17442 \cdot 6^{18}}{19 \cdot 262144} - \frac{38760 \cdot 5^{18}}{19 \cdot 262144} + \frac{62016 \cdot 4^{18}}{19 \cdot 262144} - \frac{69768 \cdot 3^{18}}{19 \cdot 262144} - \frac{16796 \cdot 2^{18}}{19 \cdot 262144} - \frac{16796 \cdot 1^{18}}{19 \cdot 262144} \right\} \Rightarrow \\
\frac{\chi_0^{(10,10)}(x)}{n\beta^{10}} &= -\frac{3}{2} \frac{1}{(9)!10!} \Theta^{10} \int_0^\infty dy \frac{f_0(y; \Theta)}{y^{18}} \left\{ 10 \frac{10^{18}}{19 \cdot 262144} - \frac{162 \cdot 9^{18}}{19 \cdot 262144} + \frac{1216 \cdot 8^{18}}{19 \cdot 262144} - \frac{5586 \cdot 7^{18}}{19 \cdot 262144} + \frac{17442 \cdot 6^{18}}{19 \cdot 262144} - \frac{38760 \cdot 5^{18}}{19 \cdot 262144} + \frac{62016 \cdot 4^{18}}{19 \cdot 262144} - \frac{69768 \cdot 3^{18}}{19 \cdot 262144} - \frac{16796 \cdot 2^{18}}{19 \cdot 262144} - \frac{16796 \cdot 1^{18}}{19 \cdot 262144} \right\} \Rightarrow \\
\frac{\chi_0^{(10,10)}(x)}{n\beta^{10}} &= -\frac{3}{2} \frac{1}{(9)!10!} \Theta^{10} \int_0^\infty dy \frac{f_0(y; \Theta)}{y^{18}} \left\{ 10^{19} - 162 \times 9^{18} + 1216 \times 8^{18} - 5586 \times 7^{18} + 17442 \times 6^{18} - 38760 \times 5^{18} + 62016 \times 4^{18} - 69768 \times 3^{18} + 50388 \times 2^{18} - 16796 \right\} \Rightarrow \\
\frac{\chi_0^{(10,10)}(x)}{n\beta^{10}} &= -\frac{3}{2} \frac{1}{(9)!10!} \Theta^{10} \left\{ 10^{19} - 162 \times 9^{18} + 1216 \times 8^{18} - 5586 \times 7^{18} + 17442 \times 6^{18} - 38760 \times 5^{18} + 62016 \times 4^{18} - 69768 \times 3^{18} + 50388 \times 2^{18} - 16796 \right\} \frac{1}{4980736} \int_0^\infty dy \frac{f_0(y; \Theta)}{y^{18}} \Rightarrow \\
\frac{\chi_0^{(10,10)}(x)}{n\beta^{10}} &= -\frac{3}{2} \frac{121645100408832000}{1316818944000} \frac{1}{4980736} \Theta^{10} \int_0^\infty dy \frac{f_0(y; \Theta)}{y^{18}} \Rightarrow \\
\frac{\chi_0^{(10,10)}(x)}{n\beta^{10}} &= -\frac{121645100408832}{877879296} \frac{1}{4980736} \Theta^{10} \int_0^\infty dy \frac{f_0(y; \Theta)}{y^{18}} \Rightarrow \\
\frac{\chi_0^{(10,10)}(x)}{n\beta^{10}} &= -\frac{121645100408832}{4372485013241856} \Theta^{10} \int_0^\infty dy \frac{f_0(y; \Theta)}{y^{18}} \Rightarrow \\
\frac{\chi_0^{(10,10)}(x)}{n\beta^{10}} &= -\frac{121645100408832}{4372485013241856} \Theta^{10} \int_0^\infty dy \frac{f_0(y; \Theta)}{y^{18}} \Rightarrow \\
\frac{\chi_0^{(10,10)}(x)}{n\beta^{10}} &= -\frac{121645100408832}{16679706624} \frac{16679706624}{4372485013241856} \Theta^{10} \int_0^\infty dy \frac{f_0(y; \Theta)}{y^{18}} \Rightarrow \\
\frac{\chi_0^{(10,10)}(x)}{n\beta^{10}} &= -\frac{7293}{262144} \Theta^{10} \int_0^\infty dy \frac{f_0(y; \Theta)}{y^{18}}.
\end{aligned}$$



## F. Summary of ideal high-order density responses

The general form reads as

$$\frac{\chi_0^{(l,l)}(\mathbf{x}, Z)}{n\beta^l} = + \frac{1}{(l-1)!} \frac{\Theta^{l-1}}{x^{2l-2}} \left[ l \frac{\chi_0(l\mathbf{x}, lZ)}{n\beta} + \sum_{m=1}^{l-1} a_m \frac{\chi_0(m\mathbf{x}, mZ)}{n\beta} \right], \quad \sum_{m=1}^{l-1} a_m m^{2\nu} = -l^{2\nu+1}, \quad \text{for } \nu = 0, 1, \dots, l-2.$$

Applications for the first nine orders lead to

$$\begin{aligned} \frac{\chi_0^{(2,2)}(\mathbf{x}, Z)}{n\beta^2} &= \frac{1}{(2-1)!} \frac{\Theta}{2!} \frac{\chi_0(2\mathbf{x}, 2Z)}{x^2} - 2 \frac{\chi_0(\mathbf{x}, Z)}{n\beta}, \\ \frac{\chi_0^{(3,3)}(\mathbf{x}, Z)}{n\beta^3} &= \frac{1}{(3-1)!} \frac{\Theta^2}{3!} \frac{\chi_0(3\mathbf{x}, 3Z)}{x^4} - 8 \frac{\chi_0(2\mathbf{x}, 2Z)}{n\beta} + 5 \frac{\chi_0(\mathbf{x}, Z)}{n\beta}, \\ \frac{\chi_0^{(4,4)}(\mathbf{x}, Z)}{n\beta^4} &= \frac{1}{(4-1)!} \frac{\Theta^3}{4!} \frac{\chi_0(4\mathbf{x}, 4Z)}{x^6} - 18 \frac{\chi_0(3\mathbf{x}, 3Z)}{n\beta} + 28 \frac{\chi_0(2\mathbf{x}, 2Z)}{n\beta} - 14 \frac{\chi_0(\mathbf{x}, Z)}{n\beta}, \\ \frac{\chi_0^{(5,5)}(\mathbf{x}, Z)}{n\beta^5} &= \frac{1}{(5-1)!} \frac{\Theta^4}{5!} \frac{\chi_0(5\mathbf{x}, 5Z)}{x^8} - 32 \frac{\chi_0(4\mathbf{x}, 4Z)}{n\beta} + 81 \frac{\chi_0(3\mathbf{x}, 3Z)}{n\beta} - 96 \frac{\chi_0(2\mathbf{x}, 2Z)}{n\beta} + 42 \frac{\chi_0(\mathbf{x}, Z)}{n\beta}, \\ \frac{\chi_0^{(6,6)}(\mathbf{x}, Z)}{n\beta^6} &= \frac{1}{(6-1)!} \frac{\Theta^5}{6!} \frac{\chi_0(6\mathbf{x}, 6Z)}{x^{10}} - 50 \frac{\chi_0(5\mathbf{x}, 5Z)}{n\beta} + 176 \frac{\chi_0(4\mathbf{x}, 4Z)}{n\beta} - 330 \frac{\chi_0(3\mathbf{x}, 3Z)}{n\beta} + 330 \frac{\chi_0(2\mathbf{x}, 2Z)}{n\beta} - 132 \frac{\chi_0(\mathbf{x}, Z)}{n\beta}, \\ \frac{\chi_0^{(7,7)}(\mathbf{x}, Z)}{n\beta^7} &= \frac{1}{(7-1)!} \frac{\Theta^6}{7!} \frac{\chi_0(7\mathbf{x}, 7Z)}{x^{12}} - 72 \frac{\chi_0(6\mathbf{x}, 6Z)}{n\beta} + 325 \frac{\chi_0(5\mathbf{x}, 5Z)}{n\beta} - 832 \frac{\chi_0(4\mathbf{x}, 4Z)}{n\beta} + 1287 \frac{\chi_0(3\mathbf{x}, 3Z)}{n\beta} - 1144 \frac{\chi_0(2\mathbf{x}, 2Z)}{n\beta} + 429 \frac{\chi_0(\mathbf{x}, Z)}{n\beta}, \\ \frac{\chi_0^{(8,8)}(\mathbf{x}, Z)}{n\beta^8} &= \frac{1}{(8-1)!} \frac{\Theta^7}{8!} \frac{\chi_0(8\mathbf{x}, 8Z)}{x^{14}} - 98 \frac{\chi_0(7\mathbf{x}, 7Z)}{n\beta} + 540 \frac{\chi_0(6\mathbf{x}, 6Z)}{n\beta} - 1750 \frac{\chi_0(5\mathbf{x}, 5Z)}{n\beta} + 3640 \frac{\chi_0(4\mathbf{x}, 4Z)}{n\beta} - 4914 \frac{\chi_0(3\mathbf{x}, 3Z)}{n\beta} + 4004 \frac{\chi_0(2\mathbf{x}, 2Z)}{n\beta} - 1430 \frac{\chi_0(\mathbf{x}, Z)}{n\beta}, \\ \frac{\chi_0^{(9,9)}(\mathbf{x}, Z)}{n\beta^9} &= \frac{1}{(9-1)!} \frac{\Theta^8}{9!} \frac{\chi_0(9\mathbf{x}, 9Z)}{x^{16}} - 128 \frac{\chi_0(8\mathbf{x}, 8Z)}{n\beta} + 833 \frac{\chi_0(7\mathbf{x}, 7Z)}{n\beta} - 3264 \frac{\chi_0(6\mathbf{x}, 6Z)}{n\beta} + 8500 \frac{\chi_0(5\mathbf{x}, 5Z)}{n\beta} - 15232 \frac{\chi_0(4\mathbf{x}, 4Z)}{n\beta} + 18564 \frac{\chi_0(3\mathbf{x}, 3Z)}{n\beta} - 14144 \frac{\chi_0(2\mathbf{x}, 2Z)}{n\beta} + 4862 \frac{\chi_0(\mathbf{x}, Z)}{n\beta}, \\ \frac{\chi_0^{(10,10)}(\mathbf{x}, Z)}{n\beta^{10}} &= \frac{1}{(10-1)!} \frac{\Theta^9}{10!} \frac{\chi_0(10\mathbf{x}, 10Z)}{x^{18}} - 162 \frac{\chi_0(9\mathbf{x}, 9Z)}{n\beta} + 1216 \frac{\chi_0(8\mathbf{x}, 8Z)}{n\beta} - 5586 \frac{\chi_0(7\mathbf{x}, 7Z)}{n\beta} + 17442 \frac{\chi_0(6\mathbf{x}, 6Z)}{n\beta} - 38760 \frac{\chi_0(5\mathbf{x}, 5Z)}{n\beta} + 62016 \frac{\chi_0(4\mathbf{x}, 4Z)}{n\beta} - 69768 \frac{\chi_0(3\mathbf{x}, 3Z)}{n\beta} + 50388 \frac{\chi_0(2\mathbf{x}, 2Z)}{n\beta} - 16796 \frac{\chi_0(\mathbf{x}, Z)}{n\beta} \end{aligned}$$
